# Supplementary material for: Rate equations for nitrogen molecules in ultrashort and intense x-ray pulses
Source: arXiv:1508.05223 ancillary file (2017-03-16)

# Configuration chart for the rate equations of a nitrogen molecule

This configuration chart shows the photoionization, Auger decay, and fragmentation pathways included in the rate equation model for a nitrogen molecule ( $N_2$ ). The molecular rate equations can be found in the *Mathematica* package `NitrogenMoleculeRateEqs.m`. Molecular configurations that are involved in rate equations are typeset in black, e.g., C223k223. If a molecular configuration does not enter the rate equations but is only used to indicate the molecular configuration prior to breakup of the molecular ion into atomic ionic fragments, it is written in green, e.g., C203k213. The breakup products are expressed in terms of a symbolic sum of fractions of atomic probabilities, e.g.,  $\frac{1}{2}(P_{203}+P_{213})$ , denoting how the molecular probability, here C203k213, is split over atomic rate equations—here the ones governing the time evolution of  $P_{203}$  and  $P_{213}$ —upon breakup. If a molecular configuration and its subsequent evolution are used again in the chart, this is indicated by typesetting the configuration in blue, e.g., C113k213.

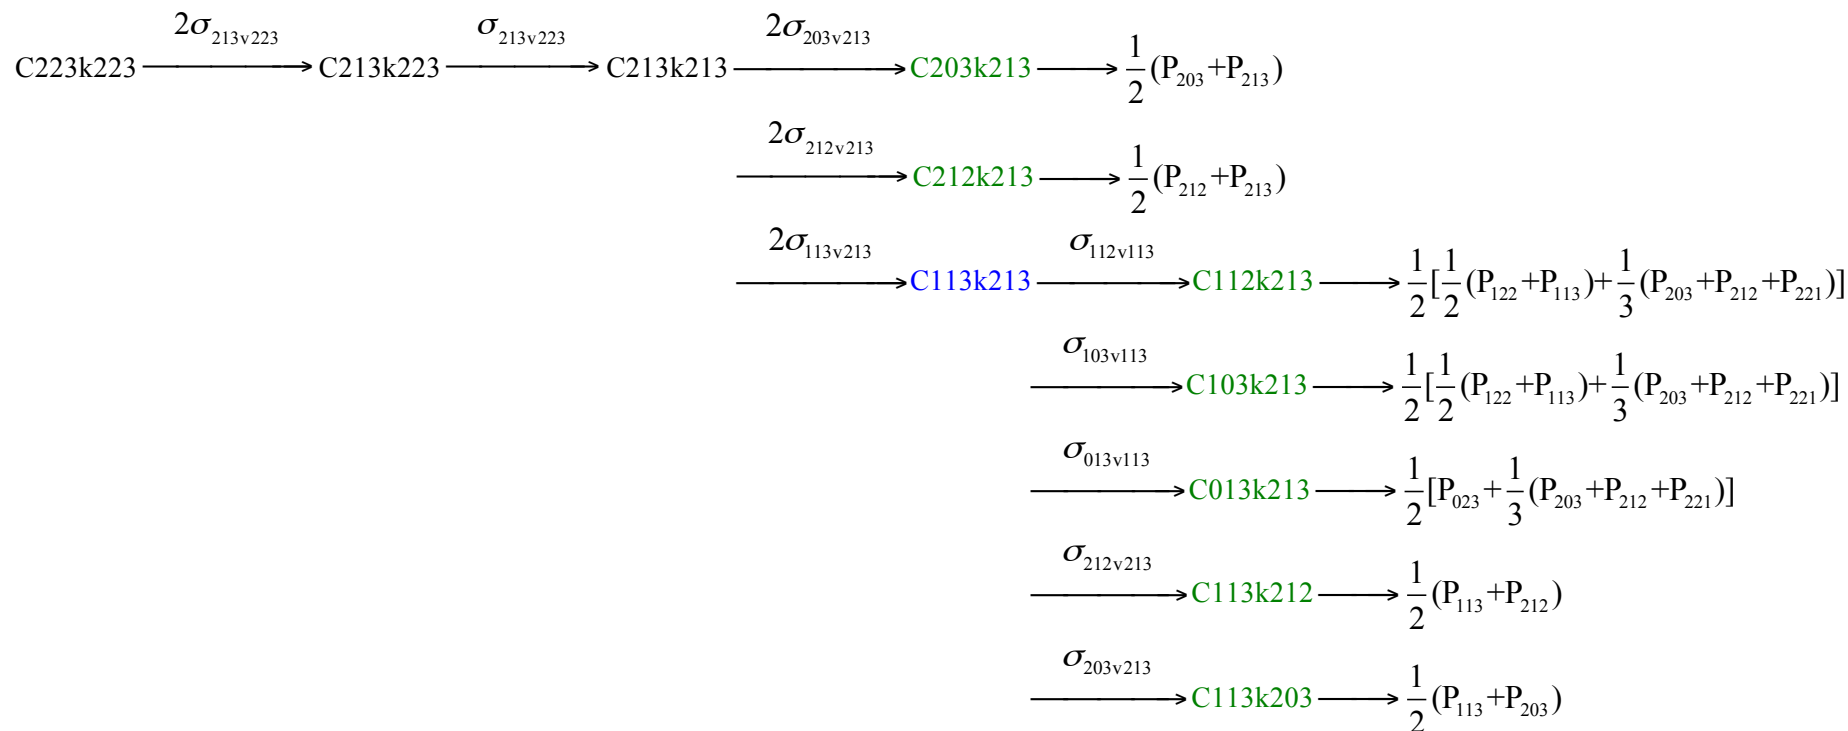

$$\begin{array}{c}
\sigma_{113\nu 213} \\
\longrightarrow \text{C113k113} \longrightarrow \text{P}_{113} \\
\Gamma_{113} \longrightarrow \frac{1}{3}(\text{P}_{203} + \text{P}_{212} + \text{P}_{221}) \\
\gamma \longrightarrow f_{\text{N+N}^{2+}} \frac{1}{2} \left[ \frac{1}{3}(\text{P}_{203} + \text{P}_{212} + \text{P}_{221}) + \text{P}_{223} \right] + f_{\text{N}^+ + \text{N}^+} \frac{1}{2}(\text{P}_{213} + \text{P}_{222})
\end{array}$$

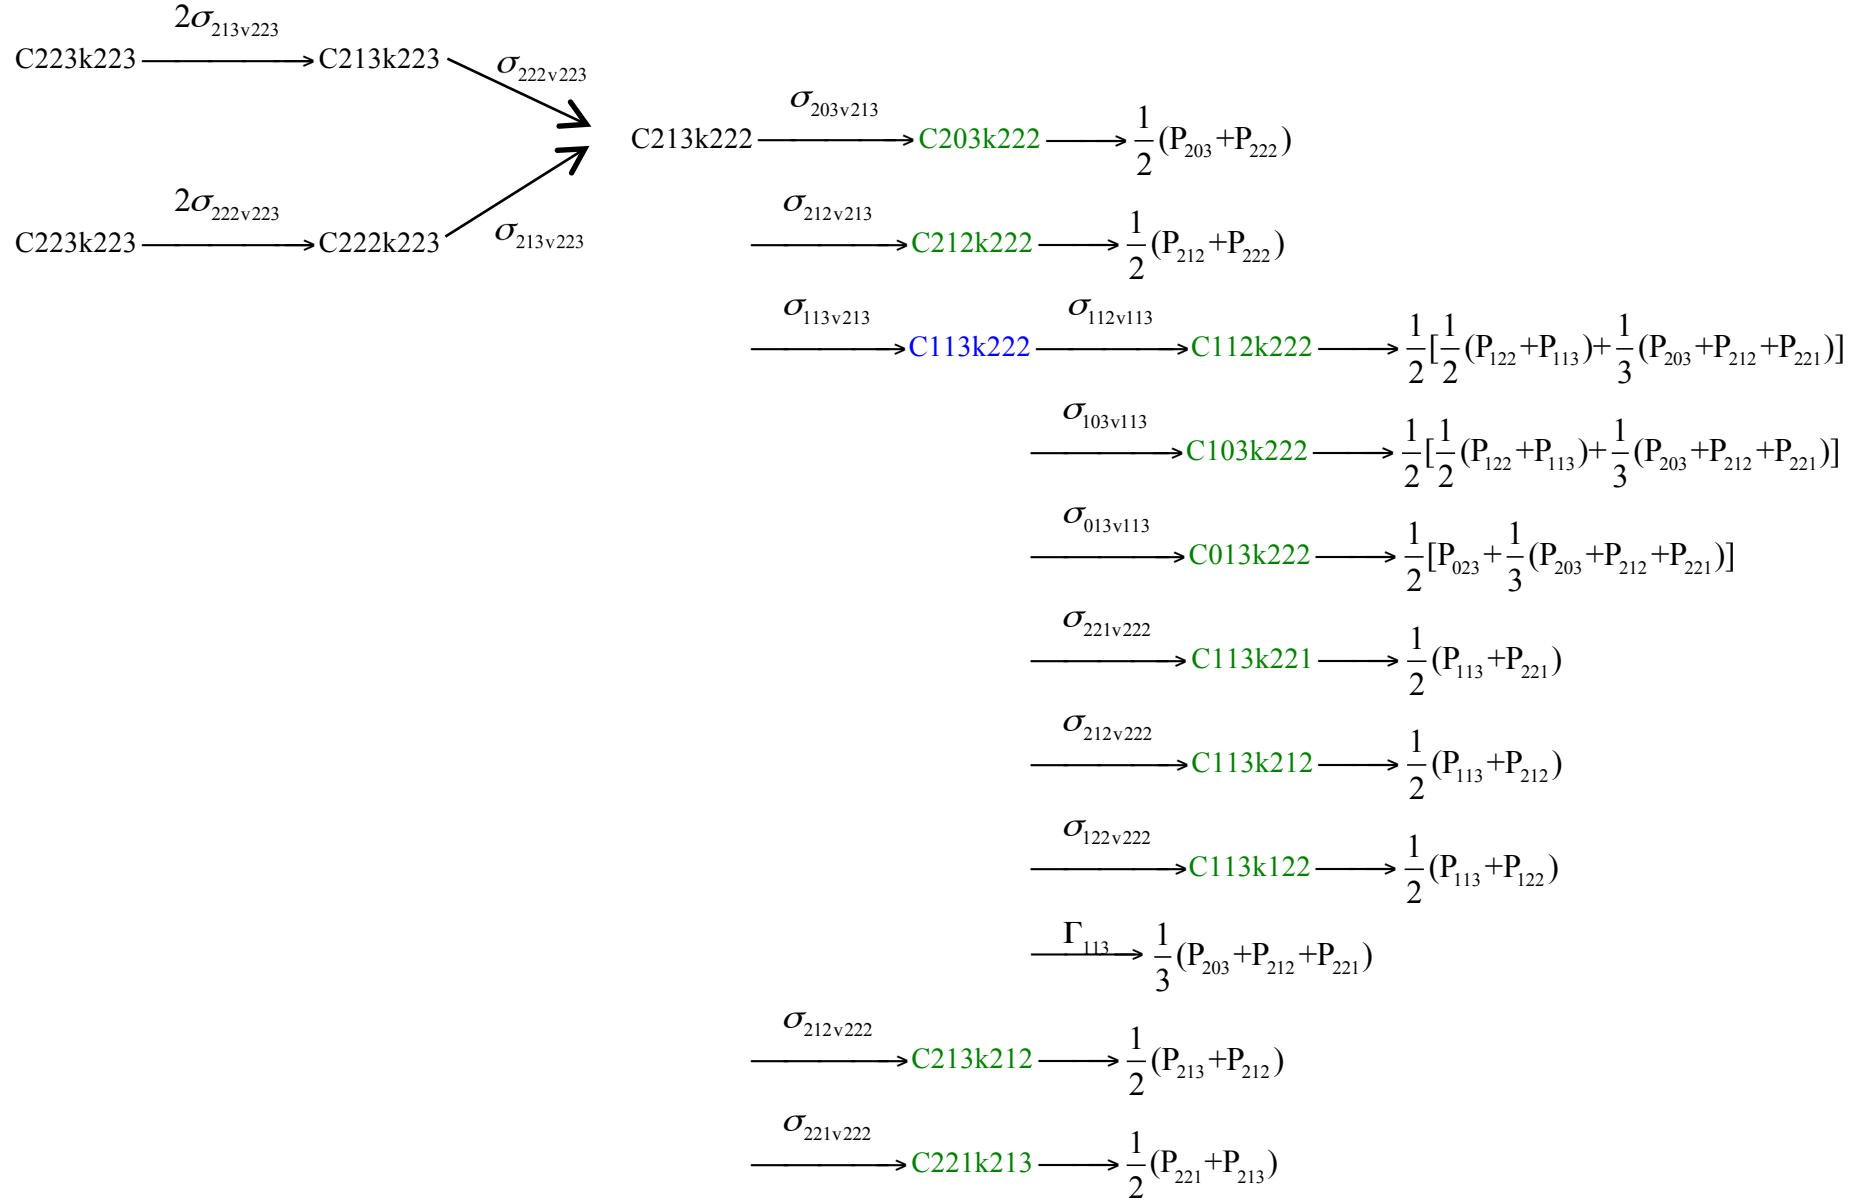

$$\begin{aligned}
& \xrightarrow{\sigma_{122v222}} \text{C122k213} \xrightarrow{\sigma_{121v122}} \text{C121k213} \longrightarrow \frac{1}{2} \left[ \frac{1}{2} (\mathbf{P}_{122} + \mathbf{P}_{113}) + \frac{1}{3} (\mathbf{P}_{203} + \mathbf{P}_{212} + \mathbf{P}_{221}) \right] \\
& \xrightarrow{\sigma_{112v122}} \text{C112k213} \longrightarrow \frac{1}{2} \left[ \frac{1}{2} (\mathbf{P}_{122} + \mathbf{P}_{113}) + \frac{1}{3} (\mathbf{P}_{203} + \mathbf{P}_{212} + \mathbf{P}_{221}) \right] \\
& \xrightarrow{\sigma_{022v122}} \text{C022k213} \longrightarrow \frac{1}{2} \left[ \mathbf{P}_{023} + \frac{1}{3} (\mathbf{P}_{203} + \mathbf{P}_{212} + \mathbf{P}_{221}) \right] \\
& \xrightarrow{\sigma_{212v213}} \text{C122k212} \longrightarrow \frac{1}{2} (\mathbf{P}_{122} + \mathbf{P}_{212}) \\
& \xrightarrow{\sigma_{203v213}} \text{C122k203} \longrightarrow \frac{1}{2} (\mathbf{P}_{122} + \mathbf{P}_{203}) \\
& \xrightarrow{\sigma_{113v213}} \text{C122k113} \longrightarrow \frac{1}{2} (\mathbf{P}_{122} + \mathbf{P}_{113}) \\
& \xrightarrow{\Gamma_{122}} \frac{1}{3} (\mathbf{P}_{203} + \mathbf{P}_{212} + \mathbf{P}_{221}) \\
& \xrightarrow{\gamma} f_{\mathbf{N}+\mathbf{N}^{2+}} \frac{1}{2} \left[ \frac{1}{3} (\mathbf{P}_{203} + \mathbf{P}_{212} + \mathbf{P}_{221}) + \mathbf{P}_{223} \right] + f_{\mathbf{N}^*+\mathbf{N}^+} \frac{1}{2} (\mathbf{P}_{213} + \mathbf{P}_{222})
\end{aligned}$$

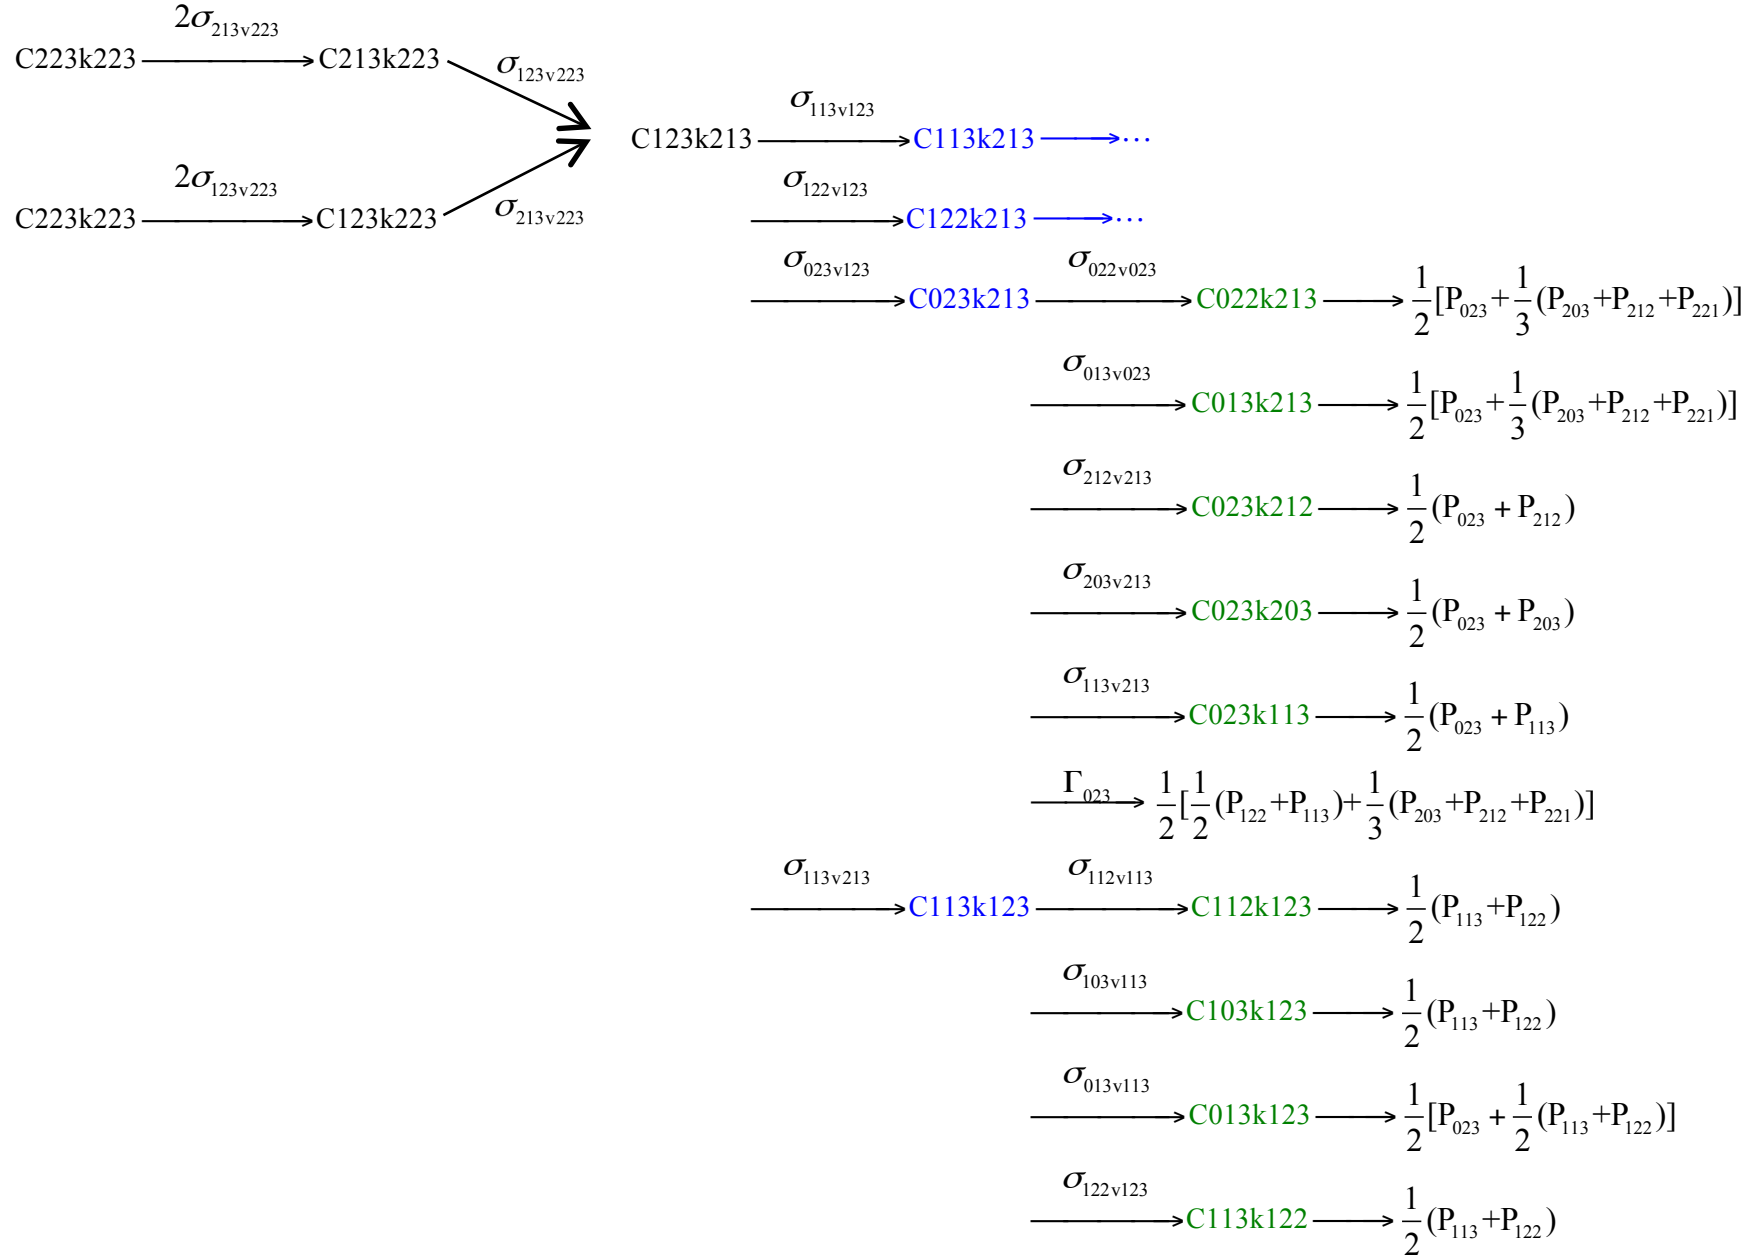

$$\begin{aligned}
& \xrightarrow{\sigma_{113v123}} \text{C113k113} \longrightarrow \text{P}_{113} \\
& \xrightarrow{\sigma_{023v123}} \text{C023k113} \longrightarrow \frac{1}{2}(\text{P}_{023} + \text{P}_{113}) \\
& \xrightarrow{\Gamma_{113}} \frac{1}{2} \left[ \frac{1}{2}(\text{P}_{122} + \text{P}_{113}) + \frac{1}{3}(\text{P}_{203} + \text{P}_{212} + \text{P}_{221}) \right] \\
& \xrightarrow{\Gamma_{203v123}} \frac{1}{2}(\text{P}_{113} + \text{P}_{203}) \\
& \xrightarrow{\Gamma_{212v123}} \frac{1}{2}(\text{P}_{113} + \text{P}_{212}) \\
& \xrightarrow{\Gamma_{221v123}} \frac{1}{2}(\text{P}_{113} + \text{P}_{221}) \\
& \xrightarrow{\sigma_{212v213}} \text{C212k123} \xrightarrow{\sigma_{211v212}} \text{C211k123} \longrightarrow \frac{1}{2} \left[ \frac{1}{2}(\text{P}_{122} + \text{P}_{113}) + \frac{1}{3}(\text{P}_{203} + \text{P}_{212} + \text{P}_{221}) \right] \\
& \xrightarrow{\sigma_{202v212}} \text{C202k123} \longrightarrow \frac{1}{2} \left[ \frac{1}{2}(\text{P}_{122} + \text{P}_{113}) + \frac{1}{3}(\text{P}_{203} + \text{P}_{212} + \text{P}_{221}) \right] \\
& \xrightarrow{\sigma_{112v212}} \text{C112k123} \longrightarrow \frac{1}{2}(\text{P}_{122} + \text{P}_{113}) \\
& \xrightarrow{\sigma_{122v123}} \text{C212k122} \longrightarrow \frac{1}{2}(\text{P}_{212} + \text{P}_{122}) \\
& \xrightarrow{\sigma_{113v123}} \text{C212k113} \longrightarrow \frac{1}{2}(\text{P}_{212} + \text{P}_{113}) \\
& \xrightarrow{\sigma_{023v123}} \text{C023k212} \longrightarrow \frac{1}{2}(\text{P}_{023} + \text{P}_{212}) \\
& \xrightarrow{\Gamma_{203v123}} \frac{1}{2}(\text{P}_{212} + \text{P}_{203})
\end{aligned}$$

$$\begin{array}{l}
\begin{array}{l}
\frac{\Gamma_{212v123}}{\longrightarrow} P_{212} \\
\frac{\Gamma_{221v123}}{\longrightarrow} \frac{1}{2}(P_{212} + P_{221})
\end{array} \\
\begin{array}{l}
\frac{\sigma_{203v213}}{\longrightarrow} \text{C203k123} \xrightarrow{\sigma_{103v203}} \text{C103k123} \longrightarrow \frac{1}{2}(P_{122} + P_{113}) \\
\frac{\sigma_{202v203}}{\longrightarrow} \text{C202k123} \longrightarrow \frac{1}{2}[\frac{1}{2}(P_{122} + P_{113}) + \frac{1}{3}(P_{203} + P_{212} + P_{221})] \\
\frac{\sigma_{122v123}}{\longrightarrow} \text{C203k122} \longrightarrow \frac{1}{2}(P_{203} + P_{122}) \\
\frac{\sigma_{113v123}}{\longrightarrow} \text{C203k113} \longrightarrow \frac{1}{2}(P_{203} + P_{113}) \\
\frac{\sigma_{023v123}}{\longrightarrow} \text{C023k203} \longrightarrow \frac{1}{2}(P_{023} + P_{203}) \\
\frac{\Gamma_{203v123}}{\longrightarrow} P_{203} \\
\frac{\Gamma_{212v123}}{\longrightarrow} \frac{1}{2}(P_{203} + P_{212}) \\
\frac{\Gamma_{221v123}}{\longrightarrow} \frac{1}{2}(P_{203} + P_{221})
\end{array} \\
\begin{array}{l}
\frac{\Gamma_{203v123}}{\longrightarrow} \frac{1}{2}(P_{213} + P_{203}) \\
\frac{\Gamma_{212v123}}{\longrightarrow} \frac{1}{2}(P_{213} + P_{212}) \\
\frac{\Gamma_{221v123}}{\longrightarrow} \frac{1}{2}(P_{213} + P_{221})
\end{array}
\end{array}$$

$$\begin{array}{lcl}
\text{C223k223} \xrightarrow{2\sigma_{213v223}} \text{C213k223} & \xrightarrow{\sigma_{212v213}} & \text{C212k223} \\
\text{C223k223} \xrightarrow{2\sigma_{222v223}} \text{C222k223} & \xrightarrow{\sigma_{212v222}} & \text{C212k223} \\
\text{C223k223} \xrightarrow{2\sigma_{123v223}} \text{C123k223} & \xrightarrow{\Gamma_{212v123}} & \text{C212k223}
\end{array}$$
  

$$\begin{array}{lcl}
\text{C212k223} \xrightarrow{\sigma_{202v212}} \text{C202k223} & \longrightarrow & \frac{1}{2} \left[ \frac{1}{2} (\text{P}_{212} + \text{P}_{203}) + \frac{1}{2} (\text{P}_{213} + \text{P}_{222}) \right] \\
\text{C212k223} \xrightarrow{\sigma_{211v212}} \text{C211k223} & \longrightarrow & \frac{1}{2} \left[ \frac{1}{2} (\text{P}_{212} + \text{P}_{221}) + \frac{1}{2} (\text{P}_{213} + \text{P}_{222}) \right] \\
\text{C212k223} \xrightarrow{\sigma_{112v212}} \text{C112k223} & \xrightarrow{\sigma_{111v112}} \text{C111k223} & \longrightarrow \frac{1}{2} \left[ \frac{1}{2} (\text{P}_{122} + \text{P}_{113}) + \frac{1}{3} (\text{P}_{203} + \text{P}_{212} + \text{P}_{221}) \right] \\
& \xrightarrow{\sigma_{102v112}} \text{C102k223} & \longrightarrow \frac{1}{2} \left[ \frac{1}{2} (\text{P}_{122} + \text{P}_{113}) + \frac{1}{3} (\text{P}_{203} + \text{P}_{212} + \text{P}_{221}) \right] \\
& \xrightarrow{\sigma_{012v112}} \text{C012k223} & \longrightarrow \frac{1}{2} \left[ \text{P}_{023} + \frac{1}{3} (\text{P}_{203} + \text{P}_{212} + \text{P}_{221}) \right] \\
& \xrightarrow{\sigma_{222v223}} \text{C112k222} & \longrightarrow \frac{1}{2} \left[ \frac{1}{2} (\text{P}_{122} + \text{P}_{113}) + \frac{1}{3} (\text{P}_{203} + \text{P}_{212} + \text{P}_{221}) \right] \\
& \xrightarrow{\sigma_{213v223}} \text{C112k213} & \longrightarrow \frac{1}{2} \left[ \frac{1}{2} (\text{P}_{122} + \text{P}_{113}) + \frac{1}{3} (\text{P}_{203} + \text{P}_{212} + \text{P}_{221}) \right] \\
& \xrightarrow{\sigma_{123v223}} \text{C112k123} & \longrightarrow \frac{1}{2} (\text{P}_{122} + \text{P}_{113}) \\
& \xrightarrow{\Gamma_{112}} & \frac{1}{3} (\text{P}_{203} + \text{P}_{212} + \text{P}_{221}) \\
& \xrightarrow{\sigma_{213v223}} \text{C212k213} & \longrightarrow \frac{1}{2} (\text{P}_{212} + \text{P}_{213}) \\
& \xrightarrow{\sigma_{222v223}} \text{C212k222} & \longrightarrow \frac{1}{2} (\text{P}_{212} + \text{P}_{222})
\end{array}$$



$$\begin{array}{l}
\sigma_{123\nu 223} \\
\longrightarrow \text{C212k123} \longrightarrow \dots \\
\gamma \longrightarrow f_{\text{N+N}^{2+}} \frac{1}{2}(\text{P}_{212}+\text{P}_{223}) + f_{\text{N}^++\text{N}^+} \frac{1}{2}(\text{P}_{213}+\text{P}_{222})
\end{array}$$

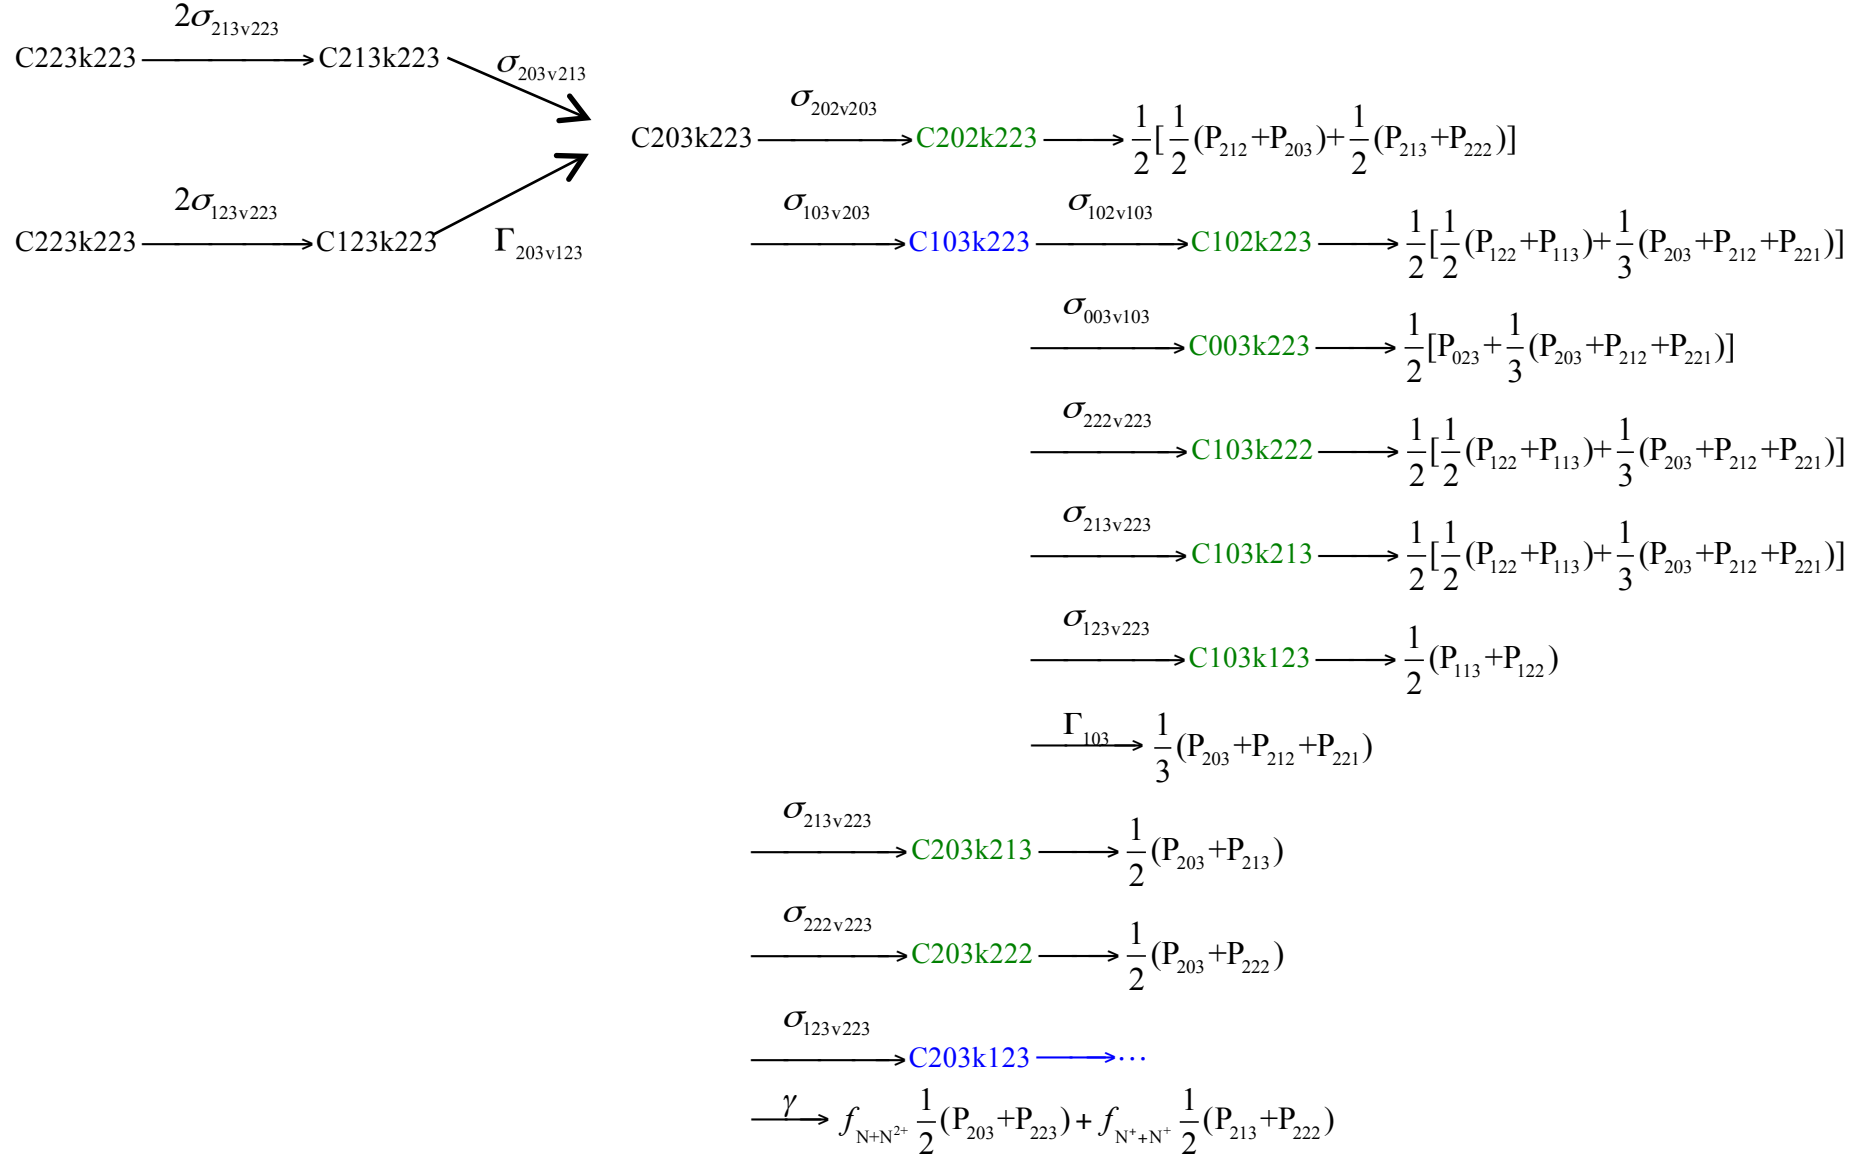

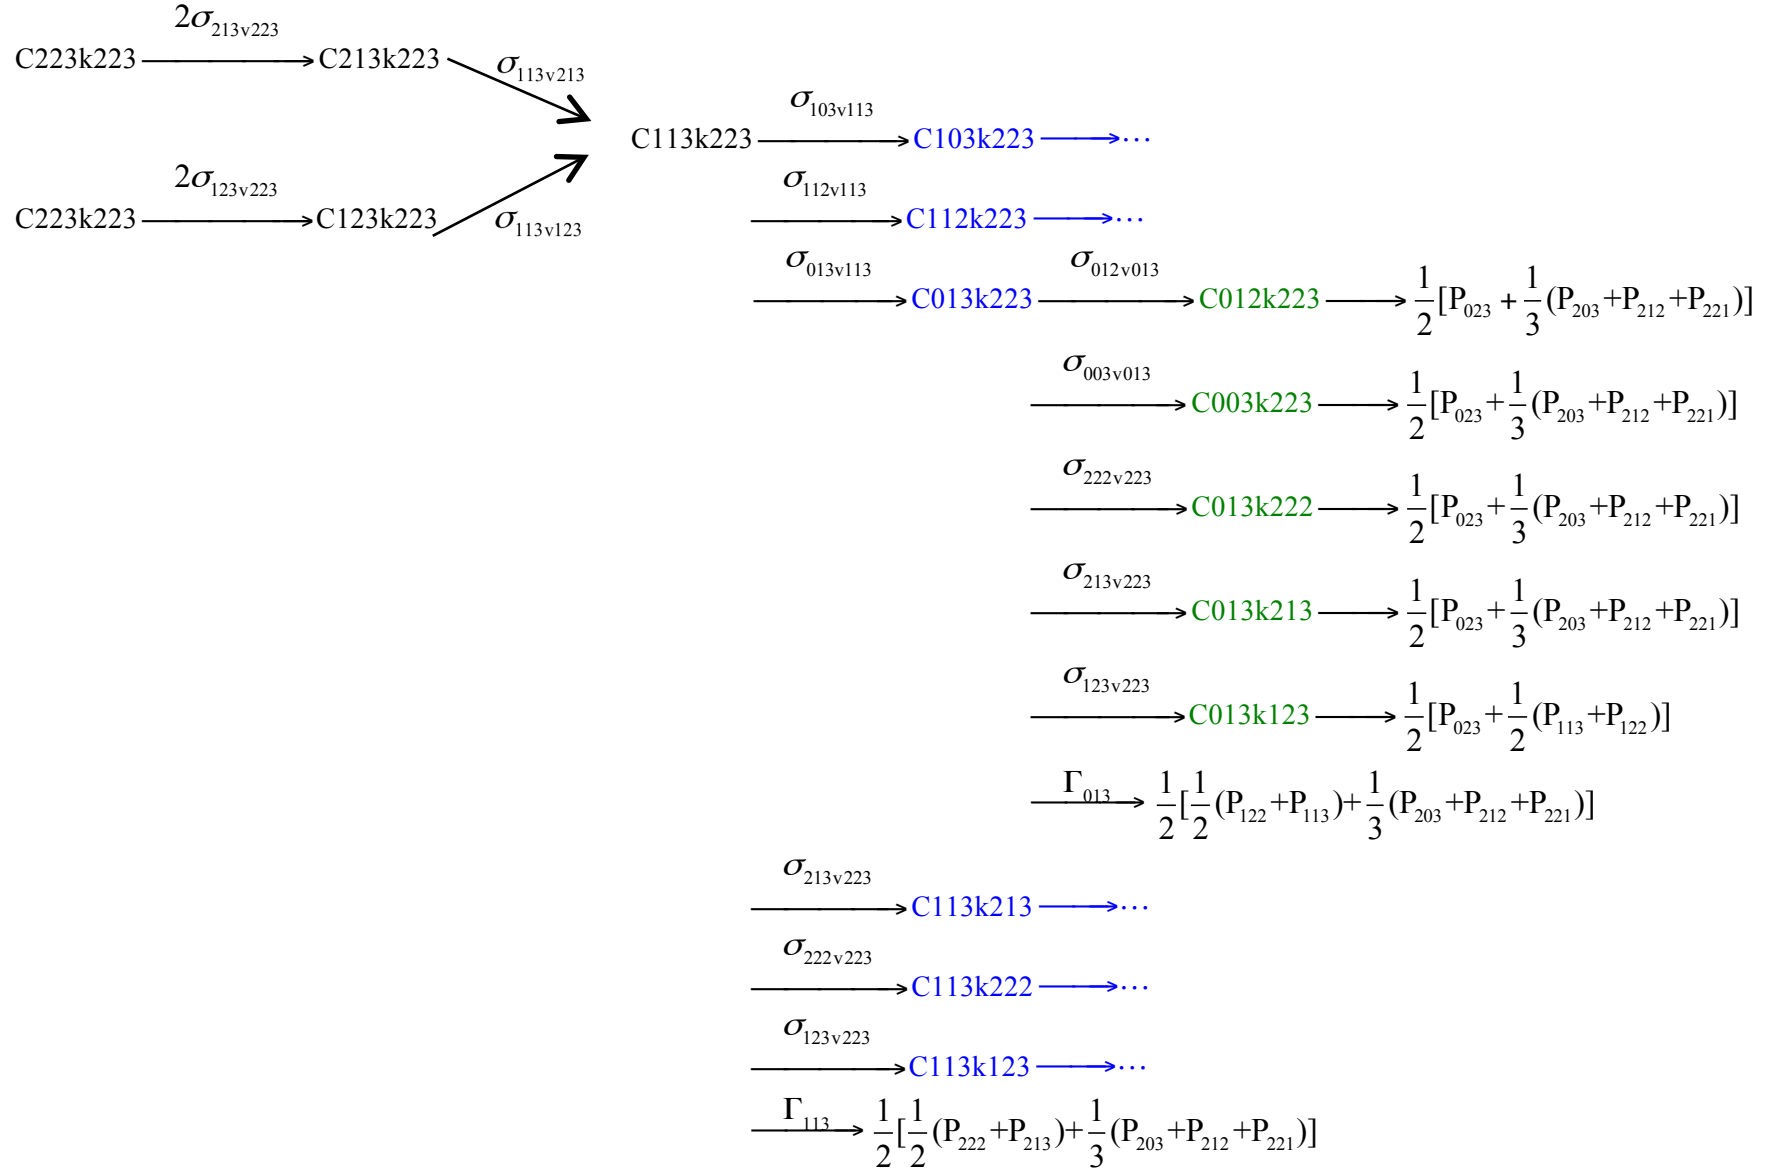

$$\begin{aligned}
\text{C223k223} &\xrightarrow{2\sigma_{222\nu223}} \text{C222k223} \xrightarrow{\sigma_{222\nu223}} \text{C222k222} \xrightarrow{2\sigma_{212\nu222}} \text{C212k222} \longrightarrow \frac{1}{2}(\text{P}_{212} + \text{P}_{222}) \\
&\xrightarrow{2\sigma_{221\nu222}} \text{C221k222} \longrightarrow \frac{1}{2}(\text{P}_{221} + \text{P}_{222}) \\
&\xrightarrow{2\sigma_{122\nu222}} \text{C122k222} \xrightarrow{\sigma_{121\nu122}} \text{C121k222} \longrightarrow \frac{1}{2}\left[\frac{1}{2}(\text{P}_{122} + \text{P}_{113}) + \frac{1}{3}(\text{P}_{203} + \text{P}_{212} + \text{P}_{221})\right] \\
&\xrightarrow{\sigma_{112\nu122}} \text{C112k222} \longrightarrow \frac{1}{2}\left[\frac{1}{2}(\text{P}_{122} + \text{P}_{113}) + \frac{1}{3}(\text{P}_{203} + \text{P}_{212} + \text{P}_{221})\right] \\
&\xrightarrow{\sigma_{022\nu122}} \text{C022k222} \longrightarrow \frac{1}{2}\left[\text{P}_{023} + \frac{1}{3}(\text{P}_{203} + \text{P}_{212} + \text{P}_{221})\right] \\
&\xrightarrow{\sigma_{221\nu222}} \text{C122k221} \longrightarrow \frac{1}{2}(\text{P}_{122} + \text{P}_{221}) \\
&\xrightarrow{\sigma_{212\nu222}} \text{C122k212} \longrightarrow \frac{1}{2}(\text{P}_{122} + \text{P}_{212}) \\
&\xrightarrow{\sigma_{122\nu222}} \text{C122k122} \longrightarrow \text{P}_{122} \\
&\xrightarrow{\Gamma_{122}} \frac{1}{3}(\text{P}_{203} + \text{P}_{212} + \text{P}_{221}) \\
&\xrightarrow{\gamma} f_{\text{N+N}^{2+}} \frac{1}{2}\left[\frac{1}{3}(\text{P}_{203} + \text{P}_{212} + \text{P}_{221}) + \text{P}_{223}\right] + f_{\text{N}^+ + \text{N}^+} \frac{1}{2}\text{P}_{222}
\end{aligned}$$

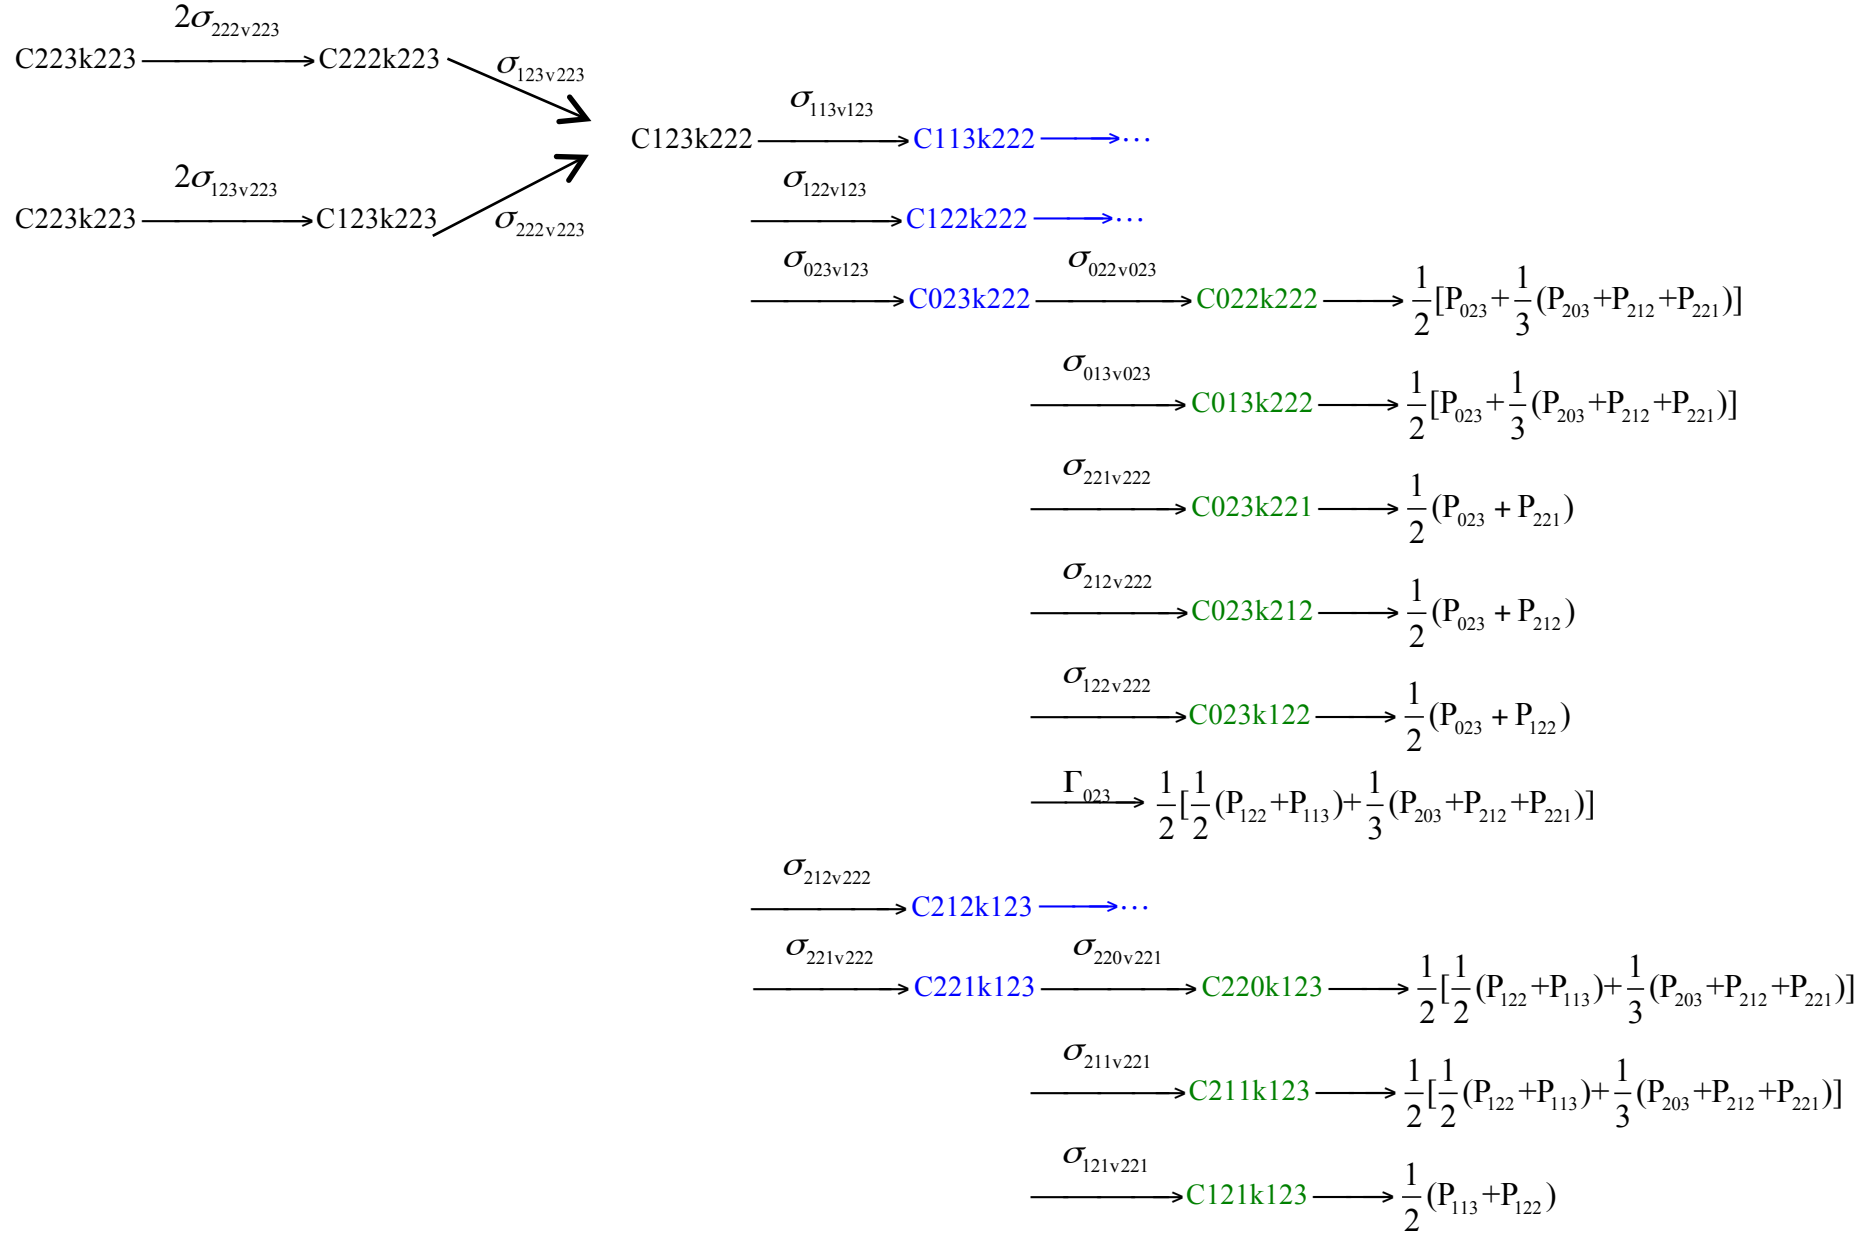

$$\begin{aligned}
& \xrightarrow{\sigma_{122v123}} \text{C221k122} \longrightarrow \frac{1}{2}(\mathbf{P}_{221} + \mathbf{P}_{122}) \\
& \xrightarrow{\sigma_{113v123}} \text{C221k113} \longrightarrow \frac{1}{2}(\mathbf{P}_{221} + \mathbf{P}_{113}) \\
& \xrightarrow{\sigma_{023v123}} \text{C023k221} \longrightarrow \frac{1}{2}(\mathbf{P}_{023} + \mathbf{P}_{221}) \\
& \xrightarrow{\Gamma_{203v123}} \frac{1}{2}(\mathbf{P}_{221} + \mathbf{P}_{203}) \\
& \xrightarrow{\Gamma_{212v123}} \frac{1}{2}(\mathbf{P}_{212} + \mathbf{P}_{221}) \\
& \xrightarrow{\Gamma_{221v123}} \mathbf{P}_{221} \\
& \xrightarrow{\sigma_{122v222}} \text{C122k123} \xrightarrow{\sigma_{121v122}} \text{C121k123} \longrightarrow \frac{1}{2}(\mathbf{P}_{122} + \mathbf{P}_{113}) \\
& \xrightarrow{\sigma_{112v122}} \text{C112k123} \longrightarrow \frac{1}{2}(\mathbf{P}_{122} + \mathbf{P}_{113}) \\
& \xrightarrow{\sigma_{022v122}} \text{C022k123} \longrightarrow \frac{1}{2}[\mathbf{P}_{023} + \frac{1}{2}(\mathbf{P}_{122} + \mathbf{P}_{113})] \\
& \xrightarrow{\sigma_{122v123}} \text{C122k122} \longrightarrow \mathbf{P}_{122} \\
& \xrightarrow{\sigma_{113v123}} \text{C122k113} \longrightarrow \frac{1}{2}(\mathbf{P}_{122} + \mathbf{P}_{113}) \\
& \xrightarrow{\sigma_{023v123}} \text{C023k122} \longrightarrow \frac{1}{2}(\mathbf{P}_{023} + \mathbf{P}_{122})
\end{aligned}$$

$$\xrightarrow{\Gamma_{122}} \quad \frac{1}{2}[\frac{1}{2}(\mathbf{P}_{122}+\mathbf{P}_{113})+\frac{1}{3}(\mathbf{P}_{203}+\mathbf{P}_{212}+\mathbf{P}_{221})]$$

$$\xrightarrow{\Gamma_{203\mathbf{v}123}} \frac{1}{2}(\mathbf{P}_{122} + \mathbf{P}_{203})$$

$$\xrightarrow{\Gamma_{212\mathbf{v}123}} \frac{1}{2}(\mathbf{P}_{122} + \mathbf{P}_{212})$$

$$\xrightarrow{\Gamma_{221\mathbf{v}123}} \frac{1}{2}(\mathbf{P}_{122} + \mathbf{P}_{221})$$

$$\xrightarrow{\Gamma_{203\mathbf{v}123}} \frac{1}{2}(\mathbf{P}_{222} + \mathbf{P}_{203})$$

$$\xrightarrow{\Gamma_{212\mathbf{v}123}} \frac{1}{2}(\mathbf{P}_{222} + \mathbf{P}_{212})$$

$$\xrightarrow{\Gamma_{221\mathbf{v}123}} \frac{1}{2}(\mathbf{P}_{222} + \mathbf{P}_{221})$$

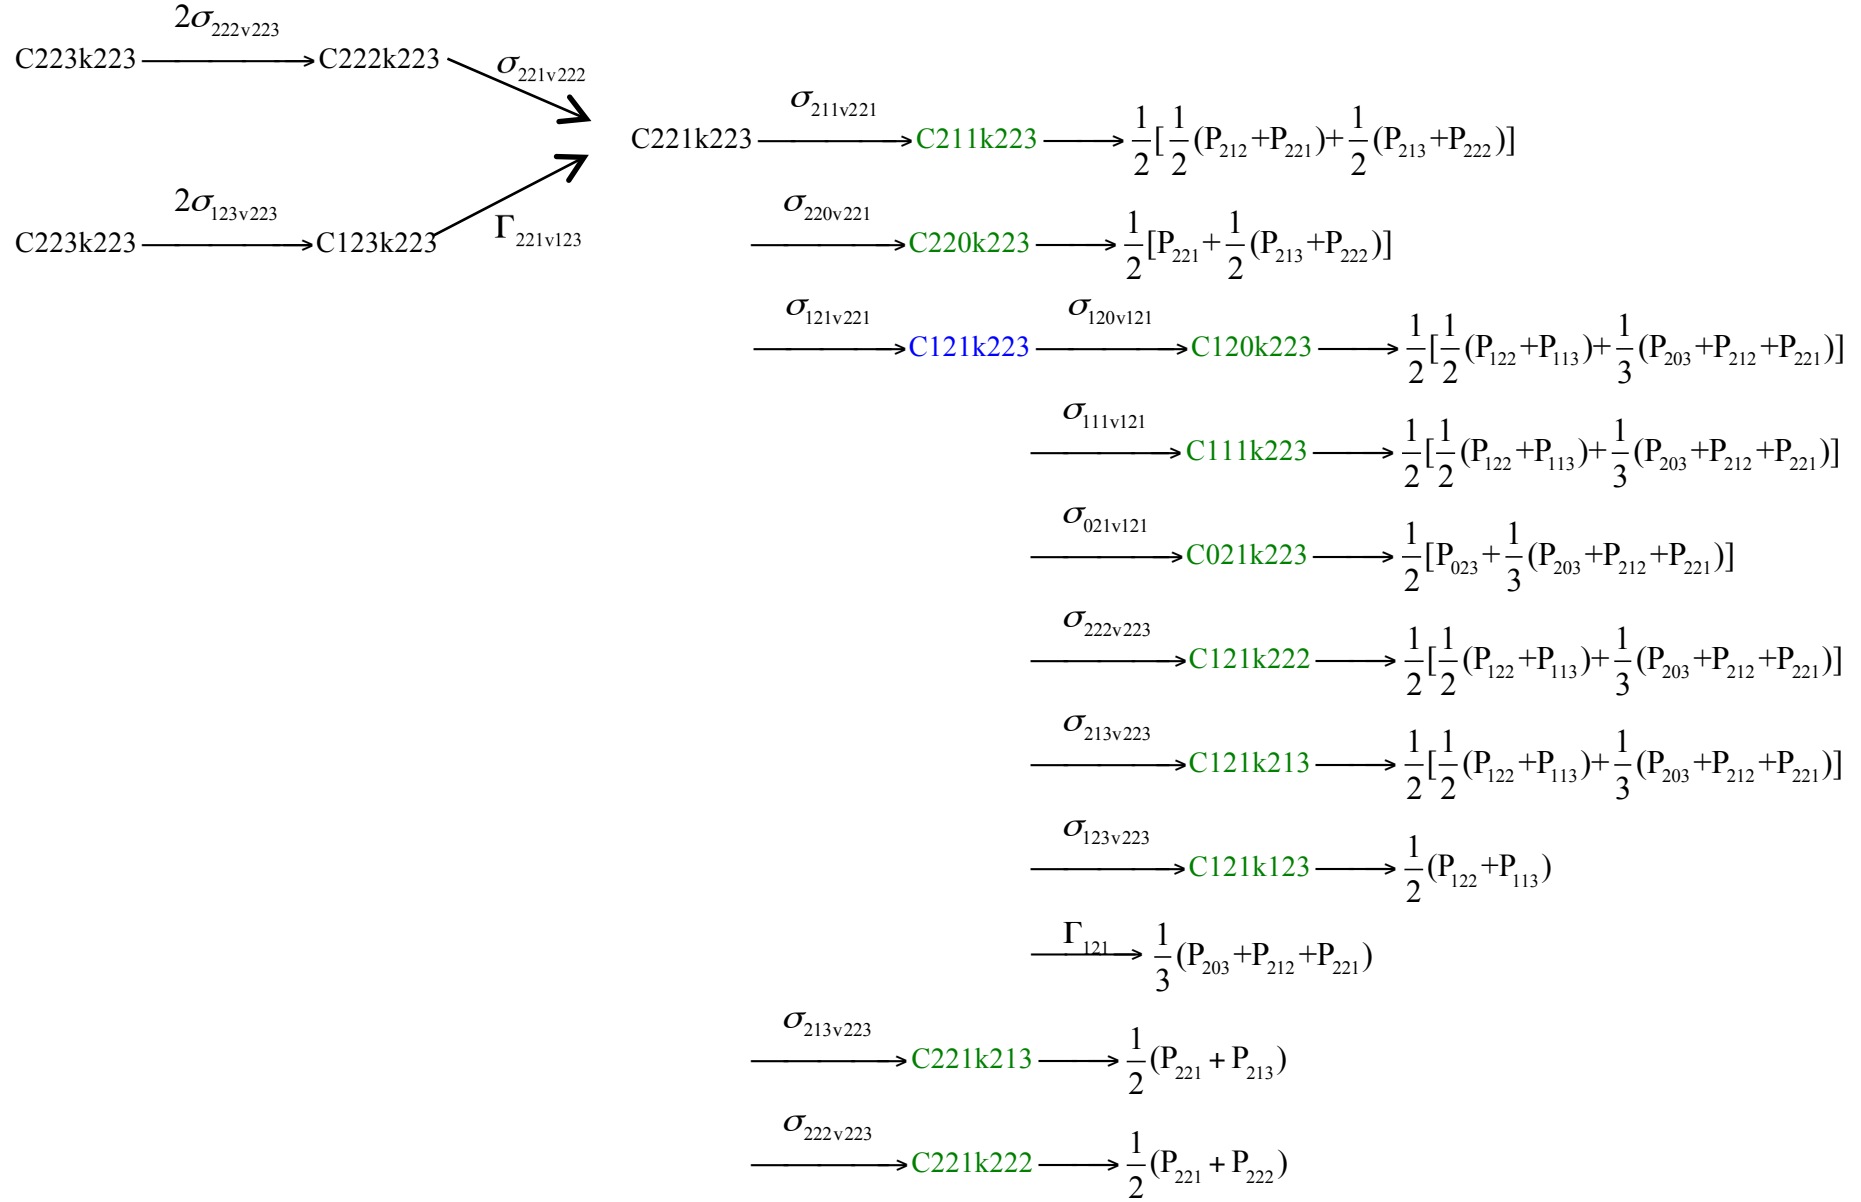



$$\begin{array}{l}
\sigma_{123\nu 223} \\
\longrightarrow \text{C221k123} \longrightarrow \dots \\
\gamma \longrightarrow f_{N+N^{2+}} \frac{1}{2} (P_{221} + P_{223}) + f_{N^++N^+} \frac{1}{2} (P_{213} + P_{222})
\end{array}$$

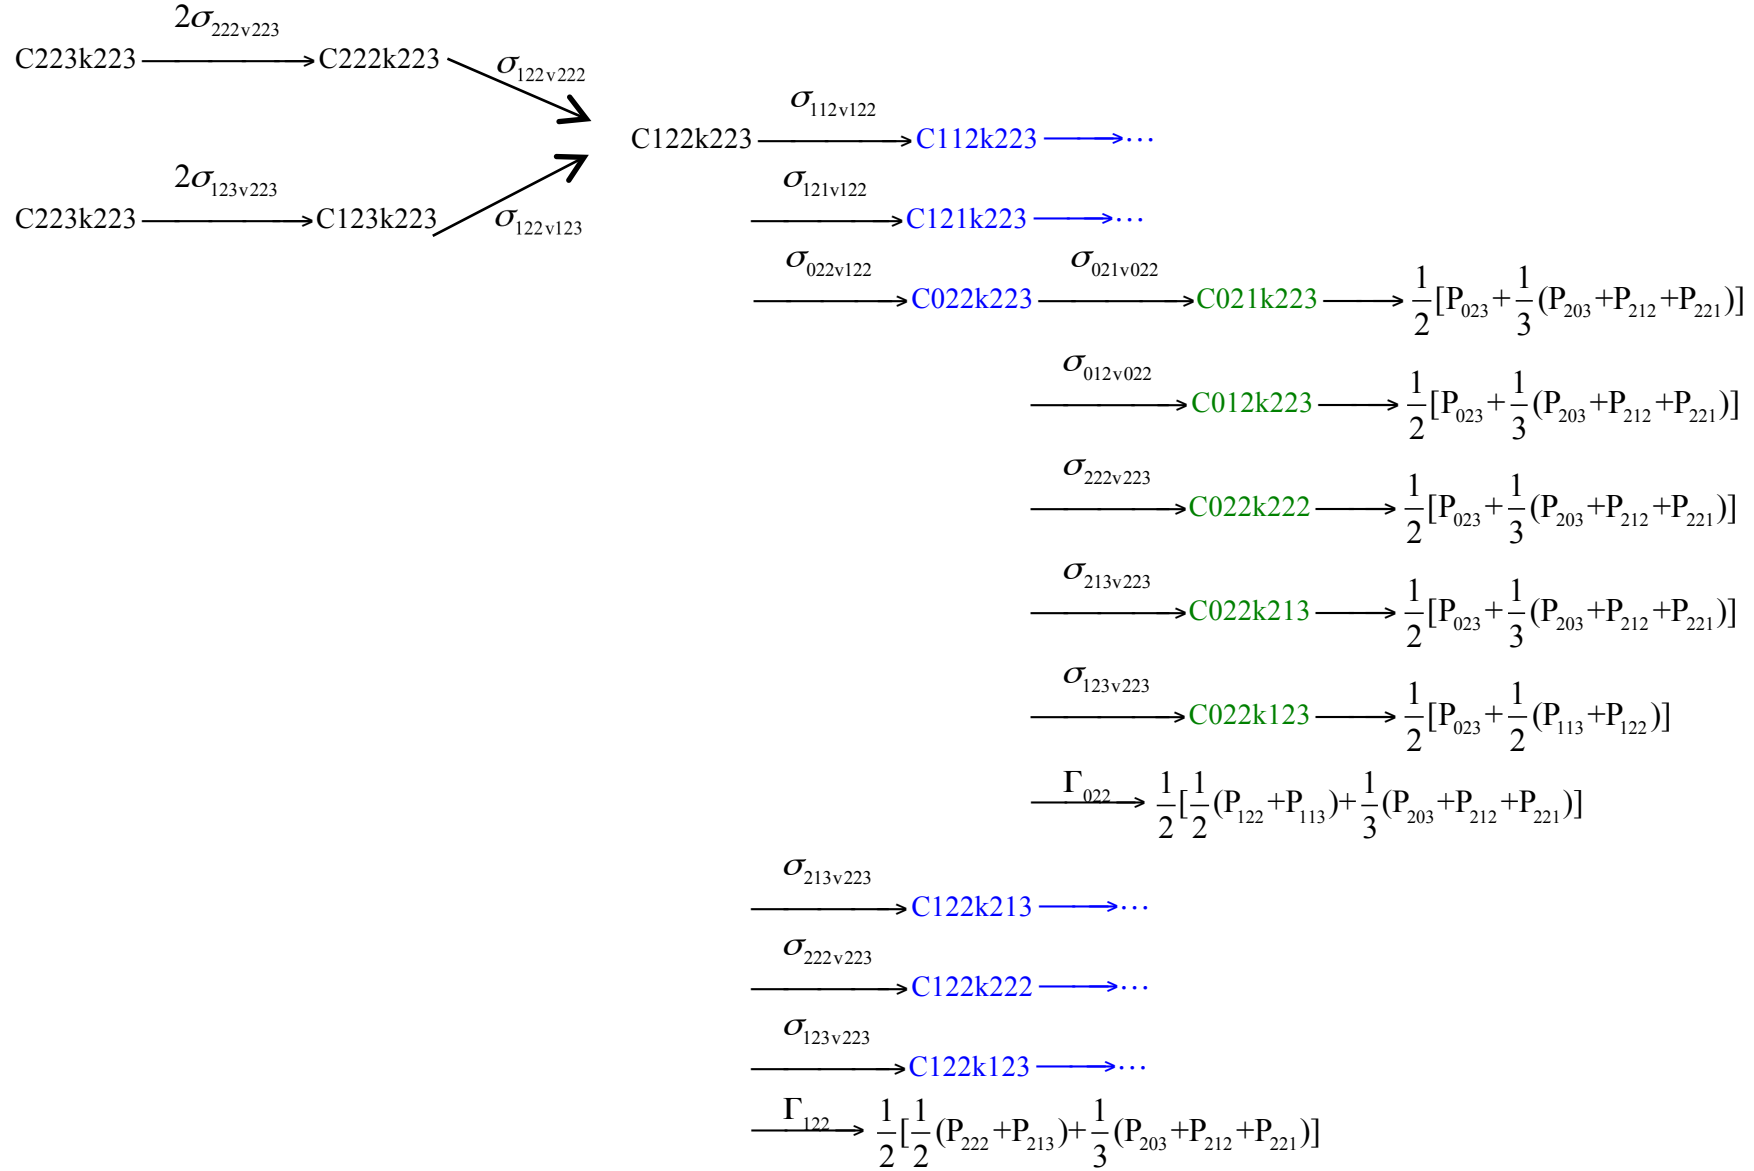

– 19 –

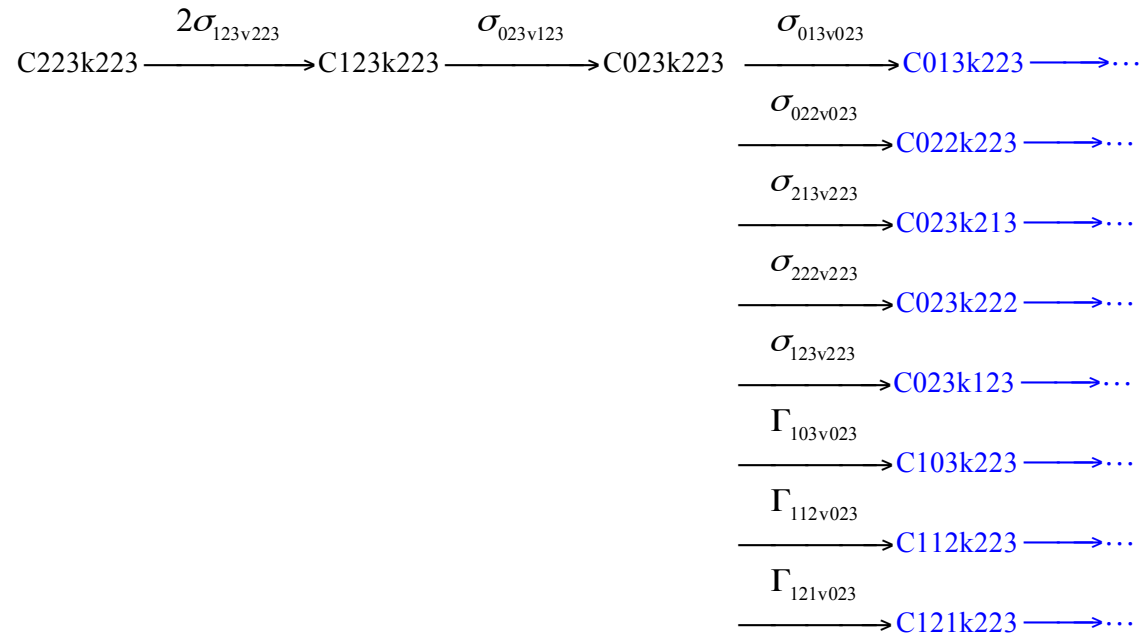

Supplement: Supplementary file 1 [file Configuration_Structure.pdf]
