# Supplementary material for: Rate equations for nitrogen molecules in ultrashort and intense x-ray pulses
Source: arXiv:1508.05223 ancillary file (2017-03-16)
Supplement: Supplementary file 2 [file MolReqEqN2_ma.pdf]

```

In[16]:= Get["NitrogenRateEquations.m", Path -> NotebookDirectory[]]
         |erhalte          |Pfad      |Notebook-Verzeichnis
         Get["NitrogenMoleculeRateEqs.m", Path -> NotebookDirectory[]]
         |erhalte          |Pfad      |Notebook-Verzeichnis

In[18]:= HartreeToeV := 27.2113845
         eVToHartree := 1 / HartreeToeV
         JouleToHartree := 2.29371269*^17
         MilliJouleToHartree := 1*^-3 * JouleToHartree
         BohrToAngstroem := 0.5291772083
         AngstroemToBohr := 1 / BohrToAngstroem
         MicrometerToBohr := 1*^4 * AngstroemToBohr
         BohrToMicrometer := 1 / MicrometerToBohr
         t0ToSecond := 24.18884326505*^-18
         t0ToFemtoSecond := 24.18884326505*^-3
         crossSectionAUtoBarn := 1*^8 * BohrToAngstroem^2
         crossSectionAUtoBarn := crossSectionAUtoBarn * 1*^-24
         crossSectioncm2toAU := 1 / crossSectionAUtoBarn

```

# Calculations for “Rate equations for nitrogen molecules in ultrashort and intense x-ray pulses”

Christian Buth, 24 September 2014

Theoretische Chemie, Physikalisch-Chemisches Institut, Ruprecht-Karls-Universität Heidelberg, Im Neuenheimer Feld 229, 69120 Heidelberg, Germany

---

## Rate of photoionization

Ratio of fragmentation time and SCH lifetime:

```

In[31]:= 200 / 6.726057633353772`
Out[31]:= 29.7351

```

Peak intensity for LCLS pulses in W/cm<sup>2</sup>:

```

In[32]:= Ip4 := 3.1*^17
         Ip280 := 9.0*^15

```

Photon energy in eV:

```

In[34]:= omegaX := 1100 * eVToHartree

```

```

In[35]:= cross := fsig123v223[omegaX] / crossSectioncm2toAU

```

Photoionization time at the peak x-ray intensity:

```
In[36]:= 1 / (cross * Ip4 / (omegaX / JouleToHartree)) * 10^15
```

```
Out[36]= 10.104
```

```
In[37]:= 1 / (cross * Ip280 / (omegaX / JouleToHartree)) * 10^15
```

```
Out[37]= 348.026
```

Lifetime of a 1s core hole in a nitrogen atom in femtoseconds:

```
In[38]:= 1 / 97.86 * 1000 * 0.658212
```

```
Out[38]= 6.72606
```

## Fragmentation times

nitrogen\_dissociation\_first.nb for 280 fs pulse duration:

```
In[39]:= 1 / (4.059357 * gammaFrag) * t0ToFemtoSecond
```

```
Out[39]= 246.344
```

nitrogen\_dissociation\_first.nb for 80 fs pulse duration:

```
In[40]:= 1 / (12.000000 * gammaFrag) * t0ToFemtoSecond
```

```
Out[40]= 83.3333
```

nitrogen\_dissociation\_short\_first.nb for 280 fs pulse duration:

```
In[41]:= 1 / (10.506791 * gammaFrag) * t0ToFemtoSecond
```

```
Out[41]= 95.1765
```

nitrogen\_dissociation\_short\_first.nb for 80 fs pulse duration:

```
In[42]:= 1 / (25.000000 * gammaFrag) * t0ToFemtoSecond
```

```
Out[42]= 40.
```

nitrogen\_dissociation\_second.nb for 280 fs pulse duration:

```
In[43]:= 1 / (4.971737 * gammaFrag) * t0ToFemtoSecond
```

```
Out[43]= 201.137
```

nitrogen\_dissociation\_second.nb for 80 fs pulse duration:

```
In[44]:= 1 / (16.800000 * gammaFrag) * t0ToFemtoSecond
```

```
Out[44]= 59.5238
```

nitrogen\_dissociation\_short\_second.nb for 280 fs pulse duration:

```
In[45]:= 1 / (13.200000 * gammaFrag) * t0ToFemtoSecond
```

```
Out[45]= 75.7576
```

nitrogen\_dissociation\_short\_second.nb for 80 fs pulse duration:

```
In[46]:= 1 / (38.864973 * gammaFrag) * t0ToFemtoSecond
```

```
Out[46]= 25.7301
```

## Ratios of pulse durations versus ratios of fragmentation times

### Concerning 280 fs pulses

In[47]:= **280 / 112.0**

Out[47]= **2.5**

In[48]:= **246 / 95.0**

Out[48]= **2.58947**

In[49]:= **201 / 76.0**

Out[49]= **2.64474**

In[50]:= **246 / 201.0**

Out[50]= **1.22388**

In[51]:= **95 / 76.0**

Out[51]= **1.25**

### Concerning 80 fs pulses

In[52]:= **80 / 40**

Out[52]= **2**

In[53]:= **83 / 40.0**

Out[53]= **2.075**

In[54]:= **60 / 26.0**

Out[54]= **2.30769**

In[55]:= **83 / 60.0**

Out[55]= **1.38333**

In[56]:= **40 / 26.0**

Out[56]= **1.53846**

### Concerning 280 fs and 80 fs pulses

In[57]:= **280 / 80.0**

Out[57]= **3.5**

In[58]:= **112 / 40.0**

Out[58]= **2.8**

In[59]:= **246 / 83.0**

Out[59]= **2.96386**

```
In[60]:= 95 / 40.0
```

```
Out[60]= 2.375
```

```
In[61]:= 201 / 60.0
```

```
Out[61]= 3.35
```

```
In[62]:= 76 / 26.0
```

```
Out[62]= 2.92308
```
