# Supplementary material for: Rate equations for nitrogen molecules in ultrashort and intense x-ray pulses
Source: arXiv:1508.05223 ancillary file (2017-03-16)
Supplement: Supplementary file 3 [file NitrogenMoleculeRateEqs.pdf]

# Rate-equation models for a nitrogen molecule (N<sub>2</sub>) in LCLS radiation

Christian Buth

Argonne National Laboratory, Argonne, Illinois 60439, USA

Max-Planck-Institut für Kernphysik, Saupfercheckweg 1, 69117 Heidelberg, Germany

The PULSE Institute for Ultrafast Energy Science, SLAC National Accelerator Laboratory, Menlo Park, California 94025, USA

Theoretische Chemie, Physikalisch-Chemisches Institut, Ruprecht-Karls-Universität Heidelberg, Im Neuenheimer Feld 229, 69120 Heidelberg, Germany

Ji-Cai Liu

Department of Mathematics and Physics, North China Electric Power University, 102206 Beijing, China

Max-Planck-Institut für Kernphysik, Saupfercheckweg 1, 69117 Heidelberg, Germany

20 August 2014

---

## Initialize package

```
BeginPackage["NitrogenMoleculeRateEqs`"]
```

```
Needs["NitrogenRateEquations`"]
```

---

## Public section

```
NitrogenMoleculeRateEqs::usage="NitrogenMoleculeRateEqs implements a rate-equation " <>
    "model for the interaction of x rays with a single nitrogen molecule (N2)."
```

---

## Crater profile

FWHM of the crater profile:

```
rhoXx:=2.2*MicrometerToBohr
rhoYy:=1.2*MicrometerToBohr
```

The crater is normalized to unity with respect to an integration over the whole xy plane:

```
craterX[rx_]:=1/rhoXx/Sqrt[Pi/Log[16]]*Exp[-4*Log[2]*(rx/rhoXx)^2]
craterY[ry_]:=1/rhoYy/Sqrt[Pi/Log[16]]*Exp[-4*Log[2]*(ry/rhoYy)^2]
crater[rx_,ry_]:=craterX[rx]*craterY[ry]
```

Number of radial integration points for the crater integration:

```
nintdata:=100
```

---

## Fluence profile

Number of x-ray photons for "monochromatic" light pulses:

```
numXRays[pulseenergy_,photonenergy_]:=pulseenergy/photonenergy
```

X-ray fluence, i.e., the number of photos per squaremeter:

```
fluence[pulseenergy_,photonenergy_,rx_,ry_]:=numXRays[pulseenergy,photonenergy]*crater[rx,ry]
```

```
peakfluence[pulseenergy_,photonenergy_]:=fluence[pulseenergy,photonenergy,0,0]
```

The peak x-ray flux at a point in the beam area:

```
J0Xfun[pulseenergy_,photonenergy_,tauX_,rx_,ry_] := 2*Sqrt[Log[2]/Pi]/tauX*fluence[pulseenergy,photonenergy,rx,ry]
```

Gaussian x-ray flux pluse shape:

```
jxgaussian[J0Xj_,tX_,t_] := J0Xj*Exp[-4*Log[2]*(t/tX)^2]*UnitStep[t+2*tX]*UnitStep[2*tX-t]
```

## Crater integration of ion yields from a single nitrogen atom

All charge states: N, N<sup>+</sup>, N<sup>(2+)</sup>, N<sup>(3+)</sup>, N<sup>(4+)</sup>, N<sup>(5+)</sup>, N<sup>(6+)</sup>, N<sup>(7+)</sup>:

```
ionyields[sol_] := {solGround[sol, posinfinity], solSingly[sol, posinfinity], solDoubly[sol, posinfinity],  
  solTriply[sol, posinfinity], solQuadruply[sol, posinfinity], solQuintuply[sol, posinfinity],  
  solSextuply[sol, posinfinity], solSeptuply[sol, posinfinity]}
```

Compute ion yields for a fraction of the peak x-ray fluences on the beam axis:

```
ionprofile[pulseenergy_,photonenergy_,tauX_,nintsteps_,nint_,truth_] := Module[{J0Xpeak,J0Xcur,sol,jxcrater},  
  J0Xpeak = 2*Sqrt[Log[2]/Pi]/tauX*peakfluence[pulseenergy,photonenergy];  
  J0Xcur = J0Xpeak/nintsteps*nint;  
  jxcrater[t_] := jxgaussian[J0Xcur,tauX,t];  
  sol = solveNitrogenRateEquations[photonenergy,jxcrater,neginfinity, posinfinity, 1/1000, truth];  
  Join[{J0Xcur}, ionyields[sol]]  
]
```

```
tabionprof[pulseenergy_,photonenergy_,tauX_,nintsteps_,truth_] := Module[{nint},  
  Table[ionprofile[pulseenergy,photonenergy,tauX,nintsteps,nint,truth],  
    {nint,nintsteps,0,-1}]  
]
```

Create interpolation functions for all charge states: N, N<sup>+</sup>, N<sup>(2+)</sup>, N<sup>(3+)</sup>, N<sup>(4+)</sup>, N<sup>(5+)</sup>, N<sup>(6+)</sup>, N<sup>(7+)</sup>:

```

interpolYields[tabdata_] := Module[{nint},
  Table[
    ListInterpolation[tabdata[[All, nint]], {tabdata[[All, 1]]}],
    {nint, 2, Length[tabdata[[1]]]}]
]

```

Evaluate all ion yields at a specific spatial point:

```

ionyieldint[funyields_, pulseenergy_, photonenergy_, tauX_, rx_, ry_] := Module[{jj0x, nint},
  jj0x = J0Xfun[pulseenergy, photonenergy, tauX, rx, ry];
  Table[funyields[[nint]][jj0x], {nint, 1, Length[funyields]}]
]

```

Integration of the ion yields of the beam area. The integral needs to be normalized to the integration area:

```

ionyieldbeam[funyields_, pulseenergy_, photonenergy_, tauX_] := Module[{iytot},
  Off[Solve::ifun];
  Off[NIntegrate::slwcon];
  iytot = 1 / ((2 * 5 * MicrometerToBohr)^2) * NIntegrate[ionyieldint[funyields,
    pulseenergy, photonenergy, tauX, rx, ry], {rx, -5 * MicrometerToBohr,
    5 * MicrometerToBohr}, {ry, -5 * MicrometerToBohr, 5 * MicrometerToBohr}, MaxRecursion -> 10000,
    Method -> "LocalAdaptive"];
  On[Solve::ifun];
  On[NIntegrate::slwcon];
  iytot
]

```

```

ionyieldcrateranalysis[pulseenergy_, photoenergy_, pulseduration_, nint_,
  inclDCH_] := Module[{tabionyi, funionyi, crationyi},
  tabionyi = tabionprof[pulseenergy, photoenergy, pulseduration, nint, inclDCH];
  funionyi = interpolYields[tabionyi];
  crationyi = ionyieldbeam[funionyi, pulseenergy, photoenergy, pulseduration]
]

```

## Independent-atom nitrogen molecule

Probabilities to find N2 in the possible molecular charge states:

```
imolGround[sol_,t1_] := solGround[sol,t1]^2
```

```
imolOne[sol_,t1_] := 2*solGround[sol,t1]*solSingly[sol,t1]
```

```
imolTwo[sol_,t1_] := 2*solGround[sol,t1]*solDoubly[sol,t1] +  
    solSingly[sol,t1]^2
```

```
imolThree[sol_,t1_] := 2*solGround[sol,t1]*solTriply[sol,t1] +  
    2*solSingly[sol,t1]*solDoubly[sol,t1]
```

```
imolFour[sol_,t1_] := 2*solGround[sol,t1]*solQuadruply[sol,t1] +  
    2*solSingly[sol,t1]*solTriply[sol,t1] +  
    solDoubly[sol,t1]^2
```

```
imolFive[sol_,t1_] := 2*solGround[sol,t1]*solQuintuply[sol,t1] +  
    2*solSingly[sol,t1]*solQuadruply[sol,t1] +  
    2*solDoubly[sol,t1]*solTriply[sol,t1]
```

```
imolSix[sol_,t1_] := 2*solGround[sol,t1]*solSextuply[sol,t1] +  
    2*solSingly[sol,t1]*solQuintuply[sol,t1] +  
    2*solDoubly[sol,t1]*solQuadruply[sol,t1] +  
    solTriply[sol,t1]^2
```

```
imolSeven[sol_,t1_] := 2*solGround[sol,t1]*solSeptuply[sol,t1] +  
    2*solSingly[sol,t1]*solSextuply[sol,t1] +  
    2*solDoubly[sol,t1]*solQuintuply[sol,t1] +  
    2*solTriply[sol,t1]*solQuadruply[sol,t1]
```

```
imolEight[sol_,t1_] := 2*solSingly[sol,t1]*solSeptuply[sol,t1] +  
    2*solDoubly[sol,t1]*solSextuply[sol,t1] +  
    2*solTriply[sol,t1]*solQuintuply[sol,t1] +  
    solQuadruply[sol,t1]^2
```

```

imolNine[sol_,t1_] := 2*solDoubly[sol,t1]*solSeptuply[sol,t1] +
  2*solTriply[sol,t1]*solSextuply[sol,t1] +
  2*solQuadruply[sol,t1]*solQuintuply[sol,t1]

```

```

imolTen[sol_,t1_] := 2*solTriply[sol,t1]*solSeptuply[sol,t1] +
  2*solQuadruply[sol,t1]*solSextuply[sol,t1] +
  solQuintuply[sol,t1]^2

```

```

imolEleven[sol_,t1_] := 2*solQuadruply[sol,t1]*solSeptuply[sol,t1] +
  2*solQuintuply[sol,t1]*solSextuply[sol,t1]

```

```

imolTwelve[sol_,t1_] := 2*solQuintuply[sol,t1]*solSeptuply[sol,t1] +
  solSextuply[sol,t1]^2

```

```

imolThirteen[sol_,t1_] := 2*solSextuply[sol,t1]*solSeptuply[sol,t1]

```

```

imolFourteen[sol_,t1_] := solSeptuply[sol,t1]^2

```

All charge states for each atom N, N<sup>+</sup>, N<sup>(2+)</sup>, N<sup>(3+)</sup>, N<sup>(4+)</sup>, N<sup>(5+)</sup>, N<sup>(6+)</sup>, N<sup>(7+)</sup>:

```

imolionyields[sol_] := {imolGround[sol,posinfinity],imolOne[sol,posinfinity],imolTwo[sol,posinfinity],
  imolThree[sol,posinfinity],imolFour[sol,posinfinity],imolFive[sol,posinfinity],
  imolSix[sol,posinfinity],imolSeven[sol,posinfinity],imolEight[sol,posinfinity],
  imolNine[sol,posinfinity],imolTen[sol,posinfinity],imolEleven[sol,posinfinity],
  imolTwelve[sol,posinfinity],imolThirteen[sol,posinfinity],imolFourteen[sol,posinfinity]}

```

Convert molecular ion yields to atomic ion yields:

```

imolatomicprob[imolprob_]:= {
    imolprob[[1]]+1/2*imolprob[[2]],
    1/2*imolprob[[2]]+imolprob[[3]]+1/2*imolprob[[4]],
    1/2*imolprob[[4]]+imolprob[[5]]+1/2*imolprob[[6]],
    1/2*imolprob[[6]]+imolprob[[7]]+1/2*imolprob[[8]],
    1/2*imolprob[[8]]+imolprob[[9]]+1/2*imolprob[[10]],
    1/2*imolprob[[10]]+imolprob[[11]]+1/2*imolprob[[12]],
    1/2*imolprob[[12]]+imolprob[[13]]+1/2*imolprob[[14]],
    1/2*imolprob[[14]]+imolprob[[15]]
}

```

Compute ion yields for a fraction of the peak x-ray fluences on the beam axis:

```

imolionprofile[pulseenergy_,photonenergy_,tauX_,nintsteps_,nint_,truth_] := Module[
{J0Xpeak,J0Xcur,sol,jxcrater},
J0Xpeak=2*Sqrt[Log[2]/Pi]/tauX*peakfluence[pulseenergy,photonenergy];
J0Xcur=J0Xpeak/nintsteps*nint;
jxcrater[t_]:=jxgaussian[J0Xcur,tauX,t];
sol=solveNitrogenRateEquations[photonenergy,jxcrater,neginfinity,posinfinity,1/1000,truth];
Join[{J0Xcur},imolionyields[sol]]
]

```

```

imoltabionprof[pulseenergy_,photonenergy_,tauX_,nintsteps_,truth_] := Table[
    imolionprofile[pulseenergy,photonenergy,tauX,nintsteps,nint,truth],{nint,nintsteps,0,-1}
]

```

Create interpolation functions for all charge states: N, N<sup>+</sup>, N<sup>(2+)</sup>, ..., N<sup>(14+)</sup>:

```

imolinterpolYields[tabdata_] := Module[{nint},
Table[
ListInterpolation[tabdata[[All,nint]],{tabdata[[All,1]]},Method->"Spline"],
{nint,2,16}]
]

```

Evaluate all ion yields at a specific spatial point:

```

imolionyieldint[funyields_,pulseenergy_,photonenergy_,tauX_,rx_,ry_] := Module[{jj0x,nint},
jj0x=J0Xfun[pulseenergy,photonenergy,tauX,rx,ry];
Table[funyields[[nint]][jj0x],{nint,1,15}]
]

```

Integration of the ion yields of the beam area. The integral needs to be normalized to the integration area:

```

imolionyieldbeam[funyields_,pulseenergy_,photonenergy_,tauX_] := Module[{iytot},
Off[Solve::ifun];
Off[NIntegrate::slwcon];
iytot=1/((2*5*MicrometerToBohr)^2)*NIntegrate[imolionyieldint[funyields,
pulseenergy,photonenergy,tauX,rx,ry],{rx,-5*MicrometerToBohr,
5*MicrometerToBohr},{ry,-5*MicrometerToBohr,5*MicrometerToBohr}];
On[Solve::ifun];
On[NIntegrate::slwcon];
iytot
]

```

```

imolionyieldcrateranalysis[pulseenergy_,photoenergy_,pulseduration_,nint_,inclDCH_] := Module[
{tabionyi,funionyi,crationyi},
tabionyi=imoltabionprof[pulseenergy,photoenergy,pulseduration,nint,inclDCH];
funionyi=imolinterpYields[tabionyi];
crationyi=imolionyieldbeam[funionyi,pulseenergy,photoenergy,pulseduration]
]

```

## Fragmentation matrix model

### Volume integration with a fragmentation matrix

All charge states: N, N<sup>+</sup>, N<sup>(2+)</sup>, N<sup>(3+)</sup>, N<sup>(4+)</sup>, N<sup>(5+)</sup>, N<sup>(6+)</sup>, N<sup>(7+)</sup>:

```
atomicprobs[sol_] := {solGround[sol, posinfinity], solSingly[sol, posinfinity], solDoubly[sol, posinfinity],
  solTriply[sol, posinfinity], solQuadruply[sol, posinfinity], solQuintuply[sol, posinfinity],
  solSextuply[sol, posinfinity], solSeptuply[sol, posinfinity]}
```

```
ics[i_, j_] := i + 1 + 8*j
```

```
molprobs[fmat_, sol_] := Module[{i, j, atmps, dirps, molps},
  atmps = atomicprobs[sol];
  dirps = Flatten[Table[atmps[[i + 1]] * atmps[[j + 1]], {j, 0, 7}, {i, 0, 7}]];
  molps = fmat.dirps;
  (* Second Table is a sanity check; both must yield the same result *)
  {Table[Sum[molps[[ics[i, j]]], {i, 0, 7}], {j, 0, 7}], Table[Sum[molps[[ics[j, i]]], {i, 0, 7}], {j, 0, 7}]}
]
```

Compute ion yields for a fraction of the peak x-ray fluences on the beam axis:

```
stationprofile[fmat_, pulseenergy_, photonenergy_, tauX_, nintsteps_, nint_, truth_] := Module[{J0Xpeak, J0Xcur, sol, jxcrater},
  J0Xpeak = 2*Sqrt[Log[2]/Pi]/tauX*peakfluence[pulseenergy, photonenergy];
  J0Xcur = J0Xpeak/nintsteps*nint;
  jxcrater[t_] := jxgaussian[J0Xcur, tauX, t];
  sol = solveNitrogenRateEquations[photonenergy, jxcrater, neginfinity, posinfinity, 1/1000, truth];
  Join[{J0Xcur}, molprobs[fmat, sol][[1]]]
]
```

```
stattabionprof[fmat_, pulseenergy_, photonenergy_, tauX_, nintsteps_, truth_] := Module[{nint},
  Table[stationprofile[fmat, pulseenergy, photonenergy, tauX, nintsteps, nint, truth],
    {nint, nintsteps, 0, -1}]
]
```

Create interpolation functions for all charge states: N, N<sup>+</sup>, N<sup>(2+)</sup>, N<sup>(3+)</sup>, N<sup>(4+)</sup>, N<sup>(5+)</sup>, N<sup>(6+)</sup>, N<sup>(7+)</sup>:

```
statinterpolYields[tabdata_] := Module[{nint},
  Table[
    ListInterpolation[tabdata[[All, nint]], {tabdata[[All, 1]]} (*, Method->"Spline"*)],
    {nint, 2, Length[tabdata[[1]]]}]
]
```

Evaluate all ion yields at a specific spatial point:

```
stationyieldint[funyields_,pulseenergy_,photonenergy_,tauX_,rx_,ry_] := Module[{jj0x,nint},
  jj0x=J0Xfun[pulseenergy,photonenergy,tauX,rx,ry];
  Table[funyields[[nint]][jj0x],{nint,1,Length[funyields]}]
]
```

Integration of the ion yields of the beam area. The integral needs to be normalized to the integration area:

```
stationyieldbeam[funyields_,pulseenergy_,photonenergy_,tauX_] := Module[{iytot},
  Off[Solve::ifun];
  Off[NIntegrate::slwcon];
  iytot=1/((2*5*MicrometerToBohr)^2)*NIntegrate[stationyieldint[funyields,
  pulseenergy,photonenergy,tauX,rx,ry],{rx,-5*MicrometerToBohr,
  5*MicrometerToBohr},{ry,-5*MicrometerToBohr,5*MicrometerToBohr},MaxRecursion->10000,
  Method->"LocalAdaptive"];
  On[Solve::ifun];
  On[NIntegrate::slwcon];
  iytot
]
```

```
stationyieldcrateranalysis[fmat_,pulseenergy_,photoenergy_,pulseduration_,nint_,
inclDCH_] := Module[{tabionyi,funionyi,crationyi},
  tabionyi=stattabionprof[fmat,pulseenergy,photoenergy,pulseduration,nint,inclDCH];
  funionyi=statinterpolYields[tabionyi];
  crationyi=stationyieldbeam[funionyi,pulseenergy,photoenergy,pulseduration]
]
```

## Transformation matrix

```

mixingmat[id1_,id2_,re1_,re2_,fac_]:=Module[{mima},
mima=IdentityMatrix[64];
mima[[id1,id1]]=1-fac;
mima[[id2,id2]]=1-fac;
mima[[re1,id1]]=fac;
mima[[re2,id2]]=fac;
mima
]

```

```

icsp[p_]:=ics[p[[1]],p[[2]]]
revp[p_]:={p[[2]],p[[1]]}

```

```

icsfl[p_]:=If[EvenQ[p[[1]]+p[[2]]],
icsp[{(p[[1]]+p[[2]])/2,(p[[1]]+p[[2]])/2}],
icsp[{(p[[1]]+p[[2]]-1)/2,(p[[1]]+p[[2]]+1)/2}]
]

```

```

icsfr[p_]:=If[EvenQ[p[[1]]+p[[2]]],
icsp[{(p[[1]]+p[[2]])/2,(p[[1]]+p[[2]])/2}],
icsp[{(p[[1]]+p[[2]]+1)/2,(p[[1]]+p[[2]]-1)/2}]
]

```

```

genTrafMatrices[]:=Module[{redpairs,compairs,i},
redpairs=Subsets[Table[i,{i,0,7}],{2}];
compairs=Select[redpairs,Abs[#[[1]]-#[[2]]]>=2&];
Table[mixingmat[icsp[compairs[[i]]],icsp[revp[compairs[[i]]]],
icsfl[compairs[[i]]],icsfr[compairs[[i]]],ToExpression["f"<>ToString[i]]],
{i,1,Length[compairs]}]
]

```

Compound final fragmentation matrix via

```

trafmats=genTrafMatrices[];
fmat=IdentityMatrix[64];

```

```

For[i=1,i<=Length[trafmats],i++,
  fmat=fmat.trafmats[[i]];
]
fmatnom4fs=fmat/.Last[fit4fs];

```

## SCHs, DCHs, and PAPAs

### Probabilities to find N2 in SCH-, DCH-, and PAPA-channels

```

solPAP[sol_,t1_]:= (Replace[Ppap121v223[t],sol[[1]]]+Replace[Ppap103v223[t],sol[[1]]] +
  Replace[Ppap112v223[t],sol[[1]]]+Replace[Ppap221v123[t],sol[[1]]] +
  Replace[Ppap203v123[t],sol[[1]]]+Replace[Ppap212v123[t],sol[[1]]])/.{t->t1}

```

```

solPAPprob[sol_,t1_]:=Replace[Ppap[t],sol[[1]]]/.{t->t1}

```

```

solPAPA[sol_,t1_]:=Replace[Ppapa[t],sol[[1]]]/.{t->t1}

```

```

solNeutral[sol_,t1_]:= (Replace[P223[t],sol[[1]]]/.{t->t1})^2

```

```

solSCH[sol_,t1_]:= (2*Replace[P223[t],sol[[1]]]*Replace[P123[t],sol[[1]]])/.{t->t1}

```

```

solSCHdecay[sol_,t1_]:=Replace[Pschd[t],sol[[1]]]/.{t->t1}

```

```

solDCHsinglesite[sol_,t1_]:= (2*Replace[P223[t],sol[[1]]] *
  Replace[P023[t],sol[[1]]])/.{t->t1}

```

```

solDCHsinglesiteDecay[sol_,t1_]:=Replace[Pssdchd[t],sol[[1]]]/.{t->t1}

```

```

solDCHtwosites[sol_,t1_]:= (Replace[P123[t],sol[[1]]]/.{t->t1})^2

```

```

solDCHtwositesDecay[sol_,t1_]:=Replace[Ptsdchd[t],sol[[1]]]/.{t->t1}

```

## Molecular rate equations

A PA cycle:

```
reqPA221v223[en_,jxpulse_] := Ppa221v223'[t] == (-fsigTot221[en] - fsigTot223[en]) *
    Ppa221v223[t] * jxpulse[t] + GamA221v123*2*P123[t]*P223[t]
ieqPA221v223[neginf_,inival_] := Ppa221v223[neginf] == inival

reqPA203v223[en_,jxpulse_] := Ppa203v223'[t] == (-fsigTot203[en] - fsigTot223[en]) *
    Ppa203v223[t] * jxpulse[t] + GamA203v123*2*P123[t]*P223[t]
ieqPA203v223[neginf_,inival_] := Ppa203v223[neginf] == inival

reqPA212v223[en_,jxpulse_] := Ppa212v223'[t] == (-fsigTot212[en] - fsigTot223[en]) *
    Ppa212v223[t] * jxpulse[t] + GamA221v123*2*P123[t]*P223[t]
ieqPA212v223[neginf_,inival_] := Ppa212v223[neginf] == inival
```

One-site PAPs:

```
reqPAP121v223[en_,jxpulse_,truth_] := Ppap121v223'[t] == (fsig121v221[en]*Ppa221v223[t] -
    (fsigTot121[en,truth] + fsigTot223[en])*Ppap121v223[t])*jxpulse[t] -
    GamATot121*Ppap121v223[t]
ieqPAP121v223[neginf_,inival_] := Ppap121v223[neginf] == inival

reqPAP103v223[en_,jxpulse_,truth_] := Ppap103v223'[t] == (fsig103v203[en]*Ppa203v223[t] -
    (fsigTot103[en,truth] + fsigTot223[en])*Ppap103v223[t])*jxpulse[t] -
    GamATot103*Ppap103v223[t]
ieqPAP103v223[neginf_,inival_] := Ppap103v223[neginf] == inival

reqPAP112v223[en_,jxpulse_,truth_] := Ppap112v223'[t] == (fsig112v212[en]*Ppa212v223[t] -
    (fsigTot112[en,truth] + fsigTot223[en])*Ppap112v223[t])*jxpulse[t] -
    GamATot112*Ppap112v223[t]
ieqPAP112v223[neginf_,inival_] := Ppap112v223[neginf] == inival
```

Two-site PAPs:

```

reqPAP221v123[en_,jxpulse_,truth_]:=Ppap221v123'[t]==(fsig123v223[en]*Ppa221v223[t] -
  (fsigTot221[en]+fsigTot123[en,truth])*Ppap221v123[t])*jxpulse[t] -
  GamATot123*Ppap221v123[t]
ieqPAP221v123[neginf_,inival_]:=Ppap221v123[neginf]==inival

reqPAP203v123[en_,jxpulse_,truth_]:=Ppap203v123'[t]==(fsig123v223[en]*Ppa203v223[t] -
  (fsigTot203[en]+fsigTot123[en,truth])*Ppap203v123[t])*jxpulse[t] -
  GamATot123*Ppap203v123[t]
ieqPAP203v123[neginf_,inival_]:=Ppap203v123[neginf]==inival

reqPAP212v123[en_,jxpulse_,truth_]:=Ppap212v123'[t]==(fsig123v223[en]*Ppa212v223[t] -
  (fsigTot212[en]+fsigTot123[en,truth])*Ppap212v123[t])*jxpulse[t] -
  GamATot123*Ppap212v123[t]
ieqPAP212v123[neginf_,inival_]:=Ppap212v123[neginf]==inival

```

```

reqPAP[en_,jxpulse_]:=Ppap'[t]==(fsig121v221[en]*Ppa221v223[t]+fsig103v203[en] *
  Ppa203v223[t]+fsig112v212[en]*Ppa212v223[t]+fsig123v223[en]*Ppa221v223[t] +
  fsig123v223[en]*Ppa203v223[t]+fsig123v223[en]*Ppa212v223[t])*jxpulse[t]
ieqPAP[neginf_,inival_]:=Ppap[neginf]==inival

```

```

reqPAPA[]:=Ppapa'[t]==GamATot121*Ppap121v223[t]+GamATot103*Ppap103v223[t] +
  GamATot112*Ppap112v223[t]+GamATot123*(Ppap221v123[t]+Ppap203v123[t] +
  Ppap212v123[t])
ieqPAPA[neginf_,inival_]:=Ppapa[neginf]==inival

```

Decay of SCHs:

```

reqSCHd[]:=Pschd'[t]==GamATot123*2*P223[t]*P123[t]
ieqSCHd[neginf_,inival_]:=Pschd[neginf]==inival

```

Decay of ssDCHs:

```

reqssDCHd[]:=Pssdchd'[t]==GamATot023*2*P223[t]*P023[t]
ieqssDCHd[neginf_,inival_]:=Pssdchd[neginf]==inival

```

Decay of tsDCHs:

```
reqtsDCHd[]:=Ptsdchd'[t]==2*GamATot123*P123[t]^2
ieqtsDCHd[neginf_,inival_]:=Ptsdchd[neginf]==inival
```

## Solve linear system of differential equations

```
papaSolveRateEqs[en_,jxfunc_,neginf_,posinf_,maxfrac_,truth_]:=
Module[{grndvec},
grndvec=unitgrndvec[];
NDSolve[{
(* Molecular rate equations *)
reqPA221v223[en,jxfunc],ieqPA221v223[neginf,0],
reqPA203v223[en,jxfunc],ieqPA203v223[neginf,0],
reqPA212v223[en,jxfunc],ieqPA212v223[neginf,0],
reqPAP121v223[en,jxfunc,truth],ieqPAP121v223[neginf,0],
reqPAP103v223[en,jxfunc,truth],ieqPAP103v223[neginf,0],
reqPAP112v223[en,jxfunc,truth],ieqPAP112v223[neginf,0],
reqPAP221v123[en,jxfunc,truth],ieqPAP221v123[neginf,0],
reqPAP203v123[en,jxfunc,truth],ieqPAP203v123[neginf,0],
reqPAP212v123[en,jxfunc,truth],ieqPAP212v123[neginf,0],
reqPAP[en,jxfunc],ieqPAP[neginf,0],
reqPAPA[],ieqPAPA[neginf,0],
reqSCHd[],ieqSCHd[neginf,0],
reqssDCHd[],ieqssDCHd[neginf,0],
reqtsDCHd[],ieqtsDCHd[neginf,0],
(* Atomic rate equations *)
req223[en,jxfunc],ieq223[neginf,grndvec[[1]]],
req213[en,jxfunc],ieq213[neginf,grndvec[[2]]],
req222[en,jxfunc],ieq222[neginf,grndvec[[3]]],
req123[en,jxfunc,truth],ieq123[neginf,grndvec[[4]]],
req212[en,jxfunc],ieq212[neginf,grndvec[[5]]],
req203[en,jxfunc],ieq203[neginf,grndvec[[6]]],
req221[en,jxfunc],ieq221[neginf,grndvec[[7]]],
req113[en,jxfunc,truth],ieq113[neginf,grndvec[[8]]],
req122[en,jxfunc,truth],ieq122[neginf,grndvec[[9]]],
```

```

req023[en,jxfunc,truth],ieq023[neginf,grndvec[[10]]],
req202[en,jxfunc],ieq202[neginf,grndvec[[11]]],
req211[en,jxfunc],ieq211[neginf,grndvec[[12]]],
req220[en,jxfunc],ieq220[neginf,grndvec[[13]]],
req103[en,jxfunc,truth],ieq103[neginf,grndvec[[14]]],
req112[en,jxfunc,truth],ieq112[neginf,grndvec[[15]]],
req121[en,jxfunc,truth],ieq121[neginf,grndvec[[16]]],
req013[en,jxfunc,truth],ieq013[neginf,grndvec[[17]]],
req022[en,jxfunc,truth],ieq022[neginf,grndvec[[18]]],
req201[en,jxfunc],ieq201[neginf,grndvec[[19]]],
req210[en,jxfunc],ieq210[neginf,grndvec[[20]]],
req102[en,jxfunc,truth],ieq102[neginf,grndvec[[21]]],
req111[en,jxfunc,truth],ieq111[neginf,grndvec[[22]]],
req120[en,jxfunc,truth],ieq120[neginf,grndvec[[23]]],
req003[en,jxfunc,truth],ieq003[neginf,grndvec[[24]]],
req012[en,jxfunc,truth],ieq012[neginf,grndvec[[25]]],
req021[en,jxfunc,truth],ieq021[neginf,grndvec[[26]]],
req200[en,jxfunc],ieq200[neginf,grndvec[[27]]],
req101[en,jxfunc,truth],ieq101[neginf,grndvec[[28]]],
req110[en,jxfunc,truth],ieq110[neginf,grndvec[[29]]],
req011[en,jxfunc,truth],ieq011[neginf,grndvec[[30]]],
req020[en,jxfunc,truth],ieq020[neginf,grndvec[[31]]],
req002[en,jxfunc,truth],ieq002[neginf,grndvec[[32]]],
req100[en,jxfunc],ieq100[neginf,grndvec[[33]]],
req010[en,jxfunc,truth],ieq010[neginf,grndvec[[34]]],
req001[en,jxfunc,truth],ieq001[neginf,grndvec[[35]]],
req000[en,jxfunc],ieq000[neginf,grndvec[[36]]] },
{Ppa221v223[t],Ppa203v223[t],Ppa212v223[t],
Ppap121v223[t],Ppap103v223[t],Ppap112v223[t],
Ppap221v123[t],Ppap203v123[t],Ppap212v123[t],
Ppap[t],Ppapa[t],Pschd[t],Pssdchd[t],Ptsdchd[t],
P223[t],P213[t],P222[t],P123[t],P212[t],P203[t],P221[t],P113[t],
P122[t],P023[t],P202[t],P211[t],P220[t],P103[t],P112[t],P121[t],
P013[t],P022[t],P201[t],P210[t],P102[t],P111[t],P120[t],P003[t],
P012[t],P021[t],P200[t],P101[t],P110[t],P011[t],P020[t],P002[t],

```

```
P100[t],P010[t],P001[t],P000[t]}, {t,neginf, posinf},
MaxStepFraction->maxfrac,MaxSteps->50000]
]
```

## Rate equation model for a nitrogen molecule with a parameter for delayed fragmentation of the $N_2^{2+}$ molecular ion

Molecular rate equations 1 + 3 + 12 + 17 = 33:

Neutral: dsmeq223k223

Minus one: dsmeq213k223 dsmeq222k223 dsmeq123k223

Minus two: dsmeq213k213 dsmeq213k222 dsmeq212k223 dsmeq203k223 dsmeq222k222  
 dsmeq221k223 dsmeq123k213 dsmeq113k223 dsmeq123k222 dsmeq122k223  
 dsmeq123k123 dsmeq023k223

Minus three: dsmeq103k223 dsmeq112k223 dsmeq121k223 dsmeq203k123 dsmeq212k123  
 dsmeq221k123 dsmeq113k213 dsmeq122k213 dsmeq113k222 dsmeq122k222  
 dsmeq113k123 dsmeq122k123 dsmeq023k213 dsmeq023k222 dsmeq013k223  
 dsmeq022k223 dsmeq023k123

Molecular-atomic rate equations 1 + 2 + 6 = 9 for feeding probability from the molecular rate equations into the atomic rate equations:

Neutral: dsreq223

Minus one: dsreq213 dsreq222

Minus two: dsreq203 dsreq212 dsreq221 dsreq113 dsreq122 dsreq023

## Model parameters

inclDCH for ssDCH and incltsDCH for tsDCH

```
incltsDCH[truth_] := If[truth, 1, 0]
```

Fragmentation value from the experimental dissociation cross section measurement "nitrogen\_paper.nb" using Ref. [10]:

```
fragNppN := 0.26
fragNpNp := 1 - fragNppN
```

Fragmentation delay constant:

```
gammaFrag = 1 / (1000 * FemtoSecondTot0)
```

## Neutral

### No core holes

```
dsmeq223k223[en_, jxpulse_] := C223k223'[t] == -2 * fsigTot223[en] * C223k223[t] * jxpulse[t]
```

(\* the state does not decay \*)

```
dsseq223k223[neginf_, inival_] := C223k223[neginf] == inival
```

```
dsreq223[en_, jxpulse_, truth_, fragNppN_, gammaFrag_] := P223'[t] == req223[en, jxpulse][[2]] +
```

(\* C203k223, C212k223, C221k223 REqs \*)

```
fragNppN * gammaFrag * 1/2 * (C203k223[t] + C212k223[t] + C221k223[t]) +
```

(\* C213k213, C213k222, C222k222 REqs \*)

```
fragNpNp * gammaFrag * 1/2 * (C213k213[t] + C213k222[t] + C222k222[t])
```

## Minus one

### No core holes

```
dsmeq213k223[en_,jxpulse_,truth_] := C213k223'[t] == (2*fsig213v223[en]*C223k223[t] -
  (fsigTot223[en]+fsigTot213[en])*C213k223[t])*jxpulse[t]
  (* the state does not fragment *) (* the state does not decay *)
dsseq213k223[neginf_,inival_] := C213k223[neginf] == inival
```

```
dsmeq222k223[en_,jxpulse_,truth_] := C222k223'[t] == (2*fsig222v223[en]*C223k223[t] -
  (fsigTot223[en]+fsigTot222[en])*C222k223[t])*jxpulse[t]
  (* the state does not fragment *) (* the state does not decay *)
dsseq222k223[neginf_,inival_] := C222k223[neginf] == inival
```

```
dsreq213[en_,jxpulse_,truth_,fragNpNp_,gammaFrag_] := P213'[t] == req213[en,jxpulse][[2]] +
  (* C203k223, C212k223, C221k223 REQs *)
  fragNpNp*gammaFrag*1/2*(C203k223[t]+C212k223[t]+C221k223[t]) +
  (* C213k213, C213k222 REQs *)
  fragNpNp*gammaFrag*1/2*(2*C213k213[t]+C213k222[t]) +
  (* C213k213, C213k222, C203k223 REQs *)
  1/2*(fsig212v222[en]+fsig221v222[en])*C213k222[t]*jxpulse[t] +
  1/2*(2*fsig212v213[en]+2*fsig203v213[en])*C213k213[t]*jxpulse[t] +
  1/2*(1/2*fsig202v203[en]+fsig213v223[en])*C203k223[t]*jxpulse[t] +
  (* C221k223, C212k223 REQs *)
  1/2*(1/2*fsig211v221[en]+1/2*fsig220v221[en]+fsig213v223[en])*C221k223[t]*jxpulse[t] +
  1/2*(1/2*fsig202v212[en]+1/2*fsig211v212[en]+fsig213v223[en])*C212k223[t]*jxpulse[t] +
  (* C113k223, C122k223 REQs *)
  1/2*GamATot123*C123k213[t]+1/2*1/2*GamATot113*C113k223[t] +
  1/2*1/2*GamATot122*C122k223[t]
```

```

dsreq222[en_,jxpulse_,truth_,fragNpNp_,gammaFrag_]:=P222'[t]==req222[en,jxpulse][[2]]+
  (* C203k222, C212k222, C221k222 REQs *)
  fragNpNp*gammaFrag*1/2*(C203k222[t]+C212k222[t]+C221k222[t])+
  (* C213k222, C222k222 REQs *)
  fragNpNp*gammaFrag*1/2*(C213k222[t]+2*C222k222[t])+
  (* C213k222, C222k222, C203k223 REQs *)
  1/2*(fsig203v213[en]+fsig212v213[en])*C213k222[t]*jxpulse[t]+
  1/2*(2*fsig212v222[en]+2*fsig221v222[en])*C222k222[t]*jxpulse[t]+
  1/2*(1/2*fsig202v203[en]+fsig222v223[en])*C203k223[t]*jxpulse[t]+
  (* C221k223, C212k223 REQs *)
  1/2*(1/2*fsig211v221[en]+1/2*fsig220v221[en]+fsig222v223[en])*C221k223[t]*jxpulse[t]+
  1/2*(1/2*fsig202v212[en]+1/2*fsig211v212[en]+fsig222v223[en])*C212k223[t]*jxpulse[t]+
  (* C113k223, C122k223 REQs *)
  1/2*1/2*GamATot113*C113k223[t]+
  1/2*GamATot123*C123k222[t]+1/2*1/2*GamATot122*C122k223[t]

```

## Single core hole

```

dsmeq123k223[en_,jxpulse_,truth_,truthTS_]:=C123k223'[t]==(2*fsig123v223[en]*C223k223[t]-
  (fsig213v223[en]+fsig222v223[en]+
  incltsDCH[truthTS]*fsig123v223[en]+fsigTot123[en,truth])*C123k223[t])*jxpulse[t]-
  GamATot123*C123k223[t]
  (* the state does not fragment *)
dsseq123k223[neginf_,inival_]:=C123k223[neginf]==inival

```

## Minus two

## No core holes

```

dsmeq213k213[en_,jxpulse_,gammaFrag_]:=C213k213'[t]==(fsig213v223[en]*C213k223[t]-
  2*fsigTot213[en]*C213k213[t])*jxpulse[t]-gammaFrag*C213k213[t]
  (* the state does not decay *)
dsseq213k213[neginf_,inival_]:=C213k213[neginf]==inival

```

C213k222 and C222k213 are the same molecular configuration

```
dsmeq213k222[en_,jxpulse_,gammaFrag_]:=C213k222'[t]==(fsig222v223[en]*C213k223[t]+
  fsig213v223[en]*C222k223[t]-(fsigTot213[en]+fsigTot222[en])*C213k222[t])*jxpulse[t]-
  gammaFrag*C213k222[t]
(* the state does not decay *)
dsseq213k222[neginf_,inival_]:=C213k222[neginf]==inival
```

```
dsmeq212k223[en_,jxpulse_,gammaFrag_]:=C212k223'[t]==(fsig212v213[en]*C213k223[t]+
  fsig212v222[en]*C222k223[t]-(fsigTot212[en]+fsigTot223[en])*C212k223[t])*jxpulse[t]+
  GamA212v123*C123k223[t]-gammaFrag*C212k223[t]
dsseq212k223[neginf_,inival_]:=C212k223[neginf]==inival
```

```
dsmeq203k223[en_,jxpulse_,gammaFrag_]:=C203k223'[t]==(fsig203v213[en]*C213k223[t]-
  (fsigTot203[en]+fsigTot223[en])*C203k223[t])*jxpulse[t]+
  GamA203v123*C123k223[t]-gammaFrag*C203k223[t]
dsseq203k223[neginf_,inival_]:=C203k223[neginf]==inival
```

```
dsmeq222k222[en_,jxpulse_,gammaFrag_]:=C222k222'[t]==(fsig222v223[en]*C222k223[t]-
  2*fsigTot222[en]*C222k222[t])*jxpulse[t]-gammaFrag*C222k222[t]
(* the state does not decay *)
dsseq222k222[neginf_,inival_]:=C222k222[neginf]==inival
```

```
dsmeq221k223[en_,jxpulse_,gammaFrag_]:=C221k223'[t]==(fsig221v222[en]*C222k223[t]-
  (fsigTot221[en]+fsigTot223[en])*C221k223[t])*jxpulse[t]+
  GamA221v123*C123k223[t]-gammaFrag*C221k223[t]
dsseq221k223[neginf_,inival_]:=C221k223[neginf]==inival
```

```
dsreq203[en_,jxpulse_,truth_,truthTS_,fragNppN_,gammaFrag_]:=P203'[t]==req203[en,jxpulse][[2]]+
  (* C213k222, C213k213, C222k222, C203k223 REqs *)
  fragNppN*gammaFrag*1/2*(1/3*C213k222[t]+1/3*C213k213[t]+1/3*C222k222[t]+C203k223[t])+
  (* C213k222, C213k213, C203k223, C212k223, C221k223 REqs *)
  1/2*fsig203v213[en]*C213k222[t]*jxpulse[t]+
  1/2*2*fsig203v213[en]*C213k213[t]*jxpulse[t]+
  1/2*(fsig213v223[en]+fsig222v223[en]+1/2*fsig202v203[en])*C203k223[t]*jxpulse[t]+
  1/2*1/2*fsig202v212[en]*C212k223[t]*jxpulse[t]+
  1/2*1/3*(fsig211v221[en]+fsig220v221[en])*C221k223[t]*jxpulse[t]+
```

```

(* C123k213, C113k223, C123k222, C122k223 REQs *)
GamA203v123*1/2*C123k213[t]+
1/2*1/3*(GamATot113*C113k223[t]+GamATot122*C122k223[t])+GamA203v123*1/2*C123k222[t]+
(* C103k223, C112k223, C121k223 REQs *)
1/2*1/3*(fsigTot103[en,truth]+fsig222v223[en]+fsig213v223[en])*C103k223[t]*jxpulse[t]+
1/2*1/3*(fsigTot112[en,truth]+fsig222v223[en]+fsig213v223[en])*C112k223[t]*jxpulse[t]+
1/2*1/3*(fsigTot121[en,truth]+fsig222v223[en]+fsig213v223[en])*C121k223[t]*jxpulse[t]+
1/3*(GamATot103*C103k223[t]+GamATot112*C112k223[t]+GamATot121*C121k223[t])+
(* C203k123, C212k123, C221k123 REQs *)
1/2*(1/3*fsig202v203[en]+fsigTot123[en,truth])*C203k123[t]*jxpulse[t]+
1/2*1/3*(fsig211v212[en]+fsig202v212[en])*C212k123[t]*jxpulse[t]+
1/2*1/3*(fsig220v221[en]+fsig211v221[en])*C221k123[t]*jxpulse[t]+
1/2*(GamATot123+GamA203v123)*C203k123[t]+1/2*GamA203v123*C212k123[t]+1/2*GamA203v123*C221k123[t]+
(* C023k213, C023k222, C013k223, C022k223, C023k123 REQs *)
inclDCH[truth]*1/2*(1/3*fsigTot023[en,truth]+fsig203v213[en])*C023k213[t]*jxpulse[t]+
inclDCH[truth]*1/2*1/3*fsigTot023[en,truth]*C023k222[t]*jxpulse[t]+
inclDCH[truth]*1/2*1/3*(fsigTot013[en,truth]+fsig222v223[en]+fsig213v223[en])*C013k223[t]*jxpulse[t]+
inclDCH[truth]*1/2*1/3*(fsigTot022[en,truth]+fsig222v223[en]+fsig213v223[en])*C022k223[t]*jxpulse[t]+
inclDCH[truth]*1/2*1/3*(GamATot023*C023k213[t]+GamATot023*C023k222[t]+
GamATot013*C013k223[t]+GamATot022*C022k223[t])+
inclDCH[truth]*1/2*GamA203v123*C023k123[t]+
(* C113k213, C113k222, C122k213, C122k222 REQs *)
1/2*(1/3*fsigTot113[en,truth]+fsig203v213[en])*C113k213[t]*jxpulse[t]+
1/2*1/3*fsigTot113[en,truth]*C113k222[t]*jxpulse[t]+
1/2*(1/3*fsigTot122[en,truth]+fsig203v213[en])*C122k213[t]*jxpulse[t]+
1/2*1/3*fsigTot122[en,truth]*C122k222[t]*jxpulse[t]+
1/3*(GamATot113*C113k213[t]+GamATot113*C113k222[t]+GamATot122*C122k213[t]+GamATot122*C122k222[t])+
(* C113k123, C122k123 REQs *)
incltsDCH[truthTS]*1/2*(1/3*GamATot113+GamA203v123)*C113k123[t]+
incltsDCH[truthTS]*1/2*(1/3*GamATot122+GamA203v123)*C122k123[t]

```

```

dsreq212[en_,jxpulse_,truth_,truthTS_,fragNppN_,gammaFrag_]:=P212'[t]==req212[en,jxpulse][[2]]+
(* C213k222, C213k213, C222k222, C212k223, C221k223 REQs *)
fragNppN*gammaFrag*1/2*(1/3*C213k222[t]+1/3*C213k213[t]+1/3*C222k222[t]+C212k223[t])+

```

```

(* C213k222, C213k213, C222k222, C203k223, C212k223 REQs *)
1/2*(fsig212v213[en]+fsig212v222[en])*C213k222[t]*jxpulse[t]+
1/2*2*fsig212v213[en]*C213k213[t]*jxpulse[t]+1/2*2*fsig212v222[en]*C222k222[t]*jxpulse[t]+
1/2*1/2*fsig202v203[en]*C203k223[t]*jxpulse[t]+
1/2*(fsig213v223[en]+fsig222v223[en]+1/2*fsig202v212[en]+1/2*fsig211v212[en])*C212k223[t]*jxpulse[t]+
1/2*1/3*(fsig211v221[en]+fsig220v221[en])*C221k223[t]*jxpulse[t]+
(* C123k213, C113k223, C123k222, C122k223 REQs *)
GamA212v123*1/2*C123k213[t]+
1/2*1/3*(GamATot113*C113k223[t]+GamATot122*C122k223[t])+GamA212v123*1/2*C123k222[t]+
(* C103k223, C112k223, C121k223 REQs *)
1/2*1/3*(fsigTot103[en,truth]+fsig222v223[en]+fsig213v223[en])*C103k223[t]*jxpulse[t]+
1/2*1/3*(fsigTot112[en,truth]+fsig222v223[en]+fsig213v223[en])*C112k223[t]*jxpulse[t]+
1/2*1/3*(fsigTot121[en,truth]+fsig222v223[en]+fsig213v223[en])*C121k223[t]*jxpulse[t]+
1/3*(GamATot103*C103k223[t]+GamATot112*C112k223[t]+GamATot121*C121k223[t])+
(* C203k123, C212k123, C221k123 REQs *)
1/2*1/3*fsig202v203[en]*C203k123[t]*jxpulse[t]+
1/2*(1/3*fsig211v212[en]+1/3*fsig202v212[en]+fsigTot123[en,truth])*C212k123[t]*jxpulse[t]+
1/2*1/3*(fsig220v221[en]+fsig211v221[en])*C221k123[t]*jxpulse[t]+
1/2*GamA212v123*C203k123[t]+1/2*(GamATot123+GamA212v123)*C212k123[t]+1/2*GamA212v123*C221k123[t]+
(* C023k213, C023k222, C013k223, C022k223, C023k123 REQs *)
inclDCH[truth]*1/2*(1/3*fsigTot023[en,truth]+fsig212v213[en])*C023k213[t]*jxpulse[t]+
inclDCH[truth]*1/2*(1/3*fsigTot023[en,truth]+fsig212v222[en])*C023k222[t]*jxpulse[t]+
inclDCH[truth]*1/2*1/3*(fsigTot013[en,truth]+fsig222v223[en]+fsig213v223[en])*C013k223[t]*jxpulse[t]+
inclDCH[truth]*1/2*1/3*(fsigTot022[en,truth]+fsig222v223[en]+fsig213v223[en])*C022k223[t]*jxpulse[t]+
inclDCH[truth]*1/2*1/3*(GamATot023*C023k213[t]+GamATot023*C023k222[t]+
GamATot013*C013k223[t]+GamATot022*C022k223[t])+
inclDCH[truth]*1/2*GamA212v123*C023k123[t]+
(* C113k213, C113k222, C122k213, C122k222 REQs *)
1/2*(1/3*fsigTot113[en,truth]+fsig212v213[en])*C113k213[t]*jxpulse[t]+
1/2*(1/3*fsigTot113[en,truth]+fsig212v222[en])*C113k222[t]*jxpulse[t]+
1/2*(1/3*fsigTot122[en,truth]+fsig212v213[en])*C122k213[t]*jxpulse[t]+
1/2*(1/3*fsigTot122[en,truth]+fsig212v222[en])*C122k222[t]*jxpulse[t]+
1/3*(GamATot113*C113k213[t]+GamATot113*C113k222[t]+GamATot122*C122k213[t]+GamATot122*C122k222[t])+
(* C113k123, C122k123 REQs *)

```

```

incltsDCH[truthTS]*1/2*(1/3*GamATot113+GamA212v123)*C113k123[t]+
incltsDCH[truthTS]*1/2*(1/3*GamATot122+GamA212v123)*C122k123[t]

```

```

dsreq221[en_,jxpulse_,truth_,truthTS_,fragNppN_,gammaFrag_]:=P221'[t]==req221[en,jxpulse][[2]]+
(* C213k222, C213k213, C222k222, C221k223 REqs *)
fragNppN*gammaFrag*1/2*(1/3*C213k222[t]+1/3*C213k213[t]+1/3*C222k222[t]+C221k223[t])+
(* C213k222, C222k222, C212k223, C221k223 REqs *)
1/2*fsig221v222[en]*C213k222[t]*jxpulse[t]+
1/2*2*fsig221v222[en]*C222k222[t]*jxpulse[t]+
1/2*1/2*fsig211v212[en]*C212k223[t]*jxpulse[t]+
1/2*(fsig222v223[en]+fsig213v223[en]+1/3*fsig211v221[en]+1/3*fsig220v221[en])*C221k223[t]*jxpulse[t]+
(* C123k213, C113k223, C123k222, C122k223 REqs *)
GamA221v123*1/2*C123k213[t]+
1/2*1/3*(GamATot113*C113k223[t]+GamATot122*C122k223[t])+GamA221v123*1/2*C123k222[t]+
(* C103k223, C112k223, C121k223 REqs *)
1/2*1/3*(fsigTot103[en,truth]+fsig222v223[en]+fsig213v223[en])*C103k223[t]*jxpulse[t]+
1/2*1/3*(fsigTot112[en,truth]+fsig222v223[en]+fsig213v223[en])*C112k223[t]*jxpulse[t]+
1/2*1/3*(fsigTot121[en,truth]+fsig222v223[en]+fsig213v223[en])*C121k223[t]*jxpulse[t]+
1/3*(GamATot103*C103k223[t]+GamATot112*C112k223[t]+GamATot121*C121k223[t])+
(* C203k123, C212k123, C221k123 REqs *)
1/2*1/3*fsig202v203[en]*C203k123[t]*jxpulse[t]+
1/2*1/3*(fsig211v212[en]+fsig202v212[en])*C212k123[t]*jxpulse[t]+
1/2*(1/3*fsig220v221[en]+1/3*fsig211v221[en]+fsigTot123[en,truth])*C221k123[t]*jxpulse[t]+
1/2*GamA221v123*C203k123[t]+1/2*(GamATot123+GamA221v123)*C221k123[t]+1/2*GamA221v123*C212k123[t]+
(* C023k213, C023k222, C013k223, C022k223, C023k123 REqs *)
inclDCH[truth]*1/2*1/3*fsigTot023[en,truth]*C023k213[t]*jxpulse[t]+
inclDCH[truth]*1/2*(1/3*fsigTot023[en,truth]+fsig221v222[en])*C023k222[t]*jxpulse[t]+
inclDCH[truth]*1/2*1/3*(fsigTot013[en,truth]+fsig222v223[en]+fsig213v223[en])*C013k223[t]*jxpulse[t]+
inclDCH[truth]*1/2*1/3*(fsigTot022[en,truth]+fsig222v223[en]+fsig213v223[en])*C022k223[t]*jxpulse[t]+
inclDCH[truth]*1/2*1/3*(GamATot023*C023k213[t]+GamATot023*C023k222[t]+
GamATot013*C013k223[t]+GamATot022*C022k223[t])+
inclDCH[truth]*1/2*GamA221v123*C023k123[t]+
(* C113k213, C113k222, C122k213, C122k222 REqs *)
1/2*1/3*fsigTot113[en,truth]*C113k213[t]*jxpulse[t]+
1/2*(1/3*fsigTot113[en,truth]+fsig221v222[en])*C113k222[t]*jxpulse[t]+

```

```

1/2*1/3*fsigTot122[en,truth]*C122k213[t]*jxpulse[t]+
1/2*(1/3*fsigTot122[en,truth]+fsig221v222[en])*C122k222[t]*jxpulse[t]+
1/3*(GamATot113*C113k213[t]+GamATot113*C113k222[t]+GamATot122*C122k213[t]+GamATot122*C122k222[t])+
(* C113k123, C122k123 REqs *)
incltsDCH[truthTS]*1/2*(1/3*GamATot113+GamA221v123)*C113k123[t]+
incltsDCH[truthTS]*1/2*(1/3*GamATot122+GamA221v123)*C122k123[t]

```

## Single core hole

```

dsmeq123k213[en_,jxpulse_,truth_,truthTS_] := C123k213'[t] == (fsig213v223[en]*C123k223[t] +
fsig123v223[en]*C213k223[t] - (fsigTot123[en,truth]+fsig203v213[en]+fsig212v213[en] +
incltsDCH[truthTS]*fsig113v213[en])*C123k213[t])*jxpulse[t] -
GamATot123*C123k213[t]
(* the state does not fragment *)
dsseq123k213[neginf_,inival_] := C123k213[neginf] == inival

```

```

dsmeq113k223[en_,jxpulse_,truth_,truthTS_] := C113k223'[t] == (fsig113v213[en]*C213k223[t] +
fsig113v123[en]*C123k223[t] - (fsigTot113[en,truth]+fsig213v223[en]+fsig222v223[en] +
incltsDCH[truthTS]*fsig123v223[en])*C113k223[t])*jxpulse[t] -
GamATot113*C113k223[t]
(* the state does not fragment *)
dsseq113k223[neginf_,inival_] := C113k223[neginf] == inival

```

```

dsmeq123k222[en_,jxpulse_,truth_,truthTS_] := C123k222'[t] == (fsig123v223[en]*C222k223[t] +
fsig222v223[en]*C123k223[t] - (fsigTot123[en,truth]+fsig212v222[en]+fsig221v222[en] +
incltsDCH[truthTS]*fsig122v222[en])*C123k222[t])*jxpulse[t] -
GamATot123*C123k222[t]
(* the state does not fragment *)
dsseq123k222[neginf_,inival_] := C123k222[neginf] == inival

```

```

dsmeq122k223[en_,jxpulse_,truth_,truthTS_]:=C122k223'[t]==(fsig122v222[en]*C222k223[t]+
  fsig122v123[en]*C123k223[t]-(fsigTot122[en,truth]+fsig213v223[en]+fsig222v223[en]+
  incltsDCH[truthTS]*fsig123v223[en])*C122k223[t])*jxpulse[t]-
  GamATot122*C122k223[t]
(* the state does not fragment *)
dsseq122k223[neginf_,inival_]:=C122k223[neginf]==inival

```

```

dsreq113[en_,jxpulse_,truth_,truthTS_]:=P113'[t]==req113[en,jxpulse,truth][[2]]+
(* C103k223, C112k223, C121k223 REQs *)
1/2*(1/2*fsig102v103[en]+1/2*fsig222v223[en]+
  1/2*fsig213v223[en]+incltsDCH[truthTS]*fsig123v223[en])*C103k223[t]*jxpulse[t]+
1/2*(1/2*fsig111v112[en]+1/2*fsig102v112[en]+
  1/2*fsig222v223[en]+1/2*fsig213v223[en]+incltsDCH[truthTS]*fsig123v223[en])*C112k223[t]*jxpulse[t]+
1/2*(1/2*fsig120v121[en]+1/2*fsig111v121[en]+
  1/2*fsig222v223[en]+1/2*fsig213v223[en]+incltsDCH[truthTS]*fsig123v223[en])*C121k223[t]*jxpulse[t]+
(* C203k123, C212k123, C221k123 REQs *)
1/2*(incltsDCH[truthTS]*fsig103v203[en]+1/2*fsig202v203[en]+fsig113v123[en])*C203k123[t]*jxpulse[t]+
1/2*(1/2*fsig211v212[en]+1/2*fsig202v212[en]+
  incltsDCH[truthTS]*fsig112v212[en]+fsig113v123[en])*C212k123[t]*jxpulse[t]+
1/2*(1/2*fsig220v221[en]+1/2*fsig211v221[en]+
  incltsDCH[truthTS]*fsig121v221[en]+fsig113v123[en])*C221k123[t]*jxpulse[t]+
(* C023k213, C023k222, C013k223, C022k223, C023k123 REQs *)
inclDCH[truth]*1/2*fsig113v213[en]*C023k213[t]*jxpulse[t]+
inclDCH[truth]*1/2*1/2*fsig123v223[en]*C013k223[t]*jxpulse[t]+
inclDCH[truth]*1/2*1/2*fsig123v223[en]*C022k223[t]*jxpulse[t]+
inclDCH[truth]*1/2*(1/2*fsigTot023[en,truth]+fsig113v123[en])*C023k123[t]*jxpulse[t]+
inclDCH[truth]*1/2*(1/2*GamATot023*C023k213[t]+1/2*GamATot023*C023k222[t]+
  1/2*GamATot013*C013k223[t]+1/2*GamATot022*C022k223[t]+GamATot023*C023k123[t])*
(* C113k213, C113k222, C122k213, C122k222 REQs *)
1/2*(1/2*fsig112v113[en]+1/2*fsig103v113[en]+fsig212v213[en]+fsig203v213[en]+
  incltsDCH[truthTS]*2*fsig113v213[en])*C113k213[t]*jxpulse[t]+
1/2*(1/2*fsig112v113[en]+1/2*fsig103v113[en]+fsig212v222[en]+fsig221v222[en]+

```

```

    incltsDCH[truthTS]*fsig122v222[en])*C113k222[t]*jxpulse[t]+
1/2*(1/2*fsig121v122[en]+1/2*fsig112v122[en]+
    incltsDCH[truthTS]*fsig113v213[en])*C122k213[t]*jxpulse[t]+
1/2*1/2*(fsig121v122[en]+fsig112v122[en])*C122k222[t]*jxpulse[t]+
(* C113k123, C122k123 REQs *)
incltsDCH[truthTS]*(
    1/2*(fsig112v113[en]+fsig103v113[en]+1/2*inclDCH[truth]*fsig013v113[en]+fsig122v123[en]+
        2*fsig113v123[en]+inclDCH[truth]*fsig023v123[en])*C113k123[t]*jxpulse[t]+
    1/2*(fsig121v122[en]+fsig112v122[en]+
        1/2*inclDCH[truth]*fsig022v122[en]+fsig113v123[en])*C122k123[t]*jxpulse[t]+
    1/2*(1/2*GamATot113+GamATot123)*C113k123[t]+
    1/2*1/2*GamATot122*C122k123[t])

```

```

dsreq122[en_,jxpulse_,truth_,truthTS_-:P122'[t]==req122[en,jxpulse,truth][[2]]+
(* C103k223, C112k223, C121k223 REQs *)
1/2*(1/2*fsig102v103[en]+1/2*fsig222v223[en]+
    1/2*fsig213v223[en]+incltsDCH[truthTS]*fsig123v223[en])*C103k223[t]*jxpulse[t]+
1/2*(1/2*fsig111v112[en]+1/2*fsig102v112[en]+
    1/2*fsig222v223[en]+1/2*fsig213v223[en]+incltsDCH[truthTS]*fsig123v223[en])*C112k223[t]*jxpulse[t]+
1/2*(1/2*fsig120v121[en]+1/2*fsig111v121[en]+
    1/2*fsig222v223[en]+1/2*fsig213v223[en]+incltsDCH[truthTS]*fsig123v223[en])*C121k223[t]*jxpulse[t]+
(* C203k123, C212k123, C221k123 REQs *)
1/2*(incltsDCH[truthTS]*fsig103v203[en]+1/2*fsig202v203[en]+fsig122v123[en])*C203k123[t]*jxpulse[t]+
1/2*(1/2*fsig211v212[en]+1/2*fsig202v212[en]+
    incltsDCH[truthTS]*fsig112v212[en]+fsig122v123[en])*C212k123[t]*jxpulse[t]+
1/2*(1/2*fsig220v221[en]+1/2*fsig211v221[en]+
    incltsDCH[truthTS]*fsig121v221[en]+fsig122v123[en])*C221k123[t]*jxpulse[t]+
(* C023k213, C023k222, C013k223, C022k223, C023k123 REQs *)
inclDCH[truth]*1/2*fsig122v222[en]*C023k222[t]*jxpulse[t]+
inclDCH[truth]*1/2*1/2*fsig123v223[en]*C013k223[t]*jxpulse[t]+
inclDCH[truth]*1/2*1/2*fsig123v223[en]*C022k223[t]*jxpulse[t]+
inclDCH[truth]*1/2*(1/2*fsigTot023[en,truth]+fsig122v123[en])*C023k123[t]*jxpulse[t]+

```

```

inclDCH[truth]*1/2*(1/2*GamATot023*C023k213[t]+1/2*GamATot023*C023k222[t]+
    1/2*GamATot013*C013k223[t]+1/2*GamATot022*C022k223[t]+GamATot023*C023k123[t])+
(* C113k213, C113k222, C122k213, C122k222 REqs *)
1/2*1/2*(fsig112v113[en]+fsig103v113[en])*C113k213[t]*jxpulse[t]+
1/2*(1/2*fsig112v113[en]+1/2*fsig103v113[en]+
    incltsDCH[truthTS]*fsig122v222[en])*C113k222[t]*jxpulse[t]+
1/2*(1/2*fsig121v122[en]+1/2*fsig112v122[en]+fsig212v213[en]+fsig203v213[en]+
    incltsDCH[truthTS]*fsig113v213[en])*C122k213[t]*jxpulse[t]+
1/2*(1/2*fsig121v122[en]+1/2*fsig112v122[en]+fsig221v222[en]+fsig212v222[en]+
    incltsDCH[truthTS]*2*fsig122v222[en])*C122k222[t]*jxpulse[t]+
(* C113k123, C122k123 REqs *)
incltsDCH[truthTS]*(
    1/2*(fsig112v113[en]+fsig103v113[en]+
        1/2*inclDCH[truth]*fsig013v113[en]+fsig122v123[en])*C113k123[t]*jxpulse[t]+
    1/2*(fsig121v122[en]+fsig112v122[en]+1/2*inclDCH[truth]*fsig022v122[en]+
        2*fsig122v123[en]+fsig113v123[en]+inclDCH[truth]*fsig023v123[en])*C122k123[t]*jxpulse[t]+
    1/2*1/2*GamATot113*C113k123[t]+
    1/2*(1/2*GamATot122+GamATot123)*C122k123[t])

```

## Double core holes

```

dsmeq123k123[en_,jxpulse_,truth_,truthTS_]:=C123k123'[t]==incltsDCH[truthTS]*(fsig123v223[en]*C123k223[t]-
    2*fsigTot123[en,truth]*C123k123[t])*jxpulse[t]-
incltsDCH[truthTS]*2*GamATot123*C123k123[t]
(* the state does not fragment *)
dsseq123k123[neginf_,inival_]:=C123k123[neginf]==inival

```

```

dsmeq023k223[en_,jxpulse_,truth_]:=C023k223'[t]==inclDCH[truth]*(
    (fsigTot023[en,truth]+fsigTot223[en])*C023k223[t])*jxpulse[t]-
    GamATot023*C023k223[t])
(* the state does not fragment *)
dsseq023k223[neginf_,inival_]:=C023k223[neginf]==inival

```

```

dsreq023[en_,jxpulse_,truth_,truthTS_-]:=P023'[t]==req023[en,jxpulse,truth][[2]]+
  (* C103k223, C112k223, C121k223 REQs *)
  inclDCH[truth]*1/2*fsig003v103[en]*C103k223[t]*jxpulse[t]+
  inclDCH[truth]*1/2*fsig012v112[en]*C112k223[t]*jxpulse[t]+
  inclDCH[truth]*1/2*fsig021v121[en]*C121k223[t]*jxpulse[t]+
  (* C203k123, C212k123, C221k123 REQs *)
  inclDCH[truth]*1/2*fsig023v123[en]*C203k123[t]*jxpulse[t]+
  inclDCH[truth]*1/2*fsig023v123[en]*C212k123[t]*jxpulse[t]+
  inclDCH[truth]*1/2*fsig023v123[en]*C221k123[t]*jxpulse[t]+
  (* C023k213, C023k222, C013k223, C022k223, C023k123 REQs *)
  inclDCH[truth]*1/2*(fsigTot023[en,truth]+fsigTot213[en])*C023k213[t]*jxpulse[t]+
  inclDCH[truth]*1/2*(fsigTot023[en,truth]+fsigTot222[en])*C023k222[t]*jxpulse[t]+
  inclDCH[truth]*1/2*(fsigTot013[en,truth]+fsigTot223[en])*C013k223[t]*jxpulse[t]+
  inclDCH[truth]*1/2*(fsigTot022[en,truth]+fsigTot223[en])*C022k223[t]*jxpulse[t]+
  inclDCH[truth]*1/2*(fsigTot023[en,truth]+fsig122v123[en]+
    fsig113v123[en]+2*fsig023v123[en])*C023k123[t]*jxpulse[t]+
  inclDCH[truth]*1/2*GamATot123*C023k123[t]+
  (* C113k213, C113k222, C122k213, C122k222 REQs *)
  1/2*inclDCH[truth]*fsig013v113[en]*C113k213[t]*jxpulse[t]+
  1/2*inclDCH[truth]*fsig013v113[en]*C113k222[t]*jxpulse[t]+
  1/2*inclDCH[truth]*fsig022v122[en]*C122k213[t]*jxpulse[t]+
  1/2*inclDCH[truth]*fsig022v122[en]*C122k222[t]*jxpulse[t]+
  (* C113k123, C122k123 REQs *)
  incltsDCH[truthTS]*
  (1/2*inclDCH[truth]*(fsig013v113[en]+fsig023v123[en])*C113k123[t]*jxpulse[t]+
  1/2*inclDCH[truth]*(fsig022v122[en]+fsig023v123[en])*C122k123[t]*jxpulse[t])

```

## Minus three

### Single core hole

```
dsseq103k223[en_,jxpulse_,truth_,truthTS_] := C103k223'[t] == fsig103v203[en]*C203k223[t]*jxpulse[t] +
  fsig103v113[en]*C113k223[t]*jxpulse[t] +
  inclDCH[truth]*GamA103v023*C023k223[t] - GamATot103*C103k223[t] -
  (fsigTot103[en,truth] + fsig213v223[en] + fsig222v223[en] +
  incltsDCH[truthTS]*fsig123v223[en])*C103k223[t]*jxpulse[t]
(* the state does not fragment *)
dsseq103k223[neginf_,inival_] := C103k223[neginf] == inival
```

```
dsseq112k223[en_,jxpulse_,truth_,truthTS_] := C112k223'[t] == fsig112v212[en]*C212k223[t]*jxpulse[t] +
  (fsig112v113[en]*C113k223[t] + fsig112v122[en]*C122k223[t])*jxpulse[t] +
  inclDCH[truth]*GamA112v023*C023k223[t] - GamATot112*C112k223[t] -
  (fsigTot112[en,truth] + fsig213v223[en] + fsig222v223[en] +
  incltsDCH[truthTS]*fsig123v223[en])*C112k223[t]*jxpulse[t]
(* the state does not fragment *)
dsseq112k223[neginf_,inival_] := C112k223[neginf] == inival
```

```
dsseq121k223[en_,jxpulse_,truth_,truthTS_] := C121k223'[t] == fsig121v221[en]*C221k223[t]*jxpulse[t] +
  fsig121v122[en]*C122k223[t]*jxpulse[t] +
  inclDCH[truth]*GamA121v023*C023k223[t] - GamATot121*C121k223[t] -
  (fsigTot121[en,truth] + fsig213v223[en] + fsig222v223[en] +
  incltsDCH[truthTS]*fsig123v223[en])*C121k223[t]*jxpulse[t]
(* the state does not fragment *)
dsseq121k223[neginf_,inival_] := C121k223[neginf] == inival
```

```

dsmeq203k123[en_,jxpulse_,truth_,truthTS_]:=C203k123'[t]==fsig123v223[en]*C203k223[t]*jxpulse[t]+
  fsig203v213[en]*C123k213[t]*jxpulse[t]+
  incltsDCH[truthTS]*2*GamA203v123*C123k123[t]-
  GamATot123*C203k123[t]-
  (fsigTot123[en,truth]+fsig202v203[en]+incltsDCH[truthTS]*fsig103v203[en])*C203k123[t]*jxpulse[t]
(* the state does not fragment *)
dsseq203k123[neginf_,inival_]:=C203k123[neginf]==inival

```

```

dsmeq212k123[en_,jxpulse_,truth_,truthTS_]:=C212k123'[t]==fsig123v223[en]*C212k223[t]*jxpulse[t]+
  (fsig212v213[en]*C123k213[t]+fsig212v222[en]*C123k222[t])*jxpulse[t]+
  incltsDCH[truthTS]*2*GamA212v123*C123k123[t]-
  GamATot123*C212k123[t]-
  (fsigTot123[en,truth]+fsig211v212[en]+fsig202v212[en]+
  incltsDCH[truthTS]*fsig112v212[en])*C212k123[t]*jxpulse[t]
(* the state does not fragment *)
dsseq212k123[neginf_,inival_]:=C212k123[neginf]==inival

```

```

dsmeq221k123[en_,jxpulse_,truth_,truthTS_]:=C221k123'[t]==fsig123v223[en]*C221k223[t]*jxpulse[t]+
  fsig221v222[en]*C123k222[t]*jxpulse[t]+
  incltsDCH[truthTS]*2*GamA221v123*C123k123[t]-
  GamATot123*C221k123[t]-
  (fsigTot123[en,truth]+fsig211v221[en]+fsig220v221[en]+
  incltsDCH[truthTS]*fsig121v221[en])*C221k123[t]*jxpulse[t]
(* the state does not fragment *)
dsseq221k123[neginf_,inival_]:=C221k123[neginf]==inival

```

```

dsmeq113k213[en_,jxpulse_,truth_,truthTS_]:=C113k213'[t]==2*fsig113v213[en]*C213k213[t]*jxpulse[t]+
  fsig113v123[en]*C123k213[t]*jxpulse[t]+fsig213v223[en]*C113k223[t]*jxpulse[t]-
  GamATot113*C113k213[t]-
  (fsigTot113[en,truth]+fsig212v213[en]+fsig203v213[en]+
  incltsDCH[truthTS]*fsig113v213[en])*C113k213[t]*jxpulse[t]
(* the state does not fragment *)
dsseq113k213[neginf_,inival_]:=C113k213[neginf]==inival

```

```

dsmeq122k213[en_,jxpulse_,truth_,truthTS_] := C122k213'[t] == fsig122v222[en]*C213k222[t]*jxpulse[t] +
  fsig122v123[en]*C123k213[t]*jxpulse[t] + fsig213v223[en]*C122k223[t]*jxpulse[t] -
  GamATot122*C122k213[t] -
  (fsigTot122[en,truth] + fsig212v213[en] + fsig203v213[en] +
  incltsDCH[truthTS]*fsig113v213[en])*C122k213[t]*jxpulse[t]
(* the state does not fragment *)
dsseq122k213[neginf_,inival_] := C122k213[neginf] == inival

```

```

dsmeq113k222[en_,jxpulse_,truth_,truthTS_] := C113k222'[t] == fsig113v213[en]*C213k222[t]*jxpulse[t] +
  fsig222v223[en]*C113k223[t]*jxpulse[t] + fsig113v123[en]*C123k222[t]*jxpulse[t] -
  GamATot113*C113k222[t] -
  (fsigTot113[en,truth] + fsig212v222[en] + fsig221v222[en] +
  incltsDCH[truthTS]*fsig122v222[en])*C113k222[t]*jxpulse[t]
(* the state does not fragment *)
dsseq113k222[neginf_,inival_] := C113k222[neginf] == inival

```

```

dsmeq122k222[en_,jxpulse_,truth_,truthTS_] := C122k222'[t] == 2*fsig122v222[en]*C222k222[t]*jxpulse[t] +
  fsig122v123[en]*C123k222[t]*jxpulse[t] + fsig222v223[en]*C122k223[t]*jxpulse[t] -
  GamATot122*C122k222[t] -
  (fsigTot122[en,truth] + fsig212v222[en] + fsig221v222[en] +
  incltsDCH[truthTS]*fsig122v222[en])*C122k222[t]*jxpulse[t]
(* the state does not fragment *)
dsseq122k222[neginf_,inival_] := C122k222[neginf] == inival

```

## Double core holes

```

dsmeq113k123[en_,jxpulse_,truth_,truthTS_] := C113k123'[t] == incltsDCH[truthTS]*
  (fsig113v213[en]*C123k213[t]*jxpulse[t] +
  fsig123v223[en]*C113k223[t]*jxpulse[t] + 2*fsig113v123[en]*C123k123[t]*jxpulse[t] -
  (GamATot113+GamATot123)*C113k123[t] -
  (fsigTot113[en,truth] + fsigTot123[en,truth])*C113k123[t]*jxpulse[t])
(* the state does not fragment *)
dsseq113k123[neginf_,inival_] := C113k123[neginf] == inival

```

```

dsmeq122k123[en_,jxpulse_,truth_,truthTS_] := C122k123'[t] == incltsDCH[truthTS] *
  (fsig122v222[en] * C123k222[t] * jxpulse[t] +
   fsig123v223[en] * C122k223[t] * jxpulse[t] + 2 * fsig122v123[en] * C123k123[t] * jxpulse[t] -
   (GamATot122 + GamATot123) * C122k123[t] -
   (fsigTot122[en,truth] + fsigTot123[en,truth]) * C122k123[t] * jxpulse[t])
(* the state does not fragment *)
dsseq122k123[neginf_,inival_] := C122k123[neginf] == inival

```

```

dsmeq023k213[en_,jxpulse_,truth_] := C023k213'[t] == inclDCH[truth] * ((fsig023v123[en] * C123k213[t] +
  fsig213v223[en] * C023k223[t]) * jxpulse[t] - GamATot023 * C023k213[t] -
  (fsigTot023[en,truth] + fsigTot213[en]) * C023k213[t] * jxpulse[t])
(* the state does not fragment *)
dsseq023k213[neginf_,inival_] := C023k213[neginf] == inival

```

```

dsmeq023k222[en_,jxpulse_,truth_] := C023k222'[t] == inclDCH[truth] * ((fsig023v123[en] * C123k222[t] +
  fsig222v223[en] * C023k223[t]) * jxpulse[t] - GamATot023 * C023k222[t] -
  (fsigTot023[en,truth] + fsigTot222[en]) * C023k222[t] * jxpulse[t])
(* the state does not fragment *)
dsseq023k222[neginf_,inival_] := C023k222[neginf] == inival

```

```

dsmeq013k223[en_,jxpulse_,truth_] := C013k223'[t] == inclDCH[truth] * ((fsig013v113[en] * C113k223[t] +
  fsig013v023[en] * C023k223[t]) * jxpulse[t] - GamATot013 * C013k223[t] -
  (fsigTot013[en,truth] + fsigTot223[en]) * C013k223[t] * jxpulse[t])
(* the state does not fragment *)
dsseq013k223[neginf_,inival_] := C013k223[neginf] == inival

```

```

dsmeq022k223[en_,jxpulse_,truth_] := C022k223'[t] == inclDCH[truth] * ((fsig022v122[en] * C122k223[t] +
  fsig022v023[en] * C023k223[t]) * jxpulse[t] - GamATot022 * C022k223[t] -
  (fsigTot022[en,truth] + fsigTot223[en]) * C022k223[t] * jxpulse[t])
(* the state does not fragment *)
dsseq022k223[neginf_,inival_] := C022k223[neginf] == inival

```

## Triple core holes

```

dsmeq023k123[en_,jxpulse_,truth_,truthTS_] := C023k123'[t] == inclDCH[truth] * (
  (incltsDCH[truthTS] * 2 * fsig023v123[en] * C123k123[t] +
    fsig123v223[en] * C023k223[t]) * jxpulse[t] -
  (GamATot023 + GamATot123) * C023k123[t] -
  (fsigTot023[en,truth] + fsigTot123[en,truth]) * C023k123[t] * jxpulse[t])
(* the state does not fragment *)
dsseq023k123[neginf_,inival_] := C023k123[neginf] == inival

```

## Solve linear system of differential equations

```
dsSolveRateEqs[en_, jxfunc_, truth_, truthTS_, maxfrac_] := dsSolveRateEqsParams[en,
jxfunc, truth, truthTS, maxfrac, fragNppN, fragNpNp, gammaFrag]
```

```
dsSolveRateEqsParams[en_, jxfunc_, truth_, truthTS_, maxfrac_, fragNppN_, fragNpNp_, gammaFrag_] :=
Module[{neginf, grndvec},
neginf=neginfinity;
grndvec=zerogrndvec[];
NDSolve[{
(* Molecular rate equations *)
dsmeq223k223[en, jxfunc], dsseq223k223[neginf, 1],
dsmeq203k223[en, jxfunc, gammaFrag], dsseq203k223[neginf, 0],
dsmeq212k223[en, jxfunc, gammaFrag], dsseq212k223[neginf, 0],
dsmeq221k223[en, jxfunc, gammaFrag], dsseq221k223[neginf, 0],
dsmeq123k223[en, jxfunc, truth, truthTS], dsseq123k223[neginf, 0],
dsmeq123k123[en, jxfunc, truth, truthTS], dsseq123k123[neginf, 0],
dsmeq023k223[en, jxfunc, truth], dsseq023k223[neginf, 0],
dsmeq113k223[en, jxfunc, truth, truthTS], dsseq113k223[neginf, 0],
dsmeq122k223[en, jxfunc, truth, truthTS], dsseq122k223[neginf, 0],
dsmeq123k222[en, jxfunc, truth, truthTS], dsseq123k222[neginf, 0],
dsmeq123k213[en, jxfunc, truth, truthTS], dsseq123k213[neginf, 0],
dsmeq213k223[en, jxfunc, truth], dsseq213k223[neginf, 0],
```

```

dsmeq222k223[en,jxfunc,truth      ],dsseq222k223[neginf,0],
dsmeq213k213[en,jxfunc,gammaFrag  ],dsseq213k213[neginf,0],
dsmeq213k222[en,jxfunc,gammaFrag  ],dsseq213k222[neginf,0],
dsmeq222k222[en,jxfunc,gammaFrag  ],dsseq222k222[neginf,0],
dsmeq023k213[en,jxfunc,truth      ],dsseq023k213[neginf,0],
dsmeq023k222[en,jxfunc,truth      ],dsseq023k222[neginf,0],
dsmeq013k223[en,jxfunc,truth      ],dsseq013k223[neginf,0],
dsmeq022k223[en,jxfunc,truth      ],dsseq022k223[neginf,0],
dsmeq023k123[en,jxfunc,truth,truthTS],dsseq023k123[neginf,0],
dsmeq103k223[en,jxfunc,truth,truthTS],dsseq103k223[neginf,0],
dsmeq112k223[en,jxfunc,truth,truthTS],dsseq112k223[neginf,0],
dsmeq121k223[en,jxfunc,truth,truthTS],dsseq121k223[neginf,0],
dsmeq203k123[en,jxfunc,truth,truthTS],dsseq203k123[neginf,0],
dsmeq212k123[en,jxfunc,truth,truthTS],dsseq212k123[neginf,0],
dsmeq221k123[en,jxfunc,truth,truthTS],dsseq221k123[neginf,0],
dsmeq113k213[en,jxfunc,truth,truthTS],dsseq113k213[neginf,0],
dsmeq122k213[en,jxfunc,truth,truthTS],dsseq122k213[neginf,0],
dsmeq113k222[en,jxfunc,truth,truthTS],dsseq113k222[neginf,0],
dsmeq122k222[en,jxfunc,truth,truthTS],dsseq122k222[neginf,0],
dsmeq113k123[en,jxfunc,truth,truthTS],dsseq113k123[neginf,0],
dsmeq122k123[en,jxfunc,truth,truthTS],dsseq122k123[neginf,0],
(* Atomic rate equations *)
(* req223[en,jxfunc      ] *)
dsreq223[en,jxfunc,truth,      fragNppN,gammaFrag],ieq223[neginf,grndvec[[ 1]]],
(* req213[en,jxfunc      ] *)
dsreq213[en,jxfunc,truth,      fragNpNp,gammaFrag],ieq213[neginf,grndvec[[ 2]]],
(* req222[en,jxfunc      ] *)
dsreq222[en,jxfunc,truth,      fragNpNp,gammaFrag],ieq222[neginf,grndvec[[ 3]]],
req123[en,jxfunc,truth],ieq123[neginf,grndvec[[ 4]]],
(* req212[en,jxfunc      ] *)
dsreq212[en,jxfunc,truth,truthTS,fragNppN,gammaFrag],ieq212[neginf,grndvec[[ 5]]],
(* req203[en,jxfunc      ] *)
dsreq203[en,jxfunc,truth,truthTS,fragNppN,gammaFrag],ieq203[neginf,grndvec[[ 6]]],
(* req221[en,jxfunc      ] *)

```

```

dsreq221[en,jxfunc,truth,truthTS,fragNppN,gammaFrag],ieq221[neginf,grndvec[[ 7]]],
(* req113[en,jxfunc,truth] *)
dsreq113[en,jxfunc,truth,truthTS],ieq113[neginf,grndvec[[ 8]]],
(* req122[en,jxfunc,truth] *)
dsreq122[en,jxfunc,truth,truthTS],ieq122[neginf,grndvec[[ 9]]],
(* req023[en,jxfunc,truth] *)
dsreq023[en,jxfunc,truth,truthTS],ieq023[neginf,grndvec[[10]]],
req202[en,jxfunc],ieq202[neginf,grndvec[[11]]],
req211[en,jxfunc],ieq211[neginf,grndvec[[12]]],
req220[en,jxfunc],ieq220[neginf,grndvec[[13]]],
req103[en,jxfunc,truth],ieq103[neginf,grndvec[[14]]],
req112[en,jxfunc,truth],ieq112[neginf,grndvec[[15]]],
req121[en,jxfunc,truth],ieq121[neginf,grndvec[[16]]],
req013[en,jxfunc,truth],ieq013[neginf,grndvec[[17]]],
req022[en,jxfunc,truth],ieq022[neginf,grndvec[[18]]],
req201[en,jxfunc],ieq201[neginf,grndvec[[19]]],
req210[en,jxfunc],ieq210[neginf,grndvec[[20]]],
req102[en,jxfunc,truth],ieq102[neginf,grndvec[[21]]],
req111[en,jxfunc,truth],ieq111[neginf,grndvec[[22]]],
req120[en,jxfunc,truth],ieq120[neginf,grndvec[[23]]],
req003[en,jxfunc,truth],ieq003[neginf,grndvec[[24]]],
req012[en,jxfunc,truth],ieq012[neginf,grndvec[[25]]],
req021[en,jxfunc,truth],ieq021[neginf,grndvec[[26]]],
req200[en,jxfunc],ieq200[neginf,grndvec[[27]]],
req101[en,jxfunc,truth],ieq101[neginf,grndvec[[28]]],
req110[en,jxfunc,truth],ieq110[neginf,grndvec[[29]]],
req011[en,jxfunc,truth],ieq011[neginf,grndvec[[30]]],
req020[en,jxfunc,truth],ieq020[neginf,grndvec[[31]]],
req002[en,jxfunc,truth],ieq002[neginf,grndvec[[32]]],
req100[en,jxfunc],ieq100[neginf,grndvec[[33]]],
req010[en,jxfunc,truth],ieq010[neginf,grndvec[[34]]],
req001[en,jxfunc,truth],ieq001[neginf,grndvec[[35]]],
req000[en,jxfunc],ieq000[neginf,grndvec[[36]]] },
{C223k223[t],C213k223[t],C222k223[t],C123k223[t],

```

```

C203k223[t],C212k223[t],C221k223[t],C213k213[t],C213k222[t],C222k222[t],
C113k223[t],C123k213[t],C122k223[t],C123k222[t],
C123k123[t],C023k223[t],
C103k223[t],C112k223[t],C121k223[t],C203k123[t],C212k123[t],C221k123[t],
C023k213[t],C023k222[t],C013k223[t],C022k223[t],C023k123[t],C113k213[t],
C122k213[t],C113k222[t],C122k222[t],C113k123[t],C122k123[t],
P223[t],P213[t],P222[t],P123[t],P212[t],P203[t],P221[t],P113[t],
P122[t],P023[t],P202[t],P211[t],P220[t],P103[t],P112[t],P121[t],
P013[t],P022[t],P201[t],P210[t],P102[t],P111[t],P120[t],P003[t],
P012[t],P021[t],P200[t],P101[t],P110[t],P011[t],P020[t],P002[t],
P100[t],P010[t],P001[t],P000[t]},{t,neginfinity,posinfinity},
MaxStepFraction->maxfrac,MaxSteps->10000]
]

```

## Crater integration of nitrogen molecule

```

dssolveionprofile[pulseenergy_,photonenergy_,tauX_,nintsteps_,nint_,truth_,truthTS_,maxfrac_,
fragNppN_,fragNpNp_,gammaFrag_]:=
Module[{J0Xpeak,J0Xcur,jxcrater,sol},
J0Xpeak=2*Sqrt[Log[2]/Pi]/tauX*peakfluence[pulseenergy,photonenergy];
J0Xcur=J0Xpeak/nintsteps*nint;
jxcrater[t_]:=jxgaussian[J0Xcur,tauX,t];
sol=dsSolveRateEqsParams[photonenergy,jxcrater,truth,truthTS,maxfrac,fragNppN,fragNpNp,gammaFrag];
{J0Xcur,sol}
]

```

```

dssolGroundRem[sol_,t1_]:=((Replace[C223k223[t],sol[[1]]]+
1/2*ReplaceAll[C213k223[t]+C222k223[t]+C123k223[t],sol[[1]]]+
1/2*ReplaceAll[C203k223[t]+C212k223[t]+C221k223[t]+
C113k223[t]+C122k223[t]+C023k223[t],sol[[1]]]+
1/2*ReplaceAll[C112k223[t]+C103k223[t]+C013k223[t]+
C121k223[t]+C022k223[t],sol[[1]]])/.{t->t1})

```

```
dssolSinglyRem[sol_,t1_] := ( (1/2*ReplaceAll[C213k223[t] +
    C222k223[t] + C123k223[t], sol[[1]]] +
    ReplaceAll[C213k213[t] + C213k222[t] + C222k222[t] +
    C123k213[t] + C123k222[t] + C123k123[t], sol[[1]]] +
    1/2*ReplaceAll[C203k123[t] + C212k123[t] + C221k123[t] +
    C122k123[t] + C023k213[t] + C023k222[t] +
    C023k123[t] + C113k213[t] + C113k123[t] +
    C113k222[t] + C122k213[t] + C122k123[t] +
    C122k222[t], sol[[1]]] ) /. {t->t1} )
```

```
dssolDoublyRem[sol_,t1_] := ( (1/2*ReplaceAll[C203k223[t] +
    C212k223[t] + C221k223[t] + C113k223[t] +
    C122k223[t] + C023k223[t], sol[[1]]] +
    1/2*ReplaceAll[C203k123[t] + C212k123[t] + C221k123[t] +
    C023k213[t] + C023k222[t] + C122k213[t] +
    C023k123[t] + C113k123[t] + C113k222[t] +
    C113k213[t] + C122k123[t] + C122k222[t], sol[[1]]] ) /. {t->t1} )
```

```
dssolTriplyRem[sol_,t1_] := ( (1/2*ReplaceAll[C103k223[t] +
    C112k223[t] + C121k223[t] + C013k223[t] +
    C022k223[t], sol[[1]]] ) /. {t->t1} )
```

```
dssolGroundTot[sol_,t1_] := dssolGroundRem[sol,t1] + solGround[sol,t1]
```

```
dssolSinglyTot[sol_,t1_] := dssolSinglyRem[sol,t1] + solSingly[sol,t1]
```

```
dssolDoublyTot[sol_,t1_] := dssolDoublyRem[sol,t1] + solDoubly[sol,t1]
```

```
dssolTriplyTot[sol_,t1_] := dssolTriplyRem[sol,t1] + solTriply[sol,t1]
```

```

dsionyields[sol_] := {dssolGroundTot[sol, posinfinity],
  dssolSinglyTot[sol, posinfinity], dssolDoublyTot[sol, posinfinity],
  dssolTriplyTot[sol, posinfinity],
  solQuadruply[sol, posinfinity], solQuintuply[sol, posinfinity],
  solSextuply[sol, posinfinity], solSeptuply[sol, posinfinity],
  dssolGroundRem[sol, posinfinity], dssolSinglyRem[sol, posinfinity],
  dssolDoublyRem[sol, posinfinity], dssolTriplyRem[sol, posinfinity]}

```

```

dsionprofile[pulseenergy_, photonenergy_, tauX_, nintsteps_, nint_, truth_, truthTS_, maxfrac_,
fragNppN_, fragNpNp_, gammaFrag_] :=
Module[{J0Xcur, sol},
{J0Xcur, sol} = dssolveionprofile[pulseenergy, photonenergy, tauX, nintsteps, nint, truth,
  truthTS, maxfrac, fragNppN, fragNpNp, gammaFrag];
Join[{J0Xcur}, dsionyields[sol]]
]

```

```

dstabionprof[pulseenergy_, photonenergy_, tauX_, nintsteps_, truth_, truthTS_, maxfrac_,
fragNppN_, fragNpNp_, gammaFrag_] := Module[{nint},
Table[
dsionprofile[pulseenergy, photonenergy, tauX, nintsteps, nint, truth, truthTS, maxfrac,
  fragNppN, fragNpNp, gammaFrag],
{nint, nintsteps, 0, -1}]
]

```

```

dsionyielddcrateranalysisparam[pulseenergy_, photoenergy_, pulseduration_, nint_,
inclDCH_, incltsDCH_, maxfrac_, fragNppN_, fragNpNp_, gammaFrag_] := Module[{tabionyi, funionyi, crationyi},
tabionyi = dstabionprof[pulseenergy, photoenergy, pulseduration, nint, inclDCH, incltsDCH, maxfrac,
  fragNppN, fragNpNp, gammaFrag];
funionyi = interpolYields[tabionyi];
crationyi = ionyielddbeam[funionyi, pulseenergy, photoenergy, pulseduration]
]

```

```
dsionyieldcrateranalysis[pulseenergy_,photoenergy_,pulseduration_,nint_,inclDCH_,incltsDCH_] :=
  dsionyieldcrateranalysisparam[pulseenergy,photoenergy,pulseduration,nint,inclDCH,
    incltsDCH,1/1000,fragNppN,fragNpNp,gammaFrag]
```

---

## Private section

```
Begin["`Private`"]
```

---

## Unit conversions

```
BohrToAngstroem:=0.5291772083
AngstroemToBohr:=1/BohrToAngstroem
MicrometerToBohr:=1*^4*AngstroemToBohr
FemtoSecondTot0:=1/24.18884326505*^-3
```

---

## Terminate package

```
End []
```

```
EndPackage []
```

---

## References

- [1] Nina Rohringer, Robin Santra, Phys. Rev. A 76, 033416 (2007), <http://dx.doi.org/10.1103/PhysRevA.76.033416>
- [2] Los Alamos National Laboratory Atomic Physics Codes, <http://aphysics2.lanl.gov/cgi-bin/ION/runlanl08a.pl>
- [3] LCLS Parameter Index for X-RAY-OPTICS / RADIATION-SOURCE, [http://www-ssrl.slac.stanford.edu/htbin/rdbweb/LCLS\\_params\\_DB\\_public](http://www-ssrl.slac.stanford.edu/htbin/rdbweb/LCLS_params_DB_public)
- [4] M. G. Makris, P. Lambropoulos, A. Mihelič, Phys. Rev. Lett. 102, 033002 (2009), <http://dx.doi.org/10.1103/PhysRevLett.102.033002>
- [5] J. L. Campbell, Tibor Papp, Widths of the atomic K–N7 levels, At. Data Nucl. Data Tables 77, 1–56 (2001), <http://dx.doi.org/10.1006/adnd.2000.0848>

- [6] Ryan Coffee, John Bozek, Christian Buth, Marcus Hertlein, Markus Gühr, Nora Berrah, Ali Belkacem, Linda Young, Louis DiMauro, Hamed Merdji, Janos Hajdu, Philip H. Bucksbaum, X-ray multiple ionization of impulsively aligned molecules, Linac Coherent Light Source, Menlo Park, California, USA, 2009, research proposal for the first round of beam time at the Linac Coherent Light Source
- [7] Mau Hsiung Chen, Phys. Rev. A 44, 239-242 (1991), <http://dx.doi.org/10.1103/PhysRevA.44.239>
- [8] Albert C. Thompson et al., X-ray data booklet, Center for X-ray Optics and Advanced Light Source, Lawrence Berkeley National Laboratory, <http://xdb.lbl.gov>
- [9] Christian Buth, Robin Santra, Phys. Rev. A 78, 043409 (2008), <http://dx.doi.org/10.1103/PhysRevA.78.043409>
- [10] W. C. Stolte, Z. X. He, J. N. Cutler, Y. Lu, J. A. R. Samson, At. Data Nucl. Data Tables 69, 171-179 (1998), <http://dx.doi.org/10.1006/adnd.1998.0775>
