# Supplementary material for: Rate equations for nitrogen molecules in ultrashort and intense x-ray pulses
Source: arXiv:1508.05223 ancillary file (2017-03-16)
Supplement: Supplementary file 5 [file nitrogen_channels.pdf]

```
<< Units`  
<< PlotLegends`
```

General::obspkg: PlotLegends` is now obsolete. The legacy version being loaded may conflict with current functionality. See the Compatibility Guide for updating information.

```
Get["NitrogenRateEquations.m", Path -> NotebookDirectory[]]  
Get["NitrogenMoleculeRateEqs.m", Path -> NotebookDirectory[]]
```

```
HartreeToeV := 27.2113845  
eVToHartree := 1 / HartreeToeV  
JouleToHartree := 2.29371269*^17  
MilliJouleToHartree := 1*^-3 * JouleToHartree  
BohrToAngstroem := 0.5291772083  
AngstroemToBohr := 1 / BohrToAngstroem  
MicrometerToBohr := 1*^4 * AngstroemToBohr  
BohrToMicrometer := 1 / MicrometerToBohr  
t0ToSecond := 24.18884326505*^-18  
t0ToFemtoSecond := 24.18884326505*^-3  
crossSectionAUtoBarn := 1*^8 * BohrToAngstroem^2  
crossSectionAUtocm2 := crossSectionAUtoBarn * 1*^-24  
crossSectioncm2toAU := 1 / crossSectionAUtocm2  
  
neginfinity := -1000 / t0ToFemtoSecond  
posinfinity := 10 000 / t0ToFemtoSecond
```

# Impact of SCH, DCHSS, and DCHTS channels on the ion yields from the microscopic molecular rate-equation model

Ji-Cai Liu

Department of Mathematics and Physics, North China Electric Power University, 102206 Beijing, China

Max-Planck-Institut für Kernphysik, Saupfercheckweg 1, 69117 Heidelberg, Germany

Christian Buth

Max-Planck-Institut für Kernphysik, Saupfercheckweg 1, 69117 Heidelberg, Germany

Theoretische Chemie, Physikalisch-Chemisches Institut, Ruprecht-Karls-Universität Heidelberg, Im Neuenheimer Feld 229, 69120 Heidelberg, Germany

25 September 2014

## Experimental parameters

Pulse energy fractions from the nitrogen\_dissociation\_first.nb *Mathematica* Notebook:

```

optdamp280 := 0.38
optdamp80 := 0.30
optdamp7 := 0.16
optdamp4 := 0.23

photonenergy := 1100 * eVToHartree
gamma280 := 4.059357 * gammaFrag
gamma80 := 12.000000 * gammaFrag
optfNppN := 0.26

newMatthias280 := {204.331, 105.281, 27.561, 13.151, 9.881, 0.587, 0.000}
normOleg280 = 1 / Total[newMatthias280] * newMatthias280
{0.56634, 0.291805, 0.0763903, 0.0364504, 0.027387, 0.00162698, 0.}

chrgExpt280 = normOleg280.Table[i, {i, 1, 7}]
1.67162

newMatthias80 := {218.068, 103.774, 26.075, 9.804, 3.315, 0.000, 0.000}
normOleg80 = 1 / Total[newMatthias80] * newMatthias80
{0.604006, 0.287434, 0.0722227, 0.0271552, 0.00918191, 0., 0.}

chrgExpt80 = normOleg80.Table[i, {i, 1, 7}]
1.55007

newMatthias7 := {221.485, 87.888, 9.342, 0.085, 0.000, 0.000, 0.000}
normOleg7 = 1 / Total[newMatthias7] * newMatthias7
{0.694746, 0.275684, 0.0293036, 0.000266625, 0., 0., 0.}

chrgExpt7 = normOleg7.Table[i, {i, 1, 7}]
1.33509

newMatthias4 := {92.985, 36.341, 1.413, 0, 0, 0, 0}
normOleg4 = 1 / Total[newMatthias4] * newMatthias4
{0.711226, 0.277966, 0.0108078, 0., 0., 0., 0.}

chrgExpt4 = normOleg4.Table[i, {i, 1, 7}]
1.29958

```

# Ion yields for 280 fs pulses

## With SCH, DCHTS, and DCHSS

```
optolegiy = dsionyieldcrateranalysisparam[
  optdamp280 * 0.26 * MilliJouleToHartree, photonenergy, 280 / t0ToFemtoSecond,
  nintdata, True, True, 1 / 1000, optfNppN, 1 - optfNppN, gamma280];
optolegiynorm := 1 / Total[optolegiy[[2 ;; 8]]] * optolegiy
charge280DCHSS = optolegiynorm[[2 ;; 8]]
{0.566536, 0.303173, 0.0513661, 0.0558475, 0.0201868, 0.00273103, 0.000159319}
```

```
BarChart[optolegiynorm[[2 ;; 8]], PlotRange → {-0.03, 0.7},
  ChartLabels → {"N+", "N2+", "N3+", "N4+", "N5+", "N6+", "N7+"},
  AxesLabel → {"", "Y( $\omega$ )"},
  AxesStyle → {{Arrowheads[Automatic], AbsoluteThickness[0.6]},
    {Arrowheads[Automatic], AbsoluteThickness[0.6]}},
  LabelStyle → {FontFamily → "Arial"},
  PlotLabel → {optdamp280, gamma280,
    chrgExpt280 - optolegiynorm[[2 ;; 8]].Table[i, {i, 1, 7}]]}
{0.38, 0.0000981912, 0.00281378}
```

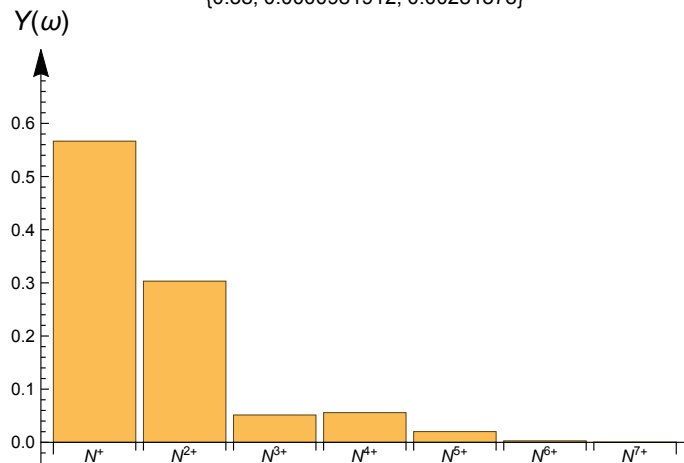

## With SCH and DCHTS

```
optolegiy = dsionyieldcrateranalysisparam[
  optdamp280 * 0.26 * MilliJouleToHartree, photonenergy, 280 / t0ToFemtoSecond,
  nintdata, False, True, 1 / 1000, optfNppN, 1 - optfNppN, gamma280];
optolegiynorm := 1 / Total[optolegiy[[2 ;; 8]]] * optolegiy
charge280DCHTS = optolegiynorm[[2 ;; 8]]
{0.568675, 0.302549, 0.0518706, 0.0552758, 0.0202775, 0.00124507, 0.000107096}
```

```

BarChart[optolegiynorm[[2 ;; 8]], PlotRange → {-0.03, 0.7},
  ChartLabels → {"N+", "N2+", "N3+", "N4+", "N5+", "N6+", "N7+"},
  AxesLabel → {"", "Y( $\omega$ )"},
  AxesStyle → {{Arrowheads[Automatic], AbsoluteThickness[0.6]},
    {Arrowheads[Automatic], AbsoluteThickness[0.6]}},
  LabelStyle → {FontFamily → "Arial"},
  PlotLabel → {optdamp280, gamma280,
    chrgExpt280 - optolegiynorm[[2 ;; 8]].Table[i, {i, 1, 7}]]]
{0.38, 0.0000981912, 0.011524}

```

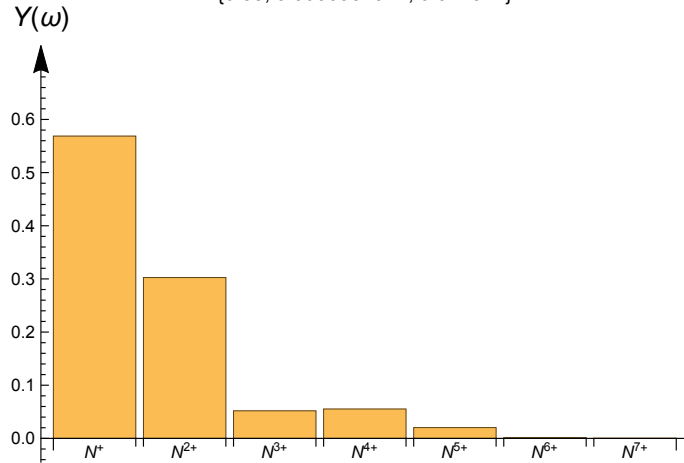

## With SCH

```

optolegiy = dsionyieldcrateranalysisparam[
  optdamp280 * 0.26 * MilliJouleToHartree, photonenergy, 280 / t0ToFemtoSecond,
  nintdata, False, False, 1 / 1000, optfNppN, 1 - optfNppN, gamma280];
optolegiynorm := 1 / Total[optolegiy[[2 ;; 8]]] * optolegiy
charge280SCH = optolegiynorm[[2 ;; 8]]
{0.572285, 0.302731, 0.0493992, 0.0550002, 0.0193671, 0.00112198, 0.0000954873}

```

```
BarChart[optolegiynorm[[2 ;; 8]], PlotRange → {-0.03, 0.7},
  ChartLabels → {"N+", "N2+", "N3+", "N4+", "N5+", "N6+", "N7+"},
  AxesLabel → {"", "Y( $\omega$ )"},
  AxesStyle → {{Arrowheads[Automatic], AbsoluteThickness[0.6]},
    {Arrowheads[Automatic], AbsoluteThickness[0.6]}},
  LabelStyle → {FontFamily → "Arial"},
  PlotLabel → {optdamp280, gamma280,
    chrgExpt280 - optolegiynorm[[2 ;; 8]].Table[i, {i, 1, 7}]]]
{0.38, 0.0000981912, 0.0214388}
```

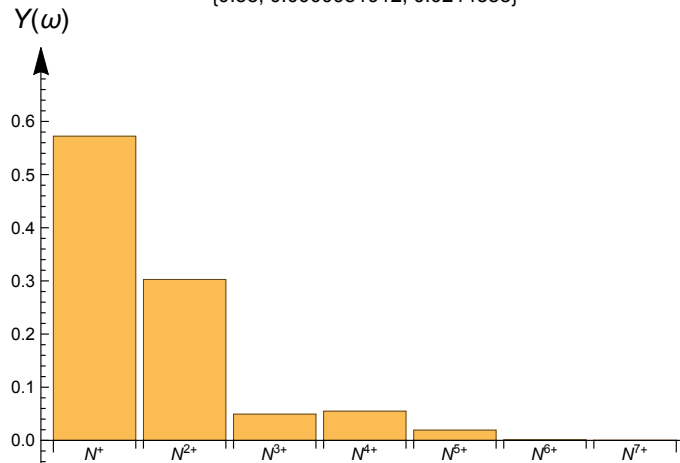

## Ion yields for 80 fs pulses

With SCH, DCHTS, and DCHSS

```
optolegiy = dsionyieldcrateranalysisparam[
  optdamp80 * 0.26 * MilliJouleToHartree, photonenergy, 80 / t0ToFemtoSecond,
  nintdata, True, True, 1 / 1000, optfNppN, 1 - optfNppN, gamma80];
optolegiynorm := 1 / Total[optolegiy[[2 ;; 8]]] * optolegiy
charge80DCHSS = optolegiynorm[[2 ;; 8]]
{0.604055, 0.303034, 0.041838, 0.0388149, 0.0111715, 0.00104697, 0.0000391357}
```

```
BarChart[optolegiynorm[[2 ;; 8]], PlotRange → {-0.03, 0.7},
  ChartLabels → {"N+", "N2+", "N3+", "N4+", "N5+", "N6+", "N7+"},
  AxesLabel → {"", "Y( $\omega$ )"},
  AxesStyle → {{Arrowheads[Automatic], AbsoluteThickness[0.6]},
    {Arrowheads[Automatic], AbsoluteThickness[0.6]}},
  LabelStyle → {FontFamily → "Arial"},
  PlotLabel → {optdamp80, gamma80,
    chrgExpt80 - optolegiynorm[[2 ;; 8]].Table[i, {i, 1, 7}]]]
{0.3, 0.000290266, -0.00323831}
```

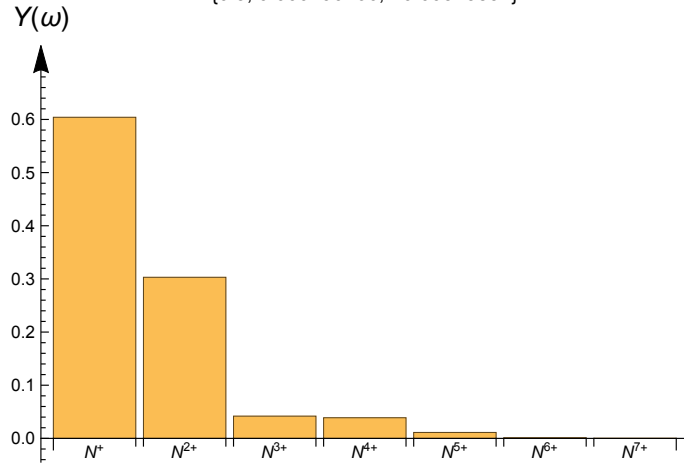

## With SCH and DCHTS

```
optolegiy = dsionyieldcrateranalysisparam[
  optdamp80 * 0.26 * MilliJouleToHartree, photonenergy, 80 / t0ToFemtoSecond,
  nintdata, False, True, 1 / 1000, optfNppN, 1 - optfNppN, gamma80];
optolegiynorm := 1 / Total[optolegiy[[2 ;; 8]]] * optolegiy
charge80DCHTS = optolegiynorm[[2 ;; 8]]
{0.61089, 0.300302, 0.0424288, 0.0366919, 0.00938077, 0.000290548, 0.0000161196}
```

```
BarChart[optolegiynorm[[2 ;; 8]], PlotRange → {-0.03, 0.7},
  ChartLabels → {"N+", "N2+", "N3+", "N4+", "N5+", "N6+", "N7+"},
  AxesLabel → {"", "Y( $\omega$ )"},
  AxesStyle → {{Arrowheads[Automatic], AbsoluteThickness[0.6]},
    {Arrowheads[Automatic], AbsoluteThickness[0.6]}},
  LabelStyle → {FontFamily → "Arial"},
  PlotLabel → {optdamp80, gamma80,
    chrgExpt80 - optolegiynorm[[2 ;; 8]].Table[i, {i, 1, 7}]]
    {0.3, 0.000290266, 0.0157652}
```

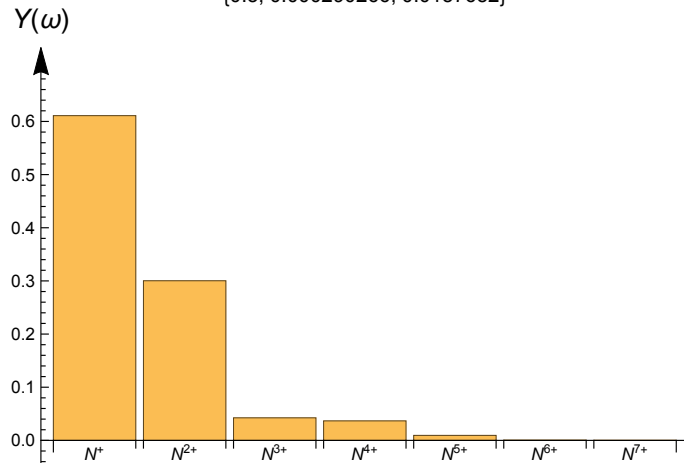

## With SCH

```
optolegiy = dsionyieldcrateranalysisparam[
  optdamp80 * 0.26 * MilliJouleToHartree, photonenergy, 80 / t0ToFemtoSecond,
  nintdata, False, False, 1 / 1000, optfNppN, 1 - optfNppN, gamma80];
optolegiynorm := 1 / Total[optolegiy[[2 ;; 8]]] * optolegiy
charge80SCH = optolegiynorm[[2 ;; 8]]
{0.622836, 0.297758, 0.0360299, 0.0352459, 0.0079003, 0.000218594, 0.0000120275}
```

```
BarChart[optolegiynorm[[2 ;; 8]], PlotRange → {-0.03, 0.7},
  ChartLabels → {"N+", "N2+", "N3+", "N4+", "N5+", "N6+", "N7+"},
  AxesLabel → {"", "Y( $\omega$ )"},
  AxesStyle → {{Arrowheads[Automatic], AbsoluteThickness[0.6]},
    {Arrowheads[Automatic], AbsoluteThickness[0.6]}},
  LabelStyle → {FontFamily → "Arial"},
  PlotLabel → {optdamp80, gamma80,
    chrgExpt80 - optolegiynorm[[2 ;; 8]].Table[i, {i, 1, 7}]]]
{0.3, 0.000290266, 0.0417511}
```

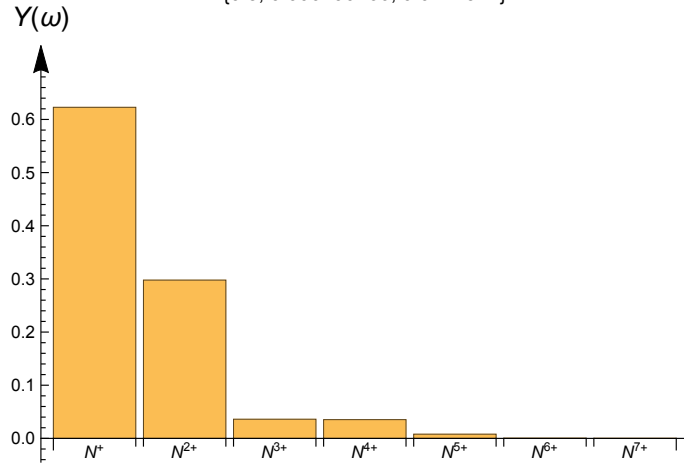

## Ion yields for 7 fs pulses

### With SCH, DCHTS, and DCHSS

```
optolegiy = dsionyieldcrateranalysisparam[
  optdamp7 * 0.26 * MilliJouleToHartree, photonenergy, 7 / t0ToFemtoSecond,
  nintdata, True, True, 1 / 1000, optfNppN, 1 - optfNppN, gamma280];
optolegiynorm := 1 / Total[optolegiy[[2 ;; 8]]] * optolegiy
charge7DCHSS = optolegiynorm[[2 ;; 8]]
{0.693304, 0.284637, 0.0148165,
  0.00627051, 0.000952154, 0.0000198823, 8.76372 × 10-8}
```



```
BarChart[optolegiynorm[[2 ;; 8]], PlotRange → {-0.03, 0.7},
  ChartLabels → {"N+", "N2+", "N3+", "N4+", "N5+", "N6+", "N7+"},
  AxesLabel → {"", "Y( $\omega$ )"},
  AxesStyle → {{Arrowheads[Automatic], AbsoluteThickness[0.6]},
    {Arrowheads[Automatic], AbsoluteThickness[0.6]}},
  LabelStyle → {FontFamily → "Arial"},
  PlotLabel → {optdamp7, gamma280,
    chrgExpt7 - optolegiynorm[[2 ;; 8]].Table[i, {i, 1, 7}]]}
{0.16, 0.0000981912, -0.00189949}
```

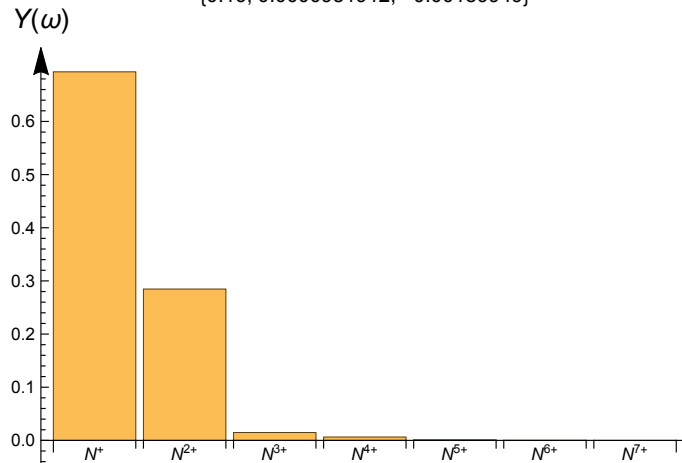

## With SCH and DCHTS

```
optolegiy = dsionyieldcrateranalysisparam[
  optdamp7 * 0.26 * MilliJouleToHartree, photonenergy, 7 / t0ToFemtoSecond,
  nintdata, False, True, 1 / 1000, optfNppN, 1 - optfNppN, gamma280];
optolegiynorm := 1 / Total[optolegiy[[2 ;; 8]]] * optolegiy
charge7DCHTS = optolegiynorm[[2 ;; 8]]
{0.723364, 0.265147, 0.00883498,
  0.00250004, 0.000154465, 3.49015 × 10-7, 7.12571 × 10-9}
```

```
BarChart[optolegiynorm[[2 ;; 8]], PlotRange → {-0.03, 0.7},
  ChartLabels → {"N+", "N2+", "N3+", "N4+", "N5+", "N6+", "N7+"},
  AxesLabel → {"", "Y( $\omega$ )"},
  AxesStyle → {{Arrowheads[Automatic], AbsoluteThickness[0.6]},
    {Arrowheads[Automatic], AbsoluteThickness[0.6]}},
  LabelStyle → {FontFamily → "Arial"},
  PlotLabel → {optdamp7, gamma280,
    chrgExpt7 - optolegiynorm[[2 ;; 8]].Table[i, {i, 1, 7}]]}
{0.16, 0.0000981912, 0.0441546}
```

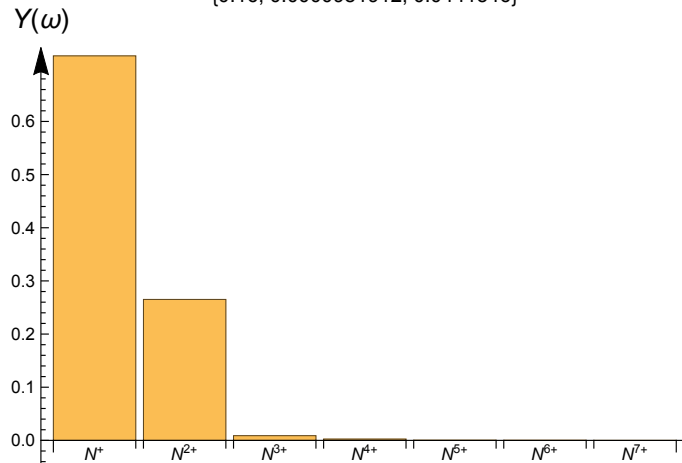

## With SCH

```
optolegiy = dsionyieldcrateranalysisparam[
  optdamp7 * 0.26 * MilliJouleToHartree, photonenergy, 7 / t0ToFemtoSecond,
  nintdata, False, False, 1 / 1000, optfNppN, 1 - optfNppN, gamma280];
optolegiynorm := 1 / Total[optolegiy[[2 ;; 8]]] * optolegiy
charge7SCH = optolegiynorm[[2 ;; 8]]
{0.780476, 0.216798, 0.000988124,
  0.00170402, 0.0000333979, 6.53004 × 10-8, 1.45946 × 10-9}
```

```
BarChart[optolegiynorm[[2 ;; 8]], PlotRange → {-0.03, 0.7},
  ChartLabels → {"N+", "N2+", "N3+", "N4+", "N5+", "N6+", "N7+"},
  AxesLabel → {"", "Y( $\omega$ )"},
  AxesStyle → {{Arrowheads[Automatic], AbsoluteThickness[0.6]},
    {Arrowheads[Automatic], AbsoluteThickness[0.6]}},
  LabelStyle → {FontFamily → "Arial"},
  PlotLabel → {optdamp7, gamma280,
    chrgExpt7 - optolegiynorm[[2 ;; 8]].Table[i, {i, 1, 7}]]]
{0.16, 0.0000981912, 0.11107}
```

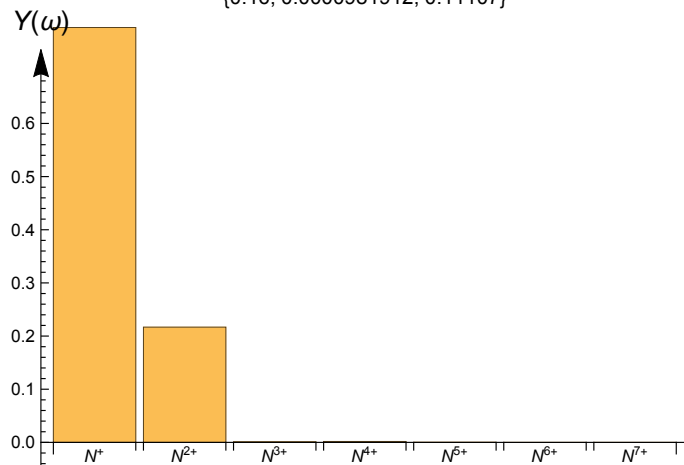

## Ion yields for 4 fs pulses

With SCH, DCHTS, and DCHSS

```
optolegiy = dsionyieldcrateranalysisparam[
  optdamp4 * 0.15 * MilliJouleToHartree, photonenergy, 4 / t0ToFemtoSecond,
  nintdata, True, True, 1 / 1000, optfNppN, 1 - optfNppN, gamma280];
optolegiynorm := 1 / Total[optolegiy[[2 ;; 8]]] * optolegiy
charge4DCHSS = optolegiynorm[[2 ;; 8]]
{0.719423, 0.265424, 0.0112227,
  0.00350494, 0.000420993, 4.84993 × 10-6, 1.04705 × 10-8}
```

```

BarChart[optolegiynorm[[2 ;; 8]], PlotRange → {-0.08, 0.8},
  ChartLabels → {"N+", "N2+", "N3+", "N4+", "N5+", "N6+", "N7+"},
  AxesLabel → {"", "Y( $\omega$ )"},
  AxesStyle → {{Arrowheads[Automatic], AbsoluteThickness[0.6]},
    {Arrowheads[Automatic], AbsoluteThickness[0.6]}},
  LabelStyle → {FontFamily → "Arial"},
  PlotLabel → {optdamp4, gamma280,
    chrgExpt4 - optolegiynorm[[2 ;; 8]].Table[i, {i, 1, 7}]]]

```

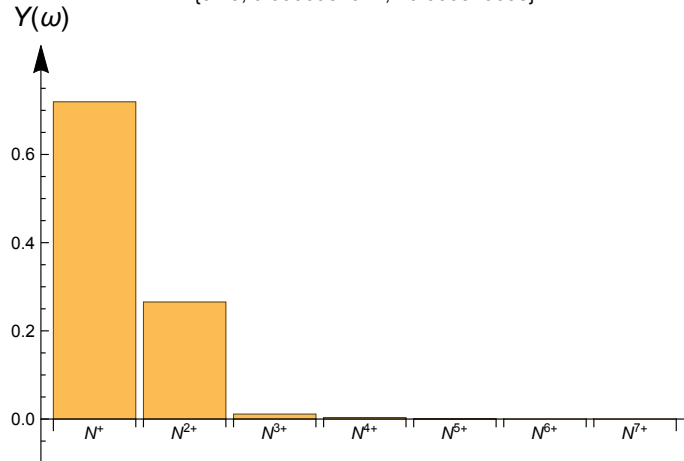

## With SCH and DCHTS

```

optolegiy = dsionyieldcrateranalysisparam[
  optdamp4 * 0.15 * MilliJouleToHartree, photonenergy, 4 / t0ToFemtoSecond,
  nintdata, False, True, 1 / 1000, optfNppN, 1 - optfNppN, gamma280];
optolegiynorm := 1 / Total[optolegiy[[2 ;; 8]]] * optolegiy
charge4DCHTS = optolegiynorm[[2 ;; 8]]

```

{0.750955, 0.242994, 0.00516319,  
0.00084948, 0.0000383766,  $4.19921 \times 10^{-8}$ ,  $6.88184 \times 10^{-10}$ }

```
BarChart[optolegiynorm[[2 ;; 8]], PlotRange → {-0.08, 0.8},
  ChartLabels → {"N+", "N2+", "N3+", "N4+", "N5+", "N6+", "N7+"},
  AxesLabel → {"", "Y( $\omega$ )"},
  AxesStyle → {{Arrowheads[Automatic], AbsoluteThickness[0.6]},
    {Arrowheads[Automatic], AbsoluteThickness[0.6]}},
  LabelStyle → {FontFamily → "Arial"},
  PlotLabel → {optdamp4, gamma280,
    chrgExpt4 - optolegiynorm[[2 ;; 8]].Table[i, {i, 1, 7}]]]
{0.23, 0.0000981912, 0.043559}
```

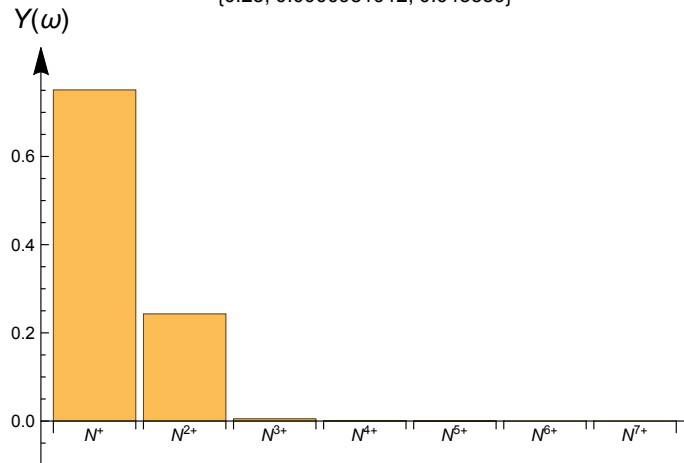

## With SCH

```
optolegiy = dsionyieldcrateranalysisparam[
  optdamp4 * 0.15 * MilliJouleToHartree, photonenergy, 4 / t0ToFemtoSecond,
  nintdata, False, False, 1 / 1000, optfNppN, 1 - optfNppN, gamma280];
optolegiynorm := 1 / Total[optolegiy[[2 ;; 8]]] * optolegiy
charge4SCH = optolegiynorm[[2 ;; 8]]
{0.810306, 0.188713, 0.000417863,
  0.000556606, 6.86875 × 10-6, 7.59625 × 10-9, 1.39609 × 10-10}
```

```
BarChart[optolegiynorm[2 ;; 8], PlotRange → {-0.08, 0.8},
  ChartLabels → {"N+", "N2+", "N3+", "N4+", "N5+", "N6+", "N7+"},
  AxesLabel → {"", "Y( $\omega$ )"},
  AxesStyle → {{Arrowheads[Automatic], AbsoluteThickness[0.6]},
    {Arrowheads[Automatic], AbsoluteThickness[0.6]}},
  LabelStyle → {FontFamily → "Arial"},
  PlotLabel → {optdamp4, gamma280,
    chrgExpt4 - optolegiynorm[2 ;; 8].Table[i, {i, 1, 7}]}]
{0.23, 0.0000981912, 0.108336}
```

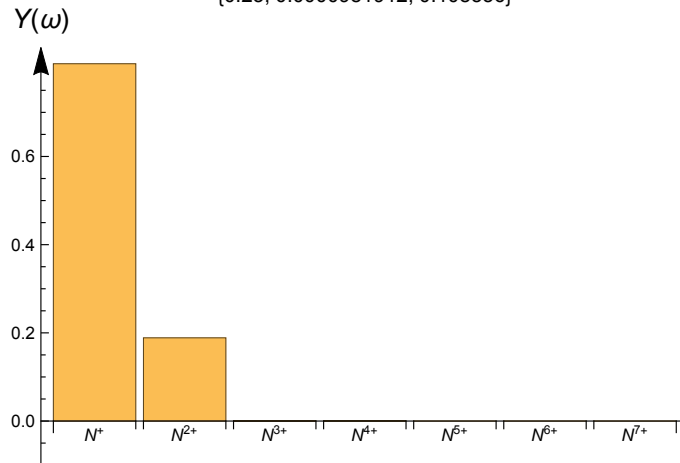

## Presentation of results

### 280 fs pulses

```
charge280 := {{normOleg280[[1]],
  charge280DCHSS[[1]], charge280DCHTS[[1]], charge280SCH[[1]]},
{normOleg280[[2]], charge280DCHSS[[2]], charge280DCHTS[[2]],
  charge280SCH[[2]]}, {normOleg280[[3]], charge280DCHSS[[3]],
  charge280DCHTS[[3]], charge280SCH[[3]]}, {normOleg280[[4]],
  charge280DCHSS[[4]], charge280DCHTS[[4]], charge280SCH[[4]]},
{normOleg280[[5]], charge280DCHSS[[5]], charge280DCHTS[[5]],
  charge280SCH[[5]]}, {normOleg280[[6]], charge280DCHSS[[6]],
  charge280DCHTS[[6]], charge280SCH[[6]]}, {normOleg280[[7]],
  charge280DCHSS[[7]], charge280DCHTS[[7]], charge280SCH[[7]]}}
```

```
BarChart[charge280, PlotRange → {-0.08, 1.0},
  ChartLabels → {Placed[{"N+", "N2+", "N3+", "N4+", "N5+", "N6+", "N7+"}, Below],
    Placed[{}, Above]},
  ChartLegends → Placed[{"Expt.", "All", "No ssDCH", "Only SCH"}, Top],
  ChartStyle → {Black, Red, Green, Blue}, AxesLabel → {"", " $\tilde{Y}$ "},
  AxesStyle → {{Arrowheads[Automatic], AbsoluteThickness[0.6]},
    {Arrowheads[Automatic], AbsoluteThickness[0.6]}},
  LabelStyle → {FontFamily → "Arial", FontSize → 18, FontSlant → Plain}]
```

■ Expt. ■ All ■ No ssDCH ■ Only SCH

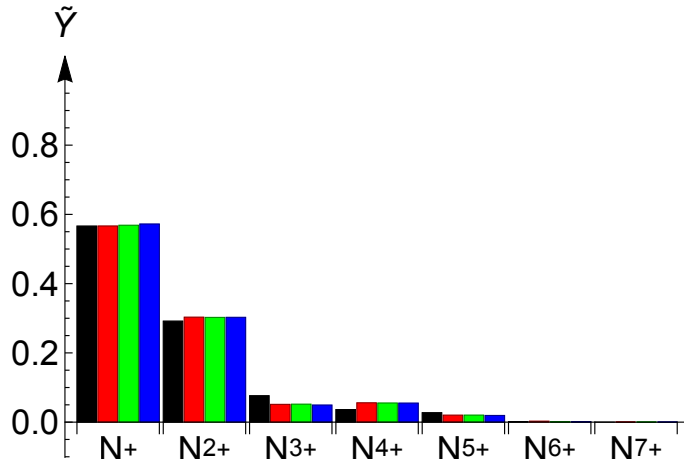

## 80 fs pulses

```
charge80 =
  {{normOleg80[[1]], charge80DCHSS[[1]], charge80DCHTS[[1]], charge80SCH[[1]]},
  {normOleg80[[2]], charge80DCHSS[[2]], charge80DCHTS[[2]], charge80SCH[[2]]},
  {normOleg80[[3]], charge80DCHSS[[3]], charge80DCHTS[[3]], charge80SCH[[3]]},
  {normOleg80[[4]], charge80DCHSS[[4]], charge80DCHTS[[4]], charge80SCH[[4]]},
  {normOleg80[[5]], charge80DCHSS[[5]], charge80DCHTS[[5]], charge80SCH[[5]]},
  {normOleg80[[6]], charge80DCHSS[[6]], charge80DCHTS[[6]], charge80SCH[[6]]},
  {normOleg80[[7]], charge80DCHSS[[7]], charge80DCHTS[[7]], charge80SCH[[7]]}};
```

```
BarChart[charge80, PlotRange → {-0.08, 1.0},
  ChartLabels → {Placed[{"N+", "N2+", "N3+", "N4+", "N5+", "N6+", "N7+"}, Below],
    Placed[{}, Above]},
  ChartLegends → Placed[{"Expt.", "All", "No ssDCH", "Only SCH"}, Top],
  ChartStyle → {Black, Red, Green, Blue}, AxesLabel → {"", " $\tilde{Y}$ "},
  AxesStyle → {{Arrowheads[Automatic], AbsoluteThickness[0.6]},
    {Arrowheads[Automatic], AbsoluteThickness[0.6]}},
  LabelStyle → {FontFamily → "Arial", FontSize → 18, FontSlant → Plain}]
```

■ Expt. ■ All ■ No ssDCH ■ Only SCH

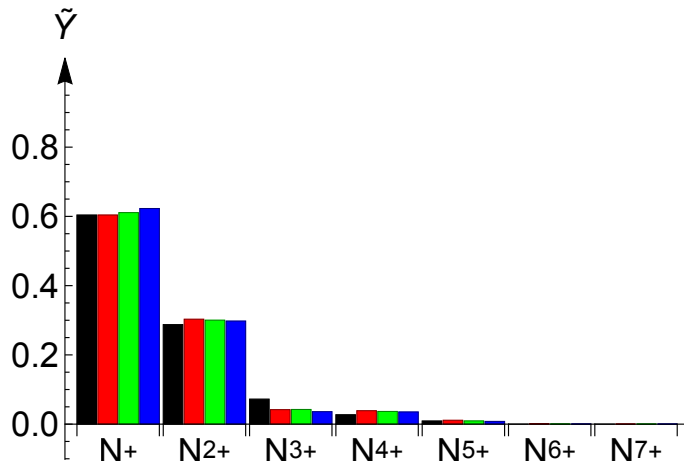

## 7 fs pulses

```
charge7 :=
  {normOleg7[[1]], charge7DCHSS[[1]], charge7DCHTS[[1]], charge7SCH[[1]]},
  {normOleg7[[2]], charge7DCHSS[[2]], charge7DCHTS[[2]], charge7SCH[[2]]},
  {normOleg7[[3]], charge7DCHSS[[3]], charge7DCHTS[[3]], charge7SCH[[3]]},
  {normOleg7[[4]], charge7DCHSS[[4]], charge7DCHTS[[4]], charge7SCH[[4]]},
  {normOleg7[[5]], charge7DCHSS[[5]], charge7DCHTS[[5]], charge7SCH[[5]]},
  {normOleg7[[6]], charge7DCHSS[[6]], charge7DCHTS[[6]], charge7SCH[[6]]},
  {normOleg7[[7]], charge7DCHSS[[7]], charge7DCHTS[[7]], charge7SCH[[7]]}
```



```
BarChart[charge7, PlotRange → {-0.08, 1.0},
  ChartLabels → {Placed[{"N+", "N2+", "N3+", "N4+", "N5+", "N6+", "N7+"}, Below],
    Placed[{}, Above]},
  ChartLegends → Placed[{"Expt.", "All", "No ssDCH", "Only SCH"}, Top],
  ChartStyle → {Black, Red, Green, Blue}, AxesLabel → {"", " $\tilde{Y}$ "},
  AxesStyle → {{Arrowheads[Automatic], AbsoluteThickness[0.6]},
    {Arrowheads[Automatic], AbsoluteThickness[0.6]}},
  LabelStyle → {FontFamily → "Arial", FontSize → 18, FontSlant → Plain}]
```

■ Expt. ■ All ■ No ssDCH ■ Only SCH

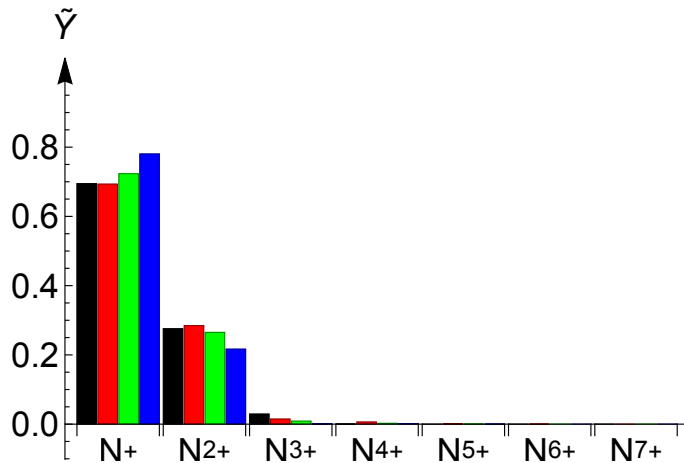

## 4 fs pulses

```
charge4 :=
  {normOleg4[[1]], charge4DCHSS[[1]], charge4DCHTS[[1]], charge4SCH[[1]]},
  {normOleg4[[2]], charge4DCHSS[[2]], charge4DCHTS[[2]], charge4SCH[[2]]},
  {normOleg4[[3]], charge4DCHSS[[3]], charge4DCHTS[[3]], charge4SCH[[3]]},
  {normOleg4[[4]], charge4DCHSS[[4]], charge4DCHTS[[4]], charge4SCH[[4]]},
  {normOleg4[[5]], charge4DCHSS[[5]], charge4DCHTS[[5]], charge4SCH[[5]]},
  {normOleg4[[6]], charge4DCHSS[[6]], charge4DCHTS[[6]], charge4SCH[[6]]},
  {normOleg4[[7]], charge4DCHSS[[7]], charge4DCHTS[[7]], charge4SCH[[7]]}
```

```
BarChart[charge4, PlotRange → {-0.08, 1.0},
  ChartLabels → {Placed[{"N+", "N2+", "N3+", "N4+", "N5+", "N6+", "N7+"}, Below],
    Placed[{}, Above]},
  ChartLegends → Placed[{"Expt.", "All", "No ssDCH", "Only SCH"}, Top],
  ChartStyle → {Black, Red, Green, Blue}, AxesLabel → {"", " $\tilde{Y}$ "},
  AxesStyle → {{Arrowheads[Automatic], AbsoluteThickness[0.6]},
    {Arrowheads[Automatic], AbsoluteThickness[0.6]}},
  LabelStyle → {FontFamily → "Arial", FontSize → 18, FontSlant → Plain}]
```

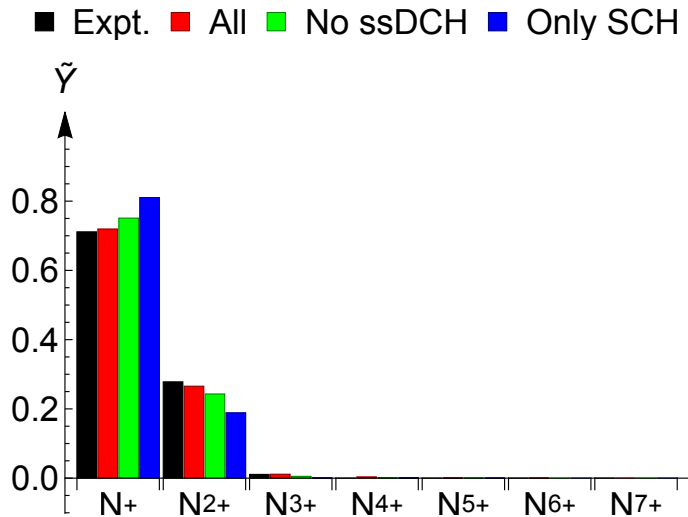

## References

[1] M. Hoener, L. Fang, O. Kornilov, O. Gessner, S. T. Pratt, M. Gühr, E. P. Kanter, C. Blaga, C. Bostedt, J. D. Bozek, P. H. Bucksbaum, C. Buth, M. Chen, R. Coffee, J. Cryan, L. DiMauro, M. Glownia, E. Hosler, E. Kukk, S. R. Leone, B. McFarland, M. Messerschmidt, B. Murphy, V. Petrovic, D. Rolles, and N. Berrah, Phys. Rev. Lett. **104**, 253002 (2010) [5 pages], <http://dx.doi.org/10.1103/PhysRevLett.104.253002>.
