# Supplementary material for: Rate equations for nitrogen molecules in ultrashort and intense x-ray pulses
Source: arXiv:1508.05223 ancillary file (2017-03-16)
Supplement: Supplementary file 6 [file nitrogen_dissociation_first.pdf]

```
<< PlotLegends`
```

General::obspkg: PlotLegends` is now obsolete. The legacy version being loaded may conflict with current functionality. See the Compatibility Guide for updating information.

```
Get["NitrogenRateEquations.m", Path -> NotebookDirectory[]]  
Get["NitrogenMoleculeRateEqs.m", Path -> NotebookDirectory[]]
```

```
HartreeToeV := 27.2113845  
eVToHartree := 1 / HartreeToeV  
JouleToHartree := 2.29371269*^17  
MilliJouleToHartree := 1*^-3 * JouleToHartree  
BohrToAngstroem := 0.5291772083  
AngstroemToBohr := 1 / BohrToAngstroem  
MicrometerToBohr := 1*^4 * AngstroemToBohr  
BohrToMicrometer := 1 / MicrometerToBohr  
t0ToSecond := 24.18884326505*^-18  
t0ToFemtoSecond := 24.18884326505*^-3  
crossSectionAUtoBarn := 1*^8 * BohrToAngstroem^2  
crossSectionAUtocm2 := crossSectionAUtoBarn * 1*^-24  
crossSectioncm2toAU := 1 / crossSectionAUtocm2  
  
neginfinity := -1000 / t0ToFemtoSecond  
posinfinity := 10 000 / t0ToFemtoSecond
```

# Fragmentation time and pulse energy

Microscopic molecular rate-equation model with nominal pulse duration and optimization for the N<sup>+</sup> yields

Christian Buth, 27 September 2014

Theoretische Chemie, Physikalisch-Chemisches Institut, Ruprecht-Karls-Universität Heidelberg, Im Neuenheimer Feld 229, 69120 Heidelberg, Germany

---

## Experimental parameters

Pulse energy fractions as determined in this *Mathematica* Notebook:

```
optdamp280 := 0.38  
optdamp80 := 0.30  
optdamp7 := 0.16  
optdamp4 := 0.23
```

Pulse energy fraction for the 4 fs pulse with respect to a pulse energy of 0.26 mJ instead of 0.15 mJ and vice versa for the 7 fs pulse:

```
optdamp4 * 0.15 / 0.26  
0.132692  
  
optdamp7 * 0.26 / 0.15  
0.277333
```

Pulse duration fractions. See Ref. [1] for measurements of LCLS pulse durations:

```
280 / 300 * 120
```

```
112
```

```
shtdur280 = 112 / 280.0
```

```
0.4
```

```
shtdur80 = 40 / 80.0
```

```
0.5
```

```
shtdur7 := 0.4
```

```
shtdur4 := 0.4
```

```
photonenergy := 1100 * eVToHartree
```

```
optfNppN := 0.26
```

```
newMatthias280 := {204.331, 105.281, 27.561, 13.151, 9.881, 0.587, 0.000}
```

```
normOleg280 = 1 / Total[newMatthias280] * newMatthias280
```

```
{0.56634, 0.291805, 0.0763903, 0.0364504, 0.027387, 0.00162698, 0.}
```

```
newMatthias80 := {218.068, 103.774, 26.075, 9.804, 3.315, 0.000, 0.000}
```

```
normOleg80 = 1 / Total[newMatthias80] * newMatthias80
```

```
{0.604006, 0.287434, 0.0722227, 0.0271552, 0.00918191, 0., 0.}
```

```
newMatthias7 := {221.485, 87.888, 9.342, 0.085, 0.000, 0.000, 0.000}
```

```
normOleg7 = 1 / Total[newMatthias7] * newMatthias7
```

```
{0.694746, 0.275684, 0.0293036, 0.000266625, 0., 0., 0.}
```

```
newMatthias4 := {92.985, 36.341, 1.413, 0, 0, 0, 0}
```

```
normOleg4 = 1 / Total[newMatthias4] * newMatthias4
```

```
{0.711226, 0.277966, 0.0108078, 0., 0., 0., 0.}
```

---

## Molecular fragmentation rate and pulse energy for a 280 fs pulse

```
tauX := 280 / t0ToFemtoSecond
```

```
normfitconsts[damp_?NumericQ, gaFra_?NumericQ] := Module[{olegiy, olegiynorm},
  olegiy =
    dsionyieldcrateranalysisparam[damp * 0.26 * MilliJouleToHartree, photonenergy,
      tauX, nintdata, True, True, 1 / 1000, optfNppN, 1 - optfNppN, gaFra];
  olegiynorm = 1 / Total[olegiy[[2 ;; 8]]] * olegiy[[2 ;; 8]];
  Norm[(olegiynorm - normOleg280) * Table[{i, {i, 1, 7}}, 1] +
    16 * Abs[olegiynorm[[1]] - normOleg280[[1]]]
]
```

### 0.36

```
damp := 0.36
```

```

tabgamma =
  Table[{gaFra, normfitconsts[damp, gaFra * gammaFrag]}, {gaFra, 1, 10, 1 / 2}];

ListPlot[tabgamma, Joined -> True,
  PlotMarkers -> Automatic, PlotStyle -> {Thick, Red}]

```

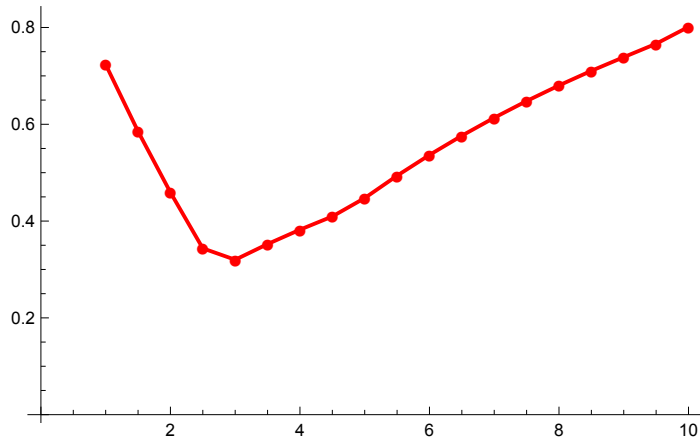

```

tabgamma =
  Table[{gaFra, normfitconsts[damp, gaFra * gammaFrag]}, {gaFra, 2, 4, 1 / 5}];

ListPlot[tabgamma, Joined -> True,
  PlotMarkers -> Automatic, PlotStyle -> {Thick, Red}]

```

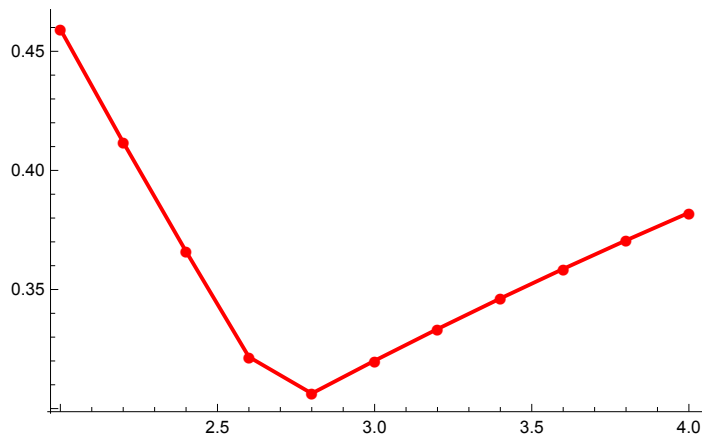

```

N[MinimalBy[tabgamma, Last]]
{{2.8, 0.306348}}

```

```

intgamma = Interpolation[tabgamma, x]

```

InterpolatingFunction[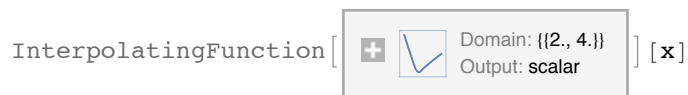 Domain: {{2., 4.}}  
Output: scalar][x]

```

mingamma = FindMinimum[intgamma, {x, 2.0, 4.0}]

```

InterpolatingFunction::dmval:

Input value {4.26425} lies outside the range of data in the interpolating function. Extrapolation will be used. >>

```

{0.306348, {x -> 2.8}}

```

```

optent = x /. mingamma[[2]]

```

```

2.8

```

```

optGaFra := optent * gammaFrag

iy = dsionyieldcrateranalysisparam[damp * 0.26 * MilliJouleToHartree, photonenergy,
  tauX, nintdata, True, True, 1 / 1000, optfNppN, 1 - optfNppN, optGaFra]
iynorm = 1 / Total[iy[[2 ;; 8]]] * iy
Total[iynorm[[2 ;; 8]]]

{0.963376, 0.020771, 0.0117167, 0.00146248, 0.00197862, 0.000613989, 0.000076855,
  3.93328 × 10-6, 0.959919, 0.000628798, 9.39488 × 10-15, -1.7828 × 10-108}

{26.3048, 0.567149, 0.319922, 0.0399327, 0.0540259, 0.0167649, 0.00209851,
  0.000107398, 26.2104, 0.0171692, 2.56526 × 10-13, -4.86792 × 10-107}

1.

plotiy = Partition[Riffle[normOleg280, iynorm[[2 ;; 8]]], 2]
{{0.56634, 0.567149}, {0.291805, 0.319922},
 {0.0763903, 0.0399327}, {0.0364504, 0.0540259},
 {0.027387, 0.0167649}, {0.00162698, 0.00209851}, {0., 0.000107398}}

BarChart[plotiy, PlotRange → {-0.1, 0.9},
  ChartLabels → {Placed[{"N+", "N2+", "N3+", "N4+", "N5+", "N6+", "N7+"}, Below],
    Placed[{}, Above]},
  ChartLegends → Placed[{"Expt.", "γfrag"}, Top],
  ChartStyle → {Black, Red}, AxesLabel → {"", "Ỹ(ω)"},
  AxesStyle → {{Arrowheads[Automatic], AbsoluteThickness[0.6]},
    {Arrowheads[Automatic], AbsoluteThickness[0.6]}},
  LabelStyle → {FontFamily → "Arial"},
  PlotLabel → {damp, optGaFra / gammaFrag,
    (iynorm[[2 ;; 8]] - normOleg280).Table[i, {i, 1, 7}]]}

■ Expt. ■ γfrag
{0.36, 2.8, -0.0315585}

```

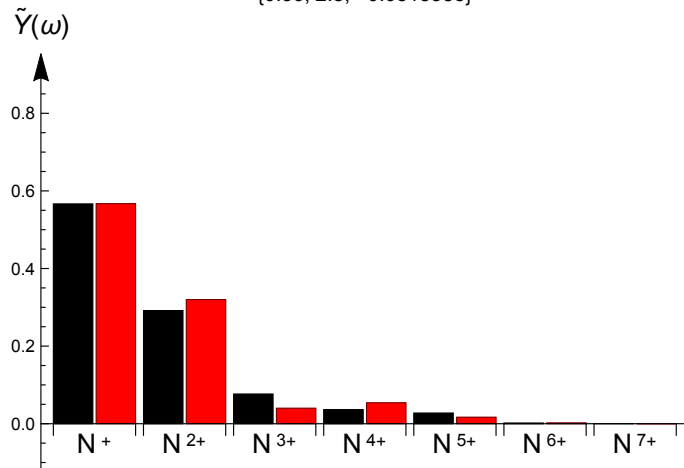

### 0.37

```

damp := 0.37

tabgamma =
  Table[{gaFra, normfitconsts[damp, gaFra * gammaFrag]}, {gaFra, 1, 10, 1 / 2}];

```

```
ListPlot[tabgamma, Joined -> True,
  PlotMarkers -> Automatic, PlotStyle -> {Thick, Red}]
```

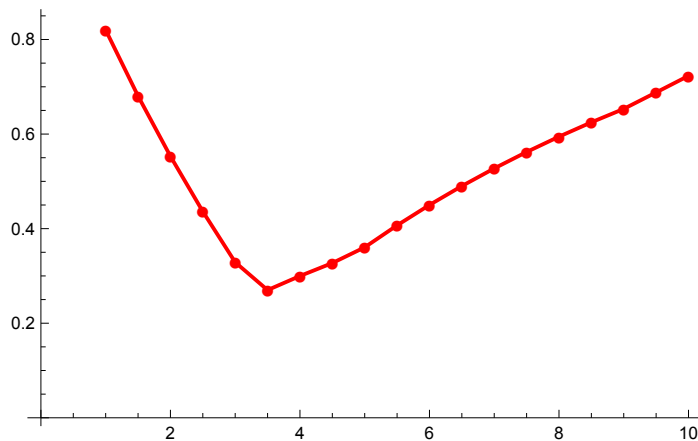

```
tabgamma =
  Table[{gaFra, normfitconsts[damp, gaFra * gammaFrag]}, {gaFra, 2, 4, 1/5}];
```

```
ListPlot[tabgamma, Joined -> True,
  PlotMarkers -> Automatic, PlotStyle -> {Thick, Red}]
```

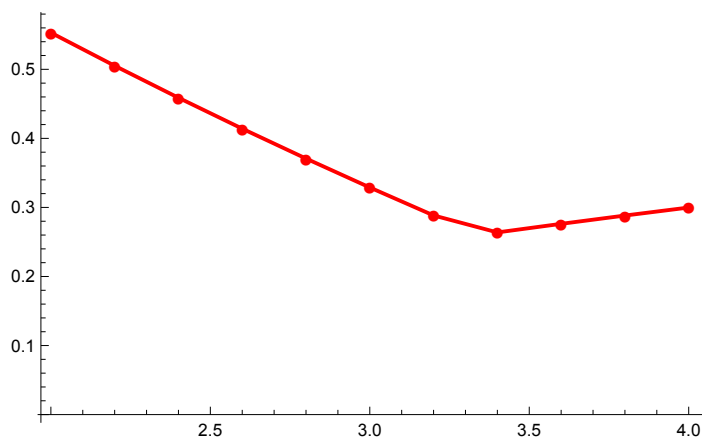

```
N[MinimalBy[tabgamma, Last]]
```

```
{{3.4, 0.263819}}
```

```
intgamma = Interpolation[tabgamma, x]
```

```
InterpolatingFunction[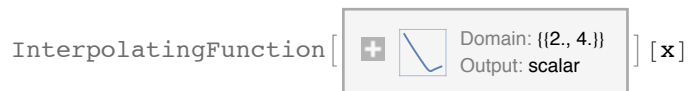 Domain: {{2., 4.}}  
Output: scalar][x]
```

```
mingamma = FindMinimum[intgamma, {x, 2.0, 4.0}]
```

```
InterpolatingFunction::dmval:
```

```
Input value {4.26425} lies outside the range of data in the interpolating function. Extrapolation will be used. >>
```

```
{0.263819, {x -> 3.4}}
```

```
optent = x /. mingamma[[2]]
```

```
3.4
```

```
optGaFra := optent * gammaFrag
```

```

iy = dsionyieldcrateranalysisparam[damp * 0.26 * MilliJouleToHartree, photonenergy,
  tauX, nintdata, True, True, 1 / 1000, optfNppN, 1 - optfNppN, optGaFra]
iynorm = 1 / Total[iy[[2 ;; 8]]] * iy
Total[iynorm[[2 ;; 8]]]

{0.96272, 0.0211292, 0.0116178, 0.00170051, 0.00205056, 0.000687514, 0.0000895245,
  4.9035 × 10-6, 0.959202, 0.000633826, 2.4216 × 10-17, 3.35031 × 10-109}

{25.824, 0.566771, 0.311636, 0.0456144, 0.0550043, 0.0184419, 0.00240141,
  0.000131532, 25.7296, 0.0170018, 6.49569 × 10-16, 8.98689 × 10-108}

1.

```

```

plotiy = Partition[Riffle[normOleg280, iynorm[[2 ;; 8]]], 2]
{{0.56634, 0.566771}, {0.291805, 0.311636},
 {0.0763903, 0.0456144}, {0.0364504, 0.0550043},
 {0.027387, 0.0184419}, {0.00162698, 0.00240141}, {0., 0.000131532}}

BarChart[plotiy, PlotRange → {-0.1, 0.9},
  ChartLabels → {Placed[{"N +", "N 2+", "N 3+", "N 4+", "N 5+", "N 6+", "N 7+"}, Below],
    Placed[{}, Above]},
  ChartLegends → Placed[{"Expt.", "γfrag"}, Top],
  ChartStyle → {Black, Red}, AxesLabel → {"", "Ỹ(ω)"},
  AxesStyle → {{Arrowheads[Automatic], AbsoluteThickness[0.6]},
    {Arrowheads[Automatic], AbsoluteThickness[0.6]}},
  LabelStyle → {FontFamily → "Arial"},
  PlotLabel → {damp, optGaFra / gammaFrag,
    (iynorm[[2 ;; 8]] - normOleg280).Table[i, {i, 1, 7}]}]

```

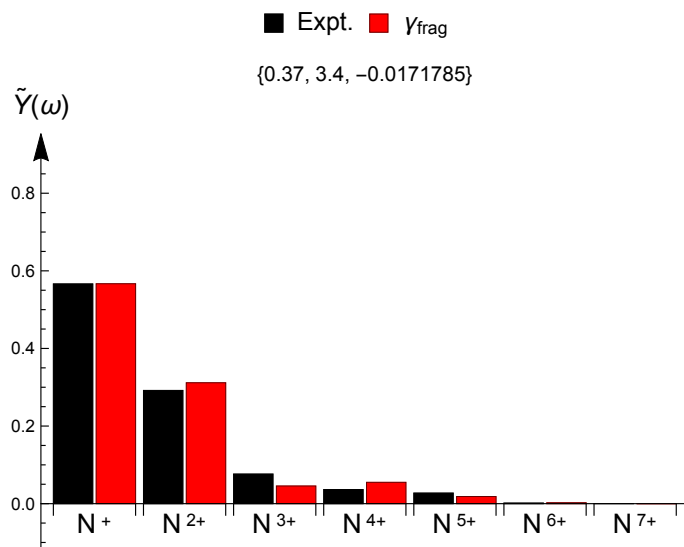

## 0.38

```

damp := 0.38

tabgamma =
  Table[{gaFra, normfitconsts[damp, gaFra * gammaFrag]}, {gaFra, 1, 10, 1 / 2}];

```

```
ListPlot[tabgamma, Joined -> True,
PlotMarkers -> Automatic, PlotStyle -> {Thick, Red}]
```

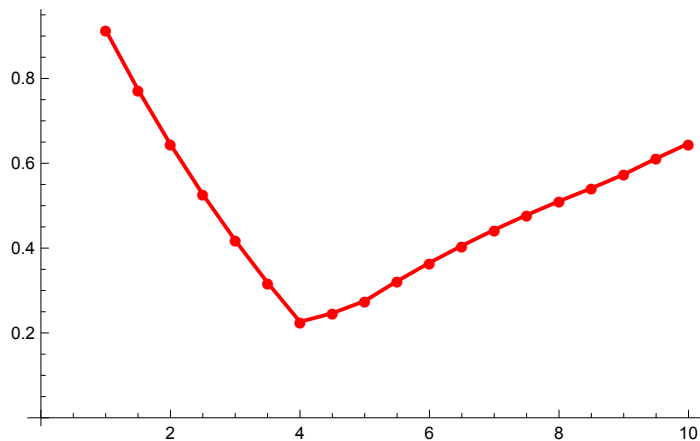

```
tabgamma =
Table[{gaFra, normfitconsts[damp, gaFra * gammaFrag]}, {gaFra, 3, 5, 1/5}];
```

```
ListPlot[tabgamma, Joined -> True,
PlotMarkers -> Automatic, PlotStyle -> {Thick, Red}]
```

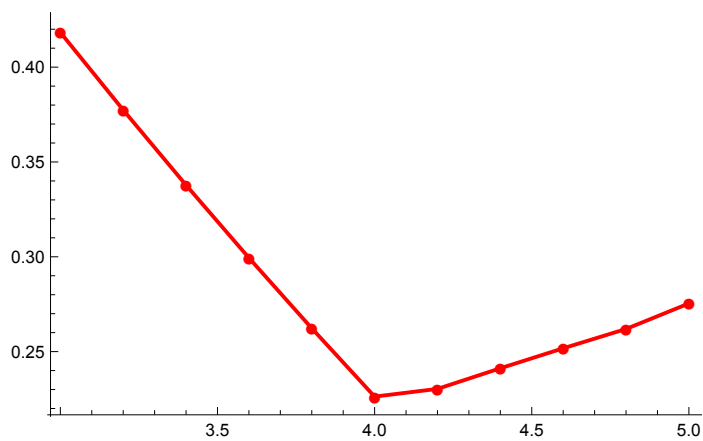

```
N[MinimalBy[tabgamma, Last]]
```

```
{{4., 0.226274}}
```

```
intgamma = Interpolation[tabgamma, x]
```

```
InterpolatingFunction[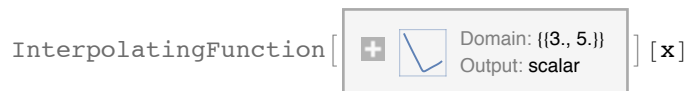 Domain: {{3., 5.}}  
Output: scalar][x]
```

```
mingamma = FindMinimum[intgamma, {x, 3.0, 5.0}]
```

```
InterpolatingFunction::dmval:
```

```
Input value {5.26425} lies outside the range of data in the interpolating function. Extrapolation will be used. >>
```

```
{0.224799, {x -> 4.05936}}
```

```
optent = x /. mingamma[[2]]
```

```
4.05936
```

```
optGaFra := optent * gammaFrag
```

```

iy = dsionyieldcrateranalysisparam[damp * 0.26 * MilliJouleToHartree, photonenergy,
  tauX, nintdata, True, True, 1 / 1000, optfNppN, 1 - optfNppN, optGaFra]
iynorm = 1 / Total[iy[[2 ;; 8]]] * iy
Total[iynorm[[2 ;; 8]]]

{0.962077, 0.0214849, 0.0114973, 0.00194797, 0.00211792, 0.000765548, 0.000103569,
  6.04188 × 10-6, 0.958498, 0.00063857, 3.46303 × 10-20, 3.26893 × 10-109}

{25.3691, 0.566536, 0.303173, 0.0513661, 0.0558475, 0.0201868, 0.00273103,
  0.000159319, 25.2747, 0.0168385, 9.13169 × 10-19, 8.61986 × 10-108}

1.

```

```

plotiy = Partition[Riffle[normOleg280, iynorm[[2 ;; 8]]], 2]
{{0.56634, 0.566536}, {0.291805, 0.303173},
 {0.0763903, 0.0513661}, {0.0364504, 0.0558475},
 {0.027387, 0.0201868}, {0.00162698, 0.00273103}, {0., 0.000159319}}

BarChart[plotiy, PlotRange → {-0.1, 0.9},
  ChartLabels → {Placed[{"N +", "N 2+", "N 3+", "N 4+", "N 5+", "N 6+", "N 7+"}, Below],
    Placed[{}, Above]},
  ChartLegends → Placed[{"Expt.", "γfrag"}, Top],
  ChartStyle → {Black, Red}, AxesLabel → {"", "Ỹ(ω)"},
  AxesStyle → {{Arrowheads[Automatic], AbsoluteThickness[0.6]},
    {Arrowheads[Automatic], AbsoluteThickness[0.6]}},
  LabelStyle → {FontFamily → "Arial"},
  PlotLabel → {damp, optGaFra / gammaFrag,
    (iynorm[[2 ;; 8]] - normOleg280).Table[i, {i, 1, 7}]]}

■ Expt. ■ γfrag
{0.38, 4.05936, -0.00281374}

```

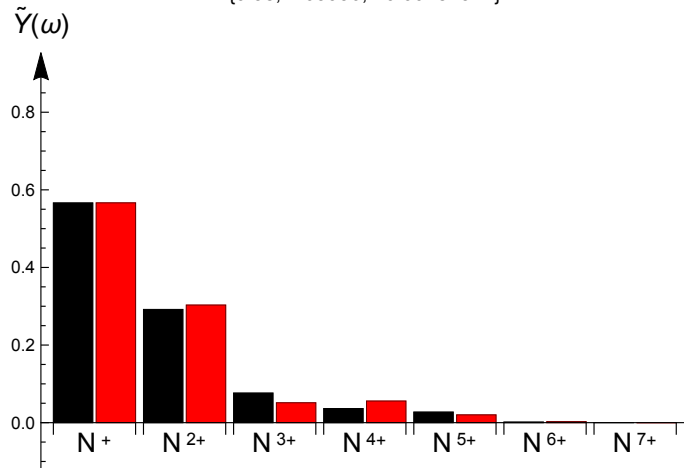

## 0.39

```

damp := 0.39

tabgamma =
  Table[{gaFra, normfitconsts[damp, gaFra * gammaFrag]}, {gaFra, 1, 10, 1 / 2}];

```



```
ListPlot[tabgamma, Joined -> True,
  PlotMarkers -> Automatic, PlotStyle -> {Thick, Red}]
```

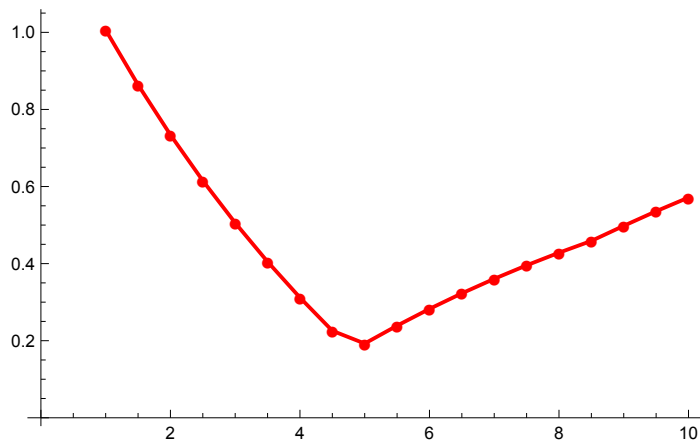

```
tabgamma =
  Table[{gaFra, normfitconsts[damp, gaFra * gammaFrag]}, {gaFra, 4, 6, 1/5}];
```

```
ListPlot[tabgamma, Joined -> True,
  PlotMarkers -> Automatic, PlotStyle -> {Thick, Red}]
```

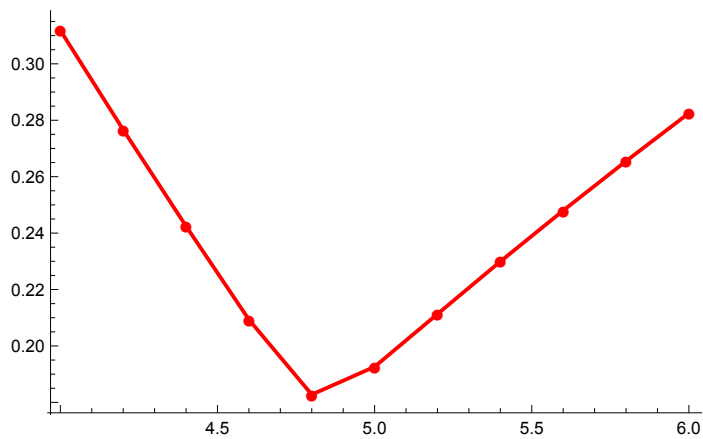

```
N[MinimalBy[tabgamma, Last]]
```

```
{{4.8, 0.182754}}
```

```
intgamma = Interpolation[tabgamma, x]
```

```
InterpolatingFunction[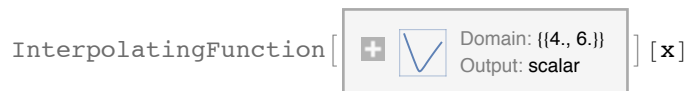 Domain: {{4., 6.}}  
Output: scalar][x]
```

```
mingamma = FindMinimum[intgamma, {x, 4.0, 6.0}]
```

```
InterpolatingFunction::dmval:
```

```
Input value {6.26425} lies outside the range of data in the interpolating function. Extrapolation will be used. >>
```

```
{0.182557, {x -> 4.82139}}
```

```
optent = x /. mingamma[[2]]
```

```
4.82139
```

```
optGaFra := optent * gammaFrag
```

```

iy = dsionyieldcrateranalysisparam[damp * 0.26 * MilliJouleToHartree, photonenergy,
  tauX, nintdata, True, True, 1 / 1000, optfNppN, 1 - optfNppN, optGaFra]
iynorm = 1 / Total[iy[[2 ;; 8]]] * iy
Total[iynorm[[2 ;; 8]]]

{0.961448, 0.0218451, 0.0113399, 0.00221276, 0.00217847, 0.000849388, 0.000119309,
  7.39496 × 10-6, 0.957808, 0.000643048, 1.80988 × 10-23, -1.58014 × 10-109}

{24.9388, 0.566635, 0.294143, 0.0573962, 0.0565069, 0.0220321, 0.00309472,
  0.000191816, 24.8444, 0.0166799, 4.6946 × 10-22, -4.09868 × 10-108}

1.

```

```

plotiy = Partition[Riffle[normOleg280, iynorm[[2 ;; 8]]], 2]
{{0.56634, 0.566635}, {0.291805, 0.294143},
 {0.0763903, 0.0573962}, {0.0364504, 0.0565069},
 {0.027387, 0.0220321}, {0.00162698, 0.00309472}, {0., 0.000191816}}

BarChart[plotiy, PlotRange → {-0.1, 0.9},
  ChartLabels → {Placed[{"N +", "N 2+", "N 3+", "N 4+", "N 5+", "N 6+", "N 7+"}, Below],
    Placed[{}, Above]},
  ChartLegends → Placed[{"Expt.", "γfrag"}, Top],
  ChartStyle → {Black, Red}, AxesLabel → {"", "Ỹ(ω)"},
  AxesStyle → {{Arrowheads[Automatic], AbsoluteThickness[0.6]},
    {Arrowheads[Automatic], AbsoluteThickness[0.6]}},
  LabelStyle → {FontFamily → "Arial"},
  PlotLabel → {damp, optGaFra / gammaFrag,
    (iynorm[[2 ;; 8]] - normOleg280).Table[i, {i, 1, 7}]}]

```

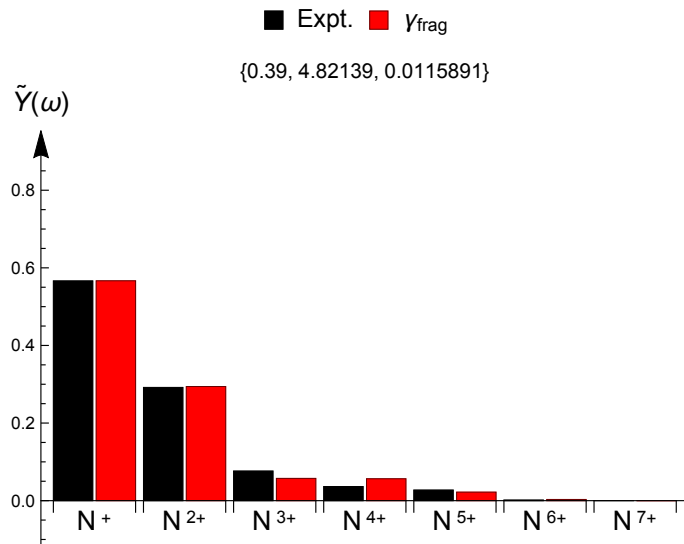

0.40

```
damp := 0.40
```

```

tabgamma =
  Table[{gaFra, normfitconsts[damp, gaFra * gammaFrag]}, {gaFra, 1, 10, 1 / 2}];

```

```
ListPlot[tabgamma, Joined -> True,
PlotMarkers -> Automatic, PlotStyle -> {Thick, Red}]
```

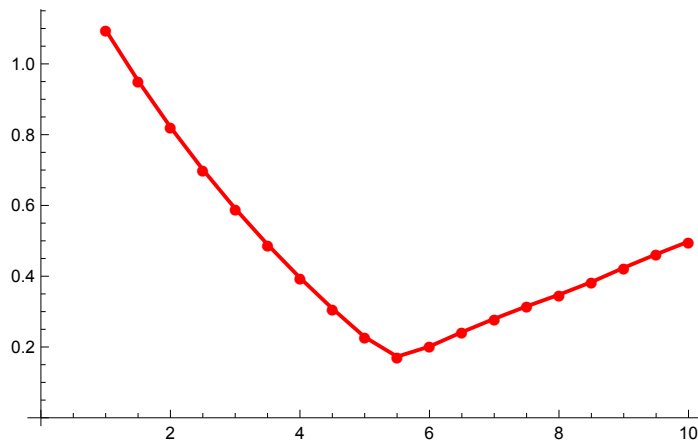

```
tabgamma =
Table[{gaFra, normfitconsts[damp, gaFra * gammaFrag]}, {gaFra, 4.5, 6.5, 1 / 5}];
```

```
ListPlot[tabgamma, Joined -> True,
PlotMarkers -> Automatic, PlotStyle -> {Thick, Red}]
```

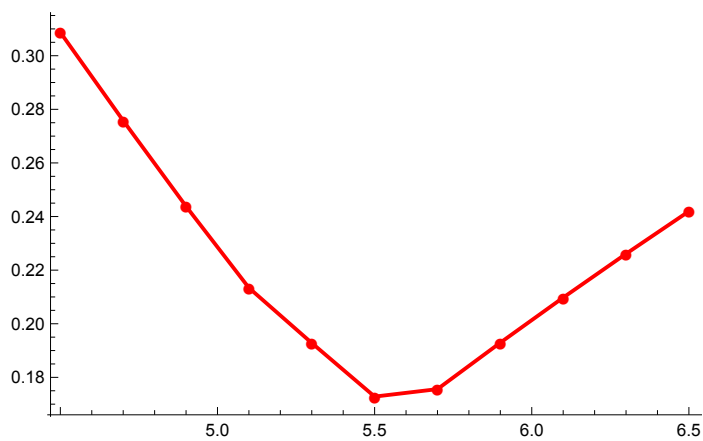

```
N[MinimalBy[tabgamma, Last]]
{{5.5, 0.172823}}
```

```
intgamma = Interpolation[tabgamma, x]
```

```
InterpolatingFunction[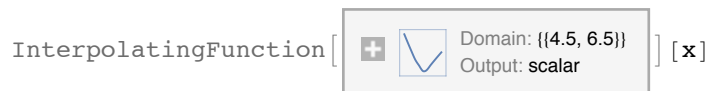 Domain: {{4.5, 6.5}}
Output: scalar ] [x]
```

```
mingamma = FindMinimum[intgamma, {x, 4.5, 6.5}]
```

```
InterpolatingFunction::dmval:
```

Input value {6.76425} lies outside the range of data in the interpolating function. Extrapolation will be used. >>

```
{0.171627, {x -> 5.56761}}
```

```
optent = x /. mingamma[[2]]
```

```
5.56761
```

```
optGaFra := optent * gammaFrag
```

```

iy = dsionyieldcrateranalysisparam[damp * 0.26 * MilliJouleToHartree, photonenergy,
  tauX, nintdata, True, True, 1 / 1000, optfNppN, 1 - optfNppN, optGaFra]
iynorm = 1 / Total[iy[[2 ;; 8]]] * iy
Total[iynorm[[2 ;; 8]]]

{0.960827, 0.0221824, 0.0112104, 0.00246227, 0.00223881, 0.000933997, 0.000135909,
  8.88442 × 10-6, 0.957131, 0.000647275, 1.32585 × 10-26, -1.1156 × 10-109}

{24.528, 0.566271, 0.28618, 0.0628568, 0.0571525, 0.0238431, 0.00346949,
  0.000226801, 24.4336, 0.0165236, 3.38462 × 10-25, -2.84791 × 10-108}

1.

plotiy = Partition[Riffle[normOleg280, iynorm[[2 ;; 8]]], 2]
{{0.56634, 0.566271}, {0.291805, 0.28618},
 {0.0763903, 0.0628568}, {0.0364504, 0.0571525},
 {0.027387, 0.0238431}, {0.00162698, 0.00346949}, {0., 0.000226801}}

BarChart[plotiy, PlotRange → {-0.1, 0.9},
  ChartLabels → {Placed[{"N+", "N2+", "N3+", "N4+", "N5+", "N6+", "N7+"}, Below],
    Placed[{}, Above]},
  ChartLegends → Placed[{"Expt.", "γfrag"}, Top],
  ChartStyle → {Black, Red}, AxesLabel → {"", "Ỹ(ω)"},
  AxesStyle → {{Arrowheads[Automatic], AbsoluteThickness[0.6]},
    {Arrowheads[Automatic], AbsoluteThickness[0.6]}},
  LabelStyle → {FontFamily → "Arial"},
  PlotLabel → {damp, optGaFra / gammaFrag,
    (iynorm[[2 ;; 8]] - normOleg280).Table[i, {i, 1, 7}]}]

```

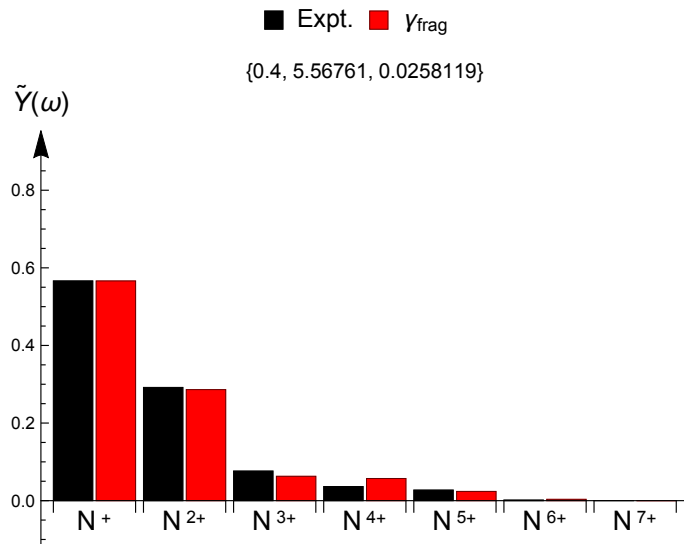

## Molecular fragmentation rate and pulse energy for a 80 fs pulse

```
tauX := 80 / t0ToFemtoSecond
```

```

normfitconsts[damp_?NumericQ, gaFra_?NumericQ] := Module[{olegiy, olegiynorm},
  olegiy =
    dsionyieldcrateranalysisparam[damp * 0.26 * MilliJouleToHartree, photonenergy,
      tauX, nintdata, True, True, 1 / 1000, optfNppN, 1 - optfNppN, gaFra];
  olegiynorm = 1 / Total[olegiy[[2 ;; 8]] * olegiy[[2 ;; 8]];
  Norm[(olegiynorm - normOleg80) * Table[i, {i, 1, 7}], 1] +
    16 * Abs[olegiynorm[[1]] - normOleg80[[1]]]
]

```

## 0.28

```
damp := 0.28
```

```

tabgamma =
  Table[{gaFra, normfitconsts[damp, gaFra * gammaFrag]}, {gaFra, 1, 20, 1 / 2}];

```

```

ListPlot[tabgamma, Joined -> True,
  PlotMarkers -> Automatic, PlotStyle -> {Thick, Red}]

```

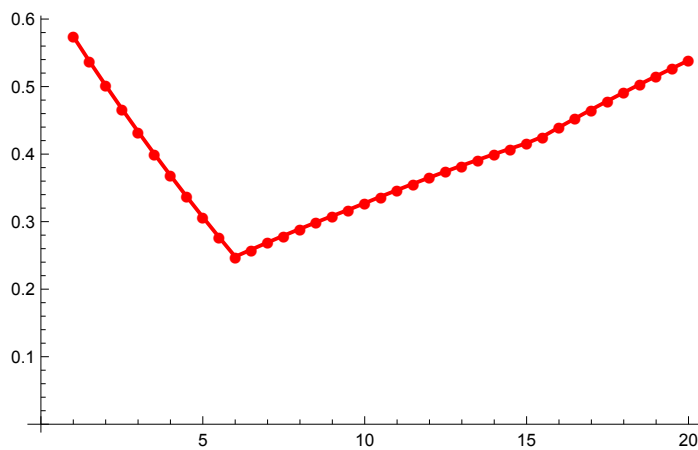

```

tabgamma =
  Table[{gaFra, normfitconsts[damp, gaFra * gammaFrag]}, {gaFra, 5, 7, 1 / 5}];

```

```

ListPlot[tabgamma, Joined -> True,
  PlotMarkers -> Automatic, PlotStyle -> {Thick, Red}]

```

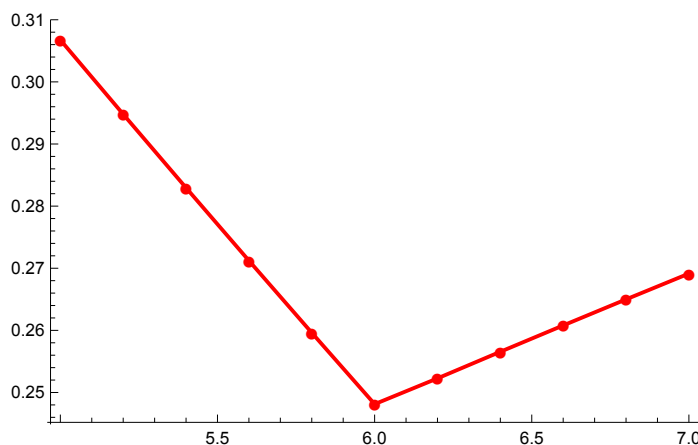

```
N[MinimalBy[tabgamma, Last]]
```

```
{{6., 0.248124}}
```

```
intgamma = Interpolation[tabgamma, x]
```

```
InterpolatingFunction[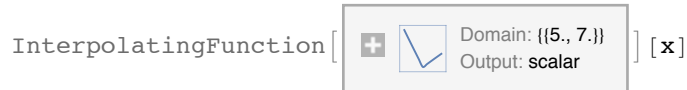 Domain: {{5., 7.}}  
Output: scalar][x]
```

```
mingamma = FindMinimum[intgamma, {x, 5.0, 7.0}]
```

InterpolatingFunction::dmval:

Input value {7.26425} lies outside the range of data in the interpolating function. Extrapolation will be used. >>

```
{0.248085, {x → 6.0144}}
```

```
optent = x /. mingamma[[2]]
```

```
6.0144
```

```
optGaFra := optent * gammaFrag
```

```
iy = dsionyielcdcrateranalysisparam[damp * 0.26 * MilliJouleToHartree, photonenergy,  
tauX, nintdata, True, True, 1 / 1000, optfNppN, 1 - optfNppN, optGaFra]
```

```
inyorm = 1 / Total[iy[[2 ;; 8]]] * iy
```

```
Total[iynorm[[2 ;; 8]]]
```

```
{0.969292, 0.0185488, 0.00991399, 0.000860147, 0.00110714, 0.000255558,  
0.000021853, 6.95061 × 10-7, 0.966197, 0.000576154, 1.03736 × 10-28, 7.46315 × 10-113}}
```

```
{31.5646, 0.604034, 0.322845, 0.0280103, 0.0360536, 0.00832213, 0.000711635,  
0.0000226344, 31.4638, 0.0187622, 3.37813 × 10-27, 2.43034 × 10-111}}
```

```
1.
```

```
plotiy = Partition[Riffle[normOleg80, iynorm[[2 ;; 8]]], 2]
```

```
{{0.604006, 0.604034}, {0.287434, 0.322845},  
{0.0722227, 0.0280103}, {0.0271552, 0.0360536},  
{0.00918191, 0.00832213}, {0., 0.000711635}, {0., 0.0000226344}}
```

```
BarChart[plotiy, PlotRange → {-0.1, 0.9},
  ChartLabels → {Placed[{"N +", "N 2+", "N 3+", "N 4+", "N 5+", "N 6+", "N 7+"}, Below],
    Placed[{}, Above]},
  ChartLegends → Placed[{"Expt.", "γfrag"}, Top],
  ChartStyle → {Black, Red}, AxesLabel → {"", "Ỹ(ω)"},
  AxesStyle → {{Arrowheads[Automatic], AbsoluteThickness[0.6]},
    {Arrowheads[Automatic], AbsoluteThickness[0.6]}},
  LabelStyle → {FontFamily → "Arial"},
  PlotLabel → {damp, optGaFra / gammaFrag,
    (iynorm[[2 ;; 8]] - normOleg80).Table[i, {i, 1, 7}]]}
```

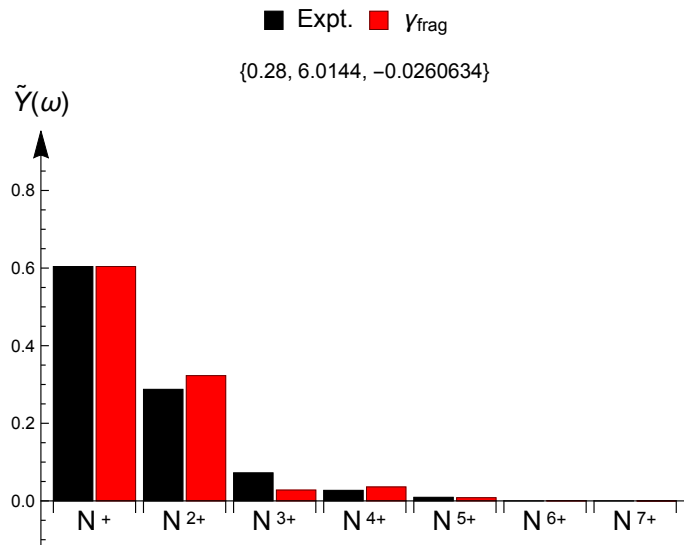

## 0.29

damp := 0.29

```
tabgamma =
  Table[{gaFra, normfitconsts[damp, gaFra * gammaFrag]}, {gaFra, 5, 15, 1 / 2}];
ListPlot[tabgamma, Joined -> True,
  PlotMarkers -> Automatic, PlotStyle -> {Thick, Red}]
```

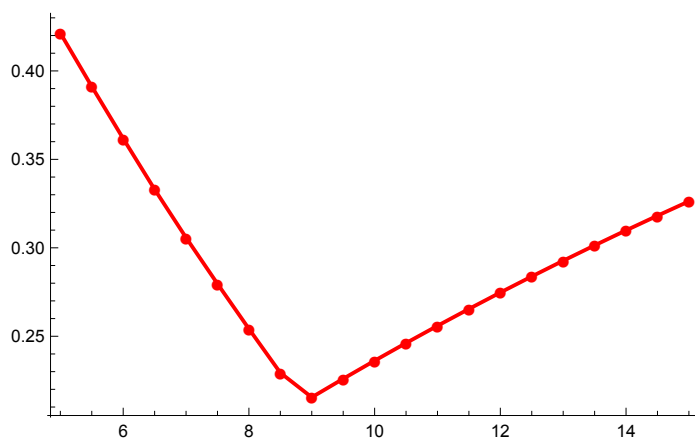

```
tabgamma =
  Table[{gaFra, normfitconsts[damp, gaFra * gammaFrag]}, {gaFra, 8, 10, 1 / 5}];
```

```
ListPlot[tabgamma, Joined -> True,
PlotMarkers -> Automatic, PlotStyle -> {Thick, Red}]
```

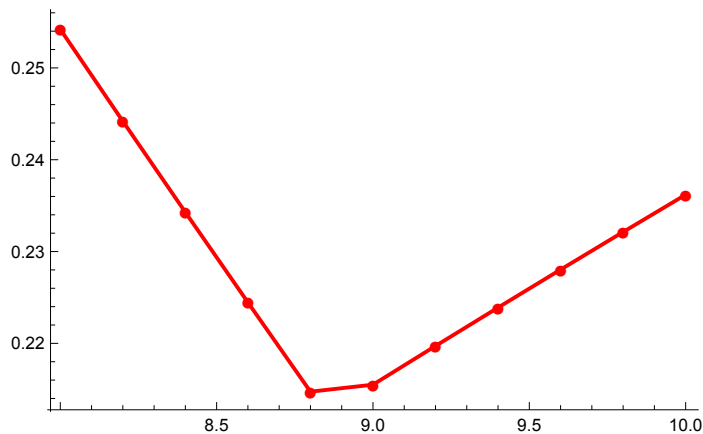

```
N[MinimalBy[tabgamma, Last]]
```

```
{{8.8, 0.214738}}
```

```
intgamma = Interpolation[tabgamma, x]
```

```
InterpolatingFunction[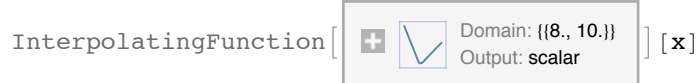 Domain: {{8., 10.}}  
Output: scalar][x]
```

```
mingamma = FindMinimum[intgamma, {x, 8.0, 10.0}]
```

```
InterpolatingFunction::dmval:
```

Input value {10.2642} lies outside the range of data in the interpolating function. Extrapolation will be used. >>

```
{0.214171, {x -> 8.87177}}
```

```
optent = x /. mingamma[[2]]
```

```
8.87177
```

```
optGaFra := optent * gammaFrag
```

```
iy = dsionyieldcrateranalysisparam[damp * 0.26 * MilliJouleToHartree, photonenergy,  
tauX, nintdata, True, True, 1 / 1000, optfNppN, 1 - optfNppN, optGaFra]
```

```
inyorm = 1 / Total[iy[[2 ;; 8]]] * iy
```

```
Total[iynorm[[2 ;; 8]]]
```

```
{0.968527, 0.019011, 0.00984659, 0.00110093, 0.00118002, 0.000305668,  
0.0000273909, 9.49682 × 10-7, 0.965355, 0.000584142, 3.99836 × 10-41, 8.2898 × 10-114}
```

```
{30.7737, 0.60405, 0.312863, 0.0349805, 0.0374936, 0.00971221, 0.000870312,  
0.0000301749, 30.6729, 0.0185604, 1.27043 × 10-39, 2.63398 × 10-112}
```

```
1.
```

```
plotiy = Partition[Riffle[normOleg80, iynorm[[2 ;; 8]]], 2]
```

```
{{0.604006, 0.60405}, {0.287434, 0.312863},  
{0.0722227, 0.0349805}, {0.0271552, 0.0374936},  
{0.00918191, 0.00971221}, {0., 0.000870312}, {0., 0.0000301749}}
```



```
BarChart[plotiy, PlotRange → {-0.1, 0.9},
  ChartLabels → {Placed[{"N +", "N 2+", "N 3+", "N 4+", "N 5+", "N 6+", "N 7+"}, Below],
    Placed[{}, Above]},
  ChartLegends → Placed[{"Expt.", "γfrag"}, Top],
  ChartStyle → {Black, Red}, AxesLabel → {"", "Ỹ(ω)",
  AxesStyle → {{Arrowheads[Automatic], AbsoluteThickness[0.6]},
    {Arrowheads[Automatic], AbsoluteThickness[0.6]}},
  LabelStyle → {FontFamily → "Arial"},
  PlotLabel → {damp, optGaFra / gammaFrag,
    (iynorm[2 ;; 8] - normOleg80).Table[i, {i, 1, 7}]]]
```

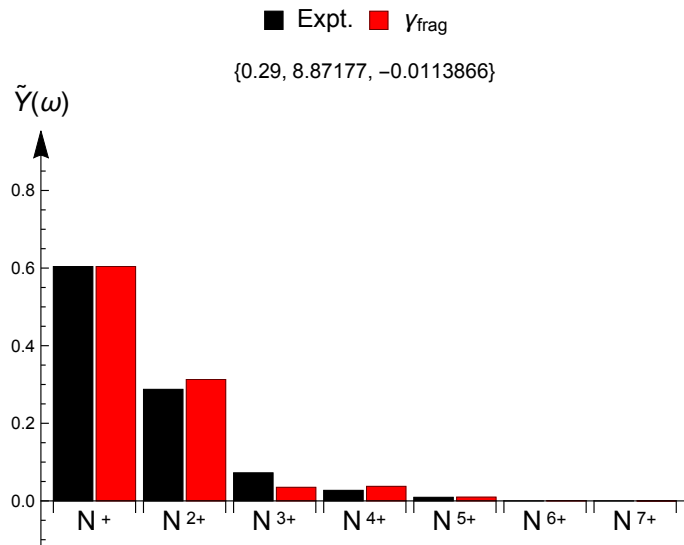

### 0.30

damp := 0.30

```
tabgamma =
  Table[{gaFra, normfitconsts[damp, gaFra * gammaFrag]}, {gaFra, 5, 15, 1 / 2}];
```

```
ListPlot[tabgamma, Joined -> True,
  PlotMarkers -> Automatic, PlotStyle -> {Thick, Red}]
```

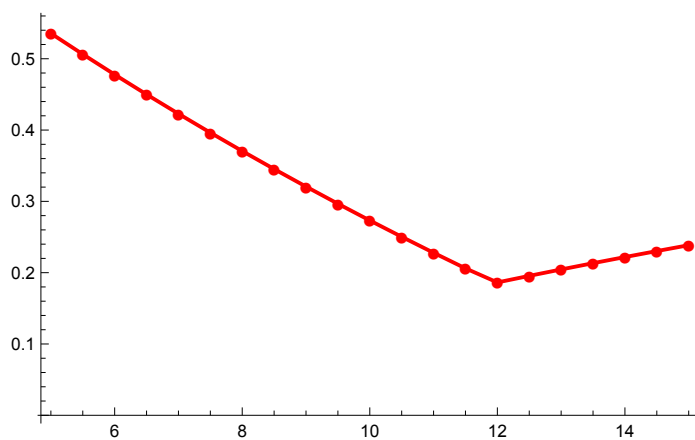

```
tabgamma =
  Table[{gaFra, normfitconsts[damp, gaFra * gammaFrag]}, {gaFra, 11, 13, 1 / 5}];
```

```
ListPlot[tabgamma, Joined -> True,
  PlotMarkers -> Automatic, PlotStyle -> {Thick, Red}]
```

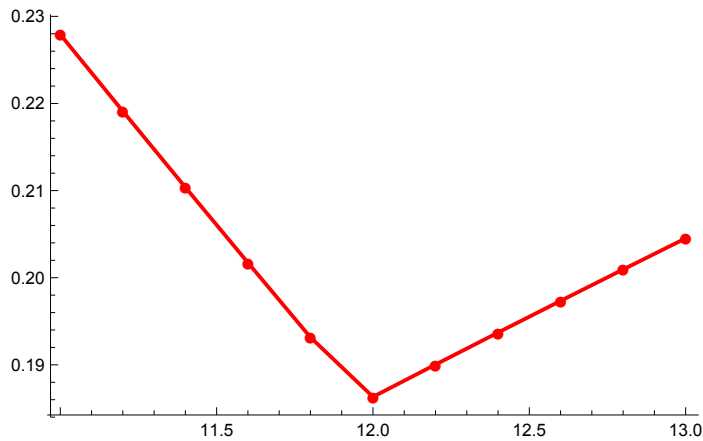

```
N[MinimalBy[tabgamma, Last]]
```

```
{{12., 0.186327}}
```

```
intgamma = Interpolation[tabgamma, x]
```

```
InterpolatingFunction[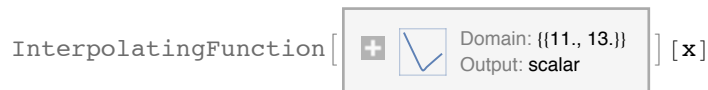 Domain: {{11., 13.}}  
Output: scalar][x]
```

```
mingamma = FindMinimum[intgamma, {x, 11, 13}]
```

```
InterpolatingFunction::dmval:
```

```
Input value {13.2642} lies outside the range of data in the interpolating function. Extrapolation will be used. >>
```

```
{0.186327, {x -> 12.}}
```

```
optent = x /. mingamma[[2]]
```

```
12.
```

```
optGaFra := optent * gammaFrag
```

```
iy = dsionyieldcrateranalysisparam[damp * 0.26 * MilliJouleToHartree, photonenergy,  
  tauX, nintdata, True, True, 1 / 1000, optfNppN, 1 - optfNppN, optGaFra]
```

```
iynorm = 1 / Total[iy[[2 ;; 8]]] * iy
```

```
Total[iynorm[[2 ;; 8]]]
```

```
{0.967779, 0.0194633, 0.00976408, 0.00134806, 0.00125066, 0.000359958,  
  0.0000337345, 1.26099 × 10-6, 0.96453, 0.000591681, 1.17802 × 10-54, 3.91019 × 10-115}}
```

```
{30.0356, 0.604055, 0.303034, 0.041838, 0.0388149, 0.0111715, 0.00104697,  
  0.0000391357, 29.9348, 0.0183632, 3.65605 × 10-53, 1.21355 × 10-113}}
```

```
1.
```

```
plotiy = Partition[Riffle[normOleg80, iynorm[[2 ;; 8]]], 2]
```

```
{{0.604006, 0.604055}, {0.287434, 0.303034},  
  {0.0722227, 0.041838}, {0.0271552, 0.0388149},  
  {0.00918191, 0.0111715}, {0., 0.00104697}, {0., 0.0000391357}}
```

```
BarChart[plotiy, PlotRange → {-0.1, 0.9},
  ChartLabels → {Placed[{"N +", "N 2+", "N 3+", "N 4+", "N 5+", "N 6+", "N 7+"}, Below],
    Placed[{}, Above]},
  ChartLegends → Placed[{"Expt.", "γfrag"}, Top],
  ChartStyle → {Black, Red}, AxesLabel → {"", "Ỹ(ω)",
  AxesStyle → {{Arrowheads[Automatic], AbsoluteThickness[0.6]},
    {Arrowheads[Automatic], AbsoluteThickness[0.6]}},
  LabelStyle → {FontFamily → "Arial"},
  PlotLabel → {damp, optGaFra / gammaFrag,
    (iynorm[2 ;; 8] - normOleg80).Table[i, {i, 1, 7}]]]
```

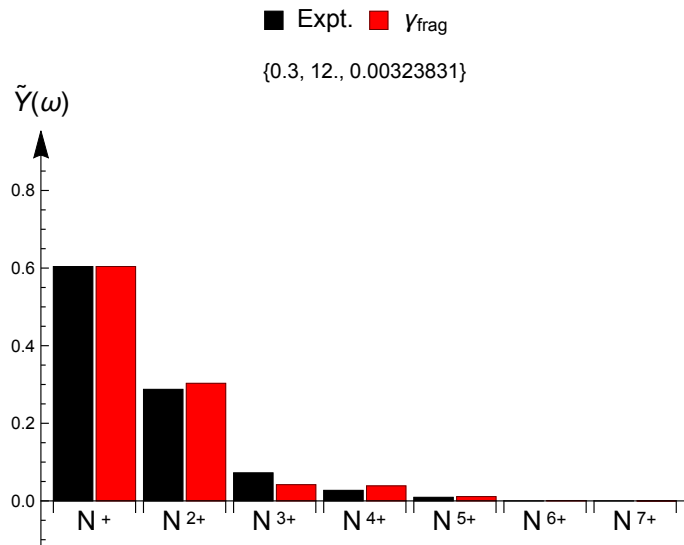

### 0.31

```
damp := 0.31
```

```
tabgamma =
  Table[{gaFra, normfitconsts[damp, gaFra * gammaFrag]}, {gaFra, 8, 18, 1 / 2}];
```

```
ListPlot[tabgamma, Joined -> True,
  PlotMarkers -> Automatic, PlotStyle -> {Thick, Red}]
```

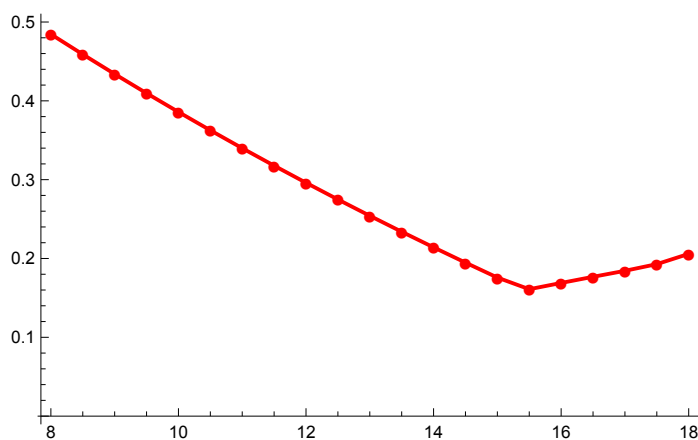

```
tabgamma = Table[
  {gaFra, normfitconsts[damp, gaFra * gammaFrag]}, {gaFra, 14.5, 16.5, 1 / 5}];
```

```
ListPlot[tabgamma, Joined -> True,
  PlotMarkers -> Automatic, PlotStyle -> {Thick, Red}]
```

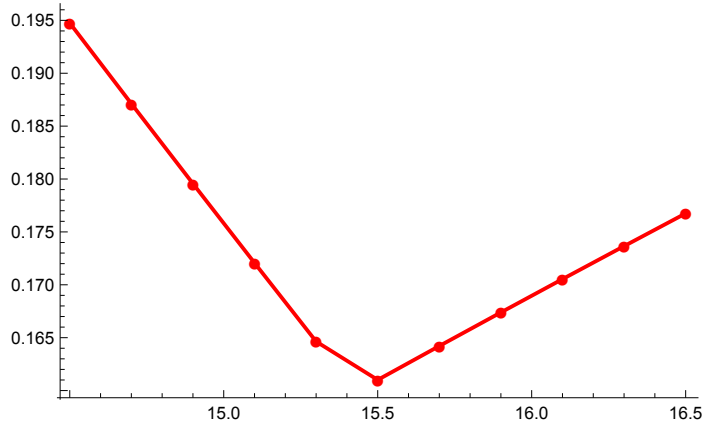

```
N[MinimalBy[tabgamma, Last]]
```

```
{{15.5, 0.161009}}
```

```
intgamma = Interpolation[tabgamma, x]
```

```
InterpolatingFunction[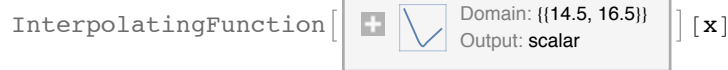 Domain: {{14.5, 16.5}}  
Output: scalar][x]
```

```
mingamma = FindMinimum[intgamma, {x, 14.5, 16.5}]
```

InterpolatingFunction::dmval:

Input value {16.7642} lies outside the range of data in the interpolating function. Extrapolation will be used. >>

```
{0.161009, {x -> 15.5}}
```

```
optent = x /. mingamma[[2]]
```

```
15.5
```

```
optGaFra := optent * gammaFrag
```

```
iy = dsionyieldcrateranalysisparam[damp * 0.26 * MilliJouleToHartree, photonenergy,
  tauX, nintdata, True, True, 1 / 1000, optfNppN, 1 - optfNppN, optGaFra]
```

```
inyorm = 1 / Total[iy[[2 ;; 8]]] * iy
```

```
Total[inyorm[[2 ;; 8]]]
```

```
{0.967046, 0.0199079, 0.00966278, 0.00160328,
  0.00131845, 0.000418757, 0.0000409797, 1.63945 × 10-6,
  0.963722, 0.000598796, 4.89803 × 10-70, -4.20318 × 10-139}}
```

```
{29.3455, 0.604116, 0.293222, 0.0486523, 0.0400091, 0.0127074, 0.00124355,
  0.00004975, 29.2446, 0.0181708, 1.48633 × 10-68, -1.27547 × 10-137}}
```

```
1.
```

```
plotiy = Partition[Riffle[normOleg80, inyorm[[2 ;; 8]]], 2]
```

```
{{0.604006, 0.604116}, {0.287434, 0.293222},
  {0.0722227, 0.0486523}, {0.0271552, 0.0400091},
  {0.00918191, 0.0127074}, {0., 0.00124355}, {0., 0.00004975}}
```

```
BarChart[plotiy, PlotRange → {-0.1, 0.9},
  ChartLabels → {Placed[{"N +", "N 2+", "N 3+", "N 4+", "N 5+", "N 6+", "N 7+"}, Below],
    Placed[{}, Above]},
  ChartLegends → Placed[{"Expt.", "γfrag"}, Top],
  ChartStyle → {Black, Red}, AxesLabel → {"", "Ỹ(ω)",
  AxesStyle → {{Arrowheads[Automatic], AbsoluteThickness[0.6]},
    {Arrowheads[Automatic], AbsoluteThickness[0.6]}},
  LabelStyle → {FontFamily → "Arial"},
  PlotLabel → {damp, optGaFra / gammaFrag,
    (iynorm[2 ;; 8] - normOleg80).Table[i, {i, 1, 7}]]]
```

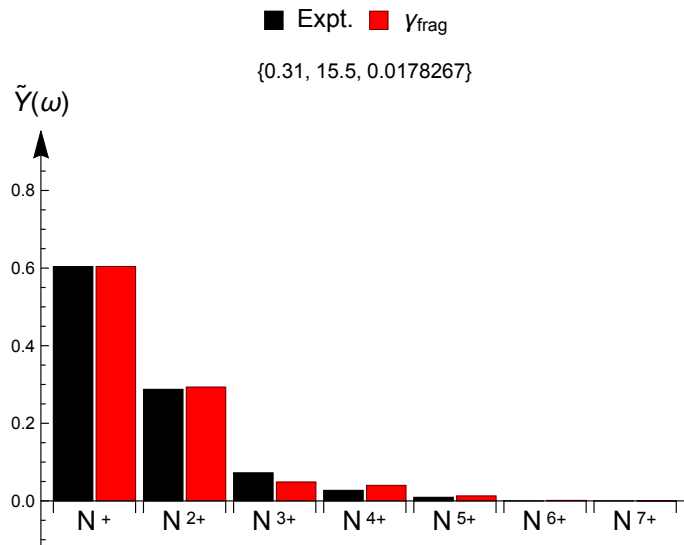

## 0.32

```
damp := 0.32
```

```
tabgamma =
  Table[{gaFra, normfitconsts[damp, gaFra * gammaFrag]}, {gaFra, 12, 22, 1 / 2}];
```

```
ListPlot[tabgamma, Joined -> True,
  PlotMarkers -> Automatic, PlotStyle -> {Thick, Red}]
```

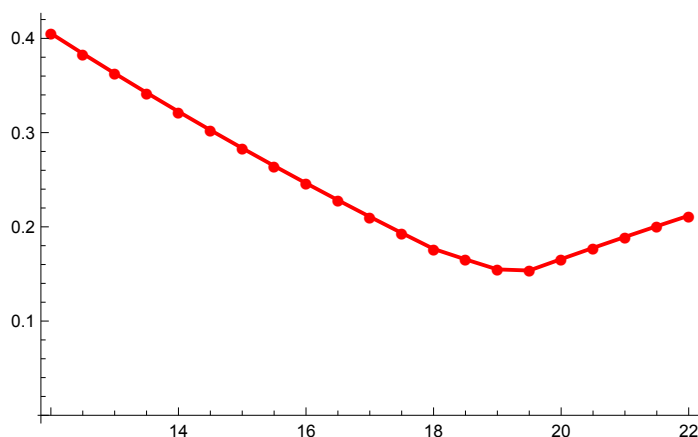

```
tabgamma = Table[
  {gaFra, normfitconsts[damp, gaFra * gammaFrag]}, {gaFra, 18.5, 20.5, 1 / 5}];
```

```
ListPlot[tabgamma, Joined -> True,
PlotMarkers -> Automatic, PlotStyle -> {Thick, Red}]
```

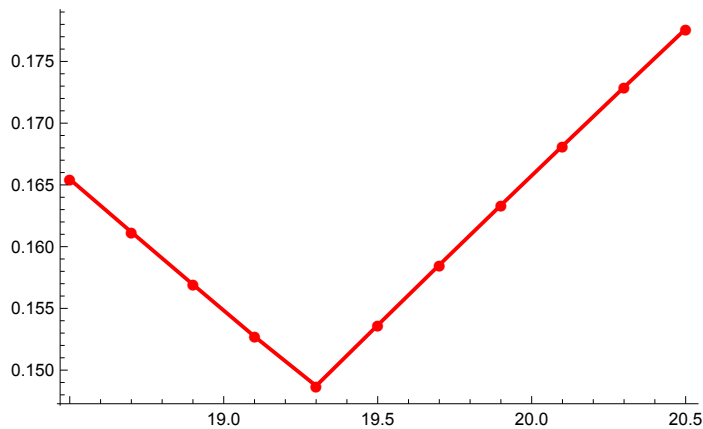

```
N[MinimalBy[tabgamma, Last]]
```

```
{{19.3, 0.148724}}
```

```
intgamma = Interpolation[tabgamma, x]
```

```
InterpolatingFunction[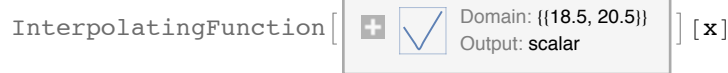 Domain: {{18.5, 20.5}}  
Output: scalar] [x]
```

```
mingamma = FindMinimum[intgamma, {x, 18.5, 20.5}]
```

```
InterpolatingFunction::dmval:
```

Input value {20.7642} lies outside the range of data in the interpolating function. Extrapolation will be used. >>

```
{0.148724, {x -> 19.3}}
```

```
optent = x /. mingamma[[2]]
```

```
19.3
```

```
optGaFra := optent * gammaFrag
```

```
iy = dsionyieldcrateranalysisparam[damp * 0.26 * MilliJouleToHartree, photonenergy,  
tauX, nintdata, True, True, 1 / 1000, optfNppN, 1 - optfNppN, optGaFra]
```

```
inyorm = 1 / Total[iy[[2 ;; 8]]] * iy
```

```
Total[inyorm[[2 ;; 8]]]
```

```
{0.966327, 0.0203386, 0.00955886, 0.00185899,  
0.00138377, 0.000481168, 0.0000490869, 2.08797 × 10-6,  
0.962931, 0.000605511, 2.67768 × 10-86, 1.58587 × 10-146}}
```

```
{28.6977, 0.604011, 0.283877, 0.0552079, 0.0410947, 0.0142896, 0.00145777,  
0.0000620079, 28.5969, 0.0179823, 7.95212 × 10-85, 4.70967 × 10-145}}
```

```
1.
```

```
plotiy = Partition[Riffle[normOleg80, inyorm[[2 ;; 8]]], 2]
```

```
{{0.604006, 0.604011}, {0.287434, 0.283877},  
{0.0722227, 0.0552079}, {0.0271552, 0.0410947},  
{0.00918191, 0.0142896}, {0., 0.00145777}, {0., 0.0000620079}}
```

```
BarChart[plotiy, PlotRange → {-0.1, 0.9},
  ChartLabels → {Placed[{"N +", "N 2+", "N 3+", "N 4+", "N 5+", "N 6+", "N 7+"}, Below],
    Placed[{}, Above]},
  ChartLegends → Placed[{"Expt.", "γfrag"}, Top],
  ChartStyle → {Black, Red}, AxesLabel → {"", "Ỹ(ω)"},
  AxesStyle → {{Arrowheads[Automatic], AbsoluteThickness[0.6]},
    {Arrowheads[Automatic], AbsoluteThickness[0.6]}},
  LabelStyle → {FontFamily → "Arial"},
  PlotLabel → {damp, optGaFra / gammaFrag,
    (iynorm[[2 ;; 8]] - normOleg80).Table[i, {i, 1, 7}]]]
```

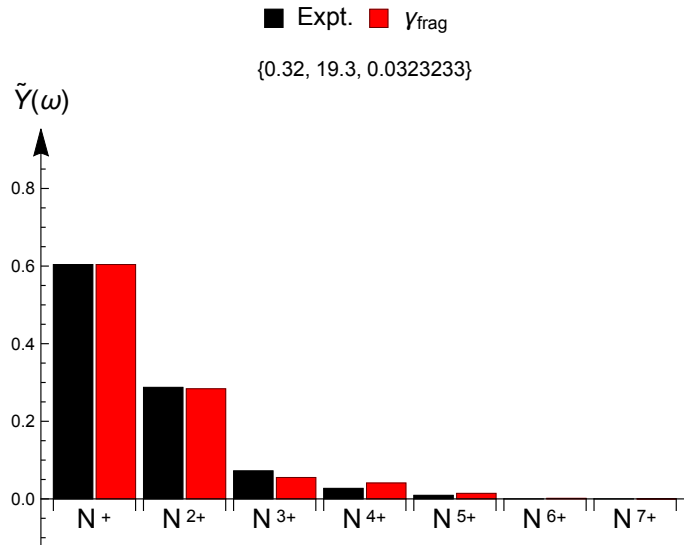

## Pulse energy for a 280 fs pulse with 280 fs fragmentation rate

```
tauX := 280 / t0ToFemtoSecond
optent := 4.059357
optGaFra := optent * gammaFrag
```

### 0.38

```
damp := 0.38
```

```
iy = dsionyieldcrateranalysisparam[damp * 0.26 * MilliJouleToHartree, photonenergy,
  tauX, nintdata, True, True, 1 / 1000, optfNppN, 1 - optfNppN, optGaFra]
iynorm = 1 / Total[iy[[2 ;; 8]]] * iy
Total[iynorm[[2 ;; 8]]]
```

```
{0.962077, 0.0214849, 0.0114973, 0.00194797, 0.00211792, 0.000765547, 0.000103569,
  6.04188 × 10-6, 0.958498, 0.00063857, 3.46375 × 10-20, -2.89667 × 10-110}}
```

```
{25.3691, 0.566536, 0.303173, 0.0513661, 0.0558475, 0.0201868, 0.00273103,
  0.000159319, 25.2747, 0.0168385, 9.13359 × 10-19, -7.63824 × 10-109}}
```

```
1.
```

```

plotiy = Partition[Riffle[normOleg280, iynorm[[2 ;; 8]]], 2]
{{0.56634, 0.566536}, {0.291805, 0.303173},
 {0.0763903, 0.0513661}, {0.0364504, 0.0558475},
 {0.027387, 0.0201868}, {0.00162698, 0.00273103}, {0., 0.000159319}}

BarChart[plotiy, PlotRange → {-0.1, 0.9},
 ChartLabels → {Placed[{"N +", "N 2+", "N 3+", "N 4+", "N 5+", "N 6+", "N 7+"}, Below],
   Placed[{}, Above]},
 ChartLegends → Placed[{"Expt.", "γfrag"}, Top],
 ChartStyle → {Black, Red}, AxesLabel → {"", "Ỹ(ω)"},
 AxesStyle → {{Arrowheads[Automatic], AbsoluteThickness[0.6]},
   {Arrowheads[Automatic], AbsoluteThickness[0.6]}},
 LabelStyle → {FontFamily → "Arial"},
 PlotLabel → {damp, optGaFra / gammaFrag,
   (iynorm[[2 ;; 8]] - normOleg280).Table[i, {i, 1, 7}]}]

```

■ Expt. ■ γ<sub>frag</sub>

{0.38, 4.05936, -0.00281378}

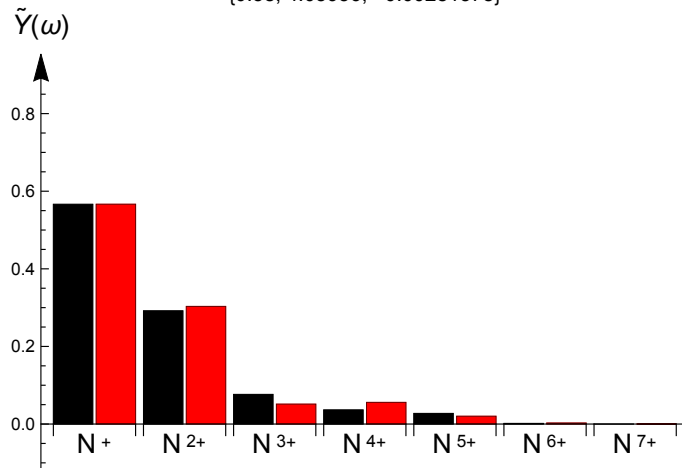

## Pulse energy for a 280 fs pulse with 80 fs fragmentation rate

```

tauX := 280 / t0ToFemtoSecond
optent := 12.000000
optGaFra := optent * gammaFrag

```

0.36

```
damp := 0.36
```



```

iy = dsionyieldcrateranalysisparam[damp * 0.26 * MilliJouleToHartree, photonenergy,
  tauX, nintdata, True, True, 1 / 1000, optfNppN, 1 - optfNppN, optGaFra]
iynorm = 1 / Total[iy[[2 ;; 8]]] * iy
Total[iynorm[[2 ;; 8]]]

```

```

{0.963623, 0.0221401, 0.00854545, 0.00305418,
 0.00165349, 0.000857835, 0.000118016, 8.03167 × 10-6,
 0.959919, 0.000628798, 3.32661 × 10-54, -9.06663 × 10-111}

```

```

{26.4898, 0.608628, 0.234913, 0.0839588, 0.0454541, 0.0235817, 0.00324425,
 0.000220789, 26.388, 0.0172856, 9.14479 × 10-53, -2.4924 × 10-109}

```

1.

```

plotiy = Partition[Riffle[normOleg280, iynorm[[2 ;; 8]]], 2]

```

```

{{0.56634, 0.608628}, {0.291805, 0.234913},
 {0.0763903, 0.0839588}, {0.0364504, 0.0454541},
 {0.027387, 0.0235817}, {0.00162698, 0.00324425}, {0., 0.000220789}}

```

```

BarChart[plotiy, PlotRange → {-0.1, 0.9},
  ChartLabels → {Placed[{"N +", "N 2+", "N 3+", "N 4+", "N 5+", "N 6+", "N 7+"}, Below],
    Placed[{}, Above]},
  ChartLegends → Placed[{"Expt.", "γfrag"}, Top],
  ChartStyle → {Black, Red}, AxesLabel → {"", "Ỹ(ω)"},
  AxesStyle → {{Arrowheads[Automatic], AbsoluteThickness[0.6]},
    {Arrowheads[Automatic], AbsoluteThickness[0.6]}},
  LabelStyle → {FontFamily → "Arial"},
  PlotLabel → {damp, optGaFra / gammaFrag,
    (iynorm[[2 ;; 8]] - normOleg280).Table[i, {i, 1, 7}]}]

```

■ Expt. ■ γ<sub>frag</sub>

{0.36, 12., -0.0205541}

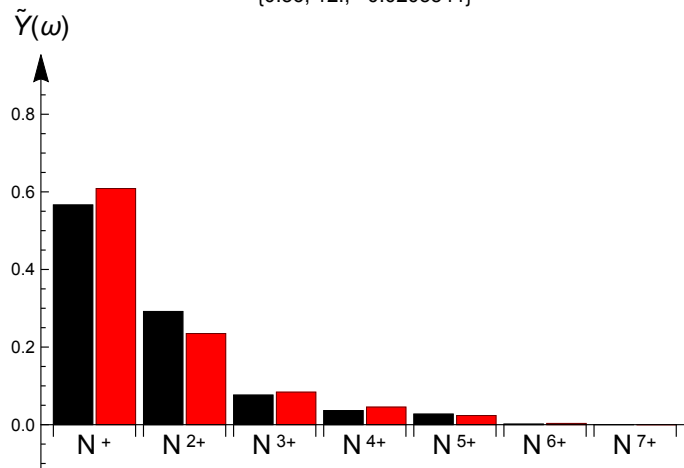

## 0.37

```
damp := 0.37
```

```

iy = dsionyieldcrateranalysisparam[damp * 0.26 * MilliJouleToHartree, photonenergy,
  tauX, nintdata, True, True, 1 / 1000, optfNppN, 1 - optfNppN, optGaFra]
iynorm = 1 / Total[iy[[2 ;; 8]]] * iy
Total[iynorm[[2 ;; 8]]]

```

```

{0.962944, 0.0223766, 0.00873078, 0.00315799,
 0.00173529, 0.000916225, 0.000129608, 9.05412 × 10-6,
 0.959202, 0.000633826, 3.36961 × 10-54, -1.54361 × 10-111}

```

```

{25.9865, 0.603866, 0.235613, 0.0852231, 0.0468295, 0.0247257, 0.00349766,
 0.000244339, 25.8855, 0.0171048, 9.09341 × 10-53, -4.16568 × 10-110}

```

1.

```

plotiy = Partition[Riffle[normOleg280, iynorm[[2 ;; 8]]], 2]

```

```

{{0.56634, 0.603866}, {0.291805, 0.235613},
 {0.0763903, 0.0852231}, {0.0364504, 0.0468295},
 {0.027387, 0.0247257}, {0.00162698, 0.00349766}, {0., 0.000244339}}

```

```

BarChart[plotiy, PlotRange → {-0.1, 0.9},
  ChartLabels → {Placed[{"N +", "N 2+", "N 3+", "N 4+", "N 5+", "N 6+", "N 7+"}, Below],
    Placed[{}, Above]},
  ChartLegends → Placed[{"Expt.", "γfrag"}, Top],
  ChartStyle → {Black, Red}, AxesLabel → {"", "Ỹ(ω)"},
  AxesStyle → {{Arrowheads[Automatic], AbsoluteThickness[0.6]},
    {Arrowheads[Automatic], AbsoluteThickness[0.6]}},
  LabelStyle → {FontFamily → "Arial"},
  PlotLabel → {damp, optGaFra / gammaFrag,
    (iynorm[[2 ;; 8]] - normOleg280).Table[i, {i, 1, 7}]}]

```

■ Expt. ■ γ<sub>frag</sub>

{0.37, 12., -0.00721442}

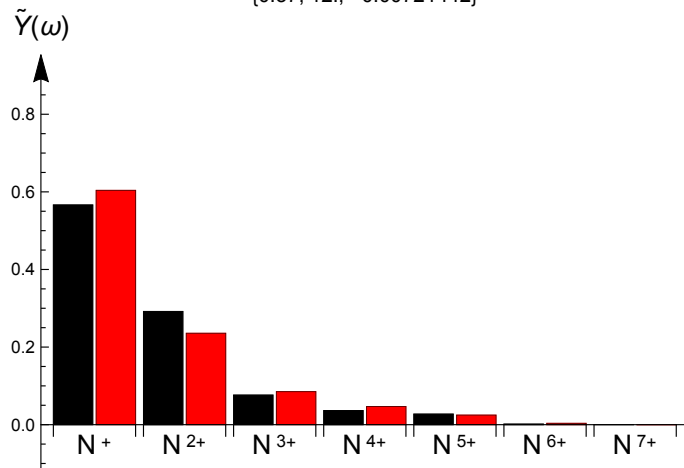

0.38

damp := 0.38

```
iy = dsionyieldcrateranalysisparam[damp * 0.26 * MilliJouleToHartree, photonenergy,
  tauX, nintdata, True, True, 1 / 1000, optfNppN, 1 - optfNppN, optGaFra]
iynorm = 1 / Total[iy[[2 ;; 8]]] * iy
Total[iynorm[[2 ;; 8]]]
```

```
{0.962278, 0.0226028, 0.00891207, 0.00326086,
  0.00181792, 0.000976418, 0.000141921, 0.0000101697,
  0.958498, 0.000638571, 3.39584 × 10-54, -2.47605 × 10-111}
```

```
{25.5097, 0.599191, 0.236256, 0.0864443, 0.0481923, 0.0258845, 0.00376226,
  0.000269595, 25.4095, 0.0169283, 9.00225 × 10-53, -6.56393 × 10-110}
```

1.

```
plotiy = Partition[Riffle[normOleg280, iynorm[[2 ;; 8]]], 2]
```

```
{{0.56634, 0.599191}, {0.291805, 0.236256},
  {0.0763903, 0.0864443}, {0.0364504, 0.0481923},
  {0.027387, 0.0258845}, {0.00162698, 0.00376226}, {0., 0.000269595}}
```

```
BarChart[plotiy, PlotRange → {-0.1, 0.9},
  ChartLabels → {Placed[{"N+", "N2+", "N3+", "N4+", "N5+", "N6+", "N7+"}, Below],
    Placed[{}, Above]},
  ChartLegends → Placed[{"Expt.", "γfrag"}, Top],
  ChartStyle → {Black, Red}, AxesLabel → {"", "Ỹ(ω)"},
  AxesStyle → {{Arrowheads[Automatic], AbsoluteThickness[0.6]},
    {Arrowheads[Automatic], AbsoluteThickness[0.6]}},
  LabelStyle → {FontFamily → "Arial"},
  PlotLabel → {damp, optGaFra / gammaFrag,
    (iynorm[[2 ;; 8]] - normOleg280).Table[i, {i, 1, 7}]}]
```

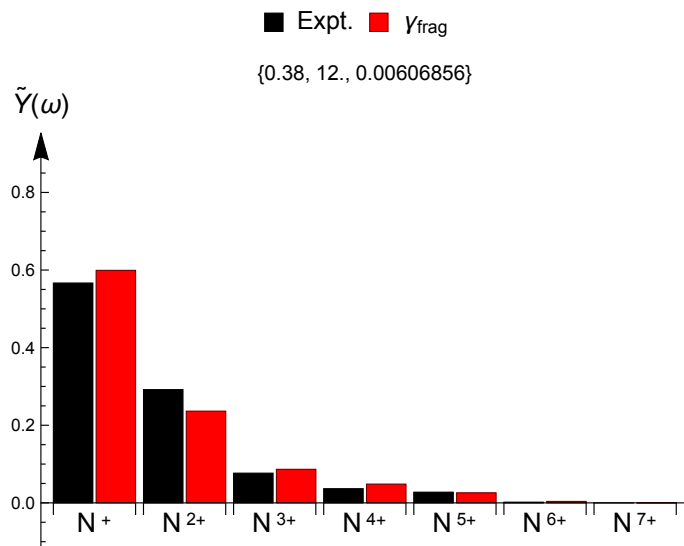

0.39

damp := 0.39

```

iy = dsionyieldcrateranalysisparam[damp * 0.26 * MilliJouleToHartree, photonenergy,
  tauX, nintdata, True, True, 1 / 1000, optfNppN, 1 - optfNppN, optGaFra]
iynorm = 1 / Total[iy[[2 ;; 8]]] * iy
Total[iynorm[[2 ;; 8]]]

{0.961623, 0.0228191, 0.00908929, 0.00336275, 0.00190128, 0.00103837, 0.000154971,
  0.0000113834, 0.957808, 0.000643049, 3.43175 × 10-54, -2.8847 × 10-111}

{25.0572, 0.594601, 0.236841, 0.0876237, 0.049542, 0.0270571, 0.00403811,
  0.000296619, 24.9578, 0.016756, 8.94217 × 10-53, -7.51671 × 10-110}

1.

```

```

plotiy = Partition[Riffle[normOleg280, iynorm[[2 ;; 8]]], 2]
{{0.56634, 0.594601}, {0.291805, 0.236841},
 {0.0763903, 0.0876237}, {0.0364504, 0.049542},
 {0.027387, 0.0270571}, {0.00162698, 0.00403811}, {0., 0.000296619}}

BarChart[plotiy, PlotRange → {-0.1, 0.9},
  ChartLabels → {Placed[{"N +", "N 2+", "N 3+", "N 4+", "N 5+", "N 6+", "N 7+"}, Below],
    Placed[{}, Above]},
  ChartLegends → Placed[{"Expt.", "γfrag"}, Top],
  ChartStyle → {Black, Red}, AxesLabel → {"", "Ỹ(ω)"},
  AxesStyle → {{Arrowheads[Automatic], AbsoluteThickness[0.6]},
    {Arrowheads[Automatic], AbsoluteThickness[0.6]}},
  LabelStyle → {FontFamily → "Arial"},
  PlotLabel → {damp, optGaFra / gammaFrag,
    (iynorm[[2 ;; 8]] - normOleg280).Table[i, {i, 1, 7}]}]

```

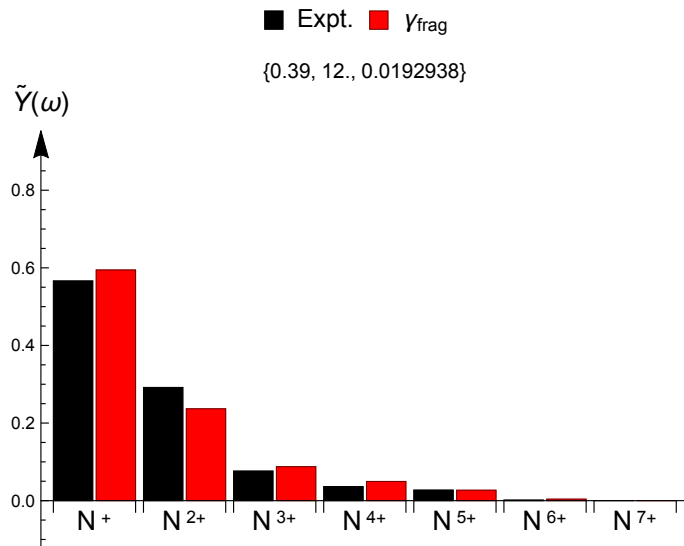

0.40

damp := 0.40

```
iy = dsionyieldcrateranalysisparam[damp * 0.26 * MilliJouleToHartree, photonenergy,
  tauX, nintdata, True, True, 1 / 1000, optfNppN, 1 - optfNppN, optGaFra]
iynorm = 1 / Total[iy[[2 ;; 8]]] * iy
Total[iynorm[[2 ;; 8]]]
```

```
{0.960979, 0.023026, 0.00926252, 0.00346358, 0.00198529, 0.00110206, 0.000168776,
  0.0000127003, 0.957131, 0.000647275, 3.45894 × 10-54, -1.68815 × 10-111}}
```

```
{24.6273, 0.590094, 0.237373, 0.0887622, 0.0508776, 0.0282427, 0.00432526,
  0.000325474, 24.5287, 0.0165879, 8.86432 × 10-53, -4.32628 × 10-110}}
```

```
1.
```

```
plotiy = Partition[Riffle[normOleg280, iynorm[[2 ;; 8]]], 2]
```

```
{{0.56634, 0.590094}, {0.291805, 0.237373},
  {0.0763903, 0.0887622}, {0.0364504, 0.0508776},
  {0.027387, 0.0282427}, {0.00162698, 0.00432526}, {0., 0.000325474}}
```

```
BarChart[plotiy, PlotRange → {-0.1, 0.9},
  ChartLabels → {Placed[{"N +", "N 2+", "N 3+", "N 4+", "N 5+", "N 6+", "N 7+"}, Below],
    Placed[{}, Above]},
  ChartLegends → Placed[{"Expt.", "γfrag"}, Top],
  ChartStyle → {Black, Red}, AxesLabel → {"", "Ỹ(ω)"},
  AxesStyle → {{Arrowheads[Automatic], AbsoluteThickness[0.6]},
    {Arrowheads[Automatic], AbsoluteThickness[0.6]}},
  LabelStyle → {FontFamily → "Arial"},
  PlotLabel → {damp, optGaFra / gammaFrag,
    (iynorm[[2 ;; 8]] - normOleg280).Table[i, {i, 1, 7}]]]
```

■ Expt. ■ γ<sub>frag</sub>

{0.4, 12., 0.0324608}

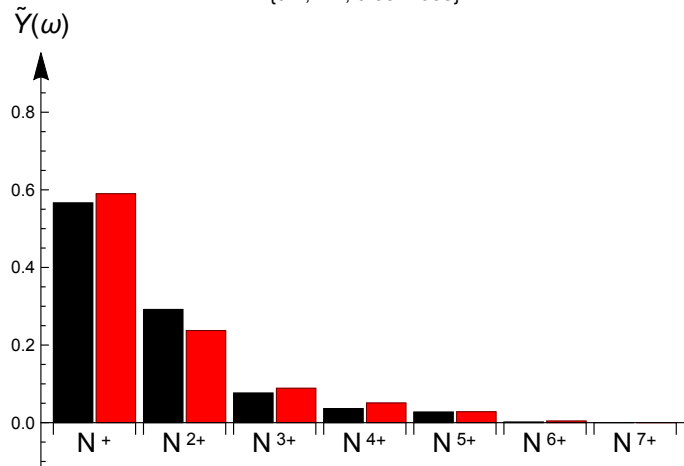

## Pulse energy for a 80 fs pulse with 280 fs fragmentation rate

```
tauX := 80 / t0ToFemtoSecond
optent := 4.059357
optGaFra := optent * gammaFrag
```

## 0.28

```
damp := 0.28
```

```
iy = dsionyieldcrateranalysisparam[damp * 0.26 * MilliJouleToHartree, photonenergy,  
  tauX, nintdata, True, True, 1 / 1000, optfNppN, 1 - optfNppN, optGaFra]
```

```
inyorm = 1 / Total[iy[[2 ;; 8]]] * iy
```

```
Total[iyorm[[2 ;; 8]]]
```

```
{0.969268, 0.0184167, 0.0102199, 0.000719674,  
  0.00111475, 0.000240014, 0.0000203645, 6.16998 × 10-7,  
  0.966197, 0.000576154, 2.82206 × 10-20, 3.27124 × 10-111}}
```

```
{31.5394, 0.599266, 0.33255, 0.0234177, 0.0362731, 0.0078099, 0.000662648,  
  0.0000200767, 31.4394, 0.0187477, 9.18282 × 10-19, 1.06444 × 10-109}}
```

```
1.
```

```
plotiy = Partition[Riffle[normOleg80, inyorm[[2 ;; 8]]], 2]
```

```
{{0.604006, 0.599266}, {0.287434, 0.33255},  
  {0.0722227, 0.0234177}, {0.0271552, 0.0362731},  
  {0.00918191, 0.0078099}, {0., 0.000662648}, {0., 0.0000200767}}
```

```
BarChart[plotiy, PlotRange → {-0.1, 0.9},  
  ChartLabels → {Placed[{"N +", "N 2+", "N 3+", "N 4+", "N 5+", "N 6+", "N 7+"}, Below],  
    Placed[{}, Above]},  
  ChartLegends → Placed[{"Expt.", "γfrag"}, Top],  
  ChartStyle → {Black, Red}, AxesLabel → {"", "Ỹ(ω)"},  
  AxesStyle → {{Arrowheads[Automatic], AbsoluteThickness[0.6]},  
    {Arrowheads[Automatic], AbsoluteThickness[0.6]}},  
  LabelStyle → {FontFamily → "Arial"},  
  PlotLabel → {damp, optGaFra / gammaFrag,  
    (inyorm[[2 ;; 8]] - normOleg80).Table[i, {i, 1, 7}]]}
```

■ Expt. ■ γ<sub>frag</sub>

{0.28, 4.05936, -0.0271939}

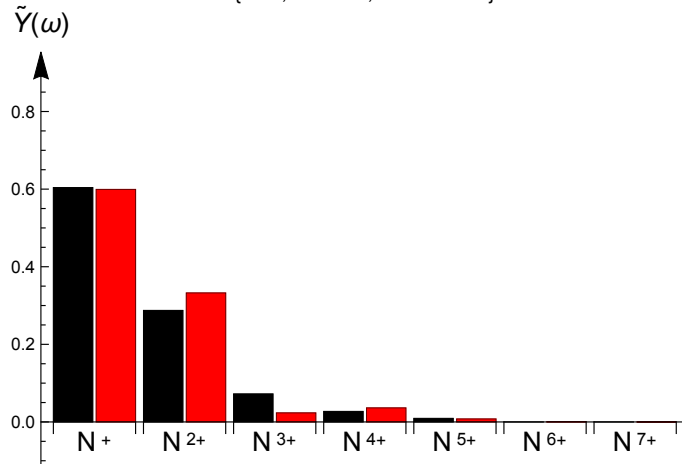

## 0.29

```
damp := 0.29
```

```

iy = dsionyieldcrateranalysisparam[damp * 0.26 * MilliJouleToHartree, photonenergy,
  tauX, nintdata, True, True, 1 / 1000, optfNppN, 1 - optfNppN, optGaFra]
iynorm = 1 / Total[iy[[2 ;; 8]]] * iy
Total[iynorm[[2 ;; 8]]]

{0.96847, 0.018695, 0.0105774, 0.000764092, 0.00120184, 0.000266895, 0.0000235044,
  7.3612 × 10-7, 0.965355, 0.000584142, 2.86171 × 10-20, -4.59726 × 10-112}

{30.7163, 0.592937, 0.335477, 0.0242342, 0.038118, 0.00846493, 0.000745473,
  0.000023347, 30.6175, 0.0185268, 9.07628 × 10-19, -1.45808 × 10-110}

1.

```

```

plotiy = Partition[Riffle[normOleg80, iynorm[[2 ;; 8]]], 2]
{{0.604006, 0.592937}, {0.287434, 0.335477},
 {0.0722227, 0.0242342}, {0.0271552, 0.038118},
 {0.00918191, 0.00846493}, {0., 0.000745473}, {0., 0.000023347}}

BarChart[plotiy, PlotRange → {-0.1, 0.9},
  ChartLabels → {Placed[{"N +", "N 2+", "N 3+", "N 4+", "N 5+", "N 6+", "N 7+"}, Below],
    Placed[{}, Above]},
  ChartLegends → Placed[{"Expt.", "γfrag"}, Top],
  ChartStyle → {Black, Red}, AxesLabel → {"", "Ỹ(ω)"},
  AxesStyle → {{Arrowheads[Automatic], AbsoluteThickness[0.6]},
    {Arrowheads[Automatic], AbsoluteThickness[0.6]}},
  LabelStyle → {FontFamily → "Arial"},
  PlotLabel → {damp, optGaFra / gammaFrag,
    (iynorm[[2 ;; 8]] - normOleg80).Table[i, {i, 1, 7}]]}

```

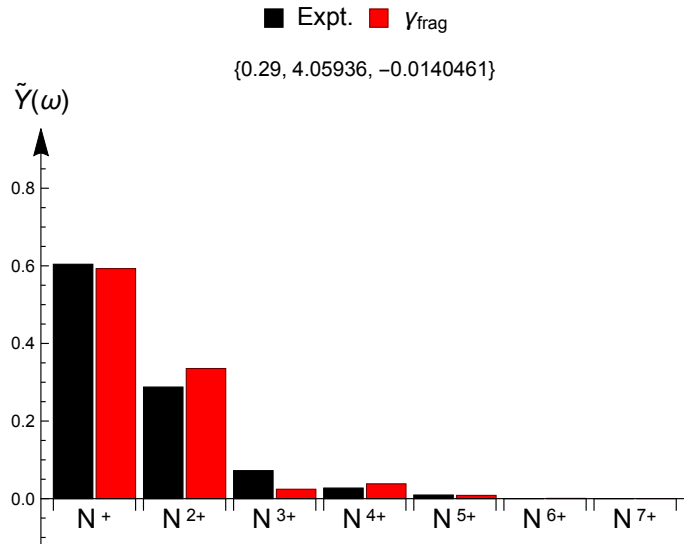

### 0.30

damp := 0.30

```

iy = dsionyieldcrateranalysisparam[damp * 0.26 * MilliJouleToHartree, photonenergy,
  tauX, nintdata, True, True, 1 / 1000, optfNppN, 1 - optfNppN, optGaFra]
iynorm = 1 / Total[iy[[2 ;; 8]]] * iy
Total[iynorm[[2 ;; 8]]]

{0.967688, 0.0189592, 0.0109289, 0.000809111, 0.0012914, 0.000295516,
  0.0000269806,  $8.72557 \times 10^{-7}$ , 0.96453, 0.000591681,  $2.90718 \times 10^{-20}$ ,  $1.57892 \times 10^{-113}$ }

{29.9483, 0.586754, 0.33823, 0.0250406, 0.0399668, 0.00914574, 0.000835005,
  0.0000270042, 29.8506, 0.0183115,  $8.99725 \times 10^{-19}$ ,  $4.88648 \times 10^{-112}$ }

1.

```

```

plotiy = Partition[Riffle[normOleg80, iynorm[[2 ;; 8]]], 2]
{{0.604006, 0.586754}, {0.287434, 0.33823},
 {0.0722227, 0.0250406}, {0.0271552, 0.0399668},
 {0.00918191, 0.00914574}, {0., 0.000835005}, {0., 0.0000270042}}

BarChart[plotiy, PlotRange → {-0.1, 0.9},
  ChartLabels → {Placed[{"N +", "N 2+", "N 3+", "N 4+", "N 5+", "N 6+", "N 7+"}, Below],
    Placed[{}, Above]},
  ChartLegends → Placed[{"Expt.", "γfrag"}, Top],
  ChartStyle → {Black, Red}, AxesLabel → {"", "Ỹ(ω)"},
  AxesStyle → {{Arrowheads[Automatic], AbsoluteThickness[0.6]},
    {Arrowheads[Automatic], AbsoluteThickness[0.6]}},
  LabelStyle → {FontFamily → "Arial"},
  PlotLabel → {damp, optGaFra / gammaFrag,
    (iynorm[[2 ;; 8]] - normOleg80).Table[i, {i, 1, 7}]]}

```

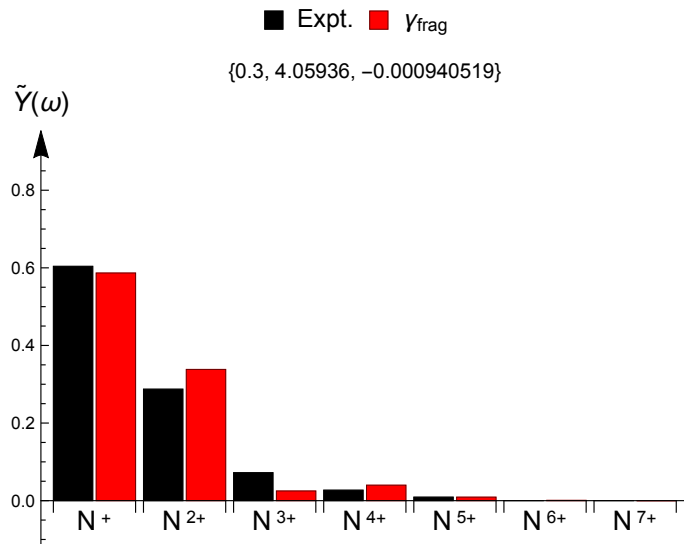

### 0.31

```
damp := 0.31
```



```

iy = dsionyielddcrateranalysisparam[damp * 0.26 * MilliJouleToHartree, photonenergy,
  tauX, nintdata, True, True, 1 / 1000, optfNppN, 1 - optfNppN, optGaFra]
iynorm = 1 / Total[iy[[2 ;; 8]]] * iy
Total[iynorm[[2 ;; 8]]]

{0.96692, 0.0192098, 0.0112741, 0.000854669, 0.0013833, 0.000325896, 0.0000308131,
  1.02802 × 10-6, 0.963722, 0.000598795, 2.94536 × 10-20, 4.49584 × 10-113}

{29.2301, 0.580713, 0.340818, 0.0258367, 0.0418172, 0.00985187, 0.000931482,
  0.0000310771, 29.1334, 0.0181016, 8.90383 × 10-19, 1.35909 × 10-111}

1.

```

```

plotiy = Partition[Riffle[normOleg80, iynorm[[2 ;; 8]]], 2]
{{0.604006, 0.580713}, {0.287434, 0.340818},
 {0.0722227, 0.0258367}, {0.0271552, 0.0418172},
 {0.00918191, 0.00985187}, {0., 0.000931482}, {0., 0.0000310771}}

BarChart[plotiy, PlotRange → {-0.1, 0.9},
  ChartLabels → {Placed[{"N +", "N 2+", "N 3+", "N 4+", "N 5+", "N 6+", "N 7+"}, Below],
    Placed[{}, Above]},
  ChartLegends → Placed[{"Expt.", "γfrag"}, Top],
  ChartStyle → {Black, Red}, AxesLabel → {"", "Ỹ(ω)"},
  AxesStyle → {{Arrowheads[Automatic], AbsoluteThickness[0.6]},
    {Arrowheads[Automatic], AbsoluteThickness[0.6]}},
  LabelStyle → {FontFamily → "Arial"},
  PlotLabel → {damp, optGaFra / gammaFrag,
    (iynorm[[2 ;; 8]] - normOleg80).Table[i, {i, 1, 7}]]}

```

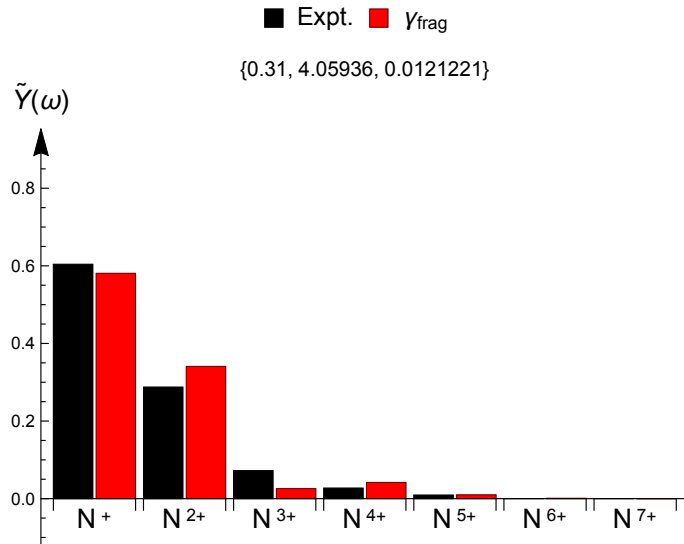

## 0.32

```
damp := 0.32
```

```

iy = dsionyieldcrateranalysisparam[damp * 0.26 * MilliJouleToHartree, photonenergy,
  tauX, nintdata, True, True, 1 / 1000, optfNppN, 1 - optfNppN, optGaFra]
iynorm = 1 / Total[iy[[2 ;; 8]]] * iy
Total[iynorm[[2 ;; 8]]]

{0.966167, 0.0194477, 0.0116131, 0.000900703, 0.0014774, 0.00035805, 0.0000350217,
  1.2043 × 10-6, 0.962931, 0.00060551, 2.96457 × 10-20, 2.87273 × 10-114}

{28.5568, 0.574811, 0.343246, 0.0266219, 0.0436671, 0.0105828, 0.00103513,
  0.0000355953, 28.4612, 0.0178969, 8.76232 × 10-19, 8.49086 × 10-113}

1.

```

```

plotiy = Partition[Riffle[normOleg80, iynorm[[2 ;; 8]]], 2]
{{0.604006, 0.574811}, {0.287434, 0.343246},
 {0.0722227, 0.0266219}, {0.0271552, 0.0436671},
 {0.00918191, 0.0105828}, {0., 0.00103513}, {0., 0.0000355953}}

BarChart[plotiy, PlotRange → {-0.1, 0.9},
  ChartLabels → {Placed[{"N+", "N2+", "N3+", "N4+", "N5+", "N6+", "N7+"}, Below],
    Placed[{}, Above]},
  ChartLegends → Placed[{"Expt.", "γfrag"}, Top],
  ChartStyle → {Black, Red}, AxesLabel → {"", "Ỹ(ω)"},
  AxesStyle → {{Arrowheads[Automatic], AbsoluteThickness[0.6]},
    {Arrowheads[Automatic], AbsoluteThickness[0.6]}},
  LabelStyle → {FontFamily → "Arial"},
  PlotLabel → {damp, optGaFra / gammaFrag,
    (iynorm[[2 ;; 8]] - normOleg80).Table[i, {i, 1, 7}]]}

■ Expt. ■ γfrag
{0.32, 4.05936, 0.0251393}

```

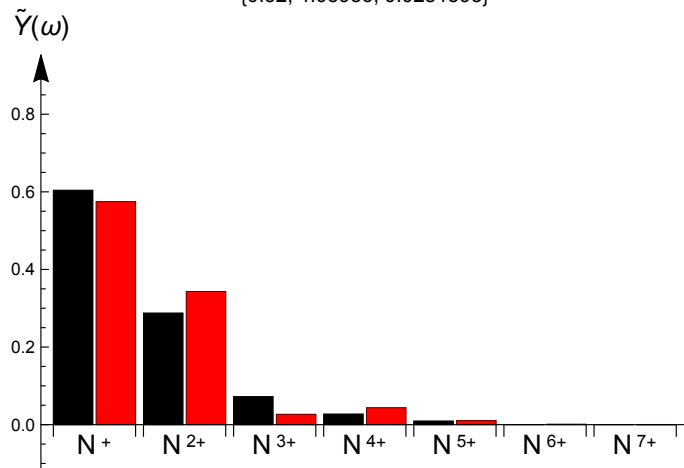

## Pulse energy for a 80 fs pulse with 80 fs fragmentation rate

```

tauX := 80 / t0ToFemtoSecond
optent := 12.000000
optGaFra := optent * gammaFrag

```

## 0.30

```
damp := 0.30
```

```
iy = dsionyieldcrateranalysisparam[damp * 0.26 * MilliJouleToHartree, photonenergy,  
tauX, nintdata, True, True, 1 / 1000, optfNppN, 1 - optfNppN, optGaFra]
```

```
iynorm = 1 / Total[iy[[2 ;; 8]]] * iy
```

```
Total[iynorm[[2 ;; 8]]]
```

```
{0.967779, 0.0194633, 0.00976408, 0.00134806,  
0.00125066, 0.000359958, 0.0000337345, 1.26099 × 10-6,  
0.96453, 0.000591681, 1.17732 × 10-54, -2.66479 × 10-116}
```

```
{30.0356, 0.604055, 0.303034, 0.041838, 0.0388149, 0.0111715, 0.00104697,  
0.0000391357, 29.9348, 0.0183632, 3.65388 × 10-53, -8.27036 × 10-115}
```

```
1.
```

```
plotiy = Partition[Riffle[normOleg80, iynorm[[2 ;; 8]]], 2]
```

```
{{0.604006, 0.604055}, {0.287434, 0.303034},  
{0.0722227, 0.041838}, {0.0271552, 0.0388149},  
{0.00918191, 0.0111715}, {0., 0.00104697}, {0., 0.0000391357}}
```

```
BarChart[plotiy, PlotRange → {-0.1, 0.9},
```

```
ChartLabels → {Placed[{"N +", "N 2+", "N 3+", "N 4+", "N 5+", "N 6+", "N 7+"}, Below],  
Placed[{}, Above]},
```

```
ChartLegends → Placed[{"Expt.", "γfrag"}, Top],
```

```
ChartStyle → {Black, Red}, AxesLabel → {"", "Ỹ(ω)",
```

```
AxesStyle → {{Arrowheads[Automatic], AbsoluteThickness[0.6]},  
{Arrowheads[Automatic], AbsoluteThickness[0.6]}},
```

```
LabelStyle → {FontFamily → "Arial"},
```

```
PlotLabel → {damp, optGaFra / gammaFrag,  
(iynorm[[2 ;; 8]] - normOleg80).Table[i, {i, 1, 7}]]}
```

■ Expt. ■ γ<sub>frag</sub>

{0.3, 12., 0.00323831}

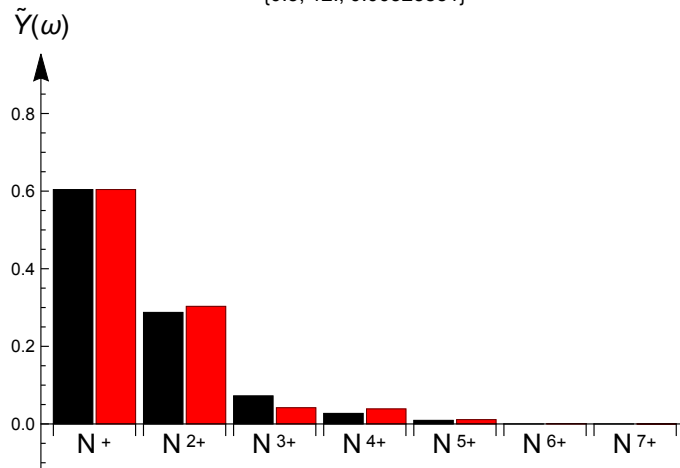

Pulse energy for a 7 fs pulse with 280 fs fragmentation

## rate

```
tauX := 7 / t0ToFemtoSecond
optent := 4.059357
optGaFra := optent * gammaFrag
```

## 0.12

```
damp := 0.12
```

```
iy = dsionyieldcrateranalysisparam[damp * 0.26 * MilliJouleToHartree, photonenergy,
  tauX, nintdata, True, True, 1 / 1000, optfNppN, 1 - optfNppN, optGaFra]
```

```
inyorm = 1 / Total[iy[[2 ;; 8]]] * iy
```

```
Total[inyorm[[2 ;; 8]]]
```

```
{0.984496, 0.0112916, 0.00400759, 0.000140454,
  0.0000576454,  $6.62618 \times 10^{-6}$ ,  $1.02596 \times 10^{-7}$ ,  $3.37403 \times 10^{-10}$ ,
   $0.982596$ ,  $0.000359602$ ,  $1.7696 \times 10^{-20}$ ,  $3.87294 \times 10^{-167}$ }
```

```
{63.4995, 0.728301, 0.258488, 0.00905924, 0.0037181, 0.000427385,  $6.61737 \times 10^{-6}$ ,
   $2.17624 \times 10^{-8}$ , 63.377, 0.0231942,  $1.14138 \times 10^{-18}$ ,  $2.49803 \times 10^{-165}$ }
```

```
1.
```

```
plotiy = Partition[Riffle[normOleg7, inyorm[[2 ;; 8]]], 2]
```

```
{ {0.694746, 0.728301}, {0.275684, 0.258488},
  {0.0293036, 0.00905924}, {0.000266625, 0.0037181},
  {0., 0.000427385}, {0.,  $6.61737 \times 10^{-6}$ }, {0.,  $2.17624 \times 10^{-8}$ }}
```

```
BarChart[plotiy, PlotRange → {-0.1, 0.9},
  ChartLabels → {Placed[{"N +", "N 2+", "N 3+", "N 4+", "N 5+", "N 6+", "N 7+"}, Below],
    Placed[{}, Above]},
  ChartLegends → Placed[{"Expt.", "γfrag"}, Top],
  ChartStyle → {Black, Red}, AxesLabel → {"", "Ỹ(ω)",
  AxesStyle → {{Arrowheads[Automatic], AbsoluteThickness[0.6]},
    {Arrowheads[Automatic], AbsoluteThickness[0.6]}},
  LabelStyle → {FontFamily → "Arial"},
  PlotLabel → {damp, optGaFra / gammaFrag,
    (iynorm[[2 ;; 8]] - normOleg7).Table[i, {i, 1, 7}]]]
```

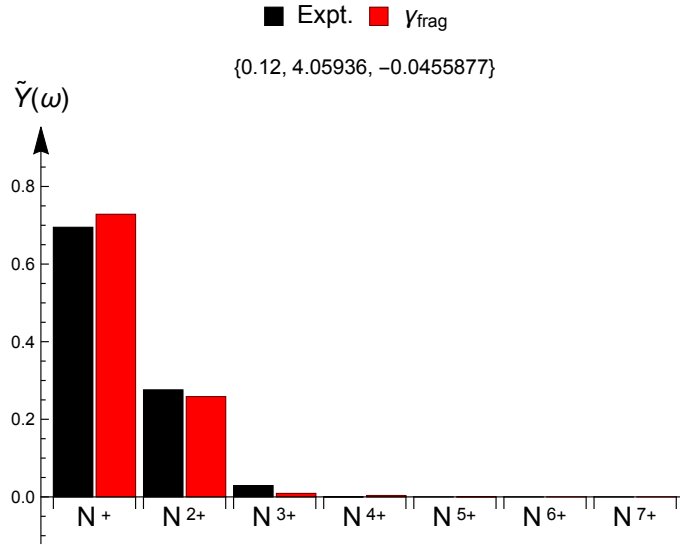

### 0.13

```
damp := 0.13

iy = dsionyieldcrateranalysisparam[damp * 0.26 * MilliJouleToHartree, photonenergy,
  tauX, nintdata, True, True, 1 / 1000, optfNppN, 1 - optfNppN, optGaFra]
iynorm = 1 / Total[iy[[2 ;; 8]]] * iy
Total[iynorm[[2 ;; 8]]]

{0.983387, 0.0119488, 0.00441056, 0.000172926,
  0.0000715362, 8.88622 × 10-6, 1.4948 × 10-7, 5.3324 × 10-10,
  0.981378, 0.000379768, 1.87066 × 10-20, -1.10683 × 10-168}

{59.1945, 0.719249, 0.265492, 0.0104092, 0.00430608, 0.000534901, 8.99789 × 10-6,
  3.20981 × 10-8, 59.0735, 0.0228599, 1.12604 × 10-18, -6.66248 × 10-167}

1.

plotiy = Partition[Riffle[normOleg7, iynorm[[2 ;; 8]]], 2]

{{0.694746, 0.719249}, {0.275684, 0.265492},
  {0.0293036, 0.0104092}, {0.000266625, 0.00430608},
  {0., 0.000534901}, {0., 8.99789 × 10-6}, {0., 3.20981 × 10-8}}
```

```
BarChart[plotiy, PlotRange → {-0.1, 0.9},
  ChartLabels → {Placed[{"N +", "N 2+", "N 3+", "N 4+", "N 5+", "N 6+", "N 7+"}, Below],
    Placed[{}, Above]},
  ChartLegends → Placed[{"Expt.", "γfrag"}, Top],
  ChartStyle → {Black, Red}, AxesLabel → {"", "Ỹ(ω)",
  AxesStyle → {{Arrowheads[Automatic], AbsoluteThickness[0.6]},
    {Arrowheads[Automatic], AbsoluteThickness[0.6]}},
  LabelStyle → {FontFamily → "Arial"},
  PlotLabel → {damp, optGaFra / gammaFrag,
    (iynorm[[2 ;; 8]] - normOleg7).Table[i, {i, 1, 7}]]]
```

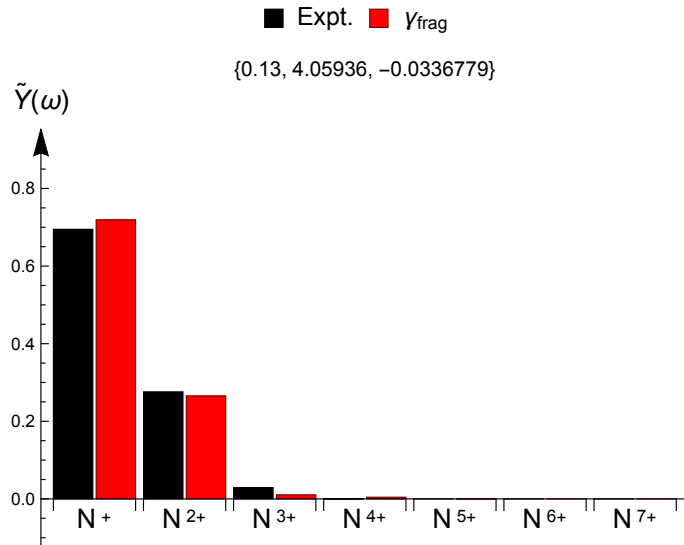

## 0.14

damp := 0.14

```
iy = dsionyieldcrateranalysisparam[damp * 0.26 * MilliJouleToHartree, photonenergy,
  tauX, nintdata, True, True, 1 / 1000, optfNppN, 1 - optfNppN, optGaFra]
```

```
iynorm = 1 / Total[iy[[2 ;; 8]]] * iy
```

```
Total[iynorm[[2 ;; 8]]]
```

```
{0.982303, 0.0125723, 0.00481684, 0.000209221, 0.0000872229, 0.0000116408,
  2.11482 × 10-7, 8.13507 × 10-10, 0.98019, 0.0003988, 1.96619 × 10-20, -7.1754 × 10-166}
```

```
{55.5054, 0.710402, 0.272177, 0.0118221, 0.00492857, 0.000657768,
  0.0000119499, 4.59676 × 10-8, 55.386, 0.0225344, 1.111 × 10-18, -4.05449 × 10-164}
```

1.

```
plotiy = Partition[Riffle[normOleg7, iynorm[[2 ;; 8]]], 2]
```

```
{{0.694746, 0.710402}, {0.275684, 0.272177},
  {0.0293036, 0.0118221}, {0.000266625, 0.00492857},
  {0., 0.000657768}, {0., 0.0000119499}, {0., 4.59676 × 10-8}}
```

```
BarChart[plotiy, PlotRange → {-0.1, 0.9},
  ChartLabels → {Placed[{"N +", "N 2+", "N 3+", "N 4+", "N 5+", "N 6+", "N 7+"}, Below],
    Placed[{}, Above]},
  ChartLegends → Placed[{"Expt.", "γfrag"}, Top],
  ChartStyle → {Black, Red}, AxesLabel → {"", "Ỹ(ω)"},
  AxesStyle → {{Arrowheads[Automatic], AbsoluteThickness[0.6]},
    {Arrowheads[Automatic], AbsoluteThickness[0.6]}},
  LabelStyle → {FontFamily → "Arial"},
  PlotLabel → {damp, optGaFra / gammaFrag,
    (iynorm[[2 ;; 8]] - normOleg7).Table[i, {i, 1, 7}]]]
```

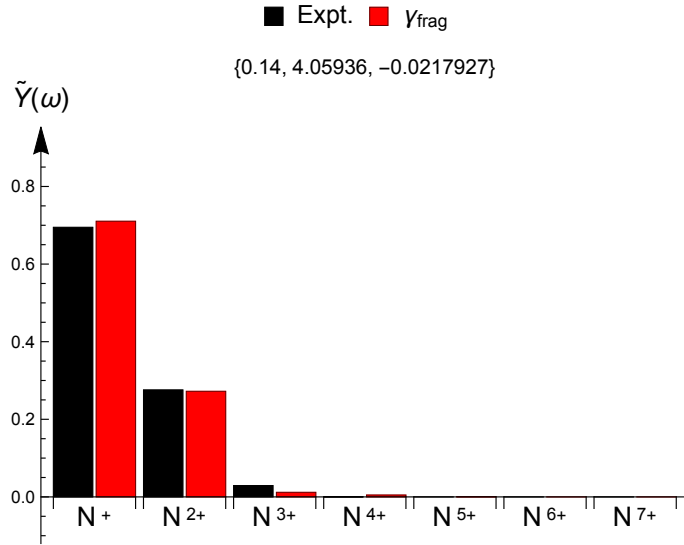

## 0.15

damp := 0.15

```
iy = dsionyieldcrateranalysisparam[damp * 0.26 * MilliJouleToHartree, photonenergy,
  tauX, nintdata, True, True, 1 / 1000, optfNppN, 1 - optfNppN, optGaFra]
```

```
iynorm = 1 / Total[iy[[2 ;; 8]]] * iy
```

```
Total[iynorm[[2 ;; 8]]]
```

```
{0.981242, 0.0131639, 0.00522529, 0.000249355,
  0.000104746, 0.000014944, 2.91716 × 10-7, 1.20387 × 10-9,
  0.979031, 0.000416761, 2.05733 × 10-20, -1.21671 × 10-147}
```

```
{52.3092, 0.701755, 0.278556, 0.0132929, 0.00558392, 0.000796652, 0.0000155511,
  6.41773 × 10-8, 52.1914, 0.0222172, 1.09675 × 10-18, -6.48616 × 10-146}
```

1.

```
plotiy = Partition[Riffle[normOleg7, iynorm[[2 ;; 8]]], 2]
```

```
{{0.694746, 0.701755}, {0.275684, 0.278556},
  {0.0293036, 0.0132929}, {0.000266625, 0.00558392},
  {0., 0.000796652}, {0., 0.0000155511}, {0., 6.41773 × 10-8}}
```

```
BarChart[plotiy, PlotRange → {-0.1, 0.9},
  ChartLabels → {Placed[{"N +", "N 2+", "N 3+", "N 4+", "N 5+", "N 6+", "N 7+"}, Below],
    Placed[{}, Above]},
  ChartLegends → Placed[{"Expt.", "γfrag"}, Top],
  ChartStyle → {Black, Red}, AxesLabel → {"", "Ỹ(ω)"},
  AxesStyle → {{Arrowheads[Automatic], AbsoluteThickness[0.6]},
    {Arrowheads[Automatic], AbsoluteThickness[0.6]}},
  LabelStyle → {FontFamily → "Arial"},
  PlotLabel → {damp, optGaFra / gammaFrag,
    (iynorm[[2 ;; 8]] - normOleg7).Table[i, {i, 1, 7}]]]
```

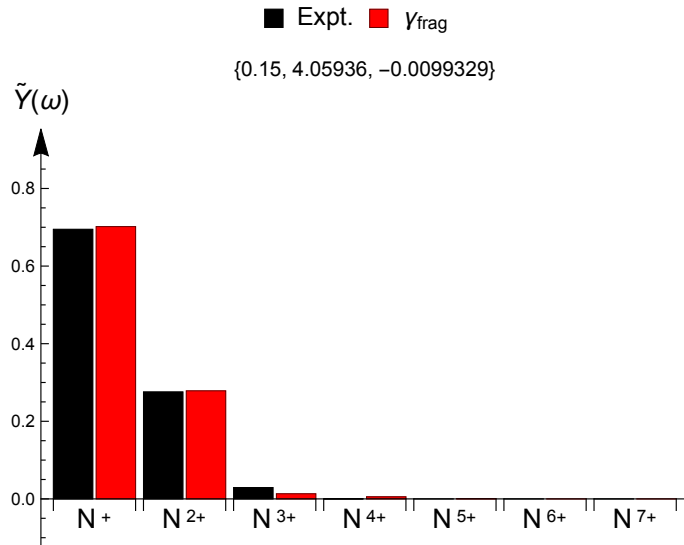

## 0.16

damp := 0.16

```
iy = dsionyieldcrateranalysisparam[damp * 0.26 * MilliJouleToHartree, photonenergy,
  tauX, nintdata, True, True, 1 / 1000, optfNppN, 1 - optfNppN, optGaFra]
```

```
iynorm = 1 / Total[iy[[2 ;; 8]]] * iy
```

```
Total[iynorm[[2 ;; 8]]]
```

```
{0.980203, 0.0137252, 0.00563491, 0.00029332, 0.000124136, 0.0000188496,
  3.93605 × 10-7, 1.73494 × 10-9, 0.9779, 0.000433713, 2.14226 × 10-20, 1.82178 × 10-146}
```

```
{49.5132, 0.693304, 0.284637, 0.0148165, 0.00627051, 0.000952154, 0.0000198823,
  8.76372 × 10-8, 49.3969, 0.0219082, 1.08212 × 10-18, 9.20238 × 10-145}
```

1.

```
plotiy = Partition[Riffle[normOleg7, iynorm[[2 ;; 8]]], 2]
```

```
{{0.694746, 0.693304}, {0.275684, 0.284637},
  {0.0293036, 0.0148165}, {0.000266625, 0.00627051},
  {0., 0.000952154}, {0., 0.0000198823}, {0., 8.76372 × 10-8}}
```



```
BarChart[plotiy, PlotRange → {-0.1, 0.9},
  ChartLabels → {Placed[{"N +", "N 2+", "N 3+", "N 4+", "N 5+", "N 6+", "N 7+"}, Below],
    Placed[{}, Above]},
  ChartLegends → Placed[{"Expt.", "γfrag"}, Top],
  ChartStyle → {Black, Red}, AxesLabel → {"", "Ỹ(ω)",
  AxesStyle → {{Arrowheads[Automatic], AbsoluteThickness[0.6]},
    {Arrowheads[Automatic], AbsoluteThickness[0.6]}},
  LabelStyle → {FontFamily → "Arial"},
  PlotLabel → {damp, optGaFra / gammaFrag,
    (iynorm[[2 ;; 8]] - normOleg7).Table[i, {i, 1, 7}]]]
```

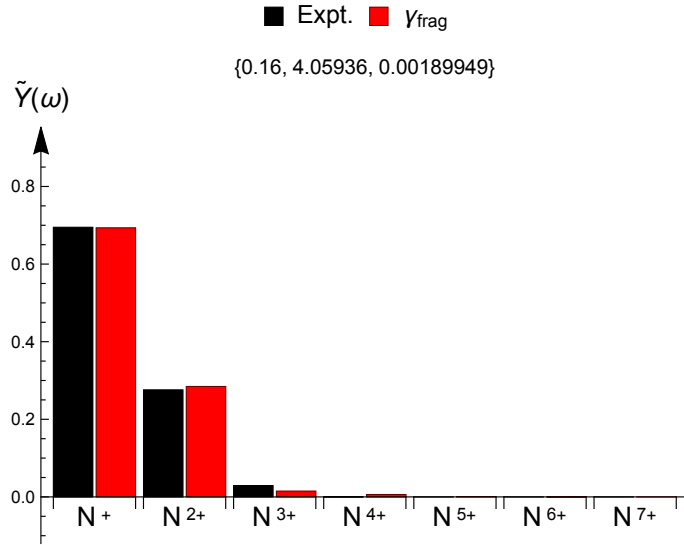

## 0.17

```
damp := 0.17

iy = dsionyieldcrateranalysisparam[damp * 0.26 * MilliJouleToHartree, photonenergy,
  tauX, nintdata, True, True, 1 / 1000, optfNppN, 1 - optfNppN, optGaFra]
iynorm = 1 / Total[iy[[2 ;; 8]]] * iy
Total[iynorm[[2 ;; 8]]]
{0.979187, 0.0142578, 0.00604476, 0.00034109,
  0.000145416, 0.0000234109, 5.20882 × 10-7, 2.44268 × 10-9,
  0.976796, 0.000449711, 2.22473 × 10-20, -2.71305 × 10-142}

{47.0469, 0.685043, 0.290432, 0.0163883, 0.00698679, 0.00112482, 0.0000250268,
  1.17363 × 10-7, 46.9321, 0.0216072, 1.06892 × 10-18, -1.30354 × 10-140}

1.

plotiy = Partition[Riffle[normOleg7, iynorm[[2 ;; 8]]], 2]
{{0.694746, 0.685043}, {0.275684, 0.290432},
  {0.0293036, 0.0163883}, {0.000266625, 0.00698679},
  {0., 0.00112482}, {0., 0.0000250268}, {0., 1.17363 × 10-7}}
```

```

BarChart[plotiy, PlotRange → {-0.1, 0.9},
  ChartLabels → {Placed[{"N +", "N 2+", "N 3+", "N 4+", "N 5+", "N 6+", "N 7+"}, Below],
    Placed[{}, Above]},
  ChartLegends → Placed[{"Expt.", "γfrag"}, Top],
  ChartStyle → {Black, Red}, AxesLabel → {"", "Ỹ(ω)"},
  AxesStyle → {{Arrowheads[Automatic], AbsoluteThickness[0.6]},
    {Arrowheads[Automatic], AbsoluteThickness[0.6]}},
  LabelStyle → {FontFamily → "Arial"},
  PlotLabel → {damp, optGaFra / gammaFrag,
    (iynorm[[2 ;; 8]] - normOleg7).Table[i, {i, 1, 7}]]}

```

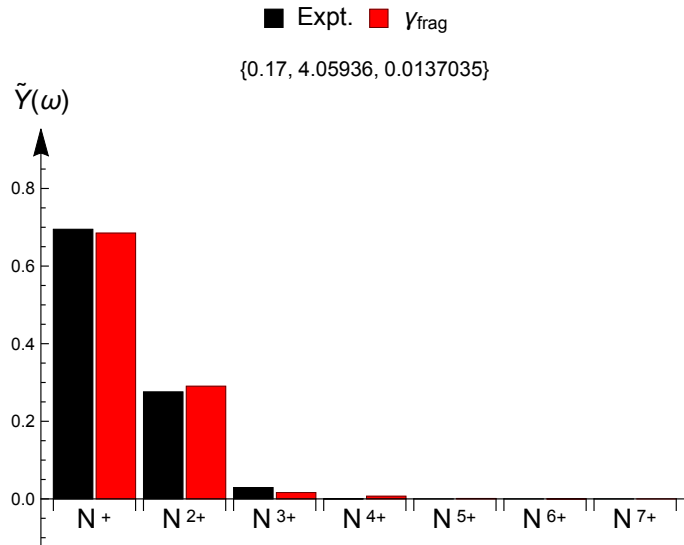

## 0.18

damp := 0.18

```

iy = dsionyieldcrateranalysisparam[damp * 0.26 * MilliJouleToHartree, photonenergy,
  tauX, nintdata, True, True, 1 / 1000, optfNppN, 1 - optfNppN, optGaFra]

```

```

iynorm = 1 / Total[iy[[2 ;; 8]]] * iy

```

```

Total[iynorm[[2 ;; 8]]]

```

```

{0.978192, 0.0147631, 0.00645401, 0.00039262,
 0.0001686, 0.0000286804, 6.77578 × 10-7, 3.36889 × 10-9,
 0.975718, 0.00046481, 2.30149 × 10-20, -2.49785 × 10-143}

```

```

{44.8553, 0.676968, 0.295951, 0.0180037, 0.00773121, 0.00131515, 0.0000310706,
 1.54482 × 10-7, 44.7419, 0.021314, 1.05535 × 10-18, -1.1454 × 10-141}

```

1.

```

plotiy = Partition[Riffle[normOleg7, iynorm[[2 ;; 8]]], 2]

```

```

{{0.694746, 0.676968}, {0.275684, 0.295951},
 {0.0293036, 0.0180037}, {0.000266625, 0.00773121},
 {0., 0.00131515}, {0., 0.0000310706}, {0., 1.54482 × 10-7}}

```

```
BarChart[plotiy, PlotRange → {-0.1, 0.9},
  ChartLabels → {Placed[{"N +", "N 2+", "N 3+", "N 4+", "N 5+", "N 6+", "N 7+"}, Below],
    Placed[{}, Above]},
  ChartLegends → Placed[{"Expt.", "γfrag"}, Top],
  ChartStyle → {Black, Red}, AxesLabel → {"", "Ỹ(ω)"},
  AxesStyle → {{Arrowheads[Automatic], AbsoluteThickness[0.6]},
    {Arrowheads[Automatic], AbsoluteThickness[0.6]}},
  LabelStyle → {FontFamily → "Arial"},
  PlotLabel → {damp, optGaFra / gammaFrag,
    (iynorm[[2 ;; 8]] - normOleg7).Table[i, {i, 1, 7}]]]
```

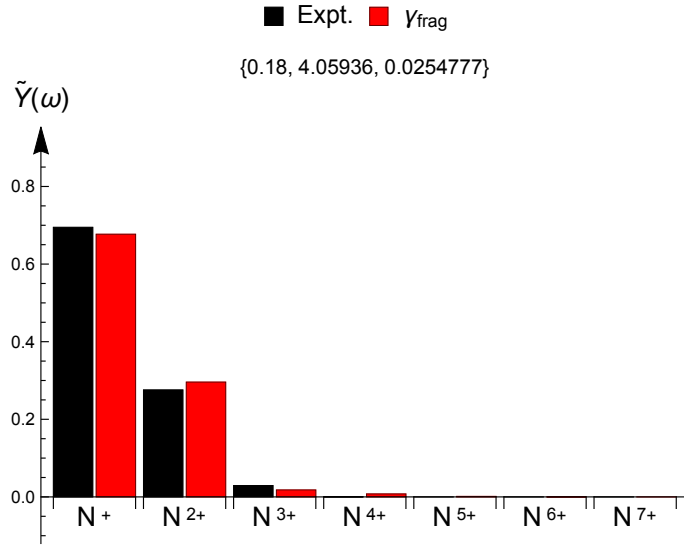

## Pulse energy for a 7 fs pulse with 80 fs fragmentation rate

```
tauX := 7 / t0ToFemtoSecond
optent := 12.000000
optGaFra := optent * gammaFrag
```

### 0.12

```
damp := 0.12

iy = dsionyieldcrateranalysisparam[damp * 0.26 * MilliJouleToHartree, photonenergy,
  tauX, nintdata, True, True, 1 / 1000, optfNppN, 1 - optfNppN, optGaFra]
iynorm = 1 / Total[iy[[2 ;; 8]]] * iy
Total[iynorm[[2 ;; 8]]]
{0.984497, 0.0112977, 0.00399335, 0.000146393,
  0.0000584917, 6.84446 × 10-6, 1.0629 × 10-7, 3.51513 × 10-10,
  0.982596, 0.000359602, 4.11943 × 10-55, -3.44731 × 10-170}

{63.5041, 0.728748, 0.257588, 0.00944293, 0.00377296, 0.000441496, 6.85612 × 10-6,
  2.2674 × 10-8, 63.3815, 0.0231958, 2.6572 × 10-53, -2.22366 × 10-168}
```

1.

```

plotiy = Partition[Riffle[normOleg7, iynorm[[2 ;; 8]]], 2]
{
  {0.694746, 0.728748}, {0.275684, 0.257588},
  {0.0293036, 0.00944293}, {0.000266625, 0.00377296},
  {0., 0.000441496}, {0.,  $6.85612 \times 10^{-6}$ }, {0.,  $2.2674 \times 10^{-8}$ }
}

BarChart[plotiy, PlotRange → {-0.1, 0.9},
  ChartLabels → {Placed[{"N +", "N 2+", "N 3+", "N 4+", "N 5+", "N 6+", "N 7+"}, Below],
    Placed[{}, Above]},
  ChartLegends → Placed[{"Expt.", " $\gamma_{\text{frag}}$ "}, Top],
  ChartStyle → {Black, Red}, AxesLabel → {"", " $\tilde{Y}(\omega)$ "},
  AxesStyle → {{Arrowheads[Automatic], AbsoluteThickness[0.6]},
    {Arrowheads[Automatic], AbsoluteThickness[0.6]}},
  LabelStyle → {FontFamily → "Arial"},
  PlotLabel → {damp, optGaFra / gammaFrag,
    (iynorm[[2 ;; 8]] - normOleg7).Table[i, {i, 1, 7}]}]

```

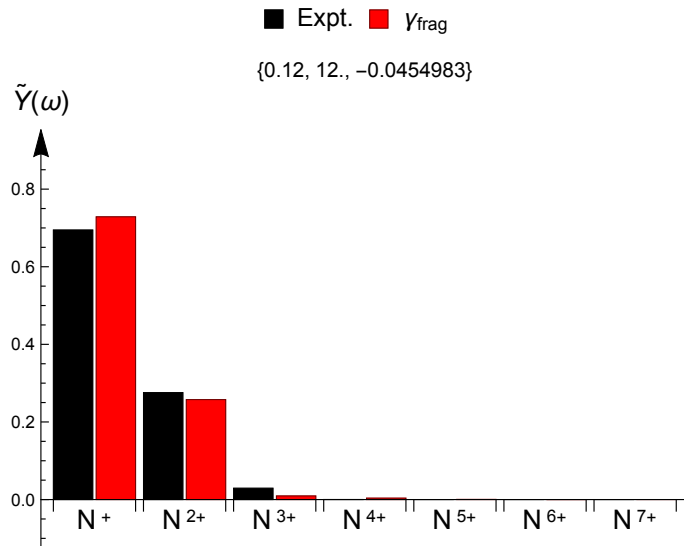

## 0.13

```

damp := 0.13

iy = dsionyieldcrateranalysisparam[damp * 0.26 * MilliJouleToHartree, photonenergy,
  tauX, nintdata, True, True, 1 / 1000, optfNppN, 1 - optfNppN, optGaFra]
iynorm = 1 / Total[iy[[2 ;; 8]]] * iy
Total[iynorm[[2 ;; 8]]]
{
  0.983388, 0.0119557, 0.00439439, 0.000179657,
  0.0000724772,  $9.1542 \times 10^{-6}$ ,  $1.54416 \times 10^{-7}$ ,  $5.53737 \times 10^{-10}$ ,
  0.981378, 0.000379768,  $4.7529 \times 10^{-55}$ ,  $1.43637 \times 10^{-162}$ 
}

{
  59.199, 0.719723, 0.264538, 0.0108152, 0.00436306, 0.000551074,
   $9.29568 \times 10^{-6}$ ,  $3.33344 \times 10^{-8}$ , 59.078, 0.0228617,  $2.8612 \times 10^{-53}$ ,  $8.64679 \times 10^{-161}$ 
}

```

1.

```
plotiy = Partition[Riffle[normOleg7, iynorm[[2 ;; 8]]], 2]
```

```
{0.694746, 0.719723}, {0.275684, 0.264538},  
{0.0293036, 0.0108152}, {0.000266625, 0.00436306},  
{0., 0.000551074}, {0.,  $9.29568 \times 10^{-6}$ }, {0.,  $3.33344 \times 10^{-8}$ }
```

```
BarChart[plotiy, PlotRange → {-0.1, 0.9},  
  ChartLabels → {Placed[{"N +", "N 2+", "N 3+", "N 4+", "N 5+", "N 6+", "N 7+"}, Below],  
    Placed[{}, Above]},  
  ChartLegends → Placed[{"Expt.", " $\gamma_{\text{frag}}$ "}, Top],  
  ChartStyle → {Black, Red}, AxesLabel → {"", " $\tilde{Y}(\omega)$ "},  
  AxesStyle → {{Arrowheads[Automatic], AbsoluteThickness[0.6]},  
    {Arrowheads[Automatic], AbsoluteThickness[0.6]}},  
  LabelStyle → {FontFamily → "Arial"},  
  PlotLabel → {damp, optGaFra / gammaFrag,  
    (iynorm[[2 ;; 8]] - normOleg7).Table[i, {i, 1, 7}]}]
```

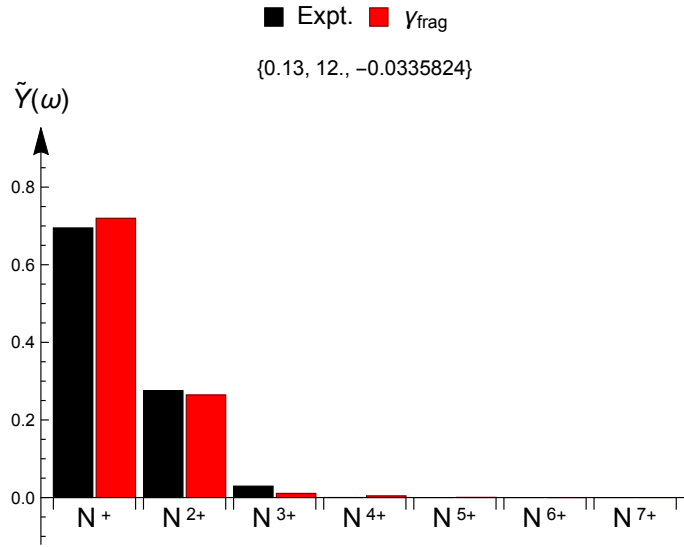

## 0.14

```
damp := 0.14
```

```
iy = dsionyieldcrateranalysisparam[damp * 0.26 * MilliJouleToHartree, photonenergy,  
  tauX, nintdata, True, True, 1 / 1000, optfNppN, 1 - optfNppN, optGaFra]
```

```
iynorm = 1 / Total[iy[[2 ;; 8]]] * iy
```

```
Total[iynorm[[2 ;; 8]]]
```

```
{0.982304, 0.0125801, 0.00479868, 0.000216763, 0.0000882564, 0.000011964,  
   $2.17922 \times 10^{-7}$ ,  $8.42416 \times 10^{-10}$ , 0.98019, 0.0003988,  $4.91967 \times 10^{-55}$ ,  $5.93138 \times 10^{-156}$ }
```

```
{55.5099, 0.710902, 0.271173, 0.0122493, 0.00498736, 0.000676086, 0.0000123148,  
   $4.76048 \times 10^{-8}$ , 55.3905, 0.0225362,  $2.7801 \times 10^{-53}$ ,  $3.35182 \times 10^{-154}$ }
```

1.

```
plotiy = Partition[Riffle[normOleg7, iynorm[[2 ;; 8]]], 2]
```

```
{0.694746, 0.710902}, {0.275684, 0.271173},  
{0.0293036, 0.0122493}, {0.000266625, 0.00498736},  
{0., 0.000676086}, {0., 0.0000123148}, {0.,  $4.76048 \times 10^{-8}$ }
```

```
BarChart[plotiy, PlotRange → {-0.1, 0.9},
  ChartLabels → {Placed[{"N +", "N 2+", "N 3+", "N 4+", "N 5+", "N 6+", "N 7+"}, Below],
    Placed[{}, Above]},
  ChartLegends → Placed[{"Expt.", "γfrag"}, Top],
  ChartStyle → {Black, Red}, AxesLabel → {"", "Ỹ(ω)"},
  AxesStyle → {{Arrowheads[Automatic], AbsoluteThickness[0.6]},
    {Arrowheads[Automatic], AbsoluteThickness[0.6]}},
  LabelStyle → {FontFamily → "Arial"},
  PlotLabel → {damp, optGaFra / gammaFrag,
    (iynorm[[2 ;; 8]] - normOleg7).Table[i, {i, 1, 7}]]]
```

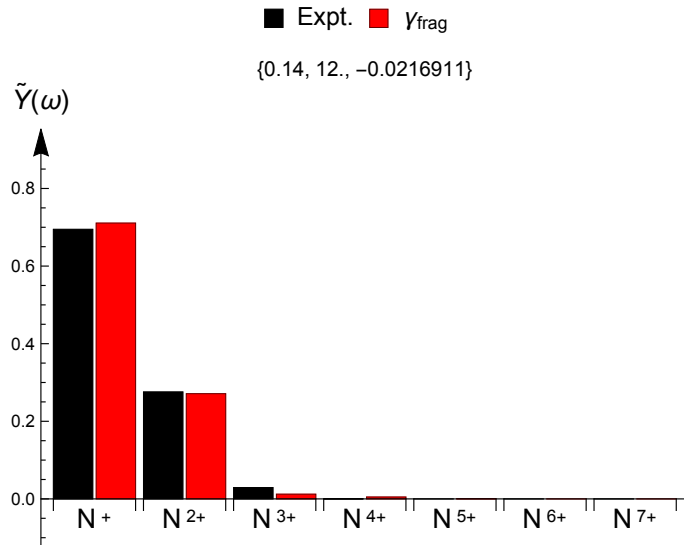

## 0.15

damp := 0.15

```
iy = dsionyieldcrateranalysisparam[damp * 0.26 * MilliJouleToHartree, photonenergy,
  tauX, nintdata, True, True, 1 / 1000, optfNppN, 1 - optfNppN, optGaFra]
```

```
iynorm = 1 / Total[iy[[2 ;; 8]]] * iy
```

```
Total[iynorm[[2 ;; 8]]]
```

```
{0.981243, 0.0131726, 0.00520511, 0.000257721,
  0.000105869, 0.0000153279, 2.99949 × 10-7, 1.24362 × 10-9,
  0.979031, 0.000416761, 5.71067 × 10-55, 6.61041 × 10-159}
```

```
{52.3137, 0.702279, 0.277503, 0.0137401, 0.00564426, 0.000817188, 0.0000159914,
  6.63017 × 10-8, 52.1957, 0.0222191, 3.04457 × 10-53, 3.52425 × 10-157}
```

1.

```
plotiy = Partition[Riffle[normOleg7, iynorm[[2 ;; 8]]], 2]
```

```
{{0.694746, 0.702279}, {0.275684, 0.277503},
  {0.0293036, 0.0137401}, {0.000266625, 0.00564426},
  {0., 0.000817188}, {0., 0.0000159914}, {0., 6.63017 × 10-8}}
```

```
BarChart[plotiy, PlotRange → {-0.1, 0.9},
  ChartLabels → {Placed[{"N +", "N 2+", "N 3+", "N 4+", "N 5+", "N 6+", "N 7+"}, Below],
    Placed[{}, Above]},
  ChartLegends → Placed[{"Expt.", "γfrag"}, Top],
  ChartStyle → {Black, Red}, AxesLabel → {"", "Ỹ(ω)",
  AxesStyle → {{Arrowheads[Automatic], AbsoluteThickness[0.6]},
    {Arrowheads[Automatic], AbsoluteThickness[0.6]}},
  LabelStyle → {FontFamily → "Arial"},
  PlotLabel → {damp, optGaFra / gammaFrag,
    (iynorm[[2 ;; 8]] - normOleg7).Table[i, {i, 1, 7}]]]
```

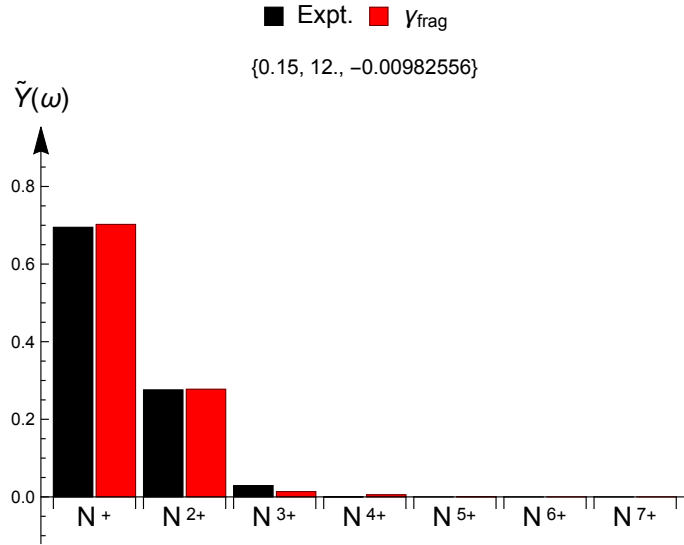

## 0.16

```
damp := 0.16

iy = dsionyieldcrateranalysisparam[damp * 0.26 * MilliJouleToHartree, photonenergy,
  tauX, nintdata, True, True, 1 / 1000, optfNppN, 1 - optfNppN, optGaFra]
iynorm = 1 / Total[iy[[2 ;; 8]]] * iy
Total[iynorm[[2 ;; 8]]]

{0.980205, 0.0137348, 0.00561268, 0.00030252, 0.000125345, 0.0000192997,
  4.03946 × 10-7, 1.78838 × 10-9, 0.9779, 0.000433713, 5.36958 × 10-55, 1.19451 × 10-159}

{49.5177, 0.69385, 0.283539, 0.0152826, 0.00633214, 0.000974974, 0.0000204064,
  9.03447 × 10-8, 49.4012, 0.0219102, 2.71259 × 10-53, 6.03437 × 10-158}

1.

plotiy = Partition[Riffle[normOleg7, iynorm[[2 ;; 8]]], 2]

{{0.694746, 0.69385}, {0.275684, 0.283539},
  {0.0293036, 0.0152826}, {0.000266625, 0.00633214},
  {0., 0.000974974}, {0., 0.0000204064}, {0., 9.03447 × 10-8}}
```

```
BarChart[plotiy, PlotRange → {-0.1, 0.9},
  ChartLabels → {Placed[{"N +", "N 2+", "N 3+", "N 4+", "N 5+", "N 6+", "N 7+"}, Below],
    Placed[{}, Above]},
  ChartLegends → Placed[{"Expt.", "γfrag"}, Top],
  ChartStyle → {Black, Red}, AxesLabel → {"", "Ỹ(ω)",
  AxesStyle → {{Arrowheads[Automatic], AbsoluteThickness[0.6]},
    {Arrowheads[Automatic], AbsoluteThickness[0.6]}},
  LabelStyle → {FontFamily → "Arial"},
  PlotLabel → {damp, optGaFra / gammaFrag,
    (iynorm[[2 ;; 8]] - normOleg7).Table[i, {i, 1, 7}]]]
```

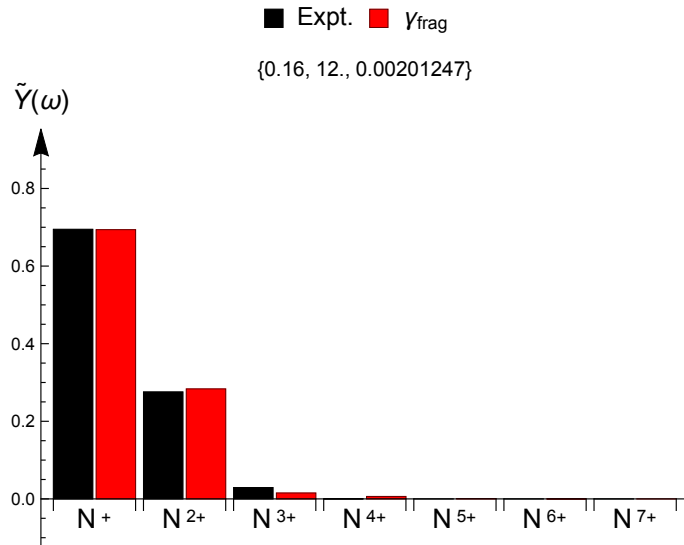

## 0.17

damp := 0.17

```
iy = dsionyieldcrateranalysisparam[damp * 0.26 * MilliJouleToHartree, photonenergy,
  tauX, nintdata, True, True, 1 / 1000, optfNppN, 1 - optfNppN, optGaFra]
```

```
iynorm = 1 / Total[iy[[2 ;; 8]]] * iy
```

```
Total[iynorm[[2 ;; 8]]]
```

```
{0.979189, 0.0142683, 0.00602046, 0.00035113,
  0.000146707, 0.0000239324, 5.3367 × 10-7, 2.51315 × 10-9,
  0.976796, 0.000449711, 6.31947 × 10-55, -8.13532 × 10-152}
```

```
{47.0513, 0.685611, 0.289291, 0.0168723, 0.00704946, 0.00114998, 0.0000256435,
  1.2076 × 10-7, 46.9364, 0.0216092, 3.03659 × 10-53, -3.90913 × 10-150}
```

1.

```
plotiy = Partition[Riffle[normOleg7, iynorm[[2 ;; 8]]], 2]
```

```
{{0.694746, 0.685611}, {0.275684, 0.289291},
  {0.0293036, 0.0168723}, {0.000266625, 0.00704946},
  {0., 0.00114998}, {0., 0.0000256435}, {0., 1.2076 × 10-7}}
```



```
BarChart[plotiy, PlotRange → {-0.1, 0.9},
  ChartLabels → {Placed[{"N +", "N 2+", "N 3+", "N 4+", "N 5+", "N 6+", "N 7+"}, Below],
    Placed[{}, Above]},
  ChartLegends → Placed[{"Expt.", "γfrag"}, Top],
  ChartStyle → {Black, Red}, AxesLabel → {"", "Ỹ(ω)"},
  AxesStyle → {{Arrowheads[Automatic], AbsoluteThickness[0.6]},
    {Arrowheads[Automatic], AbsoluteThickness[0.6]}},
  LabelStyle → {FontFamily → "Arial"},
  PlotLabel → {damp, optGaFra / gammaFrag,
    (iynorm[[2 ;; 8]] - normOleg7).Table[i, {i, 1, 7}]]]
```

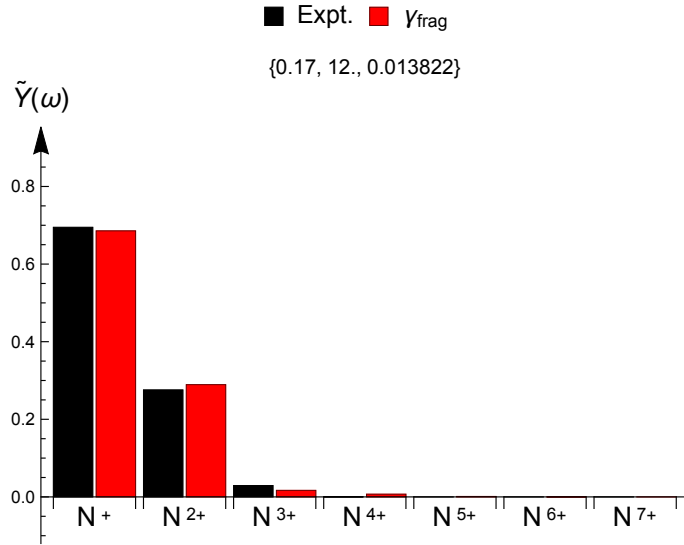

## 0.18

damp := 0.18

```
iy = dsionyieldcrateranalysisparam[damp * 0.26 * MilliJouleToHartree, photonenergy,
  tauX, nintdata, True, True, 1 / 1000, optfNppN, 1 - optfNppN, optGaFra]
```

```
iynorm = 1 / Total[iy[[2 ;; 8]]] * iy
```

```
Total[iynorm[[2 ;; 8]]]
```

```
{0.978194, 0.0147746, 0.00642762, 0.000403503, 0.000169968, 0.0000292784,
  6.93174 × 10-7, 3.46023 × 10-9, 0.975718, 0.00046481, 6.68511 × 10-55, 3.80697 × 10-153}
```

```
{44.8597, 0.677557, 0.294769, 0.0185045, 0.00779468, 0.0013427, 0.0000317888,
  1.58685 × 10-7, 44.7461, 0.021316, 3.06577 × 10-53, 1.74586 × 10-151}
```

1.

```
plotiy = Partition[Riffle[normOleg7, iynorm[[2 ;; 8]]], 2]
```

```
{{0.694746, 0.677557}, {0.275684, 0.294769},
  {0.0293036, 0.0185045}, {0.000266625, 0.00779468},
  {0., 0.0013427}, {0., 0.0000317888}, {0., 1.58685 × 10-7}}
```

```
BarChart[plotiy, PlotRange → {-0.1, 0.9},
  ChartLabels → {Placed[{"N +", "N 2+", "N 3+", "N 4+", "N 5+", "N 6+", "N 7+"}, Below],
    Placed[{}, Above]},
  ChartLegends → Placed[{"Expt.", "γfrag"}, Top],
  ChartStyle → {Black, Red}, AxesLabel → {"", "Ỹ(ω)"},
  AxesStyle → {{Arrowheads[Automatic], AbsoluteThickness[0.6]},
    {Arrowheads[Automatic], AbsoluteThickness[0.6]}},
  LabelStyle → {FontFamily → "Arial"},
  PlotLabel → {damp, optGaFra / gammaFrag,
    (iynorm[[2 ;; 8]] - normOleg7).Table[i, {i, 1, 7}]]]
```

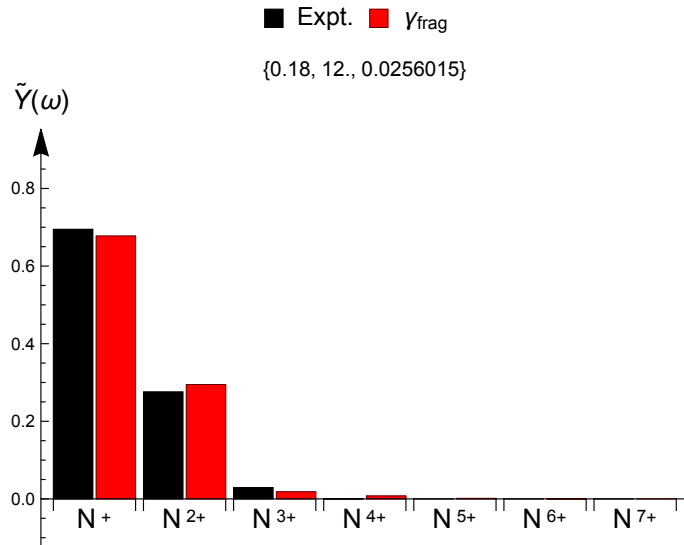

## Pulse energy for a 4 fs pulse with 280 fs fragmentation rate

```
tauX := 4 / t0ToFemtoSecond
optent := 4.059357
optGaFra := optent * gammaFrag
```

### 0.21

```
damp := 0.21

iy = dsionyieldcrateranalysisparam[damp * 0.15 * MilliJouleToHartree, photonenergy,
  tauX, nintdata, True, True, 1 / 1000, optfNppN, 1 - optfNppN, optGaFra]
iynorm = 1 / Total[iy[[2 ;; 8]]] * iy
Total[iynorm[[2 ;; 8]]]
{0.984372, 0.0114029, 0.00402388, 0.000149526,
  0.0000461274, 5.08589 × 10-6, 5.33176 × 10-8, 1.04922 × 10-10,
  0.982454, 0.000361989, 1.78375 × 10-20, -4.59838 × 10-195}

{62.9893, 0.729666, 0.257485, 0.0095681, 0.00295166, 0.000325442, 3.41176 × 10-6,
  6.71391 × 10-9, 62.8666, 0.0231634, 1.14141 × 10-18, -2.94247 × 10-193}
```

1.

```

plotiy = Partition[Riffle[normOleg4, iynorm[[2 ;; 8]]], 2]
{{0.711226, 0.729666}, {0.277966, 0.257485}, {0.0108078, 0.0095681},
 {0., 0.00295166}, {0., 0.000325442}, {0.,  $3.41176 \times 10^{-6}$ }, {0.,  $6.71391 \times 10^{-9}$ }}

```

```

BarChart[plotiy, PlotRange → {-0.1, 0.9},
  ChartLabels → {Placed[{"N +", "N 2+", "N 3+", "N 4+", "N 5+", "N 6+", "N 7+"}, Below],
    Placed[{}, Above]},
  ChartLegends → Placed[{"Expt.", " $\gamma_{\text{frag}}$ "}, Top],
  ChartStyle → {Black, Red}, AxesLabel → {"", " $\tilde{Y}(\omega)$ "},
  AxesStyle → {{Arrowheads[Automatic], AbsoluteThickness[0.6]},
    {Arrowheads[Automatic], AbsoluteThickness[0.6]}},
  LabelStyle → {FontFamily → "Arial"},
  PlotLabel → {damp, optGaFra / gammaFrag,
    (iynorm[[2 ;; 8]] - normOleg4).Table[i, {i, 1, 7}]}]

```

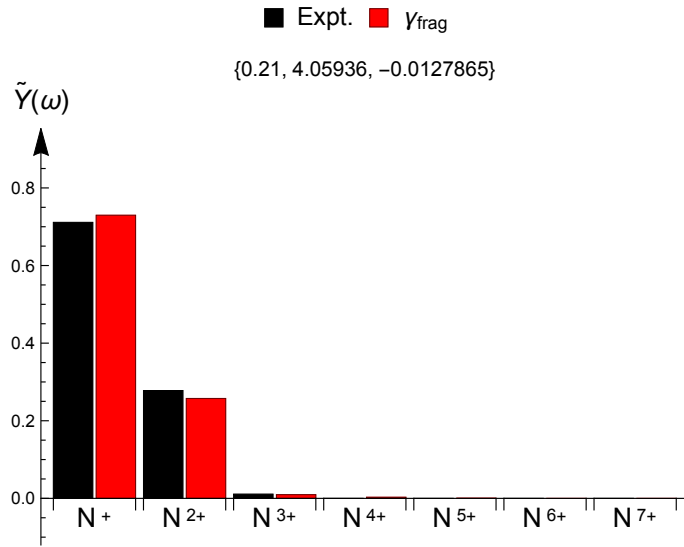

## 0.22

```

damp := 0.22

iy = dsionyieldcrateranalysisparam[damp * 0.15 * MilliJouleToHartree, photonenergy,
  tauX, nintdata, True, True, 1 / 1000, optfNppN, 1 - optfNppN, optGaFra]
iynorm = 1 / Total[iy[[2 ;; 8]]] * iy
Total[iynorm[[2 ;; 8]]]
{0.983732, 0.0117865, 0.00425425, 0.000168925,
 0.0000524342,  $6.04028 \times 10^{-6}$ ,  $6.64491 \times 10^{-8}$ ,  $1.37105 \times 10^{-10}$ ,
 0.98175, 0.000373687,  $1.84355 \times 10^{-20}$ ,  $-5.50694 \times 10^{-172}$ }

{60.4694, 0.724511, 0.261506, 0.0103837, 0.0032231, 0.000371293,  $4.08459 \times 10^{-6}$ ,
 8.42775  $\times 10^{-9}$ , 60.3476, 0.0229703,  $1.13322 \times 10^{-18}$ ,  $-3.38508 \times 10^{-170}$ }

1.

plotiy = Partition[Riffle[normOleg4, iynorm[[2 ;; 8]]], 2]
{{0.711226, 0.724511}, {0.277966, 0.261506}, {0.0108078, 0.0103837},
 {0., 0.0032231}, {0., 0.000371293}, {0.,  $4.08459 \times 10^{-6}$ }, {0.,  $8.42775 \times 10^{-9}$ }}

```

```
BarChart[plotiy, PlotRange → {-0.1, 0.9},
  ChartLabels → {Placed[{"N +", "N 2+", "N 3+", "N 4+", "N 5+", "N 6+", "N 7+"}, Below],
    Placed[{}, Above]},
  ChartLegends → Placed[{"Expt.", "γfrag"}, Top],
  ChartStyle → {Black, Red}, AxesLabel → {"", "Ỹ(ω)",
  AxesStyle → {{Arrowheads[Automatic], AbsoluteThickness[0.6]},
    {Arrowheads[Automatic], AbsoluteThickness[0.6]}},
  LabelStyle → {FontFamily → "Arial"},
  PlotLabel → {damp, optGaFra / gammaFrag,
    (iynorm[[2 ;; 8]] - normOleg4).Table[i, {i, 1, 7}]]]
```

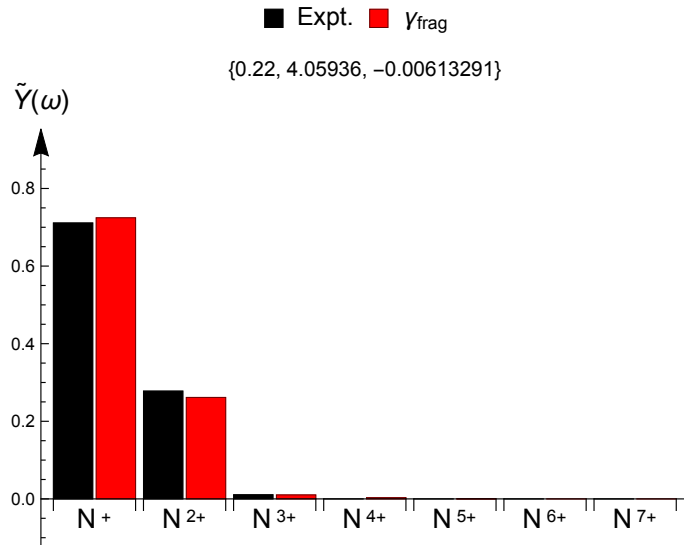

## 0.23

damp := 0.23

```
iy = dsionyieldcrateranalysisparam[damp * 0.15 * MilliJouleToHartree, photonenergy,
  tauX, nintdata, True, True, 1 / 1000, optfNppN, 1 - optfNppN, optGaFra]
```

```
iynorm = 1 / Total[iy[[2 ;; 8]]] * iy
```

```
Total[iynorm[[2 ;; 8]]]
```

```
{0.983099, 0.0121588, 0.00448586, 0.000189672,
  0.0000592361, 7.11509 × 10-6, 8.19675 × 10-8, 1.76959 × 10-10,
  0.981055, 0.000385001, 1.90071 × 10-20, -2.07211 × 10-169}
```

```
{58.169, 0.719423, 0.265424, 0.0112227, 0.00350494, 0.000420993, 4.84993 × 10-6,
  1.04705 × 10-8, 58.0481, 0.0227801, 1.12463 × 10-18, -1.22604 × 10-167}
```

1.

```
plotiy = Partition[Riffle[normOleg4, iynorm[[2 ;; 8]]], 2]
```

```
{{0.711226, 0.719423}, {0.277966, 0.265424}, {0.0108078, 0.0112227},
  {0., 0.00350494}, {0., 0.000420993}, {0., 4.84993 × 10-6}, {0., 1.04705 × 10-8}}
```

```
BarChart[plotiy, PlotRange → {-0.1, 0.9},
  ChartLabels → {Placed[{"N +", "N 2+", "N 3+", "N 4+", "N 5+", "N 6+", "N 7+"}, Below],
    Placed[{}, Above]},
  ChartLegends → Placed[{"Expt.", "γfrag"}, Top],
  ChartStyle → {Black, Red}, AxesLabel → {"", "Ỹ(ω)"},
  AxesStyle → {{Arrowheads[Automatic], AbsoluteThickness[0.6]},
    {Arrowheads[Automatic], AbsoluteThickness[0.6]}},
  LabelStyle → {FontFamily → "Arial"},
  PlotLabel → {damp, optGaFra / gammaFrag,
    (iynorm[[2 ;; 8]] - normOleg4).Table[i, {i, 1, 7}]]]
```

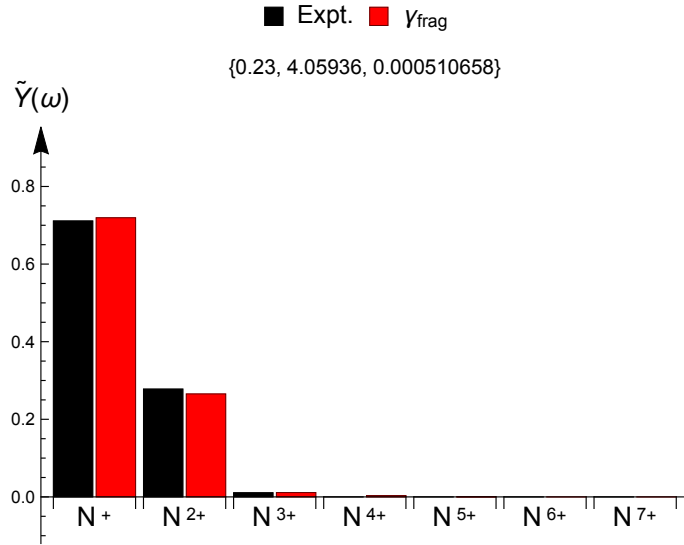

## 0.24

```
damp := 0.24

iy = dsionyieldcrateranalysisparam[damp * 0.15 * MilliJouleToHartree, photonenergy,
  tauX, nintdata, True, True, 1 / 1000, optfNppN, 1 - optfNppN, optGaFra]
iynorm = 1 / Total[iy[[2 ;; 8]]] * iy
Total[iynorm[[2 ;; 8]]]

{0.982475, 0.01252, 0.00471849, 0.000211774,
  0.0000665429, 8.31841 × 10-6, 1.00163 × 10-7, 2.25833 × 10-10,
  0.980371, 0.000395943, 1.95644 × 10-20, -7.84065 × 10-169}

{56.0606, 0.714399, 0.26924, 0.012084, 0.00379698, 0.000474653, 5.71536 × 10-6,
  1.28862 × 10-8, 55.9405, 0.0225928, 1.11636 × 10-18, -4.47392 × 10-167}

1.

plotiy = Partition[Riffle[normOleg4, iynorm[[2 ;; 8]]], 2]

{{0.711226, 0.714399}, {0.277966, 0.26924}, {0.0108078, 0.012084},
  {0., 0.00379698}, {0., 0.000474653}, {0., 5.71536 × 10-6}, {0., 1.28862 × 10-8}}
```

```

BarChart[plotiy, PlotRange → {-0.1, 0.9},
  ChartLabels → {Placed[{"N +", "N 2+", "N 3+", "N 4+", "N 5+", "N 6+", "N 7+"}, Below],
    Placed[{}, Above]},
  ChartLegends → Placed[{"Expt.", "γfrag"}, Top],
  ChartStyle → {Black, Red}, AxesLabel → {"", "Ỹ(ω)"},
  AxesStyle → {{Arrowheads[Automatic], AbsoluteThickness[0.6]},
    {Arrowheads[Automatic], AbsoluteThickness[0.6]}},
  LabelStyle → {FontFamily → "Arial"},
  PlotLabel → {damp, optGaFra / gammaFrag,
    (iynorm[[2 ;; 8]] - normOleg4).Table[i, {i, 1, 7}]]}

```

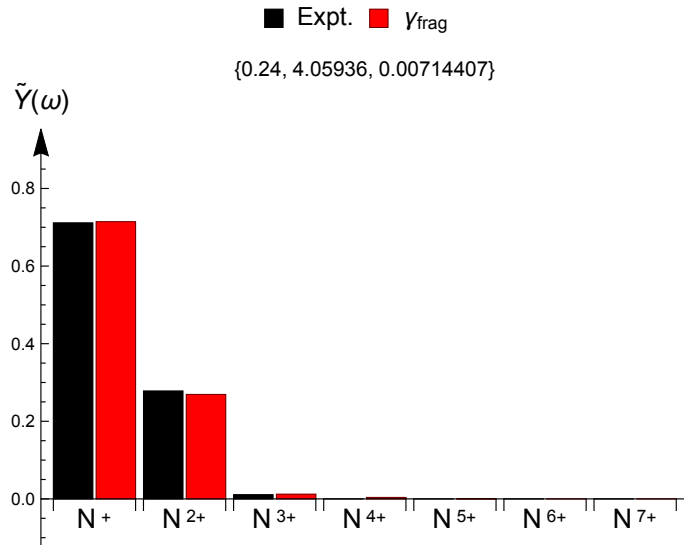

## 0.25

damp := 0.25

```

iy = dsionyieldcrateranalysisparam[damp * 0.15 * MilliJouleToHartree, photonenergy,
  tauX, nintdata, True, True, 1 / 1000, optfNppN, 1 - optfNppN, optGaFra]

```

```

iynorm = 1 / Total[iy[[2 ;; 8]]] * iy

```

```

Total[iynorm[[2 ;; 8]]]

```

```

{0.981858, 0.0128706, 0.00495193, 0.000235236,
  0.0000743639, 9.65835 × 10-6, 1.21345 × 10-7, 2.8523 × 10-10,
  0.979696, 0.000406527, 2.01025 × 10-20, 7.62829 × 10-169}

```

```

{54.1211, 0.70944, 0.272956, 0.0129665, 0.00409902, 0.000532379, 6.68867 × 10-6,
  1.57222 × 10-8, 54.0019, 0.0224082, 1.10807 × 10-18, 4.2048 × 10-167}

```

1.

```

plotiy = Partition[Riffle[normOleg4, iynorm[[2 ;; 8]]], 2]

```

```

{{0.711226, 0.70944}, {0.277966, 0.272956}, {0.0108078, 0.0129665},
  {0., 0.00409902}, {0., 0.000532379}, {0., 6.68867 × 10-6}, {0., 1.57222 × 10-8}}

```

```
BarChart[plotiy, PlotRange → {-0.1, 0.9},
  ChartLabels → {Placed[{"N +", "N 2+", "N 3+", "N 4+", "N 5+", "N 6+", "N 7+"}, Below],
    Placed[{}, Above]},
  ChartLegends → Placed[{"Expt.", "γfrag"}, Top],
  ChartStyle → {Black, Red}, AxesLabel → {"", "Ỹ(ω)"},
  AxesStyle → {{Arrowheads[Automatic], AbsoluteThickness[0.6]},
    {Arrowheads[Automatic], AbsoluteThickness[0.6]}},
  LabelStyle → {FontFamily → "Arial"},
  PlotLabel → {damp, optGaFra / gammaFrag,
    (iynorm[[2 ;; 8]] - normOleg4).Table[i, {i, 1, 7}]]]
```

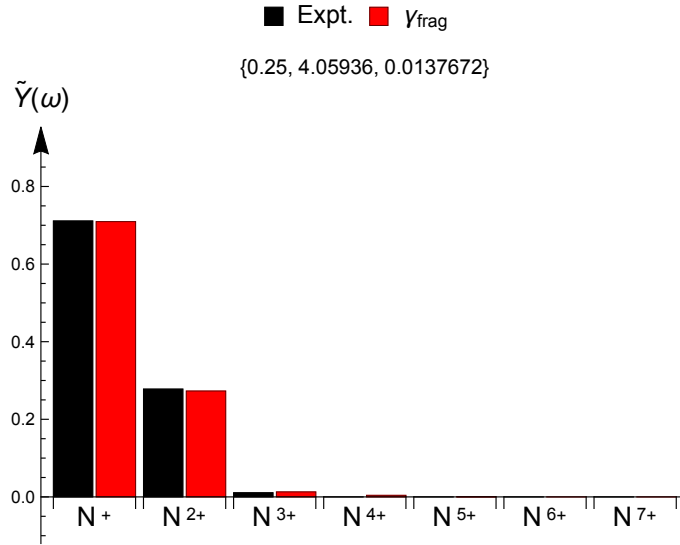

## Pulse energy for a 4 fs pulse with 80 fs fragmentation rate

```
tauX := 4 / t0ToFemtoSecond
optent := 12.000000
optGaFra := optent * gammaFrag
```

### 0.21

```
damp := 0.21

iy = dsionyieldcrateranalysisparam[damp * 0.15 * MilliJouleToHartree, photonenergy,
  tauX, nintdata, True, True, 1 / 1000, optfNppN, 1 - optfNppN, optGaFra]
iynorm = 1 / Total[iy[[2 ;; 8]]] * iy
Total[iynorm[[2 ;; 8]]]

{0.984373, 0.0114053, 0.00401848, 0.000151762,
  0.0000464639, 5.16478 × 10-6, 5.42731 × 10-8, 1.07143 × 10-10,
  0.982454, 0.000361989, 4.11556 × 10-55, -2.45643 × 10-207}

{62.991, 0.729835, 0.257147, 0.00971142, 0.00297327, 0.0003305, 3.47299 × 10-6,
  6.85622 × 10-9, 62.8683, 0.0231641, 2.63359 × 10-53, -1.5719 × 10-205}
```

1.

```

plotiy = Partition[Riffle[normOleg4, iynorm[[2 ;; 8]]], 2]
{{0.711226, 0.729835}, {0.277966, 0.257147}, {0.0108078, 0.00971142},
 {0., 0.00297327}, {0., 0.0003305}, {0.,  $3.47299 \times 10^{-6}$ }, {0.,  $6.85622 \times 10^{-9}$ }}

BarChart[plotiy, PlotRange → {-0.1, 0.9},
 ChartLabels → {Placed[{"N +", "N 2+", "N 3+", "N 4+", "N 5+", "N 6+", "N 7+"}, Below],
 Placed[{}, Above]},
 ChartLegends → Placed[{"Expt.", " $\gamma_{\text{frag}}$ "}, Top],
 ChartStyle → {Black, Red}, AxesLabel → {"", " $\tilde{Y}(\omega)$ "},
 AxesStyle → {{Arrowheads[Automatic], AbsoluteThickness[0.6]},
 {Arrowheads[Automatic], AbsoluteThickness[0.6]}},
 LabelStyle → {FontFamily → "Arial"},
 PlotLabel → {damp, optGaFra / gammaFrag,
 (iynorm[[2 ;; 8]] - normOleg4).Table[i, {i, 1, 7}]}]

```

■ Expt. ■  $\gamma_{\text{frag}}$

{0.21, 12., -0.0127529}

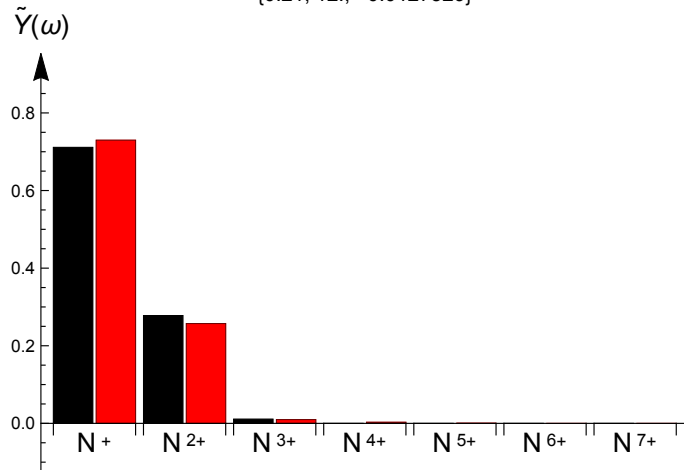

## 0.22

```

damp := 0.22

iy = dsionyieldcrateranalysisparam[damp * 0.15 * MilliJouleToHartree, photonenergy,
 tauX, nintdata, True, True, 1 / 1000, optfNppN, 1 - optfNppN, optGaFra]
iynorm = 1 / Total[iy[[2 ;; 8]]] * iy
Total[iynorm[[2 ;; 8]]]
{0.983732, 0.011789, 0.00424844, 0.000171329,
 0.0000527932,  $6.12922 \times 10^{-6}$ ,  $6.75804 \times 10^{-8}$ ,  $1.39865 \times 10^{-10}$ ,
 0.98175, 0.000373687,  $4.21216 \times 10^{-55}$ ,  $2.59109 \times 10^{-188}$ }

{60.4712, 0.724686, 0.261156, 0.0105318, 0.00324526, 0.00037677,  $4.15425 \times 10^{-6}$ ,
  $8.59768 \times 10^{-9}$ , 60.3493, 0.022971,  $2.58926 \times 10^{-53}$ ,  $1.59277 \times 10^{-186}$ }

1.

plotiy = Partition[Riffle[normOleg4, iynorm[[2 ;; 8]]], 2]
{{0.711226, 0.724686}, {0.277966, 0.261156}, {0.0108078, 0.0105318},
 {0., 0.00324526}, {0., 0.00037677}, {0.,  $4.15425 \times 10^{-6}$ }, {0.,  $8.59768 \times 10^{-9}$ }}

```



```
BarChart[plotiy, PlotRange → {-0.1, 0.9},
  ChartLabels → {Placed[{"N +", "N 2+", "N 3+", "N 4+", "N 5+", "N 6+", "N 7+"}, Below],
    Placed[{}, Above]},
  ChartLegends → Placed[{"Expt.", "γfrag"}, Top],
  ChartStyle → {Black, Red}, AxesLabel → {"", "Ỹ(ω)"},
  AxesStyle → {{Arrowheads[Automatic], AbsoluteThickness[0.6]},
    {Arrowheads[Automatic], AbsoluteThickness[0.6]}},
  LabelStyle → {FontFamily → "Arial"},
  PlotLabel → {damp, optGaFra / gammaFrag,
    (iynorm[[2 ;; 8]] - normOleg4).Table[i, {i, 1, 7}]]]
```

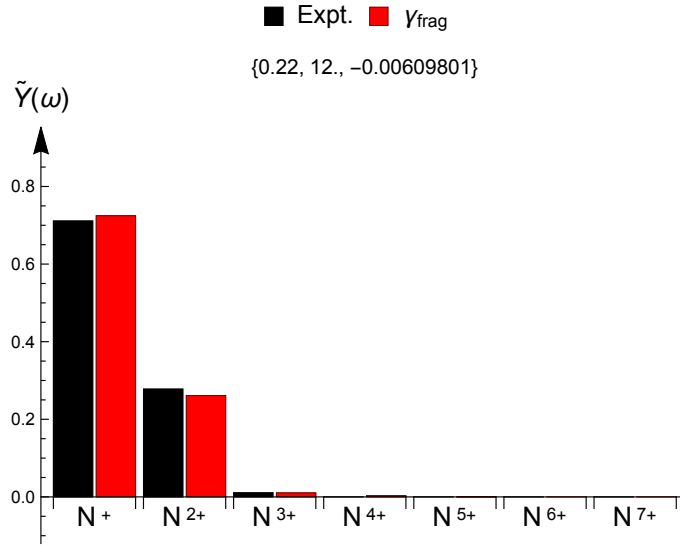

## 0.23

```
damp := 0.23

iy = dsionyieldcrateranalysisparam[damp * 0.15 * MilliJouleToHartree, photonenergy,
  tauX, nintdata, True, True, 1 / 1000, optfNppN, 1 - optfNppN, optGaFra]
iynorm = 1 / Total[iy[[2 ;; 8]]] * iy
Total[iynorm[[2 ;; 8]]]
{0.9831, 0.0121615, 0.00447963, 0.000192247,
  0.0000596175, 7.21473 × 10-6, 8.3296 × 10-8, 1.80355 × 10-10,
  0.981055, 0.000385001, 4.32618 × 10-55, -1.63838 × 10-168}

{58.1707, 0.719603, 0.265063, 0.0113754, 0.00352761, 0.000426901, 4.92868 × 10-6,
  1.06718 × 10-8, 58.0497, 0.0227808, 2.55983 × 10-53, -9.69442 × 10-167}

1.

plotiy = Partition[Riffle[normOleg4, iynorm[[2 ;; 8]]], 2]
{{0.711226, 0.719603}, {0.277966, 0.265063}, {0.0108078, 0.0113754},
  {0., 0.00352761}, {0., 0.000426901}, {0., 4.92868 × 10-6}, {0., 1.06718 × 10-8}}
```

```
BarChart[plotiy, PlotRange → {-0.1, 0.9},
  ChartLabels → {Placed[{"N +", "N 2+", "N 3+", "N 4+", "N 5+", "N 6+", "N 7+"}, Below],
    Placed[{}, Above]},
  ChartLegends → Placed[{"Expt.", "γfrag"}, Top],
  ChartStyle → {Black, Red}, AxesLabel → {"", "Ỹ(ω)"},
  AxesStyle → {{Arrowheads[Automatic], AbsoluteThickness[0.6]},
    {Arrowheads[Automatic], AbsoluteThickness[0.6]}},
  LabelStyle → {FontFamily → "Arial"},
  PlotLabel → {damp, optGaFra / gammaFrag,
    (iynorm[[2 ;; 8]] - normOleg4).Table[i, {i, 1, 7}]]]
```

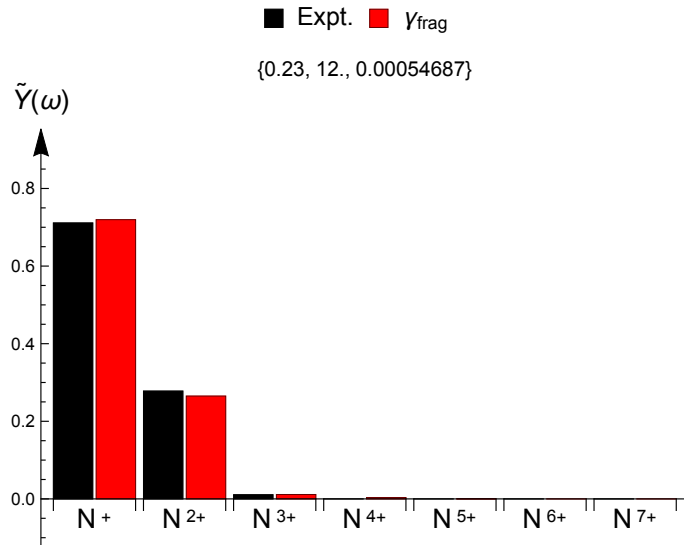

## 0.24

damp := 0.24

```
iy = dsionyieldcrateranalysisparam[damp * 0.15 * MilliJouleToHartree, photonenergy,
  tauX, nintdata, True, True, 1 / 1000, optfNppN, 1 - optfNppN, optGaFra]
```

```
iynorm = 1 / Total[iy[[2 ;; 8]]] * iy
```

```
Total[iynorm[[2 ;; 8]]]
```

```
{0.982475, 0.0125229, 0.00471183, 0.000214522,
  0.0000669466, 8.42941 × 10-6, 1.01711 × 10-7, 2.29972 × 10-10,
  0.980371, 0.000395943, 5.43737 × 10-55, -1.14678 × 10-167}
```

```
{56.0622, 0.714584, 0.268868, 0.0122411, 0.00382012, 0.000481001, 5.80388 × 10-6,
  1.31227 × 10-8, 55.9422, 0.0225934, 3.10269 × 10-53, -6.54379 × 10-166}
```

1.

```
plotiy = Partition[Riffle[normOleg4, iynorm[[2 ;; 8]]], 2]
```

```
{{0.711226, 0.714584}, {0.277966, 0.268868}, {0.0108078, 0.0122411},
  {0., 0.00382012}, {0., 0.000481001}, {0., 5.80388 × 10-6}, {0., 1.31227 × 10-8}}
```

```
BarChart[plotiy, PlotRange → {-0.1, 0.9},
  ChartLabels → {Placed[{"N +", "N 2+", "N 3+", "N 4+", "N 5+", "N 6+", "N 7+"}, Below],
    Placed[{}, Above]},
  ChartLegends → Placed[{"Expt.", "γfrag"}, Top],
  ChartStyle → {Black, Red}, AxesLabel → {"", "Ỹ(ω)",
  AxesStyle → {{Arrowheads[Automatic], AbsoluteThickness[0.6]},
    {Arrowheads[Automatic], AbsoluteThickness[0.6]}},
  LabelStyle → {FontFamily → "Arial"},
  PlotLabel → {damp, optGaFra / gammaFrag,
    (iynorm[[2 ;; 8]] - normOleg4).Table[i, {i, 1, 7}]]]
```

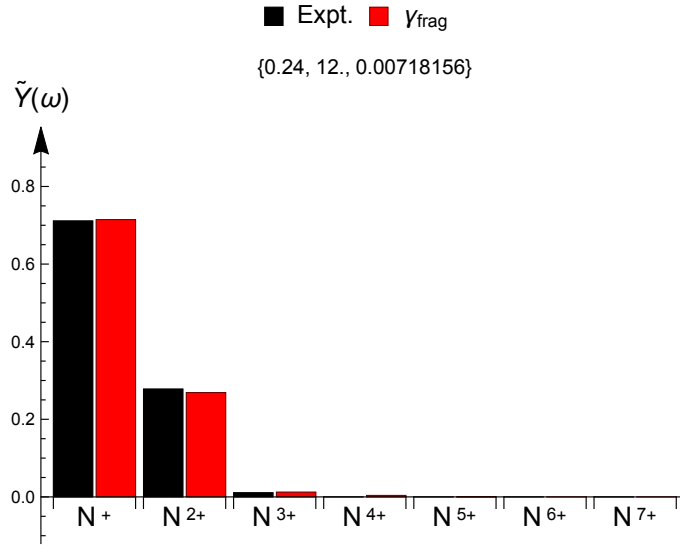

## 0.25

```
damp := 0.25

iy = dsionyieldcrateranalysisparam[damp * 0.15 * MilliJouleToHartree, photonenergy,
  tauX, nintdata, True, True, 1 / 1000, optfNppN, 1 - optfNppN, optGaFra]
iynorm = 1 / Total[iy[[2 ;; 8]]] * iy
Total[iynorm[[2 ;; 8]]]
{0.981859, 0.0128736, 0.00494483, 0.000238158,
  0.0000747896, 9.78136 × 10-6, 1.23137 × 10-7, 2.9023 × 10-10,
  0.979696, 0.000406527, 4.98419 × 10-55, -4.70467 × 10-159}

{54.1228, 0.70963, 0.272573, 0.0131279, 0.00412261, 0.000539176, 6.78766 × 10-6,
  1.59983 × 10-8, 54.0036, 0.0224089, 2.74742 × 10-53, -2.59334 × 10-157}

1.

plotiy = Partition[Riffle[normOleg4, iynorm[[2 ;; 8]]], 2]
{{0.711226, 0.70963}, {0.277966, 0.272573}, {0.0108078, 0.0131279},
  {0., 0.00412261}, {0., 0.000539176}, {0., 6.78766 × 10-6}, {0., 1.59983 × 10-8}}
```

```
BarChart[plotiy, PlotRange → {-0.1, 0.9},
  ChartLabels → {Placed[{"N +", "N 2+", "N 3+", "N 4+", "N 5+", "N 6+", "N 7+"}, Below],
    Placed[{}, Above]},
  ChartLegends → Placed[{"Expt.", "γfrag"}, Top],
  ChartStyle → {Black, Red}, AxesLabel → {"", "Ỹ(ω)"},
  AxesStyle → {{Arrowheads[Automatic], AbsoluteThickness[0.6]},
    {Arrowheads[Automatic], AbsoluteThickness[0.6]}},
  LabelStyle → {FontFamily → "Arial"},
  PlotLabel → {damp, optGaFra / gammaFrag,
    (iynorm[[2 ;; 8]] - normOleg4).Table[i, {i, 1, 7}]]]
```

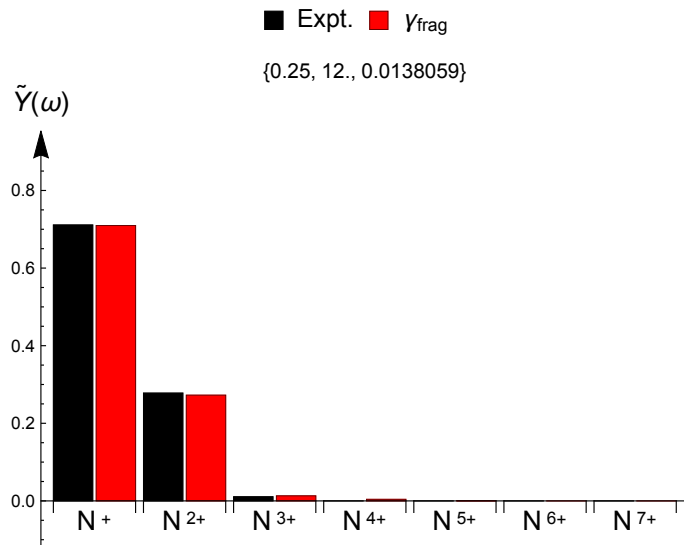

## References

- [1] S. Düsterer, P. Radcliffe, C. Bostedt, J. Bozek, A. L. Cavalieri, R. Coffee, J. T. Costello, D. Cubaynes, L. F. DiMauro, Y. Ding, G. Doumy, F. Grüner, W. Helml, W. Schweinberger, R. Kienberger, A. R. Maier, M. Messerschmidt, V. Richardson, C. Roedig, T. Tschentscher, M. Meyer, *New J. Phys.* **13**, 093024 (2011) [11 pages], *Femtosecond x-ray pulse length characterization at the Linac Coherent Light Source free-electron laser*, <http://dx.doi.org/10.1088/1367-2630/13/9/093024>
