# Supplementary material for: Rate equations for nitrogen molecules in ultrashort and intense x-ray pulses
Source: arXiv:1508.05223 ancillary file (2017-03-16)
Supplement: Supplementary file 7 [file nitrogen_dissociation_second.pdf]

```
<< PlotLegends`
```

General::obspkg: PlotLegends` is now obsolete. The legacy version being loaded may conflict with current functionality. See the Compatibility Guide for updating information.

```
Get["NitrogenRateEquations.m", Path -> NotebookDirectory[]]  
Get["NitrogenMoleculeRateEqs.m", Path -> NotebookDirectory[]]
```

```
HartreeToeV := 27.2113845  
eVToHartree := 1 / HartreeToeV  
JouleToHartree := 2.29371269*^17  
MilliJouleToHartree := 1*^-3 * JouleToHartree  
BohrToAngstroem := 0.5291772083  
AngstroemToBohr := 1 / BohrToAngstroem  
MicrometerToBohr := 1*^4 * AngstroemToBohr  
BohrToMicrometer := 1 / MicrometerToBohr  
t0ToSecond := 24.18884326505*^-18  
t0ToFemtoSecond := 24.18884326505*^-3  
crossSectionAUtoBarn := 1*^8 * BohrToAngstroem^2  
crossSectionAUtocm2 := crossSectionAUtoBarn * 1*^-24  
crossSectioncm2toAU := 1 / crossSectionAUtocm2  
  
neginfinity := -1000 / t0ToFemtoSecond  
posinfinity := 10 000 / t0ToFemtoSecond
```

# Fragmentation time and pulse energy

Microscopic molecular rate-equation model with nominal pulse duration and optimization for the N<sub>2</sub><sup>+</sup> yields

Christian Buth, 27 September 2014

Theoretische Chemie, Physikalisch-Chemisches Institut, Ruprecht-Karls-Universität Heidelberg, Im Neuenheimer Feld 229, 69120 Heidelberg, Germany

---

## Experimental parameters

Pulse energy fractions as determined in this *Mathematica* Notebook:

```
optdamp280 := 0.38  
optdamp80 := 0.30  
optdamp7 := 0.16  
optdamp4 := 0.23
```

Pulse energy fraction for the 4 fs pulse with respect to a pulse energy of 0.26 mJ instead of 0.15 mJ and vice versa for the 7 fs pulse:

```
optdamp4 * 0.15 / 0.26  
0.132692  
  
optdamp7 * 0.26 / 0.15  
0.277333
```

Pulse duration fractions. See Ref. [1] for measurements of LCLS pulse durations:

```
280 / 300 * 120
```

```
112
```

```
shtdur280 = 112 / 280.0
```

```
0.4
```

```
shtdur80 = 40 / 80.0
```

```
0.5
```

```
shtdur7 := 0.4
```

```
shtdur4 := 0.4
```

```
photonenergy := 1100 * eVToHartree
```

```
optfNppN := 0.26
```

```
newMatthias280 := {204.331, 105.281, 27.561, 13.151, 9.881, 0.587, 0.000}
```

```
normOleg280 = 1 / Total[newMatthias280] * newMatthias280
```

```
{0.56634, 0.291805, 0.0763903, 0.0364504, 0.027387, 0.00162698, 0.}
```

```
newMatthias80 := {218.068, 103.774, 26.075, 9.804, 3.315, 0.000, 0.000}
```

```
normOleg80 = 1 / Total[newMatthias80] * newMatthias80
```

```
{0.604006, 0.287434, 0.0722227, 0.0271552, 0.00918191, 0., 0.}
```

```
newMatthias7 := {221.485, 87.888, 9.342, 0.085, 0.000, 0.000, 0.000}
```

```
normOleg7 = 1 / Total[newMatthias7] * newMatthias7
```

```
{0.694746, 0.275684, 0.0293036, 0.000266625, 0., 0., 0.}
```

```
newMatthias4 := {92.985, 36.341, 1.413, 0, 0, 0, 0}
```

```
normOleg4 = 1 / Total[newMatthias4] * newMatthias4
```

```
{0.711226, 0.277966, 0.0108078, 0., 0., 0., 0.}
```

---

## Molecular fragmentation rate and pulse energy for a 280 fs pulse

```
tauX := 280 / t0ToFemtoSecond
```

```
normfitconsts[damp_?NumericQ, gaFra_?NumericQ] := Module[{olegiy, olegiynorm},
  olegiy =
    dsionyieldcrateranalysisparam[damp * 0.26 * MilliJouleToHartree, photonenergy,
      tauX, nintdata, True, True, 1 / 1000, optfNppN, 1 - optfNppN, gaFra];
  olegiynorm = 1 / Total[olegiy[[2 ;; 8]]] * olegiy[[2 ;; 8]];
  Norm[(olegiynorm - normOleg280) * Table[{i, {i, 1, 7}}, 1] +
    16 * Abs[olegiynorm[[2]] - normOleg280[[2]]]
]
```

### 0.36

```
damp := 0.36
```

```

tabgamma =
  Table[{gaFra, normfitconsts[damp, gaFra * gammaFrag]}, {gaFra, 1, 10, 1 / 2}];

ListPlot[tabgamma, Joined -> True,
  PlotMarkers -> Automatic, PlotStyle -> {Thick, Red}]

```

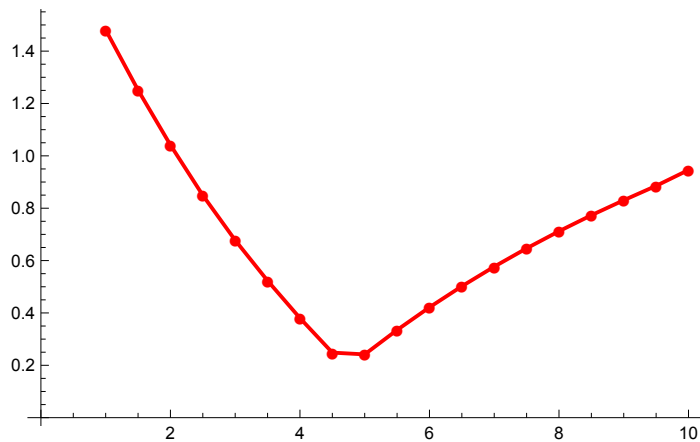

```

tabgamma =
  Table[{gaFra, normfitconsts[damp, gaFra * gammaFrag]}, {gaFra, 4, 6, 1 / 5}];

ListPlot[tabgamma, Joined -> True,
  PlotMarkers -> Automatic, PlotStyle -> {Thick, Red}]

```

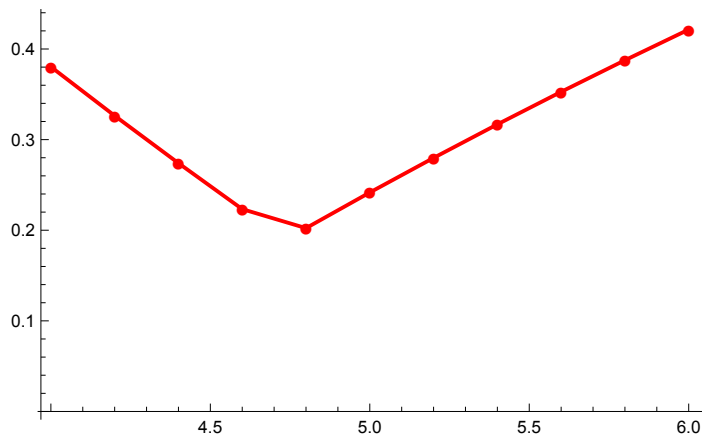

```

N[MinimalBy[tabgamma, Last]]
{{4.8, 0.20232}}

```

```

intgamma = Interpolation[tabgamma, x]

```

```

InterpolatingFunction[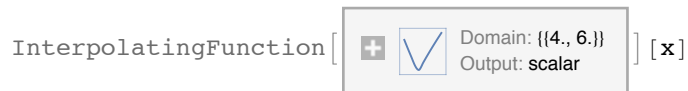 Domain: {{4., 6.}}  
Output: scalar][x]

```

```

mingamma = FindMinimum[intgamma, {x, 4.0, 6.0}]

```

```

InterpolatingFunction::dmval:

```

Input value {6.26425} lies outside the range of data in the interpolating function. Extrapolation will be used. >>

```

{0.202179, {x -> 4.78621}}

```

```

optent = x /. mingamma[[2]]

```

```

4.78621

```

```

optGaFra := optent * gammaFrag

iy = dsionyieldcrateranalysisparam[damp * 0.26 * MilliJouleToHartree, photonenergy,
  tauX, nintdata, True, True, 1 / 1000, optfNppN, 1 - optfNppN, optGaFra]
iynorm = 1 / Total[iy[[2 ;; 8]]] * iy
Total[iynorm[[2 ;; 8]]]

{0.96346, 0.0212352, 0.0106401, 0.00199675, 0.00188202, 0.000691382, 0.0000894092,
  5.15374 × 10-6, 0.959919, 0.000628799, 2.51142 × 10-23, -9.214 × 10-109}

{26.3673, 0.581149, 0.291191, 0.0546456, 0.0515059, 0.0189212, 0.00244689,
  0.000141044, 26.2704, 0.0172085, 6.87306 × 10-22, -2.52162 × 10-107}

1.

plotiy = Partition[Riffle[normOleg280, iynorm[[2 ;; 8]]], 2]
{{0.56634, 0.581149}, {0.291805, 0.291191},
 {0.0763903, 0.0546456}, {0.0364504, 0.0515059},
 {0.027387, 0.0189212}, {0.00162698, 0.00244689}, {0., 0.000141044}}

BarChart[plotiy, PlotRange → {-0.1, 0.9},
  ChartLabels → {Placed[{"N+", "N2+", "N3+", "N4+", "N5+", "N6+", "N7+"}, Below],
    Placed[{}, Above]},
  ChartLegends → Placed[{"Expt.", "γfrag"}, Top],
  ChartStyle → {Black, Red}, AxesLabel → {"", "Ỹ(ω)"},
  AxesStyle → {{Arrowheads[Automatic], AbsoluteThickness[0.6]},
    {Arrowheads[Automatic], AbsoluteThickness[0.6]}},
  LabelStyle → {FontFamily → "Arial"},
  PlotLabel → {damp, optGaFra / gammaFrag,
    (iynorm[[2 ;; 8]] - normOleg280).Table[i, {i, 1, 7}]]}

■ Expt. ■ γfrag
{0.36, 4.78621, -0.0278545}

```

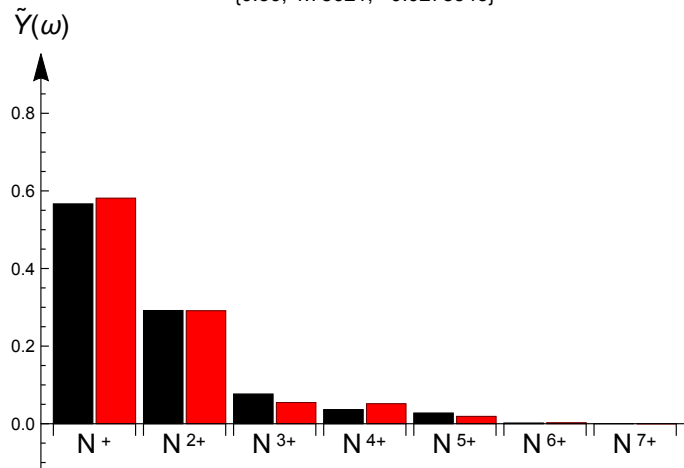

### 0.37

```

damp := 0.37

tabgamma =
  Table[{gaFra, normfitconsts[damp, gaFra * gammaFrag]}, {gaFra, 1, 10, 1 / 2}];

```

```
ListPlot[tabgamma, Joined -> True,
  PlotMarkers -> Automatic, PlotStyle -> {Thick, Red}]
```

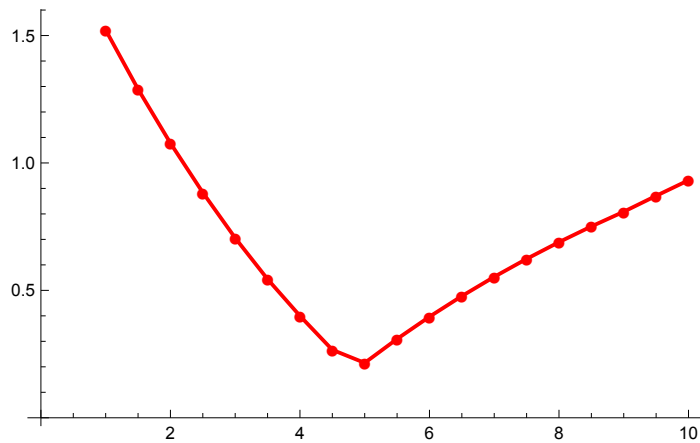

```
tabgamma =
  Table[{gaFra, normfitconsts[damp, gaFra * gammaFrag]}, {gaFra, 4, 6, 1/5}];
```

```
ListPlot[tabgamma, Joined -> True,
  PlotMarkers -> Automatic, PlotStyle -> {Thick, Red}]
```

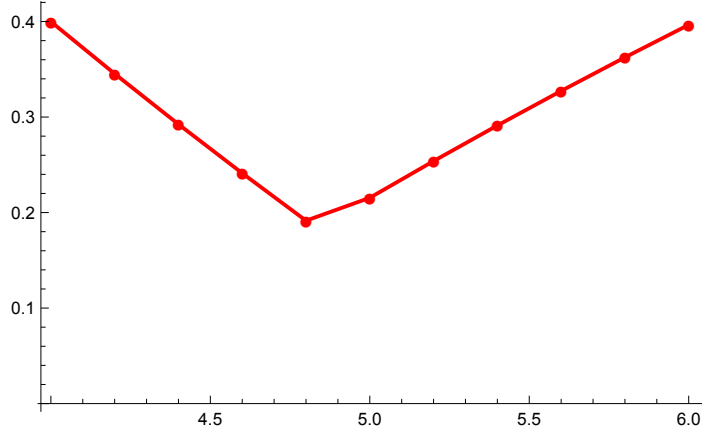

```
N[MinimalBy[tabgamma, Last]]
```

```
{{4.8, 0.191504}}
```

```
intgamma = Interpolation[tabgamma, x]
```

```
InterpolatingFunction[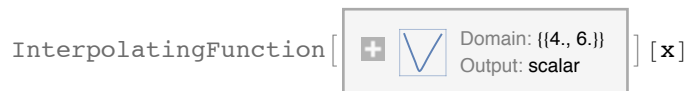 Domain: {{4., 6.}}  
Output: scalar][x]
```

```
mingamma = FindMinimum[intgamma, {x, 4, 6}]
```

```
InterpolatingFunction::dmval:
```

```
Input value {6.26425} lies outside the range of data in the interpolating function. Extrapolation will be used. >>
```

```
{0.191442, {x -> 4.80832}}
```

```
optent = x /. mingamma[[2]]
```

```
4.80832
```

```
optGaFra := optent * gammaFrag
```

```

iy = dsionyieldcrateranalysisparam[damp * 0.26 * MilliJouleToHartree, photonenergy,
  tauX, nintdata, True, True, 1 / 1000, optfNppN, 1 - optfNppN, optGaFra]
iynorm = 1 / Total[iy[[2 ;; 8]]] * iy
Total[iynorm[[2 ;; 8]]]

{0.962778, 0.0214501, 0.010874, 0.00207158, 0.00197931, 0.000742582, 0.0000987946,
  5.84053 × 10-6, 0.959202, 0.000633826, 2.0305 × 10-23, -2.9523 × 10-109}

{25.8656, 0.576271, 0.292138, 0.0556545, 0.0531754, 0.0199499, 0.00265418,
  0.00015691, 25.7696, 0.0170281, 5.45507 × 10-22, -7.93155 × 10-108}

1.

```

```

plotiy = Partition[Riffle[normOleg280, iynorm[[2 ;; 8]]], 2]
{{0.56634, 0.576271}, {0.291805, 0.292138},
 {0.0763903, 0.0556545}, {0.0364504, 0.0531754},
 {0.027387, 0.0199499}, {0.00162698, 0.00265418}, {0., 0.00015691}}

BarChart[plotiy, PlotRange → {-0.1, 0.9},
  ChartLabels → {Placed[{"N +", "N 2+", "N 3+", "N 4+", "N 5+", "N 6+", "N 7+"}, Below],
    Placed[{}, Above]},
  ChartLegends → Placed[{"Expt.", "γfrag"}, Top],
  ChartStyle → {Black, Red}, AxesLabel → {"", "Ỹ(ω)"},
  AxesStyle → {{Arrowheads[Automatic], AbsoluteThickness[0.6]},
    {Arrowheads[Automatic], AbsoluteThickness[0.6]}},
  LabelStyle → {FontFamily → "Arial"},
  PlotLabel → {damp, optGaFra / gammaFrag,
    (iynorm[[2 ;; 8]] - normOleg280).Table[i, {i, 1, 7}]}]

```

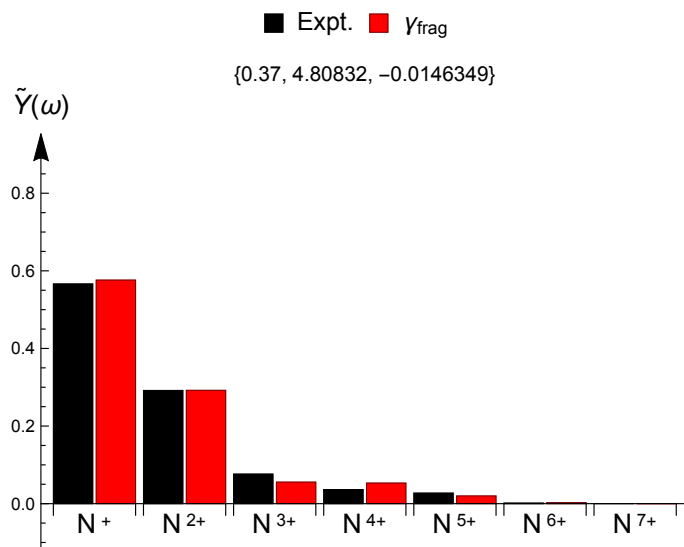

## 0.38

```

damp := 0.38

tabgamma =
  Table[{gaFra, normfitconsts[damp, gaFra * gammaFrag]}, {gaFra, 1, 10, 1 / 2}];

```

```
ListPlot[tabgamma, Joined -> True,
  PlotMarkers -> Automatic, PlotStyle -> {Thick, Red}]
```

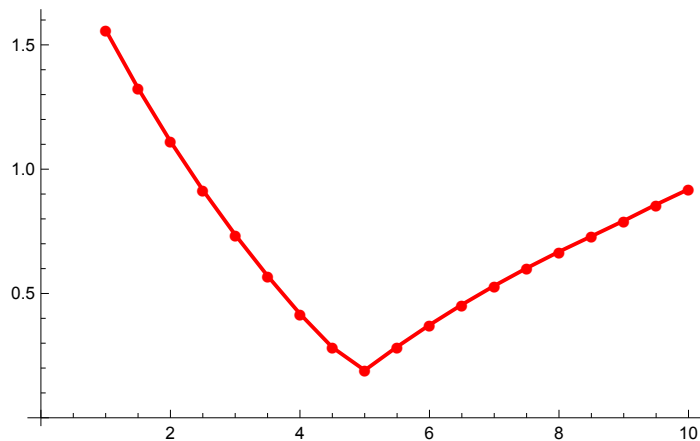

```
tabgamma =
  Table[{gaFra, normfitconsts[damp, gaFra * gammaFrag]}, {gaFra, 4, 6, 1/5}];
```

```
ListPlot[tabgamma, Joined -> True,
  PlotMarkers -> Automatic, PlotStyle -> {Thick, Red}]
```

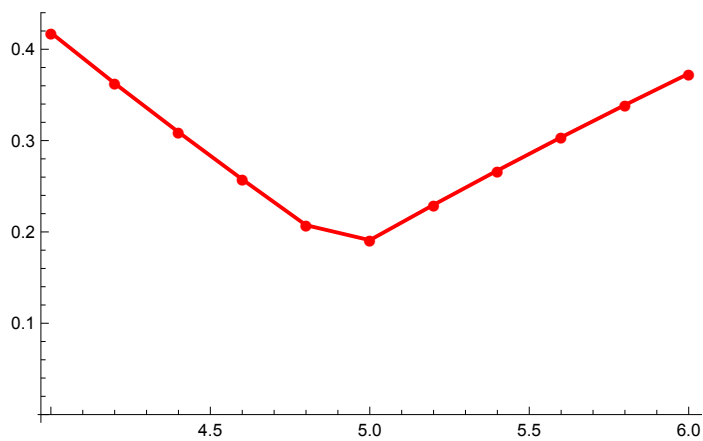

```
N[MinimalBy[tabgamma, Last]]
```

```
{{5., 0.190973}}
```

```
intgamma = Interpolation[tabgamma, x]
```

```
InterpolatingFunction[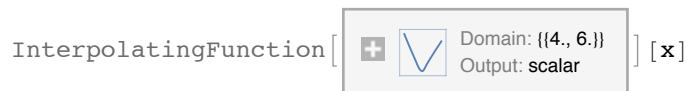 Domain: {{4., 6.}}  
Output: scalar][x]
```

```
mingamma = FindMinimum[intgamma, {x, 4, 6}]
```

```
InterpolatingFunction::dmval:
```

```
Input value {6.26425} lies outside the range of data in the interpolating function. Extrapolation will be used. >>
```

```
{0.190443, {x -> 4.97174}}
```

```
optent = x /. mingamma[[2]]
```

```
4.97174
```

```
optGaFra := optent * gammaFrag
```

```

iy = dsionyieldcrateranalysisparam[damp * 0.26 * MilliJouleToHartree, photonenergy,
  tauX, nintdata, True, True, 1 / 1000, optfNppN, 1 - optfNppN, optGaFra]
iynorm = 1 / Total[iy[[2 ;; 8]]] * iy
Total[iynorm[[2 ;; 8]]]

{0.962113, 0.0216846, 0.0110347, 0.00218008, 0.00207056, 0.000800862, 0.000109742,
  6.69068 × 10-6, 0.958498, 0.000638571, 4.01928 × 10-24, -1.60987 × 10-109}

{25.3941, 0.572345, 0.291252, 0.0575411, 0.0546505, 0.021138, 0.00289655,
  0.000176594, 25.2987, 0.0168545, 1.06085 × 10-22, -4.2491 × 10-108}

1.

```

```

plotiy = Partition[Riffle[normOleg280, iynorm[[2 ;; 8]]], 2]
{{0.56634, 0.572345}, {0.291805, 0.291252},
 {0.0763903, 0.0575411}, {0.0364504, 0.0546505},
 {0.027387, 0.021138}, {0.00162698, 0.00289655}, {0., 0.000176594}}

BarChart[plotiy, PlotRange → {-0.1, 0.9},
  ChartLabels → {Placed[{"N +", "N 2+", "N 3+", "N 4+", "N 5+", "N 6+", "N 7+"}, Below],
    Placed[{}, Above]},
  ChartLegends → Placed[{"Expt.", "γfrag"}, Top],
  ChartStyle → {Black, Red}, AxesLabel → {"", "Ỹ(ω)"},
  AxesStyle → {{Arrowheads[Automatic], AbsoluteThickness[0.6]},
    {Arrowheads[Automatic], AbsoluteThickness[0.6]}},
  LabelStyle → {FontFamily → "Arial"},
  PlotLabel → {damp, optGaFra / gammaFrag,
    (iynorm[[2 ;; 8]] - normOleg280).Table[i, {i, 1, 7}]]}

```

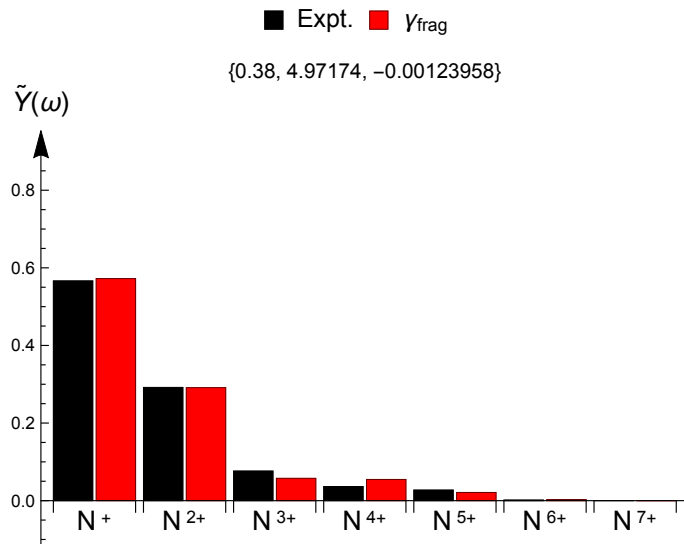

## 0.39

```

damp := 0.39

tabgamma =
  Table[{gaFra, normfitconsts[damp, gaFra * gammaFrag]}, {gaFra, 1, 10, 1 / 2}];

```

```
ListPlot[tabgamma, Joined -> True,
PlotMarkers -> Automatic, PlotStyle -> {Thick, Red}]
```

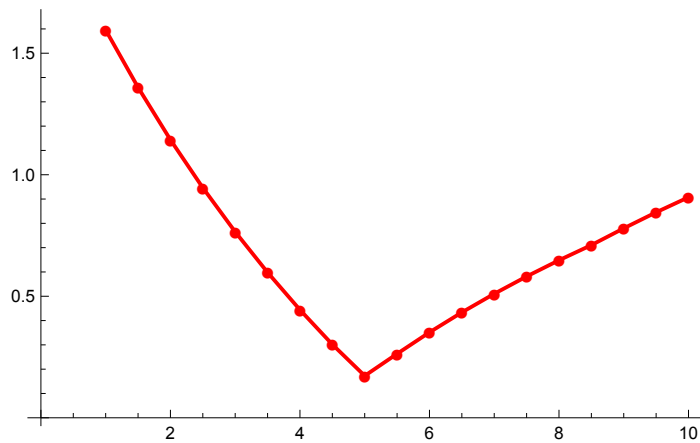

```
tabgamma =
Table[{gaFra, normfitconsts[damp, gaFra * gammaFrag]}, {gaFra, 4, 6, 1/5}];
```

```
ListPlot[tabgamma, Joined -> True,
PlotMarkers -> Automatic, PlotStyle -> {Thick, Red}]
```

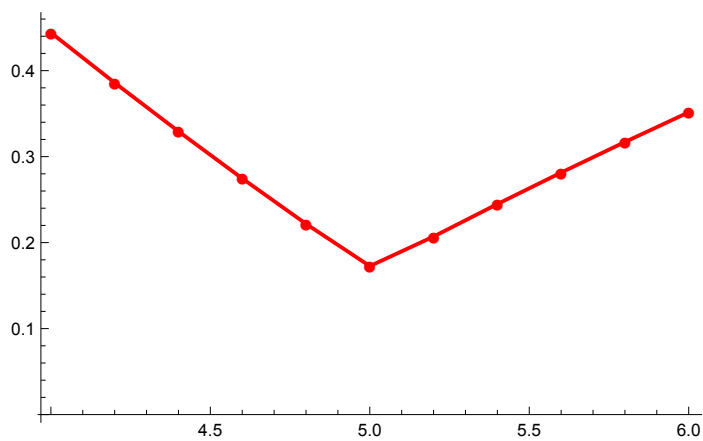

```
N[MinimalBy[tabgamma, Last]]
```

```
{{5., 0.172698}}
```

```
intgamma = Interpolation[tabgamma, x]
```

```
InterpolatingFunction[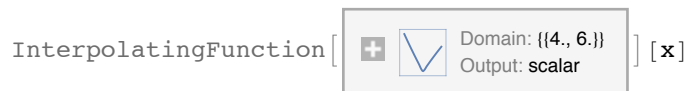 Domain: {{4., 6.}}  
Output: scalar][x]
```

```
mingamma = FindMinimum[intgamma, {x, 4.0, 6.0}]
```

```
InterpolatingFunction::dmval:
```

```
Input value {6.26425} lies outside the range of data in the interpolating function. Extrapolation will be used. >>
```

```
{0.172698, {x -> 5.}}
```

```
optent = x /. mingamma[[2]]
```

```
5.
```

```
optGaFra := optent * gammaFrag
```

```

iy = dsionyieldcrateranalysisparam[damp * 0.26 * MilliJouleToHartree, photonenergy,
  tauX, nintdata, True, True, 1 / 1000, optfNppN, 1 - optfNppN, optGaFra]
iynorm = 1 / Total[iy[[2 ;; 8]]] * iy
Total[iynorm[[2 ;; 8]]]

{0.961454, 0.0218828, 0.0112527, 0.00225677, 0.00216898, 0.000856241, 0.000120551,
  7.5306 × 10-6, 0.957808, 0.000643048, 3.0723 × 10-24, 1.82754 × 10-109}

{24.9433, 0.567713, 0.291932, 0.0585481, 0.0562705, 0.0222138, 0.00312749,
  0.000195369, 24.8487, 0.0166828, 7.97057 × 10-23, 4.74126 × 10-108}

1.

```

```

plotiy = Partition[Riffle[normOleg280, iynorm[[2 ;; 8]]], 2]
{{0.56634, 0.567713}, {0.291805, 0.291932},
 {0.0763903, 0.0585481}, {0.0364504, 0.0562705},
 {0.027387, 0.0222138}, {0.00162698, 0.00312749}, {0., 0.000195369}}

BarChart[plotiy, PlotRange → {-0.1, 0.9},
  ChartLabels → {Placed[{"N+", "N2+", "N3+", "N4+", "N5+", "N6+", "N7+"}, Below],
    Placed[{}, Above]},
  ChartLegends → Placed[{"Expt.", "γfrag"}, Top],
  ChartStyle → {Black, Red}, AxesLabel → {"", "Ỹ(ω)"},
  AxesStyle → {{Arrowheads[Automatic], AbsoluteThickness[0.6]},
    {Arrowheads[Automatic], AbsoluteThickness[0.6]}},
  LabelStyle → {FontFamily → "Arial"},
  PlotLabel → {damp, optGaFra / gammaFrag,
    (iynorm[[2 ;; 8]] - normOleg280).Table[i, {i, 1, 7}]}]

```

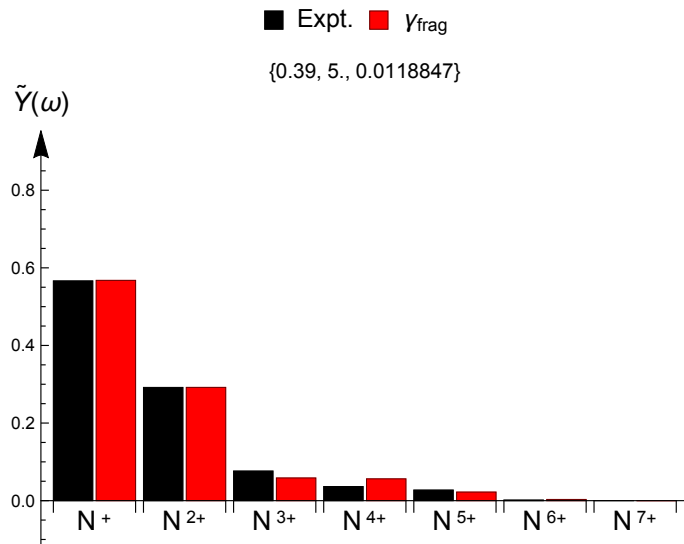

0.40

damp := 0.40

tabgamma =

Table[{gaFra, normfitconsts[damp, gaFra \* gammaFrag]}, {gaFra, 1, 10, 1 / 2}];

```
ListPlot[tabgamma, Joined -> True,
  PlotMarkers -> Automatic, PlotStyle -> {Thick, Red}]
```

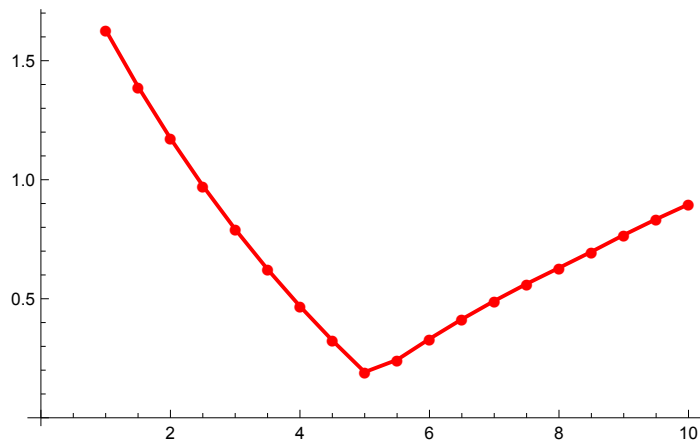

```
tabgamma =
  Table[{gaFra, normfitconsts[damp, gaFra * gammaFrag]}, {gaFra, 4, 6, 1/5}];
```

```
ListPlot[tabgamma, Joined -> True,
  PlotMarkers -> Automatic, PlotStyle -> {Thick, Red}]
```

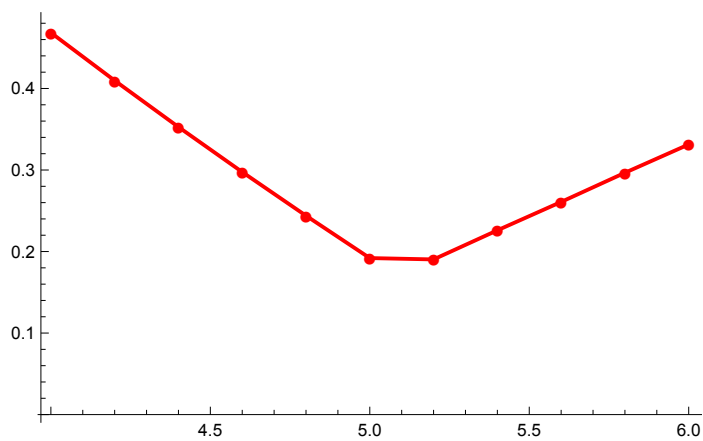

```
N[MinimalBy[tabgamma, Last]]
```

```
{{5.2, 0.190326}}
```

```
intgamma = Interpolation[tabgamma, x]
```

```
InterpolatingFunction[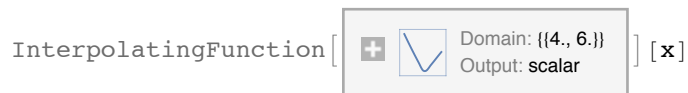 Domain: {{4., 6.}}  
Output: scalar][x]
```

```
mingamma = FindMinimum[intgamma, {x, 4.5, 6.5}]
```

```
{0.185661, {x -> 5.1051}}
```

```
optent = x /. mingamma[[2]]
```

```
5.1051
```

```
optGaFra := optent * gammaFrag
```

```

iy = dsionyieldcrateranalysisparam[damp * 0.26 * MilliJouleToHartree, photonenergy,
  tauX, nintdata, True, True, 1 / 1000, optfNppN, 1 - optfNppN, optGaFra]
iynorm = 1 / Total[iy[[2 ;; 8]]] * iy
Total[iynorm[[2 ;; 8]]]

{0.96081, 0.0220886, 0.0114273, 0.0023522, 0.00226386, 0.000916474, 0.000132617,
  8.51114 × 10-6, 0.957131, 0.000647275, 1.09069 × 10-24, 1.72836 × 10-109}

{24.517, 0.563635, 0.29159, 0.0600212, 0.0577669, 0.0233857, 0.00338398,
  0.000217179, 24.4231, 0.0165165, 2.78312 × 10-23, 4.41025 × 10-108}

1.

plotiy = Partition[Riffle[normOleg280, iynorm[[2 ;; 8]]], 2]
{{0.56634, 0.563635}, {0.291805, 0.29159},
 {0.0763903, 0.0600212}, {0.0364504, 0.0577669},
 {0.027387, 0.0233857}, {0.00162698, 0.00338398}, {0., 0.000217179}}

BarChart[plotiy, PlotRange → {-0.1, 0.9},
  ChartLabels → {Placed[{"N+", "N2+", "N3+", "N4+", "N5+", "N6+", "N7+"}, Below],
    Placed[{}, Above]},
  ChartLegends → Placed[{"Expt.", "γfrag"}, Top],
  ChartStyle → {Black, Red}, AxesLabel → {"", "Ỹ(ω)"},
  AxesStyle → {{Arrowheads[Automatic], AbsoluteThickness[0.6]},
    {Arrowheads[Automatic], AbsoluteThickness[0.6]}},
  LabelStyle → {FontFamily → "Arial"},
  PlotLabel → {damp, optGaFra / gammaFrag,
    (iynorm[[2 ;; 8]] - normOleg280).Table[i, {i, 1, 7}]}]

```

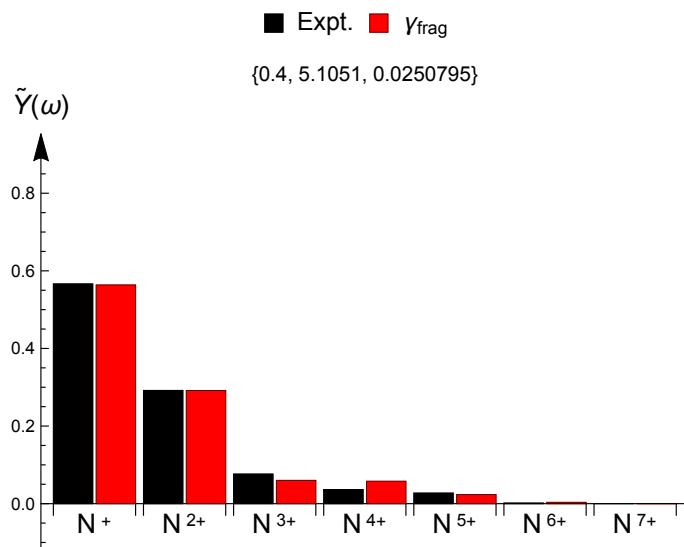

## Molecular fragmentation rate and pulse energy for a 80 fs pulse

```
tauX := 80 / t0ToFemtoSecond
```

```

normfitconsts[damp_?NumericQ, gaFra_?NumericQ] := Module[{olegiy, olegiynorm},
  olegiy =
    dsionyieldcrateranalysisparam[damp * 0.26 * MilliJouleToHartree, photonenergy,
      tauX, nintdata, True, True, 1 / 1000, optfNppN, 1 - optfNppN, gaFra];
  olegiynorm = 1 / Total[olegiy[[2 ;; 8]] * olegiy[[2 ;; 8]]];
  Norm[(olegiynorm - normOleg80) * Table[i, {i, 1, 7}], 1] +
    16 * Abs[olegiynorm[[2]] - normOleg80[[2]]]
]

```

## 0.28

```
damp := 0.28
```

```

tabgamma =
  Table[{gaFra, normfitconsts[damp, gaFra * gammaFrag]}, {gaFra, 5, 25, 1 / 2}];

```

```

ListPlot[tabgamma, Joined -> True,
  PlotMarkers -> Automatic, PlotStyle -> {Thick, Red}]

```

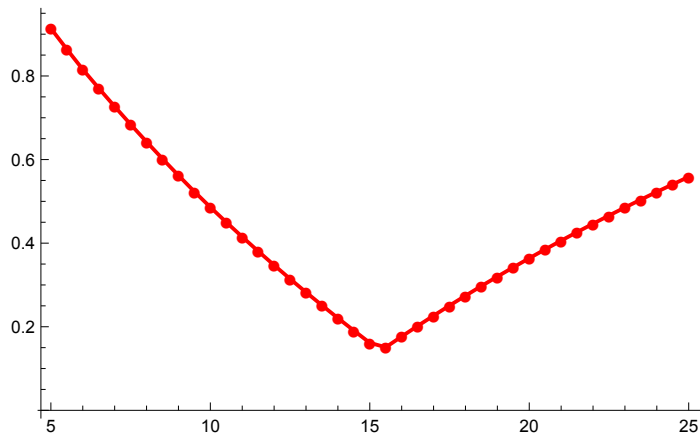

```

tabgamma =
  Table[{gaFra, normfitconsts[damp, gaFra * gammaFrag]}, {gaFra, 14, 16, 1 / 5}];

```

```

ListPlot[tabgamma, Joined -> True,
  PlotMarkers -> Automatic, PlotStyle -> {Thick, Red}]

```

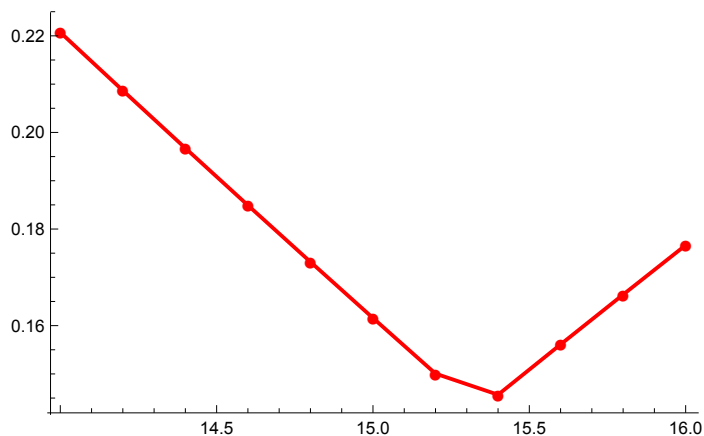

```
N[MinimalBy[tabgamma, Last]]
```

```
{{15.4, 0.145689}}
```

```
intgamma = Interpolation[tabgamma, x]
```

InterpolatingFunction[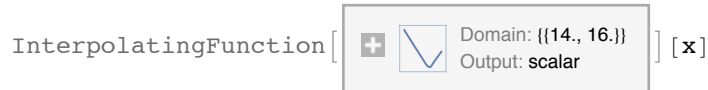 Domain: {{14., 16.}}  
Output: scalar][x]

```
mingamma = FindMinimum[intgamma, {x, 14, 16}]
```

InterpolatingFunction::dmval:

Input value {16.2642} lies outside the range of data in the interpolating function. Extrapolation will be used. >>

```
{0.145583, {x → 15.3755}}
```

```
optent = x /. mingamma[[2]]
```

```
15.3755
```

```
optGaFra := optent * gammaFrag
```

```
iy = dsionyielcdcrateranalysisparam[damp * 0.26 * MilliJouleToHartree, photonenergy,  
tauX, nintdata, True, True, 1 / 1000, optfNppN, 1 - optfNppN, optGaFra]
```

```
inyorm = 1 / Total[iy[[2 ;; 8]]] * iy
```

```
Total[iynorm[[2 ;; 8]]]
```

```
{0.969379, 0.0190314, 0.00879784, 0.00137506, 0.00107274, 0.000315385,  
0.0000277353, 1.0086 × 10-6, 0.966197, 0.000576154, 1.55441 × 10-69, 4.65779 × 10-137}
```

```
{31.6571, 0.621511, 0.287312, 0.0449056, 0.0350327, 0.0102996, 0.000905755,  
0.0000329381, 31.5532, 0.0188156, 5.07626 × 10-68, 1.5211 × 10-135}
```

```
1.
```

```
plotiy = Partition[Riffle[normOleg80, iynorm[[2 ;; 8]]], 2]
```

```
{{0.604006, 0.621511}, {0.287434, 0.287312},  
{0.0722227, 0.0449056}, {0.0271552, 0.0350327},  
{0.00918191, 0.0102996}, {0., 0.000905755}, {0., 0.0000329381}}
```

```
BarChart[plotiy, PlotRange → {-0.1, 0.9},
  ChartLabels → {Placed[{"N +", "N 2+", "N 3+", "N 4+", "N 5+", "N 6+", "N 7+"}, Below],
    Placed[{}, Above]},
  ChartLegends → Placed[{"Expt.", "γfrag"}, Top],
  ChartStyle → {Black, Red}, AxesLabel → {"", "Ỹ(ω)",
  AxesStyle → {{Arrowheads[Automatic], AbsoluteThickness[0.6]},
    {Arrowheads[Automatic], AbsoluteThickness[0.6]}},
  LabelStyle → {FontFamily → "Arial"},
  PlotLabel → {damp, optGaFra / gammaFrag,
    (iynorm[2 ;; 8] - normOleg80).Table[i, {i, 1, 7}]]]
```

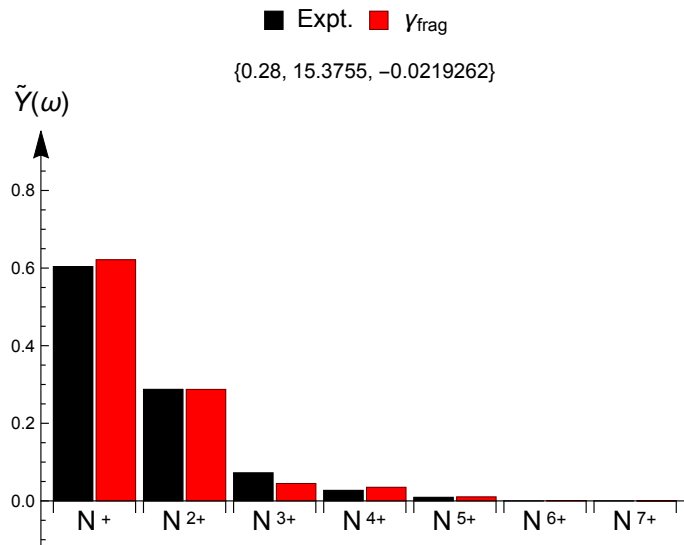

## 0.29

damp := 0.29

```
tabgamma =
  Table[{gaFra, normfitconsts[damp, gaFra * gammaFrag]}, {gaFra, 10, 20, 1 / 2}];
ListPlot[tabgamma, Joined -> True,
  PlotMarkers -> Automatic, PlotStyle -> {Thick, Red}]
```

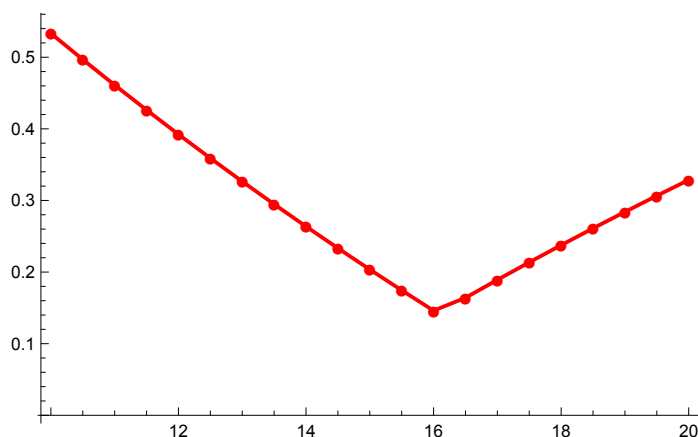

```
tabgamma =
  Table[{gaFra, normfitconsts[damp, gaFra * gammaFrag]}, {gaFra, 15, 17, 1 / 5}];
```

```
ListPlot[tabgamma, Joined -> True,
  PlotMarkers -> Automatic, PlotStyle -> {Thick, Red}]
```

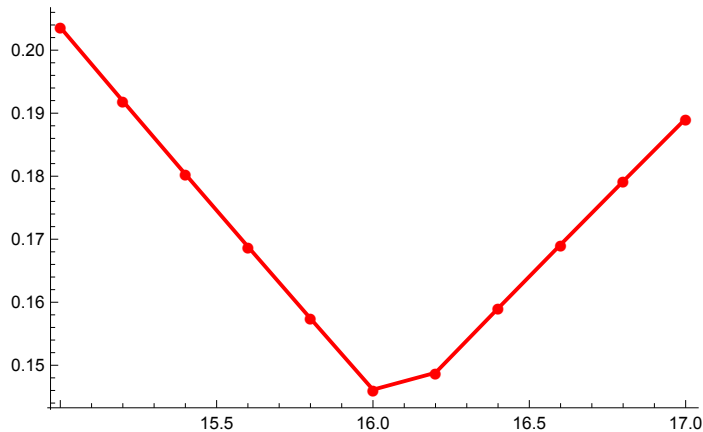

```
N[MinimalBy[tabgamma, Last]]
```

```
{{16., 0.146125}}
```

```
intgamma = Interpolation[tabgamma, x]
```

```
InterpolatingFunction[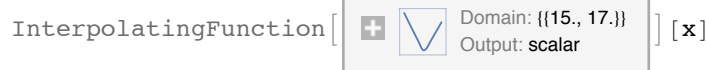 Domain: {{15., 17.}}  
Output: scalar][x]
```

```
mingamma = FindMinimum[intgamma, {x, 15, 17}]
```

```
InterpolatingFunction::dmval:
```

Input value {17.2642} lies outside the range of data in the interpolating function. Extrapolation will be used. >>

```
{0.145738, {x -> 16.0489}}
```

```
optent = x /. mingamma[[2]]
```

```
16.0489
```

```
optGaFra := optent * gammaFrag
```

```
iy = dsionyieldcrateranalysisparam[damp * 0.26 * MilliJouleToHartree, photonenergy,  
tauX, nintdata, True, True, 1 / 1000, optfNppN, 1 - optfNppN, optGaFra]
```

```
inyorm = 1 / Total[iy[[2 ;; 8]]] * iy
```

```
Total[iyorm[[2 ;; 8]]]
```

```
{0.968591, 0.0193645, 0.00903, 0.00147932, 0.00115015, 0.00035154, 0.0000321206,  
1.21413 × 10-6, 0.965355, 0.000584143, 1.78932 × 10-72, 3.86895 × 10-138}
```

```
{30.8382, 0.61653, 0.287499, 0.0470988, 0.0366187, 0.0111924, 0.00102266,  
0.0000386556, 30.7351, 0.018598, 5.69687 × 10-71, 1.2318 × 10-136}
```

```
1.
```

```
plotiy = Partition[Riffle[normOleg80, inyorm[[2 ;; 8]]], 2]
```

```
{{0.604006, 0.61653}, {0.287434, 0.287499},  
{0.0722227, 0.0470988}, {0.0271552, 0.0366187},  
{0.00918191, 0.0111924}, {0., 0.00102266}, {0., 0.0000386556}}
```

```
BarChart[plotiy, PlotRange → {-0.1, 0.9},
  ChartLabels → {Placed[{"N +", "N 2+", "N 3+", "N 4+", "N 5+", "N 6+", "N 7+"}, Below],
    Placed[{}, Above]},
  ChartLegends → Placed[{"Expt.", "γfrag"}, Top],
  ChartStyle → {Black, Red}, AxesLabel → {"", "Ỹ(ω)",
  AxesStyle → {{Arrowheads[Automatic], AbsoluteThickness[0.6]},
    {Arrowheads[Automatic], AbsoluteThickness[0.6]}},
  LabelStyle → {FontFamily → "Arial"},
  PlotLabel → {damp, optGaFra / gammaFrag,
    (iynorm[2 ;; 8] - normOleg80).Table[i, {i, 1, 7}]]]
```

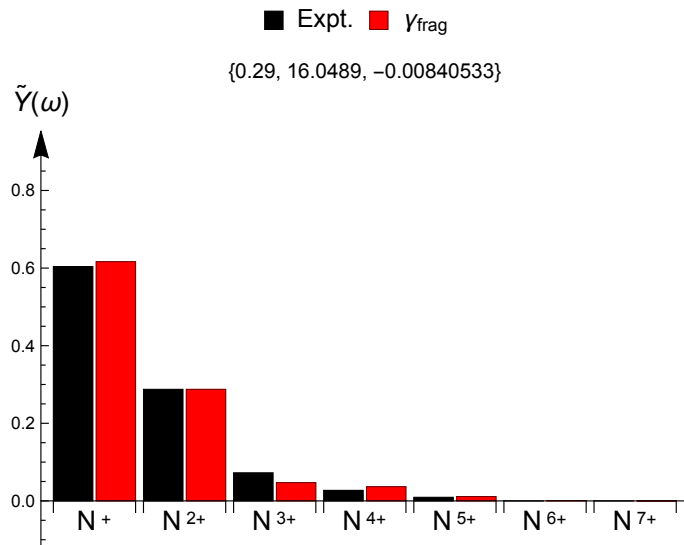

### 0.30

damp := 0.30

```
tabgamma =
  Table[{gaFra, normfitconsts[damp, gaFra * gammaFrag]}, {gaFra, 10, 20, 1 / 2}];
ListPlot[tabgamma, Joined -> True,
  PlotMarkers -> Automatic, PlotStyle -> {Thick, Red}]
```

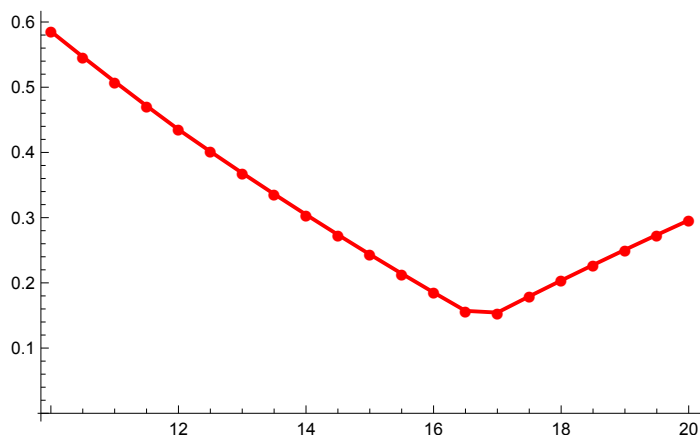

```
tabgamma =
  Table[{gaFra, normfitconsts[damp, gaFra * gammaFrag]}, {gaFra, 16, 18, 1 / 5}];
```

```
ListPlot[tabgamma, Joined -> True,
PlotMarkers -> Automatic, PlotStyle -> {Thick, Red}]
```

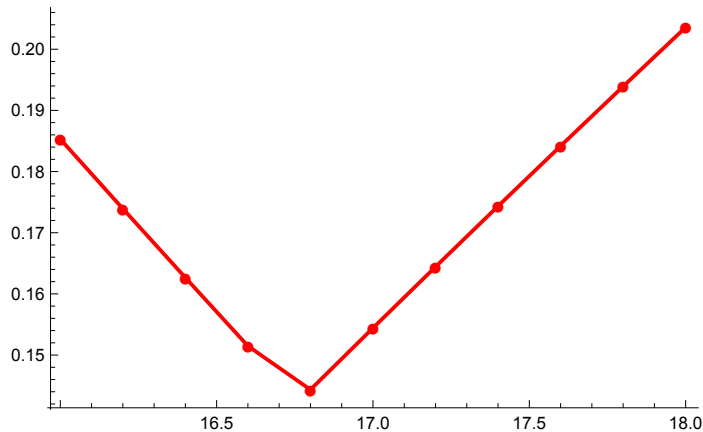

```
N[MinimalBy[tabgamma, Last]]
```

```
{{16.8, 0.14434}}
```

```
intgamma = Interpolation[tabgamma, x]
```

```
InterpolatingFunction[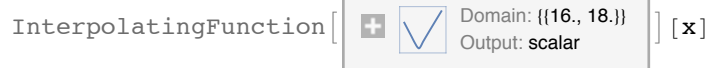 Domain: {{16., 18.}}  
Output: scalar][x]
```

```
mingamma = FindMinimum[intgamma, {x, 16, 18}]
```

```
InterpolatingFunction::dmval:
```

Input value {18.2642} lies outside the range of data in the interpolating function. Extrapolation will be used. >>

```
{0.14434, {x -> 16.8}}
```

```
optent = x /. mingamma[[2]]
```

```
16.8
```

```
optGaFra := optent * gammaFrag
```

```
iy = dsionyieldcrateranalysisparam[damp * 0.26 * MilliJouleToHartree, photonenergy,  
tauX, nintdata, True, True, 1 / 1000, optfNppN, 1 - optfNppN, optGaFra]
```

```
inyorm = 1 / Total[iy[[2 ;; 8]]] * iy
```

```
Total[iyorm[[2 ;; 8]]]
```

```
{0.967819, 0.0196877, 0.00924627, 0.00158912, 0.00122862, 0.00039041,  
0.0000370241, 1.45374 × 10-6, 0.96453, 0.000591681, 9.70701 × 10-76, 1.23411 × 10-141}}
```

```
{30.0746, 0.611788, 0.287325, 0.0493812, 0.038179, 0.0121319, 0.00115051,  
0.0000451745, 29.9724, 0.0183863, 3.01642 × 10-74, 3.83496 × 10-140}}
```

```
1.
```

```
plotiy = Partition[Riffle[normOleg80, inyorm[[2 ;; 8]]], 2]
```

```
{{0.604006, 0.611788}, {0.287434, 0.287325},  
{0.0722227, 0.0493812}, {0.0271552, 0.038179},  
{0.00918191, 0.0121319}, {0., 0.00115051}, {0., 0.0000451745}}
```

```
BarChart[plotiy, PlotRange → {-0.1, 0.9},
  ChartLabels → {Placed[{"N +", "N 2+", "N 3+", "N 4+", "N 5+", "N 6+", "N 7+"}, Below],
    Placed[{}, Above]},
  ChartLegends → Placed[{"Expt.", "γfrag"}, Top],
  ChartStyle → {Black, Red}, AxesLabel → {"", "Ỹ(ω)",
  AxesStyle → {{Arrowheads[Automatic], AbsoluteThickness[0.6]},
    {Arrowheads[Automatic], AbsoluteThickness[0.6]}},
  LabelStyle → {FontFamily → "Arial"},
  PlotLabel → {damp, optGaFra / gammaFrag,
    (iynorm[[2 ;; 8]] - normOleg80).Table[i, {i, 1, 7}]]]
```

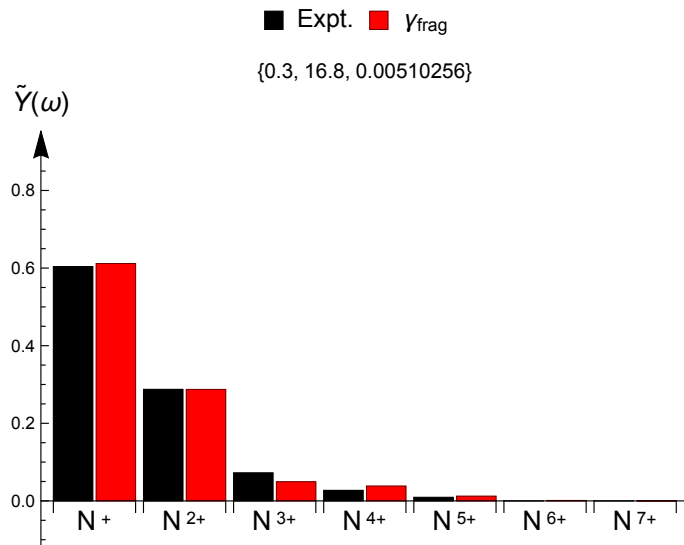

### 0.31

damp := 0.31

```
tabgamma =
  Table[{gaFra, normfitconsts[damp, gaFra * gammaFrag]}, {gaFra, 15, 25, 1 / 2}];
```

```
ListPlot[tabgamma, Joined -> True,
  PlotMarkers -> Automatic, PlotStyle -> {Thick, Red}]
```

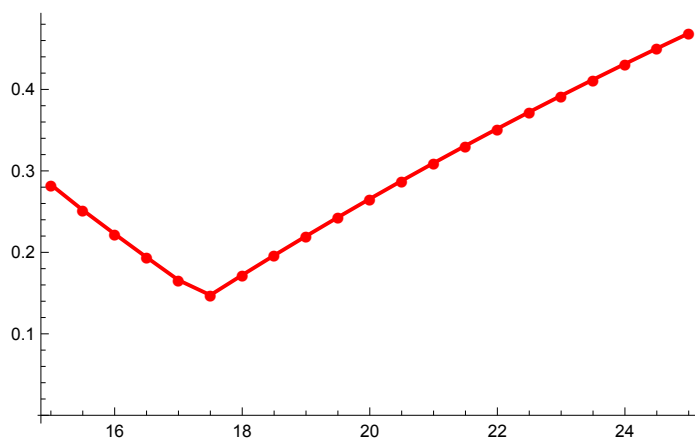

```
tabgamma = Table[
  {gaFra, normfitconsts[damp, gaFra * gammaFrag]}, {gaFra, 16.5, 18.5, 1 / 5}];
```

```
ListPlot[tabgamma, Joined -> True,
PlotMarkers -> Automatic, PlotStyle -> {Thick, Red}]
```

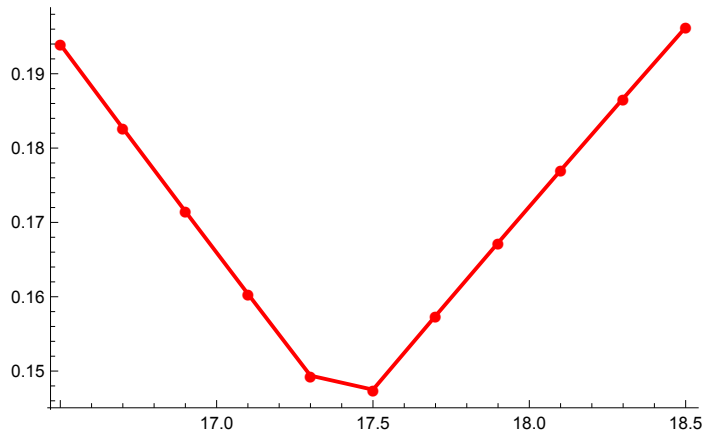

```
N[MinimalBy[tabgamma, Last]]
```

```
{{17.5, 0.147496}}
```

```
intgamma = Interpolation[tabgamma, x]
```

```
InterpolatingFunction[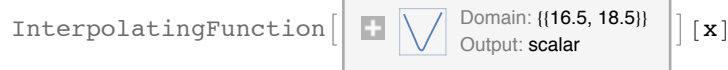 Domain: {{16.5, 18.5}}  
Output: scalar][x]
```

```
mingamma = FindMinimum[intgamma, {x, 16.5, 18.5}]
```

```
InterpolatingFunction::dmval:
```

Input value {18.7642} lies outside the range of data in the interpolating function. Extrapolation will be used. >>

```
{0.146945, {x -> 17.4374}}
```

```
optent = x /. mingamma[[2]]
```

```
17.4374
```

```
optGaFra := optent * gammaFrag
```

```
iy = dsionyieldcrateranalysisparam[damp * 0.26 * MilliJouleToHartree, photonenergy,  
tauX, nintdata, True, True, 1 / 1000, optfNppN, 1 - optfNppN, optGaFra]
```

```
inyorm = 1 / Total[iy[[2 ;; 8]]] * iy
```

```
Total[iyorm[[2 ;; 8]]]
```

```
{0.967062, 0.0199936, 0.00946534, 0.00169563,  
0.00130884, 0.000430895, 0.000042352, 1.72363 × 10-6,  
0.963722, 0.000598796, 3.01617 × 10-78, -1.11072 × 10-134}
```

```
{29.3597, 0.607, 0.287365, 0.0514788, 0.0397361, 0.0130818, 0.00128579,  
0.0000523288, 29.2583, 0.0181793, 9.157 × 10-77, -3.37211 × 10-133}
```

```
1.
```

```
plotiy = Partition[Riffle[normOleg80, inyorm[[2 ;; 8]]], 2]
```

```
{{0.604006, 0.607}, {0.287434, 0.287365},  
{0.0722227, 0.0514788}, {0.0271552, 0.0397361},  
{0.00918191, 0.0130818}, {0., 0.00128579}, {0., 0.0000523288}}
```

```
BarChart[plotiy, PlotRange → {-0.1, 0.9},
  ChartLabels → {Placed[{"N +", "N 2+", "N 3+", "N 4+", "N 5+", "N 6+", "N 7+"}, Below],
    Placed[{}, Above]},
  ChartLegends → Placed[{"Expt.", "γfrag"}, Top],
  ChartStyle → {Black, Red}, AxesLabel → {"", "Ỹ(ω)",
  AxesStyle → {{Arrowheads[Automatic], AbsoluteThickness[0.6]},
    {Arrowheads[Automatic], AbsoluteThickness[0.6]}},
  LabelStyle → {FontFamily → "Arial"},
  PlotLabel → {damp, optGaFra / gammaFrag,
    (iynorm[2 ;; 8] - normOleg80).Table[i, {i, 1, 7}]]]
```

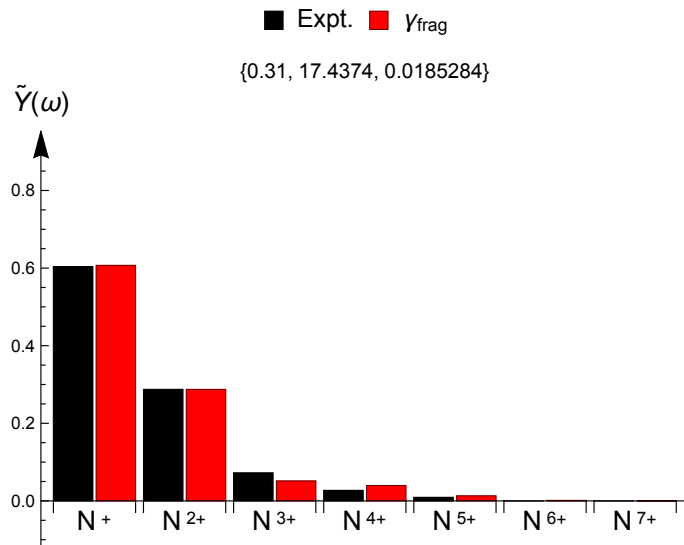

## 0.32

```
damp := 0.32
```

```
tabgamma =
  Table[{gaFra, normfitconsts[damp, gaFra * gammaFrag]}, {gaFra, 12, 22, 1 / 2}];
ListPlot[tabgamma, Joined -> True,
  PlotMarkers -> Automatic, PlotStyle -> {Thick, Red}]
```

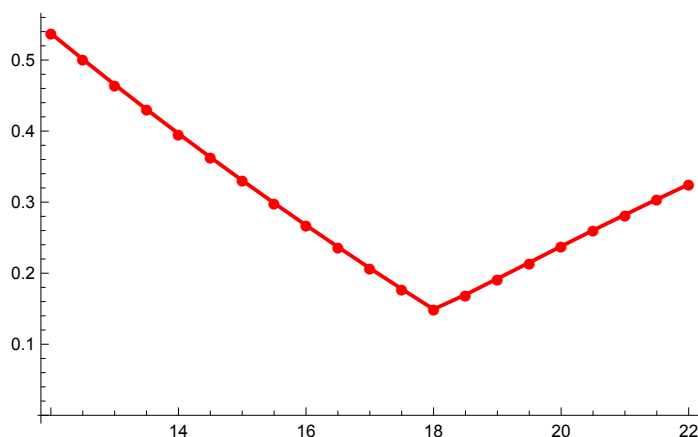

```
tabgamma =
  Table[{gaFra, normfitconsts[damp, gaFra * gammaFrag]}, {gaFra, 17, 19, 1 / 5}];
```

```
ListPlot[tabgamma, Joined -> True,
  PlotMarkers -> Automatic, PlotStyle -> {Thick, Red}]
```

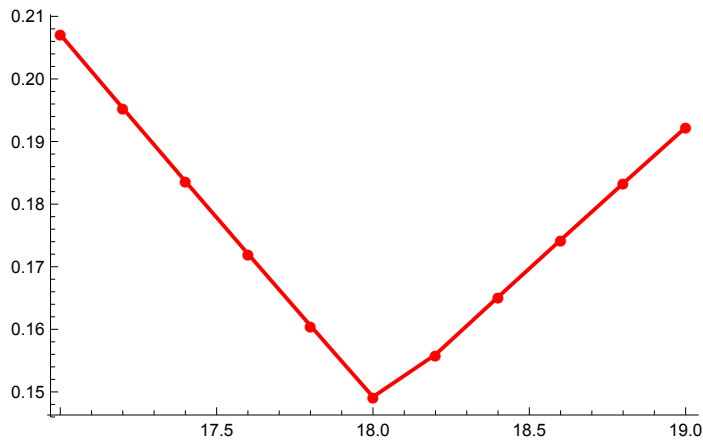

```
N[MinimalBy[tabgamma, Last]]
```

```
{{18., 0.149205}}
```

```
intgamma = Interpolation[tabgamma, x]
```

```
InterpolatingFunction[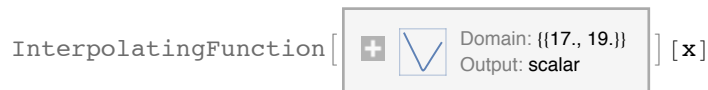 Domain: {{17., 19.}}  
Output: scalar][x]
```

```
mingamma = FindMinimum[intgamma, {x, 17, 19}]
```

```
InterpolatingFunction::dmval:
```

```
Input value {19.2642} lies outside the range of data in the interpolating function. Extrapolation will be used. >>
```

```
{0.149205, {x -> 18.}}
```

```
optent = x /. mingamma[[2]]
```

```
18.
```

```
optGaFra := optent * gammaFrag
```

```
iy = dsionyieldcrateranalysisparam[damp * 0.26 * MilliJouleToHartree, photonenergy,  
  tauX, nintdata, True, True, 1 / 1000, optfNppN, 1 - optfNppN, optGaFra]
```

```
iynorm = 1 / Total[iy[[2 ;; 8]]] * iy
```

```
Total[iynorm[[2 ;; 8]]]
```

```
{0.966318, 0.0202844, 0.0096838, 0.00180027,  
  0.00139062, 0.000473154, 0.0000481399, 2.02723 × 10-6,  
  0.962931, 0.000605511, 1.49093 × 10-62, 1.85731 × 10-108}
```

```
{28.6891, 0.602225, 0.287503, 0.0534485, 0.0412863, 0.0140475, 0.00142923,  
  0.0000601866, 28.5886, 0.0179771, 4.42642 × 10-61, 5.5142 × 10-107}
```

```
1.
```

```
plotiy = Partition[Riffle[normOleg80, iynorm[[2 ;; 8]]], 2]
```

```
{{0.604006, 0.602225}, {0.287434, 0.287503},  
  {0.0722227, 0.0534485}, {0.0271552, 0.0412863},  
  {0.00918191, 0.0140475}, {0., 0.00142923}, {0., 0.0000601866}}
```

```
BarChart[plotiy, PlotRange → {-0.1, 0.9},
  ChartLabels → {Placed[{"N +", "N 2+", "N 3+", "N 4+", "N 5+", "N 6+", "N 7+"}, Below],
    Placed[{}, Above]},
  ChartLegends → Placed[{"Expt.", "γfrag"}, Top],
  ChartStyle → {Black, Red}, AxesLabel → {"", "Ỹ(ω)"},
  AxesStyle → {{Arrowheads[Automatic], AbsoluteThickness[0.6]},
    {Arrowheads[Automatic], AbsoluteThickness[0.6]}},
  LabelStyle → {FontFamily → "Arial"},
  PlotLabel → {damp, optGaFra / gammaFrag,
    (iynorm[[2 ;; 8]] - normOleg80).Table[i, {i, 1, 7}]]}
```

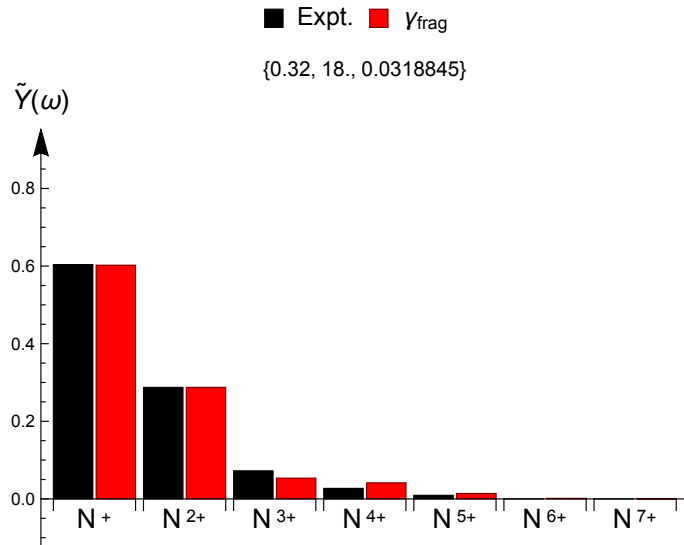

## Pulse energy for a 280 fs pulse with 280 fs fragmentation rate

```
tauX := 280 / t0ToFemtoSecond
optent := 4.971737
optGaFra := optent * gammaFrag
```

### 0.38

```
damp := 0.38
```

```
iy = dsionyieldcrateranalysisparam[damp * 0.26 * MilliJouleToHartree, photonenergy,
  tauX, nintdata, True, True, 1 / 1000, optfNppN, 1 - optfNppN, optGaFra]
iynorm = 1 / Total[iy[[2 ;; 8]]] * iy
Total[iynorm[[2 ;; 8]]]
```

```
{0.962113, 0.0216846, 0.0110348, 0.00218007, 0.00207056, 0.000800862, 0.000109742,
  6.69068 × 10-6, 0.958498, 0.000638571, 4.01935 × 10-24, -1.7145 × 10-109}
```

```
{25.3941, 0.572345, 0.291252, 0.0575411, 0.0546505, 0.021138, 0.00289654,
  0.000176594, 25.2987, 0.0168545, 1.06087 × 10-22, -4.52526 × 10-108}
```

```
1.
```

```

plotiy = Partition[Riffle[normOleg280, iynorm[[2 ;; 8]]], 2]
{{0.56634, 0.572345}, {0.291805, 0.291252},
 {0.0763903, 0.0575411}, {0.0364504, 0.0546505},
 {0.027387, 0.021138}, {0.00162698, 0.00289654}, {0., 0.000176594}}

BarChart[plotiy, PlotRange → {-0.1, 0.9},
 ChartLabels → {Placed[{"N +", "N 2+", "N 3+", "N 4+", "N 5+", "N 6+", "N 7+"}, Below],
   Placed[{}, Above]},
 ChartLegends → Placed[{"Expt.", "γfrag"}, Top],
 ChartStyle → {Black, Red}, AxesLabel → {"", "Ỹ(ω)"},
 AxesStyle → {{Arrowheads[Automatic], AbsoluteThickness[0.6]},
   {Arrowheads[Automatic], AbsoluteThickness[0.6]}},
 LabelStyle → {FontFamily → "Arial"},
 PlotLabel → {damp, optGaFra / gammaFrag,
   (iynorm[[2 ;; 8]] - normOleg280).Table[i, {i, 1, 7}]}]

```

■ Expt. ■ γ<sub>frag</sub>

{0.38, 4.97174, -0.00123957}

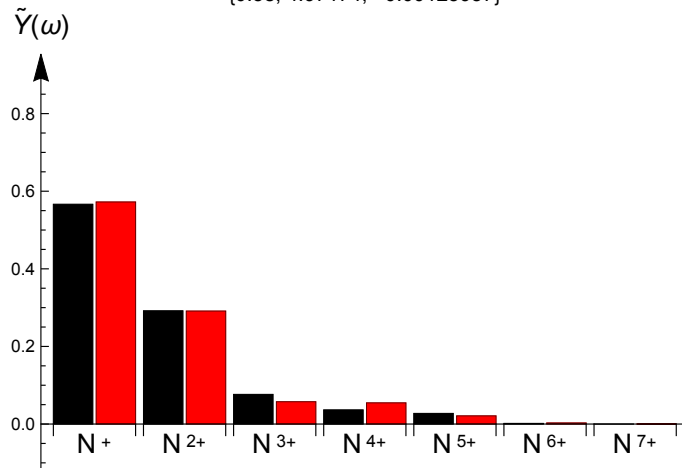

## Pulse energy for a 280 fs pulse with 80 fs fragmentation rate

```

tauX := 280 / t0ToFemtoSecond
optent := 16.800000
optGaFra := optent * gammaFrag

```

0.36

```
damp := 0.36
```

```

iy = dsionyieldcrateranalysisparam[damp * 0.26 * MilliJouleToHartree, photonenergy,
  tauX, nintdata, True, True, 1 / 1000, optfNppN, 1 - optfNppN, optGaFra]
iynorm = 1 / Total[iy[[2 ;; 8]]] * iy
Total[iynorm[[2 ;; 8]]]

```

```

{0.963676, 0.0224351, 0.00786429, 0.00340503,
 0.00156344, 0.000917978, 0.000129031,  $9.18254 \times 10^{-6}$ ,
 0.959919, 0.000628799,  $6.17453 \times 10^{-75}$ ,  $-7.48101 \times 10^{-136}$ }

```

```

{26.53, 0.617638, 0.216504, 0.0937405, 0.0430413, 0.0252719, 0.00355222,
 0.000252795, 26.4265, 0.0173108,  $1.69984 \times 10^{-73}$ ,  $-2.05952 \times 10^{-134}$ }

```

1.

```

plotiy = Partition[Riffle[normOleg280, iynorm[[2 ;; 8]]], 2]

```

```

{{0.56634, 0.617638}, {0.291805, 0.216504},
 {0.0763903, 0.0937405}, {0.0364504, 0.0430413},
 {0.027387, 0.0252719}, {0.00162698, 0.00355222}, {0., 0.000252795}}

```

```

BarChart[plotiy, PlotRange → {-0.1, 0.9},
  ChartLabels → {Placed[{"N +", "N 2+", "N 3+", "N 4+", "N 5+", "N 6+", "N 7+"}, Below],
    Placed[{}, Above]},
  ChartLegends → Placed[{"Expt.", " $\gamma_{frag}$ "}, Top],
  ChartStyle → {Black, Red}, AxesLabel → {"", " $\tilde{Y}(\omega)$ "},
  AxesStyle → {{Arrowheads[Automatic], AbsoluteThickness[0.6]},
    {Arrowheads[Automatic], AbsoluteThickness[0.6]}},
  LabelStyle → {FontFamily → "Arial"},
  PlotLabel → {damp, optGaFra / gammaFrag,
    (iynorm[[2 ;; 8]] - normOleg280).Table[i, {i, 1, 7}]]}

```

■ Expt. ■  $\gamma_{frag}$

{0.36, 16.8, -0.0181457}

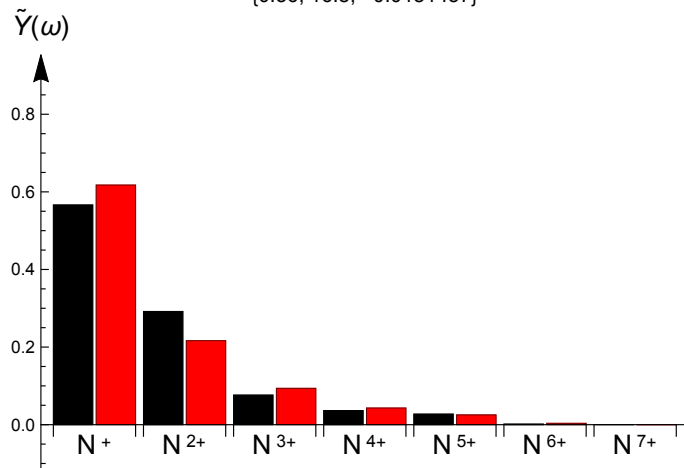

## 0.37

damp := 0.37

```

iy = dsionyieldcrateranalysisparam[damp * 0.26 * MilliJouleToHartree, photonenergy,
  tauX, nintdata, True, True, 1 / 1000, optfNppN, 1 - optfNppN, optGaFra]
iynorm = 1 / Total[iy[[2 ;; 8]]] * iy
Total[iynorm[[2 ;; 8]]]

{0.962999, 0.0226802, 0.0080301, 0.00352052, 0.00163897, 0.000979253, 0.000141527,
  0.0000103453, 0.959202, 0.000633826, 6.22133 × 10-75, 3.16044 × 10-131}

{26.0263, 0.612964, 0.217024, 0.0951467, 0.0442953, 0.0264656,
  0.00382496, 0.000279594, 25.9237, 0.01713, 1.6814 × 10-73, 8.54153 × 10-130}

1.

```

```

plotiy = Partition[Riffle[normOleg280, iynorm[[2 ;; 8]]], 2]
{{0.56634, 0.612964}, {0.291805, 0.217024},
 {0.0763903, 0.0951467}, {0.0364504, 0.0442953},
 {0.027387, 0.0264656}, {0.00162698, 0.00382496}, {0., 0.000279594}}

BarChart[plotiy, PlotRange → {-0.1, 0.9},
  ChartLabels → {Placed[{"N +", "N 2+", "N 3+", "N 4+", "N 5+", "N 6+", "N 7+"}, Below],
    Placed[{}, Above]},
  ChartLegends → Placed[{"Expt.", "γfrag"}, Top],
  ChartStyle → {Black, Red}, AxesLabel → {"", "Ỹ(ω)"},
  AxesStyle → {{Arrowheads[Automatic], AbsoluteThickness[0.6]},
    {Arrowheads[Automatic], AbsoluteThickness[0.6]}},
  LabelStyle → {FontFamily → "Arial"},
  PlotLabel → {damp, optGaFra / gammaFrag,
    (iynorm[[2 ;; 8]] - normOleg280).Table[i, {i, 1, 7}]}]

```

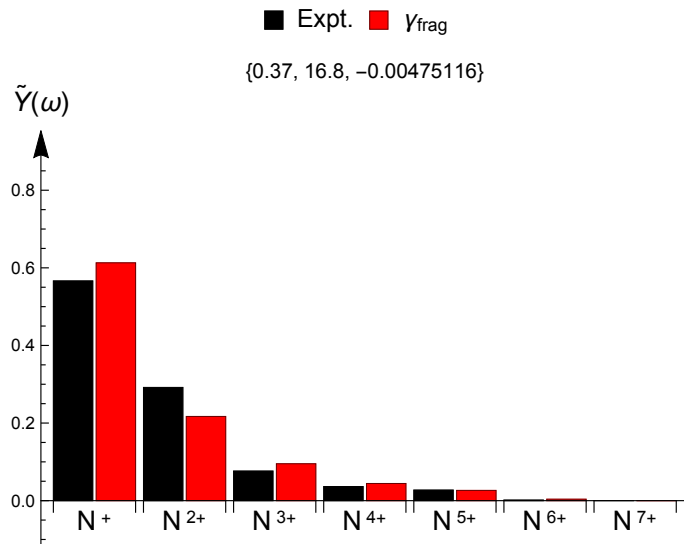

0.38

damp := 0.38

```
iy = dsionyieldcrateranalysisparam[damp * 0.26 * MilliJouleToHartree, photonenergy,
  tauX, nintdata, True, True, 1 / 1000, optfNppN, 1 - optfNppN, optGaFra]
iynorm = 1 / Total[iy[[2 ;; 8]]] * iy
Total[iynorm[[2 ;; 8]]]
```

```
{0.962334, 0.0229149, 0.00819223, 0.00363495, 0.0017152, 0.00104233, 0.000154782,
  0.000011613, 0.958498, 0.000638571, 6.27243 × 10-75, 8.61127 × 10-129}
```

```
{25.5492, 0.608371, 0.217497, 0.0965049, 0.0455371, 0.0276729, 0.00410932,
  0.000308314, 25.4473, 0.0169535, 1.66528 × 10-73, 2.28622 × 10-127}
```

1.

```
plotiy = Partition[Riffle[normOleg280, iynorm[[2 ;; 8]]], 2]
```

```
{{0.56634, 0.608371}, {0.291805, 0.217497},
  {0.0763903, 0.0965049}, {0.0364504, 0.0455371},
  {0.027387, 0.0276729}, {0.00162698, 0.00410932}, {0., 0.000308314}}
```

```
BarChart[plotiy, PlotRange → {-0.1, 0.9},
  ChartLabels → {Placed[{"N +", "N 2+", "N 3+", "N 4+", "N 5+", "N 6+", "N 7+"}, Below],
    Placed[{}, Above]},
  ChartLegends → Placed[{"Expt.", "γfrag"}, Top],
  ChartStyle → {Black, Red}, AxesLabel → {"", "Ỹ(ω)"},
  AxesStyle → {{Arrowheads[Automatic], AbsoluteThickness[0.6]},
    {Arrowheads[Automatic], AbsoluteThickness[0.6]}},
  LabelStyle → {FontFamily → "Arial"},
  PlotLabel → {damp, optGaFra / gammaFrag,
    (iynorm[[2 ;; 8]] - normOleg280).Table[i, {i, 1, 7}]}]
```

■ Expt. ■ γ<sub>frag</sub>

{0.38, 16.8, 0.00858639}

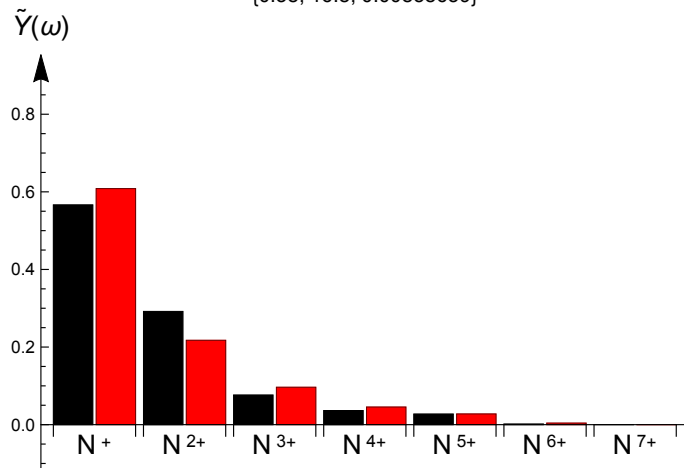

0.39

damp := 0.39

```

iy = dsionyieldcrateranalysisparam[damp * 0.26 * MilliJouleToHartree, photonenergy,
  tauX, nintdata, True, True, 1 / 1000, optfNppN, 1 - optfNppN, optGaFra]
iynorm = 1 / Total[iy[[2 ;; 8]]] * iy
Total[iynorm[[2 ;; 8]]]

```

```

{0.961681, 0.0231395, 0.00835071, 0.00374827, 0.00179205, 0.00110716, 0.00016881,
  0.0000129912, 0.957808, 0.000643049, 6.30556 × 10-75, -4.7787 × 10-129}

```

```

{25.0964, 0.603857, 0.217923, 0.0978162, 0.046766, 0.0288928, 0.00440533,
  0.000339024, 24.9953, 0.0167812, 1.64552 × 10-73, -1.24707 × 10-127}

```

1.

```

plotiy = Partition[Riffle[normOleg280, iynorm[[2 ;; 8]]], 2]

```

```

{{0.56634, 0.603857}, {0.291805, 0.217923},
 {0.0763903, 0.0978162}, {0.0364504, 0.046766},
 {0.027387, 0.0288928}, {0.00162698, 0.00440533}, {0., 0.000339024}}

```

```

BarChart[plotiy, PlotRange → {-0.1, 0.9},
  ChartLabels → {Placed[{"N +", "N 2+", "N 3+", "N 4+", "N 5+", "N 6+", "N 7+"}, Below],
    Placed[{}, Above]},
  ChartLegends → Placed[{"Expt.", "γfrag"}, Top],
  ChartStyle → {Black, Red}, AxesLabel → {"", "Ỹ(ω)"},
  AxesStyle → {{Arrowheads[Automatic], AbsoluteThickness[0.6]},
    {Arrowheads[Automatic], AbsoluteThickness[0.6]}},
  LabelStyle → {FontFamily → "Arial"},
  PlotLabel → {damp, optGaFra / gammaFrag,
    (iynorm[[2 ;; 8]] - normOleg280).Table[i, {i, 1, 7}]]}

```

■ Expt. ■ γ<sub>frag</sub>

{0.39, 16.8, 0.0218659}

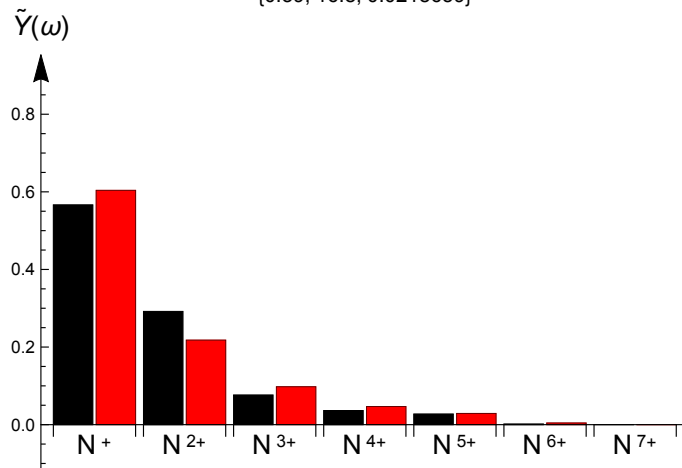

0.40

damp := 0.40

```
iy = dsionyieldcrateranalysisparam[damp * 0.26 * MilliJouleToHartree, photonenergy,
  tauX, nintdata, True, True, 1 / 1000, optfNppN, 1 - optfNppN, optGaFra]
iynorm = 1 / Total[iy[[2 ;; 8]]] * iy
Total[iynorm[[2 ;; 8]]]
```

```
{0.961038, 0.0233546, 0.00850558, 0.00386041, 0.00186945, 0.0011737, 0.000183628,
  0.0000144857, 0.957131, 0.000647275, 6.34682 × 10-75, 7.63354 × 10-131}
```

```
{24.6661, 0.599422, 0.218305, 0.0990818, 0.0479814, 0.0301243, 0.00471303,
  0.000371793, 24.5658, 0.016613, 1.62898 × 10-73, 1.95923 × 10-129}
```

1.

```
plotiy = Partition[Riffle[normOleg280, iynorm[[2 ;; 8]]], 2]
```

```
{{0.56634, 0.599422}, {0.291805, 0.218305},
  {0.0763903, 0.0990818}, {0.0364504, 0.0479814},
  {0.027387, 0.0301243}, {0.00162698, 0.00471303}, {0., 0.000371793}}
```

```
BarChart[plotiy, PlotRange → {-0.1, 0.9},
  ChartLabels → {Placed[{"N +", "N 2+", "N 3+", "N 4+", "N 5+", "N 6+", "N 7+"}, Below],
    Placed[{}, Above]},
  ChartLegends → Placed[{"Expt.", "γfrag"}, Top],
  ChartStyle → {Black, Red}, AxesLabel → {"", "Ỹ(ω)"},
  AxesStyle → {{Arrowheads[Automatic], AbsoluteThickness[0.6]},
    {Arrowheads[Automatic], AbsoluteThickness[0.6]}},
  LabelStyle → {FontFamily → "Arial"},
  PlotLabel → {damp, optGaFra / gammaFrag,
    (iynorm[[2 ;; 8]] - normOleg280).Table[i, {i, 1, 7}]}]
```

■ Expt. ■ γ<sub>frag</sub>

{0.4, 16.8, 0.0350866}

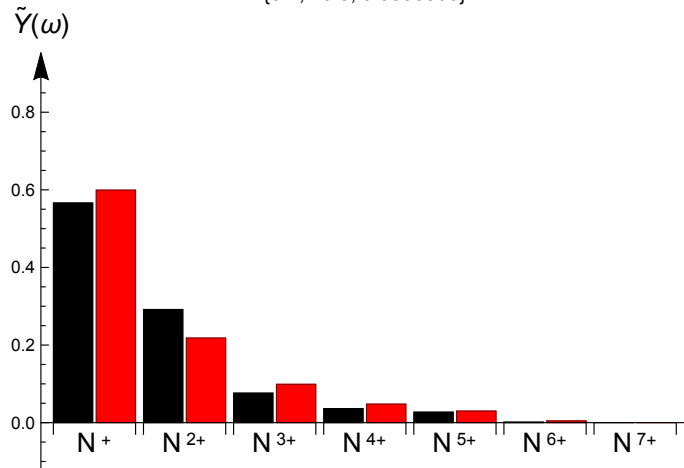

## Pulse energy for a 80 fs pulse with 280 fs fragmentation rate

```
tauX := 80 / t0ToFemtoSecond
optent := 4.971737
optGaFra := optent * gammaFrag
```

## 0.28

```
damp := 0.28
```

```
iy = dsionyieldcrateranalysisparam[damp * 0.26 * MilliJouleToHartree, photonenergy,  
tauX, nintdata, True, True, 1 / 1000, optfNppN, 1 - optfNppN, optGaFra]
```

```
iynorm = 1 / Total[iy[[2 ;; 8]]] * iy
```

```
Total[iynorm[[2 ;; 8]]]
```

```
{0.969279, 0.01848, 0.0100733, 0.000786984, 0.00111119, 0.000247424, 0.0000210723,  
6.54055 × 10-7, 0.966197, 0.000576154, 3.11164 × 10-24, 4.3326 × 10-111}
```

```
{31.5514, 0.601551, 0.3279, 0.0256175, 0.0361707, 0.00805403, 0.000685932,  
0.0000212904, 31.4511, 0.0187547, 1.01288 × 10-22, 1.41032 × 10-109}
```

```
1.
```

```
plotiy = Partition[Riffle[normOleg80, iynorm[[2 ;; 8]]], 2]
```

```
{{0.604006, 0.601551}, {0.287434, 0.3279},  
{0.0722227, 0.0256175}, {0.0271552, 0.0361707},  
{0.00918191, 0.00805403}, {0., 0.000685932}, {0., 0.0000212904}}
```

```
BarChart[plotiy, PlotRange → {-0.1, 0.9},  
ChartLabels → {Placed[{"N +", "N 2+", "N 3+", "N 4+", "N 5+", "N 6+", "N 7+"}, Below],  
Placed[{}, Above]},  
ChartLegends → Placed[{"Expt.", "γfrag"}, Top],  
ChartStyle → {Black, Red}, AxesLabel → {"", "Ỹ(ω)"},  
AxesStyle → {{Arrowheads[Automatic], AbsoluteThickness[0.6]},  
{Arrowheads[Automatic], AbsoluteThickness[0.6]}},  
LabelStyle → {FontFamily → "Arial"},  
PlotLabel → {damp, optGaFra / gammaFrag,  
(iynorm[[2 ;; 8]] - normOleg80).Table[i, {i, 1, 7}]}]
```

■ Expt. ■ γ<sub>frag</sub>

{0.28, 4.97174, -0.0266522}

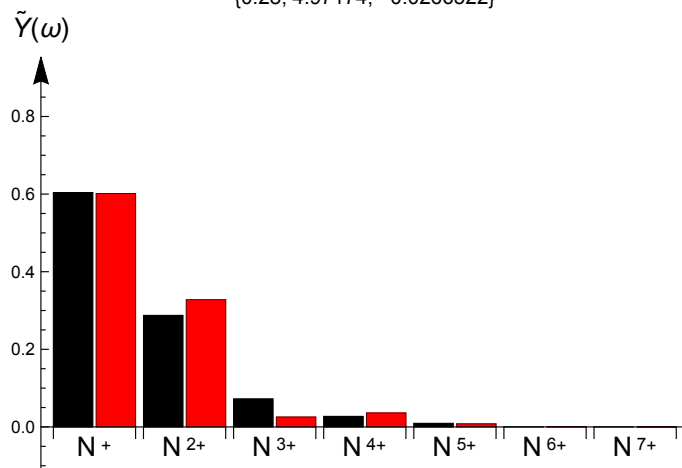

## 0.29

```
damp := 0.29
```

```
iy = dsionyieldcrateranalysisparam[damp * 0.26 * MilliJouleToHartree, photonenergy,
  tauX, nintdata, True, True, 1 / 1000, optfNppN, 1 - optfNppN, optGaFra]
iynorm = 1 / Total[iy[[2 ;; 8]]] * iy
Total[iynorm[[2 ;; 8]]]
```

```
{0.968482, 0.0187611, 0.0104246, 0.000834389,
  0.00119762, 0.000274843, 0.0000242934, 7.79219 × 10-7,
  0.965355, 0.000584142, 3.15605 × 10-24, 9.87595 × 10-114}
```

```
{30.7283, 0.595256, 0.330756, 0.0264737, 0.0379984, 0.0087203, 0.000770789,
  0.0000247233, 30.6291, 0.0185338, 1.00136 × 10-22, 3.13347 × 10-112}
```

1.

```
plotiy = Partition[Riffle[normOleg80, iynorm[[2 ;; 8]]], 2]
```

```
{{0.604006, 0.595256}, {0.287434, 0.330756},
  {0.0722227, 0.0264737}, {0.0271552, 0.0379984},
  {0.00918191, 0.0087203}, {0., 0.000770789}, {0., 0.0000247233}}
```

```
BarChart[plotiy, PlotRange → {-0.1, 0.9},
  ChartLabels → {Placed[{"N +", "N 2+", "N 3+", "N 4+", "N 5+", "N 6+", "N 7+"}, Below],
    Placed[{}, Above]},
  ChartLegends → Placed[{"Expt.", "γfrag"}, Top],
  ChartStyle → {Black, Red}, AxesLabel → {"", "Ỹ(ω)"},
  AxesStyle → {{Arrowheads[Automatic], AbsoluteThickness[0.6]},
    {Arrowheads[Automatic], AbsoluteThickness[0.6]}},
  LabelStyle → {FontFamily → "Arial"},
  PlotLabel → {damp, optGaFra / gammaFrag,
    (iynorm[[2 ;; 8]] - normOleg80).Table[i, {i, 1, 7}]]}
```

■ Expt. ■ γ<sub>frag</sub>

{0.29, 4.97174, -0.0134907}

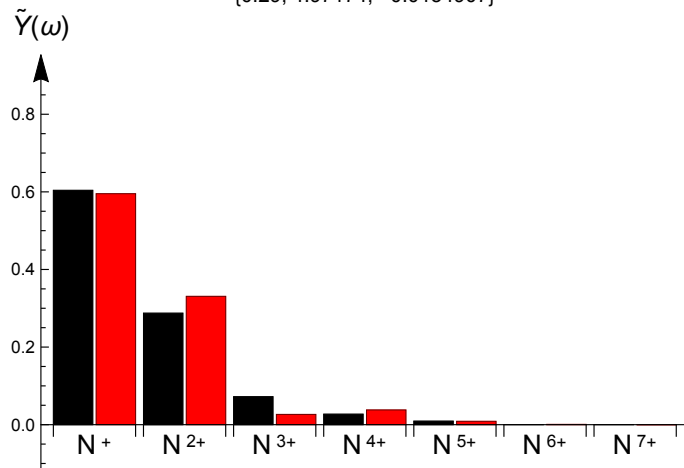

## 0.30

damp := 0.30

```

iy = dsionyieldcrateranalysisparam[damp * 0.26 * MilliJouleToHartree, photonenergy,
  tauX, nintdata, True, True, 1 / 1000, optfNppN, 1 - optfNppN, optGaFra]
iynorm = 1 / Total[iy[[2 ;; 8]]] * iy
Total[iynorm[[2 ;; 8]]]

{0.9677, 0.0190279, 0.0107701, 0.000882365, 0.00128648, 0.000304011, 0.0000278561,
  9.2239 × 10-7, 0.96453, 0.000591681, 3.20838 × 10-24, 1.04816 × 10-111}

{29.9602, 0.589106, 0.333443, 0.0273182, 0.0398296, 0.00941223, 0.000862429,
  0.0000285574, 29.862, 0.0183186, 9.93321 × 10-23, 3.24512 × 10-110}

1.

```

```

plotiy = Partition[Riffle[normOleg80, iynorm[[2 ;; 8]]], 2]
{{0.604006, 0.589106}, {0.287434, 0.333443},
 {0.0722227, 0.0273182}, {0.0271552, 0.0398296},
 {0.00918191, 0.00941223}, {0., 0.000862429}, {0., 0.0000285574}}

BarChart[plotiy, PlotRange → {-0.1, 0.9},
  ChartLabels → {Placed[{"N+", "N2+", "N3+", "N4+", "N5+", "N6+", "N7+"}, Below],
    Placed[{}, Above]},
  ChartLegends → Placed[{"Expt.", "γfrag"}, Top],
  ChartStyle → {Black, Red}, AxesLabel → {"", "Ỹ(ω)"},
  AxesStyle → {{Arrowheads[Automatic], AbsoluteThickness[0.6]},
    {Arrowheads[Automatic], AbsoluteThickness[0.6]}},
  LabelStyle → {FontFamily → "Arial"},
  PlotLabel → {damp, optGaFra / gammaFrag,
    (iynorm[[2 ;; 8]] - normOleg80).Table[i, {i, 1, 7}]]}

```

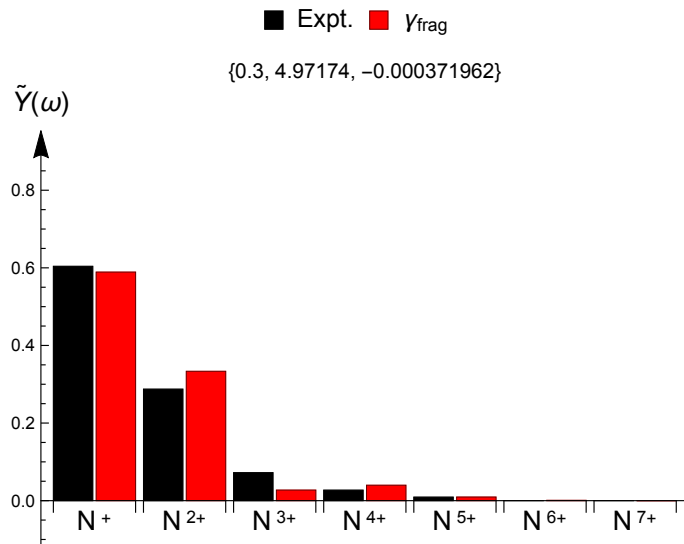

### 0.31

```
damp := 0.31
```

```

iy = dsionyieldcrateranalysisparam[damp * 0.26 * MilliJouleToHartree, photonenergy,
  tauX, nintdata, True, True, 1 / 1000, optfNppN, 1 - optfNppN, optGaFra]
iynorm = 1 / Total[iy[[2 ;; 8]]] * iy
Total[iynorm[[2 ;; 8]]]

```

```

{0.966933, 0.0192811, 0.0111094, 0.000930847,
 0.00137764, 0.000334945, 0.0000317802,  $1.08532 \times 10^{-6}$ ,
 0.963722, 0.000598795,  $3.23475 \times 10^{-24}$ ,  $-1.76045 \times 10^{-112}$ }

```

```

{29.2418, 0.583096, 0.335968, 0.0281505, 0.0416623, 0.0101294, 0.000961091,
 0.0000328221, 29.1447, 0.0181087,  $9.78248 \times 10^{-23}$ ,  $-5.32393 \times 10^{-111}$ }

```

1.

```

plotiy = Partition[Riffle[normOleg80, iynorm[[2 ;; 8]]], 2]

```

```

{{0.604006, 0.583096}, {0.287434, 0.335968},
 {0.0722227, 0.0281505}, {0.0271552, 0.0416623},
 {0.00918191, 0.0101294}, {0., 0.000961091}, {0., 0.0000328221}}

```

```

BarChart[plotiy, PlotRange → {-0.1, 0.9},
  ChartLabels → {Placed[{"N +", "N 2+", "N 3+", "N 4+", "N 5+", "N 6+", "N 7+"}, Below],
    Placed[{}, Above]},
  ChartLegends → Placed[{"Expt.", " $\gamma_{frag}$ "}, Top],
  ChartStyle → {Black, Red}, AxesLabel → {"", " $\tilde{Y}(\omega)$ "},
  AxesStyle → {{Arrowheads[Automatic], AbsoluteThickness[0.6]},
    {Arrowheads[Automatic], AbsoluteThickness[0.6]}},
  LabelStyle → {FontFamily → "Arial"},
  PlotLabel → {damp, optGaFra / gammaFrag,
    (iynorm[[2 ;; 8]] - normOleg80).Table[i, {i, 1, 7}]]}

```

■ Expt. ■  $\gamma_{frag}$

{0.31, 4.97174, 0.0127035}

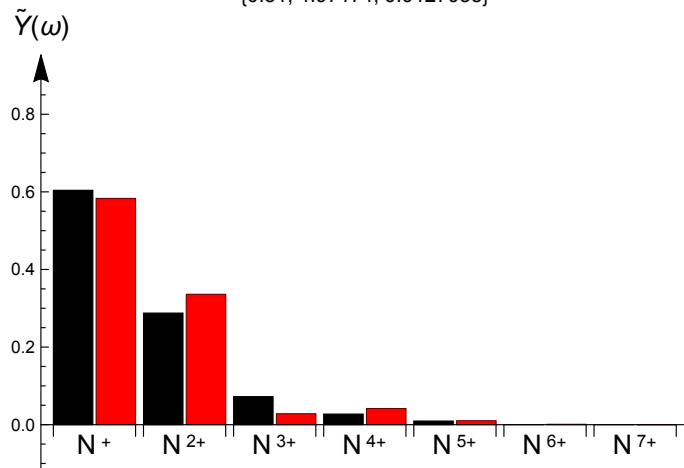

## 0.32

damp := 0.32

```

iy = dsionyieldcrateranalysisparam[damp * 0.26 * MilliJouleToHartree, photonenergy,
  tauX, nintdata, True, True, 1 / 1000, optfNppN, 1 - optfNppN, optGaFra]
iynorm = 1 / Total[iy[[2 ;; 8]]] * iy
Total[iynorm[[2 ;; 8]]]

{0.96618, 0.0195215, 0.0114425, 0.00097977, 0.00147097, 0.00036766, 0.0000360857,
  1.26986 × 10-6, 0.962931, 0.00060551, 3.2844 × 10-24, 2.04676 × 10-112}

{28.5684, 0.577222, 0.338338, 0.0289703, 0.0434942, 0.0108711, 0.001067,
  0.0000375477, 28.4724, 0.017904, 9.71145 × 10-23, 6.05196 × 10-111}

1.

plotiy = Partition[Riffle[normOleg80, iynorm[[2 ;; 8]]], 2]
{{0.604006, 0.577222}, {0.287434, 0.338338},
 {0.0722227, 0.0289703}, {0.0271552, 0.0434942},
 {0.00918191, 0.0108711}, {0., 0.001067}, {0., 0.0000375477}}

BarChart[plotiy, PlotRange → {-0.1, 0.9},
  ChartLabels → {Placed[{"N+", "N2+", "N3+", "N4+", "N5+", "N6+", "N7+"}, Below],
    Placed[{}, Above]},
  ChartLegends → Placed[{"Expt.", "γfrag"}, Top],
  ChartStyle → {Black, Red}, AxesLabel → {"", "Ỹ(ω)"},
  AxesStyle → {{Arrowheads[Automatic], AbsoluteThickness[0.6]},
    {Arrowheads[Automatic], AbsoluteThickness[0.6]}},
  LabelStyle → {FontFamily → "Arial"},
  PlotLabel → {damp, optGaFra / gammaFrag,
    (iynorm[[2 ;; 8]] - normOleg80).Table[i, {i, 1, 7}]]}

```

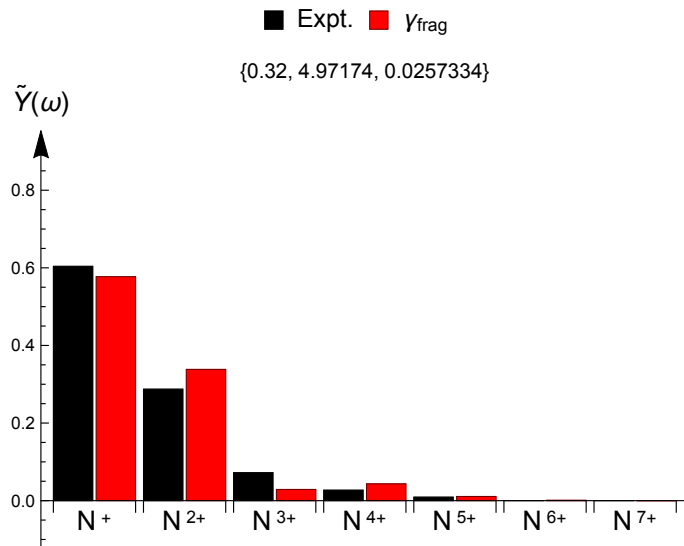

## Pulse energy for a 80 fs pulse with 80 fs fragmentation rate

```

tauX := 80 / t0ToFemtoSecond
optent := 16.800000
optGaFra := optent * gammaFrag

```

## 0.30

```
damp := 0.30
```

```
iy = dsionyieldcrateranalysisparam[damp * 0.26 * MilliJouleToHartree, photonenergy,
  tauX, nintdata, True, True, 1 / 1000, optfNppN, 1 - optfNppN, optGaFra]
```

```
iynorm = 1 / Total[iy[[2 ;; 8]]] * iy
```

```
Total[iynorm[[2 ;; 8]]]
```

```
{0.967819, 0.0196877, 0.00924627, 0.00158912,
 0.00122862, 0.00039041, 0.0000370241, 1.45374 × 10-6,
 0.96453, 0.000591681, 9.46339 × 10-76, -8.58011 × 10-130}
```

```
{30.0746, 0.611788, 0.287325, 0.0493812, 0.038179, 0.0121319, 0.00115051,
 0.0000451745, 29.9724, 0.0183863, 2.94071 × 10-74, -2.66624 × 10-128}
```

```
1.
```

```
plotiy = Partition[Riffle[normOleg80, iynorm[[2 ;; 8]]], 2]
```

```
{{0.604006, 0.611788}, {0.287434, 0.287325},
 {0.0722227, 0.0493812}, {0.0271552, 0.038179},
 {0.00918191, 0.0121319}, {0., 0.00115051}, {0., 0.0000451745}}
```

```
BarChart[plotiy, PlotRange → {-0.1, 0.9},
```

```
ChartLabels → {Placed[{"N +", "N 2+", "N 3+", "N 4+", "N 5+", "N 6+", "N 7+"}, Below],
  Placed[{}, Above]},
```

```
ChartLegends → Placed[{"Expt.", "γfrag"}, Top],
```

```
ChartStyle → {Black, Red}, AxesLabel → {"", "Ỹ(ω)",
```

```
AxesStyle → {{Arrowheads[Automatic], AbsoluteThickness[0.6]},
  {Arrowheads[Automatic], AbsoluteThickness[0.6]}},
```

```
LabelStyle → {FontFamily → "Arial"},
```

```
PlotLabel → {damp, optGaFra / gammaFrag,
  (iynorm[[2 ;; 8]] - normOleg80).Table[i, {i, 1, 7}]]}
```

■ Expt. ■ γ<sub>frag</sub>

{0.3, 16.8, 0.00510256}

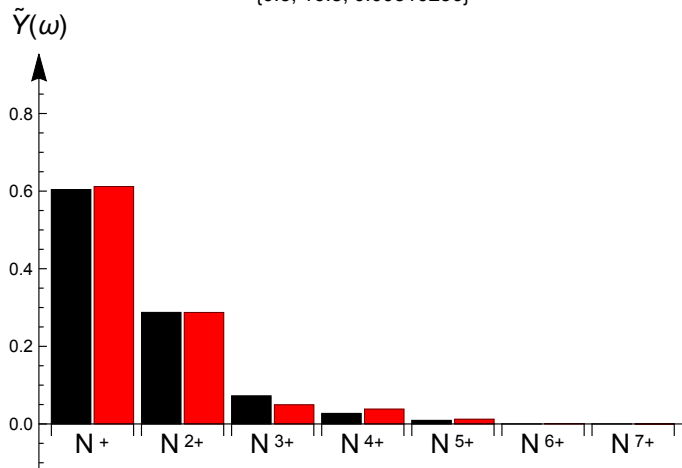

Pulse energy for a 7 fs pulse with 280 fs fragmentation

## rate

```
tauX := 7 / t0ToFemtoSecond
optent := 4.971737
optGaFra := optent * gammaFrag
```

## 0.12

```
damp := 0.12
```

```
iy = dsionyieldcrateranalysisparam[damp * 0.26 * MilliJouleToHartree, photonenergy,
  tauX, nintdata, True, True, 1 / 1000, optfNppN, 1 - optfNppN, optGaFra]
```

```
inyorm = 1 / Total[iy[[2 ;; 8]]] * iy
```

```
Total[inyorm[[2 ;; 8]]]
```

```
{0.984496, 0.0112923, 0.00400593, 0.000141148,
  0.0000577443,  $6.65158 \times 10^{-6}$ ,  $1.03025 \times 10^{-7}$ ,  $3.39041 \times 10^{-10}$ ,
   $0.982596$ ,  $0.000359602$ ,  $1.93483 \times 10^{-24}$ ,  $-3.77396 \times 10^{-174}$ }
```

```
{63.5001, 0.728353, 0.258383, 0.00910404, 0.00372451, 0.000429027,  $6.6451 \times 10^{-6}$ ,
   $2.18681 \times 10^{-8}$ , 63.3775, 0.0231944,  $1.24796 \times 10^{-22}$ ,  $-2.43421 \times 10^{-172}$ }
```

```
1.
```

```
plotiy = Partition[Riffle[normOleg7, inyorm[[2 ;; 8]]], 2]
```

```
{ {0.694746, 0.728353}, {0.275684, 0.258383},
  {0.0293036, 0.00910404}, {0.000266625, 0.00372451},
  {0., 0.000429027}, {0.,  $6.6451 \times 10^{-6}$ }, {0.,  $2.18681 \times 10^{-8}$ }}
```

```
BarChart[plotiy, PlotRange → {-0.1, 0.9},
  ChartLabels → {Placed[{"N +", "N 2+", "N 3+", "N 4+", "N 5+", "N 6+", "N 7+"}, Below],
    Placed[{}, Above]},
  ChartLegends → Placed[{"Expt.", "γfrag"}, Top],
  ChartStyle → {Black, Red}, AxesLabel → {"", "Ỹ(ω)"},
  AxesStyle → {{Arrowheads[Automatic], AbsoluteThickness[0.6]},
    {Arrowheads[Automatic], AbsoluteThickness[0.6]}},
  LabelStyle → {FontFamily → "Arial"},
  PlotLabel → {damp, optGaFra / gammaFrag,
    (iynorm[[2 ;; 8]] - normOleg7).Table[i, {i, 1, 7}]]]
```

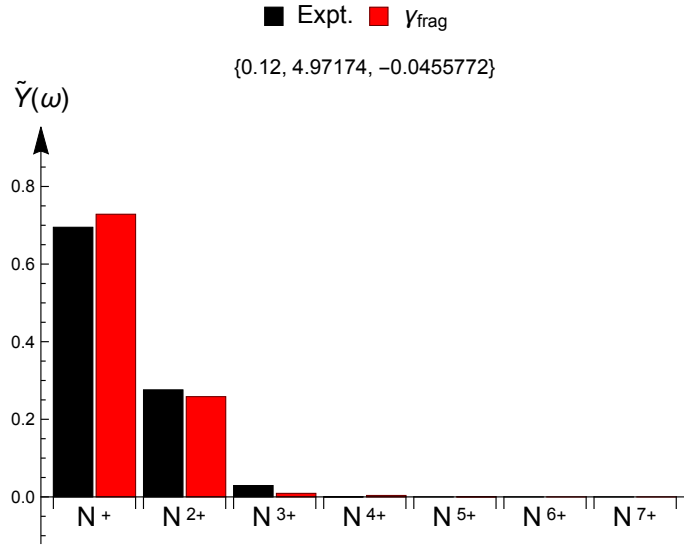

### 0.13

```
damp := 0.13

iy = dsionyieldcrateranalysisparam[damp * 0.26 * MilliJouleToHartree, photonenergy,
  tauX, nintdata, True, True, 1 / 1000, optfNppN, 1 - optfNppN, optGaFra]
iynorm = 1 / Total[iy[[2 ;; 8]]] * iy
Total[iynorm[[2 ;; 8]]]
{0.983387, 0.0119496, 0.00440868, 0.000173712,
  0.0000716462, 8.9174 × 10-6, 1.50054 × 10-7, 5.35619 × 10-10,
  0.981378, 0.000379768, 2.05046 × 10-24, 1.01374 × 10-155}

{59.195, 0.719305, 0.26538, 0.0104566, 0.00431274, 0.000536783, 9.03248 × 10-6,
  3.22416 × 10-8, 59.0741, 0.0228601, 1.23427 × 10-22, 6.10224 × 10-154}

1.

plotiy = Partition[Riffle[normOleg7, iynorm[[2 ;; 8]]], 2]
{{0.694746, 0.719305}, {0.275684, 0.26538},
  {0.0293036, 0.0104566}, {0.000266625, 0.00431274},
  {0., 0.000536783}, {0., 9.03248 × 10-6}, {0., 3.22416 × 10-8}}
```

```

BarChart[plotiy, PlotRange → {-0.1, 0.9},
  ChartLabels → {Placed[{"N +", "N 2+", "N 3+", "N 4+", "N 5+", "N 6+", "N 7+"}, Below],
    Placed[{}, Above]},
  ChartLegends → Placed[{"Expt.", "γfrag"}, Top],
  ChartStyle → {Black, Red}, AxesLabel → {"", "Ỹ(ω)",
  AxesStyle → {{Arrowheads[Automatic], AbsoluteThickness[0.6]},
    {Arrowheads[Automatic], AbsoluteThickness[0.6]}},
  LabelStyle → {FontFamily → "Arial"},
  PlotLabel → {damp, optGaFra / gammaFrag,
    (iynorm[[2 ;; 8]] - normOleg7).Table[i, {i, 1, 7}]]]

```

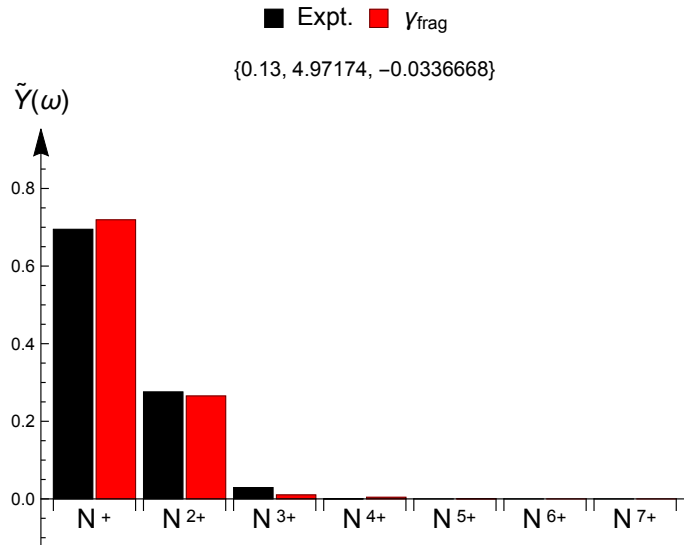

## 0.14

damp := 0.14

```

iy = dsionyieldcrateranalysisparam[damp * 0.26 * MilliJouleToHartree, photonenergy,
  tauX, nintdata, True, True, 1 / 1000, optfNppN, 1 - optfNppN, optGaFra]

```

```

iynorm = 1 / Total[iy[[2 ;; 8]]] * iy

```

```

Total[iynorm[[2 ;; 8]]]

```

```

{0.982303, 0.0125732, 0.00481472, 0.000210101, 0.0000873437, 0.0000116784,
  2.1223 × 10-7, 8.16862 × 10-10, 0.98019, 0.0003988, 2.15484 × 10-24, -8.33734 × 10-151}

```

```

{55.5059, 0.710461, 0.27206, 0.011872, 0.00493544, 0.000659899, 0.0000119923,
  4.61575 × 10-8, 55.3865, 0.0225346, 1.21761 × 10-22, -4.71109 × 10-149}

```

1.

```

plotiy = Partition[Riffle[normOleg7, iynorm[[2 ;; 8]]], 2]

```

```

{{0.694746, 0.710461}, {0.275684, 0.27206},
 {0.0293036, 0.011872}, {0.000266625, 0.00493544},
 {0., 0.000659899}, {0., 0.0000119923}, {0., 4.61575 × 10-8}}

```

```
BarChart[plotiy, PlotRange → {-0.1, 0.9},
  ChartLabels → {Placed[{"N +", "N 2+", "N 3+", "N 4+", "N 5+", "N 6+", "N 7+"}, Below],
    Placed[{}, Above]},
  ChartLegends → Placed[{"Expt.", "γfrag"}, Top],
  ChartStyle → {Black, Red}, AxesLabel → {"", "Ỹ(ω)"},
  AxesStyle → {{Arrowheads[Automatic], AbsoluteThickness[0.6]},
    {Arrowheads[Automatic], AbsoluteThickness[0.6]}},
  LabelStyle → {FontFamily → "Arial"},
  PlotLabel → {damp, optGaFra / gammaFrag,
    (iynorm[[2 ;; 8]] - normOleg7).Table[i, {i, 1, 7}]]]
```

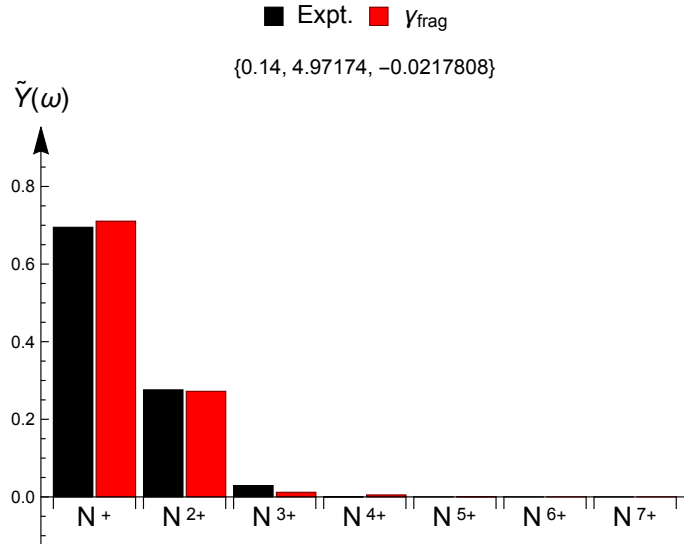

## 0.15

damp := 0.15

```
iy = dsionyieldcrateranalysisparam[damp * 0.26 * MilliJouleToHartree, photonenergy,
  tauX, nintdata, True, True, 1 / 1000, optfNppN, 1 - optfNppN, optGaFra]
```

```
iynorm = 1 / Total[iy[[2 ;; 8]]] * iy
```

```
Total[iynorm[[2 ;; 8]]]
```

```
{0.981242, 0.0131649, 0.00522293, 0.000250332, 0.000104877, 0.0000149887,
  2.92672 × 10-7, 1.20848 × 10-9, 0.979031, 0.000416761, 2.2524 × 10-24, 9.86269 × 10-152}
```

```
{52.3097, 0.701816, 0.278433, 0.0133451, 0.00559097, 0.000799041, 0.0000156022,
  6.44238 × 10-8, 52.1919, 0.0222174, 1.20075 × 10-22, 5.25777 × 10-150}
```

1.

```
plotiy = Partition[Riffle[normOleg7, iynorm[[2 ;; 8]]], 2]
```

```
{{0.694746, 0.701816}, {0.275684, 0.278433},
  {0.0293036, 0.0133451}, {0.000266625, 0.00559097},
  {0., 0.000799041}, {0., 0.0000156022}, {0., 6.44238 × 10-8}}
```

```
BarChart[plotiy, PlotRange → {-0.1, 0.9},
  ChartLabels → {Placed[{"N +", "N 2+", "N 3+", "N 4+", "N 5+", "N 6+", "N 7+"}, Below],
    Placed[{}, Above]},
  ChartLegends → Placed[{"Expt.", "γfrag"}, Top],
  ChartStyle → {Black, Red}, AxesLabel → {"", "Ỹ(ω)",
  AxesStyle → {{Arrowheads[Automatic], AbsoluteThickness[0.6]},
    {Arrowheads[Automatic], AbsoluteThickness[0.6]}},
  LabelStyle → {FontFamily → "Arial"},
  PlotLabel → {damp, optGaFra / gammaFrag,
    (iynorm[[2 ;; 8]] - normOleg7).Table[i, {i, 1, 7}]]]
```

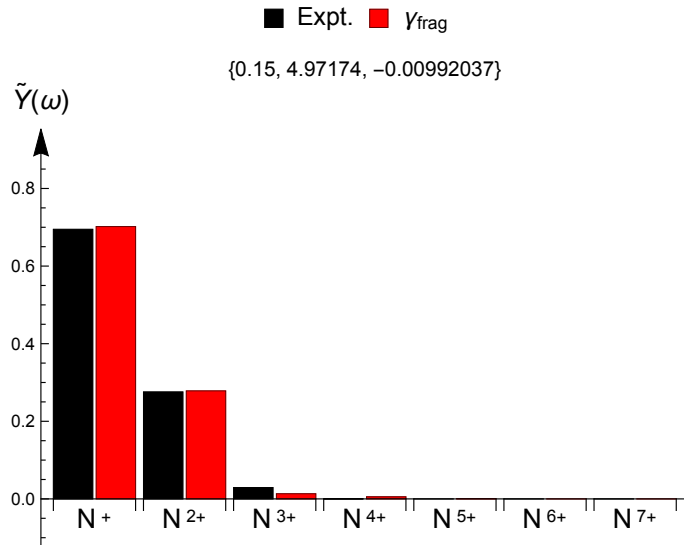

## 0.16

damp := 0.16

```
iy = dsionyieldcrateranalysisparam[damp * 0.26 * MilliJouleToHartree, photonenergy,
  tauX, nintdata, True, True, 1 / 1000, optfNppN, 1 - optfNppN, optGaFra]
```

```
iynorm = 1 / Total[iy[[2 ;; 8]]] * iy
```

```
Total[iynorm[[2 ;; 8]]]
```

```
{0.980203, 0.0137263, 0.00563231, 0.000294394, 0.000124277, 0.000018902,
  3.94806 × 10-7, 1.74114 × 10-9, 0.9779, 0.000433713, 2.34728 × 10-24, -3.80947 × 10-151}
```

```
{49.5137, 0.693367, 0.284509, 0.014871, 0.00627771, 0.000954809, 0.0000199431,
  8.79513 × 10-8, 49.3974, 0.0219085, 1.1857 × 10-22, -1.9243 × 10-149}
```

1.

```
plotiy = Partition[Riffle[normOleg7, iynorm[[2 ;; 8]]], 2]
```

```
{{0.694746, 0.693367}, {0.275684, 0.284509},
  {0.0293036, 0.014871}, {0.000266625, 0.00627771},
  {0., 0.000954809}, {0., 0.0000199431}, {0., 8.79513 × 10-8}}
```

```

BarChart[plotiy, PlotRange → {-0.1, 0.9},
  ChartLabels → {Placed[{"N +", "N 2+", "N 3+", "N 4+", "N 5+", "N 6+", "N 7+"}, Below],
    Placed[{}, Above]},
  ChartLegends → Placed[{"Expt.", "γfrag"}, Top],
  ChartStyle → {Black, Red}, AxesLabel → {"", "Ỹ(ω)"},
  AxesStyle → {{Arrowheads[Automatic], AbsoluteThickness[0.6]},
    {Arrowheads[Automatic], AbsoluteThickness[0.6]}},
  LabelStyle → {FontFamily → "Arial"},
  PlotLabel → {damp, optGaFra / gammaFrag,
    (iynorm[[2 ;; 8]] - normOleg7).Table[i, {i, 1, 7}]]]

```

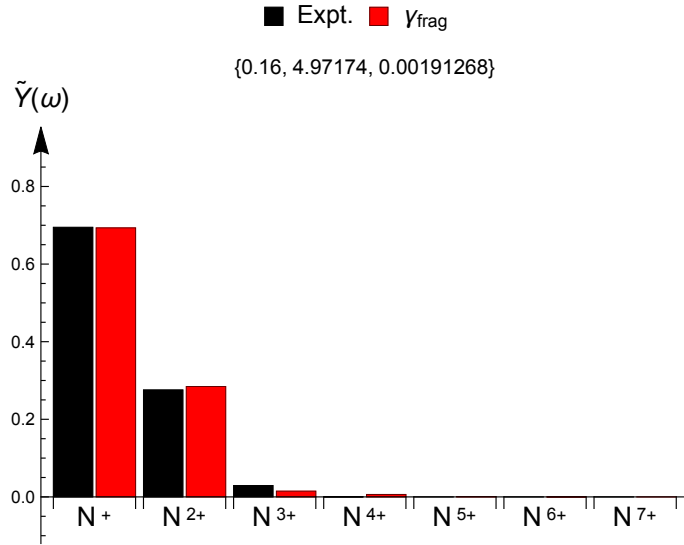

## 0.17

```

damp := 0.17

iy = dsionyieldcrateranalysisparam[damp * 0.26 * MilliJouleToHartree, photonenergy,
  tauX, nintdata, True, True, 1 / 1000, optfNppN, 1 - optfNppN, optGaFra]
iynorm = 1 / Total[iy[[2 ;; 8]]] * iy
Total[iynorm[[2 ;; 8]]]

{0.979187, 0.014259, 0.00604192, 0.000342262,
  0.000145567, 0.0000234716, 5.22367 × 10-7, 2.45086 × 10-9,
  0.976796, 0.000449711, 2.43676 × 10-24, 4.16047 × 10-148}

{47.0475, 0.685109, 0.290299, 0.0164448, 0.00699411, 0.00112775,
  0.0000250984, 1.17757 × 10-7, 46.9326, 0.0216075, 1.1708 × 10-22, 1.999 × 10-146}

1.

plotiy = Partition[Riffle[normOleg7, iynorm[[2 ;; 8]]], 2]

{{0.694746, 0.685109}, {0.275684, 0.290299},
  {0.0293036, 0.0164448}, {0.000266625, 0.00699411},
  {0., 0.00112775}, {0., 0.0000250984}, {0., 1.17757 × 10-7}}

```

```
BarChart[plotiy, PlotRange → {-0.1, 0.9},
  ChartLabels → {Placed[{"N +", "N 2+", "N 3+", "N 4+", "N 5+", "N 6+", "N 7+"}, Below],
    Placed[{}, Above]},
  ChartLegends → Placed[{"Expt.", "γfrag"}, Top],
  ChartStyle → {Black, Red}, AxesLabel → {"", "Ỹ(ω)"},
  AxesStyle → {{Arrowheads[Automatic], AbsoluteThickness[0.6]},
    {Arrowheads[Automatic], AbsoluteThickness[0.6]}},
  LabelStyle → {FontFamily → "Arial"},
  PlotLabel → {damp, optGaFra / gammaFrag,
    (iynorm[[2 ;; 8]] - normOleg7).Table[i, {i, 1, 7}]]]
```

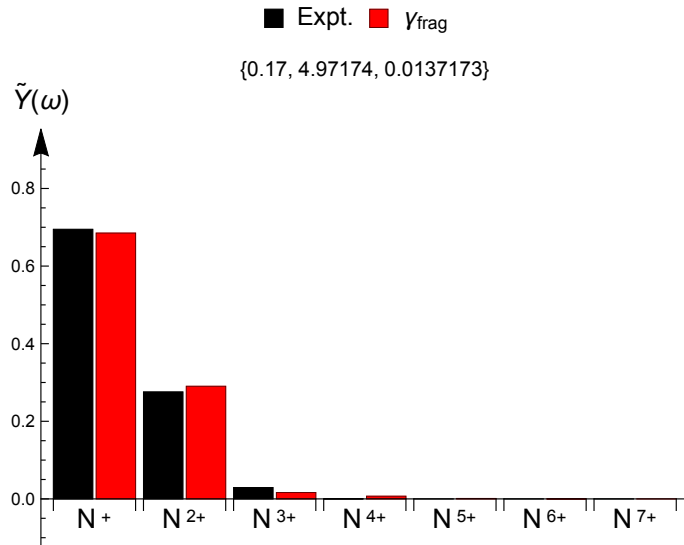

## 0.18

damp := 0.18

```
iy = dsionyieldcrateranalysisparam[damp * 0.26 * MilliJouleToHartree, photonenergy,
  tauX, nintdata, True, True, 1 / 1000, optfNppN, 1 - optfNppN, optGaFra]
```

```
iynorm = 1 / Total[iy[[2 ;; 8]]] * iy
```

```
Total[iynorm[[2 ;; 8]]]
```

```
{0.978193, 0.0147645, 0.00645093, 0.000393891, 0.00016876, 0.0000287499,
  6.79389 × 10-7, 3.37949 × 10-9, 0.975718, 0.00046481, 2.52359 × 10-24, 1.01714 × 10-147}
```

```
{44.8558, 0.677037, 0.295813, 0.0180622, 0.00773863, 0.00131835, 0.000031154,
  1.54969 × 10-7, 44.7424, 0.0213142, 1.15721 × 10-22, 4.66418 × 10-146}
```

1.

```
plotiy = Partition[Riffle[normOleg7, iynorm[[2 ;; 8]]], 2]
```

```
{{0.694746, 0.677037}, {0.275684, 0.295813},
  {0.0293036, 0.0180622}, {0.000266625, 0.00773863},
  {0., 0.00131835}, {0., 0.000031154}, {0., 1.54969 × 10-7}}
```

```
BarChart[plotiy, PlotRange → {-0.1, 0.9},
  ChartLabels → {Placed[{"N +", "N 2+", "N 3+", "N 4+", "N 5+", "N 6+", "N 7+"}, Below],
    Placed[{}, Above]},
  ChartLegends → Placed[{"Expt.", "γfrag"}, Top],
  ChartStyle → {Black, Red}, AxesLabel → {"", "Ỹ(ω)"},
  AxesStyle → {{Arrowheads[Automatic], AbsoluteThickness[0.6]},
    {Arrowheads[Automatic], AbsoluteThickness[0.6]}},
  LabelStyle → {FontFamily → "Arial"},
  PlotLabel → {damp, optGaFra / gammaFrag,
    (iynorm[[2 ;; 8]] - normOleg7).Table[i, {i, 1, 7}]]]
```

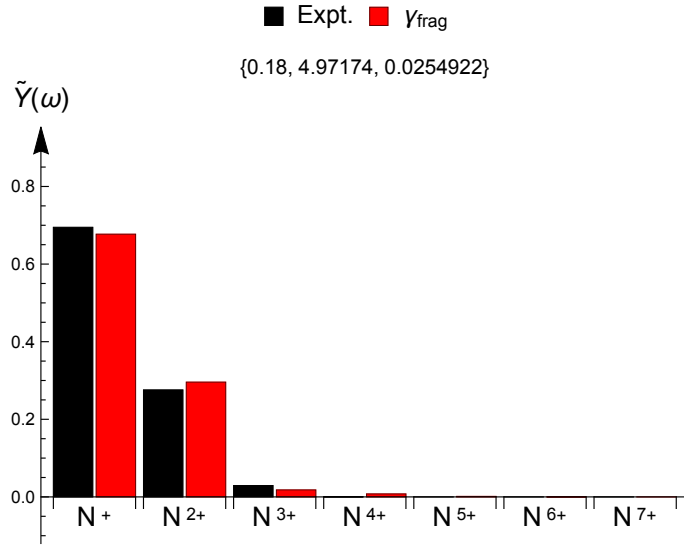

## Pulse energy for a 7 fs pulse with 80 fs fragmentation rate

```
tauX := 7 / t0ToFemtoSecond
optent := 16.800000
optGaFra := optent * gammaFrag
```

### 0.12

```
damp := 0.12

iy = dsionyieldcrateranalysisparam[damp * 0.26 * MilliJouleToHartree, photonenergy,
  tauX, nintdata, True, True, 1 / 1000, optfNppN, 1 - optfNppN, optGaFra]
iynorm = 1 / Total[iy[[2 ;; 8]]] * iy
Total[iynorm[[2 ;; 8]]]

{0.984498, 0.0113013, 0.00398498, 0.00014988, 0.0000589879, 6.97345 × 10-6,
  1.08479 × 10-7, 3.5989 × 10-10, 0.982596, 0.000359602, 2.934 × 10-76, -7.15392 × 10-170}

{63.5068, 0.729011, 0.257059, 0.00966828, 0.00380512, 0.000449835, 6.99764 × 10-6,
  2.32153 × 10-8, 63.3842, 0.0231968, 1.89263 × 10-74, -4.61477 × 10-168}

1.
```

```

plotiy = Partition[Riffle[normOleg7, iynorm[[2 ;; 8]]], 2]
{
  {0.694746, 0.729011}, {0.275684, 0.257059},
  {0.0293036, 0.00966828}, {0.000266625, 0.00380512},
  {0., 0.000449835}, {0.,  $6.99764 \times 10^{-6}$ }, {0.,  $2.32153 \times 10^{-8}$ }
}

BarChart[plotiy, PlotRange → {-0.1, 0.9},
  ChartLabels → {Placed[{"N +", "N 2+", "N 3+", "N 4+", "N 5+", "N 6+", "N 7+"}, Below],
    Placed[{}, Above]},
  ChartLegends → Placed[{"Expt.", " $\gamma_{\text{frag}}$ "}, Top],
  ChartStyle → {Black, Red}, AxesLabel → {"", " $\tilde{Y}(\omega)$ "},
  AxesStyle → {{Arrowheads[Automatic], AbsoluteThickness[0.6]},
    {Arrowheads[Automatic], AbsoluteThickness[0.6]}},
  LabelStyle → {FontFamily → "Arial"},
  PlotLabel → {damp, optGaFra / gammaFrag,
    (iynorm[[2 ;; 8]] - normOleg7).Table[i, {i, 1, 7}]}]

```

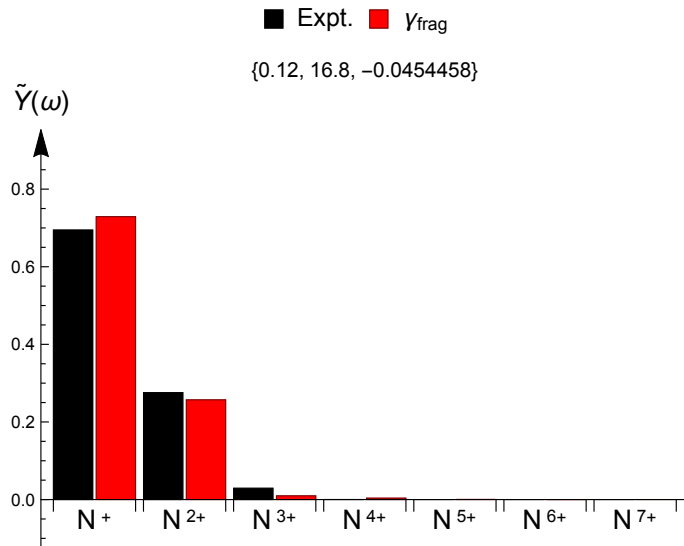

## 0.13

```

damp := 0.13

iy = dsionyieldcrateranalysisparam[damp * 0.26 * MilliJouleToHartree, photonenergy,
  tauX, nintdata, True, True, 1 / 1000, optfNppN, 1 - optfNppN, optGaFra]
iynorm = 1 / Total[iy[[2 ;; 8]]] * iy
Total[iynorm[[2 ;; 8]]]
{
  0.983389, 0.0119598, 0.00438489, 0.000183611,
  0.0000730289,  $9.31256 \times 10^{-6}$ ,  $1.57341 \times 10^{-7}$ ,  $5.65907 \times 10^{-10}$ ,
  0.981378, 0.000379768,  $3.61109 \times 10^{-76}$ ,  $6.86676 \times 10^{-164}$ 
}

{
  59.2017, 0.720002, 0.263978, 0.0110537, 0.00439646, 0.000560632,  $9.4722 \times 10^{-6}$ ,
   $3.40686 \times 10^{-8}$ , 59.0807, 0.0228627,  $2.17394 \times 10^{-74}$ ,  $4.13391 \times 10^{-162}$ 
}

```

1.

```
plotiy = Partition[Riffle[normOleg7, iynorm[[2 ;; 8]]], 2]
```

```
{ {0.694746, 0.720002}, {0.275684, 0.263978},  
  {0.0293036, 0.0110537}, {0.000266625, 0.00439646},  
  {0., 0.000560632}, {0.,  $9.4722 \times 10^{-6}$ }, {0.,  $3.40686 \times 10^{-8}$ }}
```

```
BarChart[plotiy, PlotRange → {-0.1, 0.9},  
  ChartLabels → {Placed[{"N +", "N 2+", "N 3+", "N 4+", "N 5+", "N 6+", "N 7+"}, Below],  
    Placed[{}, Above]},  
  ChartLegends → Placed[{"Expt.", " $\gamma_{\text{frag}}$ "}, Top],  
  ChartStyle → {Black, Red}, AxesLabel → {"", " $\tilde{Y}(\omega)$ "},  
  AxesStyle → {{Arrowheads[Automatic], AbsoluteThickness[0.6]},  
    {Arrowheads[Automatic], AbsoluteThickness[0.6]}},  
  LabelStyle → {FontFamily → "Arial"},  
  PlotLabel → {damp, optGaFra / gammaFrag,  
    (iynorm[[2 ;; 8]] - normOleg7).Table[i, {i, 1, 7}]}]
```

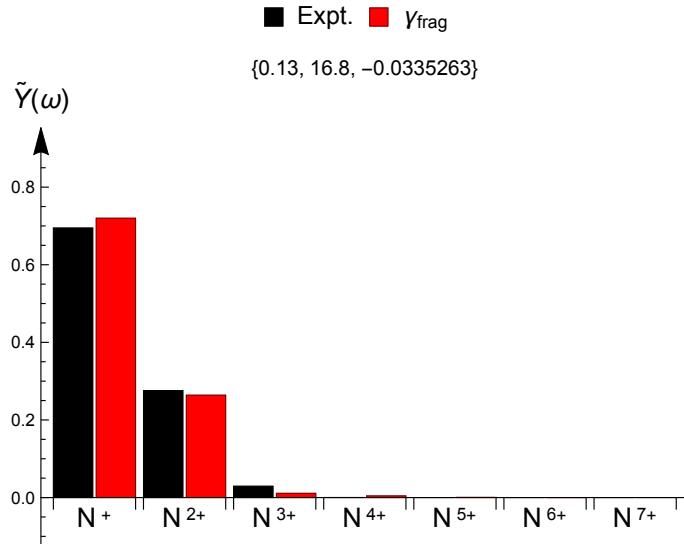

## 0.14

```
damp := 0.14
```

```
iy = dsionyieldcrateranalysisparam[damp * 0.26 * MilliJouleToHartree, photonenergy,  
  tauX, nintdata, True, True, 1 / 1000, optfNppN, 1 - optfNppN, optGaFra]
```

```
iynorm = 1 / Total[iy[[2 ;; 8]]] * iy
```

```
Total[iynorm[[2 ;; 8]]]
```

```
{0.982305, 0.0125847, 0.00478801, 0.000221193, 0.0000888623, 0.000012155,  
   $2.21739 \times 10^{-7}$ ,  $8.5958 \times 10^{-10}$ , 0.98019, 0.0003988,  $4.7709 \times 10^{-76}$ ,  $1.30609 \times 10^{-161}$ }
```

```
{55.5126, 0.711195, 0.270583, 0.0125002, 0.00502183, 0.000686911, 0.000012531,  
   $4.85771 \times 10^{-8}$ , 55.3931, 0.0225372,  $2.69616 \times 10^{-74}$ ,  $7.38105 \times 10^{-160}$ }
```

1.

```
plotiy = Partition[Riffle[normOleg7, iynorm[[2 ;; 8]]], 2]
```

```
{ {0.694746, 0.711195}, {0.275684, 0.270583},  
  {0.0293036, 0.0125002}, {0.000266625, 0.00502183},  
  {0., 0.000686911}, {0., 0.000012531}, {0.,  $4.85771 \times 10^{-8}$ }}
```

```
BarChart[plotiy, PlotRange → {-0.1, 0.9},
  ChartLabels → {Placed[{"N +", "N 2+", "N 3+", "N 4+", "N 5+", "N 6+", "N 7+"}, Below],
    Placed[{}, Above]},
  ChartLegends → Placed[{"Expt.", "γfrag"}, Top],
  ChartStyle → {Black, Red}, AxesLabel → {"", "Ỹ(ω)",
  AxesStyle → {{Arrowheads[Automatic], AbsoluteThickness[0.6]},
    {Arrowheads[Automatic], AbsoluteThickness[0.6]}},
  LabelStyle → {FontFamily → "Arial"},
  PlotLabel → {damp, optGaFra / gammaFrag,
    (iynorm[[2 ;; 8]] - normOleg7).Table[i, {i, 1, 7}]]]
```

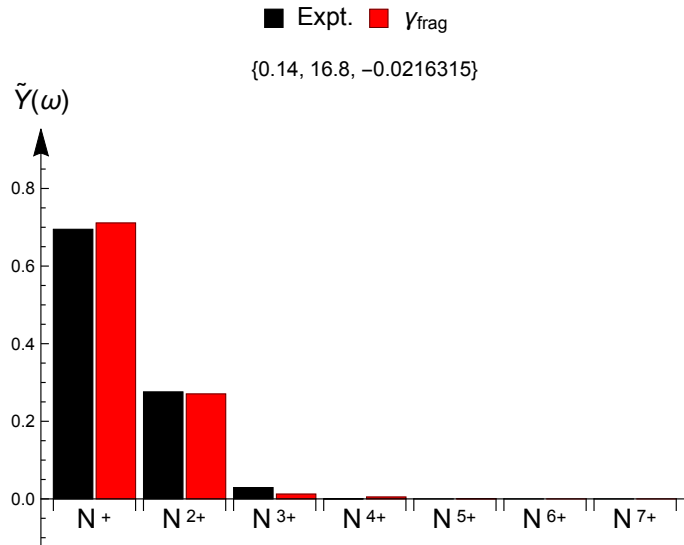

## 0.15

damp := 0.15

```
iy = dsionyieldcrateranalysisparam[damp * 0.26 * MilliJouleToHartree, photonenergy,
  tauX, nintdata, True, True, 1 / 1000, optfNppN, 1 - optfNppN, optGaFra]
```

```
iynorm = 1 / Total[iy[[2 ;; 8]]] * iy
```

```
Total[iynorm[[2 ;; 8]]]
```

```
{0.981244, 0.0131777, 0.00519326, 0.000262635,
  0.000106527, 0.0000155548, 3.04829 × 10-7, 1.26721 × 10-9,
  0.979031, 0.000416761, 2.64131 × 10-76, -9.47555 × 10-166}
```

```
{52.3163, 0.702587, 0.276885, 0.0140027, 0.00567964, 0.000829326, 0.0000162523,
  6.75631 × 10-8, 52.1983, 0.0222202, 1.40825 × 10-74, -5.05201 × 10-164}
```

1.

```
plotiy = Partition[Riffle[normOleg7, iynorm[[2 ;; 8]]], 2]
```

```
{{0.694746, 0.702587}, {0.275684, 0.276885},
  {0.0293036, 0.0140027}, {0.000266625, 0.00567964},
  {0., 0.000829326}, {0., 0.0000162523}, {0., 6.75631 × 10-8}}
```

```
BarChart[plotiy, PlotRange → {-0.1, 0.9},
  ChartLabels → {Placed[{"N +", "N 2+", "N 3+", "N 4+", "N 5+", "N 6+", "N 7+"}, Below],
    Placed[{}, Above]},
  ChartLegends → Placed[{"Expt.", "γfrag"}, Top],
  ChartStyle → {Black, Red}, AxesLabel → {"", "Ỹ(ω)",
  AxesStyle → {{Arrowheads[Automatic], AbsoluteThickness[0.6]},
    {Arrowheads[Automatic], AbsoluteThickness[0.6]}},
  LabelStyle → {FontFamily → "Arial"},
  PlotLabel → {damp, optGaFra / gammaFrag,
    (iynorm[[2 ;; 8]] - normOleg7).Table[i, {i, 1, 7}]]]
```

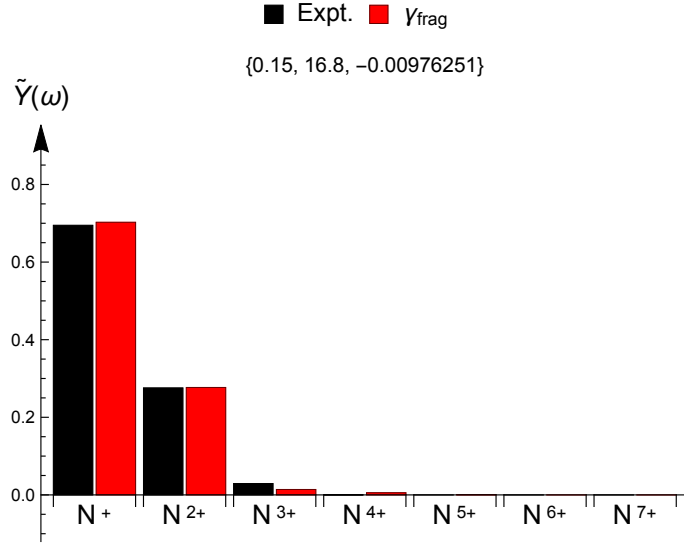

## 0.16

```
damp := 0.16

iy = dsionyieldcrateranalysisparam[damp * 0.26 * MilliJouleToHartree, photonenergy,
  tauX, nintdata, True, True, 1 / 1000, optfNppN, 1 - optfNppN, optGaFra]
iynorm = 1 / Total[iy[[2 ;; 8]]] * iy
Total[iynorm[[2 ;; 8]]]

{0.980206, 0.0137405, 0.00559962, 0.000307924, 0.000126054, 0.0000195656,
  4.10076 × 10-7, 1.82011 × 10-9, 0.9779, 0.000433713, 6.53778 × 10-76, 1.11397 × 10-159}

{49.5203, 0.694172, 0.282894, 0.0155564, 0.00636826, 0.000988462, 0.0000207171,
  9.19525 × 10-8, 49.4038, 0.0219113, 3.3029 × 10-74, 5.62779 × 10-158}

1.

plotiy = Partition[Riffle[normOleg7, iynorm[[2 ;; 8]]], 2]

{{0.694746, 0.694172}, {0.275684, 0.282894},
  {0.0293036, 0.0155564}, {0.000266625, 0.00636826},
  {0., 0.000988462}, {0., 0.0000207171}, {0., 9.19525 × 10-8}}
```

```
BarChart[plotiy, PlotRange → {-0.1, 0.9},
  ChartLabels → {Placed[{"N +", "N 2+", "N 3+", "N 4+", "N 5+", "N 6+", "N 7+"}, Below],
    Placed[{}, Above]},
  ChartLegends → Placed[{"Expt.", "γfrag"}, Top],
  ChartStyle → {Black, Red}, AxesLabel → {"", "Ỹ(ω)",
  AxesStyle → {{Arrowheads[Automatic], AbsoluteThickness[0.6]},
    {Arrowheads[Automatic], AbsoluteThickness[0.6]}},
  LabelStyle → {FontFamily → "Arial"},
  PlotLabel → {damp, optGaFra / gammaFrag,
    (iynorm[[2 ;; 8]] - normOleg7).Table[i, {i, 1, 7}]]]
```

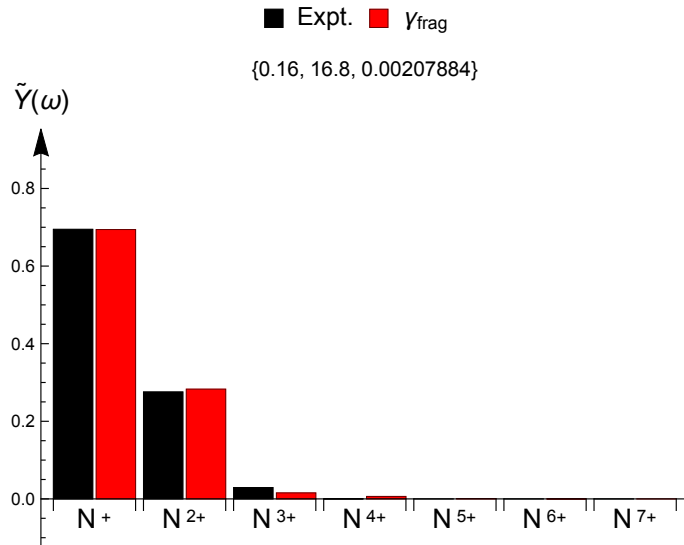

## 0.17

damp := 0.17

```
iy = dsionyieldcrateranalysisparam[damp * 0.26 * MilliJouleToHartree, photonenergy,
  tauX, nintdata, True, True, 1 / 1000, optfNppN, 1 - optfNppN, optGaFra]
```

```
iynorm = 1 / Total[iy[[2 ;; 8]]] * iy
```

```
Total[iynorm[[2 ;; 8]]]
```

```
{0.97919, 0.0142745, 0.00600618, 0.000357027, 0.000147463, 0.0000242406,
  5.41249 × 10-7, 2.555 × 10-9, 0.976796, 0.000449711, 7.46714 × 10-76, -4.92216 × 10-158}
```

```
{47.0539, 0.685946, 0.288621, 0.0171565, 0.00708618, 0.00116485, 0.0000260092,
  1.22778 × 10-7, 46.9389, 0.0216104, 3.58826 × 10-74, -2.36529 × 10-156}
```

1.

```
plotiy = Partition[Riffle[normOleg7, iynorm[[2 ;; 8]]], 2]
```

```
{{0.694746, 0.685946}, {0.275684, 0.288621},
  {0.0293036, 0.0171565}, {0.000266625, 0.00708618},
  {0., 0.00116485}, {0., 0.0000260092}, {0., 1.22778 × 10-7}}
```

```
BarChart[plotiy, PlotRange → {-0.1, 0.9},
  ChartLabels → {Placed[{"N +", "N 2+", "N 3+", "N 4+", "N 5+", "N 6+", "N 7+"}, Below],
    Placed[{}, Above]},
  ChartLegends → Placed[{"Expt.", "γfrag"}, Top],
  ChartStyle → {Black, Red}, AxesLabel → {"", "Ỹ(ω)"},
  AxesStyle → {{Arrowheads[Automatic], AbsoluteThickness[0.6]},
    {Arrowheads[Automatic], AbsoluteThickness[0.6]}},
  LabelStyle → {FontFamily → "Arial"},
  PlotLabel → {damp, optGaFra / gammaFrag,
    (iynorm[[2 ;; 8]] - normOleg7).Table[i, {i, 1, 7}]]]
```

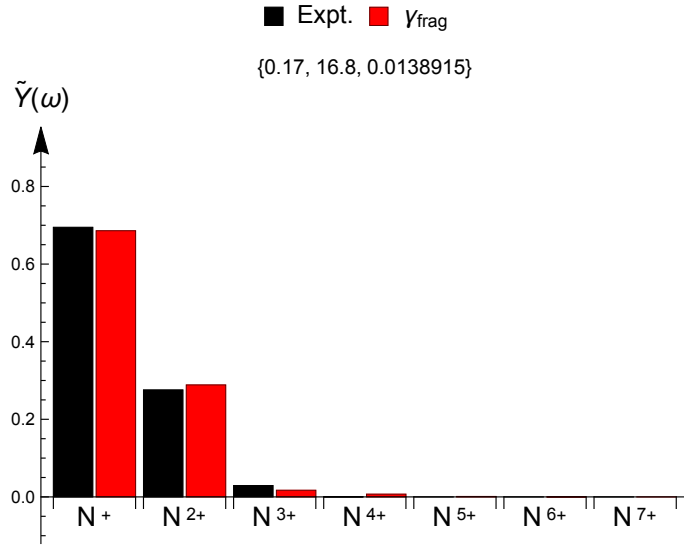

## 0.18

damp := 0.18

```
iy = dsionyieldcrateranalysisparam[damp * 0.26 * MilliJouleToHartree, photonenergy,
  tauX, nintdata, True, True, 1 / 1000, optfNppN, 1 - optfNppN, optGaFra]
```

```
iynorm = 1 / Total[iy[[2 ;; 8]]] * iy
```

```
Total[iynorm[[2 ;; 8]]]
```

```
{0.978196, 0.0147813, 0.00641212, 0.000409895,
  0.000170769, 0.0000296318, 7.02419 × 10-7, 3.51447 × 10-9,
  0.975718, 0.00046481, 6.26715 × 10-76, -4.41158 × 10-159}
```

```
{44.8622, 0.677904, 0.294074, 0.0187987, 0.00783187, 0.00135898, 0.0000322145,
  1.61182 × 10-7, 44.7486, 0.0213172, 2.87426 × 10-74, -2.02325 × 10-157}
```

1.

```
plotiy = Partition[Riffle[normOleg7, iynorm[[2 ;; 8]]], 2]
```

```
{{0.694746, 0.677904}, {0.275684, 0.294074},
  {0.0293036, 0.0187987}, {0.000266625, 0.00783187},
  {0., 0.00135898}, {0., 0.0000322145}, {0., 1.61182 × 10-7}}
```

```

BarChart[plotiy, PlotRange → {-0.1, 0.9},
  ChartLabels → {Placed[{"N +", "N 2+", "N 3+", "N 4+", "N 5+", "N 6+", "N 7+"}, Below],
    Placed[{}, Above]},
  ChartLegends → Placed[{"Expt.", "γfrag"}, Top],
  ChartStyle → {Black, Red}, AxesLabel → {"", "Ỹ(ω)"},
  AxesStyle → {{Arrowheads[Automatic], AbsoluteThickness[0.6]},
    {Arrowheads[Automatic], AbsoluteThickness[0.6]}},
  LabelStyle → {FontFamily → "Arial"},
  PlotLabel → {damp, optGaFra / gammaFrag,
    (iynorm[[2 ;; 8]] - normOleg7).Table[i, {i, 1, 7}]]]

```

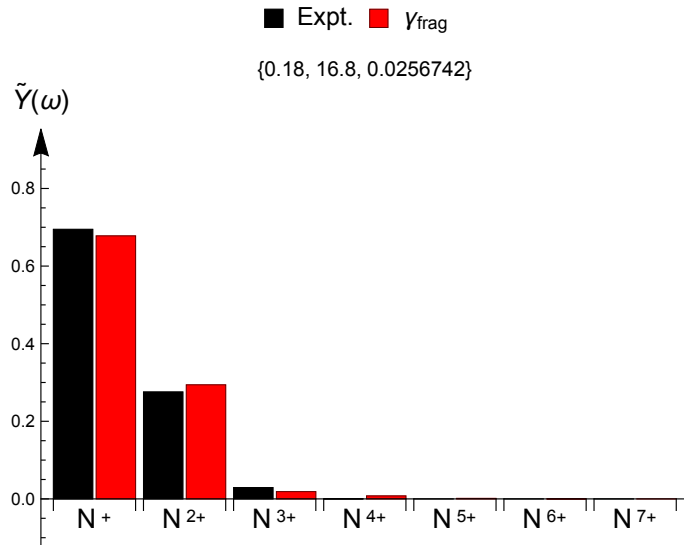

## Pulse energy for a 4 fs pulse with 280 fs fragmentation rate

```

tauX := 4 / t0ToFemtoSecond
optent := 4.971737
optGaFra := optent * gammaFrag

```

### 0.21

```

damp := 0.21

iy = dsionyieldcrateranalysisparam[damp * 0.15 * MilliJouleToHartree, photonenergy,
  tauX, nintdata, True, True, 1 / 1000, optfNppN, 1 - optfNppN, optGaFra]
iynorm = 1 / Total[iy[[2 ;; 8]]] * iy
Total[iynorm[[2 ;; 8]]]

```

{0.984372, 0.0114032, 0.00402325, 0.000149786,  
 0.0000461664, 5.09502 × 10<sup>-6</sup>, 5.34281 × 10<sup>-8</sup>, 1.05179 × 10<sup>-10</sup>,  
 0.982454, 0.000361989, 1.95157 × 10<sup>-24</sup>, -7.83825 × 10<sup>-176}}</sup>

{62.9895, 0.729686, 0.257446, 0.00958472, 0.00295417, 0.000326028, 3.41884 × 10<sup>-6</sup>,  
 6.73035 × 10<sup>-9</sup>, 62.8668, 0.0231635, 1.2488 × 10<sup>-22</sup>, -5.01566 × 10<sup>-174}}</sup>

1.

```

plotiy = Partition[Riffle[normOleg4, iynorm[[2 ;; 8]]], 2]
{{0.711226, 0.729686}, {0.277966, 0.257446}, {0.0108078, 0.00958472},
 {0., 0.00295417}, {0., 0.000326028}, {0.,  $3.41884 \times 10^{-6}$ }, {0.,  $6.73035 \times 10^{-9}$ }}

```

```

BarChart[plotiy, PlotRange → {-0.1, 0.9},
  ChartLabels → {Placed[{"N +", "N 2+", "N 3+", "N 4+", "N 5+", "N 6+", "N 7+"}, Below],
    Placed[{}, Above]},
  ChartLegends → Placed[{"Expt.", " $\gamma_{\text{frag}}$ "}, Top],
  ChartStyle → {Black, Red}, AxesLabel → {"", " $\tilde{Y}(\omega)$ "},
  AxesStyle → {{Arrowheads[Automatic], AbsoluteThickness[0.6]},
    {Arrowheads[Automatic], AbsoluteThickness[0.6]}},
  LabelStyle → {FontFamily → "Arial"},
  PlotLabel → {damp, optGaFra / gammaFrag,
    (iynorm[[2 ;; 8]] - normOleg4).Table[i, {i, 1, 7}]}]

```

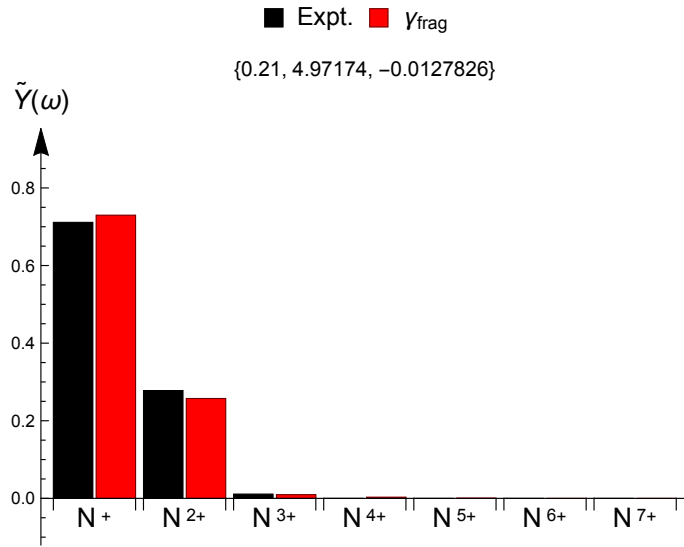

## 0.22

```
damp := 0.22
```

```

iy = dsionyieldcrateranalysisparam[damp * 0.15 * MilliJouleToHartree, photonenergy,
  tauX, nintdata, True, True, 1 / 1000, optfNppN, 1 - optfNppN, optGaFra]

```

```
iynorm = 1 / Total[iy[[2 ;; 8]]] * iy
```

```
Total[iynorm[[2 ;; 8]]]
```

```

{0.983732, 0.0117868, 0.00425357, 0.000169204,
 0.0000524759,  $6.05058 \times 10^{-6}$ ,  $6.65799 \times 10^{-8}$ ,  $1.37424 \times 10^{-10}$ ,
 0.98175, 0.000373687,  $2.01662 \times 10^{-24}$ ,  $-7.67299 \times 10^{-176}$ }

```

```

{60.4696, 0.724532, 0.261466, 0.0104009, 0.00322567, 0.000371927,  $4.09264 \times 10^{-6}$ ,
  $8.44738 \times 10^{-9}$ , 60.3478, 0.0229704,  $1.23961 \times 10^{-22}$ ,  $-4.71656 \times 10^{-174}$ }

```

1.

```
plotiy = Partition[Riffle[normOleg4, iynorm[[2 ;; 8]]], 2]
```

```

{{0.711226, 0.724532}, {0.277966, 0.261466}, {0.0108078, 0.0104009},
 {0., 0.00322567}, {0., 0.000371927}, {0.,  $4.09264 \times 10^{-6}$ }, {0.,  $8.44738 \times 10^{-9}$ }}

```

```
BarChart[plotiy, PlotRange → {-0.1, 0.9},
  ChartLabels → {Placed[{"N +", "N 2+", "N 3+", "N 4+", "N 5+", "N 6+", "N 7+"}, Below],
    Placed[{}, Above]},
  ChartLegends → Placed[{"Expt.", "γfrag"}, Top],
  ChartStyle → {Black, Red}, AxesLabel → {"", "Ỹ(ω)",
  AxesStyle → {{Arrowheads[Automatic], AbsoluteThickness[0.6]},
    {Arrowheads[Automatic], AbsoluteThickness[0.6]}},
  LabelStyle → {FontFamily → "Arial"},
  PlotLabel → {damp, optGaFra / gammaFrag,
    (iynorm[[2 ;; 8]] - normOleg4).Table[i, {i, 1, 7}]]]
```

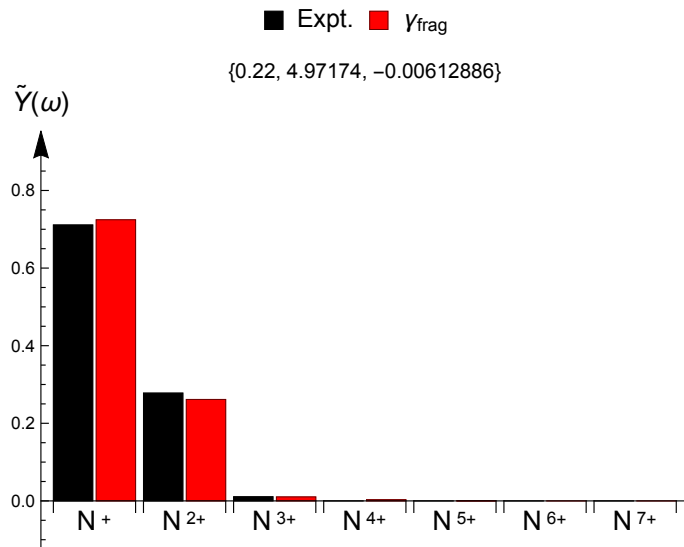

## 0.23

damp := 0.23

```
iy = dsionyieldcrateranalysisparam[damp * 0.15 * MilliJouleToHartree, photonenergy,
  tauX, nintdata, True, True, 1 / 1000, optfNppN, 1 - optfNppN, optGaFra]
```

```
iynorm = 1 / Total[iy[[2 ;; 8]]] * iy
```

```
Total[iynorm[[2 ;; 8]]]
```

```
{0.983099, 0.0121591, 0.00448514, 0.00018997,
  0.0000592803, 7.12662 × 10-6, 8.21211 × 10-8, 1.77352 × 10-10,
  0.981055, 0.000385001, 2.07941 × 10-24, 1.31534 × 10-174}
```

```
{58.1692, 0.719444, 0.265382, 0.0112404, 0.00350757, 0.000421677, 4.85904 × 10-6,
  1.04938 × 10-8, 58.0482, 0.0227802, 1.23037 × 10-22, 7.78277 × 10-173}
```

1.

```
plotiy = Partition[Riffle[normOleg4, iynorm[[2 ;; 8]]], 2]
```

```
{{0.711226, 0.719444}, {0.277966, 0.265382}, {0.0108078, 0.0112404},
  {0., 0.00350757}, {0., 0.000421677}, {0., 4.85904 × 10-6}, {0., 1.04938 × 10-8}}
```

```
BarChart[plotiy, PlotRange → {-0.1, 0.9},
  ChartLabels → {Placed[{"N +", "N 2+", "N 3+", "N 4+", "N 5+", "N 6+", "N 7+"}, Below],
    Placed[{}, Above]},
  ChartLegends → Placed[{"Expt.", "γfrag"}, Top],
  ChartStyle → {Black, Red}, AxesLabel → {"", "Ỹ(ω)"},
  AxesStyle → {{Arrowheads[Automatic], AbsoluteThickness[0.6]},
    {Arrowheads[Automatic], AbsoluteThickness[0.6]}},
  LabelStyle → {FontFamily → "Arial"},
  PlotLabel → {damp, optGaFra / gammaFrag,
    (iynorm[[2 ;; 8]] - normOleg4).Table[i, {i, 1, 7}]]]
```

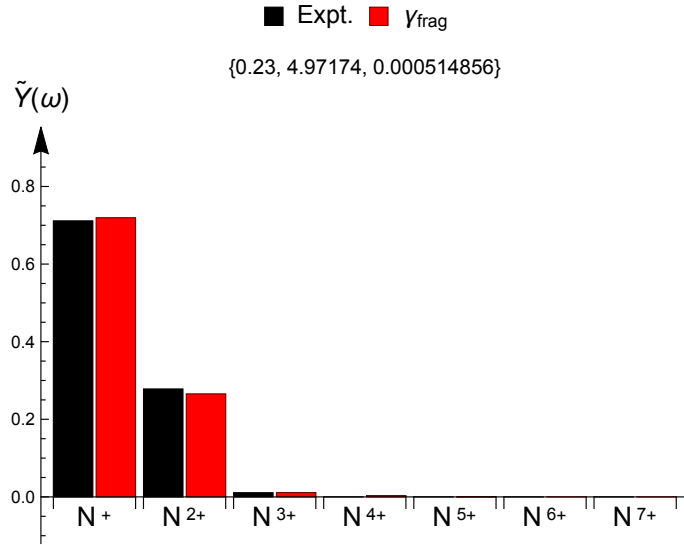

## 0.24

```
damp := 0.24

iy = dsionyieldcrateranalysisparam[damp * 0.15 * MilliJouleToHartree, photonenergy,
  tauX, nintdata, True, True, 1 / 1000, optfNppN, 1 - optfNppN, optGaFra]
iynorm = 1 / Total[iy[[2 ;; 8]]] * iy
Total[iynorm[[2 ;; 8]]]
{0.982475, 0.0125203, 0.00471772, 0.000212093,
  0.0000665897, 8.33125 × 10-6, 1.00342 × 10-7, 2.26311 × 10-10,
  0.980371, 0.000395943, 2.14011 × 10-24, -8.91075 × 10-173}

{56.0608, 0.714421, 0.269196, 0.0121022, 0.00379966, 0.000475388, 5.7256 × 10-6,
  1.29135 × 10-8, 55.9407, 0.0225928, 1.22117 × 10-22, -5.08454 × 10-171}

1.

plotiy = Partition[Riffle[normOleg4, iynorm[[2 ;; 8]]], 2]
{{0.711226, 0.714421}, {0.277966, 0.269196}, {0.0108078, 0.0121022},
  {0., 0.00379966}, {0., 0.000475388}, {0., 5.7256 × 10-6}, {0., 1.29135 × 10-8}}
```

```
BarChart[plotiy, PlotRange → {-0.1, 0.9},
  ChartLabels → {Placed[{"N +", "N 2+", "N 3+", "N 4+", "N 5+", "N 6+", "N 7+"}, Below],
    Placed[{}, Above]},
  ChartLegends → Placed[{"Expt.", "γfrag"}, Top],
  ChartStyle → {Black, Red}, AxesLabel → {"", "Ỹ(ω)"},
  AxesStyle → {{Arrowheads[Automatic], AbsoluteThickness[0.6]},
    {Arrowheads[Automatic], AbsoluteThickness[0.6]}},
  LabelStyle → {FontFamily → "Arial"},
  PlotLabel → {damp, optGaFra / gammaFrag,
    (iynorm[[2 ;; 8]] - normOleg4).Table[i, {i, 1, 7}]]]
```

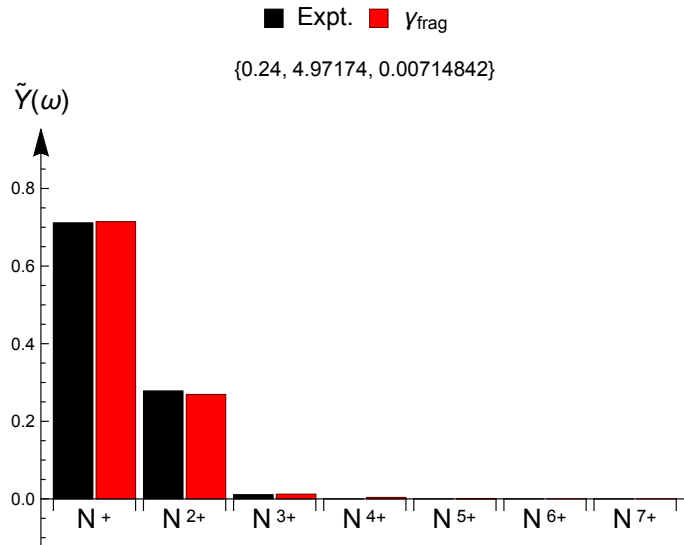

## 0.25

damp := 0.25

```
iy = dsionyieldcrateranalysisparam[damp * 0.15 * MilliJouleToHartree, photonenergy,
  tauX, nintdata, True, True, 1 / 1000, optfNppN, 1 - optfNppN, optGaFra]
```

```
iynorm = 1 / Total[iy[[2 ;; 8]]] * iy
```

```
Total[iynorm[[2 ;; 8]]]
```

```
{0.981858, 0.0128709, 0.0049511, 0.000235575,
  0.0000744133, 9.67259 × 10-6, 1.21552 × 10-7, 2.85808 × 10-10,
  0.979696, 0.000406527, 2.19904 × 10-24, 1.1715 × 10-173}
```

```
{54.1213, 0.709462, 0.272911, 0.0129852, 0.00410176, 0.000533166, 6.70012 × 10-6,
  1.57541 × 10-8, 54.0021, 0.0224083, 1.21214 × 10-22, 6.45746 × 10-172}
```

1.

```
plotiy = Partition[Riffle[normOleg4, iynorm[[2 ;; 8]]], 2]
```

```
{{0.711226, 0.709462}, {0.277966, 0.272911}, {0.0108078, 0.0129852},
  {0., 0.00410176}, {0., 0.000533166}, {0., 6.70012 × 10-6}, {0., 1.57541 × 10-8}}
```

```
BarChart[plotiy, PlotRange → {-0.1, 0.9},
  ChartLabels → {Placed[{"N +", "N 2+", "N 3+", "N 4+", "N 5+", "N 6+", "N 7+"}, Below],
    Placed[{}, Above]},
  ChartLegends → Placed[{"Expt.", "γfrag"}, Top],
  ChartStyle → {Black, Red}, AxesLabel → {"", "Ỹ(ω)"},
  AxesStyle → {{Arrowheads[Automatic], AbsoluteThickness[0.6]},
    {Arrowheads[Automatic], AbsoluteThickness[0.6]}},
  LabelStyle → {FontFamily → "Arial"},
  PlotLabel → {damp, optGaFra / gammaFrag,
    (iynorm[[2 ;; 8]] - normOleg4).Table[i, {i, 1, 7}]]]
```

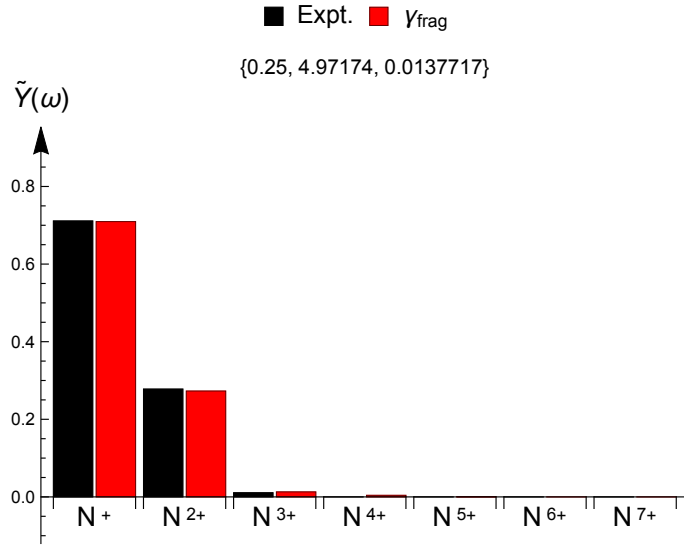

## Pulse energy for a 4 fs pulse with 80 fs fragmentation rate

```
tauX := 4 / t0ToFemtoSecond
optent := 16.800000
optGaFra := optent * gammaFrag
```

### 0.21

```
damp := 0.21

iy = dsionyieldcrateranalysisparam[damp * 0.15 * MilliJouleToHartree, photonenergy,
  tauX, nintdata, True, True, 1 / 1000, optfNppN, 1 - optfNppN, optGaFra]
iynorm = 1 / Total[iy[[2 ;; 8]]] * iy
Total[iynorm[[2 ;; 8]]]

{0.984373, 0.0114066, 0.00401527, 0.000153091,
  0.0000466639, 5.21187 × 10-6, 5.48442 × 10-8, 1.08472 × 10-10,
  0.982454, 0.000361989, 2.4308 × 10-76, 7.92573 × 10-218}

{62.9921, 0.729935, 0.256945, 0.00979664, 0.00298612, 0.000333518, 3.5096 × 10-6,
  6.94137 × 10-9, 62.8693, 0.0231644, 1.55552 × 10-74, 5.07184 × 10-216}
```

1.

```

plotiy = Partition[Riffle[normOleg4, iynorm[[2 ;; 8]]], 2]
{{0.711226, 0.729935}, {0.277966, 0.256945}, {0.0108078, 0.00979664},
 {0., 0.00298612}, {0., 0.000333518}, {0.,  $3.5096 \times 10^{-6}$ }, {0.,  $6.94137 \times 10^{-9}$ }}

BarChart[plotiy, PlotRange → {-0.1, 0.9},
  ChartLabels → {Placed[{"N +", "N 2+", "N 3+", "N 4+", "N 5+", "N 6+", "N 7+"}, Below],
    Placed[{}, Above]},
  ChartLegends → Placed[{"Expt.", " $\gamma_{\text{frag}}$ "}, Top],
  ChartStyle → {Black, Red}, AxesLabel → {"", " $\tilde{Y}(\omega)$ "},
  AxesStyle → {{Arrowheads[Automatic], AbsoluteThickness[0.6]},
    {Arrowheads[Automatic], AbsoluteThickness[0.6]}},
  LabelStyle → {FontFamily → "Arial"},
  PlotLabel → {damp, optGaFra / gammaFrag,
    (iynorm[[2 ;; 8]] - normOleg4).Table[i, {i, 1, 7}]}]

```

■ Expt. ■  $\gamma_{\text{frag}}$   
 {0.21, 16.8, -0.0127329}

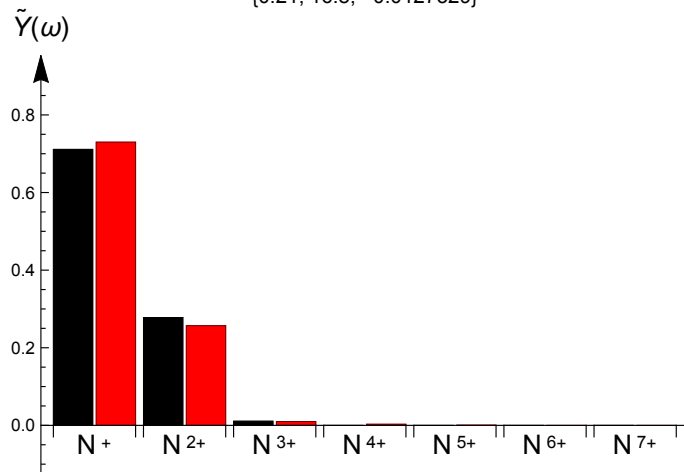

## 0.22

```

damp := 0.22

iy = dsionyieldcrateranalysisparam[damp * 0.15 * MilliJouleToHartree, photonenergy,
  tauX, nintdata, True, True, 1 / 1000, optfNppN, 1 - optfNppN, optGaFra]
iynorm = 1 / Total[iy[[2 ;; 8]]] * iy
Total[iynorm[[2 ;; 8]]]
{0.983732, 0.0117905, 0.00424498, 0.000172759,
 0.0000530065,  $6.18229 \times 10^{-6}$ ,  $6.82567 \times 10^{-8}$ ,  $1.41517 \times 10^{-10}$ ,
 0.98175, 0.000373687,  $3.0064 \times 10^{-76}$ ,  $-2.53447 \times 10^{-219}$ }

{60.4722, 0.724789, 0.260948, 0.0106199, 0.00325843, 0.000380039,  $4.19588 \times 10^{-6}$ ,
 8.69936  $\times 10^{-9}$ , 60.3503, 0.0229713,  $1.8481 \times 10^{-74}$ ,  $-1.55799 \times 10^{-217}$ }

1.

plotiy = Partition[Riffle[normOleg4, iynorm[[2 ;; 8]]], 2]
{{0.711226, 0.724789}, {0.277966, 0.260948}, {0.0108078, 0.0106199},
 {0., 0.00325843}, {0., 0.000380039}, {0.,  $4.19588 \times 10^{-6}$ }, {0.,  $8.69936 \times 10^{-9}$ }}

```

```
BarChart[plotiy, PlotRange → {-0.1, 0.9},
  ChartLabels → {Placed[{"N +", "N 2+", "N 3+", "N 4+", "N 5+", "N 6+", "N 7+"}, Below],
    Placed[{}, Above]},
  ChartLegends → Placed[{"Expt.", "γfrag"}, Top],
  ChartStyle → {Black, Red}, AxesLabel → {"", "Ỹ(ω)"},
  AxesStyle → {{Arrowheads[Automatic], AbsoluteThickness[0.6]},
    {Arrowheads[Automatic], AbsoluteThickness[0.6]}},
  LabelStyle → {FontFamily → "Arial"},
  PlotLabel → {damp, optGaFra / gammaFrag,
    (iynorm[[2 ;; 8]] - normOleg4).Table[i, {i, 1, 7}]]]
```

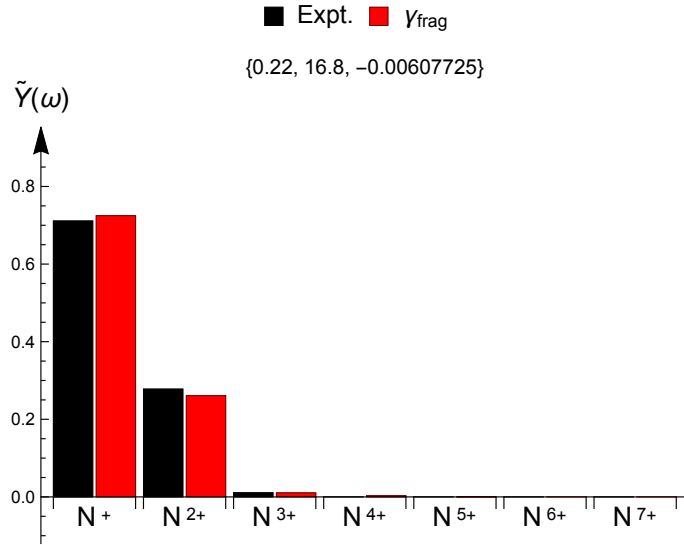

## 0.23

damp := 0.23

```
iy = dsionyieldcrateranalysisparam[damp * 0.15 * MilliJouleToHartree, photonenergy,
  tauX, nintdata, True, True, 1 / 1000, optfNppN, 1 - optfNppN, optGaFra]
```

```
iynorm = 1 / Total[iy[[2 ;; 8]]] * iy
```

```
Total[iynorm[[2 ;; 8]]]
```

```
{0.9831, 0.0121631, 0.00447592, 0.000193778,
  0.0000598441, 7.27419 × 10-6, 8.40901 × 10-8, 1.82387 × 10-10,
  0.981055, 0.000385001, 3.15261 × 10-76, 1.72172 × 10-168}
```

```
{58.1717, 0.71971, 0.264848, 0.0114662, 0.00354108, 0.000430426, 4.97575 × 10-6,
  1.07922 × 10-8, 58.0507, 0.0227812, 1.86545 × 10-74, 1.01877 × 10-166}
```

1.

```
plotiy = Partition[Riffle[normOleg4, iynorm[[2 ;; 8]]], 2]
```

```
{{0.711226, 0.71971}, {0.277966, 0.264848}, {0.0108078, 0.0114662},
  {0., 0.00354108}, {0., 0.000430426}, {0., 4.97575 × 10-6}, {0., 1.07922 × 10-8}}
```

```
BarChart[plotiy, PlotRange → {-0.1, 0.9},
  ChartLabels → {Placed[{"N +", "N 2+", "N 3+", "N 4+", "N 5+", "N 6+", "N 7+"}, Below],
    Placed[{}, Above]},
  ChartLegends → Placed[{"Expt.", "γfrag"}, Top],
  ChartStyle → {Black, Red}, AxesLabel → {"", "Ỹ(ω)",
  AxesStyle → {{Arrowheads[Automatic], AbsoluteThickness[0.6]},
    {Arrowheads[Automatic], AbsoluteThickness[0.6]}},
  LabelStyle → {FontFamily → "Arial"},
  PlotLabel → {damp, optGaFra / gammaFrag,
    (iynorm[[2 ;; 8]] - normOleg4).Table[i, {i, 1, 7}]]]
```

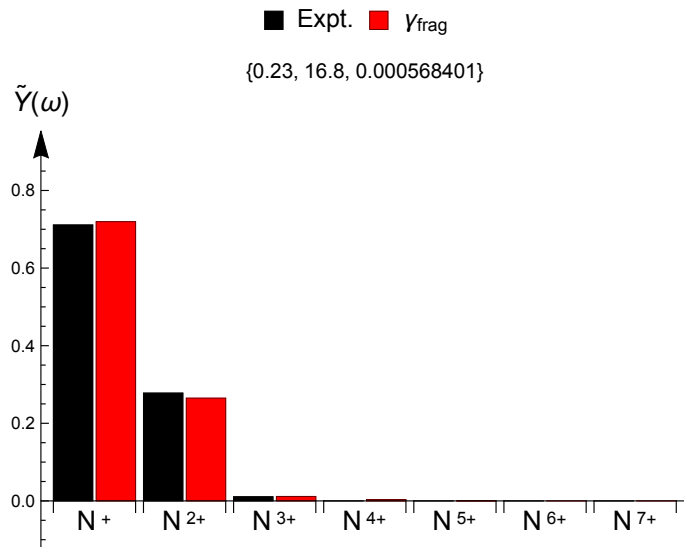

## 0.24

damp := 0.24

```
iy = dsionyieldcrateranalysisparam[damp * 0.15 * MilliJouleToHartree, photonenergy,
  tauX, nintdata, True, True, 1 / 1000, optfNppN, 1 - optfNppN, optGaFra]
```

```
iynorm = 1 / Total[iy[[2 ;; 8]]] * iy
```

```
Total[iynorm[[2 ;; 8]]]
```

```
{0.982476, 0.0125246, 0.00470787, 0.000216156,
  0.0000671865, 8.49564 × 10-6, 1.02637 × 10-7, 2.32448 × 10-10,
  0.980371, 0.000395943, 3.1498 × 10-76, 5.56527 × 10-174}
```

```
{56.0633, 0.714695, 0.268646, 0.0123345, 0.00383388, 0.000484789, 5.8568 × 10-6,
  1.32642 × 10-8, 55.9432, 0.0225938, 1.79738 × 10-74, 3.17573 × 10-172}
```

1.

```
plotiy = Partition[Riffle[normOleg4, iynorm[[2 ;; 8]]], 2]
```

```
{{0.711226, 0.714695}, {0.277966, 0.268646}, {0.0108078, 0.0123345},
  {0., 0.00383388}, {0., 0.000484789}, {0., 5.8568 × 10-6}, {0., 1.32642 × 10-8}}
```

```
BarChart[plotiy, PlotRange → {-0.1, 0.9},
  ChartLabels → {Placed[{"N +", "N 2+", "N 3+", "N 4+", "N 5+", "N 6+", "N 7+"}, Below],
    Placed[{}, Above]},
  ChartLegends → Placed[{"Expt.", "γfrag"}, Top],
  ChartStyle → {Black, Red}, AxesLabel → {"", "Ỹ(ω)",
  AxesStyle → {{Arrowheads[Automatic], AbsoluteThickness[0.6]},
    {Arrowheads[Automatic], AbsoluteThickness[0.6]}},
  LabelStyle → {FontFamily → "Arial"},
  PlotLabel → {damp, optGaFra / gammaFrag,
    (iynorm[[2 ;; 8]] - normOleg4).Table[i, {i, 1, 7}]]]
```

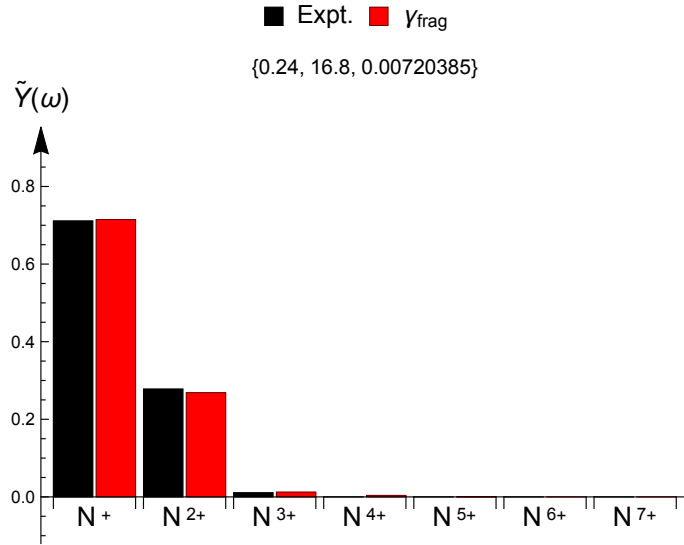

## 0.25

```
damp := 0.25

iy = dsionyieldcrateranalysisparam[damp * 0.15 * MilliJouleToHartree, photonenergy,
  tauX, nintdata, True, True, 1 / 1000, optfNppN, 1 - optfNppN, optGaFra]
iynorm = 1 / Total[iy[[2 ;; 8]]] * iy
Total[iynorm[[2 ;; 8]]]
{0.981859, 0.0128755, 0.00494062, 0.000239895,
  0.0000750426, 9.85476 × 10-6, 1.24208 × 10-7, 2.93221 × 10-10,
  0.979696, 0.000406527, 2.67533 × 10-76, -2.28275 × 10-169}

{54.1238, 0.709744, 0.272346, 0.0132239, 0.00413663, 0.000543232, 6.84683 × 10-6,
  1.61635 × 10-8, 54.0046, 0.0224093, 1.47474 × 10-74, -1.25834 × 10-167}

1.

plotiy = Partition[Riffle[normOleg4, iynorm[[2 ;; 8]]], 2]
{{0.711226, 0.709744}, {0.277966, 0.272346}, {0.0108078, 0.0132239},
  {0., 0.00413663}, {0., 0.000543232}, {0., 6.84683 × 10-6}, {0., 1.61635 × 10-8}}
```

```
BarChart[plotiy, PlotRange → {-0.1, 0.9},
  ChartLabels → {Placed[{"N +", "N 2+", "N 3+", "N 4+", "N 5+", "N 6+", "N 7+"}, Below],
    Placed[{}, Above]},
  ChartLegends → Placed[{"Expt.", "γfrag"}, Top],
  ChartStyle → {Black, Red}, AxesLabel → {"", "Ỹ(ω)"},
  AxesStyle → {{Arrowheads[Automatic], AbsoluteThickness[0.6]},
    {Arrowheads[Automatic], AbsoluteThickness[0.6]}},
  LabelStyle → {FontFamily → "Arial"},
  PlotLabel → {damp, optGaFra / gammaFrag,
    (iynorm[[2 ;; 8]] - normOleg4).Table[i, {i, 1, 7}]]]
```

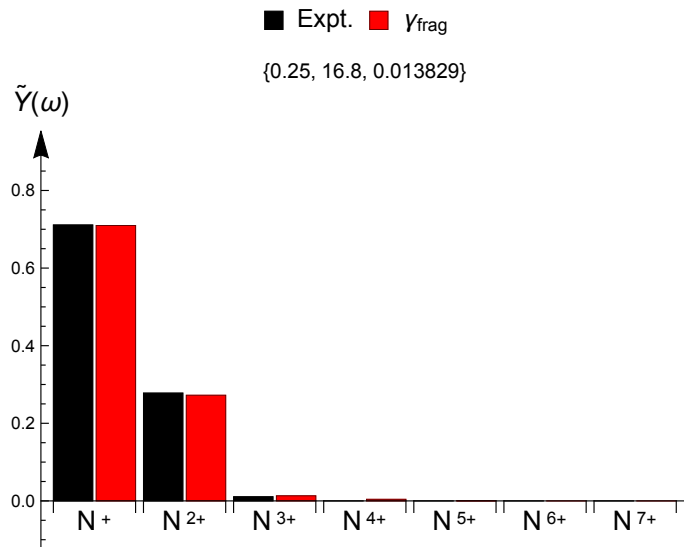

## References

- [1] S. Düsterer, P. Radcliffe, C. Bostedt, J. Bozek, A. L. Cavalieri, R. Coffee, J. T. Costello, D. Cubaynes, L. F. DiMauro, Y. Ding, G. Doumy, F. Grüner, W. Helml, W. Schweinberger, R. Kienberger, A. R. Maier, M. Messerschmidt, V. Richardson, C. Roedig, T. Tschentscher, M. Meyer, *New J. Phys.* **13**, 093024 (2011) [11 pages], *Femtosecond x-ray pulse length characterization at the Linac Coherent Light Source free-electron laser*, <http://dx.doi.org/10.1088/1367-2630/13/9/093024>
