# Supplementary material for: Rate equations for nitrogen molecules in ultrashort and intense x-ray pulses
Source: arXiv:1508.05223 ancillary file (2017-03-16)
Supplement: Supplementary file 8 [file nitrogen_dissociation_short_first.pdf]

```
<< PlotLegends`
```

General::obspkg: PlotLegends` is now obsolete. The legacy version being loaded may conflict with current functionality. See the Compatibility Guide for updating information.

```
Get["NitrogenRateEquations.m", Path -> NotebookDirectory[]]  
Get["NitrogenMoleculeRateEqs.m", Path -> NotebookDirectory[]]
```

```
HartreeToeV := 27.2113845  
eVToHartree := 1 / HartreeToeV  
JouleToHartree := 2.29371269*^-17  
MilliJouleToHartree := 1*^-3 * JouleToHartree  
BohrToAngstroem := 0.5291772083  
AngstroemToBohr := 1 / BohrToAngstroem  
MicrometerToBohr := 1*^4 * AngstroemToBohr  
BohrToMicrometer := 1 / MicrometerToBohr  
t0ToSecond := 24.18884326505*^-18  
t0ToFemtoSecond := 24.18884326505*^-3  
crossSectionAUtoBarn := 1*^8 * BohrToAngstroem^2  
crossSectionAUtocm2 := crossSectionAUtoBarn * 1*^-24  
crossSectioncm2toAU := 1 / crossSectionAUtocm2  
  
neginfinity := -1000 / t0ToFemtoSecond  
posinfinity := 10 000 / t0ToFemtoSecond
```

# Fragmentation time and pulse energy

Microscopic molecular rate-equation model with effective pulse duration and optimization for the N<sup>+</sup> yields

Christian Buth, 26 September 2014

Theoretische Chemie, Physikalisch-Chemisches Institut, Ruprecht-Karls-Universität Heidelberg, Im Neuenheimer Feld 229, 69120 Heidelberg, Germany

---

## Experimental parameters

Pulse energy fractions as determined in this *Mathematica* Notebook:

```
optdamp280 := 0.38  
optdamp80 := 0.30  
optdamp7 := 0.16  
optdamp4 := 0.23
```

Pulse energy fraction for the 4 fs pulse with respect to a pulse energy of 0.26 mJ instead of 0.15 mJ and vice versa for the 7 fs pulse:

```
optdamp4 * 0.15 / 0.26  
0.132692  
  
optdamp7 * 0.26 / 0.15  
0.277333
```

Pulse duration fractions. See Ref. [1] for measurements of LCLS pulse durations:

```
280 / 300 * 120
```

```
112
```

```
shtdur280 = 112 / 280.0
```

```
0.4
```

```
shtdur80 = 40 / 80.0
```

```
0.5
```

```
shtdur7 := 0.4
```

```
shtdur4 := 0.4
```

```
photonenergy := 1100 * eVToHartree
```

```
optfNppN := 0.26
```

```
newMatthias280 := {204.331, 105.281, 27.561, 13.151, 9.881, 0.587, 0.000}
```

```
normOleg280 = 1 / Total[newMatthias280] * newMatthias280
```

```
{0.56634, 0.291805, 0.0763903, 0.0364504, 0.027387, 0.00162698, 0.}
```

```
newMatthias80 := {218.068, 103.774, 26.075, 9.804, 3.315, 0.000, 0.000}
```

```
normOleg80 = 1 / Total[newMatthias80] * newMatthias80
```

```
{0.604006, 0.287434, 0.0722227, 0.0271552, 0.00918191, 0., 0.}
```

```
newMatthias7 := {221.485, 87.888, 9.342, 0.085, 0.000, 0.000, 0.000}
```

```
normOleg7 = 1 / Total[newMatthias7] * newMatthias7
```

```
{0.694746, 0.275684, 0.0293036, 0.000266625, 0., 0., 0.}
```

```
newMatthias4 := {92.985, 36.341, 1.413, 0, 0, 0, 0}
```

```
normOleg4 = 1 / Total[newMatthias4] * newMatthias4
```

```
{0.711226, 0.277966, 0.0108078, 0., 0., 0., 0.}
```

## Molecular fragmentation rate and pulse energy for a 280 fs pulse

```
tauX := shtdur280 * 280 / t0ToFemtoSecond
```

```
normfitconsts[damp_?NumericQ, gaFra_?NumericQ] := Module[{olegiy, olegiynorm},
  olegiy =
    dsionyieldcrateranalysisparam[damp * 0.26 * MilliJouleToHartree, photonenergy,
      tauX, nintdata, True, True, 1 / 1000, optfNppN, 1 - optfNppN, gaFra];
  olegiynorm = 1 / Total[olegiy[[2 ;; 8]]] * olegiy[[2 ;; 8]];
  Norm[(olegiynorm - normOleg280) * Table[{i, {i, 1, 7}}, 1] +
    16 * Abs[olegiynorm[[1]] - normOleg280[[1]]]
]
```

0.36

```
damp := 0.36
```

```

tabgamma =
  Table[{gaFra, normfitconsts[damp, gaFra * gammaFrag]}, {gaFra, 1, 10, 1 / 2}];

ListPlot[tabgamma, Joined -> True,
  PlotMarkers -> Automatic, PlotStyle -> {Thick, Red}]

```

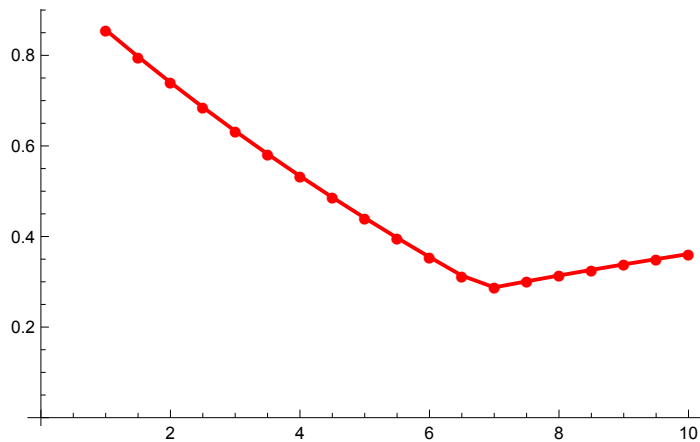

```

tabgamma =
  Table[{gaFra, normfitconsts[damp, gaFra * gammaFrag]}, {gaFra, 6, 8, 1 / 5}];

ListPlot[tabgamma, Joined -> True,
  PlotMarkers -> Automatic, PlotStyle -> {Thick, Red}]

```

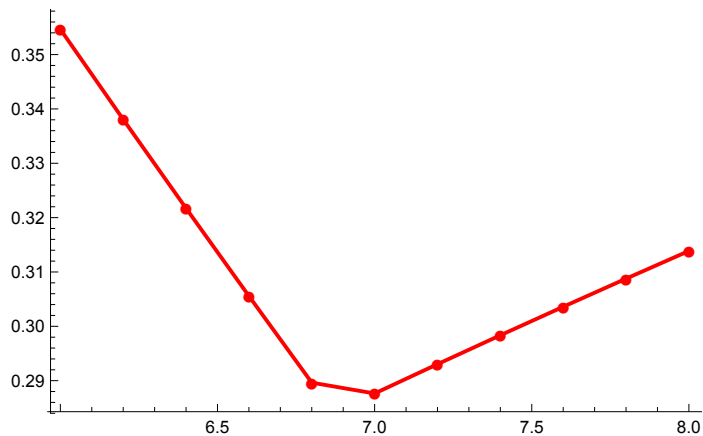

```

N[MinimalBy[tabgamma, Last]]
{{7., 0.287642}}

```

```

intgamma = Interpolation[tabgamma, x]

```

```

InterpolatingFunction[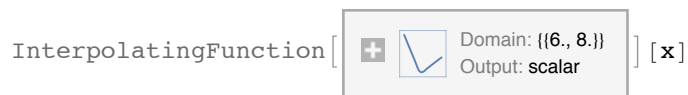 Domain: {{6., 8.}}  
Output: scalar][x]

```

```

mingamma = FindMinimum[intgamma, {x, 6.0, 8.0}]

```

```

InterpolatingFunction::dmval:

```

Input value {8.26425} lies outside the range of data in the interpolating function. Extrapolation will be used. >>

```

{0.287161, {x -> 6.93402}}

```

```

optent = x /. mingamma[[2]]

```

```

6.93402

```

```

optGaFra := optent * gammaFrag

iy = dsionyieldsanalysisparam[damp * 0.26 * MilliJouleToHartree, photonenergy,
  tauX, nintdata, True, True, 1 / 1000, optfNppN, 1 - optfNppN, optGaFra]
iynorm = 1 / Total[iy[[2 ;; 8]]] * iy
Total[iynorm[[2 ;; 8]]]

{0.963372, 0.0207511, 0.0118017, 0.00153621, 0.00187953, 0.0005874, 0.0000687927,
  3.14419 × 10-6, 0.959919, 0.000628799, 1.26705 × 10-32, -2.47521 × 10-112}

{26.3016, 0.566539, 0.322204, 0.041941, 0.0513142, 0.016037, 0.00187815,
  0.0000858415, 26.2073, 0.0171672, 3.45925 × 10-31, -6.75774 × 10-111}

1.

plotiy = Partition[Riffle[normOleg280, iynorm[[2 ;; 8]]], 2]
{{0.56634, 0.566539}, {0.291805, 0.322204},
 {0.0763903, 0.041941}, {0.0364504, 0.0513142},
 {0.027387, 0.016037}, {0.00162698, 0.00187815}, {0., 0.0000858415}}

BarChart[plotiy, PlotRange → {-0.1, 0.9},
  ChartLabels → {Placed[{"N+", "N2+", "N3+", "N4+", "N5+", "N6+", "N7+"}, Below],
    Placed[{}, Above]},
  ChartLegends → Placed[{"Expt.", "γfrag"}, Top],
  ChartStyle → {Black, Red}, AxesLabel → {"", "Ỹ(ω)"},
  AxesStyle → {{Arrowheads[Automatic], AbsoluteThickness[0.6]},
    {Arrowheads[Automatic], AbsoluteThickness[0.6]}},
  LabelStyle → {FontFamily → "Arial"},
  PlotLabel → {damp, optGaFra / gammaFrag,
    (iynorm[[2 ;; 8]] - normOleg280).Table[i, {i, 1, 7}]]}

■ Expt. ■ γfrag
{0.36, 6.93402, -0.0375369}

```

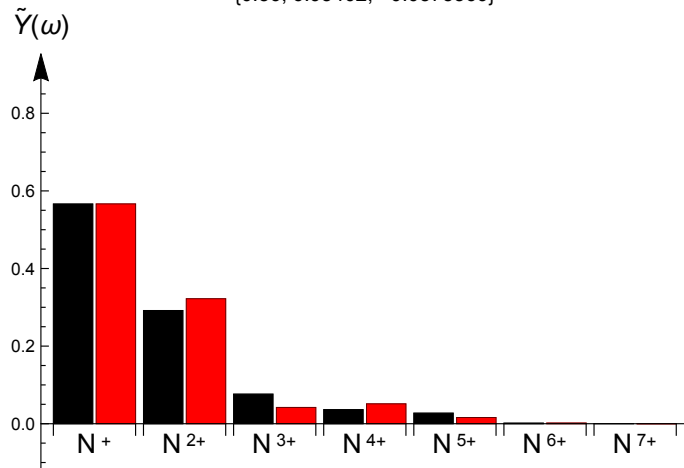

### 0.37

```

damp := 0.37

tabgamma =
  Table[{gaFra, normfitconsts[damp, gaFra * gammaFrag]}, {gaFra, 5, 15, 1 / 2}];

```

```
ListPlot[tabgamma, Joined -> True,
PlotMarkers -> Automatic, PlotStyle -> {Thick, Red}]
```

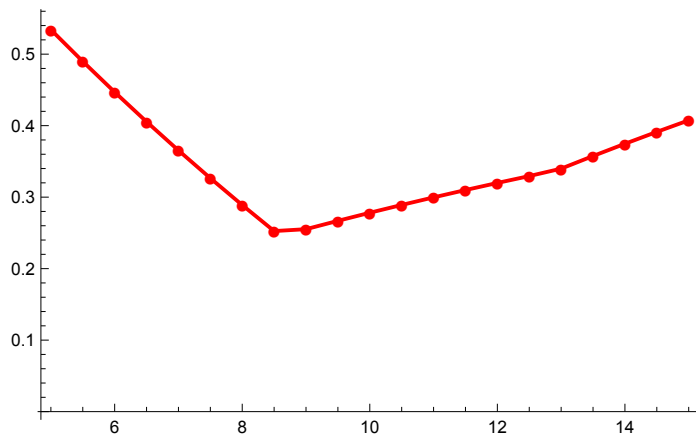

```
tabgamma =
Table[{gaFra, normfitconsts[damp, gaFra * gammaFrag]}, {gaFra, 7.5, 9.5, 1 / 5}];
```

```
ListPlot[tabgamma, Joined -> True,
PlotMarkers -> Automatic, PlotStyle -> {Thick, Red}]
```

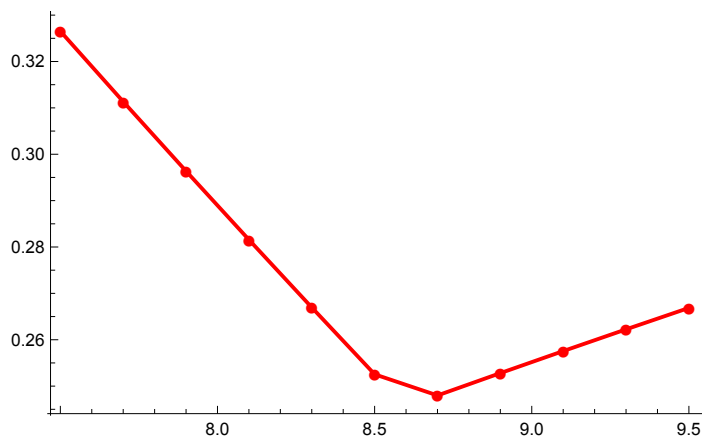

```
N[MinimalBy[tabgamma, Last]]
```

```
{{8.7, 0.247991}}
```

```
intgamma = Interpolation[tabgamma, x]
```

```
InterpolatingFunction[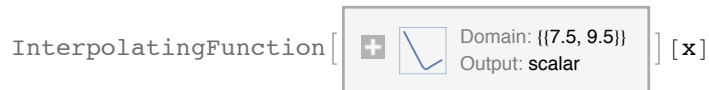 Domain: {{7.5, 9.5}}  
Output: scalar] [x]
```

```
mingamma = FindMinimum[intgamma, {x, 7.5, 9.5}]
```

```
InterpolatingFunction::dmval:
```

```
Input value {9.76425} lies outside the range of data in the interpolating function. Extrapolation will be used. >>
```

```
{0.247988, {x -> 8.69543}}
```

```
optent = x /. mingamma[[2]]
```

```
8.69543
```

```
optGaFra := optent * gammaFrag
```

```

iy = dsionyieldcrateranalysisparam[damp * 0.26 * MilliJouleToHartree, photonenergy,
  tauX, nintdata, True, True, 1 / 1000, optfNppN, 1 - optfNppN, optGaFra]
iynorm = 1 / Total[iy[[2 ;; 8]]] * iy
Total[iynorm[[2 ;; 8]]]

```

```

{0.962718, 0.0211242, 0.0116709, 0.00179078,
 0.00195072, 0.000660812, 0.0000803139,  $3.91436 \times 10^{-6}$ ,
 0.959202, 0.000633827,  $2.85961 \times 10^{-40}$ ,  $3.59304 \times 10^{-113}$ }

```

```

{25.8228, 0.566612, 0.313046, 0.0480337, 0.0523238, 0.0177249, 0.00215425,
 0.000104994, 25.7285, 0.017001,  $7.67029 \times 10^{-39}$ ,  $9.63756 \times 10^{-112}$ }

```

1.

```

plotiy = Partition[Riffle[normOleg280, iynorm[[2 ;; 8]]], 2]

```

```

{{0.56634, 0.566612}, {0.291805, 0.313046},
 {0.0763903, 0.0480337}, {0.0364504, 0.0523238},
 {0.027387, 0.0177249}, {0.00162698, 0.00215425}, {0., 0.000104994}}

```

```

BarChart[plotiy, PlotRange → {-0.1, 0.9},
  ChartLabels → {Placed[{"N +", "N 2+", "N 3+", "N 4+", "N 5+", "N 6+", "N 7+"}, Below],
    Placed[{}, Above]},
  ChartLegends → Placed[{"Expt.", " $\gamma_{frag}$ "}, Top],
  ChartStyle → {Black, Red}, AxesLabel → {"", " $\tilde{Y}(\omega)$ "},
  AxesStyle → {{Arrowheads[Automatic], AbsoluteThickness[0.6]},
    {Arrowheads[Automatic], AbsoluteThickness[0.6]}},
  LabelStyle → {FontFamily → "Arial"},
  PlotLabel → {damp, optGaFra / gammaFrag,
    (iynorm[[2 ;; 8]] - normOleg280).Table[i, {i, 1, 7}]}]

```

■ Expt. ■  $\gamma_{frag}$

{0.37, 8.69543, -0.0232341}

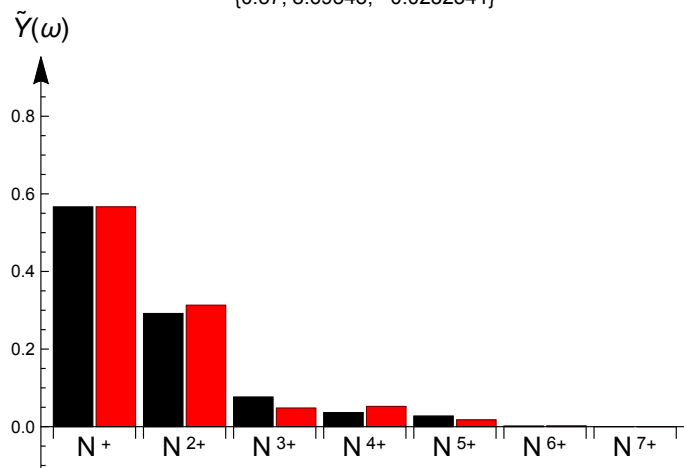

## 0.38

```

damp := 0.38

```

```

tabgamma =
  Table[{gaFra, normfitconsts[damp, gaFra * gammaFrag]}, {gaFra, 5, 15, 1 / 2}];

```

```
ListPlot[tabgamma, Joined -> True,
PlotMarkers -> Automatic, PlotStyle -> {Thick, Red}]
```

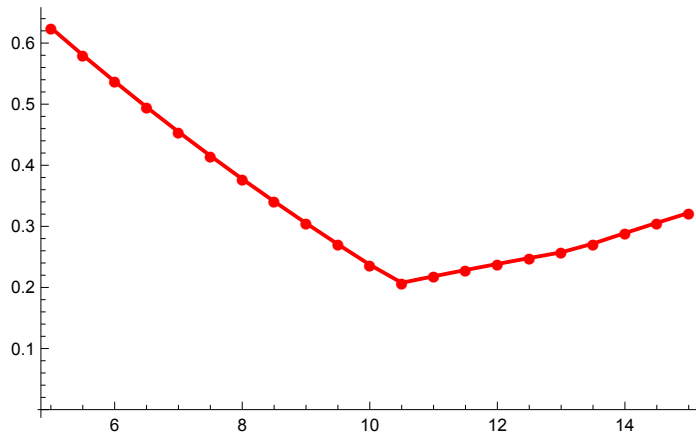

```
tabgamma =
Table[{gaFra, normfitconsts[damp, gaFra * gammaFrag]}, {gaFra, 9.5, 11.5, 1 / 5}];
```

```
ListPlot[tabgamma, Joined -> True,
PlotMarkers -> Automatic, PlotStyle -> {Thick, Red}]
```

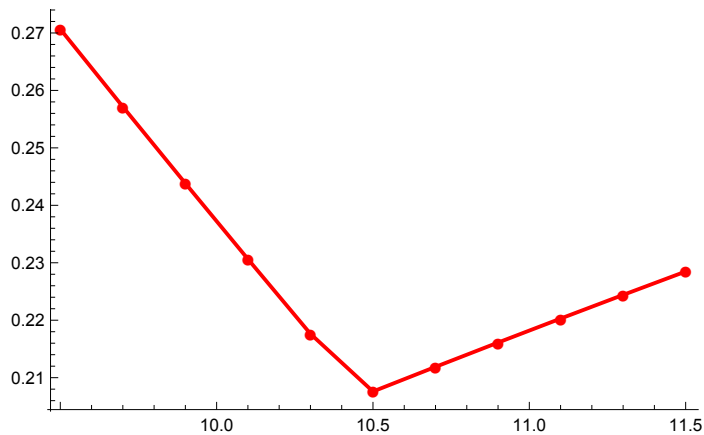

```
N[MinimalBy[tabgamma, Last]]
```

```
{{10.5, 0.207596}}
```

```
intgamma = Interpolation[tabgamma, x]
```

InterpolatingFunction[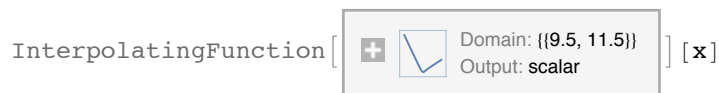 Domain: {{9.5, 11.5}}  
Output: scalar] [x]

```
mingamma = FindMinimum[intgamma, {x, 9.5, 11.5}]
```

```
InterpolatingFunction::dmval:
```

```
Input value {11.7642} lies outside the range of data in the interpolating function. Extrapolation will be used. >>
```

```
{0.207588, {x -> 10.5068}}
```

```
optent = x /. mingamma[[2]]
```

```
10.5068
```

```
optGaFra := optent * gammaFrag
```

```

iy = dsionyieldcrateranalysisparam[damp * 0.26 * MilliJouleToHartree, photonenergy,
  tauX, nintdata, True, True, 1 / 1000, optfNppN, 1 - optfNppN, optGaFra]
iynorm = 1 / Total[iy[[2 ;; 8]]] * iy
Total[iynorm[[2 ;; 8]]]

{0.962076, 0.021482, 0.0115483, 0.00204007, 0.00201987, 0.000736734, 0.0000927799,
  4.78928 × 10-6, 0.958498, 0.000638571, 4.28088 × 10-48, -3.18053 × 10-95}

{25.3682, 0.56644, 0.304508, 0.0537928, 0.0532602, 0.0194263, 0.00244644,
  0.000126284, 25.2739, 0.016838, 1.12879 × 10-46, -8.38648 × 10-94}

1.

```

```

plotiy = Partition[Riffle[normOleg280, iynorm[[2 ;; 8]]], 2]
{{0.56634, 0.56644}, {0.291805, 0.304508},
 {0.0763903, 0.0537928}, {0.0364504, 0.0532602},
 {0.027387, 0.0194263}, {0.00162698, 0.00244644}, {0., 0.000126284}}

BarChart[plotiy, PlotRange → {-0.1, 0.9},
  ChartLabels → {Placed[{"N +", "N 2+", "N 3+", "N 4+", "N 5+", "N 6+", "N 7+"}, Below],
    Placed[{}, Above]},
  ChartLegends → Placed[{"Expt.", "γfrag"}, Top],
  ChartStyle → {Black, Red}, AxesLabel → {"", "Ỹ(ω)"},
  AxesStyle → {{Arrowheads[Automatic], AbsoluteThickness[0.6]},
    {Arrowheads[Automatic], AbsoluteThickness[0.6]}},
  LabelStyle → {FontFamily → "Arial"},
  PlotLabel → {damp, optGaFra / gammaFrag,
    (iynorm[[2 ;; 8]] - normOleg280).Table[i, {i, 1, 7}]]}

■ Expt. ■ γfrag
{0.38, 10.5068, -0.00905058}

```

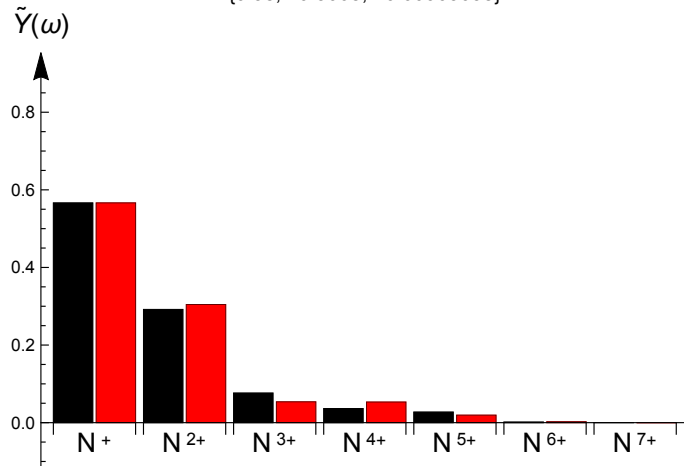

### 0.39

```

damp := 0.39

tabgamma =
  Table[{gaFra, normfitconsts[damp, gaFra * gammaFrag]}, {gaFra, 8, 18, 1 / 2}];

```



```
ListPlot[tabgamma, Joined -> True,
PlotMarkers -> Automatic, PlotStyle -> {Thick, Red}]
```

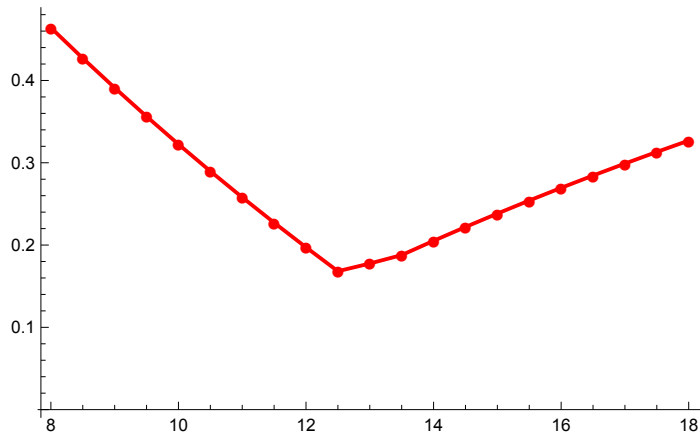

```
tabgamma = Table[
{gaFra, normfitconsts[damp, gaFra * gammaFrag]}, {gaFra, 11.5, 13.5, 1/5}];
```

```
ListPlot[tabgamma, Joined -> True,
PlotMarkers -> Automatic, PlotStyle -> {Thick, Red}]
```

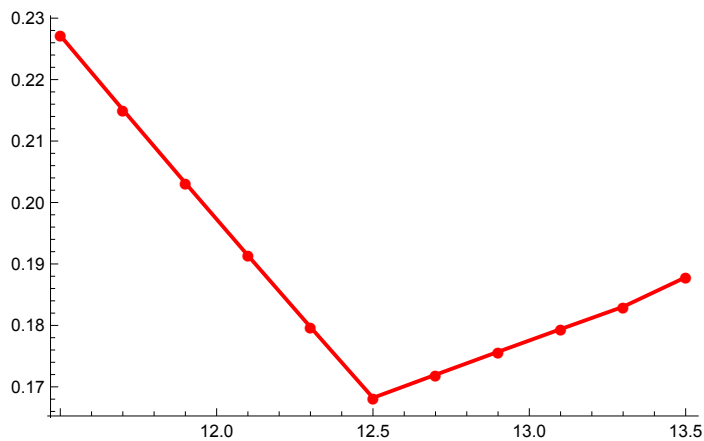

```
N[MinimalBy[tabgamma, Last]]
```

```
{{12.5, 0.168212}}
```

```
intgamma = Interpolation[tabgamma, x]
```

```
InterpolatingFunction[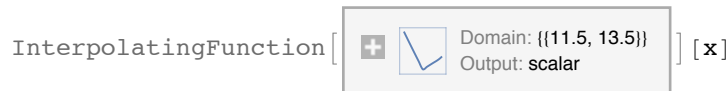 Domain: {{11.5, 13.5}}  
Output: scalar][x]
```

```
mingamma = FindMinimum[intgamma, {x, 11.5, 13.5}]
```

```
InterpolatingFunction::dmval:
```

```
Input value {13.7642} lies outside the range of data in the interpolating function. Extrapolation will be used. >>
```

```
{0.168152, {x -> 12.5183}}
```

```
optent = x /. mingamma[[2]]
```

```
12.5183
```

```
optGaFra := optent * gammaFrag
```

```

iy = dsionyieldcrateranalysisparam[damp * 0.26 * MilliJouleToHartree, photonenergy,
  tauX, nintdata, True, True, 1 / 1000, optfNppN, 1 - optfNppN, optGaFra]
iynorm = 1 / Total[iy[[2 ;; 8]]] * iy
Total[iynorm[[2 ;; 8]]]

{0.961445, 0.0218366, 0.0114068, 0.00229721, 0.00208464, 0.000817078, 0.000106528,
  5.80568 × 10-6, 0.957808, 0.00064305, 8.32536 × 10-57, -2.08176 × 10-114}

{24.9372, 0.56638, 0.29586, 0.0595833, 0.0540698, 0.0211927, 0.00276304,
  0.000150583, 24.8429, 0.0166789, 2.15937 × 10-55, -5.39952 × 10-113}

1.

```

```

plotiy = Partition[Riffle[normOleg280, iynorm[[2 ;; 8]]], 2]
{{0.56634, 0.56638}, {0.291805, 0.29586},
 {0.0763903, 0.0595833}, {0.0364504, 0.0540698},
 {0.027387, 0.0211927}, {0.00162698, 0.00276304}, {0., 0.000150583}}

BarChart[plotiy, PlotRange → {-0.1, 0.9},
  ChartLabels → {Placed[{"N +", "N 2+", "N 3+", "N 4+", "N 5+", "N 6+", "N 7+"}, Below],
    Placed[{}, Above]},
  ChartLegends → Placed[{"Expt.", "γfrag"}, Top],
  ChartStyle → {Black, Red}, AxesLabel → {"", "Ỹ(ω)"},
  AxesStyle → {{Arrowheads[Automatic], AbsoluteThickness[0.6]},
    {Arrowheads[Automatic], AbsoluteThickness[0.6]}},
  LabelStyle → {FontFamily → "Arial"},
  PlotLabel → {damp, optGaFra / gammaFrag,
    (iynorm[[2 ;; 8]] - normOleg280).Table[i, {i, 1, 7}]}]

```

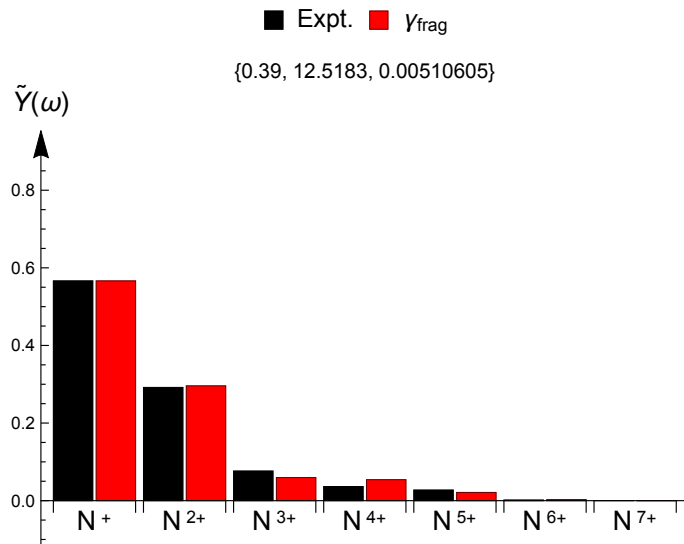

0.40

damp := 0.40

tabgamma =

Table[{gaFra, normfitconsts[damp, gaFra \* gammaFrag]}, {gaFra, 8, 18, 1 / 2}];

```
ListPlot[tabgamma, Joined -> True,
  PlotMarkers -> Automatic, PlotStyle -> {Thick, Red}]
```

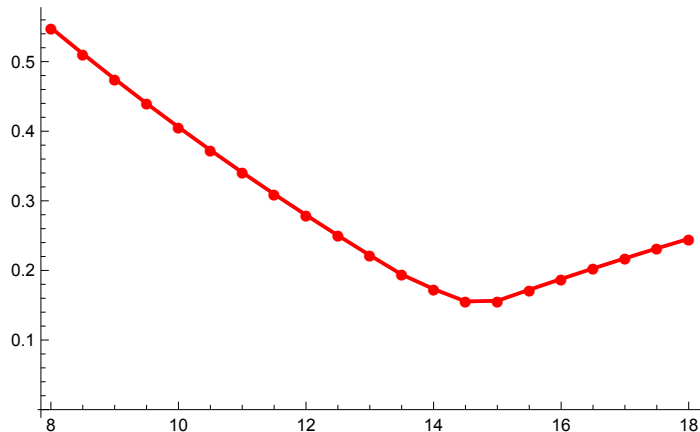

```
tabgamma = Table[
  {gaFra, normfitconsts[damp, gaFra * gammaFrag]}, {gaFra, 13.5, 15.5, 1/5}];
```

```
ListPlot[tabgamma, Joined -> True,
  PlotMarkers -> Automatic, PlotStyle -> {Thick, Red}]
```

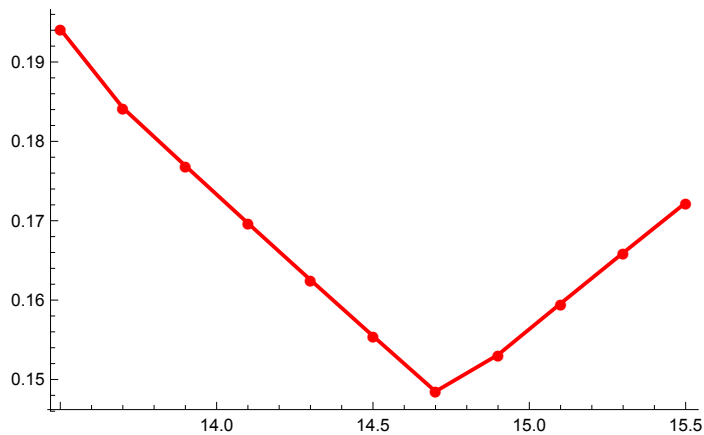

```
N[MinimalBy[tabgamma, Last]]
```

```
{{14.7, 0.148487}}
```

```
intgamma = Interpolation[tabgamma, x]
```

InterpolatingFunction[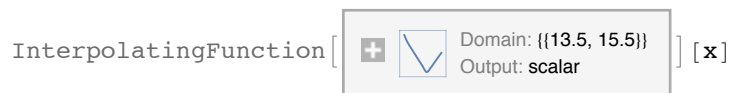 Domain: {{13.5, 15.5}}  
Output: scalar][x]

```
mingamma = FindMinimum[intgamma, {x, 13.5, 15.5}]
```

```
InterpolatingFunction::dmval:
```

```
Input value {17.2069} lies outside the range of data in the interpolating function. Extrapolation will be used. >>
```

```
{0.148487, {x -> 14.7}}
```

```
optent = x /. mingamma[[2]]
```

```
14.7
```

```
optGaFra := optent * gammaFrag
```

```

iy = dsionyieldcrateranalysisparam[damp * 0.26 * MilliJouleToHartree, photonenergy,
  tauX, nintdata, True, True, 1 / 1000, optfNppN, 1 - optfNppN, optGaFra]
iynorm = 1 / Total[iy[[2 ;; 8]]] * iy
Total[iynorm[[2 ;; 8]]]

{0.960827, 0.0221832, 0.0112586, 0.00255629, 0.00214574, 0.000900966, 0.000121489,
  6.96667 × 10-6, 0.957131, 0.000647275, 3.40843 × 10-57, -2.08626 × 10-95}

{24.5276, 0.566284, 0.287406, 0.0652559, 0.0547757, 0.0229995, 0.00310134,
  0.000177842, 24.4333, 0.0165234, 8.70092 × 10-56, -5.32572 × 10-94}

1.

```

```

plotiy = Partition[Riffle[normOleg280, iynorm[[2 ;; 8]]], 2]
{{0.56634, 0.566284}, {0.291805, 0.287406},
 {0.0763903, 0.0652559}, {0.0364504, 0.0547757},
 {0.027387, 0.0229995}, {0.00162698, 0.00310134}, {0., 0.000177842}}

BarChart[plotiy, PlotRange → {-0.1, 0.9},
  ChartLabels → {Placed[{"N+", "N2+", "N3+", "N4+", "N5+", "N6+", "N7+"}, Below],
    Placed[{}, Above]},
  ChartLegends → Placed[{"Expt.", "γfrag"}, Top],
  ChartStyle → {Black, Red}, AxesLabel → {"", "Ỹ(ω)"},
  AxesStyle → {{Arrowheads[Automatic], AbsoluteThickness[0.6]},
    {Arrowheads[Automatic], AbsoluteThickness[0.6]}},
  LabelStyle → {FontFamily → "Arial"},
  PlotLabel → {damp, optGaFra / gammaFrag,
    (iynorm[[2 ;; 8]] - normOleg280).Table[i, {i, 1, 7}]]}

■ Expt. ■ γfrag
{0.4, 14.7, 0.0191968}

```

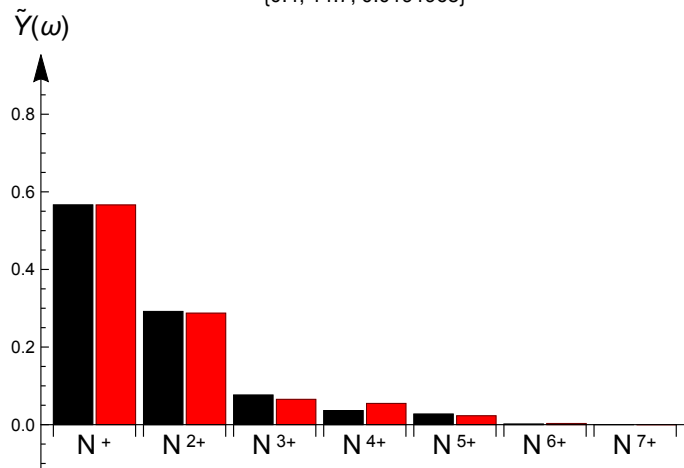

## Molecular fragmentation rate and pulse energy for a 80 fs pulse

```
tauX := shtdur80 * 80 / t0ToFemtoSecond
```

```

normfitconsts[damp_?NumericQ, gaFra_?NumericQ] := Module[{olegiy, olegiynorm},
  olegiy =
    dsionyieldcrateranalysisparam[damp * 0.26 * MilliJouleToHartree, photonenergy,
      tauX, nintdata, True, True, 1 / 1000, optfNppN, 1 - optfNppN, gaFra];
  olegiynorm = 1 / Total[olegiy[[2 ;; 8]] * olegiy[[2 ;; 8]]];
  Norm[(olegiynorm - normOleg80) * Table[i, {i, 1, 7}], 1] +
    16 * Abs[olegiynorm[[1]] - normOleg80[[1]]]
]

```

## 0.28

```
damp := 0.28
```

```

tabgamma =
  Table[{gaFra, normfitconsts[damp, gaFra * gammaFrag]}, {gaFra, 1, 20, 1 / 2}];

```

```

ListPlot[tabgamma, Joined -> True,
  PlotMarkers -> Automatic, PlotStyle -> {Thick, Red}]

```

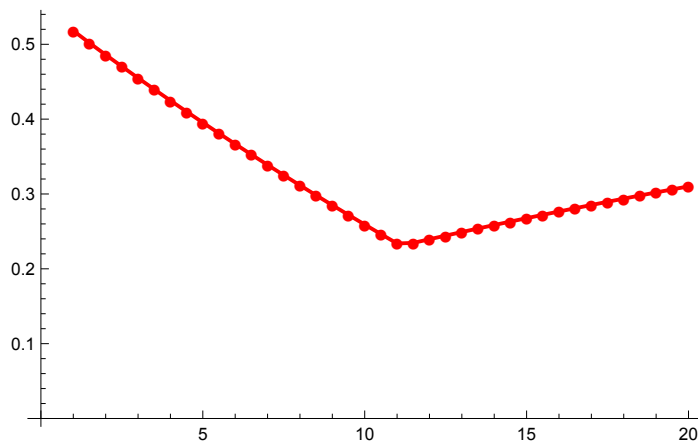

```

tabgamma =
  Table[{gaFra, normfitconsts[damp, gaFra * gammaFrag]}, {gaFra, 10, 12, 1 / 5}];

```

```

ListPlot[tabgamma, Joined -> True,
  PlotMarkers -> Automatic, PlotStyle -> {Thick, Red}]

```

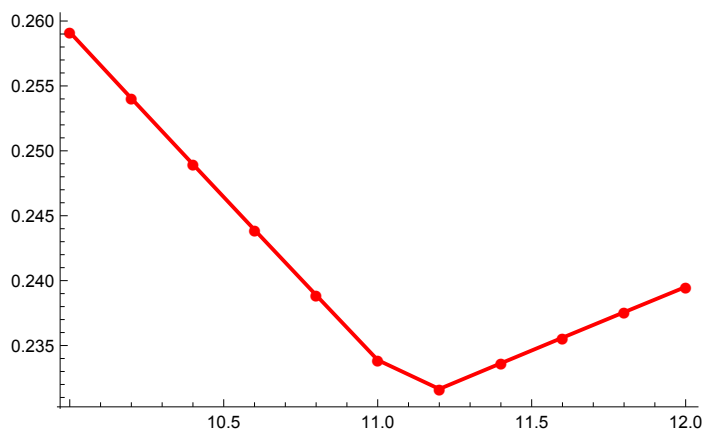

```
N[MinimalBy[tabgamma, Last]]
```

```
{{11.2, 0.23165}}
```

```
intgamma = Interpolation[tabgamma, x]
```

```
InterpolatingFunction[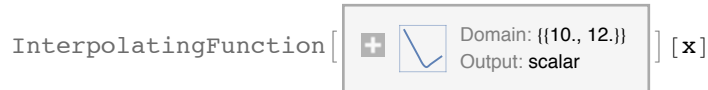 Domain: {{10., 12.}}  
Output: scalar ] [x]
```

```
mingamma = FindMinimum[intgamma, {x, 10.0, 12.0}]
```

InterpolatingFunction::dmval:

Input value {12.2642} lies outside the range of data in the interpolating function. Extrapolation will be used. >>

```
{0.23165, {x → 11.2}}
```

```
optent = x /. mingamma[[2]]
```

```
11.2
```

```
optGaFra := optent * gammaFrag
```

```
iy = dsionyieldcrateranalysisparam[damp * 0.26 * MilliJouleToHartree, photonenergy,  
tauX, nintdata, True, True, 1 / 1000, optfNppN, 1 - optfNppN, optGaFra]
```

```
inyorm = 1 / Total[iy[[2 ;; 8]]] * iy
```

```
Total[iynorm[[2 ;; 8]]]
```

```
{0.969291, 0.0185509, 0.0099918, 0.000942977,  
0.000973042, 0.000231964, 0.000017834, 4.63845 × 10-7,  
0.966197, 0.000576154, 2.68903 × 10-51, -5.36711 × 10-136}
```

```
{31.5638, 0.604087, 0.325371, 0.0307069, 0.0316859, 0.00755361, 0.000580742,  
0.0000151045, 31.463, 0.0187618, 8.75649 × 10-50, -1.74773 × 10-134}
```

```
1.
```

```
plotiy = Partition[Riffle[normOleg80, iynorm[[2 ;; 8]]], 2]
```

```
{{0.604006, 0.604087}, {0.287434, 0.325371},  
{0.0722227, 0.0307069}, {0.0271552, 0.0316859},  
{0.00918191, 0.00755361}, {0., 0.000580742}, {0., 0.0000151045}}
```

```
BarChart[plotiy, PlotRange → {-0.1, 0.9},
  ChartLabels → {Placed[{"N +", "N 2+", "N 3+", "N 4+", "N 5+", "N 6+", "N 7+"}, Below],
    Placed[{}, Above]},
  ChartLegends → Placed[{"Expt.", " $\gamma_{frag}$ "}, Top],
  ChartStyle → {Black, Red}, AxesLabel → {"", " $\tilde{Y}(\omega)$ "},
  AxesStyle → {{Arrowheads[Automatic], AbsoluteThickness[0.6]},
    {Arrowheads[Automatic], AbsoluteThickness[0.6]}},
  LabelStyle → {FontFamily → "Arial"},
  PlotLabel → {damp, optGaFra / gammaFrag,
    (iynorm[2 ;; 8] - normOleg80).Table[i, {i, 1, 7}]]}
```

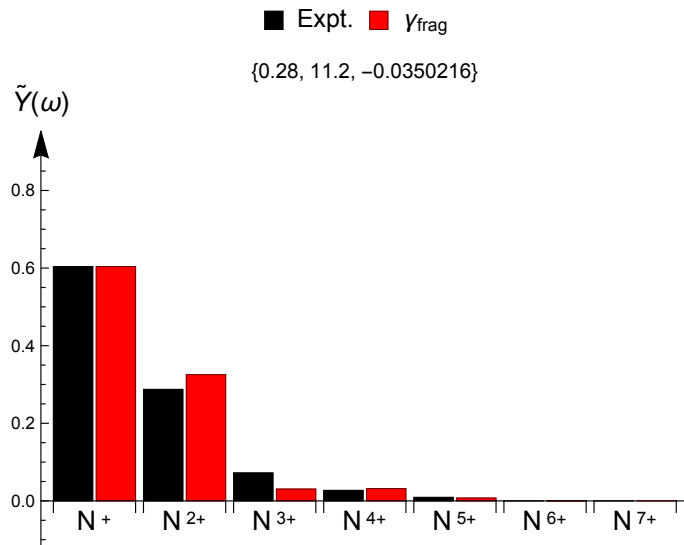

## 0.29

damp := 0.29

```
tabgamma =
  Table[{gaFra, normfitconsts[damp, gaFra * gammaFrag]}, {gaFra, 14, 24, 1/2}];
ListPlot[tabgamma, Joined -> True,
  PlotMarkers -> Automatic, PlotStyle -> {Thick, Red}]
```

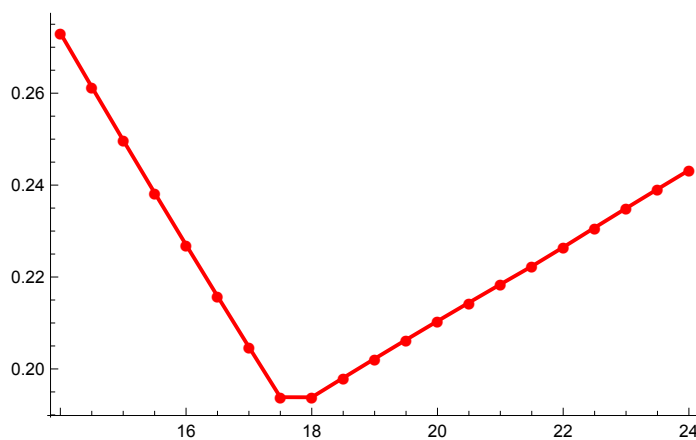

```
tabgamma =
  Table[{gaFra, normfitconsts[damp, gaFra * gammaFrag]}, {gaFra, 17, 19, 1/5}];
```

```
ListPlot[tabgamma, Joined -> True,
  PlotMarkers -> Automatic, PlotStyle -> {Thick, Red}]
```

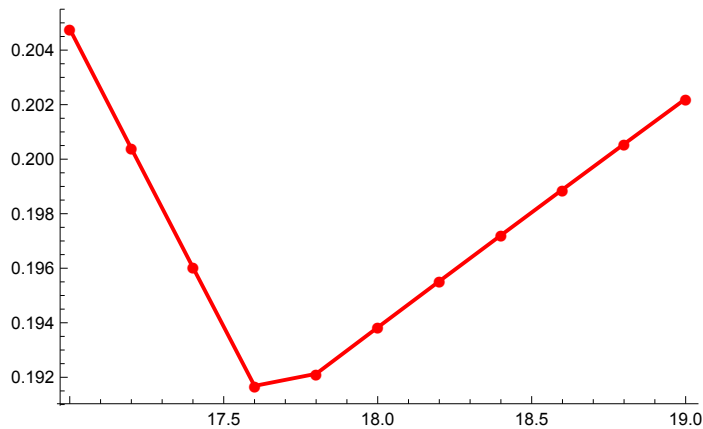

```
N[MinimalBy[tabgamma, Last]]
```

```
{{17.6, 0.191685}}
```

```
intgamma = Interpolation[tabgamma, x]
```

```
InterpolatingFunction[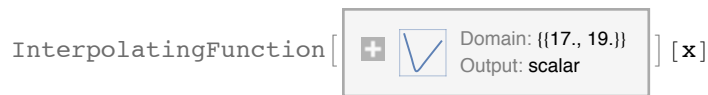 Domain: {{17., 19.}}  
Output: scalar] [x]
```

```
mingamma = FindMinimum[intgamma, {x, 17.0, 19.0}]
```

InterpolatingFunction::dmval:

Input value {19.2642} lies outside the range of data in the interpolating function. Extrapolation will be used. >>

```
{0.191474, {x -> 17.6646}}
```

```
optent = x /. mingamma[[2]]
```

```
17.6646
```

```
optGaFra := optent * gammaFrag
```

```
iy = dsionyieldcrateranalysisparam[damp * 0.26 * MilliJouleToHartree, photonenergy,  
  tauX, nintdata, True, True, 1 / 1000, optfNppN, 1 - optfNppN, optGaFra]
```

```
iynorm = 1 / Total[iy[[2 ;; 8]]] * iy
```

```
Total[iynorm[[2 ;; 8]]]
```

```
{0.968526, 0.019011, 0.00993423, 0.00118319,  
  0.00104471, 0.000277703, 0.0000223098, 6.22615 × 10-7,  
  0.965355, 0.000584142, 1.27134 × 10-79, -5.1043 × 10-136}}
```

```
{30.7725, 0.604026, 0.315636, 0.037593, 0.033193, 0.00882333, 0.000708838,  
  0.0000197821, 30.6718, 0.0185597, 4.03936 × 10-78, -1.62177 × 10-134}}
```

```
1.
```

```
plotiy = Partition[Riffle[normOleg80, iynorm[[2 ;; 8]]], 2]
```

```
{{0.604006, 0.604026}, {0.287434, 0.315636},  
  {0.0722227, 0.037593}, {0.0271552, 0.033193},  
  {0.00918191, 0.00882333}, {0., 0.000708838}, {0., 0.0000197821}}
```



```
BarChart[plotiy, PlotRange → {-0.1, 0.9},
  ChartLabels → {Placed[{"N +", "N 2+", "N 3+", "N 4+", "N 5+", "N 6+", "N 7+"}, Below],
    Placed[{}, Above]},
  ChartLegends → Placed[{"Expt.", "γfrag"}, Top],
  ChartStyle → {Black, Red}, AxesLabel → {"", "Ỹ(ω)",
  AxesStyle → {{Arrowheads[Automatic], AbsoluteThickness[0.6]},
    {Arrowheads[Automatic], AbsoluteThickness[0.6]}},
  LabelStyle → {FontFamily → "Arial"},
  PlotLabel → {damp, optGaFra / gammaFrag,
    (iynorm[2 ;; 8] - normOleg80).Table[i, {i, 1, 7}]]]
```

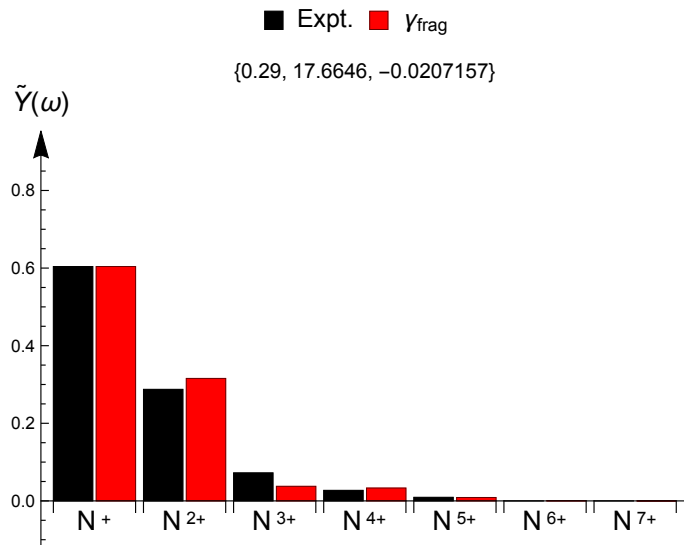

### 0.30

```
damp := 0.30
```

```
tabgamma =
  Table[{gaFra, normfitconsts[damp, gaFra * gammaFrag]}, {gaFra, 10, 30, 1 / 2}];
```

```
ListPlot[tabgamma, Joined -> True,
  PlotMarkers -> Automatic, PlotStyle -> {Thick, Red}]
```

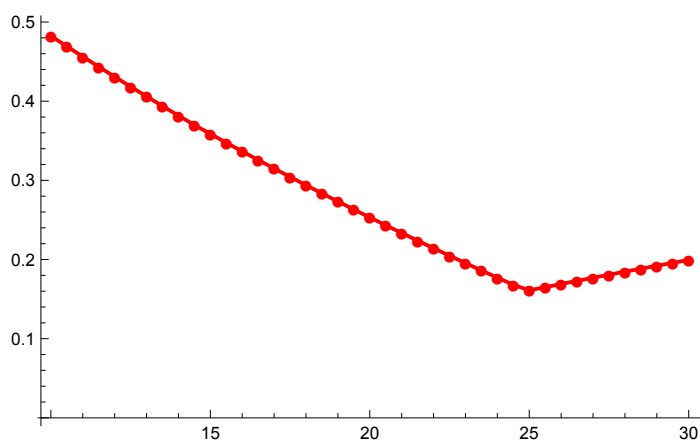

```
tabgamma =
  Table[{gaFra, normfitconsts[damp, gaFra * gammaFrag]}, {gaFra, 24, 26, 1 / 5}];
```

```
ListPlot[tabgamma, Joined -> True,
PlotMarkers -> Automatic, PlotStyle -> {Thick, Red}]
```

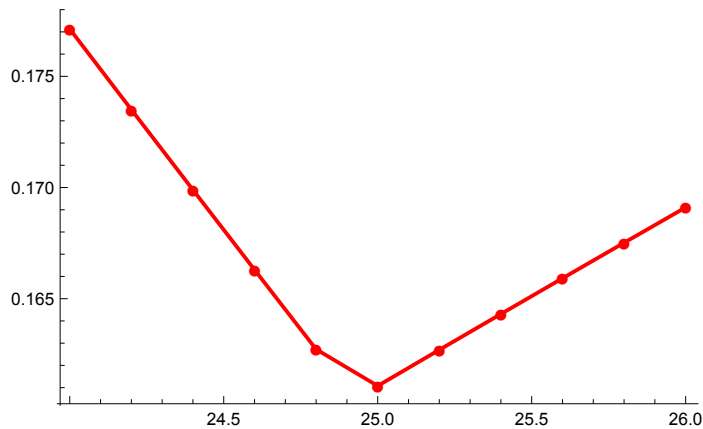

```
N[MinimalBy[tabgamma, Last]]
```

```
{{25., 0.161079}}
```

```
intgamma = Interpolation[tabgamma, x]
```

```
InterpolatingFunction[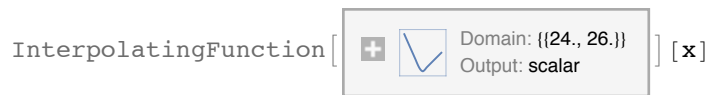 Domain: {{24., 26.}}  
Output: scalar][x]
```

```
mingamma = FindMinimum[intgamma, {x, 24.0, 26.0}]
```

```
InterpolatingFunction::dmval:
```

Input value {26.2642} lies outside the range of data in the interpolating function. Extrapolation will be used. >>

```
{0.161079, {x -> 25.}}
```

```
optent = x /. mingamma[[2]]
```

```
25.
```

```
optGaFra := optent * gammaFrag
```

```
iy = dsionyieldcrateranalysisparam[damp * 0.26 * MilliJouleToHartree, photonenergy,  
tauX, nintdata, True, True, 1 / 1000, optfNppN, 1 - optfNppN, optGaFra]
```

```
inyorm = 1 / Total[iy[[2 ;; 8]]] * iy
```

```
Total[inyorm[[2 ;; 8]]]
```

```
{0.967778, 0.0194641, 0.00985479, 0.00143238,  
0.0011147, 0.000327756, 0.0000274821, 8.17639 × 10-7,  
0.96453, 0.000591681, 8.25338 × 10-112, -2.09891 × 10-138}
```

```
{30.0346, 0.604063, 0.30584, 0.0444532, 0.0345943, 0.0101718, 0.000852896,  
0.0000253751, 29.9338, 0.0183626, 2.5614 × 10-110, -6.51388 × 10-137}
```

```
1.
```

```
plotiy = Partition[Riffle[normOleg80, inyorm[[2 ;; 8]]], 2]
```

```
{{0.604006, 0.604063}, {0.287434, 0.30584},  
{0.0722227, 0.0444532}, {0.0271552, 0.0345943},  
{0.00918191, 0.0101718}, {0., 0.000852896}, {0., 0.0000253751}}
```

```
BarChart[plotiy, PlotRange → {-0.1, 0.9},
  ChartLabels → {Placed[{"N +", "N 2+", "N 3+", "N 4+", "N 5+", "N 6+", "N 7+"}, Below],
    Placed[{}, Above]},
  ChartLegends → Placed[{"Expt.", "γfrag"}, Top],
  ChartStyle → {Black, Red}, AxesLabel → {"", "Ỹ(ω)",
  AxesStyle → {{Arrowheads[Automatic], AbsoluteThickness[0.6]},
    {Arrowheads[Automatic], AbsoluteThickness[0.6]}},
  LabelStyle → {FontFamily → "Arial"},
  PlotLabel → {damp, optGaFra / gammaFrag,
    (iynorm[2 ;; 8] - normOleg80).Table[i, {i, 1, 7}]]]
```

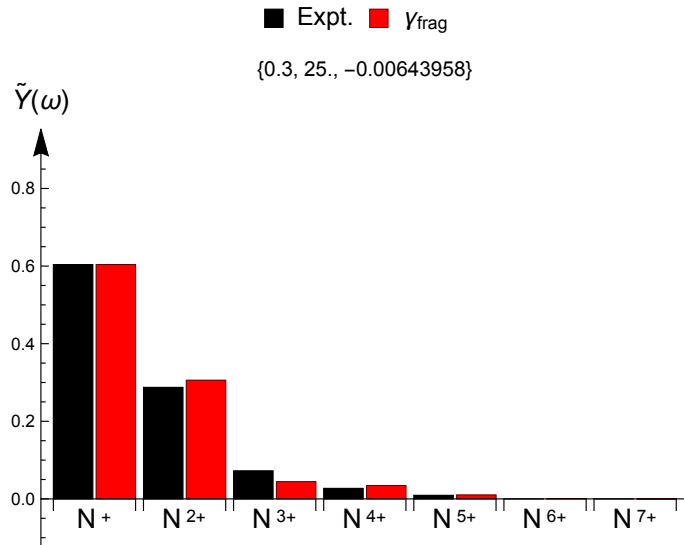

### 0.31

```
damp := 0.31
```

```
tabgamma =
  Table[{gaFra, normfitconsts[damp, gaFra * gammaFrag]}, {gaFra, 15, 35, 1 / 2}];
```

```
ListPlot[tabgamma, Joined -> True,
  PlotMarkers -> Automatic, PlotStyle -> {Thick, Red}]
```

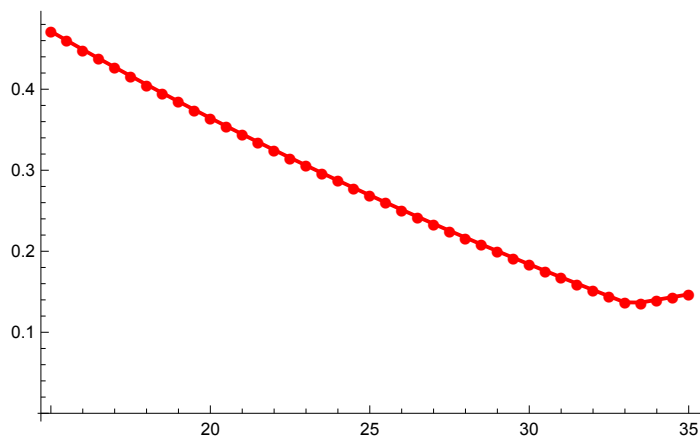

```
tabgamma =
  Table[{gaFra, normfitconsts[damp, gaFra * gammaFrag]}, {gaFra, 32, 34, 1 / 5}];
```

```
ListPlot[tabgamma, Joined -> True,
PlotMarkers -> Automatic, PlotStyle -> {Thick, Red}]
```

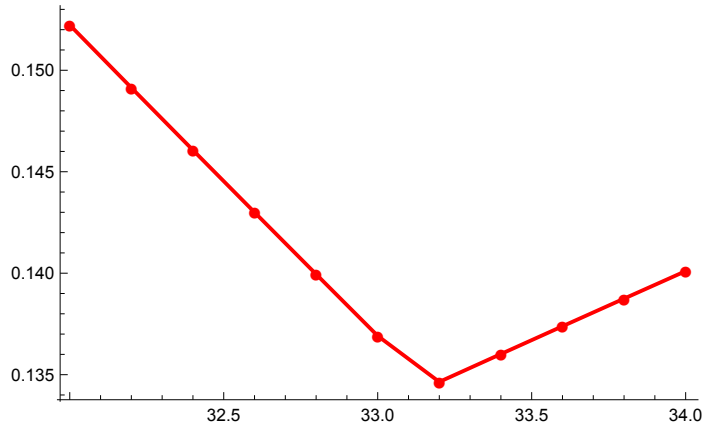

```
N[MinimalBy[tabgamma, Last]]
```

```
{{33.2, 0.134645}}
```

```
intgamma = Interpolation[tabgamma, x]
```

```
InterpolatingFunction[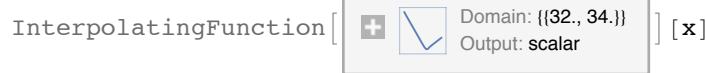 Domain: {{32., 34.}}  
Output: scalar] [x]
```

```
mingamma = FindMinimum[intgamma, {x, 32, 34}]
```

```
InterpolatingFunction::dmval:
```

Input value {34.2642} lies outside the range of data in the interpolating function. Extrapolation will be used. >>

```
{0.134645, {x -> 33.2}}
```

```
optent = x /. mingamma[[2]]
```

```
33.2
```

```
optGaFra := optent * gammaFrag
```

```
iy = dsionyieldcrateranalysisparam[damp * 0.26 * MilliJouleToHartree, photonenergy,  
tauX, nintdata, True, True, 1 / 1000, optfNppN, 1 - optfNppN, optGaFra]
```

```
inyorm = 1 / Total[iy[[2 ;; 8]]] * iy
```

```
Total[inyorm[[2 ;; 8]]]
```

```
{0.967045, 0.019906, 0.00976535, 0.0016852, 0.00118278, 0.000381647, 0.0000333601,  
1.05235 × 10-6, 0.963722, 0.000598795, -2.31576 × 10-133, 3.12151 × 10-143}
```

```
{29.3441, 0.604029, 0.29632, 0.0511357, 0.0358905, 0.0115807, 0.00101228,  
0.0000319327, 29.2432, 0.0181699, -7.02697 × 10-132, 9.47193 × 10-142}
```

```
1.
```

```
plotiy = Partition[Riffle[normOleg80, inyorm[[2 ;; 8]]], 2]
```

```
{{0.604006, 0.604029}, {0.287434, 0.29632},  
{0.0722227, 0.0511357}, {0.0271552, 0.0358905},  
{0.00918191, 0.0115807}, {0., 0.00101228}, {0., 0.0000319327}}
```

```
BarChart[plotiy, PlotRange → {-0.1, 0.9},
  ChartLabels → {Placed[{"N +", "N 2+", "N 3+", "N 4+", "N 5+", "N 6+", "N 7+"}, Below],
    Placed[{}, Above]},
  ChartLegends → Placed[{"Expt.", "γfrag"}, Top],
  ChartStyle → {Black, Red}, AxesLabel → {"", "Ỹ(ω)",
  AxesStyle → {{Arrowheads[Automatic], AbsoluteThickness[0.6]},
    {Arrowheads[Automatic], AbsoluteThickness[0.6]}},
  LabelStyle → {FontFamily → "Arial"},
  PlotLabel → {damp, optGaFra / gammaFrag,
    (iynorm[[2 ;; 8]] - normOleg80).Table[i, {i, 1, 7}]]]
```

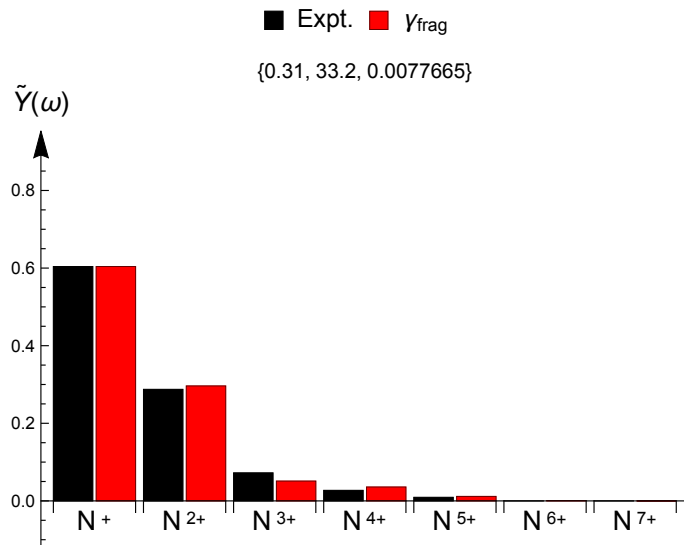

## 0.32

damp := 0.32

```
tabgamma =
  Table[{gaFra, normfitconsts[damp, gaFra * gammaFrag]}, {gaFra, 35, 55, 1 / 2}];
ListPlot[tabgamma, Joined -> True,
  PlotMarkers -> Automatic, PlotStyle -> {Thick, Red}]
```

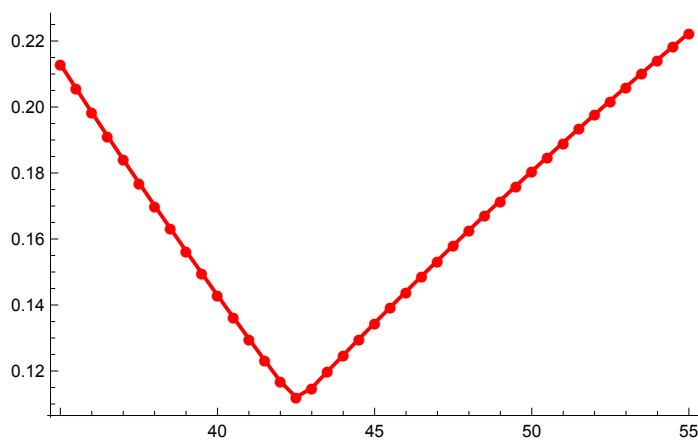

```
tabgamma = Table[
  {gaFra, normfitconsts[damp, gaFra * gammaFrag]}, {gaFra, 41.5, 43.5, 1 / 5}];
```

```
ListPlot[tabgamma, Joined -> True,
PlotMarkers -> Automatic, PlotStyle -> {Thick, Red}]
```

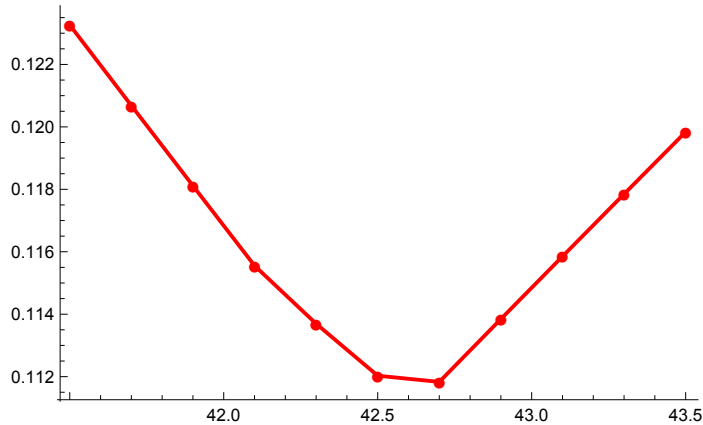

```
N[MinimalBy[tabgamma, Last]]
```

```
{{42.7, 0.111832}}
```

```
intgamma = Interpolation[tabgamma, x]
```

```
InterpolatingFunction[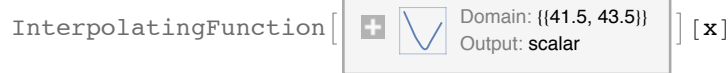 Domain: {{41.5, 43.5}}  
Output: scalar][x]
```

```
mingamma = FindMinimum[intgamma, {x, 41.5, 43.5}]
```

```
InterpolatingFunction::dmval:
```

```
Input value {43.7642} lies outside the range of data in the interpolating function. Extrapolation will be used. >>
```

```
{0.111687, {x -> 42.6242}}
```

```
optent = x /. mingamma[[2]]
```

```
42.6242
```

```
optGaFra := optent * gammaFrag
```

```
iy = dsionyieldcrateranalysisparam[damp * 0.26 * MilliJouleToHartree, photonenergy,  
tauX, nintdata, True, True, 1 / 1000, optfNppN, 1 - optfNppN, optGaFra]
```

```
inyorm = 1 / Total[iy[[2 ;; 8]]] * iy
```

```
Total[inyorm[[2 ;; 8]]]
```

```
{0.966326, 0.0203392, 0.00966125, 0.00194369, 0.00124848, 0.000439733,  
0.0000400308, 1.33389 × 10-6, 0.962931, 0.00060551, 1.80375 × 10-52, -3.60031 × 10-96}
```

```
{28.6967, 0.604008, 0.286908, 0.0577212, 0.0370757, 0.0130586, 0.00118879,  
0.0000396121, 28.5959, 0.0179817, 5.35655 × 10-51, -1.06917 × 10-94}
```

```
1.
```

```
plotiy = Partition[Riffle[normOleg80, inyorm[[2 ;; 8]]], 2]
```

```
{{0.604006, 0.604008}, {0.287434, 0.286908},  
{0.0722227, 0.0577212}, {0.0271552, 0.0370757},  
{0.00918191, 0.0130586}, {0., 0.00118879}, {0., 0.0000396121}}
```

```
BarChart[plotiy, PlotRange → {-0.1, 0.9},
  ChartLabels → {Placed[{"N +", "N 2+", "N 3+", "N 4+", "N 5+", "N 6+", "N 7+"}, Below],
    Placed[{}, Above]},
  ChartLegends → Placed[{"Expt.", "γfrag"}, Top],
  ChartStyle → {Black, Red}, AxesLabel → {"", "Ỹ(ω)"},
  AxesStyle → {{Arrowheads[Automatic], AbsoluteThickness[0.6]},
    {Arrowheads[Automatic], AbsoluteThickness[0.6]}},
  LabelStyle → {FontFamily → "Arial"},
  PlotLabel → {damp, optGaFra / gammaFrag,
    (iynorm[[2 ;; 8]] - normOleg80).Table[i, {i, 1, 7}]]}
```

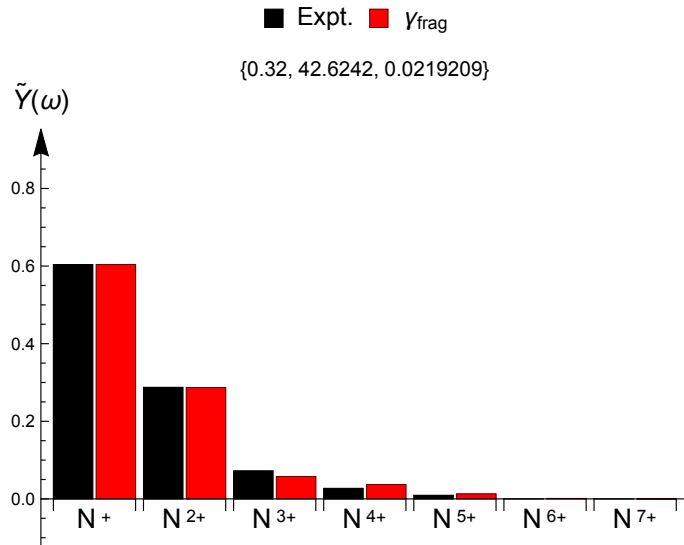

## Pulse energy for a 280 fs pulse with 280 fs fragmentation rate

```
tauX := shtdur280 * 280 / t0ToFemtoSecond
optent := 10.506791
optGaFra := optent * gammaFrag
```

### 0.38

```
damp := 0.38
```

```
iy = dsionyieldcrateranalysisparam[damp * 0.26 * MilliJouleToHartree, photonenergy,
  tauX, nintdata, True, True, 1 / 1000, optfNppN, 1 - optfNppN, optGaFra]
```

```
iynorm = 1 / Total[iy[[2 ;; 8]]] * iy
```

```
Total[iynorm[[2 ;; 8]]]
```

```
{0.962076, 0.021482, 0.0115483, 0.00204007, 0.00201987, 0.000736734, 0.0000927799,
  4.78928 × 10-6, 0.958498, 0.000638571, 4.24414 × 10-48, 1.41791 × 10-94}
```

```
{25.3682, 0.56644, 0.304508, 0.0537928, 0.0532602, 0.0194263,
  0.00244644, 0.000126284, 25.2739, 0.016838, 1.1191 × 10-46, 3.73877 × 10-93}
```

```
1.
```

```

plotiy = Partition[Riffle[normOleg280, iynorm[[2 ;; 8]]], 2]
{{0.56634, 0.56644}, {0.291805, 0.304508},
 {0.0763903, 0.0537928}, {0.0364504, 0.0532602},
 {0.027387, 0.0194263}, {0.00162698, 0.00244644}, {0., 0.000126284}}

BarChart[plotiy, PlotRange → {-0.1, 0.9},
 ChartLabels → {Placed[{"N +", "N 2+", "N 3+", "N 4+", "N 5+", "N 6+", "N 7+"}, Below],
   Placed[{}, Above]},
 ChartLegends → Placed[{"Expt.", "γfrag"}, Top],
 ChartStyle → {Black, Red}, AxesLabel → {"", "Ỹ(ω)"},
 AxesStyle → {{Arrowheads[Automatic], AbsoluteThickness[0.6]},
   {Arrowheads[Automatic], AbsoluteThickness[0.6]}},
 LabelStyle → {FontFamily → "Arial"},
 PlotLabel → {damp, optGaFra / gammaFrag,
   (iynorm[[2 ;; 8]] - normOleg280).Table[i, {i, 1, 7}]}]

```

■ Expt. ■ γ<sub>frag</sub>

{0.38, 10.5068, -0.00905058}

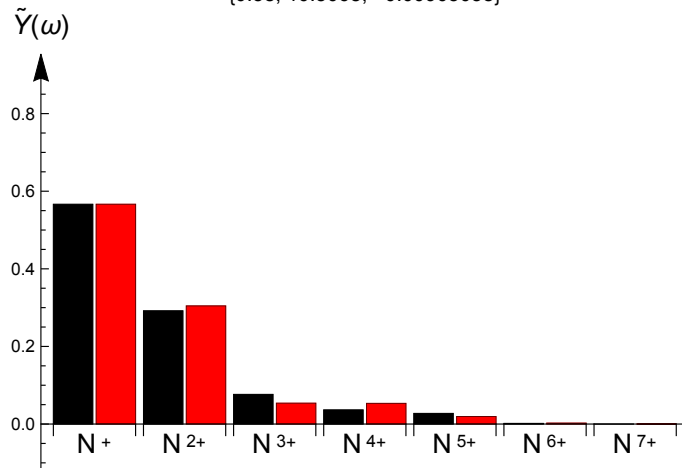

## Pulse energy for a 280 fs pulse with 80 fs fragmentation rate

```

tauX := shtdur280 * 280 / t0ToFemtoSecond
optent := 25.000000
optGaFra := optent * gammaFrag

```

0.36

```
damp := 0.36
```



```

iy = dsionyieldcrateranalysisparam[damp * 0.26 * MilliJouleToHartree, photonenergy,
  tauX, nintdata, True, True, 1 / 1000, optfNppN, 1 - optfNppN, optGaFra]
iynorm = 1 / Total[iy[[2 ;; 8]]] * iy
Total[iynorm[[2 ;; 8]]]

{0.963576, 0.021886, 0.00918877, 0.00280319, 0.00166601, 0.000777788,
  0.0000963414, 5.44183 × 10-6, 0.959918, 0.0006288, 4.17241 × 10-111, 5.33844 × 10-136}

{26.4548, 0.600875, 0.252275, 0.0769609, 0.0457399, 0.021354, 0.00264503,
  0.000149404, 26.3543, 0.0172635, 1.14553 × 10-109, 1.46566 × 10-134}

1.

```

```

plotiy = Partition[Riffle[normOleg280, iynorm[[2 ;; 8]]], 2]
{{0.56634, 0.600875}, {0.291805, 0.252275},
 {0.0763903, 0.0769609}, {0.0364504, 0.0457399},
 {0.027387, 0.021354}, {0.00162698, 0.00264503}, {0., 0.000149404}}

BarChart[plotiy, PlotRange → {-0.1, 0.9},
  ChartLabels → {Placed[{"N +", "N 2+", "N 3+", "N 4+", "N 5+", "N 6+", "N 7+"}, Below],
    Placed[{}, Above]},
  ChartLegends → Placed[{"Expt.", "γfrag"}, Top],
  ChartStyle → {Black, Red}, AxesLabel → {"", "Ỹ(ω)"},
  AxesStyle → {{Arrowheads[Automatic], AbsoluteThickness[0.6]},
    {Arrowheads[Automatic], AbsoluteThickness[0.6]}},
  LabelStyle → {FontFamily → "Arial"},
  PlotLabel → {damp, optGaFra / gammaFrag,
    (iynorm[[2 ;; 8]] - normOleg280).Table[i, {i, 1, 7}]}]

```

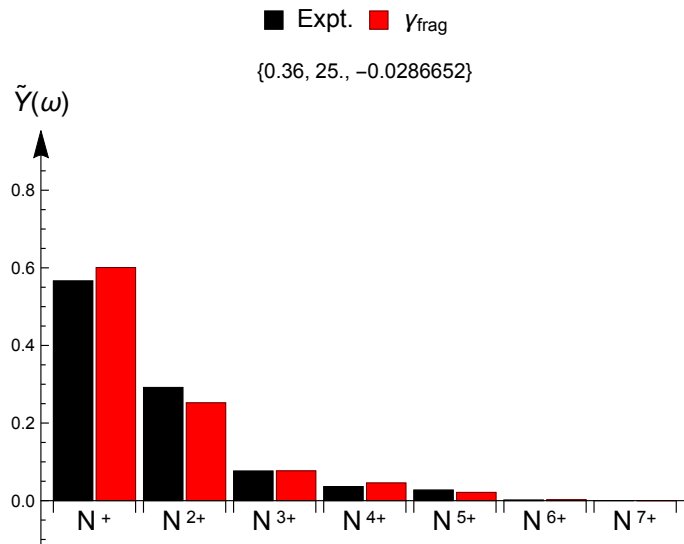

### 0.37

damp := 0.37

```

iy = dsionyieldcrateranalysisparam[damp * 0.26 * MilliJouleToHartree, photonenergy,
  tauX, nintdata, True, True, 1 / 1000, optfNppN, 1 - optfNppN, optGaFra]
iynorm = 1 / Total[iy[[2 ;; 8]]] * iy
Total[iynorm[[2 ;; 8]]]

{0.962897, 0.0221149, 0.00939234, 0.00290129, 0.00175027, 0.000832321, 0.00010608,
  6.14933 × 10-6, 0.959202, 0.000633827, 1.36102 × 10-11, 5.29084 × 10-138}

{25.9518, 0.596035, 0.25314, 0.0781949, 0.0471728, 0.0224325, 0.00285903,
  0.000165735, 25.8522, 0.0170828, 3.6682 × 10-110, 1.42597 × 10-136}

1.

```

```

plotiy = Partition[Riffle[normOleg280, iynorm[[2 ;; 8]]], 2]
{{0.56634, 0.596035}, {0.291805, 0.25314},
 {0.0763903, 0.0781949}, {0.0364504, 0.0471728},
 {0.027387, 0.0224325}, {0.00162698, 0.00285903}, {0., 0.000165735}}

BarChart[plotiy, PlotRange → {-0.1, 0.9},
  ChartLabels → {Placed[{"N +", "N 2+", "N 3+", "N 4+", "N 5+", "N 6+", "N 7+"}, Below],
    Placed[{}, Above]},
  ChartLegends → Placed[{"Expt.", "γfrag"}, Top],
  ChartStyle → {Black, Red}, AxesLabel → {"", "Ỹ(ω)"},
  AxesStyle → {{Arrowheads[Automatic], AbsoluteThickness[0.6]},
    {Arrowheads[Automatic], AbsoluteThickness[0.6]}},
  LabelStyle → {FontFamily → "Arial"},
  PlotLabel → {damp, optGaFra / gammaFrag,
    (iynorm[[2 ;; 8]] - normOleg280).Table[i, {i, 1, 7}]]}

```

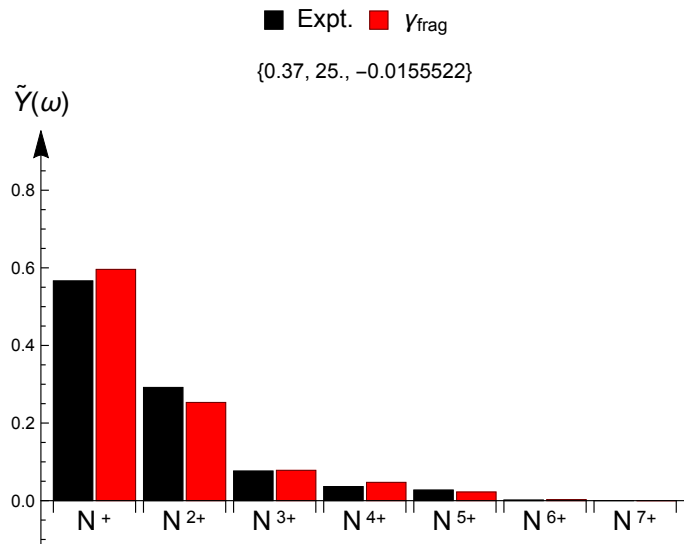

0.38

damp := 0.38

```

iy = dsionyieldcrateranalysisparam[damp * 0.26 * MilliJouleToHartree, photonenergy,
  tauX, nintdata, True, True, 1 / 1000, optfNppN, 1 - optfNppN, optGaFra]
iynorm = 1 / Total[iy[[2 ;; 8]]] * iy
Total[iynorm[[2 ;; 8]]]

{0.962229, 0.0223336, 0.00959147, 0.00299867, 0.00183546, 0.000888663,
  0.000116454,  $6.92336 \times 10^{-6}$ , 0.958498, 0.000638571,  $1.44062 \times 10^{-11}$ ,  $1.60767 \times 10^{-133}$ }

{25.4752, 0.591286, 0.253936, 0.0793903, 0.0485942, 0.0235275, 0.00308315,
  0.000183297, 25.3764, 0.0169063,  $3.81407 \times 10^{-110}$ ,  $4.25632 \times 10^{-132}$ }

1.

```

```

plotiy = Partition[Riffle[normOleg280, iynorm[[2 ;; 8]]], 2]
{{0.56634, 0.591286}, {0.291805, 0.253936},
 {0.0763903, 0.0793903}, {0.0364504, 0.0485942},
 {0.027387, 0.0235275}, {0.00162698, 0.00308315}, {0., 0.000183297}}

BarChart[plotiy, PlotRange → {-0.1, 0.9},
  ChartLabels → {Placed[{"N +", "N 2+", "N 3+", "N 4+", "N 5+", "N 6+", "N 7+"}, Below],
    Placed[{}, Above]},
  ChartLegends → Placed[{"Expt.", "Yfrag"}, Top],
  ChartStyle → {Black, Red}, AxesLabel → {"", "Ỹ(ω)"},
  AxesStyle → {{Arrowheads[Automatic], AbsoluteThickness[0.6]},
    {Arrowheads[Automatic], AbsoluteThickness[0.6]}},
  LabelStyle → {FontFamily → "Arial"},
  PlotLabel → {damp, optGaFra / gammaFrag,
    (iynorm[[2 ;; 8]] - normOleg280).Table[i, {i, 1, 7}]]}

■ Expt. ■ Yfrag
{0.38, 25., -0.00249499}

```

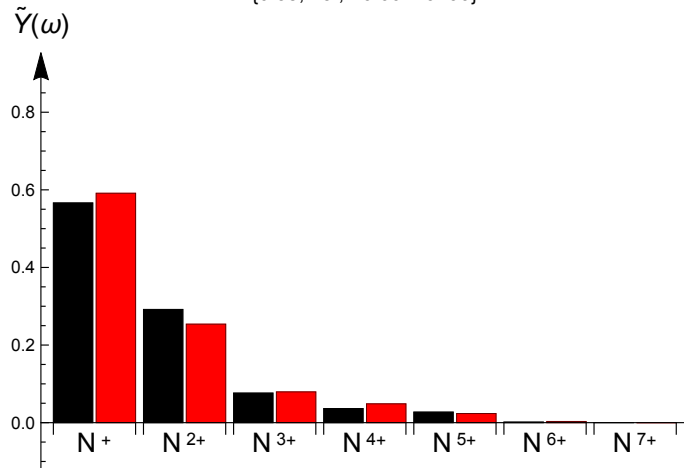

0.39

damp := 0.39

```

iy = dsionyieldcrateranalysisparam[damp * 0.26 * MilliJouleToHartree, photonenergy,
  tauX, nintdata, True, True, 1 / 1000, optfNppN, 1 - optfNppN, optGaFra]
iynorm = 1 / Total[iy[[2 ;; 8]]] * iy
Total[iynorm[[2 ;; 8]]]

{0.961572, 0.0225426, 0.0097862, 0.00309526, 0.0019215, 0.000946786, 0.000127483,
  7.76775 × 10-6, 0.957808, 0.000643049, 1.46088 × 10-111, -1.99593 × 10-135}

{25.023, 0.586625, 0.254666, 0.080548, 0.0500032, 0.0246382, 0.00331749,
  0.00020214, 24.925, 0.0167341, 3.80165 × 10-110, -5.19402 × 10-134}

1.

```

```

plotiy = Partition[Riffle[normOleg280, iynorm[[2 ;; 8]]], 2]
{{0.56634, 0.586625}, {0.291805, 0.254666},
 {0.0763903, 0.080548}, {0.0364504, 0.0500032},
 {0.027387, 0.0246382}, {0.00162698, 0.00331749}, {0., 0.00020214}}

BarChart[plotiy, PlotRange → {-0.1, 0.9},
  ChartLabels → {Placed[{"N +", "N 2+", "N 3+", "N 4+", "N 5+", "N 6+", "N 7+"}, Below],
    Placed[{}, Above]},
  ChartLegends → Placed[{"Expt.", "γfrag"}, Top],
  ChartStyle → {Black, Red}, AxesLabel → {"", "Ỹ(ω)"},
  AxesStyle → {{Arrowheads[Automatic], AbsoluteThickness[0.6]},
    {Arrowheads[Automatic], AbsoluteThickness[0.6]}},
  LabelStyle → {FontFamily → "Arial"},
  PlotLabel → {damp, optGaFra / gammaFrag,
    (iynorm[[2 ;; 8]] - normOleg280).Table[i, {i, 1, 7}]}]

```

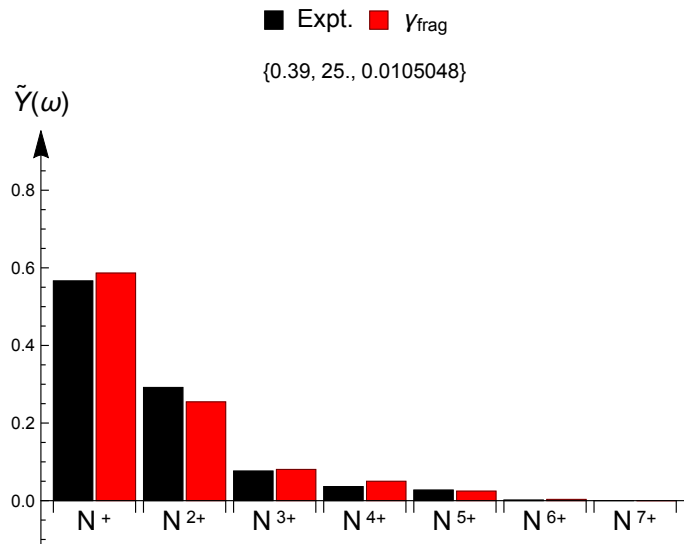

0.40

damp := 0.40

```

iy = dsionyieldcrateranalysisparam[damp * 0.26 * MilliJouleToHartree, photonenergy,
  tauX, nintdata, True, True, 1 / 1000, optfNppN, 1 - optfNppN, optGaFra]
iynorm = 1 / Total[iy[[2 ;; 8]]] * iy
Total[iynorm[[2 ;; 8]]]

```

```

{0.960927, 0.0227423, 0.00997654, 0.00319101, 0.0020083, 0.00100666, 0.000139182,
  8.68639 × 10-6, 0.957131, 0.000647276, 1.43037 × 10-11, -5.34218 × 10-132}

```

```

{24.5933, 0.582051, 0.255333, 0.0816686, 0.051399, 0.0257637, 0.00356213,
  0.000222314, 24.4962, 0.0165659, 3.66079 × 10-110, -1.36724 × 10-130}

```

1.

```

plotiy = Partition[Riffle[normOleg280, iynorm[[2 ;; 8]]], 2]
{{0.56634, 0.582051}, {0.291805, 0.255333},
 {0.0763903, 0.0816686}, {0.0364504, 0.051399},
 {0.027387, 0.0257637}, {0.00162698, 0.00356213}, {0., 0.000222314}}

```

```

BarChart[plotiy, PlotRange → {-0.1, 0.9},
  ChartLabels → {Placed[{"N+", "N2+", "N3+", "N4+", "N5+", "N6+", "N7+"}, Below],
    Placed[{}, Above]},
  ChartLegends → Placed[{"Expt.", "γfrag"}, Top],
  ChartStyle → {Black, Red}, AxesLabel → {"", "Ỹ(ω)"},
  AxesStyle → {{Arrowheads[Automatic], AbsoluteThickness[0.6]},
    {Arrowheads[Automatic], AbsoluteThickness[0.6]}},
  LabelStyle → {FontFamily → "Arial"},
  PlotLabel → {damp, optGaFra / gammaFrag,
    (iynorm[[2 ;; 8]] - normOleg280).Table[i, {i, 1, 7}]}]

```

■ Expt. ■ γ<sub>frag</sub>

{0.4, 25., 0.0234468}

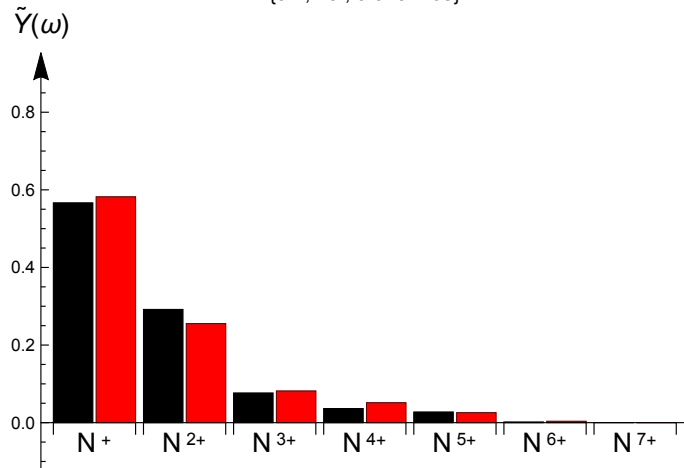

## Pulse energy for a 80 fs pulse with 280 fs fragmentation rate

```

tauX := shtdur80 * 80 / t0ToFemtoSecond
optent := 10.506791
optGaFra := optent * gammaFrag

```

## 0.28

```
damp := 0.28
```

```
iy = dsionyieldcrateranalysisparam[damp * 0.26 * MilliJouleToHartree, photonenergy,  
tauX, nintdata, True, True, 1 / 1000, optfNppN, 1 - optfNppN, optGaFra]
```

```
inyorm = 1 / Total[iy[[2 ;; 8]]] * iy
```

```
Total[iyorm[[2 ;; 8]]]
```

```
{0.969287, 0.0185311, 0.0100373, 0.000922805,  
0.000973343, 0.000229845, 0.0000176582, 4.57184 × 10-7,  
0.966197, 0.000576154, 2.87662 × 10-48, -7.41581 × 10-138}
```

```
{31.56, 0.603372, 0.326816, 0.0300465, 0.031692, 0.00748375, 0.000574951,  
0.0000148859, 31.4594, 0.0187596, 9.36627 × 10-47, -2.41459 × 10-136}
```

```
1.
```

```
plotiy = Partition[Riffle[normOleg80, inyorm[[2 ;; 8]]], 2]
```

```
{{0.604006, 0.603372}, {0.287434, 0.326816},  
{0.0722227, 0.0300465}, {0.0271552, 0.031692},  
{0.00918191, 0.00748375}, {0., 0.000574951}, {0., 0.0000148859}}
```

```
BarChart[plotiy, PlotRange → {-0.1, 0.9},  
ChartLabels → {Placed[{"N +", "N 2+", "N 3+", "N 4+", "N 5+", "N 6+", "N 7+"}, Below],  
Placed[{}, Above]},  
ChartLegends → Placed[{"Expt.", "γfrag"}, Top],  
ChartStyle → {Black, Red}, AxesLabel → {"", "Ỹ(ω)"},  
AxesStyle → {{Arrowheads[Automatic], AbsoluteThickness[0.6]},  
{Arrowheads[Automatic], AbsoluteThickness[0.6]}},  
LabelStyle → {FontFamily → "Arial"},  
PlotLabel → {damp, optGaFra / gammaFrag,  
(inyorm[[2 ;; 8]] - normOleg80).Table[i, {i, 1, 7}]]}
```

■ Expt. ■ γ<sub>frag</sub>

{0.28, 10.5068, -0.0351887}

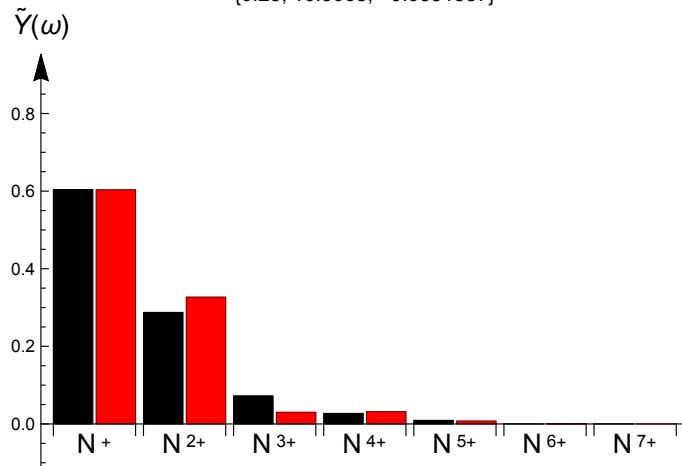

## 0.29

```
damp := 0.29
```

```
iy = dsionyieldcrateranalysisparam[damp * 0.26 * MilliJouleToHartree, photonenergy,
  tauX, nintdata, True, True, 1 / 1000, optfNppN, 1 - optfNppN, optGaFra]
iynorm = 1 / Total[iy[[2 ;; 8]]] * iy
Total[iynorm[[2 ;; 8]]]
```

```
{0.968491, 0.0188139, 0.0103868, 0.000982261,
  0.00104965, 0.000255662, 0.0000203938, 5.46595 × 10-7,
  0.965355, 0.000584142, 2.92929 × 10-48, -1.53124 × 10-137}
```

```
{30.7367, 0.597092, 0.329643, 0.0311737, 0.0333125, 0.00811389, 0.000647232,
  0.0000173471, 30.6372, 0.0185387, 9.2966 × 10-47, -4.85966 × 10-136}
```

1.

```
plotiy = Partition[Riffle[normOleg80, iynorm[[2 ;; 8]]], 2]
```

```
{{0.604006, 0.597092}, {0.287434, 0.329643},
  {0.0722227, 0.0311737}, {0.0271552, 0.0333125},
  {0.00918191, 0.00811389}, {0., 0.000647232}, {0., 0.0000173471}}
```

```
BarChart[plotiy, PlotRange → {-0.1, 0.9},
  ChartLabels → {Placed[{"N +", "N 2+", "N 3+", "N 4+", "N 5+", "N 6+", "N 7+"}, Below],
    Placed[{}, Above]},
  ChartLegends → Placed[{"Expt.", "γfrag"}, Top],
  ChartStyle → {Black, Red}, AxesLabel → {"", "Ỹ(ω)"},
  AxesStyle → {{Arrowheads[Automatic], AbsoluteThickness[0.6]},
    {Arrowheads[Automatic], AbsoluteThickness[0.6]}},
  LabelStyle → {FontFamily → "Arial"},
  PlotLabel → {damp, optGaFra / gammaFrag,
    (iynorm[[2 ;; 8]] - normOleg80).Table[i, {i, 1, 7}]]}
```

■ Expt. ■ γ<sub>frag</sub>

{0.29, 10.5068, -0.0223488}

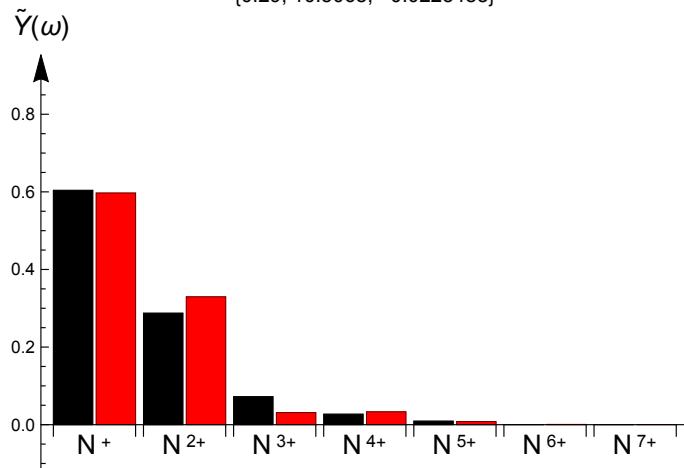

### 0.30

damp := 0.30

```

iy = dsionyieldcrateranalysisparam[damp * 0.26 * MilliJouleToHartree, photonenergy,
  tauX, nintdata, True, True, 1 / 1000, optfNppN, 1 - optfNppN, optGaFra]
iynorm = 1 / Total[iy[[2 ;; 8]]] * iy
Total[iynorm[[2 ;; 8]]]

{0.967709, 0.0190825, 0.0107303, 0.00104269, 0.00112818, 0.000283166,
  0.0000234248,  $6.49217 \times 10^{-7}$ , 0.96453, 0.000591681,  $2.96579 \times 10^{-48}$ ,  $3.67816 \times 10^{-116}$ }

{29.9685, 0.590955, 0.332302, 0.0322904, 0.0349381, 0.00876922,
  0.00072543, 0.0000201052, 29.87, 0.0183235,  $9.18461 \times 10^{-47}$ ,  $1.13907 \times 10^{-114}$ }

1.

```

```

plotiy = Partition[Riffle[normOleg80, iynorm[[2 ;; 8]]], 2]
{{0.604006, 0.590955}, {0.287434, 0.332302},
 {0.0722227, 0.0322904}, {0.0271552, 0.0349381},
 {0.00918191, 0.00876922}, {0., 0.00072543}, {0., 0.0000201052}}

BarChart[plotiy, PlotRange → {-0.1, 0.9},
  ChartLabels → {Placed[{"N +", "N 2+", "N 3+", "N 4+", "N 5+", "N 6+", "N 7+"}, Below],
    Placed[{}, Above]},
  ChartLegends → Placed[{"Expt.", "γfrag"}, Top],
  ChartStyle → {Black, Red}, AxesLabel → {"", "Ỹ(ω)"},
  AxesStyle → {{Arrowheads[Automatic], AbsoluteThickness[0.6]},
    {Arrowheads[Automatic], AbsoluteThickness[0.6]}},
  LabelStyle → {FontFamily → "Arial"},
  PlotLabel → {damp, optGaFra / gammaFrag,
    (iynorm[[2 ;; 8]] - normOleg80).Table[i, {i, 1, 7}]]}

```

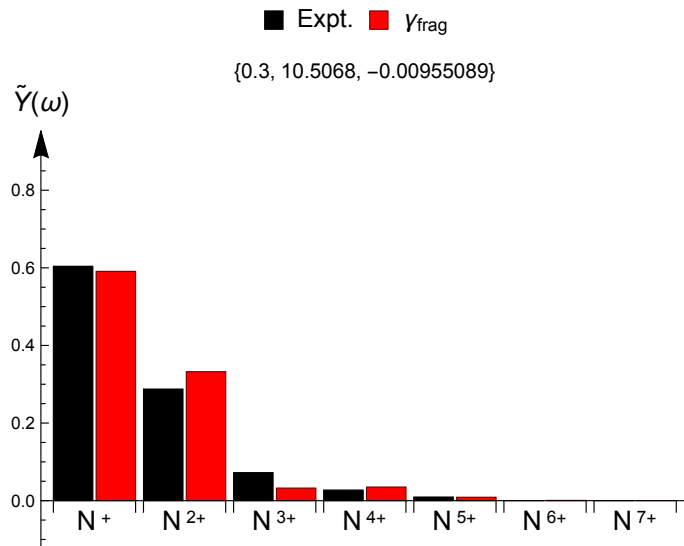

### 0.31

```
damp := 0.31
```



```

iy = dsionyieldcrateranalysisparam[damp * 0.26 * MilliJouleToHartree, photonenergy,
  tauX, nintdata, True, True, 1 / 1000, optfNppN, 1 - optfNppN, optGaFra]
iynorm = 1 / Total[iy[[2 ;; 8]]] * iy
Total[iynorm[[2 ;; 8]]]

{0.966942, 0.0193374, 0.0110678, 0.00110399, 0.00120882, 0.000312376, 0.000026769,
  7.66386 × 10-7, 0.963722, 0.000598796, 3.02407 × 10-48, -3.30203 × 10-113}}

{29.2499, 0.584956, 0.3348, 0.0333956, 0.0365668, 0.00944934, 0.00080976,
  0.0000231831, 29.1525, 0.0181135, 9.1478 × 10-47, -9.98861 × 10-112}}

1.

```

```

plotiy = Partition[Riffle[normOleg80, iynorm[[2 ;; 8]]], 2]
{{0.604006, 0.584956}, {0.287434, 0.3348},
 {0.0722227, 0.0333956}, {0.0271552, 0.0365668},
 {0.00918191, 0.00944934}, {0., 0.00080976}, {0., 0.0000231831}}

BarChart[plotiy, PlotRange → {-0.1, 0.9},
  ChartLabels → {Placed[{"N +", "N 2+", "N 3+", "N 4+", "N 5+", "N 6+", "N 7+"}, Below],
    Placed[{}, Above]},
  ChartLegends → Placed[{"Expt.", "γfrag"}, Top],
  ChartStyle → {Black, Red}, AxesLabel → {"", "Ỹ(ω)"},
  AxesStyle → {{Arrowheads[Automatic], AbsoluteThickness[0.6]},
    {Arrowheads[Automatic], AbsoluteThickness[0.6]}},
  LabelStyle → {FontFamily → "Arial"},
  PlotLabel → {damp, optGaFra / gammaFrag,
    (iynorm[[2 ;; 8]] - normOleg80).Table[i, {i, 1, 7}]]}

```

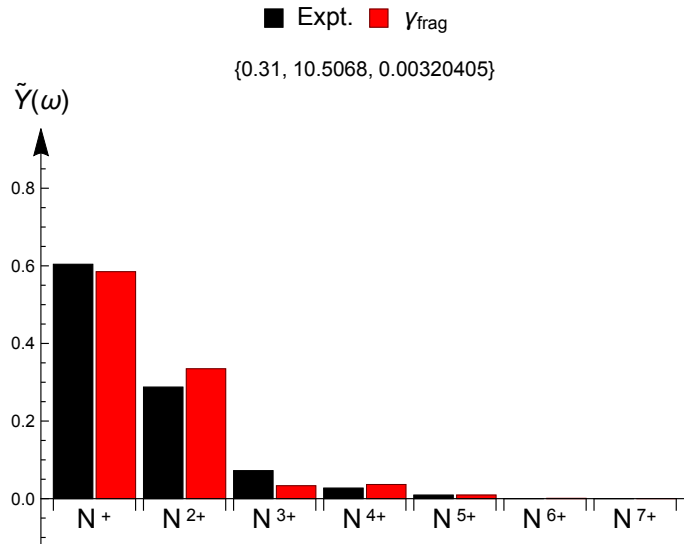

## 0.32

```
damp := 0.32
```

```

iy = dsionyieldcrateranalysisparam[damp * 0.26 * MilliJouleToHartree, photonenergy,
  tauX, nintdata, True, True, 1 / 1000, optfNppN, 1 - optfNppN, optGaFra]
iynorm = 1 / Total[iy[[2 ;; 8]]] * iy
Total[iynorm[[2 ;; 8]]]

{0.966189, 0.0195795, 0.011399, 0.00116609, 0.00129146, 0.000343308, 0.0000304443,
  8.9951 × 10-7, 0.962931, 0.00060551, 3.51537 × 10-48, -7.7947 × 10-112}

{28.5764, 0.579091, 0.337142, 0.0344887, 0.0381969, 0.0101538, 0.000900433,
  0.0000266043, 28.4801, 0.0179088, 1.03972 × 10-46, -2.30539 × 10-110}

1.

```

```

plotiy = Partition[Riffle[normOleg80, iynorm[[2 ;; 8]]], 2]
{{0.604006, 0.579091}, {0.287434, 0.337142},
 {0.0722227, 0.0344887}, {0.0271552, 0.0381969},
 {0.00918191, 0.0101538}, {0., 0.000900433}, {0., 0.0000266043}}

BarChart[plotiy, PlotRange → {-0.1, 0.9},
  ChartLabels → {Placed[{"N+", "N2+", "N3+", "N4+", "N5+", "N6+", "N7+"}, Below],
    Placed[{}, Above]},
  ChartLegends → Placed[{"Expt.", "γfrag"}, Top],
  ChartStyle → {Black, Red}, AxesLabel → {"", "Ỹ(ω)"},
  AxesStyle → {{Arrowheads[Automatic], AbsoluteThickness[0.6]},
    {Arrowheads[Automatic], AbsoluteThickness[0.6]}},
  LabelStyle → {FontFamily → "Arial"},
  PlotLabel → {damp, optGaFra / gammaFrag,
    (iynorm[[2 ;; 8]] - normOleg80).Table[i, {i, 1, 7}]]}

```

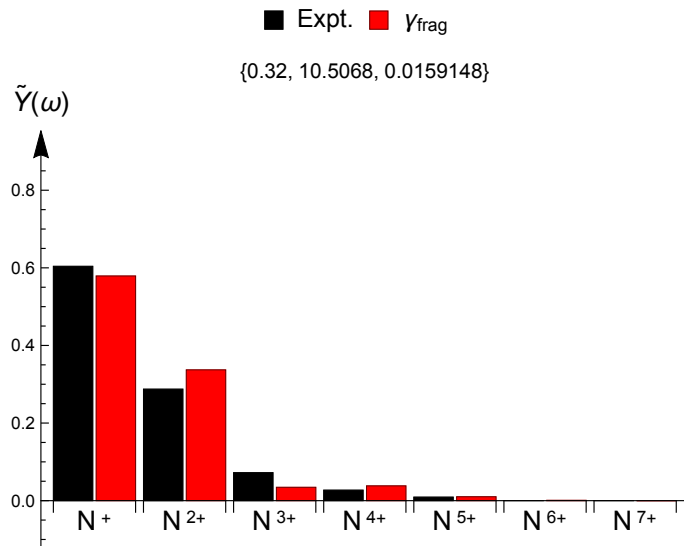

## Pulse energy for a 80 fs pulse with 80 fs fragmentation rate

```

tauX := shtdur80 * 80 / t0ToFemtoSecond
optent := 25.000000
optGaFra := optent * gammaFrag

```

## 0.30

```
damp := 0.30
```

```
iy = dsionyieldcrateranalysisparam[damp * 0.26 * MilliJouleToHartree, photonenergy,  
tauX, nintdata, True, True, 1 / 1000, optfNppN, 1 - optfNppN, optGaFra]
```

```
iynorm = 1 / Total[iy[[2 ;; 8]]] * iy
```

```
Total[iynorm[[2 ;; 8]]]
```

```
{0.967778, 0.0194641, 0.00985479, 0.00143238, 0.0011147, 0.000327756,  
0.0000274821, 8.17639 × 10-7, 0.96453, 0.000591681, 4.74752 × 10-66, 1.36502 × 10-103}
```

```
{30.0346, 0.604063, 0.30584, 0.0444532, 0.0345943, 0.0101718, 0.000852896,  
0.0000253751, 29.9338, 0.0183626, 1.47338 × 10-64, 4.2363 × 10-102}
```

```
1.
```

```
plotiy = Partition[Riffle[normOleg80, iynorm[[2 ;; 8]]], 2]
```

```
{{0.604006, 0.604063}, {0.287434, 0.30584},  
{0.0722227, 0.0444532}, {0.0271552, 0.0345943},  
{0.00918191, 0.0101718}, {0., 0.000852896}, {0., 0.0000253751}}
```

```
BarChart[plotiy, PlotRange → {-0.1, 0.9},  
ChartLabels → {Placed[{"N +", "N 2+", "N 3+", "N 4+", "N 5+", "N 6+", "N 7+"}, Below],  
Placed[{}, Above]},  
ChartLegends → Placed[{"Expt.", "γfrag"}, Top],  
ChartStyle → {Black, Red}, AxesLabel → {"", "Ỹ(ω)"},  
AxesStyle → {{Arrowheads[Automatic], AbsoluteThickness[0.6]},  
{Arrowheads[Automatic], AbsoluteThickness[0.6]}},  
LabelStyle → {FontFamily → "Arial"},  
PlotLabel → {damp, optGaFra / gammaFrag,  
(iynorm[[2 ;; 8]] - normOleg80).Table[i, {i, 1, 7}]}]
```

■ Expt. ■ γ<sub>frag</sub>  
{0.3, 25., -0.00643958}

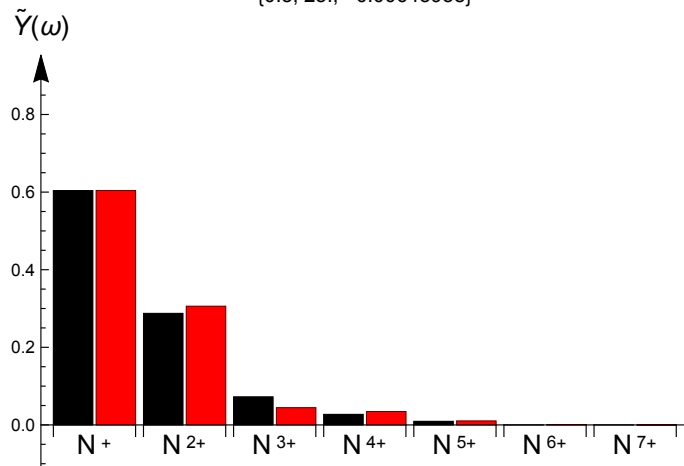

## Pulse energy for a 7 fs pulse with 280 fs fragmentation rate

```
tauX := shtdur7 * 7 / t0ToFemtoSecond
optent := 10.506791
optGaFra := optent * gammaFrag
```

### 0.12

```
damp := 0.12

iy = dsionyieldsanalysisparam[damp * 0.26 * MilliJouleToHartree, photonenergy,
    tauX, nintdata, True, True, 1 / 1000, optfNppN, 1 - optfNppN, optGaFra]
iynorm = 1 / Total[iy[[2 ;; 8]]] * iy
Total[iynorm[[2 ;; 8]]]
{0.984504, 0.0113425, 0.00396137, 0.000147958,
  0.0000397234,  $3.94399 \times 10^{-6}$ ,  $3.07841 \times 10^{-8}$ ,  $4.25786 \times 10^{-11}$ ,
   $0.982596$ ,  $0.000359602$ ,  $1.50994 \times 10^{-48}$ ,  $-1.59713 \times 10^{-214}$ }

{63.5347, 0.731986, 0.255646, 0.0095484, 0.00256354, 0.000254524,  $1.98664 \times 10^{-6}$ ,
   $2.7478 \times 10^{-9}$ , 63.4115, 0.0232068,  $9.74437 \times 10^{-47}$ ,  $-1.0307 \times 10^{-212}$ }

1.

plotiy = Partition[Riffle[normOleg7, iynorm[[2 ;; 8]]], 2]
{{0.694746, 0.731986}, {0.275684, 0.255646},
 {0.0293036, 0.0095484}, {0.000266625, 0.00256354},
 {0., 0.000254524}, {0.,  $1.98664 \times 10^{-6}$ }, {0.,  $2.7478 \times 10^{-9}$ }}
```

```
BarChart[plotiy, PlotRange → {-0.1, 0.9},
  ChartLabels → {Placed[{"N +", "N 2+", "N 3+", "N 4+", "N 5+", "N 6+", "N 7+"}, Below],
    Placed[{}, Above]},
  ChartLegends → Placed[{"Expt.", "γfrag"}, Top],
  ChartStyle → {Black, Red}, AxesLabel → {"", "Ỹ(ω)"},
  AxesStyle → {{Arrowheads[Automatic], AbsoluteThickness[0.6]},
    {Arrowheads[Automatic], AbsoluteThickness[0.6]}},
  LabelStyle → {FontFamily → "Arial"},
  PlotLabel → {damp, optGaFra / gammaFrag,
    (iynorm[[2 ;; 8]] - normOleg7).Table[i, {i, 1, 7}]]]
```

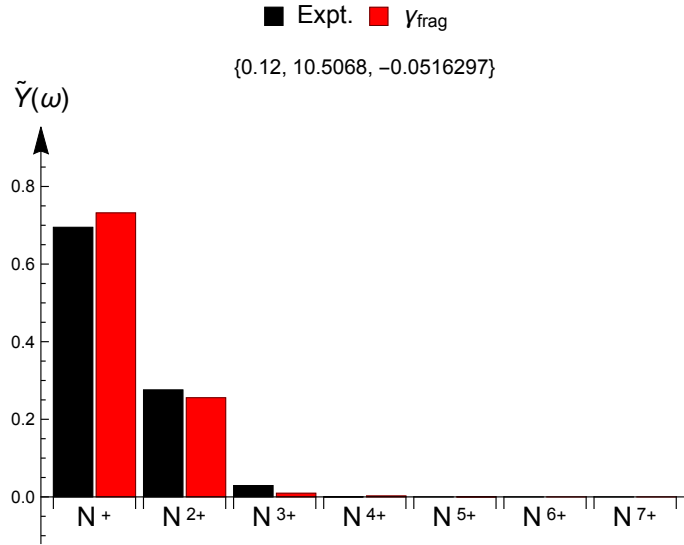

### 0.13

damp := 0.13

```
iy = dsionyieldcrateranalysisparam[damp * 0.26 * MilliJouleToHartree, photonenergy,
  tauX, nintdata, True, True, 1 / 1000, optfNppN, 1 - optfNppN, optGaFra]
```

```
iynorm = 1 / Total[iy[[2 ;; 8]]] * iy
```

```
Total[iynorm[[2 ;; 8]]]
```

```
{0.983397, 0.0120065, 0.00435924, 0.00018249,
  0.0000496508, 5.30461 × 10-6, 4.49862 × 10-8, 6.75073 × 10-11,
  0.981378, 0.000379768, 1.59549 × 10-48, -4.1903 × 10-206}
```

```
{59.2292, 0.723143, 0.262554, 0.0109912, 0.00299043, 0.000319493, 2.70948 × 10-6,
  4.06591 × 10-9, 59.1076, 0.0228731, 9.60952 × 10-47, -2.52378 × 10-204}
```

1.

```
plotiy = Partition[Riffle[normOleg7, iynorm[[2 ;; 8]]], 2]
```

```
{{0.694746, 0.723143}, {0.275684, 0.262554},
  {0.0293036, 0.0109912}, {0.000266625, 0.00299043},
  {0., 0.000319493}, {0., 2.70948 × 10-6}, {0., 4.06591 × 10-9}}
```

```
BarChart[plotiy, PlotRange → {-0.1, 0.9},
  ChartLabels → {Placed[{"N +", "N 2+", "N 3+", "N 4+", "N 5+", "N 6+", "N 7+"}, Below],
    Placed[{}, Above]},
  ChartLegends → Placed[{"Expt.", "γfrag"}, Top],
  ChartStyle → {Black, Red}, AxesLabel → {"", "Ỹ(ω)",
  AxesStyle → {{Arrowheads[Automatic], AbsoluteThickness[0.6]},
    {Arrowheads[Automatic], AbsoluteThickness[0.6]}},
  LabelStyle → {FontFamily → "Arial"},
  PlotLabel → {damp, optGaFra / gammaFrag,
    (iynorm[[2 ;; 8]] - normOleg7).Table[i, {i, 1, 7}]]]
```

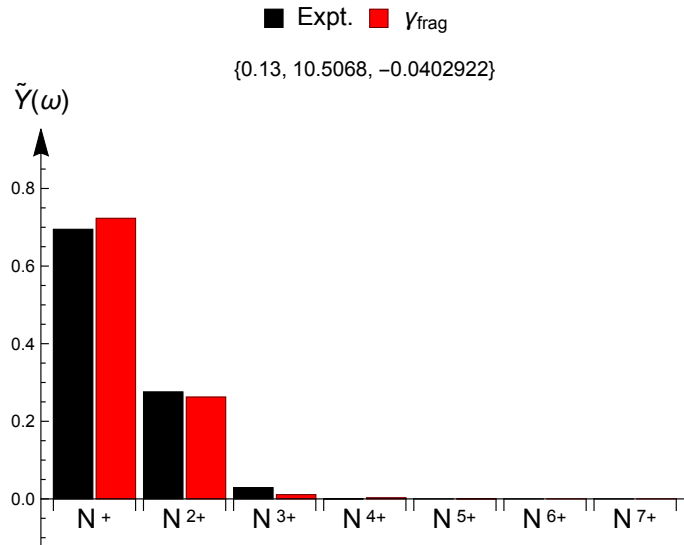

## 0.14

damp := 0.14

```
iy = dsionyieldcrateranalysisparam[damp * 0.26 * MilliJouleToHartree, photonenergy,
  tauX, nintdata, True, True, 1 / 1000, optfNppN, 1 - optfNppN, optGaFra]
```

```
iynorm = 1 / Total[iy[[2 ;; 8]]] * iy
```

```
Total[iynorm[[2 ;; 8]]]
```

```
{0.982313, 0.012637, 0.00476053, 0.000221156, 0.0000609671, 6.96883 × 10-6,
  6.38333 × 10-8, 1.03314 × 10-10, 0.98019, 0.0003988, 1.72753 × 10-48, 1.9907 × 10-189}
```

```
{55.5397, 0.714492, 0.269159, 0.0125041, 0.00344706, 0.000394016,
  3.60911 × 10-6, 5.84134 × 10-9, 55.4196, 0.022548, 9.7674 × 10-47, 1.12553 × 10-187}
```

1.

```
plotiy = Partition[Riffle[normOleg7, iynorm[[2 ;; 8]]], 2]
```

```
{{0.694746, 0.714492}, {0.275684, 0.269159},
  {0.0293036, 0.0125041}, {0.000266625, 0.00344706},
  {0., 0.000394016}, {0., 3.60911 × 10-6}, {0., 5.84134 × 10-9}}
```

```
BarChart[plotiy, PlotRange → {-0.1, 0.9},
  ChartLabels → {Placed[{"N +", "N 2+", "N 3+", "N 4+", "N 5+", "N 6+", "N 7+"}, Below],
    Placed[{}, Above]},
  ChartLegends → Placed[{"Expt.", "γfrag"}, Top],
  ChartStyle → {Black, Red}, AxesLabel → {"", "Ỹ(ω)"},
  AxesStyle → {{Arrowheads[Automatic], AbsoluteThickness[0.6]},
    {Arrowheads[Automatic], AbsoluteThickness[0.6]}},
  LabelStyle → {FontFamily → "Arial"},
  PlotLabel → {damp, optGaFra / gammaFrag,
    (iynorm[[2 ;; 8]] - normOleg7).Table[i, {i, 1, 7}]]]
```

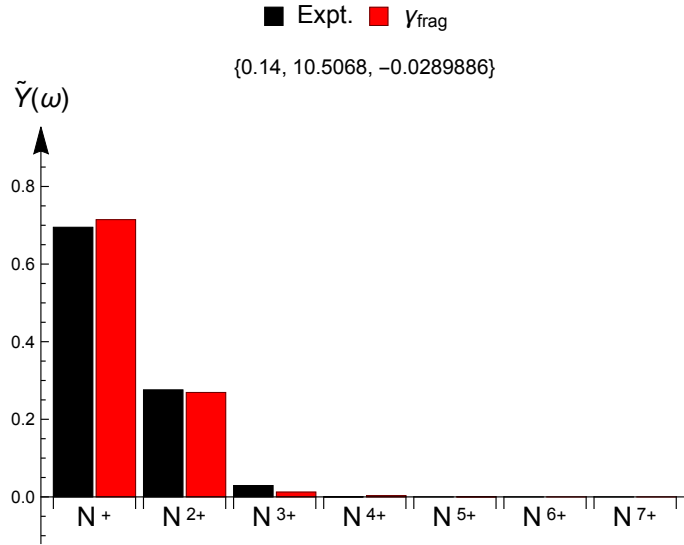

## 0.15

damp := 0.15

```
iy = dsionyieldcrateranalysisparam[damp * 0.26 * MilliJouleToHartree, photonenergy,
  tauX, nintdata, True, True, 1 / 1000, optfNppN, 1 - optfNppN, optGaFra]
```

```
iynorm = 1 / Total[iy[[2 ;; 8]]] * iy
```

```
Total[iynorm[[2 ;; 8]]]
```

```
{0.981253, 0.0132356, 0.00516416, 0.000263985,
  0.0000737255, 8.97151 × 10-6, 8.83068 × 10-8, 1.53366 × 10-10,
  0.979031, 0.000416761, 1.72198 × 10-48, -9.53985 × 10-165}
```

```
{52.3431, 0.70603, 0.275472, 0.0140818, 0.00393274, 0.000478568, 4.71055 × 10-6,
  8.18102 × 10-9, 52.2245, 0.0222313, 9.18559 × 10-47, -5.08885 × 10-163}
```

1.

```
plotiy = Partition[Riffle[normOleg7, iynorm[[2 ;; 8]]], 2]
```

```
{{0.694746, 0.70603}, {0.275684, 0.275472},
  {0.0293036, 0.0140818}, {0.000266625, 0.00393274},
  {0., 0.000478568}, {0., 4.71055 × 10-6}, {0., 8.18102 × 10-9}}
```

```

BarChart[plotiy, PlotRange → {-0.1, 0.9},
  ChartLabels → {Placed[{"N +", "N 2+", "N 3+", "N 4+", "N 5+", "N 6+", "N 7+"}, Below],
    Placed[{}, Above]},
  ChartLegends → Placed[{"Expt.", "γfrag"}, Top],
  ChartStyle → {Black, Red}, AxesLabel → {"", "Ỹ(ω)"},
  AxesStyle → {{Arrowheads[Automatic], AbsoluteThickness[0.6]},
    {Arrowheads[Automatic], AbsoluteThickness[0.6]}},
  LabelStyle → {FontFamily → "Arial"},
  PlotLabel → {damp, optGaFra / gammaFrag,
    (iynorm[[2 ;; 8]] - normOleg7).Table[i, {i, 1, 7}]]]

```

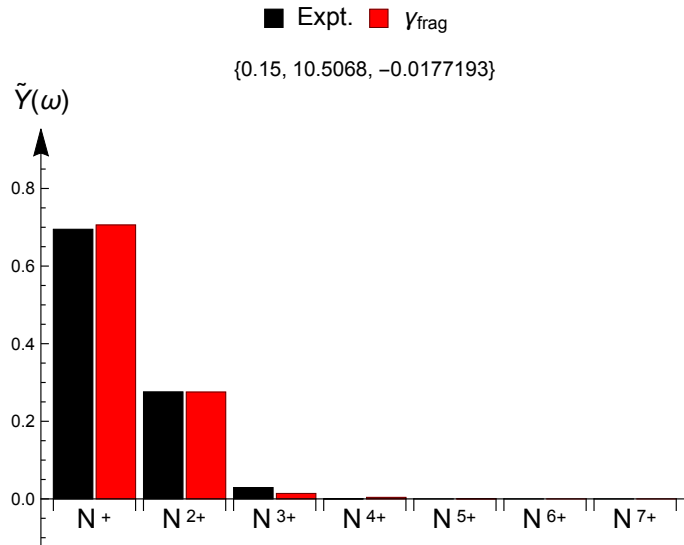

## 0.16

damp := 0.16

```

iy = dsionyieldcrateranalysisparam[damp * 0.26 * MilliJouleToHartree, photonenergy,
  tauX, nintdata, True, True, 1 / 1000, optfNppN, 1 - optfNppN, optGaFra]

```

```

iynorm = 1 / Total[iy[[2 ;; 8]]] * iy

```

```

Total[iynorm[[2 ;; 8]]]

```

```

{0.980216, 0.0138041, 0.00556915, 0.000310978, 0.0000879724, 0.0000113477,
  1.19493 × 10-7, 2.21703 × 10-10, 0.9779, 0.000433713, 1.9883 × 10-48, 5.29193 × 10-162}

```

```

{49.5467, 0.697752, 0.281502, 0.0157189, 0.00444672, 0.000573587, 6.03997 × 10-6,
  1.12064 × 10-8, 49.4297, 0.0219228, 1.00502 × 10-46, 2.6749 × 10-160}

```

1.

```

plotiy = Partition[Riffle[normOleg7, iynorm[[2 ;; 8]]], 2]

```

```

{{0.694746, 0.697752}, {0.275684, 0.281502},
 {0.0293036, 0.0157189}, {0.000266625, 0.00444672},
 {0., 0.000573587}, {0., 6.03997 × 10-6}, {0., 1.12064 × 10-8}}

```



```
BarChart[plotiy, PlotRange → {-0.1, 0.9},
  ChartLabels → {Placed[{"N +", "N 2+", "N 3+", "N 4+", "N 5+", "N 6+", "N 7+"}, Below],
    Placed[{}, Above]},
  ChartLegends → Placed[{"Expt.", "γfrag"}, Top],
  ChartStyle → {Black, Red}, AxesLabel → {"", "Ỹ(ω)"},
  AxesStyle → {{Arrowheads[Automatic], AbsoluteThickness[0.6]},
    {Arrowheads[Automatic], AbsoluteThickness[0.6]}},
  LabelStyle → {FontFamily → "Arial"},
  PlotLabel → {damp, optGaFra / gammaFrag,
    (iynorm[[2 ;; 8]] - normOleg7).Table[i, {i, 1, 7}]]]
```

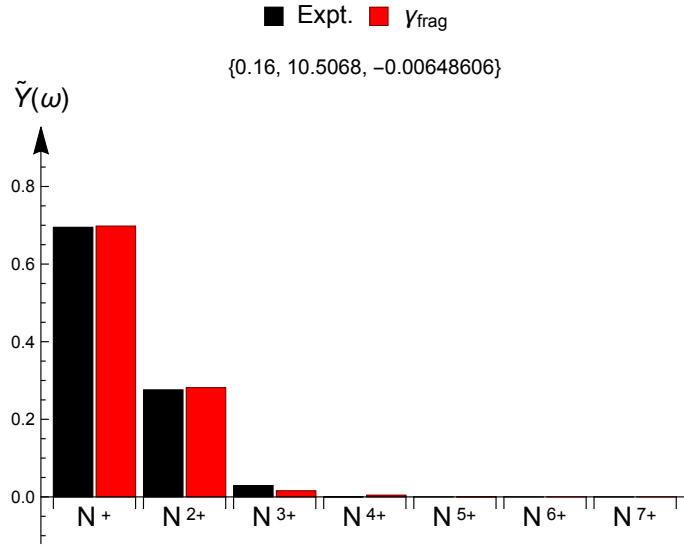

## 0.17

damp := 0.17

```
iy = dsionyieldcrateranalysisparam[damp * 0.26 * MilliJouleToHartree, photonenergy,
  tauX, nintdata, True, True, 1 / 1000, optfNppN, 1 - optfNppN, optGaFra]
```

```
iynorm = 1 / Total[iy[[2 ;; 8]]] * iy
```

```
Total[iynorm[[2 ;; 8]]]
```

```
{0.979201, 0.0143439, 0.0059746, 0.000362118, 0.000103749, 0.0000141323,
  1.58582 × 10-7, 3.131 × 10-10, 0.976796, 0.000449711, 1.96433 × 10-48, 3.62823 × 10-144}
```

```
{47.0801, 0.689655, 0.287259, 0.0174107, 0.00498826, 0.000679483, 7.62464 × 10-6,
  1.50538 × 10-8, 46.9644, 0.0216221, 9.44453 × 10-47, 1.74446 × 10-142}
```

1.

```
plotiy = Partition[Riffle[normOleg7, iynorm[[2 ;; 8]]], 2]
```

```
{{0.694746, 0.689655}, {0.275684, 0.287259},
  {0.0293036, 0.0174107}, {0.000266625, 0.00498826},
  {0., 0.000679483}, {0., 7.62464 × 10-6}, {0., 1.50538 × 10-8}}
```

```
BarChart[plotiy, PlotRange → {-0.1, 0.9},
  ChartLabels → {Placed[{"N +", "N 2+", "N 3+", "N 4+", "N 5+", "N 6+", "N 7+"}, Below],
    Placed[{}, Above]},
  ChartLegends → Placed[{"Expt.", "γfrag"}, Top],
  ChartStyle → {Black, Red}, AxesLabel → {"", "Ỹ(ω)",
  AxesStyle → {{Arrowheads[Automatic], AbsoluteThickness[0.6]},
    {Arrowheads[Automatic], AbsoluteThickness[0.6]}},
  LabelStyle → {FontFamily → "Arial"},
  PlotLabel → {damp, optGaFra / gammaFrag,
    (iynorm[[2 ;; 8]] - normOleg7).Table[i, {i, 1, 7}]]]
```

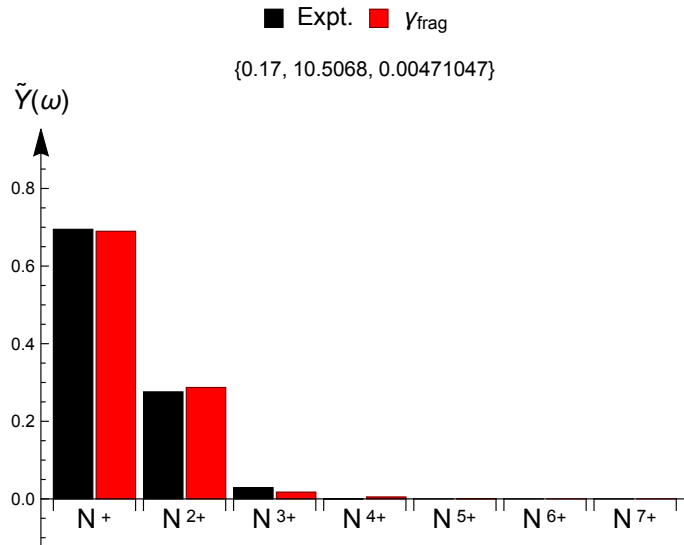

## 0.18

damp := 0.18

```
iy = dsionyieldcrateranalysisparam[damp * 0.26 * MilliJouleToHartree, photonenergy,
  tauX, nintdata, True, True, 1 / 1000, optfNppN, 1 - optfNppN, optGaFra]
```

```
iynorm = 1 / Total[iy[[2 ;; 8]]] * iy
```

```
Total[iynorm[[2 ;; 8]]]
```

```
{0.978208, 0.0148564, 0.00637969, 0.000417368,
  0.00012109, 0.0000173603, 2.06869 × 10-7, 4.3313 × 10-10,
  0.975718, 0.000464809, 1.95267 × 10-48, -1.23247 × 10-153}}
```

```
{44.8881, 0.681733, 0.292752, 0.0191522, 0.00555661, 0.000796633, 9.49283 × 10-6,
  1.98755 × 10-8, 44.7739, 0.0213292, 8.96044 × 10-47, -5.65559 × 10-152}}
```

1.

```
plotiy = Partition[Riffle[normOleg7, iynorm[[2 ;; 8]]], 2]
```

```
{{0.694746, 0.681733}, {0.275684, 0.292752},
  {0.0293036, 0.0191522}, {0.000266625, 0.00555661},
  {0., 0.000796633}, {0., 9.49283 × 10-6}, {0., 1.98755 × 10-8}}
```

```
BarChart[plotiy, PlotRange → {-0.1, 0.9},
  ChartLabels → {Placed[{"N +", "N 2+", "N 3+", "N 4+", "N 5+", "N 6+", "N 7+"}, Below],
    Placed[{}, Above]},
  ChartLegends → Placed[{"Expt.", "γfrag"}, Top],
  ChartStyle → {Black, Red}, AxesLabel → {"", "Ỹ(ω)"},
  AxesStyle → {{Arrowheads[Automatic], AbsoluteThickness[0.6]},
    {Arrowheads[Automatic], AbsoluteThickness[0.6]}},
  LabelStyle → {FontFamily → "Arial"},
  PlotLabel → {damp, optGaFra / gammaFrag,
    (iynorm[[2 ;; 8]] - normOleg7).Table[i, {i, 1, 7}]]]
```

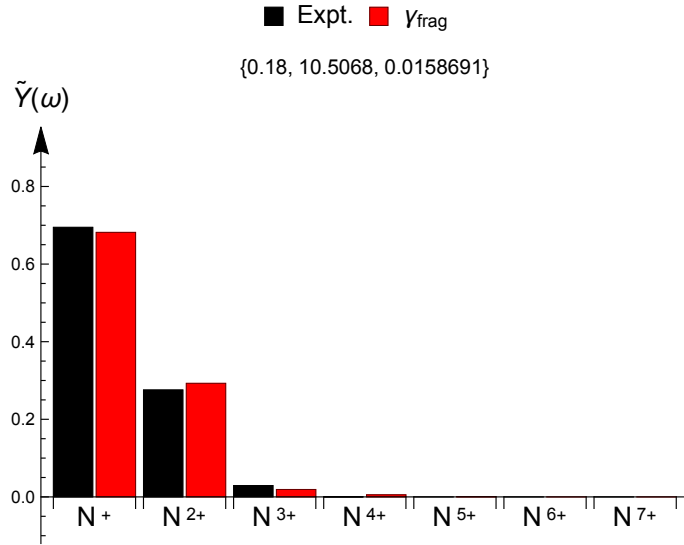

## Pulse energy for a 7 fs pulse with 80 fs fragmentation rate

```
tauX := shtdur7 * 7 / t0ToFemtoSecond
optent := 25.000000
optGaFra := optent * gammaFrag
```

### 0.12

```
damp := 0.12

iy = dsionyieldcrateranalysisparam[damp * 0.26 * MilliJouleToHartree, photonenergy,
  tauX, nintdata, True, True, 1 / 1000, optfNppN, 1 - optfNppN, optGaFra]
iynorm = 1 / Total[iy[[2 ;; 8]]] * iy
Total[iynorm[[2 ;; 8]]]

{0.984505, 0.0113447, 0.00395643, 0.000150001,
  0.0000400386, 4.01412 × 10-6, 3.14443 × 10-8, 4.36833 × 10-11,
  0.982596, 0.000359602, 4.79394 × 10-113, 6.07182 × 10-224}

{63.5363, 0.732141, 0.255333, 0.0096805, 0.00258394, 0.000259056, 2.0293 × 10-6,
  2.81916 × 10-9, 63.4131, 0.0232074, 3.09383 × 10-111, 3.91852 × 10-222}

1.
```

```

plotiy = Partition[Riffle[normOleg7, iynorm[[2 ;; 8]]], 2]
{
  {0.694746, 0.732141}, {0.275684, 0.255333},
  {0.0293036, 0.0096805}, {0.000266625, 0.00258394},
  {0., 0.000259056}, {0.,  $2.0293 \times 10^{-6}$ }, {0.,  $2.81916 \times 10^{-9}$ }
}

BarChart[plotiy, PlotRange → {-0.1, 0.9},
  ChartLabels → {Placed[{"N +", "N 2+", "N 3+", "N 4+", "N 5+", "N 6+", "N 7+"}, Below],
    Placed[{}, Above]},
  ChartLegends → Placed[{"Expt.", " $\gamma_{\text{frag}}$ "}, Top],
  ChartStyle → {Black, Red}, AxesLabel → {"", " $\tilde{Y}(\omega)$ "},
  AxesStyle → {{Arrowheads[Automatic], AbsoluteThickness[0.6]},
    {Arrowheads[Automatic], AbsoluteThickness[0.6]}},
  LabelStyle → {FontFamily → "Arial"},
  PlotLabel → {damp, optGaFra / gammaFrag,
    (iynorm[[2 ;; 8]] - normOleg7).Table[i, {i, 1, 7}]}]

```

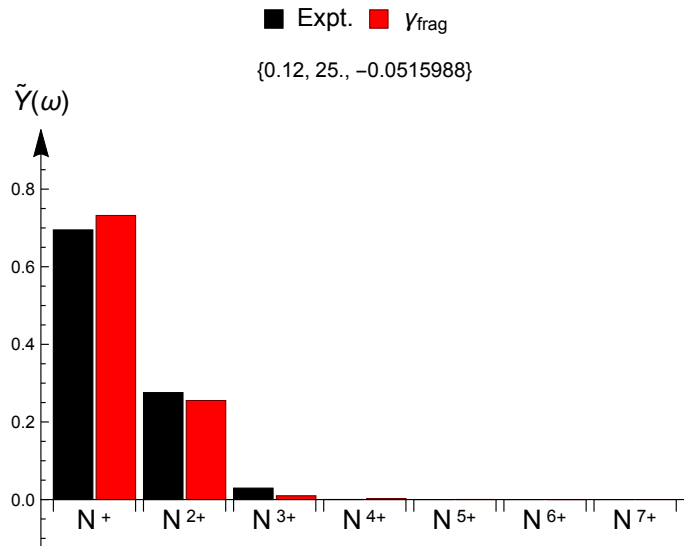

## 0.13

```

damp := 0.13

iy = dsionyieldcrateranalysisparam[damp * 0.26 * MilliJouleToHartree, photonenergy,
  tauX, nintdata, True, True, 1 / 1000, optfNppN, 1 - optfNppN, optGaFra]
iynorm = 1 / Total[iy[[2 ;; 8]]] * iy
Total[iynorm[[2 ;; 8]]]
{
  0.983397, 0.0120089, 0.00435362, 0.000184804,
  0.0000500036,  $5.3908 \times 10^{-6}$ ,  $4.58693 \times 10^{-8}$ ,  $6.91139 \times 10^{-11}$ ,
  0.981378, 0.000379768,  $5.45365 \times 10^{-113}$ ,  $5.0911 \times 10^{-227}$ 
}

{
  59.2308, 0.723308, 0.262222, 0.0111309, 0.00301176, 0.000324692,  $2.76274 \times 10^{-6}$ ,
   $4.16278 \times 10^{-9}$ , 59.1092, 0.0228737,  $3.28477 \times 10^{-111}$ ,  $3.06641 \times 10^{-225}$ 
}

```

1.

```
plotiy = Partition[Riffle[normOleg7, iynorm[[2 ;; 8]]], 2]
```

```
{ {0.694746, 0.723308}, {0.275684, 0.262222},  
  {0.0293036, 0.0111309}, {0.000266625, 0.00301176},  
  {0., 0.000324692}, {0.,  $2.76274 \times 10^{-6}$ }, {0.,  $4.16278 \times 10^{-9}$ }}
```

```
BarChart[plotiy, PlotRange → {-0.1, 0.9},  
  ChartLabels → {Placed[{"N +", "N 2+", "N 3+", "N 4+", "N 5+", "N 6+", "N 7+"}, Below],  
    Placed[{}, Above]},  
  ChartLegends → Placed[{"Expt.", " $\gamma_{\text{frag}}$ "}, Top],  
  ChartStyle → {Black, Red}, AxesLabel → {"", " $\tilde{Y}(\omega)$ "},  
  AxesStyle → {{Arrowheads[Automatic], AbsoluteThickness[0.6]},  
    {Arrowheads[Automatic], AbsoluteThickness[0.6]}},  
  LabelStyle → {FontFamily → "Arial"},  
  PlotLabel → {damp, optGaFra / gammaFrag,  
    (iynorm[[2 ;; 8]] - normOleg7).Table[i, {i, 1, 7}]}]
```

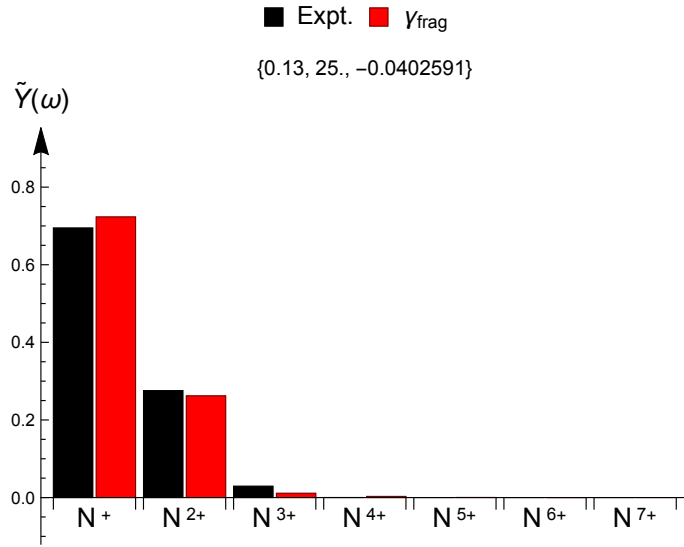

## 0.14

```
damp := 0.14
```

```
iy = dsionyieldcrateranalysisparam[damp * 0.26 * MilliJouleToHartree, photonenergy,  
  tauX, nintdata, True, True, 1 / 1000, optfNppN, 1 - optfNppN, optGaFra]
```

```
iynorm = 1 / Total[iy[[2 ;; 8]]] * iy
```

```
Total[iynorm[[2 ;; 8]]]
```

```
{0.982314, 0.0126397, 0.00475422, 0.000223747, 0.0000613575,  $7.0729 \times 10^{-6}$ ,  
   $6.49868 \times 10^{-8}$ ,  $1.05582 \times 10^{-10}$ , 0.98019, 0.0003988,  $6.65676 \times 10^{-113}$ ,  $4.87996 \times 10^{-257}$ }
```

```
{55.5413, 0.714666, 0.26881, 0.012651, 0.00346923, 0.000399911,  $3.67444 \times 10^{-6}$ ,  
   $5.96974 \times 10^{-9}$ , 55.4212, 0.0225487,  $3.76382 \times 10^{-111}$ ,  $2.75919 \times 10^{-255}$ }
```

1.

```
plotiy = Partition[Riffle[normOleg7, iynorm[[2 ;; 8]]], 2]
```

```
{ {0.694746, 0.714666}, {0.275684, 0.26881},  
  {0.0293036, 0.012651}, {0.000266625, 0.00346923},  
  {0., 0.000399911}, {0.,  $3.67444 \times 10^{-6}$ }, {0.,  $5.96974 \times 10^{-9}$ }}
```

```
BarChart[plotiy, PlotRange → {-0.1, 0.9},
  ChartLabels → {Placed[{"N +", "N 2+", "N 3+", "N 4+", "N 5+", "N 6+", "N 7+"}, Below],
    Placed[{}, Above]},
  ChartLegends → Placed[{"Expt.", "γfrag"}, Top],
  ChartStyle → {Black, Red}, AxesLabel → {"", "Ỹ(ω)",
  AxesStyle → {{Arrowheads[Automatic], AbsoluteThickness[0.6]},
    {Arrowheads[Automatic], AbsoluteThickness[0.6]}},
  LabelStyle → {FontFamily → "Arial"},
  PlotLabel → {damp, optGaFra / gammaFrag,
    (iynorm[[2 ;; 8]] - normOleg7).Table[i, {i, 1, 7}]]]
```

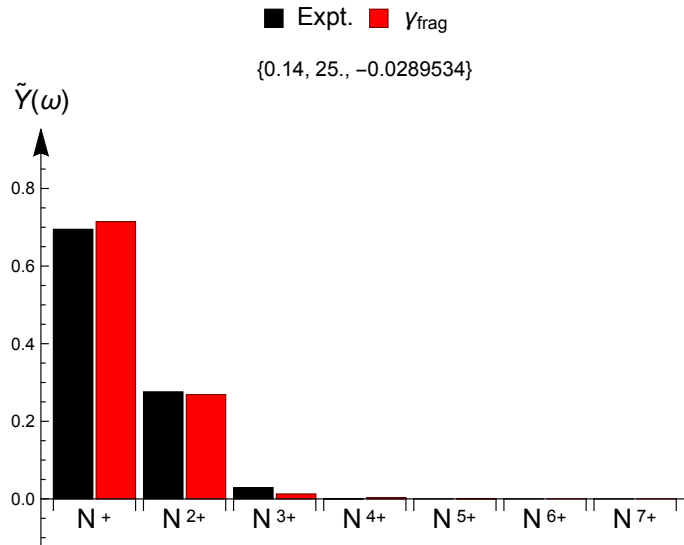

## 0.15

damp := 0.15

```
iy = dsionyieldcrateranalysisparam[damp * 0.26 * MilliJouleToHartree, photonenergy,
  tauX, nintdata, True, True, 1 / 1000, optfNppN, 1 - optfNppN, optGaFra]
```

```
iynorm = 1 / Total[iy[[2 ;; 8]]] * iy
```

```
Total[iynorm[[2 ;; 8]]]
```

```
{0.981254, 0.0132387, 0.00515715, 0.000266857,
  0.0000741529, 9.09527 × 10-6, 8.97833 × 10-8, 1.56488 × 10-10,
  0.979031, 0.000416761, 7.0692 × 10-113, 2.55826 × 10-207}
```

```
{52.3446, 0.706213, 0.275106, 0.0142354, 0.00395566, 0.000485184, 4.78946 × 10-6,
  8.34777 × 10-9, 52.2261, 0.022232, 3.77104 × 10-111, 1.3647 × 10-205}
```

1.

```
plotiy = Partition[Riffle[normOleg7, iynorm[[2 ;; 8]]], 2]
```

```
{{0.694746, 0.706213}, {0.275684, 0.275106},
  {0.0293036, 0.0142354}, {0.000266625, 0.00395566},
  {0., 0.000485184}, {0., 4.78946 × 10-6}, {0., 8.34777 × 10-9}}
```

```
BarChart[plotiy, PlotRange → {-0.1, 0.9},
  ChartLabels → {Placed[{"N +", "N 2+", "N 3+", "N 4+", "N 5+", "N 6+", "N 7+"}, Below],
    Placed[{}, Above]},
  ChartLegends → Placed[{"Expt.", "γfrag"}, Top],
  ChartStyle → {Black, Red}, AxesLabel → {"", "Ỹ(ω)",
  AxesStyle → {{Arrowheads[Automatic], AbsoluteThickness[0.6]},
    {Arrowheads[Automatic], AbsoluteThickness[0.6]}},
  LabelStyle → {FontFamily → "Arial"},
  PlotLabel → {damp, optGaFra / gammaFrag,
    (iynorm[[2 ;; 8]] - normOleg7).Table[i, {i, 1, 7}]]]
```

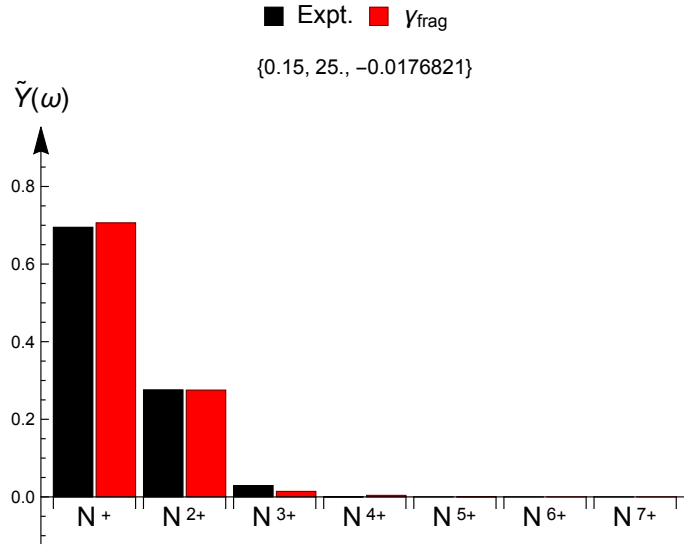

## 0.16

damp := 0.16

```
iy = dsionyieldcrateranalysisparam[damp * 0.26 * MilliJouleToHartree, photonenergy,
  tauX, nintdata, True, True, 1 / 1000, optfNppN, 1 - optfNppN, optGaFra]
```

```
iynorm = 1 / Total[iy[[2 ;; 8]]] * iy
```

```
Total[iynorm[[2 ;; 8]]]
```

```
{0.980217, 0.0138075, 0.00556143, 0.000314134, 0.0000884361, 0.0000114929,
  1.21349 × 10-7, 2.25905 × 10-10, 0.9779, 0.000433713, 6.29898 × 10-113, 5.45533 × 10-230}
```

```
{49.5483, 0.697943, 0.281121, 0.0158789, 0.00447029, 0.000580946, 6.134 × 10-6,
  1.14191 × 10-8, 49.4312, 0.0219234, 3.18403 × 10-111, 2.75757 × 10-228}
```

1.

```
plotiy = Partition[Riffle[normOleg7, iynorm[[2 ;; 8]]], 2]
```

```
{{0.694746, 0.697943}, {0.275684, 0.281121},
  {0.0293036, 0.0158789}, {0.000266625, 0.00447029},
  {0., 0.000580946}, {0., 6.134 × 10-6}, {0., 1.14191 × 10-8}}
```

```
BarChart[plotiy, PlotRange → {-0.1, 0.9},
  ChartLabels → {Placed[{"N +", "N 2+", "N 3+", "N 4+", "N 5+", "N 6+", "N 7+"}, Below],
    Placed[{}, Above]},
  ChartLegends → Placed[{"Expt.", "γfrag"}, Top],
  ChartStyle → {Black, Red}, AxesLabel → {"", "Ỹ(ω)"},
  AxesStyle → {{Arrowheads[Automatic], AbsoluteThickness[0.6]},
    {Arrowheads[Automatic], AbsoluteThickness[0.6]}},
  LabelStyle → {FontFamily → "Arial"},
  PlotLabel → {damp, optGaFra / gammaFrag,
    (iynorm[[2 ;; 8]] - normOleg7).Table[i, {i, 1, 7}]]]
```

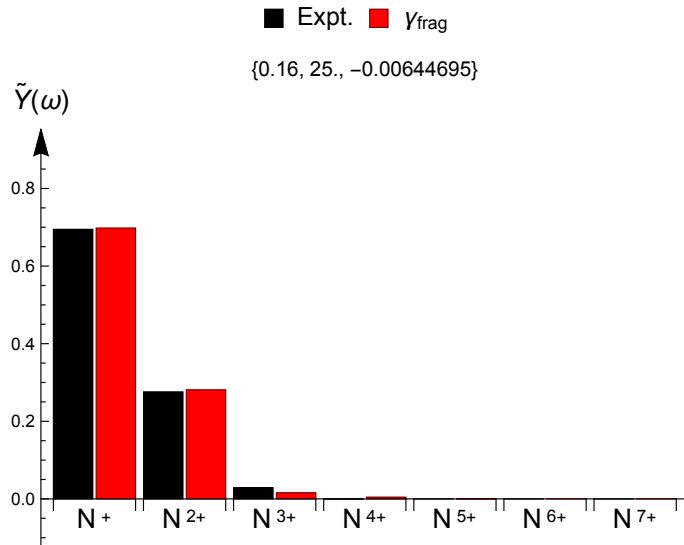

## 0.17

```
damp := 0.17
```

```
iy = dsionyieldcrateranalysisparam[damp * 0.26 * MilliJouleToHartree, photonenergy,
  tauX, nintdata, True, True, 1 / 1000, optfNppN, 1 - optfNppN, optGaFra]
```

```
iynorm = 1 / Total[iy[[2 ;; 8]]] * iy
```

```
Total[iynorm[[2 ;; 8]]]
```

```
{0.979202, 0.0143475, 0.00596616, 0.000365559,
  0.000104248, 0.0000143008, 1.60881 × 10-7, 3.18646 × 10-10,
  0.976796, 0.000449711, 6.3144 × 10-113, -1.3282 × 10-228}
```

```
{47.0816, 0.689853, 0.286863, 0.0175767, 0.00501241, 0.000687605, 7.7354 × 10-6,
  1.5321 × 10-8, 46.9659, 0.0216228, 3.03606 × 10-111, -6.38621 × 10-227}
```

```
1.
```

```
plotiy = Partition[Riffle[normOleg7, iynorm[[2 ;; 8]]], 2]
```

```
{{0.694746, 0.689853}, {0.275684, 0.286863},
  {0.0293036, 0.0175767}, {0.000266625, 0.00501241},
  {0., 0.000687605}, {0., 7.7354 × 10-6}, {0., 1.5321 × 10-8}}
```



```
BarChart[plotiy, PlotRange → {-0.1, 0.9},
  ChartLabels → {Placed[{"N +", "N 2+", "N 3+", "N 4+", "N 5+", "N 6+", "N 7+"}, Below],
    Placed[{}, Above]},
  ChartLegends → Placed[{"Expt.", "γfrag"}, Top],
  ChartStyle → {Black, Red}, AxesLabel → {"", "Ỹ(ω)"},
  AxesStyle → {{Arrowheads[Automatic], AbsoluteThickness[0.6]},
    {Arrowheads[Automatic], AbsoluteThickness[0.6]}},
  LabelStyle → {FontFamily → "Arial"},
  PlotLabel → {damp, optGaFra / gammaFrag,
    (iynorm[[2 ;; 8]] - normOleg7).Table[i, {i, 1, 7}]]]
```

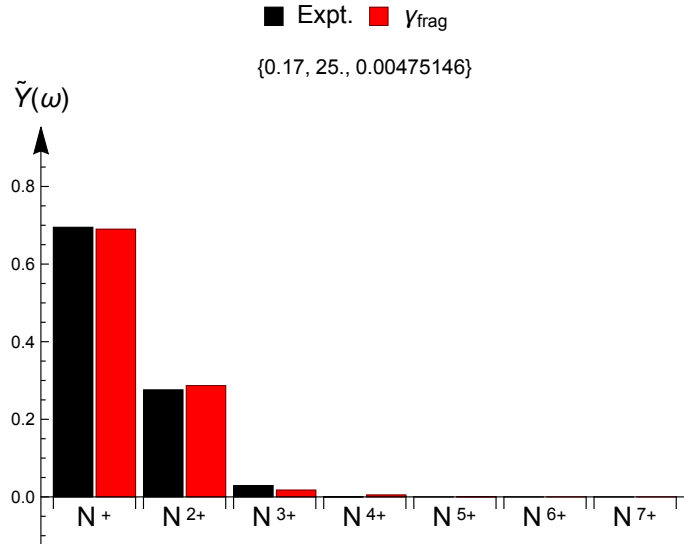

## 0.18

damp := 0.18

```
iy = dsionyieldcrateranalysisparam[damp * 0.26 * MilliJouleToHartree, photonenergy,
  tauX, nintdata, True, True, 1 / 1000, optfNppN, 1 - optfNppN, optGaFra]
```

```
iynorm = 1 / Total[iy[[2 ;; 8]]] * iy
```

```
Total[iynorm[[2 ;; 8]]]
```

```
{0.978209, 0.0148604, 0.00637053, 0.000421094,
  0.000121624, 0.0000175538, 2.09676 × 10-7, 4.40326 × 10-10,
  0.975718, 0.000464809, 5.71859 × 10-113, 4.66383 × 10-229}
```

```
{44.8896, 0.681939, 0.292341, 0.0193239, 0.00558126, 0.000805535, 9.62194 × 10-6,
  2.02064 × 10-8, 44.7753, 0.0213299, 2.62424 × 10-111, 2.14021 × 10-227}
```

1.

```
plotiy = Partition[Riffle[normOleg7, iynorm[[2 ;; 8]]], 2]
```

```
{{0.694746, 0.681939}, {0.275684, 0.292341},
  {0.0293036, 0.0193239}, {0.000266625, 0.00558126},
  {0., 0.000805535}, {0., 9.62194 × 10-6}, {0., 2.02064 × 10-8}}
```

```
BarChart[plotiy, PlotRange → {-0.1, 0.9},
  ChartLabels → {Placed[{"N +", "N 2+", "N 3+", "N 4+", "N 5+", "N 6+", "N 7+"}, Below],
    Placed[{}, Above]},
  ChartLegends → Placed[{"Expt.", "γfrag"}, Top],
  ChartStyle → {Black, Red}, AxesLabel → {"", "Ỹ(ω)"},
  AxesStyle → {{Arrowheads[Automatic], AbsoluteThickness[0.6]},
    {Arrowheads[Automatic], AbsoluteThickness[0.6]}},
  LabelStyle → {FontFamily → "Arial"},
  PlotLabel → {damp, optGaFra / gammaFrag,
    (iynorm[[2 ;; 8]] - normOleg7).Table[i, {i, 1, 7}]]]
```

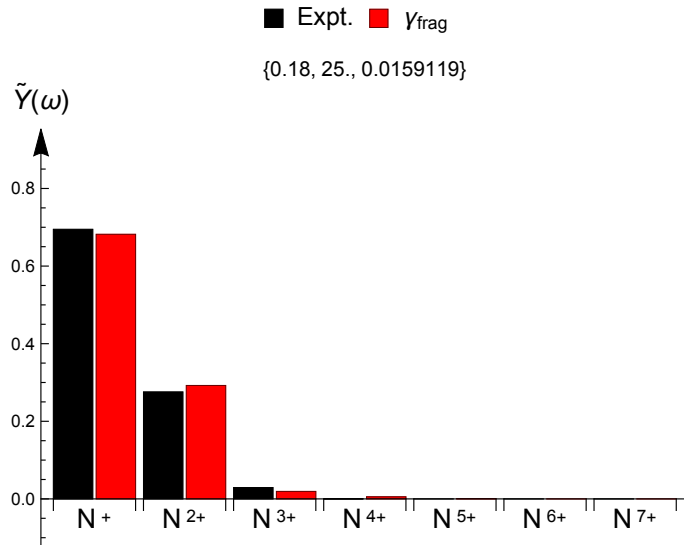

## Pulse energy for a 4 fs pulse with 280 fs fragmentation rate

```
tauX := shtdur4 * 4 / t0ToFemtoSecond
optent := 10.506791
optGaFra := optent * gammaFrag
```

### 0.21

```
damp := 0.21

iy = dsionyieldcrateranalysisparam[damp * 0.15 * MilliJouleToHartree, photonenergy,
  tauX, nintdata, True, True, 1 / 1000, optfNppN, 1 - optfNppN, optGaFra]
iynorm = 1 / Total[iy[[2 ;; 8]]] * iy
Total[iynorm[[2 ;; 8]]]
```

{0.984378, 0.0114397, 0.00399257, 0.000151183,  
 0.0000352676,  $2.7238 \times 10^{-6}$ ,  $1.32795 \times 10^{-8}$ ,  $1.07499 \times 10^{-11}$ ,  
 0.982454, 0.000361989,  $1.59086 \times 10^{-48}$ ,  $-3.5497 \times 10^{-221}$ }

{63.0143, 0.732307, 0.255582, 0.00967789, 0.00225763, 0.000174362,  $8.50078 \times 10^{-7}$ ,  
 $6.88148 \times 10^{-10}$ , 62.8911, 0.0231725,  $1.01838 \times 10^{-46}$ ,  $-2.27231 \times 10^{-219}$ }

1.

```

plotiy = Partition[Riffle[normOleg4, iynorm[[2 ;; 8]]], 2]
{{0.711226, 0.732307}, {0.277966, 0.255582}, {0.0108078, 0.00967789},
 {0., 0.00225763}, {0., 0.000174362}, {0.,  $8.50078 \times 10^{-7}$ }, {0.,  $6.88148 \times 10^{-10}$ }}

```

```

BarChart[plotiy, PlotRange → {-0.1, 0.9},
 ChartLabels → {Placed[{"N +", "N 2+", "N 3+", "N 4+", "N 5+", "N 6+", "N 7+"}, Below],
 Placed[{}, Above]},
 ChartLegends → Placed[{"Expt.", " $\gamma_{frag}$ "}, Top],
 ChartStyle → {Black, Red}, AxesLabel → {"", " $\tilde{Y}(\omega)$ "},
 AxesStyle → {{Arrowheads[Automatic], AbsoluteThickness[0.6]},
 {Arrowheads[Automatic], AbsoluteThickness[0.6]}},
 LabelStyle → {FontFamily → "Arial"},
 PlotLabel → {damp, optGaFra / gammaFrag,
 (iynorm[[2 ;; 8]] - normOleg4).Table[i, {i, 1, 7}]}]

```

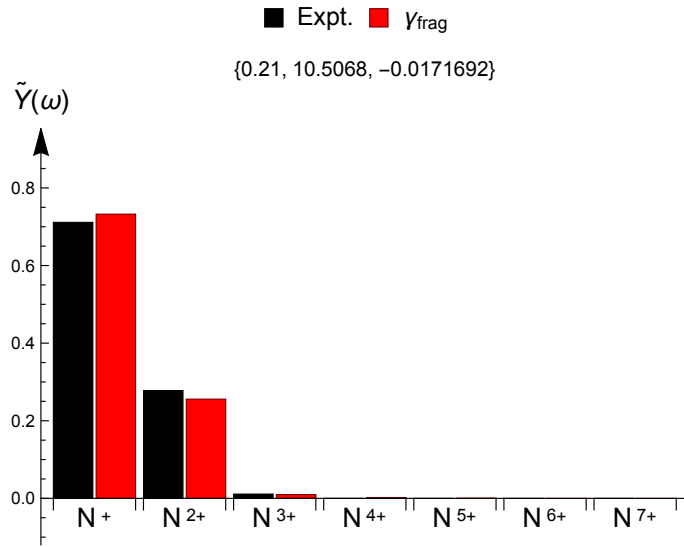

## 0.22

```
damp := 0.22
```

```

iy = dsionyieldcrateranalysisparam[damp * 0.15 * MilliJouleToHartree, photonenergy,
 tauX, nintdata, True, True, 1 / 1000, optfNppN, 1 - optfNppN, optGaFra]

```

```
iynorm = 1 / Total[iy[[2 ;; 8]]] * iy
```

```
Total[iynorm[[2 ;; 8]]]
```

```

{0.983738, 0.0118261, 0.00422114, 0.000170896, 0.0000402634,  $3.24099 \times 10^{-6}$ ,
  $1.65874 \times 10^{-8}$ ,  $1.40834 \times 10^{-11}$ , 0.98175, 0.000373687,  $1.5903 \times 10^{-48}$ ,  $1.82354 \times 10^{-219}$ }

```

```

{60.4943, 0.727239, 0.259576, 0.0105091, 0.00247597, 0.000199302,  $1.02003 \times 10^{-6}$ ,
  $8.66046 \times 10^{-10}$ , 60.372, 0.0229796,  $9.77945 \times 10^{-47}$ ,  $1.12137 \times 10^{-217}$ }

```

1.

```
plotiy = Partition[Riffle[normOleg4, iynorm[[2 ;; 8]]], 2]
```

```

{{0.711226, 0.727239}, {0.277966, 0.259576}, {0.0108078, 0.0105091},
 {0., 0.00247597}, {0., 0.000199302}, {0.,  $1.02003 \times 10^{-6}$ }, {0.,  $8.66046 \times 10^{-10}$ }}

```

```
BarChart[plotiy, PlotRange → {-0.1, 0.9},
  ChartLabels → {Placed[{"N +", "N 2+", "N 3+", "N 4+", "N 5+", "N 6+", "N 7+"}, Below],
    Placed[{}, Above]},
  ChartLegends → Placed[{"Expt.", "γfrag"}, Top],
  ChartStyle → {Black, Red}, AxesLabel → {"", "Ỹ(ω)",
  AxesStyle → {{Arrowheads[Automatic], AbsoluteThickness[0.6]},
    {Arrowheads[Automatic], AbsoluteThickness[0.6]}},
  LabelStyle → {FontFamily → "Arial"},
  PlotLabel → {damp, optGaFra / gammaFrag,
    (iynorm[[2 ;; 8]] - normOleg4).Table[i, {i, 1, 7}]]]
```

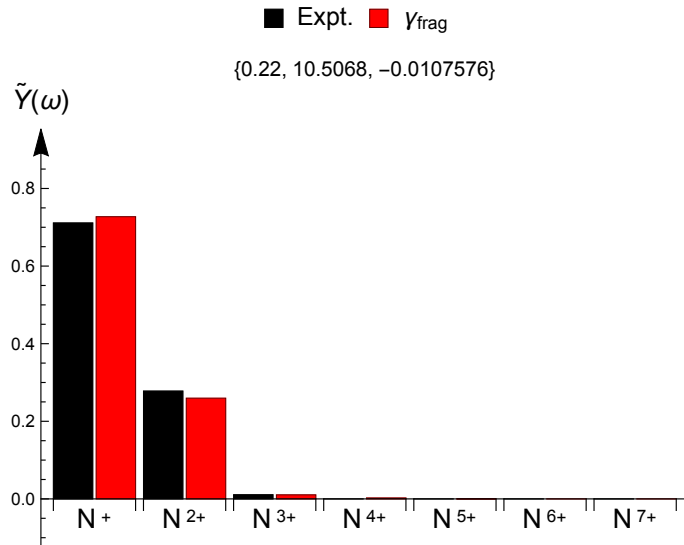

## 0.23

damp := 0.23

```
iy = dsionyieldcrateranalysisparam[damp * 0.15 * MilliJouleToHartree, photonenergy,
  tauX, nintdata, True, True, 1 / 1000, optfNppN, 1 - optfNppN, optGaFra]
```

```
iynorm = 1 / Total[iy[[2 ;; 8]]] * iy
```

```
Total[iynorm[[2 ;; 8]]]
```

```
{0.983106, 0.0122012, 0.00445098, 0.000191992, 0.000045681, 3.82479 × 10-6,
  2.05072 × 10-8, 1.82239 × 10-11, 0.981055, 0.000385, 1.61039 × 10-48, -2.7442 × 10-210}
```

```
{58.1937, 0.722234, 0.26347, 0.0113647, 0.00270403, 0.000226403, 1.21389 × 10-6,
  1.07874 × 10-9, 58.0723, 0.0227896, 9.53249 × 10-47, -1.6244 × 10-208}
```

1.

```
plotiy = Partition[Riffle[normOleg4, iynorm[[2 ;; 8]]], 2]
```

```
{{0.711226, 0.722234}, {0.277966, 0.26347}, {0.0108078, 0.0113647},
  {0., 0.00270403}, {0., 0.000226403}, {0., 1.21389 × 10-6}, {0., 1.07874 × 10-9}}
```

```
BarChart[plotiy, PlotRange → {-0.1, 0.9},
  ChartLabels → {Placed[{"N +", "N 2+", "N 3+", "N 4+", "N 5+", "N 6+", "N 7+"}, Below],
    Placed[{}, Above]},
  ChartLegends → Placed[{"Expt.", "γfrag"}, Top],
  ChartStyle → {Black, Red}, AxesLabel → {"", "Ỹ(ω)"},
  AxesStyle → {{Arrowheads[Automatic], AbsoluteThickness[0.6]},
    {Arrowheads[Automatic], AbsoluteThickness[0.6]}},
  LabelStyle → {FontFamily → "Arial"},
  PlotLabel → {damp, optGaFra / gammaFrag,
    (iynorm[[2 ;; 8]] - normOleg4).Table[i, {i, 1, 7}]]]
```

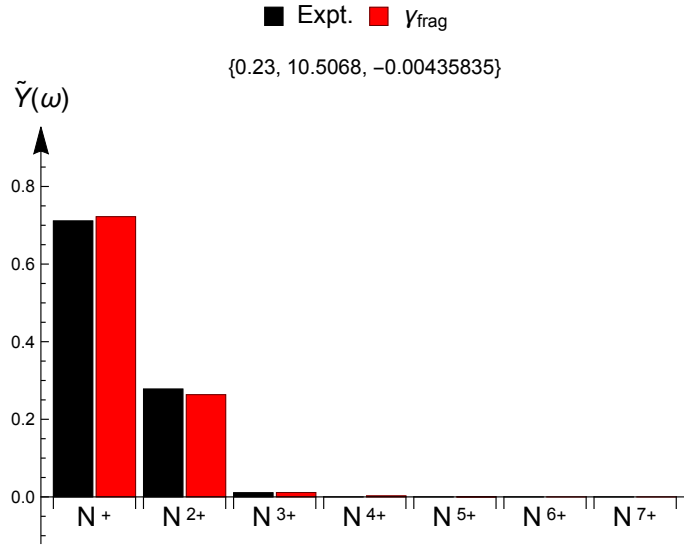

## 0.24

```
damp := 0.24

iy = dsionyieldcrateranalysisparam[damp * 0.15 * MilliJouleToHartree, photonenergy,
  tauX, nintdata, True, True, 1 / 1000, optfNppN, 1 - optfNppN, optGaFra]
iynorm = 1 / Total[iy[[2 ;; 8]]] * iy
Total[iynorm[[2 ;; 8]]]
{0.982482, 0.0125653, 0.0046819, 0.000214481,
  0.0000515326, 4.4799 × 10-6, 2.51154 × 10-8, 2.33165 × 10-11,
  0.980371, 0.000395944, 1.65479 × 10-48, -2.29224 × 10-212}

{56.085, 0.717291, 0.267267, 0.0122437, 0.00294174, 0.000255735, 1.43371 × 10-6,
  1.33103 × 10-9, 55.9645, 0.0226025, 9.44635 × 10-47, -1.30853 × 10-210}

1.

plotiy = Partition[Riffle[normOleg4, iynorm[[2 ;; 8]]], 2]
{{0.711226, 0.717291}, {0.277966, 0.267267}, {0.0108078, 0.0122437},
  {0., 0.00294174}, {0., 0.000255735}, {0., 1.43371 × 10-6}, {0., 1.33103 × 10-9}}
```

```
BarChart[plotiy, PlotRange → {-0.1, 0.9},
  ChartLabels → {Placed[{"N +", "N 2+", "N 3+", "N 4+", "N 5+", "N 6+", "N 7+"}, Below],
    Placed[{}, Above]},
  ChartLegends → Placed[{"Expt.", "γfrag"}, Top],
  ChartStyle → {Black, Red}, AxesLabel → {"", "Ỹ(ω)"},
  AxesStyle → {{Arrowheads[Automatic], AbsoluteThickness[0.6]},
    {Arrowheads[Automatic], AbsoluteThickness[0.6]}},
  LabelStyle → {FontFamily → "Arial"},
  PlotLabel → {damp, optGaFra / gammaFrag,
    (iynorm[[2 ;; 8]] - normOleg4).Table[i, {i, 1, 7}]]]
```

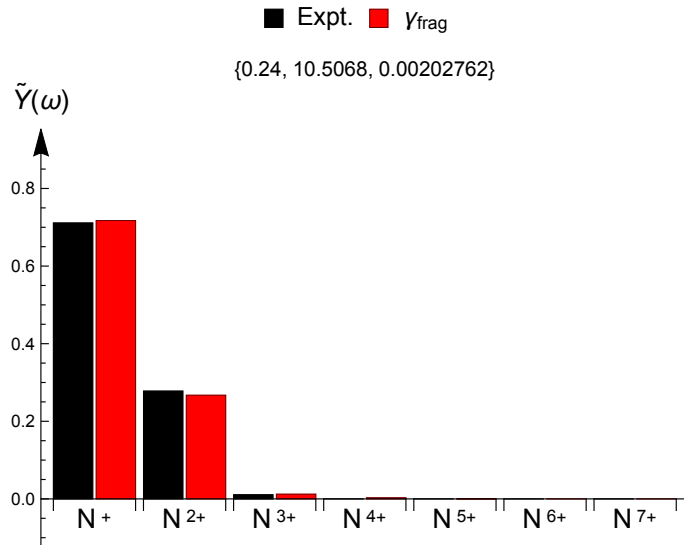

## 0.25

damp := 0.25

```
iy = dsionyieldcrateranalysisparam[damp * 0.15 * MilliJouleToHartree, photonenergy,
  tauX, nintdata, True, True, 1 / 1000, optfNppN, 1 - optfNppN, optGaFra]
```

```
iynorm = 1 / Total[iy[[2 ;; 8]]] * iy
```

```
Total[iynorm[[2 ;; 8]]]
```

```
{0.981866, 0.0129187, 0.00491368, 0.000238369,
  0.0000578295, 5.21108 × 10-6, 3.04942 × 10-8, 2.95241 × 10-11,
  0.979696, 0.000406526, 1.72635 × 10-48, 8.82125 × 10-218}
```

```
{54.1455, 0.712409, 0.270968, 0.013145, 0.00318904, 0.000287368, 1.68162 × 10-6,
  1.62812 × 10-9, 54.0259, 0.0224181, 9.52004 × 10-47, 4.86452 × 10-216}
```

1.

```
plotiy = Partition[Riffle[normOleg4, iynorm[[2 ;; 8]]], 2]
```

```
{{0.711226, 0.712409}, {0.277966, 0.270968}, {0.0108078, 0.013145},
  {0., 0.00318904}, {0., 0.000287368}, {0., 1.68162 × 10-6}, {0., 1.62812 × 10-9}}
```

```
BarChart[plotiy, PlotRange → {-0.1, 0.9},
  ChartLabels → {Placed[{"N +", "N 2+", "N 3+", "N 4+", "N 5+", "N 6+", "N 7+"}, Below],
    Placed[{}, Above]},
  ChartLegends → Placed[{"Expt.", "γfrag"}, Top],
  ChartStyle → {Black, Red}, AxesLabel → {"", "Ỹ(ω)"},
  AxesStyle → {{Arrowheads[Automatic], AbsoluteThickness[0.6]},
    {Arrowheads[Automatic], AbsoluteThickness[0.6]}},
  LabelStyle → {FontFamily → "Arial"},
  PlotLabel → {damp, optGaFra / gammaFrag,
    (iynorm[[2 ;; 8]] - normOleg4).Table[i, {i, 1, 7}]]]
```

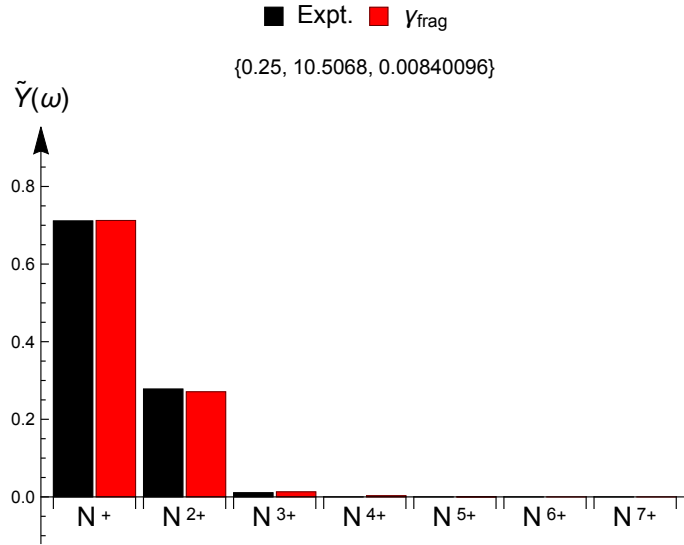

## Pulse energy for a 4 fs pulse with 80 fs fragmentation rate

```
tauX := shtdur4 * 4 / t0ToFemtoSecond
optent := 25.000000
optGaFra := optent * gammaFrag
```

### 0.21

```
damp := 0.21

iy = dsionyieldcrateranalysisparam[damp * 0.15 * MilliJouleToHartree, photonenergy,
  tauX, nintdata, True, True, 1 / 1000, optfNppN, 1 - optfNppN, optGaFra]
iynorm = 1 / Total[iy[[2 ;; 8]]] * iy
Total[iynorm[[2 ;; 8]]]

{0.984379, 0.0114405, 0.00399082, 0.000151905,
  0.0000353816, 2.74823 × 10-6, 1.34355 × 10-8, 1.09118 × 10-11,
  0.982454, 0.000361989, 6.01268 × 10-113, -1.2863 × 10-216}

{63.0149, 0.732362, 0.255472, 0.00972421, 0.00226495, 0.000175927, 8.6007 × 10-7,
  6.98517 × 10-10, 62.8917, 0.0231727, 3.84901 × 10-111, -8.23423 × 10-215}

1.
```

```

plotiy = Partition[Riffle[normOleg4, iynorm[[2 ;; 8]]], 2]
{{0.711226, 0.732362}, {0.277966, 0.255472}, {0.0108078, 0.00972421},
 {0., 0.00226495}, {0., 0.000175927}, {0.,  $8.6007 \times 10^{-7}$ }, {0.,  $6.98517 \times 10^{-10}$ }}

BarChart[plotiy, PlotRange → {-0.1, 0.9},
  ChartLabels → {Placed[{"N +", "N 2+", "N 3+", "N 4+", "N 5+", "N 6+", "N 7+"}, Below],
    Placed[{}, Above]},
  ChartLegends → Placed[{"Expt.", " $\gamma_{\text{frag}}$ "}, Top],
  ChartStyle → {Black, Red}, AxesLabel → {"", " $\tilde{Y}(\omega)$ "},
  AxesStyle → {{Arrowheads[Automatic], AbsoluteThickness[0.6]},
    {Arrowheads[Automatic], AbsoluteThickness[0.6]}},
  LabelStyle → {FontFamily → "Arial"},
  PlotLabel → {damp, optGaFra / gammaFrag,
    (iynorm[[2 ;; 8]] - normOleg4).Table[i, {i, 1, 7}]}]

```

■ Expt. ■  $\gamma_{\text{frag}}$

{0.21, 25., -0.0171583}

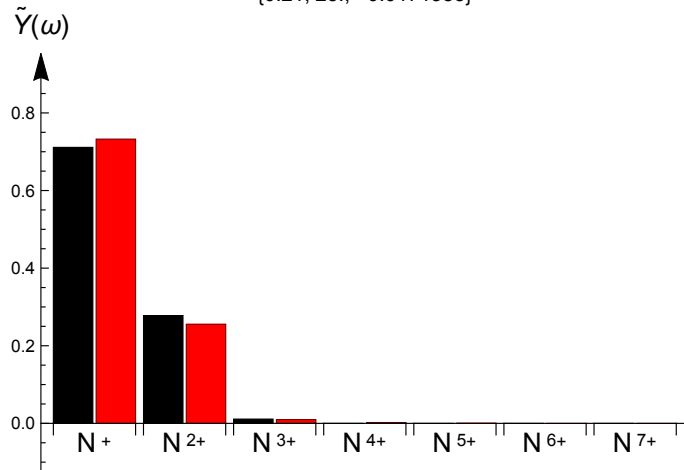

## 0.22

```

damp := 0.22

iy = dsionyieldcrateranalysisparam[damp * 0.15 * MilliJouleToHartree, photonenergy,
  tauX, nintdata, True, True, 1 / 1000, optfNppN, 1 - optfNppN, optGaFra]
iynorm = 1 / Total[iy[[2 ;; 8]]] * iy
Total[iynorm[[2 ;; 8]]]
{0.983738, 0.0118269, 0.00421925, 0.000171672,
 0.0000403853,  $3.26854 \times 10^{-6}$ ,  $1.67722 \times 10^{-8}$ ,  $1.42848 \times 10^{-11}$ ,
 0.98175, 0.000373687,  $1.91688 \times 10^{-112}$ ,  $2.33482 \times 10^{-173}$ }

{60.4948, 0.727296, 0.259462, 0.0105569, 0.00248349, 0.000200998,  $1.03141 \times 10^{-6}$ ,
  $8.7844 \times 10^{-10}$ , 60.3725, 0.0229798,  $1.17878 \times 10^{-110}$ ,  $1.4358 \times 10^{-171}$ }

1.

plotiy = Partition[Riffle[normOleg4, iynorm[[2 ;; 8]]], 2]
{{0.711226, 0.727296}, {0.277966, 0.259462}, {0.0108078, 0.0105569},
 {0., 0.00248349}, {0., 0.000200998}, {0.,  $1.03141 \times 10^{-6}$ }, {0.,  $8.7844 \times 10^{-10}$ }}

```



```
BarChart[plotiy, PlotRange → {-0.1, 0.9},
  ChartLabels → {Placed[{"N +", "N 2+", "N 3+", "N 4+", "N 5+", "N 6+", "N 7+"}, Below],
    Placed[{}, Above]},
  ChartLegends → Placed[{"Expt.", "γfrag"}, Top],
  ChartStyle → {Black, Red}, AxesLabel → {"", "Ỹ(ω)",
  AxesStyle → {{Arrowheads[Automatic], AbsoluteThickness[0.6]},
    {Arrowheads[Automatic], AbsoluteThickness[0.6]}},
  LabelStyle → {FontFamily → "Arial"},
  PlotLabel → {damp, optGaFra / gammaFrag,
    (iynorm[[2 ;; 8]] - normOleg4).Table[i, {i, 1, 7}]]]
```

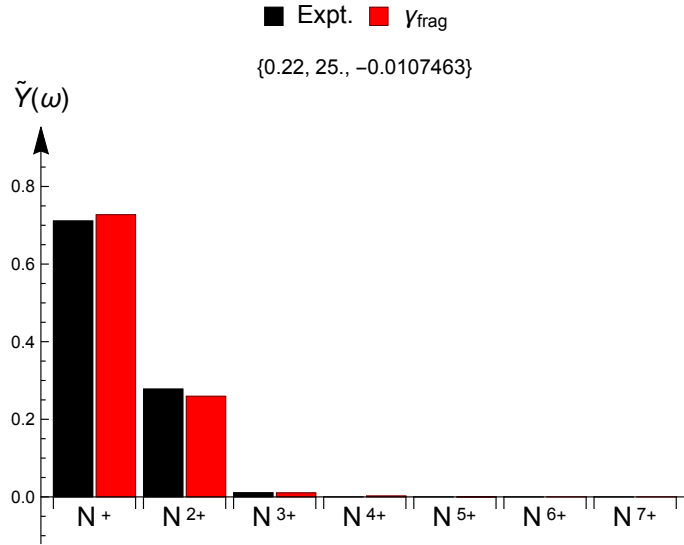

## 0.23

damp := 0.23

```
iy = dsionyieldcrateranalysisparam[damp * 0.15 * MilliJouleToHartree, photonenergy,
  tauX, nintdata, True, True, 1 / 1000, optfNppN, 1 - optfNppN, optGaFra]
```

```
iynorm = 1 / Total[iy[[2 ;; 8]]] * iy
```

```
Total[iynorm[[2 ;; 8]]]
```

```
{0.983106, 0.0122021, 0.00444895, 0.000192823, 0.0000458109, 3.85567 × 10-6,
  2.07243 × 10-8, 1.84719 × 10-11, 0.981055, 0.000385, 5.81955 × 10-113, 5.95021 × 10-259}
```

```
{58.1943, 0.722292, 0.263353, 0.011414, 0.00271174, 0.000228234, 1.22676 × 10-6,
  1.09343 × 10-9, 58.0729, 0.0227898, 3.44484 × 10-111, 3.52219 × 10-257}
```

1.

```
plotiy = Partition[Riffle[normOleg4, iynorm[[2 ;; 8]]], 2]
```

```
{{0.711226, 0.722292}, {0.277966, 0.263353}, {0.0108078, 0.011414},
  {0., 0.00271174}, {0., 0.000228234}, {0., 1.22676 × 10-6}, {0., 1.09343 × 10-9}}
```

```
BarChart[plotiy, PlotRange → {-0.1, 0.9},
  ChartLabels → {Placed[{"N +", "N 2+", "N 3+", "N 4+", "N 5+", "N 6+", "N 7+"}, Below],
    Placed[{}, Above]},
  ChartLegends → Placed[{"Expt.", "γfrag"}, Top],
  ChartStyle → {Black, Red}, AxesLabel → {"", "Ỹ(ω)"},
  AxesStyle → {{Arrowheads[Automatic], AbsoluteThickness[0.6]},
    {Arrowheads[Automatic], AbsoluteThickness[0.6]}},
  LabelStyle → {FontFamily → "Arial"},
  PlotLabel → {damp, optGaFra / gammaFrag,
    (iynorm[[2 ;; 8]] - normOleg4).Table[i, {i, 1, 7}]]]
```

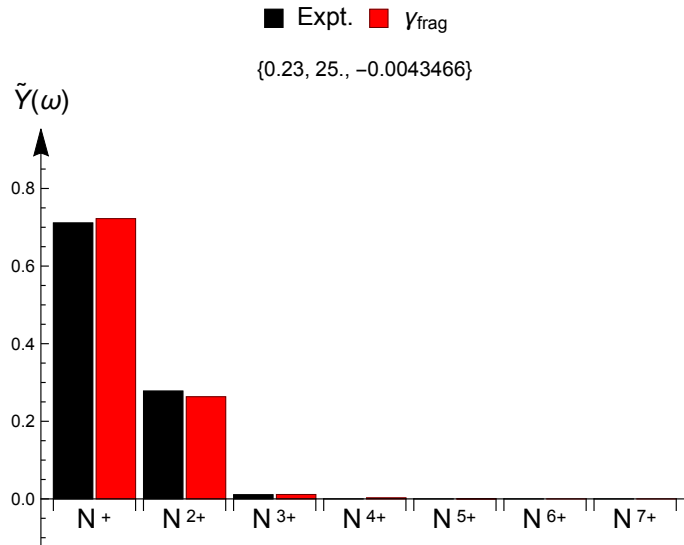

## 0.24

damp := 0.24

```
iy = dsionyieldcrateranalysisparam[damp * 0.15 * MilliJouleToHartree, photonenergy,
  tauX, nintdata, True, True, 1 / 1000, optfNppN, 1 - optfNppN, optGaFra]
```

```
iynorm = 1 / Total[iy[[2 ;; 8]]] * iy
```

```
Total[iynorm[[2 ;; 8]]]
```

```
{0.982482, 0.0125662, 0.00467974, 0.000215368,
  0.0000516704, 4.51432 × 10-6, 2.53687 × 10-8, 2.3619 × 10-11,
  0.980371, 0.000395944, 5.40396 × 10-113, -1.25231 × 10-179}
```

```
{56.0856, 0.717351, 0.267146, 0.0122944, 0.00294963, 0.000257703, 1.44819 × 10-6,
  1.3483 × 10-9, 55.9651, 0.0226027, 3.08488 × 10-111, -7.14889 × 10-178}
```

1.

```
plotiy = Partition[Riffle[normOleg4, iynorm[[2 ;; 8]]], 2]
```

```
{{0.711226, 0.717351}, {0.277966, 0.267146}, {0.0108078, 0.0122944},
  {0., 0.00294963}, {0., 0.000257703}, {0., 1.44819 × 10-6}, {0., 1.3483 × 10-9}}
```

```
BarChart[plotiy, PlotRange → {-0.1, 0.9},
  ChartLabels → {Placed[{"N +", "N 2+", "N 3+", "N 4+", "N 5+", "N 6+", "N 7+"}, Below],
    Placed[{}, Above]},
  ChartLegends → Placed[{"Expt.", "γfrag"}, Top],
  ChartStyle → {Black, Red}, AxesLabel → {"", "Ỹ(ω)",
  AxesStyle → {{Arrowheads[Automatic], AbsoluteThickness[0.6]},
    {Arrowheads[Automatic], AbsoluteThickness[0.6]}},
  LabelStyle → {FontFamily → "Arial"},
  PlotLabel → {damp, optGaFra / gammaFrag,
    (iynorm[[2 ;; 8]] - normOleg4).Table[i, {i, 1, 7}]]]
```

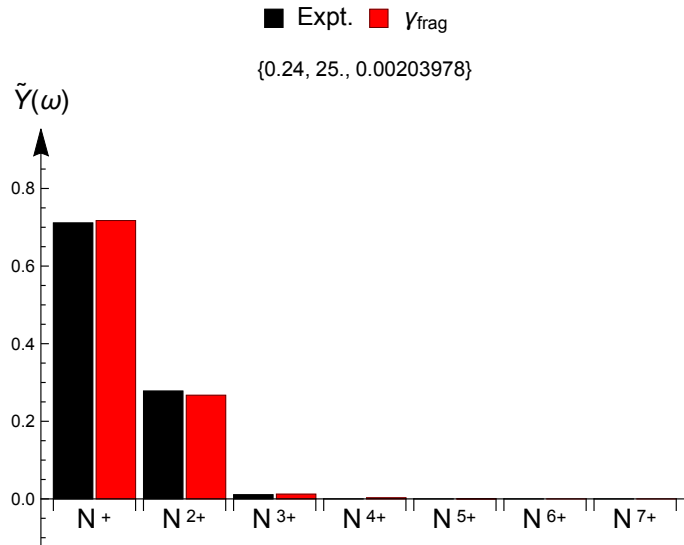

## 0.25

damp := 0.25

```
iy = dsionyieldcrateranalysisparam[damp * 0.15 * MilliJouleToHartree, photonenergy,
  tauX, nintdata, True, True, 1 / 1000, optfNppN, 1 - optfNppN, optGaFra]
```

```
iynorm = 1 / Total[iy[[2 ;; 8]]] * iy
```

```
Total[iynorm[[2 ;; 8]]]
```

```
{0.981866, 0.0129197, 0.00491138, 0.000239312,
  0.0000579751, 5.24925 × 10-6, 3.07876 × 10-8, 2.98898 × 10-11,
  0.979696, 0.000406526, 9.03745 × 10-113, 1.2066 × 10-174}
```

```
{54.1461, 0.712471, 0.270843, 0.0131971, 0.0031971, 0.000289475, 1.69781 × 10-6,
  1.64831 × 10-9, 54.0264, 0.0224183, 4.9838 × 10-111, 6.65392 × 10-173}
```

1.

```
plotiy = Partition[Riffle[normOleg4, iynorm[[2 ;; 8]]], 2]
```

```
{{0.711226, 0.712471}, {0.277966, 0.270843}, {0.0108078, 0.0131971},
  {0., 0.0031971}, {0., 0.000289475}, {0., 1.69781 × 10-6}, {0., 1.64831 × 10-9}}
```

```
BarChart[plotiy, PlotRange → {-0.1, 0.9},
  ChartLabels → {Placed[{"N +", "N 2+", "N 3+", "N 4+", "N 5+", "N 6+", "N 7+"}, Below],
    Placed[{}, Above]},
  ChartLegends → Placed[{"Expt.", "γfrag"}, Top],
  ChartStyle → {Black, Red}, AxesLabel → {"", "Ỹ(ω)"},
  AxesStyle → {{Arrowheads[Automatic], AbsoluteThickness[0.6]},
    {Arrowheads[Automatic], AbsoluteThickness[0.6]}},
  LabelStyle → {FontFamily → "Arial"},
  PlotLabel → {damp, optGaFra / gammaFrag,
    (iynorm[[2 ;; 8]] - normOleg4).Table[i, {i, 1, 7}]]]
```

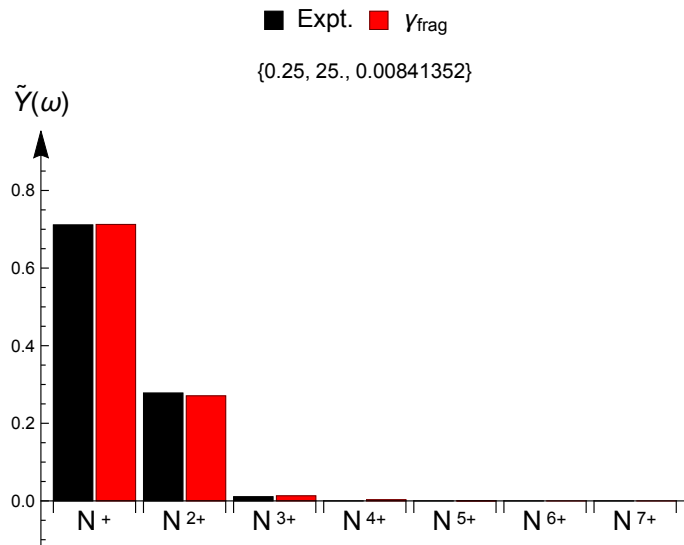

## References

- [1] S. Düsterer, P. Radcliffe, C. Bostedt, J. Bozek, A. L. Cavalieri, R. Coffee, J. T. Costello, D. Cubaynes, L. F. DiMauro, Y. Ding, G. Doumy, F. Grüner, W. Helml, W. Schweinberger, R. Kienberger, A. R. Maier, M. Messerschmidt, V. Richardson, C. Roedig, T. Tschentscher, M. Meyer, *New J. Phys.* **13**, 093024 (2011) [11 pages], *Femtosecond x-ray pulse length characterization at the Linac Coherent Light Source free-electron laser*, <http://dx.doi.org/10.1088/1367-2630/13/9/093024>
