# Supplementary material for: Rate equations for nitrogen molecules in ultrashort and intense x-ray pulses
Source: arXiv:1508.05223 ancillary file (2017-03-16)
Supplement: Supplementary file 9 [file nitrogen_dissociation_short_second.pdf]

```
<< PlotLegends`
```

General::obspkg: PlotLegends` is now obsolete. The legacy version being loaded may conflict with current functionality. See the Compatibility Guide for updating information.

```
Get["NitrogenRateEquations.m", Path -> NotebookDirectory[]]  
Get["NitrogenMoleculeRateEqs.m", Path -> NotebookDirectory[]]
```

```
HartreeToeV := 27.2113845  
eVToHartree := 1 / HartreeToeV  
JouleToHartree := 2.29371269*^-17  
MilliJouleToHartree := 1*^-3 * JouleToHartree  
BohrToAngstroem := 0.5291772083  
AngstroemToBohr := 1 / BohrToAngstroem  
MicrometerToBohr := 1*^4 * AngstroemToBohr  
BohrToMicrometer := 1 / MicrometerToBohr  
t0ToSecond := 24.18884326505*^-18  
t0ToFemtoSecond := 24.18884326505*^-3  
crossSectionAUtoBarn := 1*^8 * BohrToAngstroem^2  
crossSectionAUtocm2 := crossSectionAUtoBarn * 1*^-24  
crossSectioncm2toAU := 1 / crossSectionAUtocm2  
  
neginfinity := -1000 / t0ToFemtoSecond  
posinfinity := 10 000 / t0ToFemtoSecond
```

# Fragmentation time and pulse energy

Microscopic molecular rate-equation model with effective pulse duration and optimization for the N<sub>2</sub><sup>+</sup> yields

Christian Buth, 25 September 2014

Theoretische Chemie, Physikalisch-Chemisches Institut, Ruprecht-Karls-Universität Heidelberg, Im Neuenheimer Feld 229, 69120 Heidelberg, Germany

---

## Experimental parameters

Pulse energy fractions as determined in this *Mathematica* Notebook:

```
optdamp280 := 0.38  
optdamp80 := 0.30  
optdamp7 := 0.16  
optdamp4 := 0.23
```

Pulse energy fraction for the 4 fs pulse with respect to a pulse energy of 0.26 mJ instead of 0.15 mJ and vice versa for the 7 fs pulse:

```
optdamp4 * 0.15 / 0.26  
0.132692  
  
optdamp7 * 0.26 / 0.15  
0.277333
```

Pulse duration fractions. See Ref. [1] for measurements of LCLS pulse durations:

```
280 / 300 * 120
```

```
112
```

```
shtdur280 = 112 / 280.0
```

```
0.4
```

```
shtdur80 = 40 / 80.0
```

```
0.5
```

```
shtdur7 := 0.4
```

```
shtdur4 := 0.4
```

```
photonenergy := 1100 * eVToHartree
```

```
optfNppN := 0.26
```

```
newMatthias280 := {204.331, 105.281, 27.561, 13.151, 9.881, 0.587, 0.000}
```

```
normOleg280 = 1 / Total[newMatthias280] * newMatthias280
```

```
{0.56634, 0.291805, 0.0763903, 0.0364504, 0.027387, 0.00162698, 0.}
```

```
newMatthias80 := {218.068, 103.774, 26.075, 9.804, 3.315, 0.000, 0.000}
```

```
normOleg80 = 1 / Total[newMatthias80] * newMatthias80
```

```
{0.604006, 0.287434, 0.0722227, 0.0271552, 0.00918191, 0., 0.}
```

```
newMatthias7 := {221.485, 87.888, 9.342, 0.085, 0.000, 0.000, 0.000}
```

```
normOleg7 = 1 / Total[newMatthias7] * newMatthias7
```

```
{0.694746, 0.275684, 0.0293036, 0.000266625, 0., 0., 0.}
```

```
newMatthias4 := {92.985, 36.341, 1.413, 0, 0, 0, 0}
```

```
normOleg4 = 1 / Total[newMatthias4] * newMatthias4
```

```
{0.711226, 0.277966, 0.0108078, 0., 0., 0., 0.}
```

---

## Molecular fragmentation rate and pulse energy for a 280 fs pulse

```
tauX := shtdur280 * 280 / t0ToFemtoSecond
```

```
normfitconsts[damp_?NumericQ, gaFra_?NumericQ] := Module[{olegiy, olegiynorm},
  olegiy =
    dsionyieldcrateranalysisparam[damp * 0.26 * MilliJouleToHartree, photonenergy,
      tauX, nintdata, True, True, 1 / 1000, optfNppN, 1 - optfNppN, gaFra];
  olegiynorm = 1 / Total[olegiy[[2 ;; 8]]] * olegiy[[2 ;; 8]];
  Norm[(olegiynorm - normOleg280) * Table[{i, {i, 1, 7}}, 1] +
    16 * Abs[olegiynorm[[2]] - normOleg280[[2]]]
]
```

0.36

```
damp := 0.36
```

```

tabgamma =
  Table[{gaFra, normfitconsts[damp, gaFra * gammaFrag]}, {gaFra, 6, 16, 1 / 2}];

ListPlot[tabgamma, Joined -> True,
  PlotMarkers -> Automatic, PlotStyle -> {Thick, Red}]

```

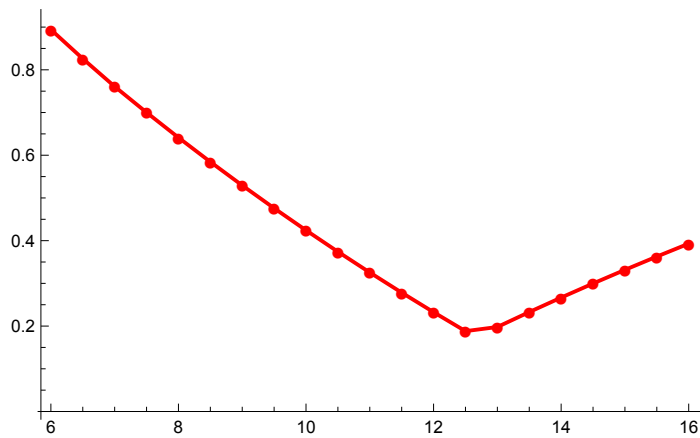

```

tabgamma = Table[
  {gaFra, normfitconsts[damp, gaFra * gammaFrag]}, {gaFra, 11.5, 13.5, 1 / 5}];

ListPlot[tabgamma, Joined -> True,
  PlotMarkers -> Automatic, PlotStyle -> {Thick, Red}]

```

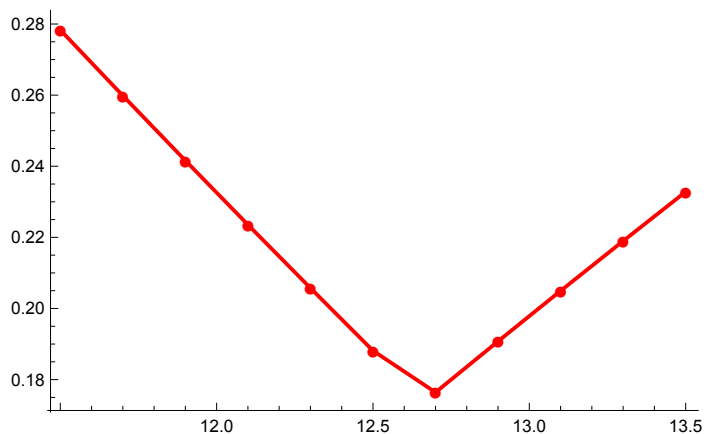

```

N[MinimalBy[tabgamma, Last]]
{{12.7, 0.176411}}

```

```

intgamma = Interpolation[tabgamma, x]

```

```

InterpolatingFunction[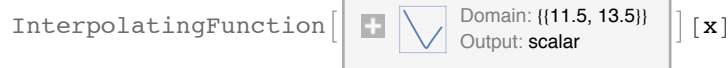 Domain: {{11.5, 13.5}}  
Output: scalar][x]

```

```

mingamma = FindMinimum[intgamma, {x, 11.5, 13.5}]

```

InterpolatingFunction::dmval:

Input value {13.7642} lies outside the range of data in the interpolating function. Extrapolation will be used. >>

```

{0.176411, {x -> 12.7}}

```

```

optent = x /. mingamma[[2]]

```

```

12.7

```

```

optGaFra := optent * gammaFrag

```

```

iy = dsionyieldcrateranalysisparam[damp * 0.26 * MilliJouleToHartree, photonenergy,
  tauX, nintdata, True, True, 1 / 1000, optfNppN, 1 - optfNppN, optGaFra]
iynorm = 1 / Total[iy[[2 ;; 8]]] * iy
Total[iynorm[[2 ;; 8]]]
{0.963462, 0.021248, 0.0106563, 0.0020876, 0.00179569, 0.000666769, 0.0000799583,
  4.05917 × 10-6, 0.959918, 0.000628799, 1.31526 × 10-57, -2.05435 × 10-116}

{26.3685, 0.581525, 0.291647, 0.0571344, 0.0491453, 0.0182485, 0.00218834,
  0.000111093, 26.2715, 0.0172093, 3.59966 × 10-56, -5.62244 × 10-115}

1.

```

```

plotiy = Partition[Riffle[normOleg280, iynorm[[2 ;; 8]]], 2]
{{0.56634, 0.581525}, {0.291805, 0.291647},
 {0.0763903, 0.0571344}, {0.0364504, 0.0491453},
 {0.027387, 0.0182485}, {0.00162698, 0.00218834}, {0., 0.000111093}}

BarChart[plotiy, PlotRange → {-0.1, 0.9},
  ChartLabels → {Placed[{"N +", "N 2+", "N 3+", "N 4+", "N 5+", "N 6+", "N 7+"}, Below],
    Placed[{}, Above]},
  ChartLegends → Placed[{"Expt.", "γfrag"}, Top],
  ChartStyle → {Black, Red}, AxesLabel → {"", "Ỹ(ω)"},
  AxesStyle → {{Arrowheads[Automatic], AbsoluteThickness[0.6]},
    {Arrowheads[Automatic], AbsoluteThickness[0.6]}},
  LabelStyle → {FontFamily → "Arial"},
  PlotLabel → {damp, optGaFra / gammaFrag,
    (iynorm[[2 ;; 8]] - normOleg280).Table[i, {i, 1, 7}]}]

```

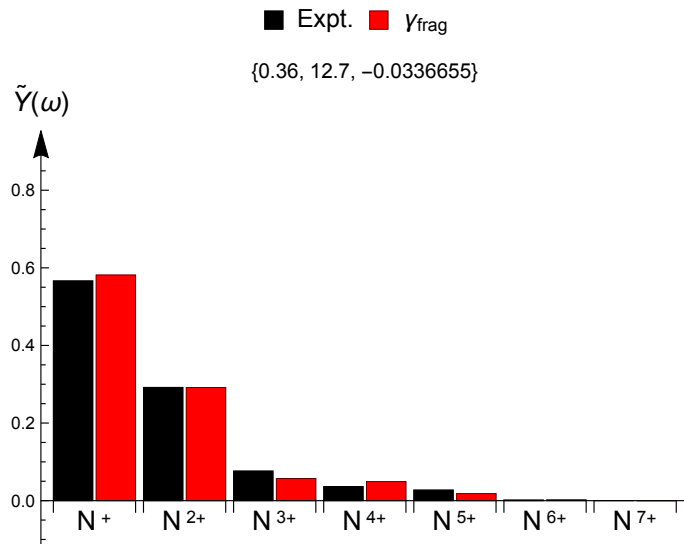

## 0.37

```

damp := 0.37

tabgamma =
  Table[{gaFra, normfitconsts[damp, gaFra * gammaFrag]}, {gaFra, 8, 18, 1 / 2}];

```

```
ListPlot[tabgamma, Joined -> True,
  PlotMarkers -> Automatic, PlotStyle -> {Thick, Red}]
```

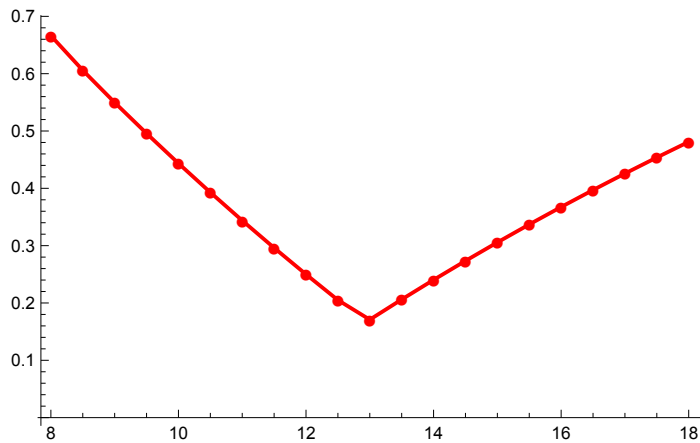

```
tabgamma =
  Table[{gaFra, normfitconsts[damp, gaFra * gammaFrag]}, {gaFra, 12, 14, 1/5}];
```

```
ListPlot[tabgamma, Joined -> True,
  PlotMarkers -> Automatic, PlotStyle -> {Thick, Red}]
```

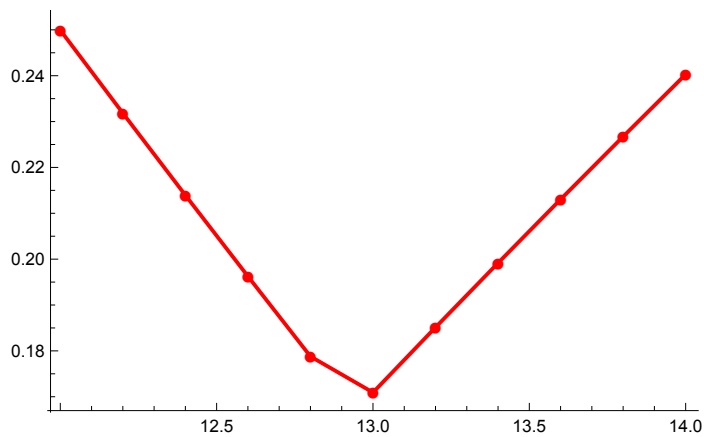

```
N[MinimalBy[tabgamma, Last]]
```

```
{{13., 0.170926}}
```

```
intgamma = Interpolation[tabgamma, x]
```

```
InterpolatingFunction[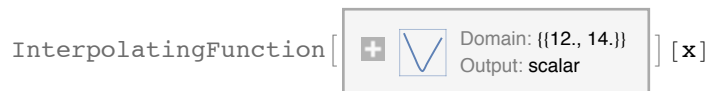 Domain: {{12., 14.}}  
Output: scalar] [x]
```

```
mingamma = FindMinimum[intgamma, {x, 12.0, 14.0}]
```

```
InterpolatingFunction::dmval:
```

```
Input value {14.2642} lies outside the range of data in the interpolating function. Extrapolation will be used. >>
```

```
{0.170899, {x -> 12.9899}}
```

```
optent = x /. mingamma[[2]]
```

```
12.9899
```

```
optGaFra := optent * gammaFrag
```

```

iy = dsionyieldcrateranalysisparam[damp * 0.26 * MilliJouleToHartree, photonenergy,
  tauX, nintdata, True, True, 1 / 1000, optfNppN, 1 - optfNppN, optGaFra]
iynorm = 1 / Total[iy[[2 ;; 8]]] * iy
Total[iynorm[[2 ;; 8]]]
{0.962782, 0.0214797, 0.0108522, 0.00218686, 0.00188584, 0.000719471,
  0.0000888846,  $4.645 \times 10^{-6}$ , 0.959202, 0.000633826,  $7.37654 \times 10^{-59}$ ,  $-5.43931 \times 10^{-116}$ }

{25.869, 0.577138, 0.291588, 0.0587586, 0.0506707, 0.0193315, 0.00238824,
  0.000124806, 25.7728, 0.0170303,  $1.982 \times 10^{-57}$ ,  $-1.46149 \times 10^{-114}$ }

1.

```

```

plotiy = Partition[Riffle[normOleg280, iynorm[[2 ;; 8]]], 2]
{{0.56634, 0.577138}, {0.291805, 0.291588},
 {0.0763903, 0.0587586}, {0.0364504, 0.0506707},
 {0.027387, 0.0193315}, {0.00162698, 0.00238824}, {0., 0.000124806}}

BarChart[plotiy, PlotRange → {-0.1, 0.9},
  ChartLabels → {Placed[{"N +", "N 2+", "N 3+", "N 4+", "N 5+", "N 6+", "N 7+"}, Below],
    Placed[{}, Above]},
  ChartLegends → Placed[{"Expt.", "γfrag"}, Top],
  ChartStyle → {Black, Red}, AxesLabel → {"", "Ỹ(ω)"},
  AxesStyle → {{Arrowheads[Automatic], AbsoluteThickness[0.6]},
    {Arrowheads[Automatic], AbsoluteThickness[0.6]}},
  LabelStyle → {FontFamily → "Arial"},
  PlotLabel → {damp, optGaFra / gammaFrag,
    (iynorm[[2 ;; 8]] - normOleg280).Table[i, {i, 1, 7}]]}

```

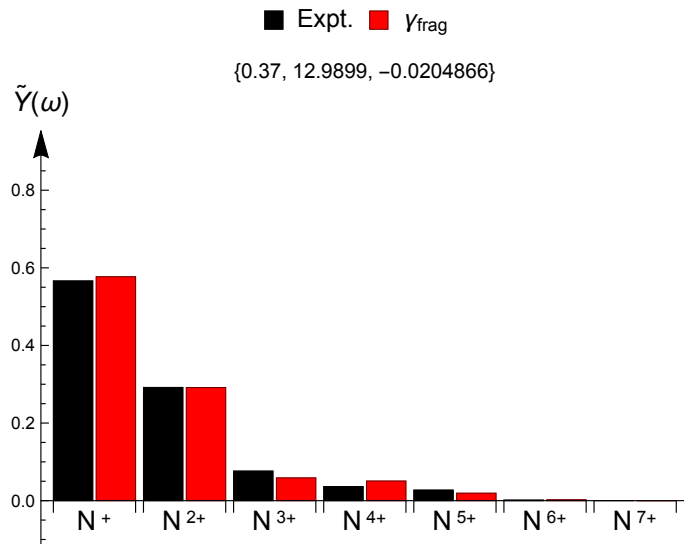

## 0.38

```

damp := 0.38

tabgamma =
  Table[{gaFra, normfitconsts[damp, gaFra * gammaFrag]}, {gaFra, 8, 18, 1 / 2}];

```

```
ListPlot[tabgamma, Joined -> True,
  PlotMarkers -> Automatic, PlotStyle -> {Thick, Red}]
```

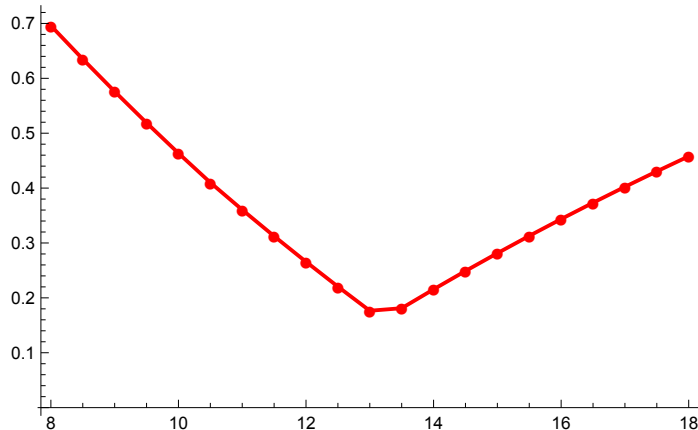

```
tabgamma =
  Table[{gaFra, normfitconsts[damp, gaFra * gammaFrag]}, {gaFra, 12, 14, 1 / 5}];
```

```
ListPlot[tabgamma, Joined -> True,
  PlotMarkers -> Automatic, PlotStyle -> {Thick, Red}]
```

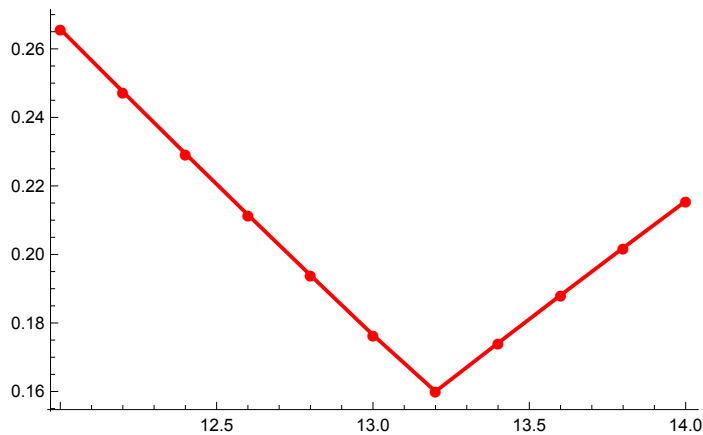

```
N[MinimalBy[tabgamma, Last]]
```

```
{{13.2, 0.160004}}
```

```
intgamma = Interpolation[tabgamma, x]
```

```
InterpolatingFunction[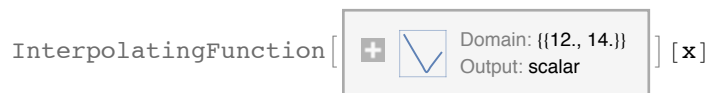 Domain: {{12., 14.}}  
Output: scalar][x]
```

```
mingamma = FindMinimum[intgamma, {x, 12.0, 14.0}]
```

```
InterpolatingFunction::dmval:
```

```
Input value {14.2642} lies outside the range of data in the interpolating function. Extrapolation will be used. >>
```

```
{0.160004, {x -> 13.2}}
```

```
optent = x /. mingamma[[2]]
```

```
13.2
```

```
optGaFra := optent * gammaFrag
```

```

iy = dsionyieldcrateranalysisparam[damp * 0.26 * MilliJouleToHartree, photonenergy,
  tauX, nintdata, True, True, 1 / 1000, optfNppN, 1 - optfNppN, optGaFra]
iynorm = 1 / Total[iy[[2 ;; 8]]] * iy
Total[iynorm[[2 ;; 8]]]

```

```

{0.962114, 0.0216966, 0.0110545, 0.00228013,
 0.00197778, 0.000773247, 0.0000983146, 5.27966 × 10-6,
 0.958498, 0.000638571, 9.10316 × 10-60, -1.69363 × 10-112}

```

```

{25.3951, 0.572683, 0.291785, 0.0601843, 0.0522036, 0.0204099, 0.00259502,
 0.000139357, 25.2996, 0.0168551, 2.40278 × 10-58, -4.47035 × 10-111}

```

1.

```

plotiy = Partition[Riffle[normOleg280, iynorm[[2 ;; 8]]], 2]

```

```

{{0.56634, 0.572683}, {0.291805, 0.291785},
 {0.0763903, 0.0601843}, {0.0364504, 0.0522036},
 {0.027387, 0.0204099}, {0.00162698, 0.00259502}, {0., 0.000139357}}

```

```

BarChart[plotiy, PlotRange → {-0.1, 0.9},
  ChartLabels → {Placed[{"N +", "N 2+", "N 3+", "N 4+", "N 5+", "N 6+", "N 7+"}, Below],
    Placed[{}, Above]},
  ChartLegends → Placed[{"Expt.", "γfrag"}, Top],
  ChartStyle → {Black, Red}, AxesLabel → {"", "Ỹ(ω)"},
  AxesStyle → {{Arrowheads[Automatic], AbsoluteThickness[0.6]},
    {Arrowheads[Automatic], AbsoluteThickness[0.6]}},
  LabelStyle → {FontFamily → "Arial"},
  PlotLabel → {damp, optGaFra / gammaFrag,
    (iynorm[[2 ;; 8]] - normOleg280).Table[i, {i, 1, 7}]}]

```

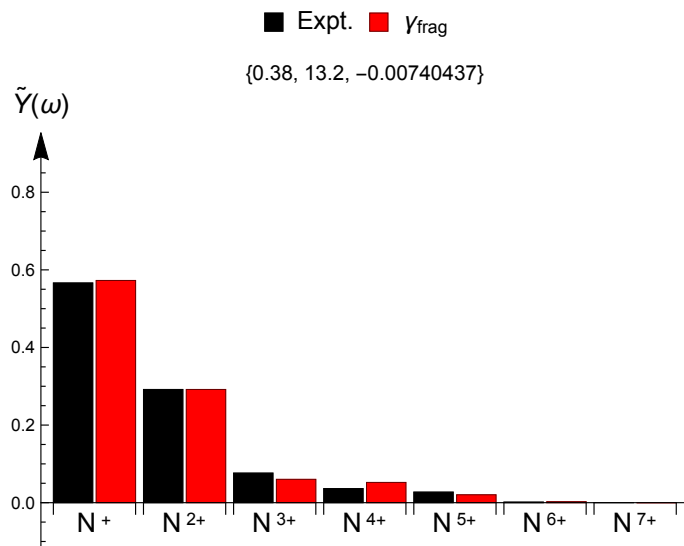

## 0.39

```

damp := 0.39

```

```

tabgamma =
  Table[{gaFra, normfitconsts[damp, gaFra * gammaFrag]}, {gaFra, 8, 18, 1 / 2}];

```



```
ListPlot[tabgamma, Joined -> True,
PlotMarkers -> Automatic, PlotStyle -> {Thick, Red}]
```

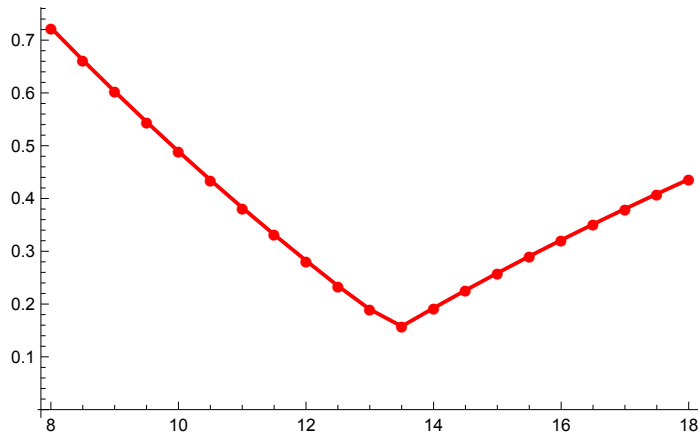

```
tabgamma = Table[
{gaFra, normfitconsts[damp, gaFra * gammaFrag]}, {gaFra, 12.5, 14.5, 1/5}];
```

```
ListPlot[tabgamma, Joined -> True,
PlotMarkers -> Automatic, PlotStyle -> {Thick, Red}]
```

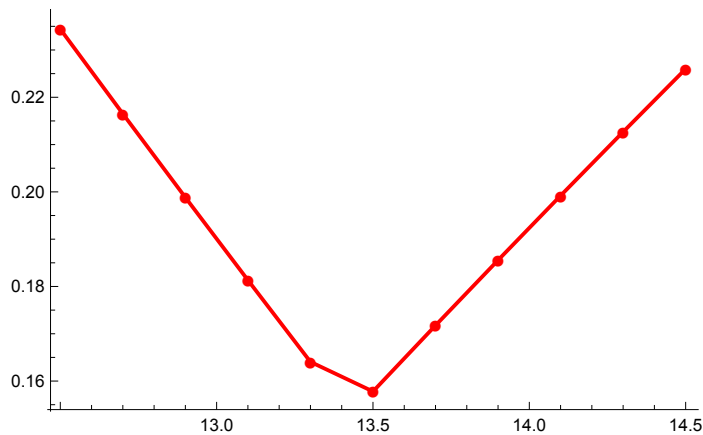

```
N[MinimalBy[tabgamma, Last]]
```

```
{{13.5, 0.157796}}
```

```
intgamma = Interpolation[tabgamma, x]
```

InterpolatingFunction[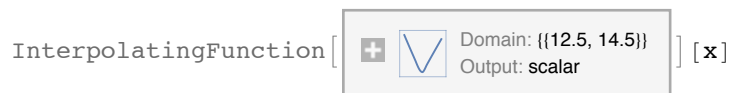 Domain: {{12.5, 14.5}}  
Output: scalar][x]

```
mingamma = FindMinimum[intgamma, {x, 12.5, 14.5}]
```

```
InterpolatingFunction::dmval:
```

```
Input value {14.7642} lies outside the range of data in the interpolating function. Extrapolation will be used. >>
```

```
{0.157661, {x -> 13.4765}}
```

```
optent = x /. mingamma[[2]]
```

```
13.4765
```

```
optGaFra := optent * gammaFrag
```

```

iy = dsionyieldcrateranalysisparam[damp * 0.26 * MilliJouleToHartree, photonenergy,
  tauX, nintdata, True, True, 1 / 1000, optfNppN, 1 - optfNppN, optGaFra]
iynorm = 1 / Total[iy[[2 ;; 8]]] * iy
Total[iynorm[[2 ;; 8]]]

{0.961459, 0.0219096, 0.0112389, 0.00237923, 0.00206929, 0.000829884, 0.000108541,
  5.99102 × 10-6, 0.957808, 0.00064305, 2.85332 × 10-52, 6.63507 × 10-97}

{24.9461, 0.568468, 0.291606, 0.0617317, 0.0536899, 0.0215322, 0.00281621,
  0.000155443, 24.8514, 0.0166846, 7.40325 × 10-51, 1.72154 × 10-95}

1.

```

```

plotiy = Partition[Riffle[normOleg280, iynorm[[2 ;; 8]]], 2]
{{0.56634, 0.568468}, {0.291805, 0.291606},
 {0.0763903, 0.0617317}, {0.0364504, 0.0536899},
 {0.027387, 0.0215322}, {0.00162698, 0.00281621}, {0., 0.000155443}}

BarChart[plotiy, PlotRange → {-0.1, 0.9},
  ChartLabels → {Placed[{"N+", "N2+", "N3+", "N4+", "N5+", "N6+", "N7+"}, Below],
    Placed[{}, Above]},
  ChartLegends → Placed[{"Expt.", "γfrag"}, Top],
  ChartStyle → {Black, Red}, AxesLabel → {"", "Ỹ(ω)"},
  AxesStyle → {{Arrowheads[Automatic], AbsoluteThickness[0.6]},
    {Arrowheads[Automatic], AbsoluteThickness[0.6]}},
  LabelStyle → {FontFamily → "Arial"},
  PlotLabel → {damp, optGaFra / gammaFrag,
    (iynorm[[2 ;; 8]] - normOleg280).Table[i, {i, 1, 7}]}]

```

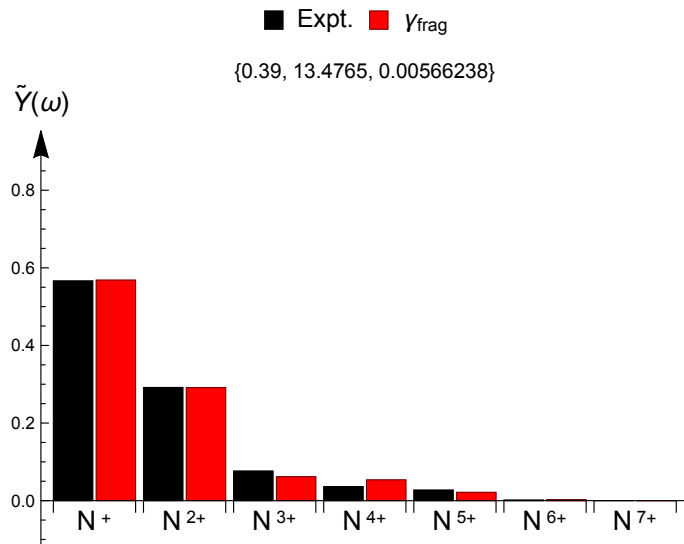

0.40

```
damp := 0.40
```

```
tabgamma =
```

```
Table[{gaFra, normfitconsts[damp, gaFra * gammaFrag]}, {gaFra, 10, 20, 1 / 2}];
```

```
ListPlot[tabgamma, Joined -> True,
PlotMarkers -> Automatic, PlotStyle -> {Thick, Red}]
```

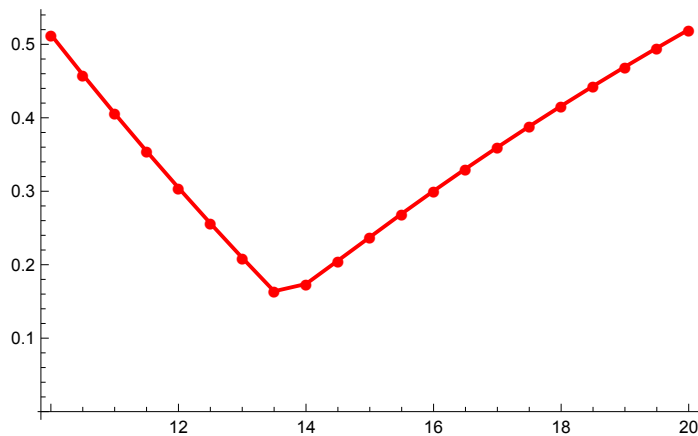

```
tabgamma = Table[
{gaFra, normfitconsts[damp, gaFra * gammaFrag]}, {gaFra, 12.5, 14.5, 1/5}];
```

```
ListPlot[tabgamma, Joined -> True,
PlotMarkers -> Automatic, PlotStyle -> {Thick, Red}]
```

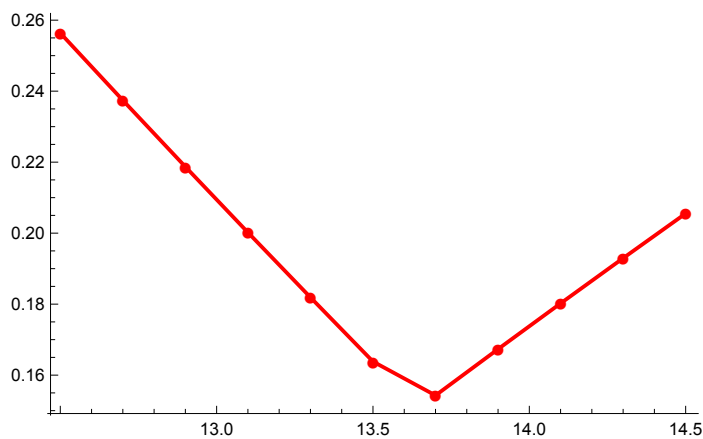

```
N[MinimalBy[tabgamma, Last]]
```

```
{{13.7, 0.154288}}
```

```
intgamma = Interpolation[tabgamma, x]
```

```
InterpolatingFunction[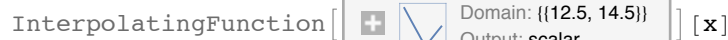 Domain: {{12.5, 14.5}}  
Output: scalar][x]
```

```
mingamma = FindMinimum[intgamma, {x, 12.5, 14.5}]
```

```
InterpolatingFunction::dmval:
```

```
Input value {14.7642} lies outside the range of data in the interpolating function. Extrapolation will be used. >>
```

```
{0.154288, {x -> 13.7}}
```

```
optent = x /. mingamma[[2]]
```

```
13.7
```

```
optGaFra := optent * gammaFrag
```

```

iy = dsionyieldcrateranalysisparam[damp * 0.26 * MilliJouleToHartree, photonenergy,
  tauX, nintdata, True, True, 1 / 1000, optfNppN, 1 - optfNppN, optGaFra]
iynorm = 1 / Total[iy[[2 ;; 8]]] * iy
Total[iynorm[[2 ;; 8]]]

{0.960814, 0.0221104, 0.0114257, 0.00247421, 0.00216208, 0.000887826, 0.000119348,
  6.76203 × 10-6, 0.957131, 0.000647275, 4.46375 × 10-62, 8.21844 × 10-114}

{24.5191, 0.564238, 0.291574, 0.0631396, 0.0551742, 0.0226565, 0.00304566,
  0.000172561, 24.4251, 0.0165179, 1.13911 × 10-60, 2.09727 × 10-112}

1.

plotiy = Partition[Riffle[normOleg280, iynorm[[2 ;; 8]]], 2]
{{0.56634, 0.564238}, {0.291805, 0.291574},
 {0.0763903, 0.0631396}, {0.0364504, 0.0551742},
 {0.027387, 0.0226565}, {0.00162698, 0.00304566}, {0., 0.000172561}}

BarChart[plotiy, PlotRange → {-0.1, 0.9},
  ChartLabels → {Placed[{"N+", "N2+", "N3+", "N4+", "N5+", "N6+", "N7+"}, Below],
    Placed[{}, Above]},
  ChartLegends → Placed[{"Expt.", "γfrag"}, Top],
  ChartStyle → {Black, Red}, AxesLabel → {"", "Ỹ(ω)"},
  AxesStyle → {{Arrowheads[Automatic], AbsoluteThickness[0.6]},
    {Arrowheads[Automatic], AbsoluteThickness[0.6]}},
  LabelStyle → {FontFamily → "Arial"},
  PlotLabel → {damp, optGaFra / gammaFrag,
    (iynorm[[2 ;; 8]] - normOleg280).Table[i, {i, 1, 7}]]}

■ Expt. ■ γfrag

{0.4, 13.7, 0.0186458}

```

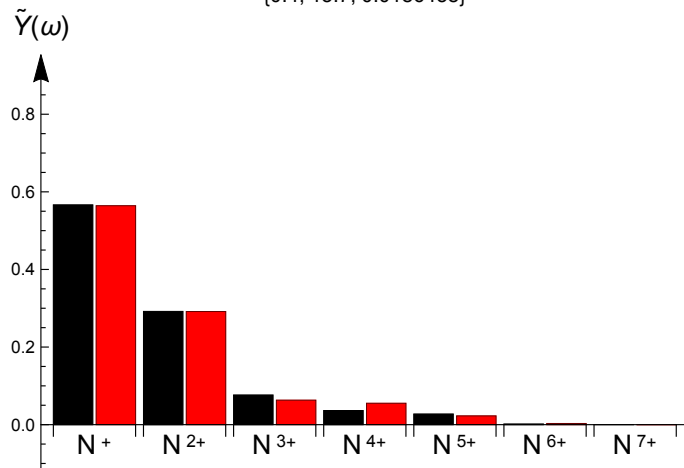

## Molecular fragmentation rate and pulse energy for a 80 fs pulse

```
tauX := shtdur80 * 80 / t0ToFemtoSecond
```

```

normfitconsts[damp_?NumericQ, gaFra_?NumericQ] := Module[{olegiy, olegiynorm},
  olegiy =
    dsionyieldcrateranalysisparam[damp * 0.26 * MilliJouleToHartree, photonenergy,
      tauX, nintdata, True, True, 1 / 1000, optfNppN, 1 - optfNppN, gaFra];
  olegiynorm = 1 / Total[olegiy[[2 ;; 8]] * olegiy[[2 ;; 8]]];
  Norm[(olegiynorm - normOleg80) * Table[i, {i, 1, 7}], 1] +
    16 * Abs[olegiynorm[[2]] - normOleg80[[2]]]
]

```

## 0.28

```
damp := 0.28
```

```

tabgamma =
  Table[{gaFra, normfitconsts[damp, gaFra * gammaFrag]}, {gaFra, 30, 40, 1 / 2}];

```

```

ListPlot[tabgamma, Joined -> True,
  PlotMarkers -> Automatic, PlotStyle -> {Thick, Red}]

```

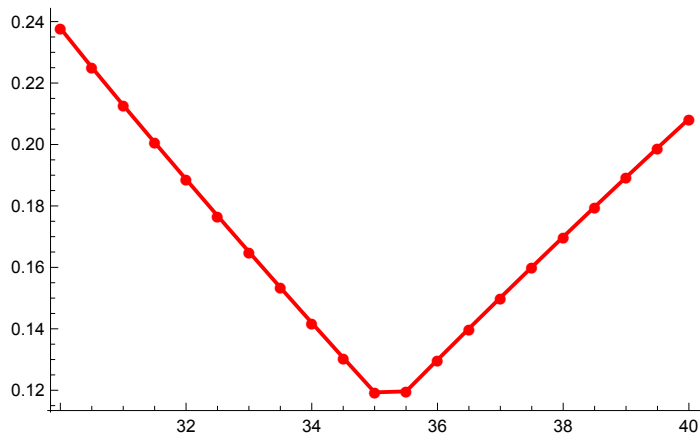

```

tabgamma =
  Table[{gaFra, normfitconsts[damp, gaFra * gammaFrag]}, {gaFra, 34, 36, 1 / 5}];

```

```

ListPlot[tabgamma, Joined -> True,
  PlotMarkers -> Automatic, PlotStyle -> {Thick, Red}]

```

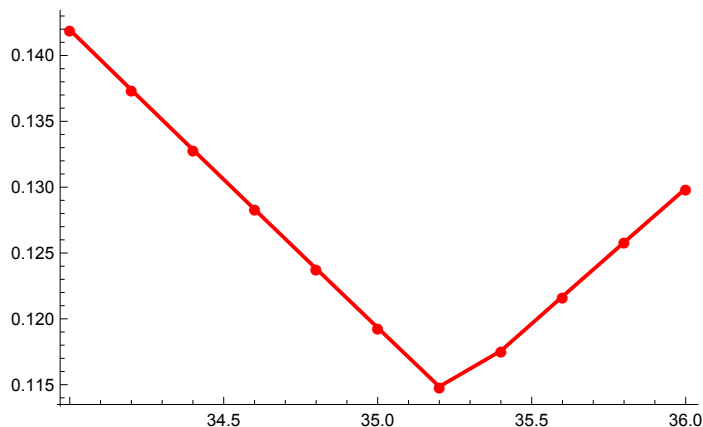

```
N[MinimalBy[tabgamma, Last]]
```

```
{{35.2, 0.114852}}
```

```
intgamma = Interpolation[tabgamma, x]
```

```
InterpolatingFunction[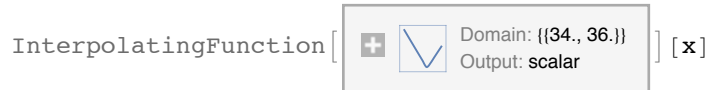 Domain: {{34., 36.}}  
Output: scalar ] [x]
```

```
mingamma = FindMinimum[intgamma, {x, 34.0, 36.0}]
```

```
InterpolatingFunction::dmval:
```

```
Input value {36.2642} lies outside the range of data in the interpolating function. Extrapolation will be used. >>
```

```
{0.114852, {x → 35.2}}
```

```
optent = x /. mingamma[[2]]
```

```
35.2
```

```
optGaFra := optent * gammaFrag
```

```
iy = dsionyieldcrateranalysisparam[damp * 0.26 * MilliJouleToHartree, photonenergy,  
tauX, nintdata, True, True, 1 / 1000, optfNppN, 1 - optfNppN, optGaFra]
```

```
iynorm = 1 / Total[iy[[2 ;; 8]]] * iy
```

```
Total[iynorm[[2 ;; 8]]]
```

```
{0.969385, 0.0190693, 0.00880114, 0.00147196,  
0.00095918, 0.000290467, 0.0000228198, 6.55974 × 10-7,  
0.966197, 0.000576154, 3.25056 × 10-72, 3.08081 × 10-113}}
```

```
{31.6632, 0.622863, 0.287474, 0.0480791, 0.0313299, 0.00948757, 0.000745369,  
0.0000214262, 31.5591, 0.018819, 1.06174 × 10-70, 1.00629 × 10-111}}
```

```
1.
```

```
plotiy = Partition[Riffle[normOleg80, iynorm[[2 ;; 8]]], 2]
```

```
{{0.604006, 0.622863}, {0.287434, 0.287474},  
{0.0722227, 0.0480791}, {0.0271552, 0.0313299},  
{0.00918191, 0.00948757}, {0., 0.000745369}, {0., 0.0000214262}}
```

```
BarChart[plotiy, PlotRange → {-0.1, 0.9},
  ChartLabels → {Placed[{"N +", "N 2+", "N 3+", "N 4+", "N 5+", "N 6+", "N 7+"}, Below],
    Placed[{}, Above]},
  ChartLegends → Placed[{"Expt.", "γfrag"}, Top],
  ChartStyle → {Black, Red}, AxesLabel → {"", "Ỹ(ω)"},
  AxesStyle → {{Arrowheads[Automatic], AbsoluteThickness[0.6]},
    {Arrowheads[Automatic], AbsoluteThickness[0.6]}},
  LabelStyle → {FontFamily → "Arial"},
  PlotLabel → {damp, optGaFra / gammaFrag,
    (iynorm[[2 ;; 8]] - normOleg80).Table[i, {i, 1, 7}]]}
```

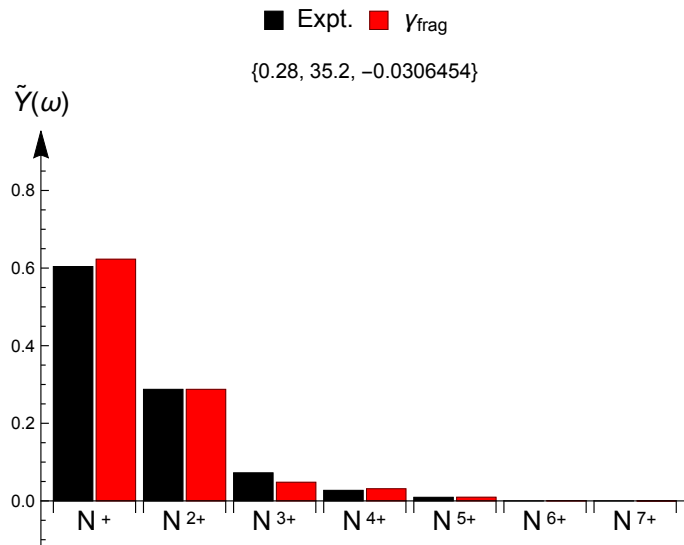

## 0.29

damp := 0.29

```
tabgamma =
  Table[{gaFra, normfitconsts[damp, gaFra * gammaFrag]}, {gaFra, 30, 40, 1 / 2}];
ListPlot[tabgamma, Joined -> True,
  PlotMarkers -> Automatic, PlotStyle -> {Thick, Red}]
```

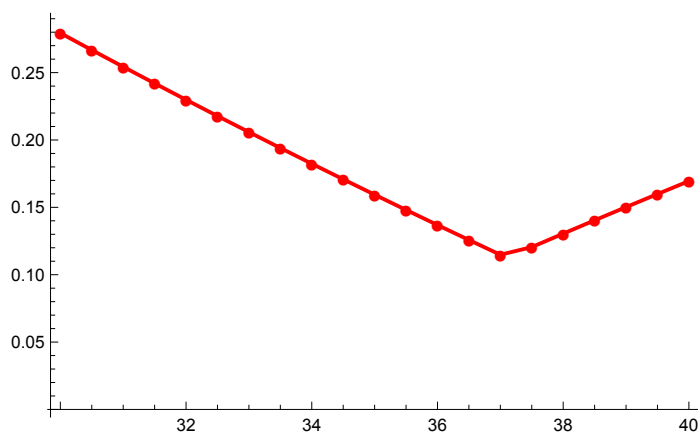

```
tabgamma =
  Table[{gaFra, normfitconsts[damp, gaFra * gammaFrag]}, {gaFra, 36, 38, 1 / 5}];
```

```
ListPlot[tabgamma, Joined -> True,
PlotMarkers -> Automatic, PlotStyle -> {Thick, Red}]
```

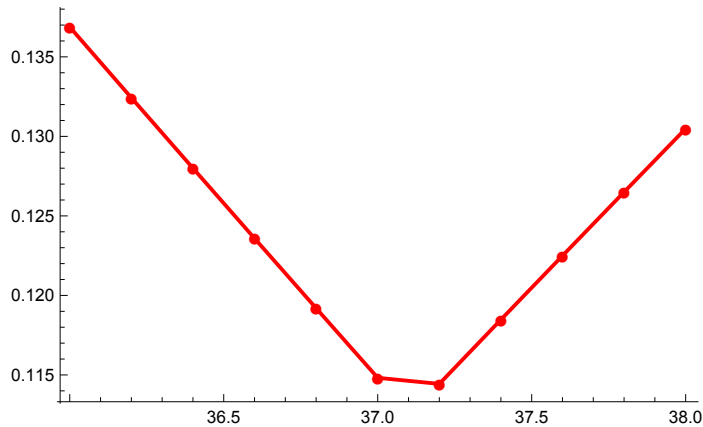

```
N[MinimalBy[tabgamma, Last]]
```

```
{{37.2, 0.114437}}
```

```
intgamma = Interpolation[tabgamma, x]
```

```
InterpolatingFunction[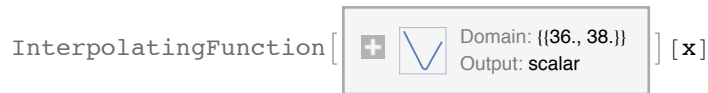 Domain: {{36., 38.}}  
Output: scalar][x]
```

```
mingamma = FindMinimum[intgamma, {x, 36.0, 38.0}]
```

```
InterpolatingFunction::dmval:
```

```
Input value {38.2642} lies outside the range of data in the interpolating function. Extrapolation will be used. >>
```

```
{0.114084, {x -> 37.1189}}
```

```
optent = x /. mingamma[[2]]
```

```
37.1189
```

```
optGaFra := optent * gammaFrag
```

```
iy = dsionyieldcrateranalysisparam[damp * 0.26 * MilliJouleToHartree, photonenergy,  
tauX, nintdata, True, True, 1 / 1000, optfNppN, 1 - optfNppN, optGaFra]
```

```
inyorm = 1 / Total[iy[[2 ;; 8]]] * iy
```

```
Total[inyorm[[2 ;; 8]]]
```

```
{0.968598, 0.0194072, 0.00902558, 0.00158805,  
0.00102953, 0.000324653, 0.0000265114, 7.92405 × 10-7,  
0.965355, 0.000584142, -8.67162 × 10-67, 2.15484 × 10-104}
```

```
{30.8448, 0.618018, 0.287418, 0.0505711, 0.0327852, 0.0103385, 0.000844251,  
0.000025234, 30.7416, 0.0186019, -2.76146 × 10-65, 6.86205 × 10-103}
```

```
1.
```

```
plotiy = Partition[Riffle[normOleg80, inyorm[[2 ;; 8]]], 2]
```

```
{{0.604006, 0.618018}, {0.287434, 0.287418},  
{0.0722227, 0.0505711}, {0.0271552, 0.0327852},  
{0.00918191, 0.0103385}, {0., 0.000844251}, {0., 0.000025234}}
```



```
BarChart[plotiy, PlotRange → {-0.1, 0.9},
  ChartLabels → {Placed[{"N +", "N 2+", "N 3+", "N 4+", "N 5+", "N 6+", "N 7+"}, Below],
    Placed[{}, Above]},
  ChartLegends → Placed[{"Expt.", "γfrag"}, Top],
  ChartStyle → {Black, Red}, AxesLabel → {"", "Ỹ(ω)"},
  AxesStyle → {{Arrowheads[Automatic], AbsoluteThickness[0.6]},
    {Arrowheads[Automatic], AbsoluteThickness[0.6]}},
  LabelStyle → {FontFamily → "Arial"},
  PlotLabel → {damp, optGaFra / gammaFrag,
    (iynorm[2 ;; 8] - normOleg80).Table[i, {i, 1, 7}]]}
```

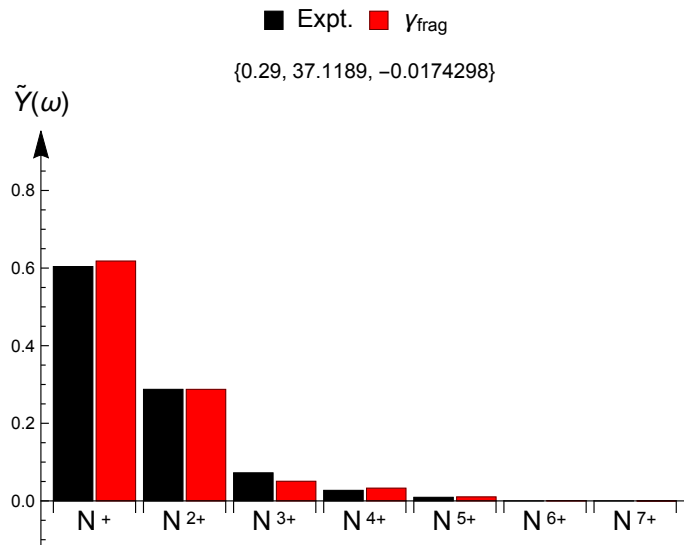

### 0.30

```
damp := 0.30
```

```
tabgamma =
  Table[{gaFra, normfitconsts[damp, gaFra * gammaFrag]}, {gaFra, 30, 50, 1 / 2}];
```

```
ListPlot[tabgamma, Joined -> True,
  PlotMarkers -> Automatic, PlotStyle -> {Thick, Red}]
```

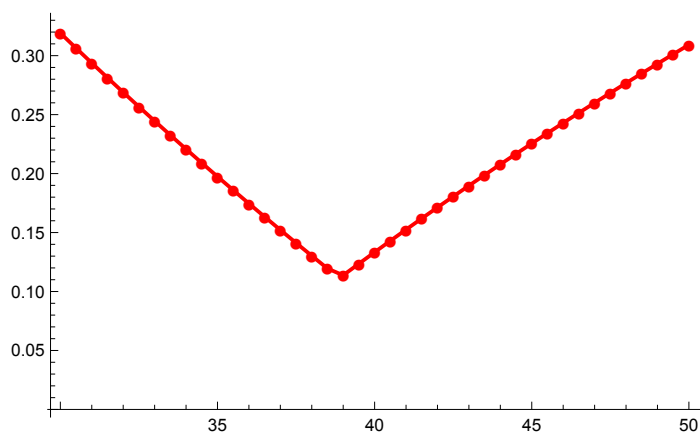

```
tabgamma =
  Table[{gaFra, normfitconsts[damp, gaFra * gammaFrag]}, {gaFra, 38, 40, 1 / 5}];
```

```
ListPlot[tabgamma, Joined -> True,
PlotMarkers -> Automatic, PlotStyle -> {Thick, Red}]
```

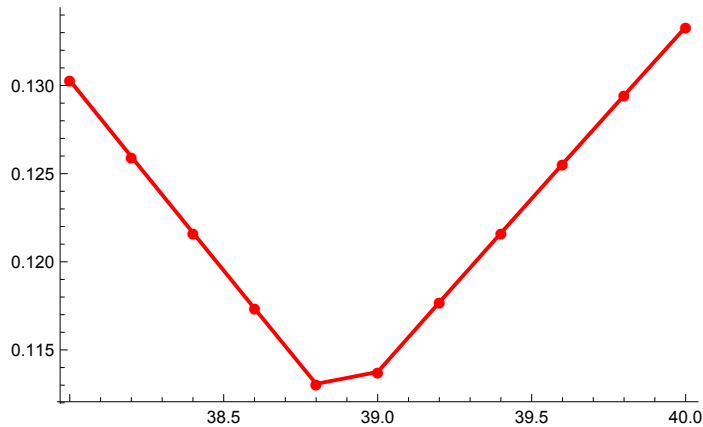

```
N[MinimalBy[tabgamma, Last]]
```

```
{{38.8, 0.113073}}
```

```
intgamma = Interpolation[tabgamma, x]
```

```
InterpolatingFunction[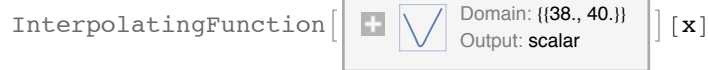 Domain: {{38., 40.}}  
Output: scalar][x]
```

```
mingamma = FindMinimum[intgamma, {x, 38.0, 40.0}]
```

```
InterpolatingFunction::dmval:
```

Input value {40.2642} lies outside the range of data in the interpolating function. Extrapolation will be used. >>

```
{0.112831, {x -> 38.865}}
```

```
optent = x /. mingamma[[2]]
```

```
38.865
```

```
optGaFra := optent * gammaFrag
```

```
iy = dsionyieldcrateranalysisparam[damp * 0.26 * MilliJouleToHartree, photonenergy,  
tauX, nintdata, True, True, 1 / 1000, optfNppN, 1 - optfNppN, optGaFra]
```

```
inyorm = 1 / Total[iy[[2 ;; 8]]] * iy
```

```
Total[inyorm[[2 ;; 8]]]
```

```
{0.967826, 0.0197289, 0.00924854, 0.00170332, 0.00110139, 0.000360656,  
0.0000305707, 9.48392 × 10-7, 0.96453, 0.000591681, 1.94366 × 10-58, 1.10512 × 10-95}}
```

```
{30.0807, 0.613188, 0.287451, 0.0529402, 0.0342319, 0.0112094, 0.000950158,  
0.0000294767, 29.9782, 0.0183898, 6.04103 × 10-57, 3.43478 × 10-94}}
```

```
1.
```

```
plotiy = Partition[Riffle[normOleg80, inyorm[[2 ;; 8]]], 2]
```

```
{{0.604006, 0.613188}, {0.287434, 0.287451},  
{0.0722227, 0.0529402}, {0.0271552, 0.0342319},  
{0.00918191, 0.0112094}, {0., 0.000950158}, {0., 0.0000294767}}
```

```
BarChart[plotiy, PlotRange → {-0.1, 0.9},
  ChartLabels → {Placed[{"N +", "N 2+", "N 3+", "N 4+", "N 5+", "N 6+", "N 7+"}, Below],
    Placed[{}, Above]},
  ChartLegends → Placed[{"Expt.", "γfrag"}, Top],
  ChartStyle → {Black, Red}, AxesLabel → {"", "Ỹ(ω)",
  AxesStyle → {{Arrowheads[Automatic], AbsoluteThickness[0.6]},
    {Arrowheads[Automatic], AbsoluteThickness[0.6]}},
  LabelStyle → {FontFamily → "Arial"},
  PlotLabel → {damp, optGaFra / gammaFrag,
    (iynorm[2 ;; 8] - normOleg80).Table[i, {i, 1, 7}]]]
```

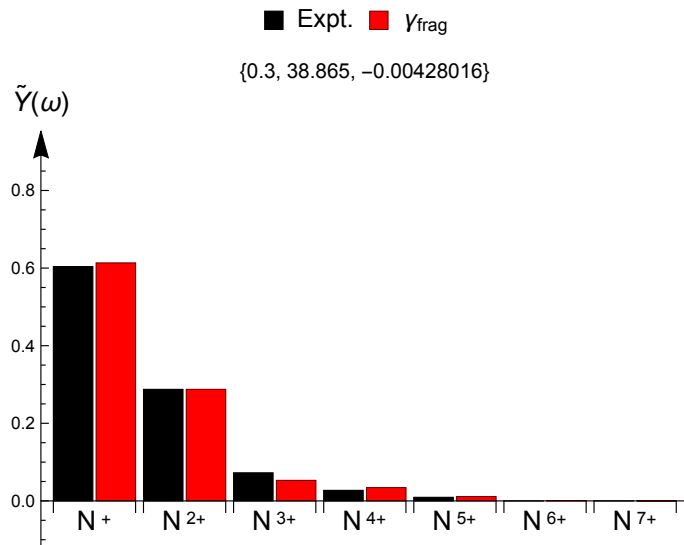

### 0.31

```
damp := 0.31
```

```
tabgamma =
  Table[{gaFra, normfitconsts[damp, gaFra * gammaFrag]}, {gaFra, 30, 50, 1 / 2}];
```

```
ListPlot[tabgamma, Joined -> True,
  PlotMarkers -> Automatic, PlotStyle -> {Thick, Red}]
```

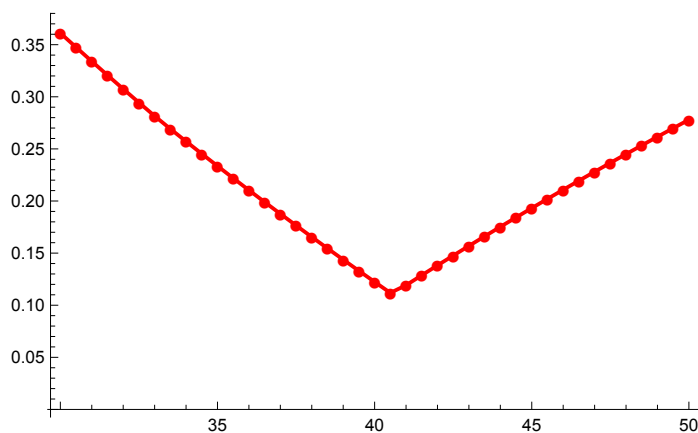

```
tabgamma = Table[
  {gaFra, normfitconsts[damp, gaFra * gammaFrag]}, {gaFra, 39.5, 41.5, 1 / 5}];
```

```
ListPlot[tabgamma, Joined -> True,
PlotMarkers -> Automatic, PlotStyle -> {Thick, Red}]
```

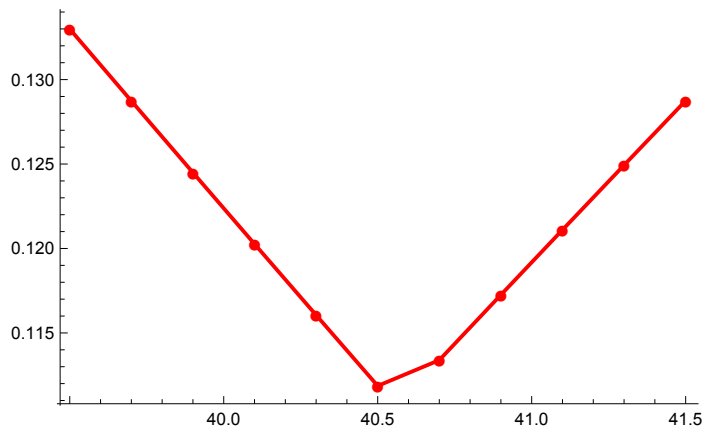

```
N[MinimalBy[tabgamma, Last]]
```

```
{{40.5, 0.111864}}
```

```
intgamma = Interpolation[tabgamma, x]
```

```
InterpolatingFunction[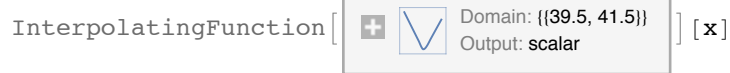 Domain: {{39.5, 41.5}}  
Output: scalar][x]
```

```
mingamma = FindMinimum[intgamma, {x, 39.5, 41.5}]
```

```
InterpolatingFunction::dmval:
```

Input value {41.7642} lies outside the range of data in the interpolating function. Extrapolation will be used. >>

```
{0.111811, {x -> 40.5281}}
```

```
optent = x /. mingamma[[2]]
```

```
40.5281
```

```
optGaFra := optent * gammaFrag
```

```
iy = dsionyieldcrateranalysisparam[damp * 0.26 * MilliJouleToHartree, photonenergy,
tauX, nintdata, True, True, 1 / 1000, optfNppN, 1 - optfNppN, optGaFra]
```

```
inyorm = 1 / Total[iy[[2 ;; 8]]] * iy
```

```
Total[inyorm[[2 ;; 8]]]
```

```
{0.967068, 0.0200366, 0.00946685, 0.00181903,
0.00117461, 0.000398636, 0.0000350314, 1.1264 × 10-6,
0.963722, 0.000598796, -6.36001 × 10-127, -2.20547 × 10-138}}
```

```
{29.3657, 0.608425, 0.287468, 0.055236, 0.035668, 0.0121049, 0.00106375,
0.000034204, 29.2641, 0.0181829, -1.93126 × 10-125, -6.69708 × 10-137}}
```

```
1.
```

```
plotiy = Partition[Riffle[normOleg80, inyorm[[2 ;; 8]]], 2]
```

```
{{0.604006, 0.608425}, {0.287434, 0.287468},
{0.0722227, 0.055236}, {0.0271552, 0.035668},
{0.00918191, 0.0121049}, {0., 0.00106375}, {0., 0.000034204}}
```

```
BarChart[plotiy, PlotRange → {-0.1, 0.9},
  ChartLabels → {Placed[{"N +", "N 2+", "N 3+", "N 4+", "N 5+", "N 6+", "N 7+"}, Below],
    Placed[{}, Above]},
  ChartLegends → Placed[{"Expt.", "γfrag"}, Top],
  ChartStyle → {Black, Red}, AxesLabel → {"", "Ỹ(ω)",
  AxesStyle → {{Arrowheads[Automatic], AbsoluteThickness[0.6]},
    {Arrowheads[Automatic], AbsoluteThickness[0.6]}},
  LabelStyle → {FontFamily → "Arial"},
  PlotLabel → {damp, optGaFra / gammaFrag,
    (iynorm[2 ;; 8] - normOleg80).Table[i, {i, 1, 7}]]]
```

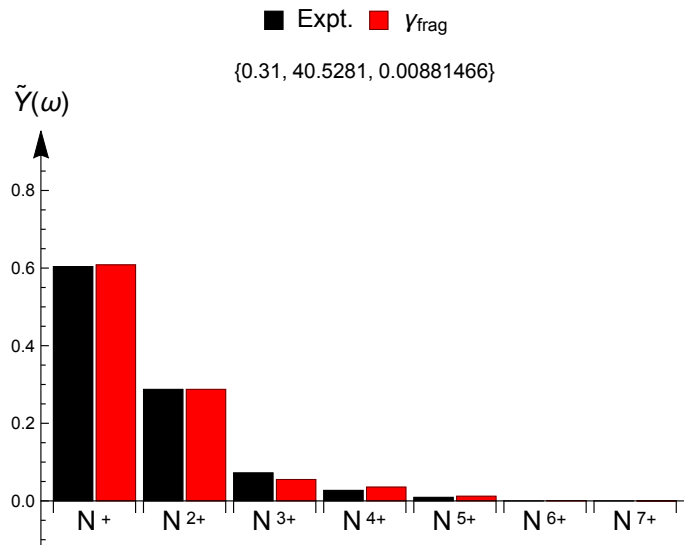

## 0.32

```
damp := 0.32
```

```
tabgamma =
  Table[{gaFra, normfitconsts[damp, gaFra * gammaFrag]}, {gaFra, 35, 55, 1 / 2}];
```

```
ListPlot[tabgamma, Joined -> True,
  PlotMarkers -> Automatic, PlotStyle -> {Thick, Red}]
```

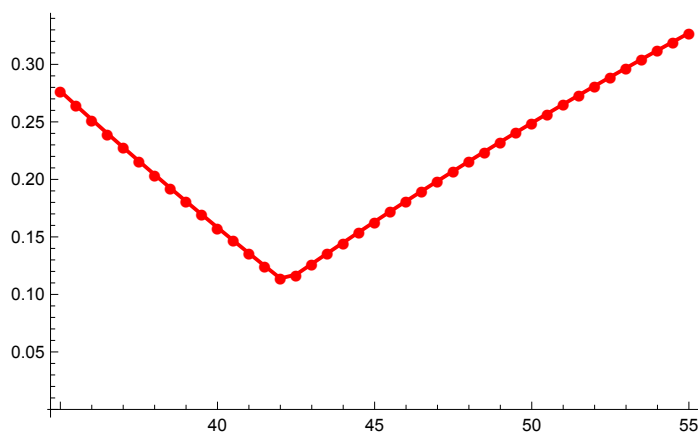

```
tabgamma =
  Table[{gaFra, normfitconsts[damp, gaFra * gammaFrag]}, {gaFra, 41, 43, 1 / 5}];
```

```
ListPlot[tabgamma, Joined -> True,
PlotMarkers -> Automatic, PlotStyle -> {Thick, Red}]
```

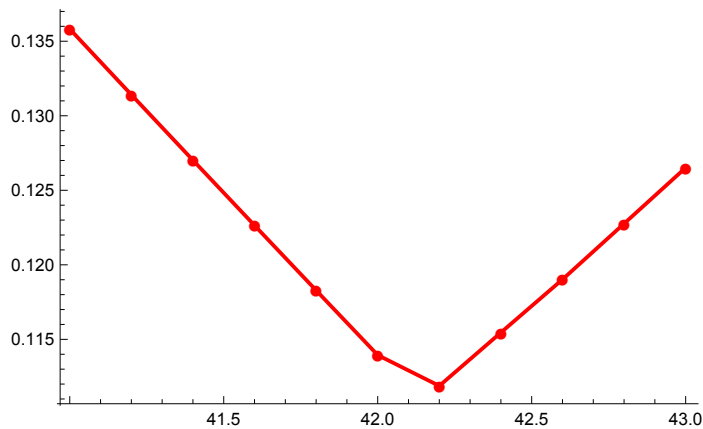

```
N[MinimalBy[tabgamma, Last]]
```

```
{{42.2, 0.111878}}
```

```
intgamma = Interpolation[tabgamma, x]
```

```
InterpolatingFunction[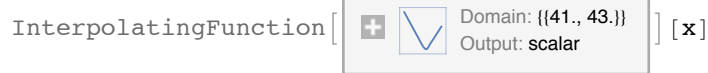 Domain: {{41., 43.}}  
Output: scalar][x]
```

```
mingamma = FindMinimum[intgamma, {x, 41.0, 43.0}]
```

InterpolatingFunction::dmval:

Input value {43.2642} lies outside the range of data in the interpolating function. Extrapolation will be used. >>

```
{0.111874, {x -> 42.1931}}
```

```
optent = x /. mingamma[[2]]
```

```
42.1931
```

```
optGaFra := optent * gammaFrag
```

```
iy = dsionyieldcrateranalysisparam[damp * 0.26 * MilliJouleToHartree, photonenergy,
tauX, nintdata, True, True, 1 / 1000, optfNppN, 1 - optfNppN, optGaFra]
```

```
iy = 1 / Total[iy[[2 ;; 8]]] * iy
```

```
Total[iy[[2 ;; 8]]]
```

```
{0.966325, 0.0203321, 0.00967749, 0.00193639,
0.00124901, 0.000438765, 0.0000399311, 1.32927 × 10-6,
0.962931, 0.00060551, -4.1454 × 10-124, -8.11507 × 10-136}}
```

```
{28.6956, 0.603774, 0.287379, 0.0575022, 0.0370902, 0.0130294, 0.00118578,
0.0000394734, 28.5948, 0.017981, -1.231 × 10-122, -2.40982 × 10-134}}
```

```
1.
```

```
plotiy = Partition[Riffle[normOleg80, iy[[2 ;; 8]]], 2]
```

```
{{0.604006, 0.603774}, {0.287434, 0.287379},
{0.0722227, 0.0575022}, {0.0271552, 0.0370902},
{0.00918191, 0.0130294}, {0., 0.00118578}, {0., 0.0000394734}}
```

```
BarChart[plotiy, PlotRange → {-0.1, 0.9},
  ChartLabels → {Placed[{"N +", "N 2+", "N 3+", "N 4+", "N 5+", "N 6+", "N 7+"}, Below],
    Placed[{}, Above]},
  ChartLegends → Placed[{"Expt.", "γfrag"}, Top],
  ChartStyle → {Black, Red}, AxesLabel → {"", "Ỹ(ω)"},
  AxesStyle → {{Arrowheads[Automatic], AbsoluteThickness[0.6]},
    {Arrowheads[Automatic], AbsoluteThickness[0.6]}},
  LabelStyle → {FontFamily → "Arial"},
  PlotLabel → {damp, optGaFra / gammaFrag,
    (iynorm[[2 ;; 8]] - normOleg80).Table[i, {i, 1, 7}]]}
```

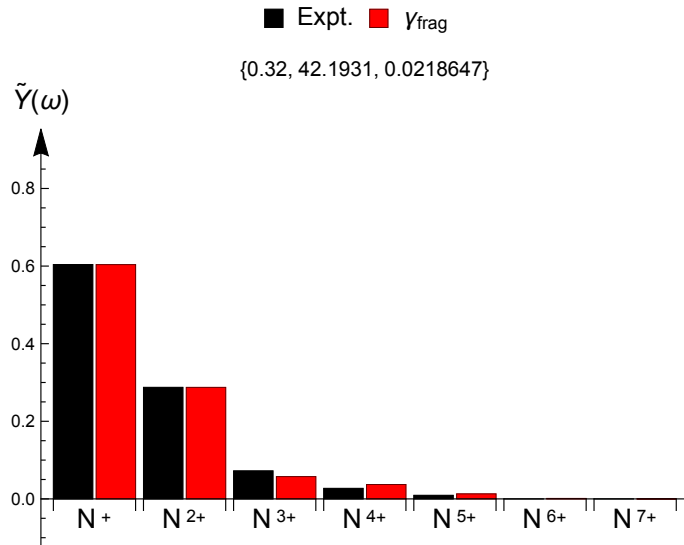

## Pulse energy for a 280 fs pulse with 280 fs fragmentation rate

```
tauX := shtdur280 * 280 / t0ToFemtoSecond
optent := 13.200000
optGaFra := optent * gammaFrag
```

### 0.38

```
damp := 0.38
```

```
iy = dsionyieldcrateranalysisparam[damp * 0.26 * MilliJouleToHartree, photonenergy,
  tauX, nintdata, True, True, 1 / 1000, optfNppN, 1 - optfNppN, optGaFra]
```

```
iynorm = 1 / Total[iy[[2 ;; 8]]] * iy
```

```
Total[iynorm[[2 ;; 8]]]
```

```
{0.962114, 0.0216966, 0.0110545, 0.00228013,
  0.00197778, 0.000773247, 0.0000983146, 5.27966 × 10-6,
  0.958498, 0.000638571, 9.18917 × 10-60, 6.02328 × 10-113}}
```

```
{25.3951, 0.572683, 0.291785, 0.0601843, 0.0522036, 0.0204099, 0.00259502,
  0.000139357, 25.2996, 0.0168551, 2.42549 × 10-58, 1.58985 × 10-111}}
```

```
1.
```

```

plotiy = Partition[Riffle[normOleg280, iynorm[[2 ;; 8]]], 2]
{{0.56634, 0.572683}, {0.291805, 0.291785},
 {0.0763903, 0.0601843}, {0.0364504, 0.0522036},
 {0.027387, 0.0204099}, {0.00162698, 0.00259502}, {0., 0.000139357}}

BarChart[plotiy, PlotRange → {-0.1, 0.9},
 ChartLabels → {Placed[{"N +", "N 2+", "N 3+", "N 4+", "N 5+", "N 6+", "N 7+"}, Below],
 Placed[{}, Above]},
 ChartLegends → Placed[{"Expt.", "γfrag"}, Top],
 ChartStyle → {Black, Red}, AxesLabel → {"", "Ỹ(ω)"},
 AxesStyle → {{Arrowheads[Automatic], AbsoluteThickness[0.6]},
 {Arrowheads[Automatic], AbsoluteThickness[0.6]}},
 LabelStyle → {FontFamily → "Arial"},
 PlotLabel → {damp, optGaFra / gammaFrag,
 (iynorm[[2 ;; 8]] - normOleg280).Table[i, {i, 1, 7}]}]

```

■ Expt. ■ γ<sub>frag</sub>

{0.38, 13.2, -0.00740437}

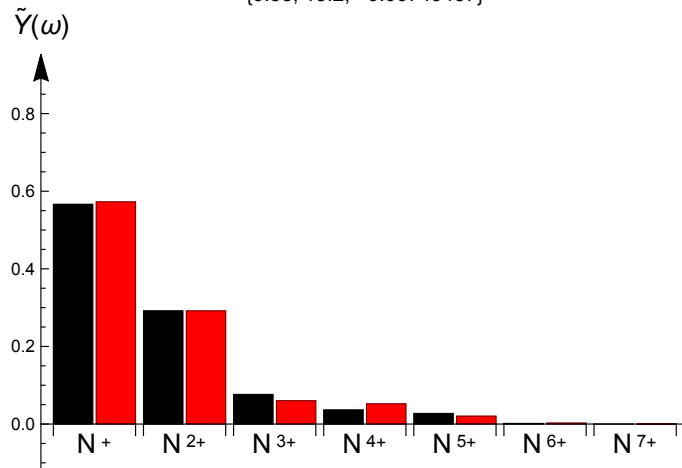

## Pulse energy for a 280 fs pulse with 80 fs fragmentation rate

```

tauX := shtdur280 * 280 / t0ToFemtoSecond
optent := 38.864973
optGaFra := optent * gammaFrag

```

0.36

```
damp := 0.36
```



```

iy = dsionyieldcrateranalysisparam[damp * 0.26 * MilliJouleToHartree, photonenergy,
  tauX, nintdata, True, True, 1 / 1000, optfNppN, 1 - optfNppN, optGaFra]
iynorm = 1 / Total[iy[[2 ;; 8]]] * iy
Total[iynorm[[2 ;; 8]]]

```

```

{0.963646, 0.0222733, 0.00830014, 0.00324322, 0.00157119, 0.000851699,
  0.000107858, 6.44739 × 10-6, 0.959918, 0.0006288, 1.54154 × 10-126, 1.35849 × 10-139}

```

```

{26.5074, 0.612681, 0.228315, 0.0892126, 0.0432192, 0.023428, 0.00296689,
  0.000177351, 26.4049, 0.0172966, 4.24037 × 10-125, 3.73685 × 10-138}

```

1.

```

plotiy = Partition[Riffle[normOleg280, iynorm[[2 ;; 8]]], 2]

```

```

{{0.56634, 0.612681}, {0.291805, 0.228315},
 {0.0763903, 0.0892126}, {0.0364504, 0.0432192},
 {0.027387, 0.023428}, {0.00162698, 0.00296689}, {0., 0.000177351}}

```

```

BarChart[plotiy, PlotRange → {-0.1, 0.9},
  ChartLabels → {Placed[{"N +", "N 2+", "N 3+", "N 4+", "N 5+", "N 6+", "N 7+"}, Below],
    Placed[{}, Above]},
  ChartLegends → Placed[{"Expt.", "γfrag"}, Top],
  ChartStyle → {Black, Red}, AxesLabel → {"", "Ỹ(ω)"},
  AxesStyle → {{Arrowheads[Automatic], AbsoluteThickness[0.6]},
    {Arrowheads[Automatic], AbsoluteThickness[0.6]}},
  LabelStyle → {FontFamily → "Arial"},
  PlotLabel → {damp, optGaFra / gammaFrag,
    (iynorm[[2 ;; 8]] - normOleg280).Table[i, {i, 1, 7}]}]

```

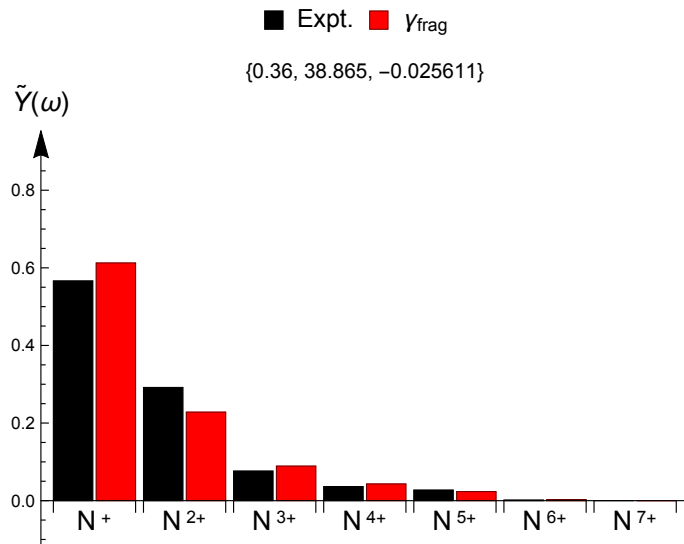

## 0.37

```

damp := 0.37

```

```

iy = dsionyieldcrateranalysisparam[damp * 0.26 * MilliJouleToHartree, photonenergy,
  tauX, nintdata, True, True, 1 / 1000, optfNppN, 1 - optfNppN, optGaFra]
iynorm = 1 / Total[iy[[2 ;; 8]]] * iy
Total[iynorm[[2 ;; 8]]]

```

```

{0.962968, 0.0225135, 0.00847852, 0.00335549,
 0.00164849, 0.000909835, 0.000118542,  $7.27682 \times 10^{-6}$ ,
 0.959202, 0.000633827,  $-1.25961 \times 10^{-127}$ ,  $1.92684 \times 10^{-134}$ }

```

```

{26.0039, 0.607953, 0.228953, 0.0906115, 0.0445157, 0.0245691, 0.0032011,
 0.000196503, 25.9022, 0.0171158,  $-3.40143 \times 10^{-126}$ ,  $5.20323 \times 10^{-133}$ }

```

```
1.
```

```

plotiy = Partition[Riffle[normOleg280, iynorm[[2 ;; 8]]], 2]

```

```

{{0.56634, 0.607953}, {0.291805, 0.228953},
 {0.0763903, 0.0906115}, {0.0364504, 0.0445157},
 {0.027387, 0.0245691}, {0.00162698, 0.0032011}, {0., 0.000196503}}

```

```

BarChart[plotiy, PlotRange → {-0.1, 0.9},
  ChartLabels → {Placed[{"N +", "N 2+", "N 3+", "N 4+", "N 5+", "N 6+", "N 7+"}, Below],
    Placed[{}, Above]},
  ChartLegends → Placed[{"Expt.", " $\gamma_{frag}$ "}, Top],
  ChartStyle → {Black, Red}, AxesLabel → {"", " $\tilde{Y}(\omega)$ "},
  AxesStyle → {{Arrowheads[Automatic], AbsoluteThickness[0.6]},
    {Arrowheads[Automatic], AbsoluteThickness[0.6]}},
  LabelStyle → {FontFamily → "Arial"},
  PlotLabel → {damp, optGaFra / gammaFrag,
    (iynorm[[2 ;; 8]] - normOleg280).Table[i, {i, 1, 7}]]}

```

■ Expt. ■  $\gamma_{frag}$

{0.37, 38.865, -0.0124352}

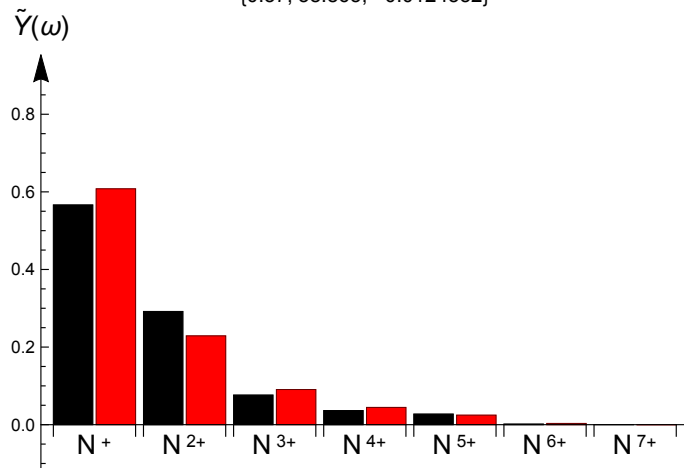

0.38

damp := 0.38

```
iy = dsionyieldcrateranalysisparam[damp * 0.26 * MilliJouleToHartree, photonenergy,
  tauX, nintdata, True, True, 1 / 1000, optfNppN, 1 - optfNppN, optGaFra]
iynorm = 1 / Total[iy[[2 ;; 8]]] * iy
Total[iynorm[[2 ;; 8]]]
```

```
{0.962302, 0.0227433, 0.00865298, 0.00346687,
  0.00172658, 0.000969783, 0.000129901, 8.18304 × 10-6,
  0.958498, 0.000638572, -1.45216 × 10-126, 9.78856 × 10-137}
```

```
{25.5269, 0.603309, 0.229537, 0.0919654, 0.0458009, 0.0257254, 0.00344588,
  0.000217071, 25.426, 0.0169393, -3.85214 × 10-125, 2.5966 × 10-135}
```

1.

```
plotiy = Partition[Riffle[normOleg280, iynorm[[2 ;; 8]]], 2]
```

```
{{0.56634, 0.603309}, {0.291805, 0.229537},
  {0.0763903, 0.0919654}, {0.0364504, 0.0458009},
  {0.027387, 0.0257254}, {0.00162698, 0.00344588}, {0., 0.000217071}}
```

```
BarChart[plotiy, PlotRange → {-0.1, 0.9},
  ChartLabels → {Placed[{"N +", "N 2+", "N 3+", "N 4+", "N 5+", "N 6+", "N 7+"}, Below],
    Placed[{}, Above]},
  ChartLegends → Placed[{"Expt.", "γfrag"}, Top],
  ChartStyle → {Black, Red}, AxesLabel → {"", "Ỹ(ω)"},
  AxesStyle → {{Arrowheads[Automatic], AbsoluteThickness[0.6]},
    {Arrowheads[Automatic], AbsoluteThickness[0.6]}},
  LabelStyle → {FontFamily → "Arial"},
  PlotLabel → {damp, optGaFra / gammaFrag,
    (iynorm[[2 ;; 8]] - normOleg280).Table[i, {i, 1, 7}]}]
```

■ Expt. ■ γ<sub>frag</sub>

{0.38, 38.865, 0.00068397}

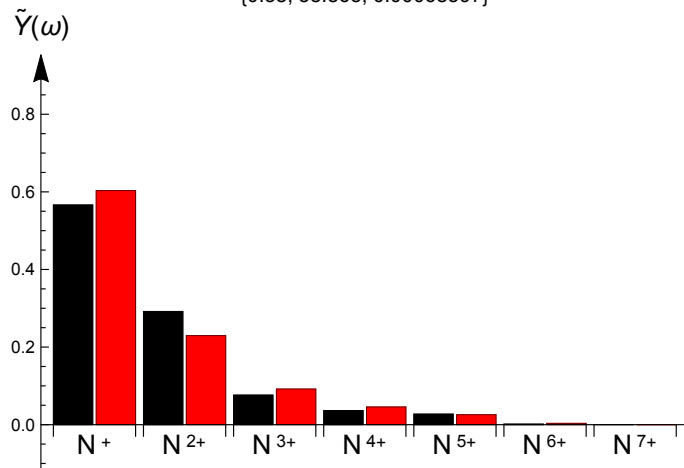

0.39

damp := 0.39

```

iy = dsionyieldcrateranalysisparam[damp * 0.26 * MilliJouleToHartree, photonenergy,
  tauX, nintdata, True, True, 1 / 1000, optfNppN, 1 - optfNppN, optGaFra]
iynorm = 1 / Total[iy[[2 ;; 8]]] * iy
Total[iynorm[[2 ;; 8]]]

{0.961347, 0.0213467, 0.0139328, 0.00237795, 0.000821609, 0.000170816,
  2.9334 × 10-6, 8.06592 × 10-9, 0.957808, 0.00064305, -3.71778 × 10-98, -1.8606 × 10-149}

{24.8713, 0.552268, 0.36046, 0.0615207, 0.0212561, 0.00441922, 0.0000758909,
  2.08676 × 10-7, 24.7797, 0.0166365, -9.61838 × 10-97, -4.81361 × 10-148}

1.

```

```

plotiy = Partition[Riffle[normOleg280, iynorm[[2 ;; 8]]], 2]

{{0.56634, 0.552268}, {0.291805, 0.36046},
 {0.0763903, 0.0615207}, {0.0364504, 0.0212561}, {0.027387, 0.00441922},
 {0.00162698, 0.0000758909}, {0., 2.08676 × 10-7}}

BarChart[plotiy, PlotRange → {-0.1, 0.9},
  ChartLabels → {Placed[{"N +", "N 2+", "N 3+", "N 4+", "N 5+", "N 6+", "N 7+"}, Below],
    Placed[{}, Above]},
  ChartLegends → Placed[{"Expt.", "γfrag"}, Top],
  ChartStyle → {Black, Red}, AxesLabel → {"", "Ỹ(ω)"},
  AxesStyle → {{Arrowheads[Automatic], AbsoluteThickness[0.6]},
    {Arrowheads[Automatic], AbsoluteThickness[0.6]}},
  LabelStyle → {FontFamily → "Arial"},
  PlotLabel → {damp, optGaFra / gammaFrag,
    (iynorm[[2 ;; 8]] - normOleg280).Table[i, {i, 1, 7}]}]

```

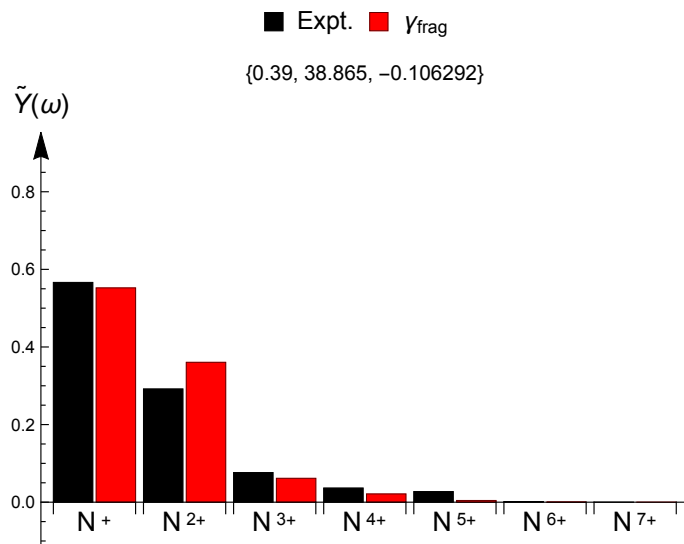

0.40

damp := 0.40

```
iy = dsionyieldcrateranalysisparam[damp * 0.26 * MilliJouleToHartree, photonenergy,
  tauX, nintdata, True, True, 1 / 1000, optfNppN, 1 - optfNppN, optGaFra]
iynorm = 1 / Total[iy[[2 ;; 8]]] * iy
Total[iynorm[[2 ;; 8]]]
```

```
{0.960696, 0.0215134, 0.0142301, 0.00249783,
  0.000873897, 0.000185375,  $3.27461 \times 10^{-6}$ ,  $9.25091 \times 10^{-9}$ ,
  0.957131, 0.000647276,  $-5.85829 \times 10^{-132}$ ,  $8.518 \times 10^{-153}$ }
```

```
{24.4428, 0.547362, 0.362052, 0.0635517, 0.0222344, 0.00471646, 0.0000833152,
   $2.35369 \times 10^{-7}$ , 24.3521, 0.0164685,  $-1.49051 \times 10^{-130}$ ,  $2.16722 \times 10^{-151}$ }
```

1.

```
plotiy = Partition[Riffle[normOleg280, iynorm[[2 ;; 8]]], 2]
```

```
{{0.56634, 0.547362}, {0.291805, 0.362052},
  {0.0763903, 0.0635517}, {0.0364504, 0.0222344}, {0.027387, 0.00471646},
  {0.00162698, 0.0000833152}, {0.,  $2.35369 \times 10^{-7}$ }}
```

```
BarChart[plotiy, PlotRange → {-0.1, 0.9},
  ChartLabels → {Placed[{"N +", "N 2+", "N 3+", "N 4+", "N 5+", "N 6+", "N 7+"}, Below],
    Placed[{}, Above]},
  ChartLegends → Placed[{"Expt.", "γfrag"}, Top],
  ChartStyle → {Black, Red}, AxesLabel → {"", "Ỹ(ω)"},
  AxesStyle → {{Arrowheads[Automatic], AbsoluteThickness[0.6]},
    {Arrowheads[Automatic], AbsoluteThickness[0.6]}},
  LabelStyle → {FontFamily → "Arial"},
  PlotLabel → {damp, optGaFra / gammaFrag,
    (iynorm[[2 ;; 8]] - normOleg280).Table[i, {i, 1, 7}]}]
```

■ Expt. ■ γ<sub>frag</sub>

{0.4, 38.865, -0.096477}

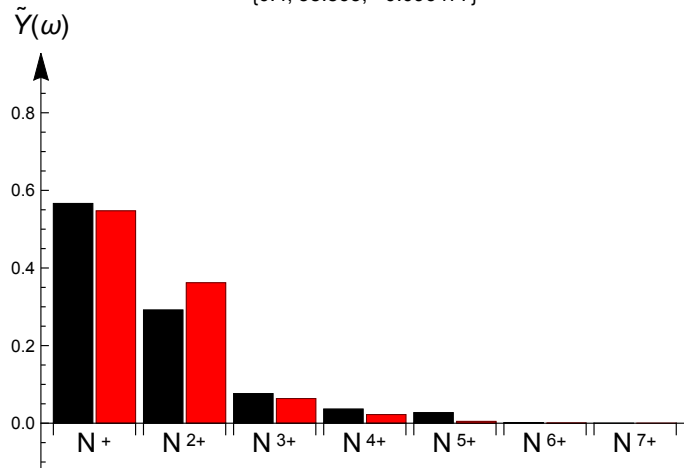

## Pulse energy for a 80 fs pulse with 280 fs fragmentation rate

```
tauX := shtdur80 * 80 / t0ToFemtoSecond
optent := 13.200000
optGaFra := optent * gammaFrag
```

### 0.28

```
damp := 0.28
```

```
iy = dsionyieldsanalysisparam[damp * 0.26 * MilliJouleToHartree, photonenergy,
  tauX, nintdata, True, True, 1 / 1000, optfNppN, 1 - optfNppN, optGaFra]
```

```
inyorm = 1 / Total[iy[[2 ;; 8]]] * iy
```

```
Total[inyorm[[2 ;; 8]]]
```

```
{0.969301, 0.0186061, 0.00986477, 0.000999262, 0.000972123, 0.000237915,
  0.0000183295,  $4.82658 \times 10^{-7}$ , 0.966197, 0.000576154,  $4.93852 \times 10^{-60}$ ,  $4.0538 \times 10^{-133}$ }
```

```
{31.5743, 0.606082, 0.321338, 0.0325503, 0.0316663, 0.00774993, 0.00059707,
  0.0000157223, 31.4732, 0.0187678,  $1.60869 \times 10^{-58}$ ,  $1.3205 \times 10^{-131}$ }
```

```
1.
```

```
plotiy = Partition[Riffle[normOleg80, inyorm[[2 ;; 8]]], 2]
```

```
{{0.604006, 0.606082}, {0.287434, 0.321338},
  {0.0722227, 0.0325503}, {0.0271552, 0.0316663},
  {0.00918191, 0.00774993}, {0., 0.00059707}, {0., 0.0000157223}}
```

```
BarChart[plotiy, PlotRange → {-0.1, 0.9},
  ChartLabels → {Placed[{"N +", "N 2+", "N 3+", "N 4+", "N 5+", "N 6+", "N 7+"}, Below],
    Placed[{}, Above]},
  ChartLegends → Placed[{"Expt.", "γfrag"}, Top],
  ChartStyle → {Black, Red}, AxesLabel → {"", "Ỹ(ω)",
  AxesStyle → {{Arrowheads[Automatic], AbsoluteThickness[0.6]},
    {Arrowheads[Automatic], AbsoluteThickness[0.6]}},
  LabelStyle → {FontFamily → "Arial"},
  PlotLabel → {damp, optGaFra / gammaFrag,
    (iynorm[[2 ;; 8]] - normOleg80).Table[i, {i, 1, 7}]]}]
```

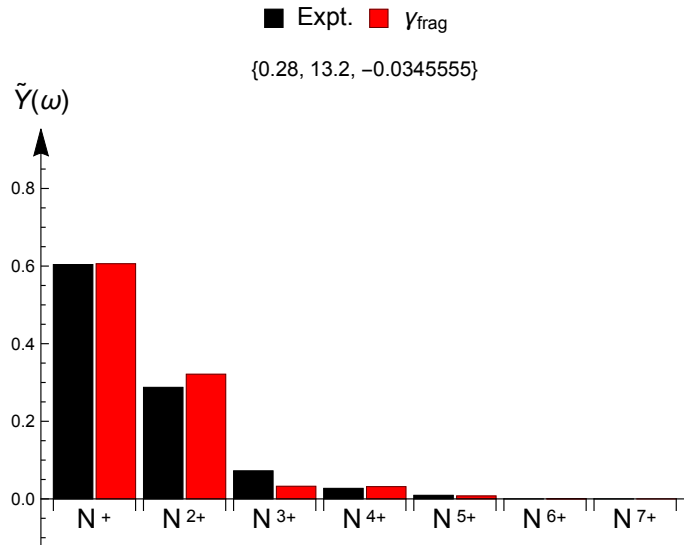

## 0.29

damp := 0.29

```
iy = dsionyieldcrateranalysisparam[damp * 0.26 * MilliJouleToHartree, photonenergy,
  tauX, nintdata, True, True, 1 / 1000, optfNppN, 1 - optfNppN, optGaFra]
```

```
iynorm = 1 / Total[iy[[2 ;; 8]]] * iy
```

```
Total[iynorm[[2 ;; 8]]]
```

```
{0.968505, 0.0188922, 0.0102071, 0.00106201,
  0.00104787, 0.000264321, 0.0000211425, 5.76202 × 10-7,
  0.965355, 0.000584142, 4.98555 × 10-60, -8.18928 × 10-135}}
```

```
{30.7509, 0.599844, 0.324083, 0.0337199, 0.0332709, 0.00839243, 0.000671293,
  0.0000182949, 30.6509, 0.0185471, 1.58296 × 10-58, -2.60017 × 10-133}}
```

1.

```
plotiy = Partition[Riffle[normOleg80, iynorm[[2 ;; 8]]], 2]
```

```
{{0.604006, 0.599844}, {0.287434, 0.324083},
  {0.0722227, 0.0337199}, {0.0271552, 0.0332709},
  {0.00918191, 0.00839243}, {0., 0.000671293}, {0., 0.0000182949}}
```

```
BarChart[plotiy, PlotRange → {-0.1, 0.9},
  ChartLabels → {Placed[{"N +", "N 2+", "N 3+", "N 4+", "N 5+", "N 6+", "N 7+"}, Below],
    Placed[{}, Above]},
  ChartLegends → Placed[{"Expt.", "γfrag"}, Top],
  ChartStyle → {Black, Red}, AxesLabel → {"", "Ỹ(ω)",
  AxesStyle → {{Arrowheads[Automatic], AbsoluteThickness[0.6]},
    {Arrowheads[Automatic], AbsoluteThickness[0.6]}},
  LabelStyle → {FontFamily → "Arial"},
  PlotLabel → {damp, optGaFra / gammaFrag,
    (iynorm[[2 ;; 8]] - normOleg80).Table[i, {i, 1, 7}]]}
```

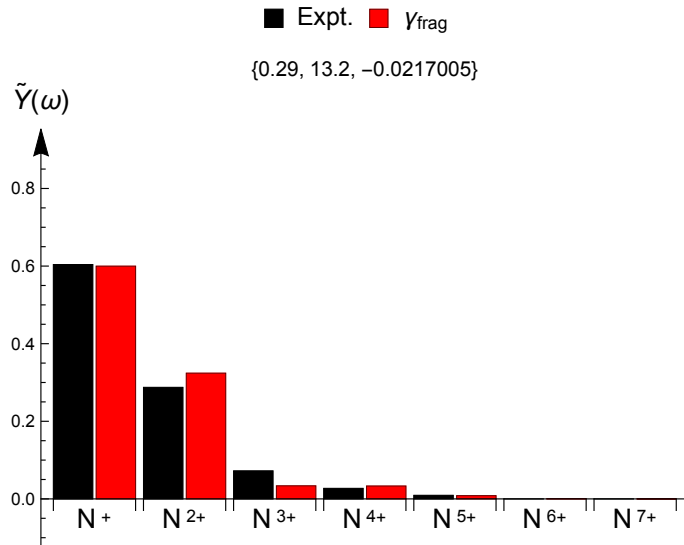

### 0.30

damp := 0.30

```
iy = dsionyieldcrateranalysisparam[damp * 0.26 * MilliJouleToHartree, photonenergy,
  tauX, nintdata, True, True, 1 / 1000, optfNppN, 1 - optfNppN, optGaFra]
```

```
iynorm = 1 / Total[iy[[2 ;; 8]]] * iy
```

```
Total[iynorm[[2 ;; 8]]]
```

```
{0.967724, 0.0191638, 0.0105435, 0.00112569, 0.00112581, 0.000292423,
  0.0000242559, 6.83427 × 10-7, 0.96453, 0.000591681, 5.18903 × 10-60, 1.74729 × 10-134}
```

```
{29.9826, 0.593745, 0.326665, 0.0348768, 0.0348804, 0.00906001, 0.000751509,
  0.0000211743, 29.8836, 0.0183318, 1.60769 × 10-58, 5.41355 × 10-133}
```

1.

```
plotiy = Partition[Riffle[normOleg80, iynorm[[2 ;; 8]]], 2]
```

```
{{0.604006, 0.593745}, {0.287434, 0.326665},
  {0.0722227, 0.0348768}, {0.0271552, 0.0348804},
  {0.00918191, 0.00906001}, {0., 0.000751509}, {0., 0.0000211743}}
```



```
BarChart[plotiy, PlotRange → {-0.1, 0.9},
  ChartLabels → {Placed[{"N +", "N 2+", "N 3+", "N 4+", "N 5+", "N 6+", "N 7+"}, Below],
    Placed[{}, Above]},
  ChartLegends → Placed[{"Expt.", "γfrag"}, Top],
  ChartStyle → {Black, Red}, AxesLabel → {"", "Ỹ(ω)"},
  AxesStyle → {{Arrowheads[Automatic], AbsoluteThickness[0.6]},
    {Arrowheads[Automatic], AbsoluteThickness[0.6]}},
  LabelStyle → {FontFamily → "Arial"},
  PlotLabel → {damp, optGaFra / gammaFrag,
    (iynorm[[2 ;; 8]] - normOleg80).Table[i, {i, 1, 7}]]}
```

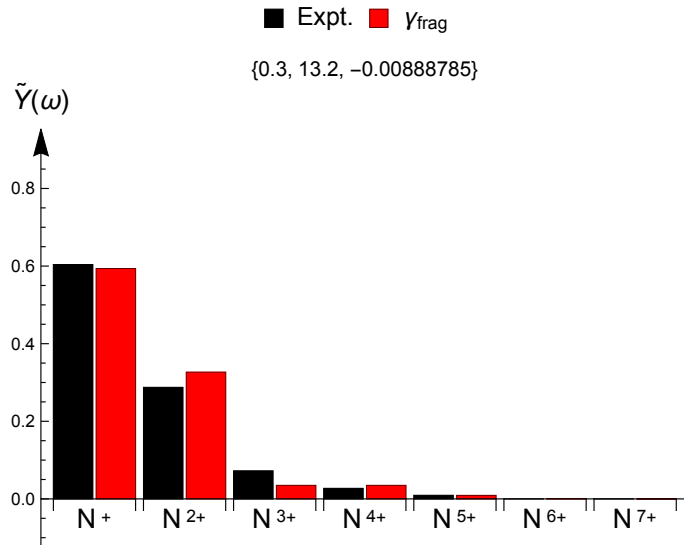

### 0.31

damp := 0.31

```
iy = dsionyieldcrateranalysisparam[damp * 0.26 * MilliJouleToHartree, photonenergy,
  tauX, nintdata, True, True, 1 / 1000, optfNppN, 1 - optfNppN, optGaFra]
```

```
iynorm = 1 / Total[iy[[2 ;; 8]]] * iy
```

```
Total[iynorm[[2 ;; 8]]]
```

```
{0.966957, 0.0194219, 0.010874, 0.00119021, 0.00120581, 0.00032224, 0.0000276875,
  8.05698 × 10-7, 0.963722, 0.000598796, 5.24712 × 10-60, 2.40686 × 10-139}
```

```
{29.2639, 0.587782, 0.329091, 0.0360203, 0.0364926, 0.00975225, 0.000837931,
  0.0000243836, 29.166, 0.0181219, 1.58798 × 10-58, 7.28408 × 10-138}
```

1.

```
plotiy = Partition[Riffle[normOleg80, iynorm[[2 ;; 8]]], 2]
```

```
{{0.604006, 0.587782}, {0.287434, 0.329091},
  {0.0722227, 0.0360203}, {0.0271552, 0.0364926},
  {0.00918191, 0.00975225}, {0., 0.000837931}, {0., 0.0000243836}}
```

```
BarChart[plotiy, PlotRange → {-0.1, 0.9},
  ChartLabels → {Placed[{"N +", "N 2+", "N 3+", "N 4+", "N 5+", "N 6+", "N 7+"}, Below],
    Placed[{}, Above]},
  ChartLegends → Placed[{"Expt.", "γfrag"}, Top],
  ChartStyle → {Black, Red}, AxesLabel → {"", "Ỹ(ω)"},
  AxesStyle → {{Arrowheads[Automatic], AbsoluteThickness[0.6]},
    {Arrowheads[Automatic], AbsoluteThickness[0.6]}},
  LabelStyle → {FontFamily → "Arial"},
  PlotLabel → {damp, optGaFra / gammaFrag,
    (iynorm[[2 ;; 8]] - normOleg80).Table[i, {i, 1, 7}]]}
```

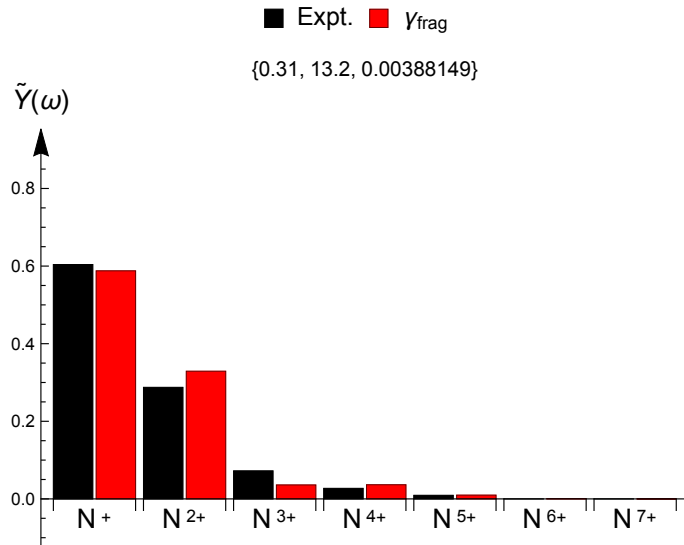

## 0.32

damp := 0.32

```
iy = dsionyieldcrateranalysisparam[damp * 0.26 * MilliJouleToHartree, photonenergy,
  tauX, nintdata, True, True, 1 / 1000, optfNppN, 1 - optfNppN, optGaFra]
```

```
iynorm = 1 / Total[iy[[2 ;; 8]]] * iy
```

```
Total[iynorm[[2 ;; 8]]]
```

```
{0.966205, 0.019667, 0.0111984, 0.00125547, 0.00128779, 0.000353788, 0.0000314553,
  9.44453 × 10-7, 0.962931, 0.00060551, 7.07597 × 10-60, -4.58678 × 10-134}
```

```
{28.5903, 0.581952, 0.331365, 0.0371498, 0.038106, 0.0104687, 0.00093077,
  0.0000279466, 28.4934, 0.0179172, 2.0938 × 10-58, -1.35724 × 10-132}
```

1.

```
plotiy = Partition[Riffle[normOleg80, iynorm[[2 ;; 8]]], 2]
```

```
{{0.604006, 0.581952}, {0.287434, 0.331365},
  {0.0722227, 0.0371498}, {0.0271552, 0.038106},
  {0.00918191, 0.0104687}, {0., 0.00093077}, {0., 0.0000279466}}
```

```
BarChart[plotiy, PlotRange → {-0.1, 0.9},
  ChartLabels → {Placed[{"N +", "N 2+", "N 3+", "N 4+", "N 5+", "N 6+", "N 7+"}, Below],
    Placed[{}, Above]},
  ChartLegends → Placed[{"Expt.", "γfrag"}, Top],
  ChartStyle → {Black, Red}, AxesLabel → {"", "Ỹ(ω)"},
  AxesStyle → {{Arrowheads[Automatic], AbsoluteThickness[0.6]},
    {Arrowheads[Automatic], AbsoluteThickness[0.6]}},
  LabelStyle → {FontFamily → "Arial"},
  PlotLabel → {damp, optGaFra / gammaFrag,
    (iynorm[[2 ;; 8]] - normOleg80).Table[i, {i, 1, 7}]]}
```

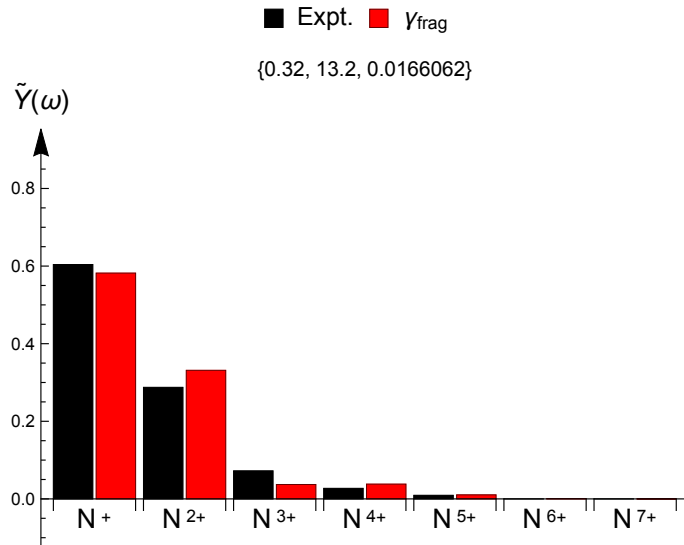

## Pulse energy for a 80 fs pulse with 80 fs fragmentation rate

```
tauX := shtdur80 * 80 / t0ToFemtoSecond
optent := 38.864973
optGaFra := optent * gammaFrag
```

### 0.30

```
damp := 0.30
```

```
iy = dsionyieldcrateranalysisparam[damp * 0.26 * MilliJouleToHartree, photonenergy,
  tauX, nintdata, True, True, 1 / 1000, optfNppN, 1 - optfNppN, optGaFra]
```

```
iynorm = 1 / Total[iy[[2 ;; 8]]] * iy
```

```
Total[iynorm[[2 ;; 8]]]
```

```
{0.967826, 0.0197289, 0.00924854, 0.00170332, 0.00110139, 0.000360656,
  0.0000305707, 9.48392 × 10-7, 0.96453, 0.000591681, -1.04224 × 10-58, 2.61202 × 10-97}
```

```
{30.0807, 0.613188, 0.287451, 0.0529402, 0.0342319, 0.0112094, 0.000950158,
  0.0000294767, 29.9782, 0.0183898, -3.23935 × 10-57, 8.11835 × 10-96}
```

```
1.
```

```

plotiy = Partition[Riffle[normOleg80, iynorm[[2 ;; 8]]], 2]
{{0.604006, 0.613188}, {0.287434, 0.287451},
 {0.0722227, 0.0529402}, {0.0271552, 0.0342319},
 {0.00918191, 0.0112094}, {0., 0.000950158}, {0., 0.0000294767}}

BarChart[plotiy, PlotRange → {-0.1, 0.9},
 ChartLabels → {Placed[{"N +", "N 2+", "N 3+", "N 4+", "N 5+", "N 6+", "N 7+"}, Below],
   Placed[{}, Above]},
 ChartLegends → Placed[{"Expt.", "γfrag"}, Top],
 ChartStyle → {Black, Red}, AxesLabel → {"", "Ỹ(ω)"},
 AxesStyle → {{Arrowheads[Automatic], AbsoluteThickness[0.6]},
   {Arrowheads[Automatic], AbsoluteThickness[0.6]}},
 LabelStyle → {FontFamily → "Arial"},
 PlotLabel → {damp, optGaFra / gammaFrag,
   (iynorm[[2 ;; 8]] - normOleg80).Table[i, {i, 1, 7}]}]

■ Expt. ■ γfrag
{0.3, 38.865, -0.00428016}

```

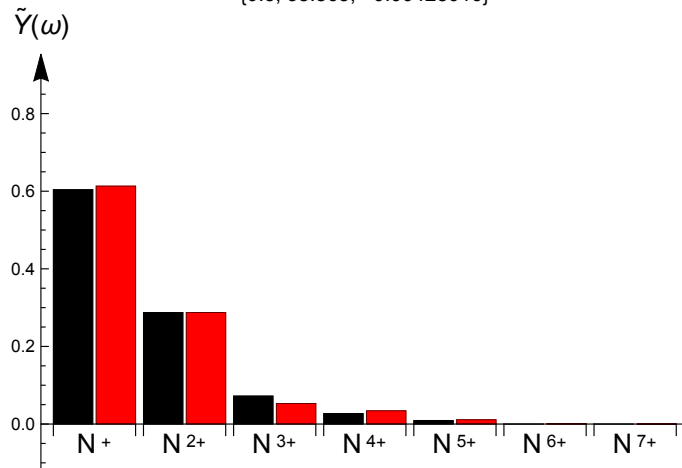

## Pulse energy for a 7 fs pulse with 280 fs fragmentation rate

```

tauX := shtdur7 * 7 / t0ToFemtoSecond
optent := 13.200000
optGaFra := optent * gammaFrag

```

### 0.12

```
damp := 0.12
```

```
iy = dsionyieldcrateranalysisparam[damp * 0.26 * MilliJouleToHartree, photonenergy,
  tauX, nintdata, True, True, 1 / 1000, optfNppN, 1 - optfNppN, optGaFra]
iynorm = 1 / Total[iy[[2 ;; 8]]] * iy
Total[iynorm[[2 ;; 8]]]
```

```
{0.984505, 0.0113429, 0.00396044, 0.000148341,
  0.0000397826,  $3.95713 \times 10^{-6}$ ,  $3.09077 \times 10^{-8}$ ,  $4.27852 \times 10^{-11}$ ,
  0.982596, 0.000359602,  $2.48372 \times 10^{-60}$ ,  $1.24196 \times 10^{-217}$ }
```

```
{63.535, 0.732015, 0.255587, 0.00957321, 0.00256737, 0.000255374,  $1.99463 \times 10^{-6}$ ,
   $2.76114 \times 10^{-9}$ , 63.4118, 0.0232069,  $1.60287 \times 10^{-58}$ ,  $8.01496 \times 10^{-216}$ }
```

1.

```
plotiy = Partition[Riffle[normOleg7, iynorm[[2 ;; 8]]], 2]
```

```
{{0.694746, 0.732015}, {0.275684, 0.255587},
  {0.0293036, 0.00957321}, {0.000266625, 0.00256737},
  {0., 0.000255374}, {0.,  $1.99463 \times 10^{-6}$ }, {0.,  $2.76114 \times 10^{-9}$ }}
```

```
BarChart[plotiy, PlotRange → {-0.1, 0.9},
  ChartLabels → {Placed[{"N +", "N 2+", "N 3+", "N 4+", "N 5+", "N 6+", "N 7+"}, Below],
    Placed[{}, Above]},
  ChartLegends → Placed[{"Expt.", "γfrag"}, Top],
  ChartStyle → {Black, Red}, AxesLabel → {"", "Ỹ(ω)"},
  AxesStyle → {{Arrowheads[Automatic], AbsoluteThickness[0.6]},
    {Arrowheads[Automatic], AbsoluteThickness[0.6]}},
  LabelStyle → {FontFamily → "Arial"},
  PlotLabel → {damp, optGaFra / gammaFrag,
    (iynorm[[2 ;; 8]] - normOleg7).Table[i, {i, 1, 7}]}]
```

■ Expt. ■ γ<sub>frag</sub>  
{0.12, 13.2, -0.0516239}

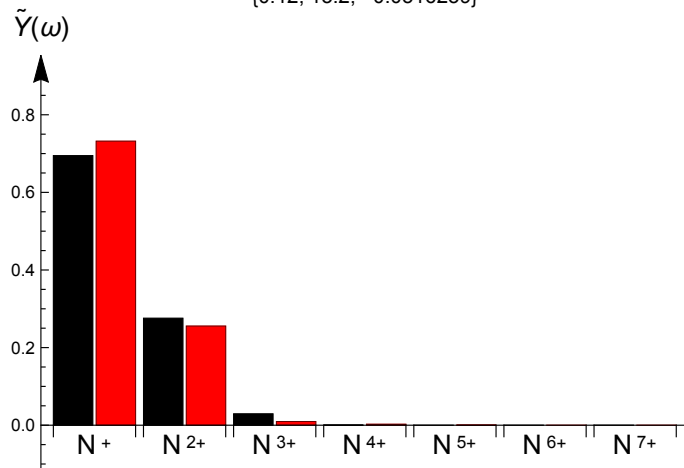

## 0.13

```
damp := 0.13
```

```

iy = dsionyieldcrateranalysisparam[damp * 0.26 * MilliJouleToHartree, photonenergy,
  tauX, nintdata, True, True, 1 / 1000, optfNppN, 1 - optfNppN, optGaFra]
iynorm = 1 / Total[iy[[2 ;; 8]]] * iy
Total[iynorm[[2 ;; 8]]]

```

```

{0.983397, 0.012007, 0.00435818, 0.000182924,
 0.0000497171, 5.32076 × 10-6, 4.51515 × 10-8, 6.78078 × 10-11,
 0.981378, 0.000379768, 2.21264 × 10-60, 1.41677 × 10-244}

```

```

{59.2295, 0.723174, 0.262491, 0.0110174, 0.00299443, 0.000320467, 2.71945 × 10-6,
 4.08403 × 10-9, 59.1079, 0.0228732, 1.33266 × 10-58, 8.53316 × 10-243}

```

1.

```

plotiy = Partition[Riffle[normOleg7, iynorm[[2 ;; 8]]], 2]

```

```

{{0.694746, 0.723174}, {0.275684, 0.262491},
 {0.0293036, 0.0110174}, {0.000266625, 0.00299443},
 {0., 0.000320467}, {0., 2.71945 × 10-6}, {0., 4.08403 × 10-9}}

```

```

BarChart[plotiy, PlotRange → {-0.1, 0.9},
  ChartLabels → {Placed[{"N +", "N 2+", "N 3+", "N 4+", "N 5+", "N 6+", "N 7+"}, Below],
    Placed[{}, Above]},
  ChartLegends → Placed[{"Expt.", "γfrag"}, Top],
  ChartStyle → {Black, Red}, AxesLabel → {"", "Ỹ(ω)"},
  AxesStyle → {{Arrowheads[Automatic], AbsoluteThickness[0.6]},
    {Arrowheads[Automatic], AbsoluteThickness[0.6]}},
  LabelStyle → {FontFamily → "Arial"},
  PlotLabel → {damp, optGaFra / gammaFrag,
    (iynorm[[2 ;; 8]] - normOleg7).Table[i, {i, 1, 7}]}]

```

■ Expt. ■ γ<sub>frag</sub>

{0.13, 13.2, -0.040286}

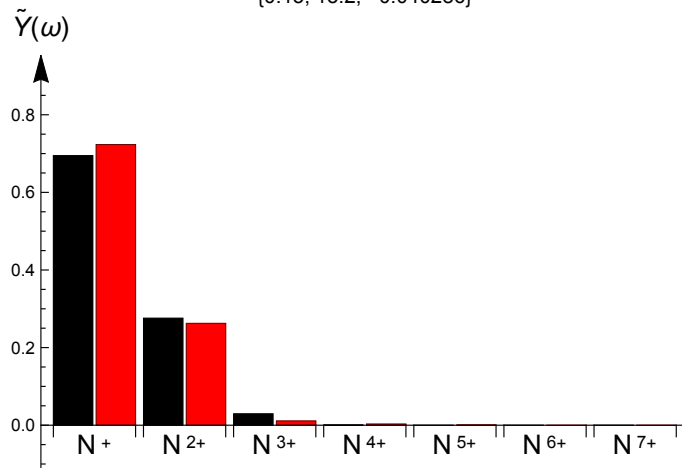

## 0.14

```

damp := 0.14

```

```
iy = dsionyieldcrateranalysisparam[damp * 0.26 * MilliJouleToHartree, photonenergy,
  tauX, nintdata, True, True, 1 / 1000, optfNppN, 1 - optfNppN, optGaFra]
iynorm = 1 / Total[iy[[2 ;; 8]]] * iy
Total[iynorm[[2 ;; 8]]]
```

```
{0.982313, 0.0126375, 0.00475934, 0.000221643, 0.0000610405, 6.98833 × 10-6,
  6.40492 × 10-8, 1.03738 × 10-10, 0.98019, 0.0003988, 2.62103 × 10-60, -7.14829 × 10-192}
```

```
{55.54, 0.714525, 0.269093, 0.0125317, 0.00345123, 0.00039512, 3.62134 × 10-6,
  5.86535 × 10-9, 55.4199, 0.0225482, 1.48193 × 10-58, -4.04164 × 10-190}
```

1.

```
plotiy = Partition[Riffle[normOleg7, iynorm[[2 ;; 8]]], 2]
```

```
{ {0.694746, 0.714525}, {0.275684, 0.269093},
  {0.0293036, 0.0125317}, {0.000266625, 0.00345123},
  {0., 0.00039512}, {0., 3.62134 × 10-6}, {0., 5.86535 × 10-9} }
```

```
BarChart[plotiy, PlotRange → {-0.1, 0.9},
  ChartLabels → {Placed[{"N +", "N 2+", "N 3+", "N 4+", "N 5+", "N 6+", "N 7+"}, Below],
    Placed[{}, Above]},
  ChartLegends → Placed[{"Expt.", "γfrag"}, Top],
  ChartStyle → {Black, Red}, AxesLabel → {"", "Ỹ(ω)"},
  AxesStyle → {{Arrowheads[Automatic], AbsoluteThickness[0.6]},
    {Arrowheads[Automatic], AbsoluteThickness[0.6]}},
  LabelStyle → {FontFamily → "Arial"},
  PlotLabel → {damp, optGaFra / gammaFrag,
    (iynorm[[2 ;; 8]] - normOleg7).Table[i, {i, 1, 7}]}]
```

■ Expt. ■ γ<sub>frag</sub>

{0.14, 13.2, -0.028982}

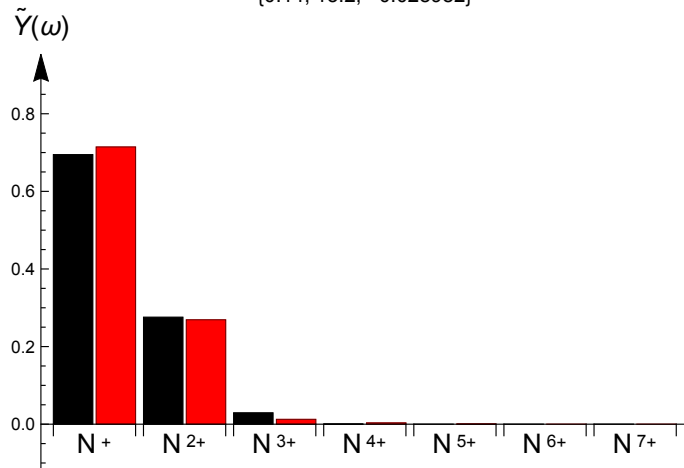

## 0.15

```
damp := 0.15
```

```

iy = dsionyieldcrateranalysisparam[damp * 0.26 * MilliJouleToHartree, photonenergy,
  tauX, nintdata, True, True, 1 / 1000, optfNppN, 1 - optfNppN, optGaFra]
iynorm = 1 / Total[iy[[2 ;; 8]]] * iy
Total[iynorm[[2 ;; 8]]]

```

```

{0.981254, 0.0132362, 0.00516284, 0.000264524,
 0.0000738058,  $8.9947 \times 10^{-6}$ ,  $8.85831 \times 10^{-8}$ ,  $1.5395 \times 10^{-10}$ ,
 0.979031, 0.000416761,  $2.32158 \times 10^{-60}$ ,  $2.46208 \times 10^{-168}$ }

```

```

{52.3434, 0.706064, 0.275403, 0.0141106, 0.00393705, 0.000479808,  $4.72532 \times 10^{-6}$ ,
  $8.21221 \times 10^{-9}$ , 52.2248, 0.0222315,  $1.23841 \times 10^{-58}$ ,  $1.31336 \times 10^{-166}$ }

```

```
1.
```

```

plotiy = Partition[Riffle[normOleg7, iynorm[[2 ;; 8]]], 2]

```

```

{{0.694746, 0.706064}, {0.275684, 0.275403},
 {0.0293036, 0.0141106}, {0.000266625, 0.00393705},
 {0., 0.000479808}, {0.,  $4.72532 \times 10^{-6}$ }, {0.,  $8.21221 \times 10^{-9}$ }}

```

```

BarChart[plotiy, PlotRange -> {-0.1, 0.9},
  ChartLabels -> {Placed[{"N +", "N 2+", "N 3+", "N 4+", "N 5+", "N 6+", "N 7+"}, Below],
    Placed[{}, Above]},
  ChartLegends -> Placed[{"Expt.", " $\gamma_{frag}$ "}, Top],
  ChartStyle -> {Black, Red}, AxesLabel -> {"", " $\tilde{Y}(\omega)$ "},
  AxesStyle -> {{Arrowheads[Automatic], AbsoluteThickness[0.6]},
    {Arrowheads[Automatic], AbsoluteThickness[0.6]}},
  LabelStyle -> {FontFamily -> "Arial"},
  PlotLabel -> {damp, optGaFra / gammaFrag,
    (iynorm[[2 ;; 8]] - normOleg7).Table[i, {i, 1, 7}]}]

```

■ Expt. ■  $\gamma_{frag}$

{0.15, 13.2, -0.0177123}

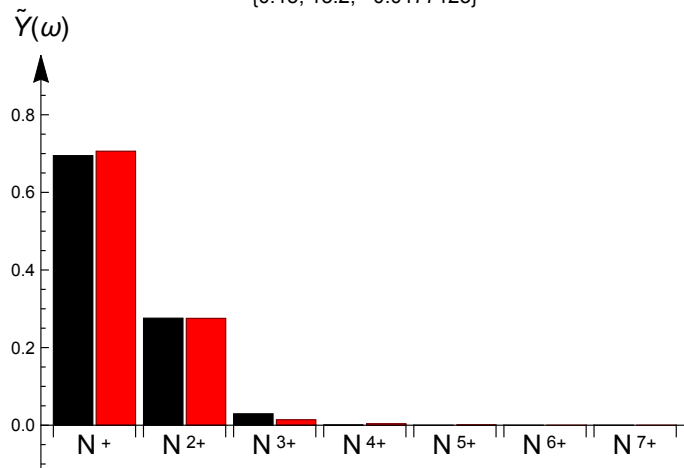

## 0.16

```
damp := 0.16
```



```
iy = dsionyieldcrateranalysisparam[damp * 0.26 * MilliJouleToHartree, photonenergy,
  tauX, nintdata, True, True, 1 / 1000, optfNppN, 1 - optfNppN, optGaFra]
iynorm = 1 / Total[iy[[2 ;; 8]]] * iy
Total[iynorm[[2 ;; 8]]]
```

```
{0.980216, 0.0138047, 0.0055677, 0.000311571, 0.0000880595, 0.0000113749,
  1.1984 × 10-7, 2.22489 × 10-10, 0.9779, 0.000433713, 2.98187 × 10-60, -1.29039 × 10-165}
```

```
{49.547, 0.697788, 0.281431, 0.015749, 0.00445115, 0.000574966, 6.05757 × 10-6,
  1.12462 × 10-8, 49.4299, 0.0219229, 1.50725 × 10-58, -6.52251 × 10-164}
```

1.

```
plotiy = Partition[Riffle[normOleg7, iynorm[[2 ;; 8]]], 2]
```

```
{ {0.694746, 0.697788}, {0.275684, 0.281431},
  {0.0293036, 0.015749}, {0.000266625, 0.00445115},
  {0., 0.000574966}, {0., 6.05757 × 10-6}, {0., 1.12462 × 10-8} }
```

```
BarChart[plotiy, PlotRange → {-0.1, 0.9},
  ChartLabels → {Placed[{"N +", "N 2+", "N 3+", "N 4+", "N 5+", "N 6+", "N 7+"}, Below],
    Placed[{}, Above]},
  ChartLegends → Placed[{"Expt.", "γfrag"}, Top],
  ChartStyle → {Black, Red}, AxesLabel → {"", "Ỹ(ω)"},
  AxesStyle → {{Arrowheads[Automatic], AbsoluteThickness[0.6]},
    {Arrowheads[Automatic], AbsoluteThickness[0.6]}},
  LabelStyle → {FontFamily → "Arial"},
  PlotLabel → {damp, optGaFra / gammaFrag,
    (iynorm[[2 ;; 8]] - normOleg7).Table[i, {i, 1, 7}]}]
```

■ Expt. ■ γ<sub>frag</sub>

{0.16, 13.2, -0.00647872}

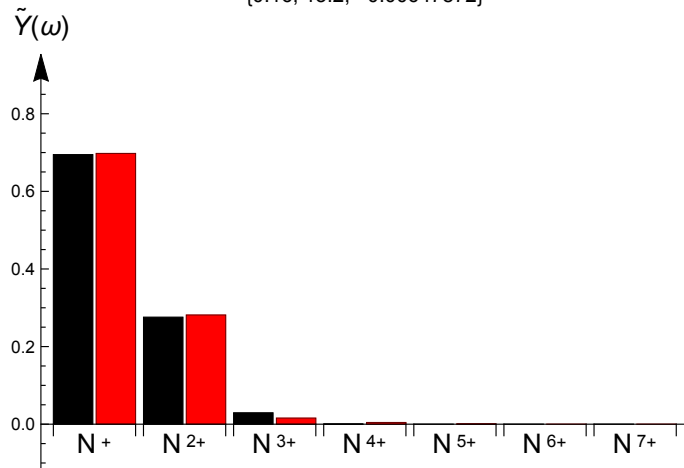

## 0.17

```
damp := 0.17
```

```

iy = dsionyieldcrateranalysisparam[damp * 0.26 * MilliJouleToHartree, photonenergy,
  tauX, nintdata, True, True, 1 / 1000, optfNppN, 1 - optfNppN, optGaFra]
iynorm = 1 / Total[iy[[2 ;; 8]]] * iy
Total[iynorm[[2 ;; 8]]]

```

```

{0.979201, 0.0143446, 0.00597302, 0.000362764,
 0.000103843, 0.0000141639, 1.59012 × 10-7, 3.14137 × 10-10,
 0.976796, 0.000449711, 2.8138 × 10-60, 3.54158 × 10-156}

```

```

{47.0804, 0.689692, 0.287185, 0.0174418, 0.0049928, 0.000681004, 7.64537 × 10-6,
 1.51038 × 10-8, 46.9647, 0.0216223, 1.35289 × 10-58, 1.7028 × 10-154}

```

1.

```

plotiy = Partition[Riffle[normOleg7, iynorm[[2 ;; 8]]], 2]

```

```

{{0.694746, 0.689692}, {0.275684, 0.287185},
 {0.0293036, 0.0174418}, {0.000266625, 0.0049928},
 {0., 0.000681004}, {0., 7.64537 × 10-6}, {0., 1.51038 × 10-8}}

```

```

BarChart[plotiy, PlotRange → {-0.1, 0.9},
  ChartLabels → {Placed[{"N +", "N 2+", "N 3+", "N 4+", "N 5+", "N 6+", "N 7+"}, Below],
    Placed[{}, Above]},
  ChartLegends → Placed[{"Expt.", "γfrag"}, Top],
  ChartStyle → {Black, Red}, AxesLabel → {"", "Ỹ(ω)"},
  AxesStyle → {{Arrowheads[Automatic], AbsoluteThickness[0.6]},
    {Arrowheads[Automatic], AbsoluteThickness[0.6]}},
  LabelStyle → {FontFamily → "Arial"},
  PlotLabel → {damp, optGaFra / gammaFrag,
    (iynorm[[2 ;; 8]] - normOleg7).Table[i, {i, 1, 7}]}]

```

■ Expt. ■ γ<sub>frag</sub>  
 {0.17, 13.2, 0.00471816}

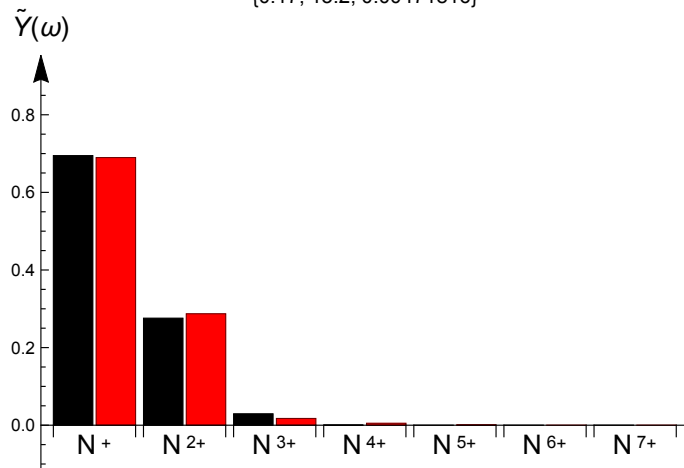

0.18

```

damp := 0.18

```

```
iy = dsionyieldcrateranalysisparam[damp * 0.26 * MilliJouleToHartree, photonenergy,
  tauX, nintdata, True, True, 1 / 1000, optfNppN, 1 - optfNppN, optGaFra]
iynorm = 1 / Total[iy[[2 ;; 8]]] * iy
Total[iynorm[[2 ;; 8]]]
```

```
{0.978208, 0.0148572, 0.00637797, 0.000418068,
  0.000121191, 0.0000173966,  $2.07394 \times 10^{-7}$ ,  $4.34476 \times 10^{-10}$ ,
  0.975718, 0.000464809,  $3.08005 \times 10^{-60}$ ,  $-1.24937 \times 10^{-159}$ }
```

```
{44.8884, 0.681772, 0.292675, 0.0191844, 0.00556124, 0.000798301,  $9.51699 \times 10^{-6}$ ,
   $1.99374 \times 10^{-8}$ , 44.7741, 0.0213294,  $1.41338 \times 10^{-58}$ ,  $-5.73318 \times 10^{-158}$ }
```

1.

```
plotiy = Partition[Riffle[normOleg7, iynorm[[2 ;; 8]]], 2]
```

```
{{0.694746, 0.681772}, {0.275684, 0.292675},
  {0.0293036, 0.0191844}, {0.000266625, 0.00556124},
  {0., 0.000798301}, {0.,  $9.51699 \times 10^{-6}$ }, {0.,  $1.99374 \times 10^{-8}$ }}
```

```
BarChart[plotiy, PlotRange → {-0.1, 0.9},
  ChartLabels → {Placed[{"N +", "N 2+", "N 3+", "N 4+", "N 5+", "N 6+", "N 7+"}, Below],
    Placed[{}, Above]},
  ChartLegends → Placed[{"Expt.", "γfrag"}, Top],
  ChartStyle → {Black, Red}, AxesLabel → {"", "Ỹ(ω)"},
  AxesStyle → {{Arrowheads[Automatic], AbsoluteThickness[0.6]},
    {Arrowheads[Automatic], AbsoluteThickness[0.6]}},
  LabelStyle → {FontFamily → "Arial"},
  PlotLabel → {damp, optGaFra / gammaFrag,
    (iynorm[[2 ;; 8]] - normOleg7).Table[i, {i, 1, 7}]}]
```

■ Expt. ■ γ<sub>frag</sub>

{0.18, 13.2, 0.0158772}

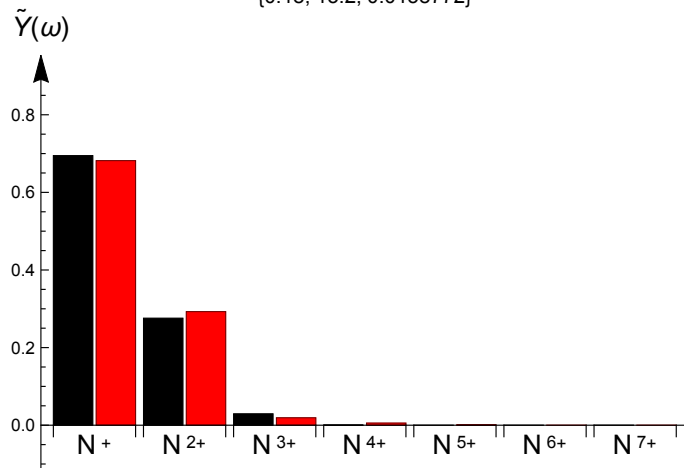

## Pulse energy for a 7 fs pulse with 80 fs fragmentation rate

```
tauX := shtdur7 * 7 / t0ToFemtoSecond
optent := 38.864973
optGaFra := optent * gammaFrag
```

## 0.12

```

damp := 0.12

iy = dsionyieldcrateranalysisparam[damp * 0.26 * MilliJouleToHartree, photonenergy,
  tauX, nintdata, True, True, 1 / 1000, optfNppN, 1 - optfNppN, optGaFra]
iynorm = 1 / Total[iy[[2 ;; 8]]] * iy
Total[iynorm[[2 ;; 8]]]

{0.984505, 0.0113466, 0.00395181, 0.000151907,
  0.0000403323,  $4.07988 \times 10^{-6}$ ,  $3.20651 \times 10^{-8}$ ,  $4.47235 \times 10^{-11}$ ,
  0.982596, 0.000359602,  $2.37445 \times 10^{-130}$ ,  $3.84033 \times 10^{-163}$ }

{63.5378, 0.732287, 0.255041, 0.00980372, 0.00260296, 0.000263306,  $2.06941 \times 10^{-6}$ ,
   $2.88635 \times 10^{-9}$ , 63.4145, 0.0232079,  $1.53242 \times 10^{-128}$ ,  $2.47846 \times 10^{-161}$ }

1.

plotiy = Partition[Riffle[normOleg7, iynorm[[2 ;; 8]]], 2]

{{0.694746, 0.732287}, {0.275684, 0.255041},
 {0.0293036, 0.00980372}, {0.000266625, 0.00260296},
 {0., 0.000263306}, {0.,  $2.06941 \times 10^{-6}$ }, {0.,  $2.88635 \times 10^{-9}$ }}

BarChart[plotiy, PlotRange → {-0.1, 0.9},
  ChartLabels → {Placed[{"N +", "N 2+", "N 3+", "N 4+", "N 5+", "N 6+", "N 7+"}, Below],
    Placed[{}, Above]},
  ChartLegends → Placed[{"Expt.", " $\gamma_{frag}$ "}, Top],
  ChartStyle → {Black, Red}, AxesLabel → {"", " $\tilde{Y}(\omega)$ "},
  AxesStyle → {{Arrowheads[Automatic], AbsoluteThickness[0.6]},
    {Arrowheads[Automatic], AbsoluteThickness[0.6]}},
  LabelStyle → {FontFamily → "Arial"},
  PlotLabel → {damp, optGaFra / gammaFrag,
    (iynorm[[2 ;; 8]] - normOleg7).Table[i, {i, 1, 7}]]}

```

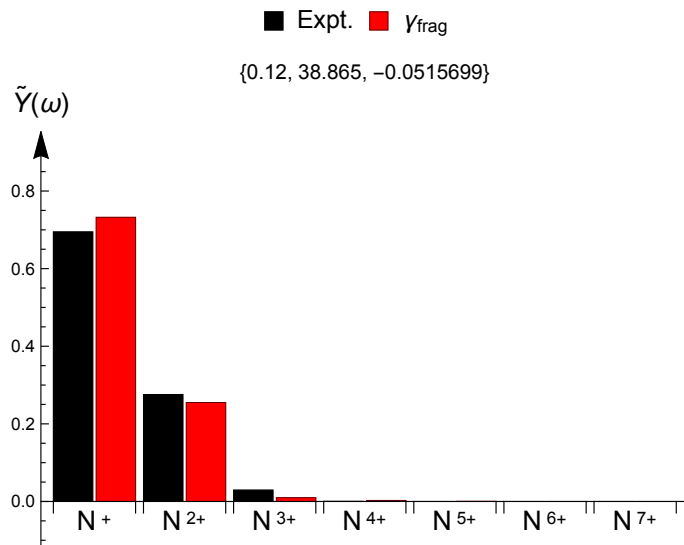

## 0.13

```

damp := 0.13

```

```

iy = dsionyieldcrateranalysisparam[damp * 0.26 * MilliJouleToHartree, photonenergy,
  tauX, nintdata, True, True, 1 / 1000, optfNppN, 1 - optfNppN, optGaFra]
iynorm = 1 / Total[iy[[2 ;; 8]]] * iy
Total[iynorm[[2 ;; 8]]]

{0.983398, 0.0120112, 0.00434838, 0.000186963, 0.0000503325, 5.47162 × 10-6,
  4.66996 × 10-8, 7.06266 × 10-11, 0.981378, 0.000379768, 1.41918 × 10-174, 3.541 × 10-225}

{59.2323, 0.723462, 0.261913, 0.0112612, 0.00303164, 0.000329568, 2.81282 × 10-6,
  4.254 × 10-9, 59.1106, 0.0228743, 8.54803 × 10-173, 2.13282 × 10-223}

1.

```

```

plotiy = Partition[Riffle[normOleg7, iynorm[[2 ;; 8]]], 2]

```

```

{{0.694746, 0.723462}, {0.275684, 0.261913},
 {0.0293036, 0.0112612}, {0.000266625, 0.00303164},
 {0., 0.000329568}, {0., 2.81282 × 10-6}, {0., 4.254 × 10-9}}

```

```

BarChart[plotiy, PlotRange → {-0.1, 0.9},
  ChartLabels → {Placed[{"N +", "N 2+", "N 3+", "N 4+", "N 5+", "N 6+", "N 7+"}, Below],
    Placed[{}, Above]},
  ChartLegends → Placed[{"Expt.", "γfrag"}, Top],
  ChartStyle → {Black, Red}, AxesLabel → {"", "Ỹ(ω)"},
  AxesStyle → {{Arrowheads[Automatic], AbsoluteThickness[0.6]},
    {Arrowheads[Automatic], AbsoluteThickness[0.6]}},
  LabelStyle → {FontFamily → "Arial"},
  PlotLabel → {damp, optGaFra / gammaFrag,
    (iynorm[[2 ;; 8]] - normOleg7).Table[i, {i, 1, 7}]}]

```

■ Expt. ■ γ<sub>frag</sub>

{0.13, 38.865, -0.0402282}

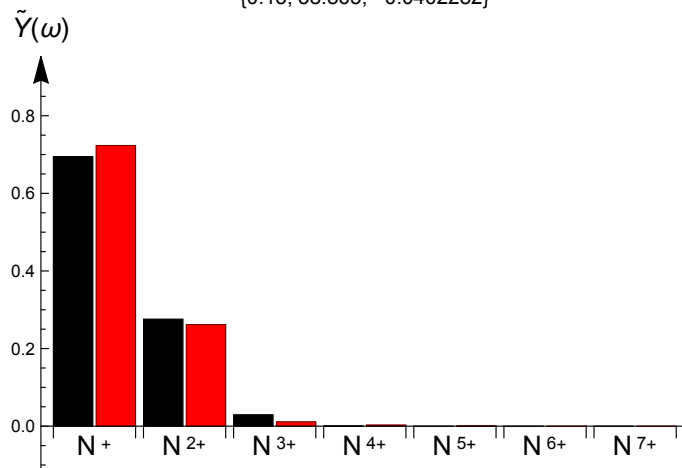

## 0.14

damp := 0.14

```

iy = dsionyieldcrateranalysisparam[damp * 0.26 * MilliJouleToHartree, photonenergy,
  tauX, nintdata, True, True, 1 / 1000, optfNppN, 1 - optfNppN, optGaFra]
iynorm = 1 / Total[iy[[2 ;; 8]]] * iy
Total[iynorm[[2 ;; 8]]]

{0.982314, 0.0126423, 0.00474834, 0.000226164, 0.0000617213,  $7.1705 \times 10^{-6}$ ,
   $6.60715 \times 10^{-8}$ ,  $1.07718 \times 10^{-10}$ , 0.98019, 0.0003988,  $-4.87223 \times 10^{-132}$ ,  $1.31792 \times 10^{-164}$ }

{55.5427, 0.714829, 0.268484, 0.0127879, 0.00348989, 0.00040544,  $3.73586 \times 10^{-6}$ ,
   $6.09066 \times 10^{-9}$ , 55.4226, 0.0225493,  $-2.75489 \times 10^{-130}$ ,  $7.45186 \times 10^{-163}$ }

1.

```

```

plotiy = Partition[Riffle[normOleg7, iynorm[[2 ;; 8]]], 2]

```

```

{{0.694746, 0.714829}, {0.275684, 0.268484},
 {0.0293036, 0.0127879}, {0.000266625, 0.00348989},
 {0., 0.00040544}, {0.,  $3.73586 \times 10^{-6}$ }, {0.,  $6.09066 \times 10^{-9}$ }}

```

```

BarChart[plotiy, PlotRange → {-0.1, 0.9},
  ChartLabels → {Placed[{"N +", "N 2+", "N 3+", "N 4+", "N 5+", "N 6+", "N 7+"}, Below],
    Placed[{}, Above]},
  ChartLegends → Placed[{"Expt.", "γfrag"}, Top],
  ChartStyle → {Black, Red}, AxesLabel → {"", "Ỹ(ω)"},
  AxesStyle → {{Arrowheads[Automatic], AbsoluteThickness[0.6]},
    {Arrowheads[Automatic], AbsoluteThickness[0.6]}},
  LabelStyle → {FontFamily → "Arial"},
  PlotLabel → {damp, optGaFra / gammaFrag,
    (iynorm[[2 ;; 8]] - normOleg7).Table[i, {i, 1, 7}]}]

```

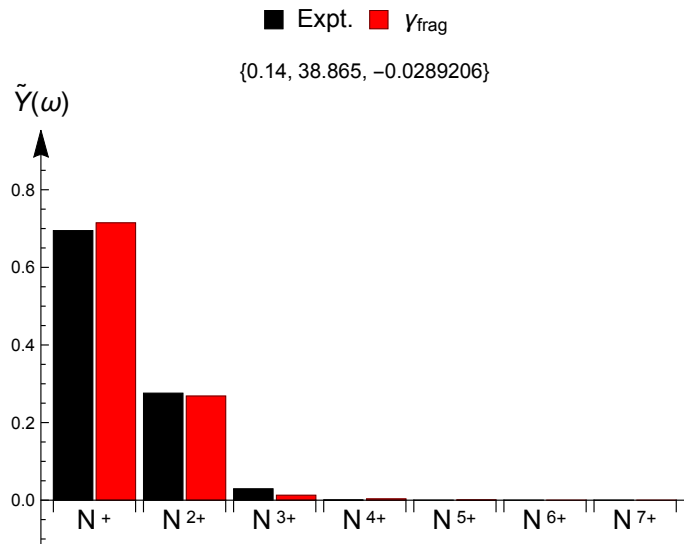

## 0.15

```
damp := 0.15
```

```
iy = dsionyieldcrateranalysisparam[damp * 0.26 * MilliJouleToHartree, photonenergy,
  tauX, nintdata, True, True, 1 / 1000, optfNppN, 1 - optfNppN, optGaFra]
iynorm = 1 / Total[iy[[2 ;; 8]]] * iy
Total[iynorm[[2 ;; 8]]]
```

```
{0.981254, 0.0132415, 0.00515062, 0.000269535,
  0.0000745511,  $9.21134 \times 10^{-6}$ ,  $9.11717 \times 10^{-8}$ ,  $1.59427 \times 10^{-10}$ ,
  0.979031, 0.000416761,  $-8.7268 \times 10^{-141}$ ,  $-2.70209 \times 10^{-168}$ }
```

```
{52.3461, 0.706383, 0.274765, 0.0143787, 0.00397701, 0.000491389,  $4.86365 \times 10^{-6}$ ,
   $8.50481 \times 10^{-9}$ , 52.2275, 0.0222326,  $-4.65541 \times 10^{-139}$ ,  $-1.44146 \times 10^{-166}$ }
```

1.

```
plotiy = Partition[Riffle[normOleg7, iynorm[[2 ;; 8]]], 2]
```

```
{{0.694746, 0.706383}, {0.275684, 0.274765},
  {0.0293036, 0.0143787}, {0.000266625, 0.00397701},
  {0., 0.000491389}, {0.,  $4.86365 \times 10^{-6}$ }, {0.,  $8.50481 \times 10^{-9}$ }}
```

```
BarChart[plotiy, PlotRange → {-0.1, 0.9},
  ChartLabels → {Placed[{"N +", "N 2+", "N 3+", "N 4+", "N 5+", "N 6+", "N 7+"}, Below],
    Placed[{}, Above]},
  ChartLegends → Placed[{"Expt.", "γfrag"}, Top],
  ChartStyle → {Black, Red}, AxesLabel → {"", "Ỹ(ω)"},
  AxesStyle → {{Arrowheads[Automatic], AbsoluteThickness[0.6]},
    {Arrowheads[Automatic], AbsoluteThickness[0.6]}},
  LabelStyle → {FontFamily → "Arial"},
  PlotLabel → {damp, optGaFra / gammaFrag,
    (iynorm[[2 ;; 8]] - normOleg7).Table[i, {i, 1, 7}]}]
```

■ Expt. ■ γ<sub>frag</sub>

{0.15, 38.865, -0.0176475}

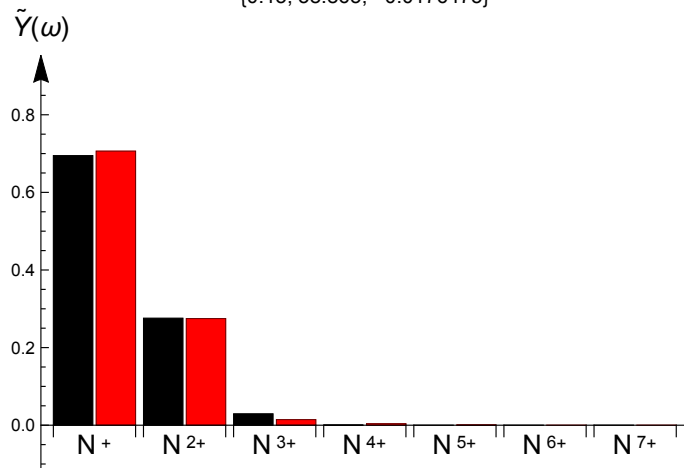

## 0.16

```
damp := 0.16
```

```
iy = dsionyieldcrateranalysisparam[damp * 0.26 * MilliJouleToHartree, photonenergy,
  tauX, nintdata, True, True, 1 / 1000, optfNppN, 1 - optfNppN, optGaFra]
iynorm = 1 / Total[iy[[2 ;; 8]]] * iy
Total[iynorm[[2 ;; 8]]]
```

```
{0.980217, 0.0138106, 0.00555423, 0.000317077,
  0.0000888681, 0.0000116291, 1.23095 × 10-7, 2.29861 × 10-10,
  0.9779, 0.000433713, 4.38104 × 10-176, -6.95805 × 10-236}
```

```
{49.5497, 0.698121, 0.280765, 0.0160281, 0.00449226, 0.000587848, 6.22243 × 10-6,
  1.16194 × 10-8, 49.4326, 0.0219241, 2.2146 × 10-174, -3.51727 × 10-234}
```

```
1.
```

```
plotiy = Partition[Riffle[normOleg7, iynorm[[2 ;; 8]]], 2]
```

```
{{0.694746, 0.698121}, {0.275684, 0.280765},
 {0.0293036, 0.0160281}, {0.000266625, 0.00449226},
 {0., 0.000587848}, {0., 6.22243 × 10-6}, {0., 1.16194 × 10-8}}
```

```
BarChart[plotiy, PlotRange → {-0.1, 0.9},
  ChartLabels → {Placed[{"N +", "N 2+", "N 3+", "N 4+", "N 5+", "N 6+", "N 7+"}, Below],
    Placed[{}, Above]},
  ChartLegends → Placed[{"Expt.", "γfrag"}, Top],
  ChartStyle → {Black, Red}, AxesLabel → {"", "Ỹ(ω)"},
  AxesStyle → {{Arrowheads[Automatic], AbsoluteThickness[0.6]},
    {Arrowheads[Automatic], AbsoluteThickness[0.6]}},
  LabelStyle → {FontFamily → "Arial"},
  PlotLabel → {damp, optGaFra / gammaFrag,
    (iynorm[[2 ;; 8]] - normOleg7).Table[i, {i, 1, 7}]}]
```

■ Expt. ■ γ<sub>frag</sub>

{0.16, 38.865, -0.00641046}

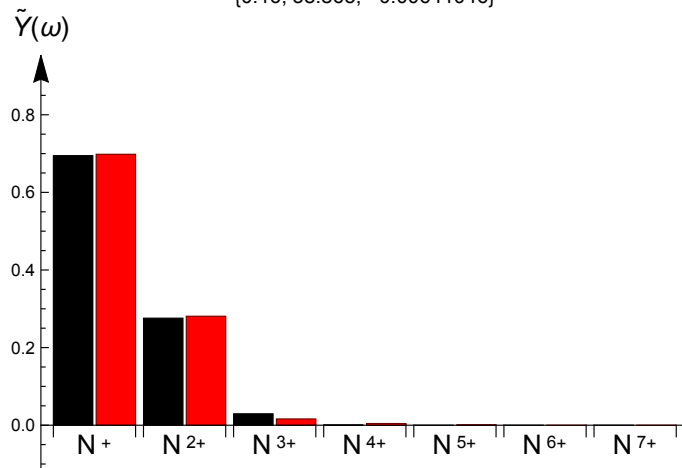

## 0.17

```
damp := 0.17
```



```
iy = dsionyieldcrateranalysisparam[damp * 0.26 * MilliJouleToHartree, photonenergy,
  tauX, nintdata, True, True, 1 / 1000, optfNppN, 1 - optfNppN, optGaFra]
iynorm = 1 / Total[iy[[2 ;; 8]]] * iy
Total[iynorm[[2 ;; 8]]]
```

```
{0.979203, 0.014351, 0.00595829, 0.000368768,
  0.000104713, 0.0000144588,  $1.63042 \times 10^{-7}$ ,  $3.23869 \times 10^{-10}$ ,
  0.976796, 0.000449711,  $1.49606 \times 10^{-174}$ ,  $-6.15202 \times 10^{-233}$ }
```

```
{47.083, 0.690038, 0.286493, 0.0177315, 0.00503491, 0.000695223,  $7.83955 \times 10^{-6}$ ,
   $1.55726 \times 10^{-8}$ , 46.9673, 0.0216235,  $7.1935 \times 10^{-173}$ ,  $-2.95808 \times 10^{-231}$ }
```

```
1.
```

```
plotiy = Partition[Riffle[normOleg7, iynorm[[2 ;; 8]]], 2]
```

```
{{0.694746, 0.690038}, {0.275684, 0.286493},
  {0.0293036, 0.0177315}, {0.000266625, 0.00503491},
  {0., 0.000695223}, {0.,  $7.83955 \times 10^{-6}$ }, {0.,  $1.55726 \times 10^{-8}$ }}
```

```
BarChart[plotiy, PlotRange → {-0.1, 0.9},
  ChartLabels → {Placed[{"N +", "N 2+", "N 3+", "N 4+", "N 5+", "N 6+", "N 7+"}, Below],
    Placed[{}, Above]},
  ChartLegends → Placed[{"Expt.", "γfrag"}, Top],
  ChartStyle → {Black, Red}, AxesLabel → {"", "Ỹ(ω)"},
  AxesStyle → {{Arrowheads[Automatic], AbsoluteThickness[0.6]},
    {Arrowheads[Automatic], AbsoluteThickness[0.6]}},
  LabelStyle → {FontFamily → "Arial"},
  PlotLabel → {damp, optGaFra / gammaFrag,
    (iynorm[[2 ;; 8]] - normOleg7).Table[i, {i, 1, 7}]}]
```

■ Expt. ■ γ<sub>frag</sub>

{0.17, 38.865, 0.0047897}

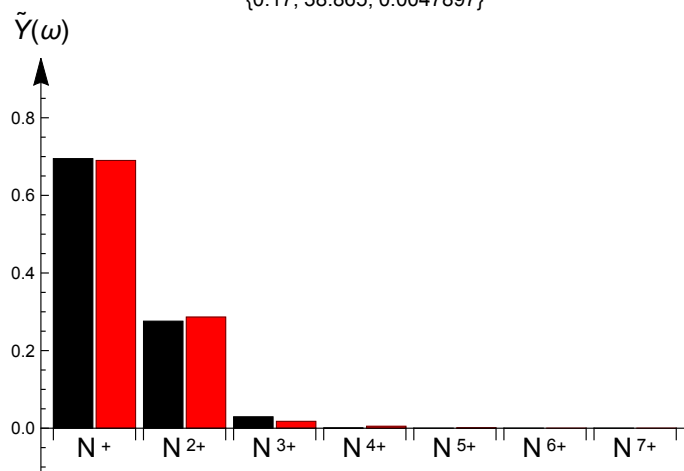

0.18

```
damp := 0.18
```

```
iy = dsionyieldcrateranalysisparam[damp * 0.26 * MilliJouleToHartree, photonenergy,
  tauX, nintdata, True, True, 1 / 1000, optfNppN, 1 - optfNppN, optGaFra]
iynorm = 1 / Total[iy[[2 ;; 8]]] * iy
Total[iynorm[[2 ;; 8]]]
```

```
{0.978209, 0.0148641, 0.00636198, 0.00042457,
  0.00012212, 0.0000177352,  $2.12315 \times 10^{-7}$ ,  $4.47103 \times 10^{-10}$ ,
  0.975718, 0.000464809,  $-5.70388 \times 10^{-131}$ ,  $4.32665 \times 10^{-165}$ }
```

```
{44.891, 0.68213, 0.291958, 0.019484, 0.00560423, 0.000813885,  $9.74335 \times 10^{-6}$ ,
   $2.0518 \times 10^{-8}$ , 44.7767, 0.0213306,  $-2.61757 \times 10^{-129}$ ,  $1.98554 \times 10^{-163}$ }
```

```
1.
```

```
plotiy = Partition[Riffle[normOleg7, iynorm[[2 ;; 8]]], 2]
```

```
{{0.694746, 0.68213}, {0.275684, 0.291958},
  {0.0293036, 0.019484}, {0.000266625, 0.00560423},
  {0., 0.000813885}, {0.,  $9.74335 \times 10^{-6}$ }, {0.,  $2.0518 \times 10^{-8}$ }}
```

```
BarChart[plotiy, PlotRange → {-0.1, 0.9},
  ChartLabels → {Placed[{"N +", "N 2+", "N 3+", "N 4+", "N 5+", "N 6+", "N 7+"}, Below],
    Placed[{}, Above]},
  ChartLegends → Placed[{"Expt.", "γfrag"}, Top],
  ChartStyle → {Black, Red}, AxesLabel → {"", "Ỹ(ω)"},
  AxesStyle → {{Arrowheads[Automatic], AbsoluteThickness[0.6]},
    {Arrowheads[Automatic], AbsoluteThickness[0.6]}},
  LabelStyle → {FontFamily → "Arial"},
  PlotLabel → {damp, optGaFra / gammaFrag,
    (iynorm[[2 ;; 8]] - normOleg7).Table[i, {i, 1, 7}]}]
```

■ Expt. ■ γ<sub>frag</sub>

{0.18, 38.865, 0.0159519}

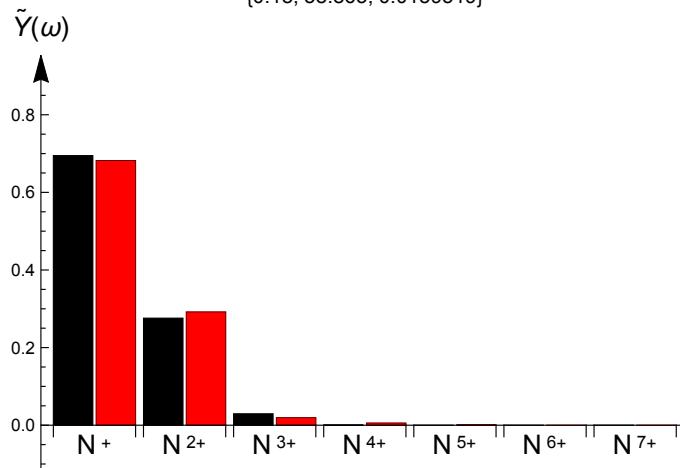

## Pulse energy for a 4 fs pulse with 280 fs fragmentation rate

```
tauX := shtdur4 * 4 / t0ToFemtoSecond
optent := 13.200000
optGaFra := optent * gammaFrag
```

### 0.21

```
damp := 0.21

iy = dsionyieldsanalysisparam[damp * 0.15 * MilliJouleToHartree, photonenergy,
    tauX, nintdata, True, True, 1 / 1000, optfNppN, 1 - optfNppN, optGaFra]
iynorm = 1 / Total[iy[[2 ;; 8]]] * iy
Total[iynorm[[2 ;; 8]]]
{0.984379, 0.0114399, 0.00399225, 0.000151318,
  0.0000352889,  $2.72836 \times 10^{-6}$ ,  $1.33086 \times 10^{-8}$ ,  $1.07801 \times 10^{-11}$ ,
   $0.982454$ ,  $0.000361989$ ,  $2.69594 \times 10^{-60}$ ,  $-3.76671 \times 10^{-245}$ }

{63.0144, 0.732317, 0.255561, 0.00968655, 0.002259, 0.000174655,  $8.51943 \times 10^{-7}$ ,
   $6.90082 \times 10^{-10}$ , 62.8912, 0.0231725,  $1.72579 \times 10^{-58}$ ,  $-2.41124 \times 10^{-243}$ }

1.

plotiy = Partition[Riffle[normOleg4, iynorm[[2 ;; 8]]], 2]
{{0.711226, 0.732317}, {0.277966, 0.255561}, {0.0108078, 0.00968655},
  {0., 0.002259}, {0., 0.000174655}, {0.,  $8.51943 \times 10^{-7}$ }, {0.,  $6.90082 \times 10^{-10}$ }}
```

```
BarChart[plotiy, PlotRange → {-0.1, 0.9},
  ChartLabels → {Placed[{"N +", "N 2+", "N 3+", "N 4+", "N 5+", "N 6+", "N 7+"}, Below],
    Placed[{}, Above]},
  ChartLegends → Placed[{"Expt.", "γfrag"}, Top],
  ChartStyle → {Black, Red}, AxesLabel → {"", "Ỹ(ω)",
  AxesStyle → {{Arrowheads[Automatic], AbsoluteThickness[0.6]},
    {Arrowheads[Automatic], AbsoluteThickness[0.6]}},
  LabelStyle → {FontFamily → "Arial"},
  PlotLabel → {damp, optGaFra / gammaFrag,
    (iynorm[[2 ;; 8]] - normOleg4).Table[i, {i, 1, 7}]]]
```

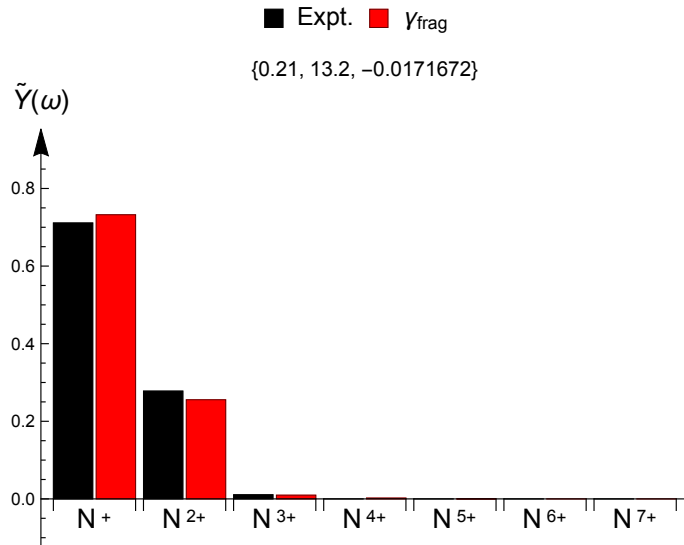

## 0.22

damp := 0.22

```
iy = dsionyieldcrateranalysisparam[damp * 0.15 * MilliJouleToHartree, photonenergy,
  tauX, nintdata, True, True, 1 / 1000, optfNppN, 1 - optfNppN, optGaFra]
```

```
iynorm = 1 / Total[iy[[2 ;; 8]]] * iy
```

```
Total[iynorm[[2 ;; 8]]]
```

```
{0.983738, 0.0118263, 0.00422078, 0.000171041, 0.0000402862, 3.24613 × 10-6,
  1.66219 × 10-8, 1.41209 × 10-11, 0.98175, 0.000373687, 2.7054 × 10-60, 1.74042 × 10-231}
```

```
{60.4944, 0.72725, 0.259554, 0.010518, 0.00247737, 0.000199619, 1.02215 × 10-6,
  8.68358 × 10-10, 60.3721, 0.0229796, 1.66367 × 10-58, 1.07026 × 10-229}
```

1.

```
plotiy = Partition[Riffle[normOleg4, iynorm[[2 ;; 8]]], 2]
```

```
{{0.711226, 0.72725}, {0.277966, 0.259554}, {0.0108078, 0.010518},
  {0., 0.00247737}, {0., 0.000199619}, {0., 1.02215 × 10-6}, {0., 8.68358 × 10-10}}
```

```
BarChart[plotiy, PlotRange → {-0.1, 0.9},
  ChartLabels → {Placed[{"N +", "N 2+", "N 3+", "N 4+", "N 5+", "N 6+", "N 7+"}, Below],
    Placed[{}, Above]},
  ChartLegends → Placed[{"Expt.", "γfrag"}, Top],
  ChartStyle → {Black, Red}, AxesLabel → {"", "Ỹ(ω)",
  AxesStyle → {{Arrowheads[Automatic], AbsoluteThickness[0.6]},
    {Arrowheads[Automatic], AbsoluteThickness[0.6]}},
  LabelStyle → {FontFamily → "Arial"},
  PlotLabel → {damp, optGaFra / gammaFrag,
    (iynorm[[2 ;; 8]] - normOleg4).Table[i, {i, 1, 7}]]]
```

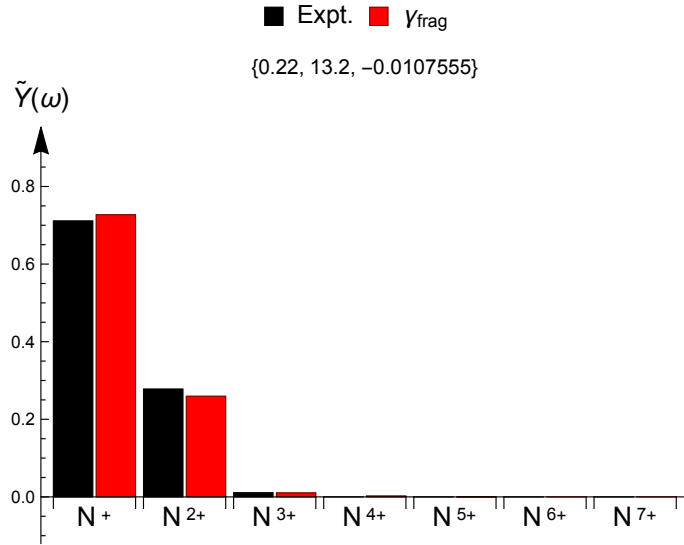

## 0.23

damp := 0.23

```
iy = dsionyieldcrateranalysisparam[damp * 0.15 * MilliJouleToHartree, photonenergy,
  tauX, nintdata, True, True, 1 / 1000, optfNppN, 1 - optfNppN, optGaFra]
```

```
iynorm = 1 / Total[iy[[2 ;; 8]]] * iy
```

```
Total[iynorm[[2 ;; 8]]]
```

```
{0.983106, 0.0122013, 0.0044506, 0.000192147, 0.0000457053, 3.83055 × 10-6,
  2.05477 × 10-8, 1.82701 × 10-11, 0.981055, 0.000385, 2.92124 × 10-60, -2.28113 × 10-182}
```

```
{58.1938, 0.722245, 0.263448, 0.0113739, 0.00270547, 0.000226745, 1.2163 × 10-6,
  1.08148 × 10-9, 58.0724, 0.0227896, 1.72919 × 10-58, -1.35029 × 10-180}
```

1.

```
plotiy = Partition[Riffle[normOleg4, iynorm[[2 ;; 8]]], 2]
```

```
{{0.711226, 0.722245}, {0.277966, 0.263448}, {0.0108078, 0.0113739},
  {0., 0.00270547}, {0., 0.000226745}, {0., 1.2163 × 10-6}, {0., 1.08148 × 10-9}}
```

```
BarChart[plotiy, PlotRange → {-0.1, 0.9},
  ChartLabels → {Placed[{"N +", "N 2+", "N 3+", "N 4+", "N 5+", "N 6+", "N 7+"}, Below],
    Placed[{}, Above]},
  ChartLegends → Placed[{"Expt.", "γfrag"}, Top],
  ChartStyle → {Black, Red}, AxesLabel → {"", "Ỹ(ω)"},
  AxesStyle → {{Arrowheads[Automatic], AbsoluteThickness[0.6]},
    {Arrowheads[Automatic], AbsoluteThickness[0.6]}},
  LabelStyle → {FontFamily → "Arial"},
  PlotLabel → {damp, optGaFra / gammaFrag,
    (iynorm[[2 ;; 8]] - normOleg4).Table[i, {i, 1, 7}]]]
```

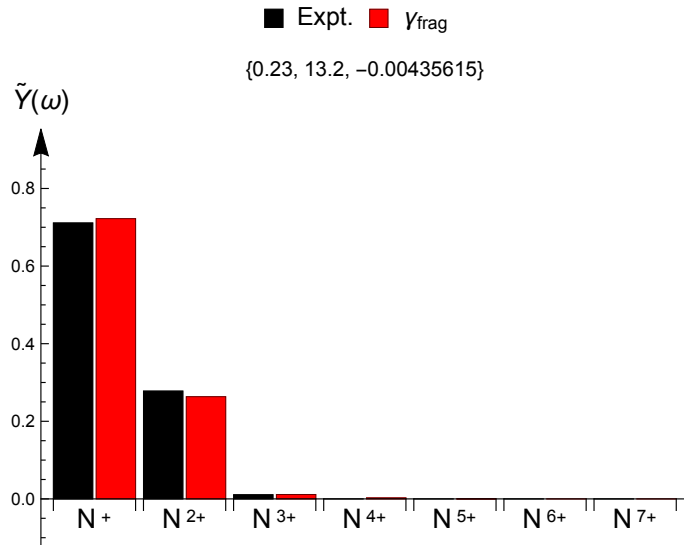

## 0.24

damp := 0.24

```
iy = dsionyieldcrateranalysisparam[damp * 0.15 * MilliJouleToHartree, photonenergy,
  tauX, nintdata, True, True, 1 / 1000, optfNppN, 1 - optfNppN, optGaFra]
```

```
iynorm = 1 / Total[iy[[2 ;; 8]]] * iy
```

```
Total[iynorm[[2 ;; 8]]]
```

```
{0.982482, 0.0125655, 0.0046815, 0.000214647,
  0.0000515584, 4.48633 × 10-6, 2.51627 × 10-8, 2.33729 × 10-11,
  0.980371, 0.000395944, 2.44739 × 10-60, 1.29476 × 10-219}
```

```
{56.0852, 0.717302, 0.267244, 0.0122532, 0.00294322, 0.000256103, 1.43641 × 10-6,
  1.33425 × 10-9, 55.9646, 0.0226025, 1.39709 × 10-58, 7.39117 × 10-218}
```

1.

```
plotiy = Partition[Riffle[normOleg4, iynorm[[2 ;; 8]]], 2]
```

```
{{0.711226, 0.717302}, {0.277966, 0.267244}, {0.0108078, 0.0122532},
  {0., 0.00294322}, {0., 0.000256103}, {0., 1.43641 × 10-6}, {0., 1.33425 × 10-9}}
```

```
BarChart[plotiy, PlotRange → {-0.1, 0.9},
  ChartLabels → {Placed[{"N +", "N 2+", "N 3+", "N 4+", "N 5+", "N 6+", "N 7+"}, Below],
    Placed[{}, Above]},
  ChartLegends → Placed[{"Expt.", "γfrag"}, Top],
  ChartStyle → {Black, Red}, AxesLabel → {"", "Ỹ(ω)",
  AxesStyle → {{Arrowheads[Automatic], AbsoluteThickness[0.6]},
    {Arrowheads[Automatic], AbsoluteThickness[0.6]}},
  LabelStyle → {FontFamily → "Arial"},
  PlotLabel → {damp, optGaFra / gammaFrag,
    (iynorm[[2 ;; 8]] - normOleg4).Table[i, {i, 1, 7}]]]
```

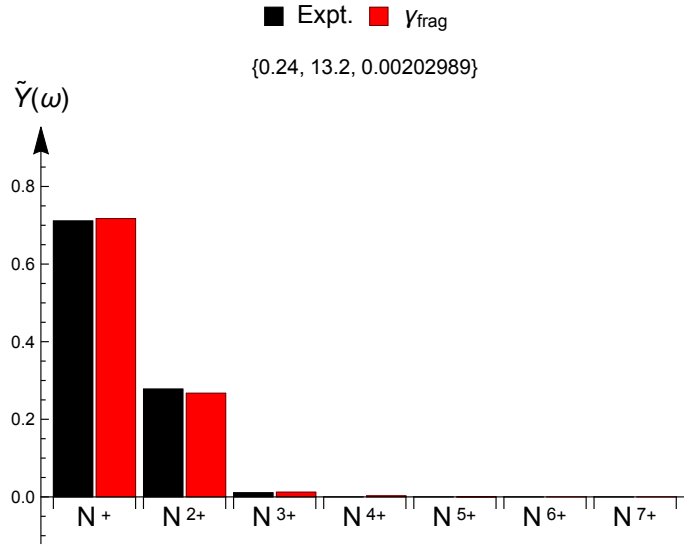

## 0.25

damp := 0.25

```
iy = dsionyieldcrateranalysisparam[damp * 0.15 * MilliJouleToHartree, photonenergy,
  tauX, nintdata, True, True, 1 / 1000, optfNppN, 1 - optfNppN, optGaFra]
```

```
iynorm = 1 / Total[iy[[2 ;; 8]]] * iy
```

```
Total[iynorm[[2 ;; 8]]]
```

```
{0.981866, 0.0129189, 0.00491325, 0.000238545,
  0.0000578567, 5.21821 × 10-6, 3.05489 × 10-8, 2.95923 × 10-11,
  0.979696, 0.000406526, 2.82149 × 10-60, 1.02578 × 10-215}
```

```
{54.1456, 0.712421, 0.270944, 0.0131547, 0.00319055, 0.000287761, 1.68464 × 10-6,
  1.63189 × 10-9, 54.026, 0.0224181, 1.55593 × 10-58, 5.65673 × 10-214}
```

1.

```
plotiy = Partition[Riffle[normOleg4, iynorm[[2 ;; 8]]], 2]
```

```
{{0.711226, 0.712421}, {0.277966, 0.270944}, {0.0108078, 0.0131547},
  {0., 0.00319055}, {0., 0.000287761}, {0., 1.68464 × 10-6}, {0., 1.63189 × 10-9}}
```

```
BarChart[plotiy, PlotRange → {-0.1, 0.9},
  ChartLabels → {Placed[{"N +", "N 2+", "N 3+", "N 4+", "N 5+", "N 6+", "N 7+"}, Below],
    Placed[{}, Above]},
  ChartLegends → Placed[{"Expt.", "γfrag"}, Top],
  ChartStyle → {Black, Red}, AxesLabel → {"", "Ỹ(ω)"},
  AxesStyle → {{Arrowheads[Automatic], AbsoluteThickness[0.6]},
    {Arrowheads[Automatic], AbsoluteThickness[0.6]}},
  LabelStyle → {FontFamily → "Arial"},
  PlotLabel → {damp, optGaFra / gammaFrag,
    (iynorm[[2 ;; 8]] - normOleg4).Table[i, {i, 1, 7}]]]
```

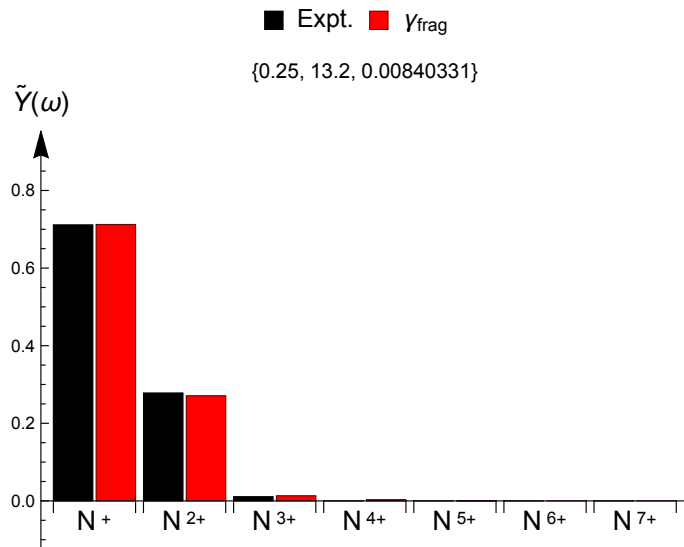

## Pulse energy for a 4 fs pulse with 80 fs fragmentation rate

```
tauX := shtdur4 * 4 / t0ToFemtoSecond
optent := 38.864973
optGaFra := optent * gammaFrag
```

### 0.21

```
damp := 0.21

iy = dsionyieldcrateranalysisparam[damp * 0.15 * MilliJouleToHartree, photonenergy,
  tauX, nintdata, True, True, 1 / 1000, optfNppN, 1 - optfNppN, optGaFra]
iynorm = 1 / Total[iy[[2 ;; 8]]] * iy
Total[iynorm[[2 ;; 8]]]
{0.984379, 0.0114412, 0.00398917, 0.000152586,
  0.0000354891, 2.77133 × 10-6, 1.35832 × 10-8, 1.10653 × 10-11,
  0.982454, 0.000361989, 5.35813 × 10-148, -3.46688 × 10-179}

{63.0154, 0.732414, 0.255368, 0.00976788, 0.00227185, 0.000177408, 8.69534 × 10-7,
  7.08348 × 10-10, 62.8922, 0.0231729, 3.43003 × 10-146, -2.21934 × 10-177}

1.
```



```

plotiy = Partition[Riffle[normOleg4, iynorm[[2 ;; 8]]], 2]
{{0.711226, 0.732414}, {0.277966, 0.255368}, {0.0108078, 0.00976788},
 {0., 0.00227185}, {0., 0.000177408}, {0.,  $8.69534 \times 10^{-7}$ }, {0.,  $7.08348 \times 10^{-10}$ }}

```

```

BarChart[plotiy, PlotRange → {-0.1, 0.9},
  ChartLabels → {Placed[{"N +", "N 2+", "N 3+", "N 4+", "N 5+", "N 6+", "N 7+"}, Below],
    Placed[{}, Above]},
  ChartLegends → Placed[{"Expt.", " $\gamma_{\text{frag}}$ "}, Top],
  ChartStyle → {Black, Red}, AxesLabel → {"", " $\tilde{Y}(\omega)$ "},
  AxesStyle → {{Arrowheads[Automatic], AbsoluteThickness[0.6]},
    {Arrowheads[Automatic], AbsoluteThickness[0.6]}},
  LabelStyle → {FontFamily → "Arial"},
  PlotLabel → {damp, optGaFra / gammaFrag,
    (iynorm[[2 ;; 8]] - normOleg4).Table[i, {i, 1, 7}]}]

```

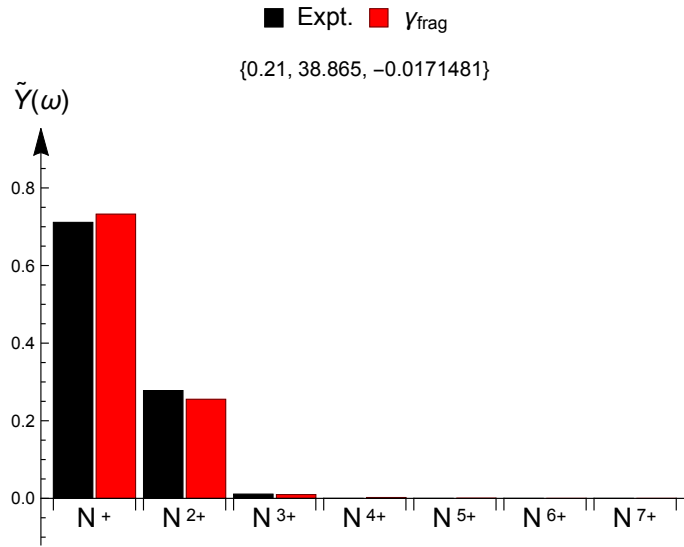

## 0.22

```
damp := 0.22
```

```

iy = dsionyieldcrateranalysisparam[damp * 0.15 * MilliJouleToHartree, photonenergy,
  tauX, nintdata, True, True, 1 / 1000, optfNppN, 1 - optfNppN, optGaFra]

```

```
iynorm = 1 / Total[iy[[2 ;; 8]]] * iy
```

```
Total[iynorm[[2 ;; 8]]]
```

```

{0.983739, 0.0118277, 0.00421747, 0.000172404,
 0.0000405002,  $3.2946 \times 10^{-6}$ ,  $1.69473 \times 10^{-8}$ ,  $1.44757 \times 10^{-11}$ ,
 0.98175, 0.000373687,  $-1.88587 \times 10^{-147}$ ,  $2.15614 \times 10^{-174}$ }

```

```

{60.4953, 0.727349, 0.259355, 0.0106021, 0.00249058, 0.000202602,  $1.04218 \times 10^{-6}$ ,
  $8.90189 \times 10^{-10}$ , 60.373, 0.02298,  $-1.15972 \times 10^{-145}$ ,  $1.32593 \times 10^{-172}$ }

```

1.

```
plotiy = Partition[Riffle[normOleg4, iynorm[[2 ;; 8]]], 2]
```

```

{{0.711226, 0.727349}, {0.277966, 0.259355}, {0.0108078, 0.0106021},
 {0., 0.00249058}, {0., 0.000202602}, {0.,  $1.04218 \times 10^{-6}$ }, {0.,  $8.90189 \times 10^{-10}$ }}

```

```
BarChart[plotiy, PlotRange → {-0.1, 0.9},
  ChartLabels → {Placed[{"N +", "N 2+", "N 3+", "N 4+", "N 5+", "N 6+", "N 7+"}, Below],
    Placed[{}, Above]},
  ChartLegends → Placed[{"Expt.", "γfrag"}, Top],
  ChartStyle → {Black, Red}, AxesLabel → {"", "Ỹ(ω)"},
  AxesStyle → {{Arrowheads[Automatic], AbsoluteThickness[0.6]},
    {Arrowheads[Automatic], AbsoluteThickness[0.6]}},
  LabelStyle → {FontFamily → "Arial"},
  PlotLabel → {damp, optGaFra / gammaFrag,
    (iynorm[[2 ;; 8]] - normOleg4).Table[i, {i, 1, 7}]]]
```

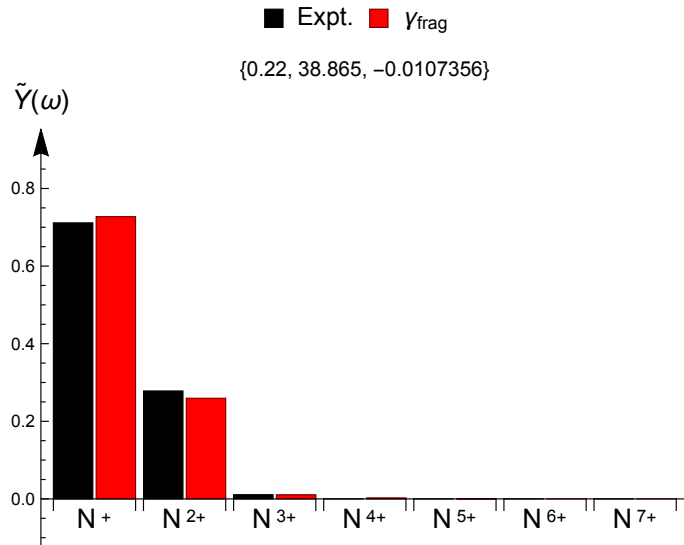

## 0.23

damp := 0.23

```
iy = dsionyieldcrateranalysisparam[damp * 0.15 * MilliJouleToHartree, photonenergy,
  tauX, nintdata, True, True, 1 / 1000, optfNppN, 1 - optfNppN, optGaFra]
```

```
iynorm = 1 / Total[iy[[2 ;; 8]]] * iy
```

```
Total[iynorm[[2 ;; 8]]]
```

```
{0.983107, 0.0122029, 0.00444704, 0.000193607, 0.0000459333, 3.88488 × 10-6,
  2.093 × 10-8, 1.8707 × 10-11, 0.981055, 0.000385, 1.01061 × 10-174, -2.53544 × 10-229}
```

```
{58.1948, 0.722347, 0.263242, 0.0114606, 0.00271901, 0.000229964, 1.23895 × 10-6,
  1.10736 × 10-9, 58.0734, 0.02279, 5.98228 × 10-173, -1.50085 × 10-227}
```

1.

```
plotiy = Partition[Riffle[normOleg4, iynorm[[2 ;; 8]]], 2]
```

```
{{0.711226, 0.722347}, {0.277966, 0.263242}, {0.0108078, 0.0114606},
  {0., 0.00271901}, {0., 0.000229964}, {0., 1.23895 × 10-6}, {0., 1.10736 × 10-9}}
```

```
BarChart[plotiy, PlotRange → {-0.1, 0.9},
  ChartLabels → {Placed[{"N +", "N 2+", "N 3+", "N 4+", "N 5+", "N 6+", "N 7+"}, Below],
    Placed[{}, Above]},
  ChartLegends → Placed[{"Expt.", "γfrag"}, Top],
  ChartStyle → {Black, Red}, AxesLabel → {"", "Ỹ(ω)",
  AxesStyle → {{Arrowheads[Automatic], AbsoluteThickness[0.6]},
    {Arrowheads[Automatic], AbsoluteThickness[0.6]}},
  LabelStyle → {FontFamily → "Arial"},
  PlotLabel → {damp, optGaFra / gammaFrag,
    (iynorm[[2 ;; 8]] - normOleg4).Table[i, {i, 1, 7}]]]
```

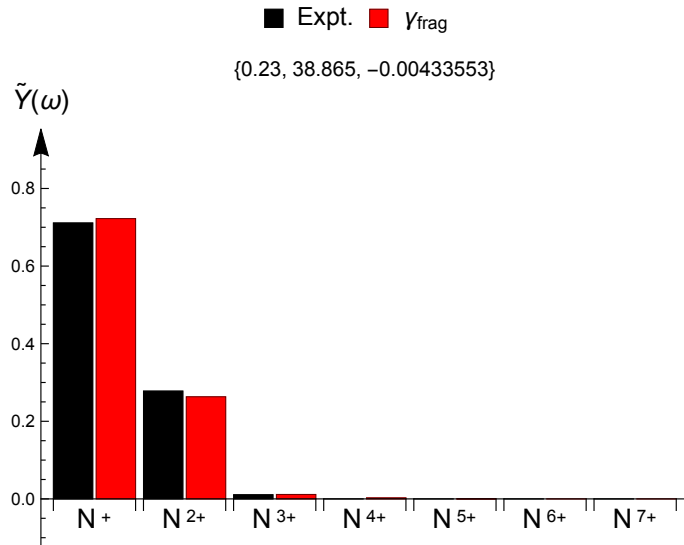

## 0.24

damp := 0.24

```
iy = dsionyieldcrateranalysisparam[damp * 0.15 * MilliJouleToHartree, photonenergy,
  tauX, nintdata, True, True, 1 / 1000, optfNppN, 1 - optfNppN, optGaFra]
```

```
iynorm = 1 / Total[iy[[2 ;; 8]]] * iy
```

```
Total[iynorm[[2 ;; 8]]]
```

```
{0.982483, 0.0125671, 0.0046777, 0.000216205,
  0.0000518002, 4.54688 × 10-6, 2.56086 × 10-8, 2.39058 × 10-11,
  0.980371, 0.000395944, -9.64172 × 10-133, 7.5627 × 10-165}
```

```
{56.0861, 0.717408, 0.267032, 0.0123423, 0.00295707, 0.000259564, 1.46189 × 10-6,
  1.36469 × 10-9, 55.9656, 0.0226029, -5.50408 × 10-131, 4.31725 × 10-163}
```

1.

```
plotiy = Partition[Riffle[normOleg4, iynorm[[2 ;; 8]]], 2]
```

```
{{0.711226, 0.717408}, {0.277966, 0.267032}, {0.0108078, 0.0123423},
  {0., 0.00295707}, {0., 0.000259564}, {0., 1.46189 × 10-6}, {0., 1.36469 × 10-9}}
```

```
BarChart[plotiy, PlotRange → {-0.1, 0.9},
  ChartLabels → {Placed[{"N +", "N 2+", "N 3+", "N 4+", "N 5+", "N 6+", "N 7+"}, Below],
    Placed[{}, Above]},
  ChartLegends → Placed[{"Expt.", "γfrag"}, Top],
  ChartStyle → {Black, Red}, AxesLabel → {"", "Ỹ(ω)"},
  AxesStyle → {{Arrowheads[Automatic], AbsoluteThickness[0.6]},
    {Arrowheads[Automatic], AbsoluteThickness[0.6]}},
  LabelStyle → {FontFamily → "Arial"},
  PlotLabel → {damp, optGaFra / gammaFrag,
    (iynorm[[2 ;; 8]] - normOleg4).Table[i, {i, 1, 7}]]]
```

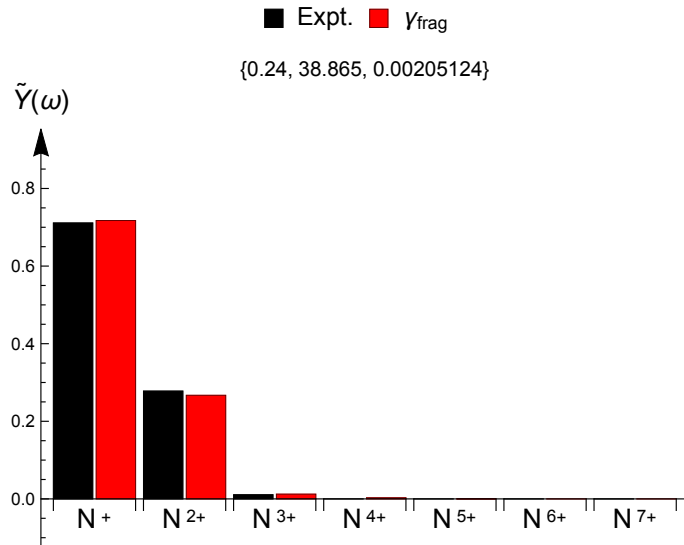

## 0.25

damp := 0.25

```
iy = dsionyieldcrateranalysisparam[damp * 0.15 * MilliJouleToHartree, photonenergy,
  tauX, nintdata, True, True, 1 / 1000, optfNppN, 1 - optfNppN, optGaFra]
```

```
iynorm = 1 / Total[iy[[2 ;; 8]]] * iy
```

```
Total[iynorm[[2 ;; 8]]]
```

```
{0.981867, 0.0129207, 0.0049092, 0.000240201,
  0.0000581124, 5.28535 × 10-6, 3.10654 × 10-8, 3.02366 × 10-11,
  0.979696, 0.000406526, 1.30073 × 10-131, -1.40994 × 10-165}
```

```
{54.1466, 0.71253, 0.270726, 0.0132463, 0.0032047, 0.000291469, 1.71315 × 10-6,
  1.66744 × 10-9, 54.0269, 0.0224185, 7.17311 × 10-130, -7.77532 × 10-164}
```

1.

```
plotiy = Partition[Riffle[normOleg4, iynorm[[2 ;; 8]]], 2]
```

```
{{0.711226, 0.71253}, {0.277966, 0.270726}, {0.0108078, 0.0132463},
  {0., 0.0032047}, {0., 0.000291469}, {0., 1.71315 × 10-6}, {0., 1.66744 × 10-9}}
```

```
BarChart[plotiy, PlotRange → {-0.1, 0.9},
  ChartLabels → {Placed[{"N +", "N 2+", "N 3+", "N 4+", "N 5+", "N 6+", "N 7+"}, Below],
    Placed[{}, Above]},
  ChartLegends → Placed[{"Expt.", "γfrag"}, Top],
  ChartStyle → {Black, Red}, AxesLabel → {"", "Ỹ(ω)"},
  AxesStyle → {{Arrowheads[Automatic], AbsoluteThickness[0.6]},
    {Arrowheads[Automatic], AbsoluteThickness[0.6]}},
  LabelStyle → {FontFamily → "Arial"},
  PlotLabel → {damp, optGaFra / gammaFrag,
    (iynorm[[2 ;; 8]] - normOleg4).Table[i, {i, 1, 7}]]]
```

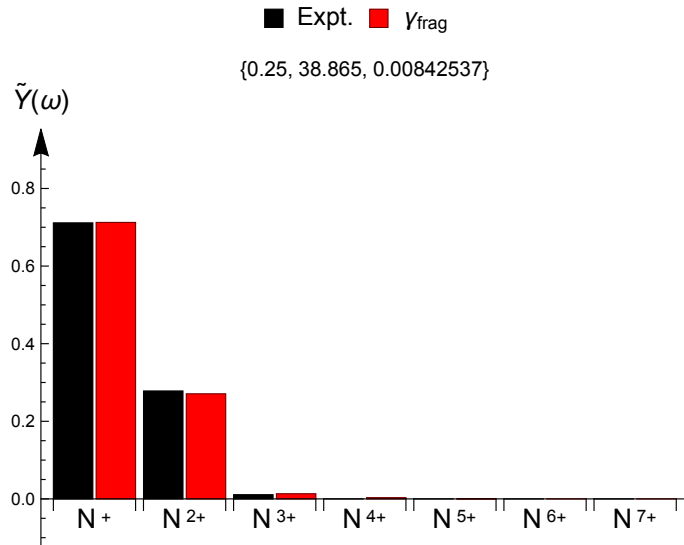

## References

- [1] S. Düsterer, P. Radcliffe, C. Bostedt, J. Bozek, A. L. Cavalieri, R. Coffee, J. T. Costello, D. Cubaynes, L. F. DiMauro, Y. Ding, G. Doumy, F. Grüner, W. Helml, W. Schweinberger, R. Kienberger, A. R. Maier, M. Messerschmidt, V. Richardson, C. Roedig, T. Tschentscher, M. Meyer, *New J. Phys.* **13**, 093024 (2011) [11 pages], *Femtosecond x-ray pulse length characterization at the Linac Coherent Light Source free-electron laser*, <http://dx.doi.org/10.1088/1367-2630/13/9/093024>
