# Supplementary material for: Rate equations for nitrogen molecules in ultrashort and intense x-ray pulses
Source: arXiv:1508.05223 ancillary file (2017-03-16)

<< PlotLegends`

General::obspkg: PlotLegends` is now obsolete. The legacy version being loaded may conflict with current functionality. See the Compatibility Guide for updating information.

```
Get["NitrogenRateEquations.m", Path -> NotebookDirectory[]]  
Get["NitrogenMoleculeRateEqs.m", Path -> NotebookDirectory[]]
```

```
HartreeToeV := 27.2113845  
eVToHartree := 1 / HartreeToeV  
JouleToHartree := 2.29371269*^17  
MilliJouleToHartree := 1*^-3 * JouleToHartree  
BohrToAngstroem := 0.5291772083  
AngstroemToBohr := 1 / BohrToAngstroem  
MicrometerToBohr := 1*^4 * AngstroemToBohr  
BohrToMicrometer := 1 / MicrometerToBohr  
t0ToSecond := 24.18884326505*^-18  
t0ToFemtoSecond := 24.18884326505*^-3  
crossSectionAUtoBarn := 1*^8 * BohrToAngstroem^2  
crossSectionAUtocm2 := crossSectionAUtoBarn * 1*^-24  
crossSectioncm2toAU := 1 / crossSectionAUtocm2  
  
neginfinity := -1000 / t0ToFemtoSecond  
posinfinity := 10 000 / t0ToFemtoSecond
```

# Average charge state from the microscopic model

Ji-Cai Liu

Department of Mathematics and Physics, North China Electric Power University, 102206 Beijing, China

Max-Planck-Institut für Kernphysik, Saupfercheckweg 1, 69117 Heidelberg, Germany

Christian Buth

Max-Planck-Institut für Kernphysik, Saupfercheckweg 1, 69117 Heidelberg, Germany

Theoretische Chemie, Physikalisch-Chemisches Institut, Ruprecht-Karls-Universität Heidelberg, Im Neuenheimer Feld 229, 69120 Heidelberg, Germany

23 September 2014

---

## Experimental parameters

Pulse energy fractions from the nitrogen\_dissociation\_first.nb *Mathematica* Notebook:

```

optdamp280 := 0.38
optdamp80 := 0.30
optdamp7 := 0.16
optdamp4 := 0.23

```

Pulse energy fraction for the 4 fs pulse with respect to a pulse energy of 0.26 mJ instead of 0.15 mJ and vice versa for the 7 fs pulse:

```

optdamp4 * 0.15 / 0.26
0.132692

```

```

optdamp7 * 0.26 / 0.15
0.277333

```

```

photonenergy := 1100 * eVToHartree
gamma280 := 4.059357 * gammaFrag
gamma80 := 12.000000 * gammaFrag
optfNppN := 0.26

```

```

newMatthias280 := {204.331, 105.281, 27.561, 13.151, 9.881, 0.587, 0.000}
normOleg280 = 1 / Total[newMatthias280] * newMatthias280
{0.56634, 0.291805, 0.0763903, 0.0364504, 0.027387, 0.00162698, 0.}

```

```

chrgExpt280 = normOleg280.Table[i, {i, 1, 7}]
1.67162

```

```

newMatthias80 := {218.068, 103.774, 26.075, 9.804, 3.315, 0.000, 0.000}
normOleg80 = 1 / Total[newMatthias80] * newMatthias80
{0.604006, 0.287434, 0.0722227, 0.0271552, 0.00918191, 0., 0.}

```

```

chrgExpt80 = normOleg80.Table[i, {i, 1, 7}]
1.55007

```

```

newMatthias7 := {221.485, 87.888, 9.342, 0.085, 0.000, 0.000, 0.000}
normOleg7 = 1 / Total[newMatthias7] * newMatthias7
{0.694746, 0.275684, 0.0293036, 0.000266625, 0., 0., 0.}

```

```

chrgExpt7 = normOleg7.Table[i, {i, 1, 7}]
1.33509

```

```

newMatthias4 := {92.985, 36.341, 1.413, 0, 0, 0, 0}
normOleg4 = 1 / Total[newMatthias4] * newMatthias4
{0.711226, 0.277966, 0.0108078, 0., 0., 0., 0.}

```

```

chrgExpt4 = normOleg4.Table[i, {i, 1, 7}]
1.29958

```

## Average charge state for 280 fs

### With SCH, DCHTS, and DCHSS and constant pulse energy

```
optolegiy = dsionyieldcrateranalysisparam[
  optdamp280 * 0.26 * MilliJouleToHartree, photonenergy, 280 / t0ToFemtoSecond,
  nintdata, True, True, 1 / 1000, optfNppN, 1 - optfNppN, gamma280]
{0.962077, 0.0214849, 0.0114973, 0.00194797, 0.00211792, 0.000765547, 0.000103569,
  6.04188 × 10-6, 0.958498, 0.00063857, 3.46375 × 10-20, -2.89667 × 10-110}

Total[optolegiy[[1 ;; 8]]]
1.

optolegiynorm := 1 / Total[optolegiy[[2 ;; 8]]] * optolegiy
optolegiynorm[[2 ;; 8]]
{0.566536, 0.303173, 0.0513661, 0.0558475, 0.0201868, 0.00273103, 0.000159319}

chrgConst280 = optolegiynorm[[2 ;; 8]].Table[i, {i, 1, 7}]
1.66881
```

### With SCH, DCHTS, and DCHSS

```
optolegiy = dsionyieldcrateranalysisparam[
  optdamp280 * 0.26 * MilliJouleToHartree, photonenergy, 280 / t0ToFemtoSecond,
  nintdata, True, True, 1 / 1000, optfNppN, 1 - optfNppN, gamma280]
{0.962077, 0.0214849, 0.0114973, 0.00194797, 0.00211792, 0.000765547, 0.000103569,
  6.04188 × 10-6, 0.958498, 0.00063857, 3.46375 × 10-20, -2.89667 × 10-110}

Total[optolegiy[[1 ;; 8]]]
1.

optolegiynorm := 1 / Total[optolegiy[[2 ;; 8]]] * optolegiy
optolegiynorm[[2 ;; 8]]
{0.566536, 0.303173, 0.0513661, 0.0558475, 0.0201868, 0.00273103, 0.000159319}

chrgDCHSS280 = optolegiynorm[[2 ;; 8]].Table[i, {i, 1, 7}]
1.66881
```

### With SCH and DCHTS

```
optolegiy = dsionyieldcrateranalysisparam[
  optdamp280 * 0.26 * MilliJouleToHartree, photonenergy, 280 / t0ToFemtoSecond,
  nintdata, False, True, 1 / 1000, optfNppN, 1 - optfNppN, gamma280]
{0.962089, 0.0215589, 0.0114699, 0.00196646,
  0.00209555, 0.000768736, 0.0000472017, 4.06011 × 10-6,
  0.958498, 0.000638571, 3.47146 × 10-20, 5.84574 × 10-118}

Total[optolegiy[[1 ;; 8]]]
1.
```

```

optolegiynorm := 1 / Total[optolegiy[[2 ;; 8]]] * optolegiy
optolegiynorm[[2 ;; 8]]
{0.568675, 0.302549, 0.0518706, 0.0552758, 0.0202775, 0.00124507, 0.000107096}

chrgDCHTS280 = optolegiynorm[[2 ;; 8]].Table[i, {i, 1, 7}]
1.6601

```

## With SCH

```

optolegiy = dsionyieldcrateranalysisparam[
  optdamp280 * 0.26 * MilliJouleToHartree, photonenergy, 280 / t0ToFemtoSecond,
  nintdata, False, False, 1 / 1000, optfNppN, 1 - optfNppN, gamma280]
{0.96211, 0.0216838, 0.0114704, 0.00187173, 0.00208395, 0.000733817, 0.0000425118,
  3.618 × 10-6, 0.958498, 0.000638572, 3.48796 × 10-20, 2.60333 × 10-113}

Total[optolegiy[[1 ;; 8]]]
1.

optolegiynorm := 1 / Total[optolegiy[[2 ;; 8]]] * optolegiy
optolegiynorm[[2 ;; 8]]
{0.572285, 0.302731, 0.0493992, 0.0550002, 0.0193671, 0.00112198, 0.0000954873}

chrgSCH280 = optolegiynorm[[2 ;; 8]].Table[i, {i, 1, 7}]
1.65018

```

---

## Average charge state for 80 fs

### With SCH, DCHTS, and DCHSS and constant pulse energy

```

optolegiy = dsionyieldcrateranalysisparam[
  optdamp280 * 0.26 * MilliJouleToHartree, photonenergy, 80 / t0ToFemtoSecond,
  nintdata, True, True, 1 / 1000, optfNppN, 1 - optfNppN, gamma80]
{0.962041, 0.0212905, 0.0120186, 0.00188791,
  0.00198807, 0.000687742, 0.0000828146, 3.85623 × 10-6,
  0.958498, 0.000638571, 1.05828 × 10-54, 2.11595 × 10-115}

Total[optolegiy[[1 ;; 8]]]
1.

optolegiynorm := 1 / Total[optolegiy[[2 ;; 8]]] * optolegiy
optolegiynorm[[2 ;; 8]]
{0.560875, 0.316616, 0.049735, 0.0523735, 0.0181178, 0.00218166, 0.000101588}

chrgConst80 = optolegiynorm[[2 ;; 8]].Table[i, {i, 1, 7}]
1.6572

```

## With SCH, DCHTS, and DCHSS

```
optolegiy = dsionyieldcrateranalysisparam[
  optdamp80 * 0.26 * MilliJouleToHartree, photonenergy, 80 / t0ToFemtoSecond,
  nintdata, True, True, 1 / 1000, optfNppN, 1 - optfNppN, gamma80]
{0.967779, 0.0194633, 0.00976408, 0.00134806,
 0.00125066, 0.000359958, 0.0000337345, 1.26099 × 10-6,
 0.96453, 0.000591681, 1.17732 × 10-54, -2.66479 × 10-116}

Total[optolegiy[[1 ;; 8]]]
1.

optolegiynorm := 1 / Total[optolegiy[[2 ;; 8]]] * optolegiy
optolegiynorm[[2 ;; 8]]
{0.604055, 0.303034, 0.041838, 0.0388149, 0.0111715, 0.00104697, 0.0000391357}

chrgDCHSS80 = optolegiynorm[[2 ;; 8]].Table[i, {i, 1, 7}]
1.55331
```

## With SCH and DCHTS

```
optolegiy = dsionyieldcrateranalysisparam[
  optdamp80 * 0.26 * MilliJouleToHartree, photonenergy, 80 / t0ToFemtoSecond,
  nintdata, False, True, 1 / 1000, optfNppN, 1 - optfNppN, gamma80]
{0.967813, 0.0196629, 0.00966588, 0.00136567, 0.00118101, 0.000301941,
 9.35193 × 10-6, 5.18844 × 10-7, 0.96453, 0.000591681, -4.8649 × 10-44, 6.17881 × 10-157}

Total[optolegiy[[1 ;; 8]]]
1.

optolegiynorm := 1 / Total[optolegiy[[2 ;; 8]]] * optolegiy
optolegiynorm[[2 ;; 8]]
{0.61089, 0.300302, 0.0424288, 0.0366919, 0.00938077, 0.000290548, 0.0000161196}

chrgDCHTS80 = optolegiynorm[[2 ;; 8]].Table[i, {i, 1, 7}]
1.53431
```

## With only SCH

```
optolegiy = dsionyieldcrateranalysisparam[
  optdamp80 * 0.26 * MilliJouleToHartree, photonenergy, 80 / t0ToFemtoSecond,
  nintdata, False, False, 1 / 1000, optfNppN, 1 - optfNppN, gamma80]
{0.967872, 0.0200107, 0.00956646, 0.00115758, 0.00113239, 0.000253824,
 7.02306 × 10-6, 3.86425 × 10-7, 0.96453, 0.000591681, 9.70764 × 10-55, -1.2991 × 10-154}

Total[optolegiy[[1 ;; 8]]]
1.
```

```

optolegiynorm := 1 / Total[optolegiy[[2 ;; 8]]] * optolegiy
optolegiynorm[[2 ;; 8]]
{0.622836, 0.297758, 0.0360299, 0.0352459, 0.0079003, 0.000218594, 0.0000120275}

chrgSCH80 = optolegiynorm[[2 ;; 8]].Table[i, {i, 1, 7}]
1.50832

```

## Average charge state for 7 fs

### With SCH, DCHTS, and DCHSS and constant pulse energy

```

optolegiy = dsionyieldcrateranalysisparam[
  optdamp280 * 0.26 * MilliJouleToHartree, photonenergy, 7 / t0ToFemtoSecond,
  nintdata, True, True, 1 / 1000, optfNppN, 1 - optfNppN, gamma280]
{0.961957, 0.020865, 0.0137438, 0.0020588, 0.00100753, 0.00034911, 0.0000183815,
  1.97924 × 10-7, 0.958498, 0.000638571, 3.21255 × 10-20, 6.77686 × 10-114}

Total[optolegiy[[1 ;; 8]]]
1.

optolegiynorm := 1 / Total[optolegiy[[2 ;; 8]]] * optolegiy
optolegiynorm[[2 ;; 8]]
{0.548461, 0.361272, 0.054118, 0.026484, 0.00917677, 0.000483179, 5.20266 × 10-6}

chrgConst7 = optolegiynorm[[2 ;; 8]].Table[i, {i, 1, 7}]
1.58811

```

### With SCH, DCHTS, and DCHSS

```

optolegiy = dsionyieldcrateranalysisparam[
  optdamp7 * 0.26 * MilliJouleToHartree, photonenergy, 7 / t0ToFemtoSecond,
  nintdata, True, True, 1 / 1000, optfNppN, 1 - optfNppN, gamma280]
{0.980203, 0.0137252, 0.00563491, 0.00029332, 0.000124136, 0.0000188496,
  3.93605 × 10-7, 1.73494 × 10-9, 0.9779, 0.000433713, 2.14226 × 10-20, 1.82178 × 10-146}

Total[optolegiy[[1 ;; 8]]]
1.

optolegiynorm := 1 / Total[optolegiy[[2 ;; 8]]] * optolegiy
optolegiynorm[[2 ;; 8]]
{0.693304, 0.284637, 0.0148165,
  0.00627051, 0.000952154, 0.0000198823, 8.76372 × 10-8}

chrgDCHSS7 = optolegiynorm[[2 ;; 8]].Table[i, {i, 1, 7}]
1.33699

```

## With SCH and DCHTS

```
optolegiy = dsionyieldcrateranalysisparam[
  optdamp7 * 0.26 * MilliJouleToHartree, photonenergy, 7 / t0ToFemtoSecond,
  nintdata, False, True, 1 / 1000, optfNppN, 1 - optfNppN, gamma280]
{0.980294, 0.0142545, 0.00522493, 0.0001741, 0.0000492653, 3.04385 × 10-6,
  6.87761 × 10-9, 1.40418 × 10-10, 0.9779, 0.000433713, 2.21697 × 10-20, 1.20916 × 10-200}

Total[optolegiy[[1 ;; 8]]]
1.

optolegiynorm := 1 / Total[optolegiy[[2 ;; 8]]] * optolegiy
optolegiynorm[[2 ;; 8]]
{0.723364, 0.265147, 0.00883498,
  0.00250004, 0.000154465, 3.49015 × 10-7, 7.12571 × 10-9}

chrgDCHTS7 = optolegiynorm[[2 ;; 8]].Table[i, {i, 1, 7}]
1.29094
```

## With only SCH

```
optolegiy = dsionyieldcrateranalysisparam[
  optdamp7 * 0.26 * MilliJouleToHartree, photonenergy, 7 / t0ToFemtoSecond,
  nintdata, False, False, 1 / 1000, optfNppN, 1 - optfNppN, gamma280]
{0.980465, 0.0152468, 0.00423521, 0.0000193033, 0.0000332884, 6.52437 × 10-7,
  1.27566 × 10-9, 2.85109 × 10-11, 0.9779, 0.000433713, 2.3709 × 10-20, -3.5113 × 10-199}

Total[optolegiy[[1 ;; 8]]]
1.

optolegiynorm := 1 / Total[optolegiy[[2 ;; 8]]] * optolegiy
optolegiynorm[[2 ;; 8]]
{0.780476, 0.216798, 0.000988124,
  0.00170402, 0.0000333979, 6.53004 × 10-8, 1.45946 × 10-9}

chrgSCH7 = optolegiynorm[[2 ;; 8]].Table[i, {i, 1, 7}]
1.22402
```

---

## Average charge state for 4 fs

### With SCH, DCHTS, and DCHSS and constant pulse energy

```
optolegiy = dsionyieldcrateranalysisparam[
  optdamp280 * 0.26 * MilliJouleToHartree, photonenergy, 4 / t0ToFemtoSecond,
  nintdata, True, True, 1 / 1000, optfNppN, 1 - optfNppN, gamma280]
{0.961982, 0.0210078, 0.0136785, 0.00218792,
  0.000864123, 0.000270533, 9.54871 × 10-6, 6.10978 × 10-8,
  0.958498, 0.000638571, 3.23311 × 10-20, -1.71625 × 10-113}
```

```
Total[optolegiy[[1 ;; 8]]]
```

```
1.
```

```
optolegiynorm := 1 / Total[optolegiy[[2 ;; 8]]] * optolegiy  
optolegiynorm[[2 ;; 8]]
```

```
{0.552567, 0.359786, 0.057549, 0.022729, 0.00711583, 0.00025116, 1.60706 × 10-6}
```

```
chrgConst4 = optolegiynorm[[2 ;; 8]].Table[i, {i, 1, 7}]
```

```
1.5728
```

## With SCH, DCHTS, and DCHSS

```
optolegiy = dsionyieldcrateranalysisparam[  
  optdamp4 * 0.15 * MilliJouleToHartree, photonenergy, 4 / t0ToFemtoSecond,  
  nintdata, True, True, 1 / 1000, optfNppN, 1 - optfNppN, gamma280]
```

```
{0.983099, 0.0121588, 0.00448586, 0.000189672,  
  0.0000592361, 7.11509 × 10-6, 8.19675 × 10-8, 1.76959 × 10-10,  
  0.981055, 0.000385001, 1.90071 × 10-20, -2.07211 × 10-169}
```

```
Total[optolegiy[[1 ;; 8]]]
```

```
1.
```

```
optolegiynorm := 1 / Total[optolegiy[[2 ;; 8]]] * optolegiy  
optolegiynorm[[2 ;; 8]]
```

```
{0.719423, 0.265424, 0.0112227,  
  0.00350494, 0.000420993, 4.84993 × 10-6, 1.04705 × 10-8}
```

```
chrgDCHSS4 = optolegiynorm[[2 ;; 8]].Table[i, {i, 1, 7}]
```

```
1.30009
```

## With SCH and DCHTS

```
optolegiy = dsionyieldcrateranalysisparam[  
  optdamp4 * 0.15 * MilliJouleToHartree, photonenergy, 4 / t0ToFemtoSecond,  
  nintdata, False, True, 1 / 1000, optfNppN, 1 - optfNppN, gamma280]
```

```
{0.983181, 0.0126306, 0.004087, 0.0000868415,  
  0.0000142877, 6.45468 × 10-7, 7.0628 × 10-10, 1.15748 × 10-11,  
  0.981055, 0.000385001, 1.96434 × 10-20, 5.10973 × 10-219}
```

```
Total[optolegiy[[1 ;; 8]]]
```

```
1.
```

```
optolegiynorm := 1 / Total[optolegiy[[2 ;; 8]]] * optolegiy  
optolegiynorm[[2 ;; 8]]
```

```
{0.750955, 0.242994, 0.00516319,  
  0.00084948, 0.0000383766, 4.19921 × 10-8, 6.88184 × 10-10}
```

```
chrgDCHTS4 = optolegiynorm[[2 ;; 8]].Table[i, {i, 1, 7}]
```

```
1.25602
```



## With only SCH

```
optolegiy = dsionyieldcrateranalysisparam[
  optdamp4 * 0.15 * MilliJouleToHartree, photonenergy, 4 / t0ToFemtoSecond,
  nintdata, False, False, 1 / 1000, optfNppN, 1 - optfNppN, gamma280]
{0.983332, 0.0135064, 0.00314552, 6.96506 × 10-6,
 9.27765 × 10-6, 1.1449 × 10-7, 1.26616 × 10-10, 2.32704 × 10-12,
 0.981055, 0.000385001, 2.10981 × 10-20, -1.89641 × 10-216}

Total[optolegiy[[1 ;; 8]]]
1.

optolegiynorm := 1 / Total[optolegiy[[2 ;; 8]]] * optolegiy
optolegiynorm[[2 ;; 8]]
{0.810306, 0.188713, 0.000417863,
 0.000556606, 6.86875 × 10-6, 7.59625 × 10-9, 1.39609 × 10-10}

chrgSCH4 = optolegiynorm[[2 ;; 8]].Table[i, {i, 1, 7}]
1.19125
```

---

## Presentation of results

```
chrgExpt := {{4, chrgExpt4}, {7, chrgExpt7}, {80, chrgExpt80}, {280, chrgExpt280}}
chrgSCH := {{4, chrgSCH4}, {7, chrgSCH7}, {80, chrgSCH80}, {280, chrgSCH280}}
chrgDCHTS :=
  {{4, chrgDCHTS4}, {7, chrgDCHTS7}, {80, chrgDCHTS80}, {280, chrgDCHTS280}}
chrgDCHSS := {{4, chrgDCHSS4}, {7, chrgDCHSS7},
  {80, chrgDCHSS80}, {280, chrgDCHSS280}}
chrgConst := {{4, chrgConst4}, {7, chrgConst7},
  {80, chrgConst80}, {280, chrgConst280}}

contplt = ListPlot[{chrgExpt, chrgDCHSS, chrgDCHTS, chrgSCH, chrgConst},
  Joined → True, PlotRange → All, PlotMarkers → None,
  PlotStyle → {{Thick, Black}, {Dotted, Red}, {Thick, Green},
  {Thick, Blue}, {Thick, Magenta}}, Frame → True, Axes → False,
  FrameLabel → {"Pulse duration [fs]", "Average charge state"},
  LabelStyle → {FontFamily → "Arial", FontSize → 11, FontSlant → Plain},
  InterpolationOrder → 3];

markerplt = ListPlot[{chrgExpt, chrgDCHSS, chrgDCHTS, chrgSCH, chrgConst},
  Joined → False, PlotRange → All, PlotMarkers → Automatic,
  PlotStyle → {{Thick, Black}, {Dotted, Red}, {Thick, Green},
  {Thick, Blue}, {Thick, Magenta}}, Frame → True, Axes → False,
  FrameLabel → {"Pulse duration [fs]", "Average charge state"},
  LabelStyle → {FontFamily → "Arial", FontSize → 11, FontSlant → Plain}];
```

```
Show[contplt, markerplt]
```

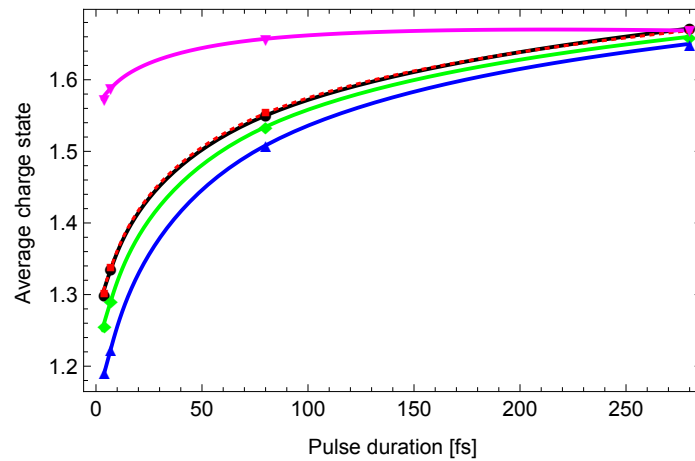

```
contpltlegend = ListPlot[{chrgExpt, chrgDCHSS, chrgDCHTS, chrgSCH, chrgConst},
  Joined -> True, PlotRange -> {{0, 290}, {1.18, 1.69}}, PlotMarkers -> None,
  PlotStyle -> {{Thick, Black}, {Dotted, Red}, {Thick, Green},
    {Thick, Blue}, {Thick, Magenta}}, Frame -> True, Axes -> False,
  FrameLabel -> {"Pulse duration [fs]", "Average charge state"},
  LabelStyle -> {FontFamily -> "Arial", FontSize -> 11, FontSlant -> Plain},
  InterpolationOrder -> 3, PlotLegend ->
    {"Experiment", "All channels", "Only tsDCH, SCH", "Only SCH", "Constant energy"},
  LegendPosition -> {0.21, -0.3}, LegendSize -> {0.56, 0.5},
  LegendTextSpace -> 7, LegendShadow -> None];
```

```
markerpltlegend = ListPlot[{chrgExpt, chrgDCHSS, chrgDCHTS, chrgSCH, chrgConst},
  Joined -> False, PlotRange -> {{0, 290}, {1.18, 1.69}}, PlotMarkers -> Automatic,
  PlotStyle -> {{Thick, Black}, {Dotted, Red}, {Thick, Green},
    {Thick, Blue}, {Thick, Magenta}}, Frame -> True, Axes -> False,
  FrameLabel -> {"Pulse duration [fs]", "Average charge state"},
  LabelStyle -> {FontFamily -> "Arial", FontSize -> 11, FontSlant -> Plain},
  PlotLegend -> {"Experiment", "All channels", "Only tsDCH, SCH",
    "Only SCH", "Constant energy"}, LegendPosition -> {0.21, -0.3},
  LegendSize -> {0.56, 0.5}, LegendTextSpace -> 7, LegendShadow -> None];
```

```
Show[contpltlegend, markerpltlegend]
```

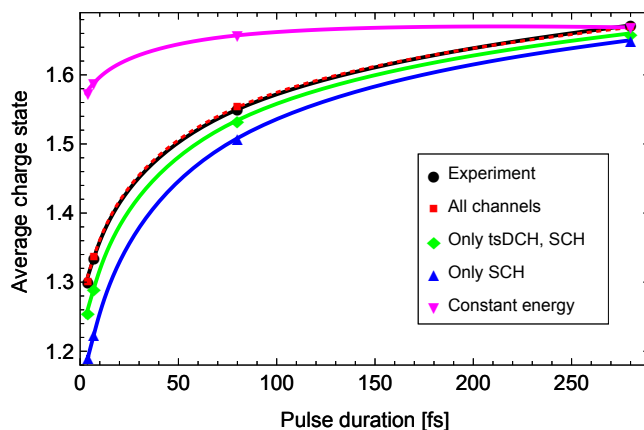

Supplement: Supplementary file 10 [file nitrogen_microscopic.pdf]
