# Supplementary material for: Rate equations for nitrogen molecules in ultrashort and intense x-ray pulses
Source: arXiv:1508.05223 ancillary file (2017-03-16)

```
<< PlotLegends`
```

General::obspkg: PlotLegends` is now obsolete. The legacy version being loaded may conflict with current functionality. See the Compatibility Guide for updating information.

```
Get["NitrogenRateEquations.m", Path -> NotebookDirectory[]]  
Get["NitrogenMoleculeRateEqs.m", Path -> NotebookDirectory[]]
```

```
HartreeToeV := 27.2113845  
eVToHartree := 1 / HartreeToeV  
JouleToHartree := 2.29371269*^17  
MilliJouleToHartree := 1*^-3 * JouleToHartree  
BohrToAngstroem := 0.5291772083  
AngstroemToBohr := 1 / BohrToAngstroem  
MicrometerToBohr := 1*^4 * AngstroemToBohr  
BohrToMicrometer := 1 / MicrometerToBohr  
t0ToSecond := 24.18884326505*^-18  
t0ToFemtoSecond := 24.18884326505*^-3  
crossSectionAUtoBarn := 1*^8 * BohrToAngstroem^2  
crossSectionAUtocm2 := crossSectionAUtoBarn * 1*^-24  
crossSectioncm2toAU := 1 / crossSectionAUtocm2  
  
neginfinity := -1000 / t0ToFemtoSecond  
posinfinity := 10 000 / t0ToFemtoSecond
```

# Impact of fragmentation time on the ion yields from the microscopic molecular rate-equation model

Ji-Cai Liu

Department of Mathematics and Physics, North China Electric Power University, 102206 Beijing, China

Max-Planck-Institut für Kernphysik, Saupfercheckweg 1, 69117 Heidelberg, Germany

Christian Buth

Max-Planck-Institut für Kernphysik, Saupfercheckweg 1, 69117 Heidelberg, Germany

Theoretische Chemie, Physikalisch-Chemisches Institut, Ruprecht-Karls-Universität Heidelberg, Im Neuenheimer Feld 229, 69120 Heidelberg, Germany

26 September 2014

---

## Experimental parameters

Pulse energy fractions from the nitrogen\_dissociation\_first.nb *Mathematica* Notebook:

```

optdamp280 := 0.38
optdamp80 := 0.30
optdamp7 := 0.16
optdamp4 := 0.23

photonenergy := 1100 * eVToHartree
optfNppN := 0.26

newMatthias280 := {204.331, 105.281, 27.561, 13.151, 9.881, 0.587, 0.000}
normOleg280 = 1 / Total[newMatthias280] * newMatthias280
{0.56634, 0.291805, 0.0763903, 0.0364504, 0.027387, 0.00162698, 0.}

chrgExpt280 = normOleg280.Table[i, {i, 1, 7}]
1.67162

newMatthias80 := {218.068, 103.774, 26.075, 9.804, 3.315, 0.000, 0.000}
normOleg80 = 1 / Total[newMatthias80] * newMatthias80
{0.604006, 0.287434, 0.0722227, 0.0271552, 0.00918191, 0., 0.}

chrgExpt80 = normOleg80.Table[i, {i, 1, 7}]
1.55007

newMatthias7 := {221.485, 87.888, 9.342, 0.085, 0.000, 0.000, 0.000}
normOleg7 = 1 / Total[newMatthias7] * newMatthias7
{0.694746, 0.275684, 0.0293036, 0.000266625, 0., 0., 0.}

chrgExpt7 = normOleg7.Table[i, {i, 1, 7}]
1.33509

newMatthias4 := {92.985, 36.341, 1.413, 0, 0, 0, 0}
normOleg4 = 1 / Total[newMatthias4] * newMatthias4
{0.711226, 0.277966, 0.0108078, 0., 0., 0., 0.}

chrgExpt4 = normOleg4.Table[i, {i, 1, 7}]
1.29958

```

---

## Ion yields for 280 fs pulses

### Atomic ion yields

```

ionyi = ionyieldcrateranalysis[optdamp280 * 0.26 * MilliJouleToHartree,
  photonenergy, 280 / t0ToFemtoSecond, nintdata, True];
ionyinorm = 1 / Total[ionyi[[2 ;;]]] * ionyi
charge280atom := ionyinorm[[2 ;;]]
{37.74, 0.037233, 0.746864, 0.0140445,
  0.159545, 0.037227, 0.00495192, 0.000134553}

```

```
BarChart[ionynorm[[2 ;;]], PlotRange → {-0.03, 0.9},
  ChartLabels → {"N+", "N2+", "N3+", "N4+", "N5+", "N6+", "N7+"},
  AxesLabel → {"", "Y( $\omega$ )"},
  AxesStyle → {{Arrowheads[Automatic], AbsoluteThickness[0.6]},
    {Arrowheads[Automatic], AbsoluteThickness[0.6]}},
  LabelStyle → {FontFamily → "Arial"}, PlotLabel →
    {optdamp280, chrgExpt280 - ionynorm[[2 ;; 8]].Table[i, {i, 1, 7}]]]
{0.38, -0.756443}
```

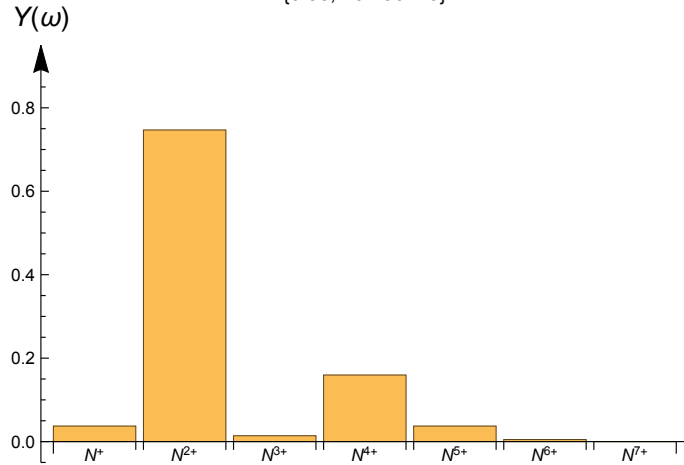

$\gamma_{\text{frag}} = 0$  meV; with SCH, DCHTS, and DCHSS

```
optolegiy = dsionyieldcrateranalysisparam[
  optdamp280 * 0.26 * MilliJouleToHartree, photonenergy, 280 / t0ToFemtoSecond,
  nintdata, True, True, 1 / 1000, optfNppN, 1 - optfNppN, 0 * gammaFrag];
optolegiynorm := 1 / Total[optolegiy[[2 ;; 8]]] * optolegiy
charge280DCHSSnogamma = optolegiynorm[[2 ;; 8]]
{0.0404701, 0.842416, 0.0124704, 0.0834323, 0.0188328, 0.00230109, 0.0000767658}
```

```
BarChart[optolegiynorm[[2 ;; 8]], PlotRange → {-0.08, 0.9},
  ChartLabels → {"N+", "N2+", "N3+", "N4+", "N5+", "N6+", "N7+"},
  AxesLabel → {"", "Y( $\omega$ )"},
  AxesStyle → {{Arrowheads[Automatic], AbsoluteThickness[0.6]},
    {Arrowheads[Automatic], AbsoluteThickness[0.6]}},
  LabelStyle → {FontFamily → "Arial"},
  PlotLabel → {optdamp280, 0 * gammaFrag,
    chrgExpt280 - optolegiynorm[[2 ;; 8]].Table[i, {i, 1, 7}]]]
{0.38, 0., -0.533332}
```

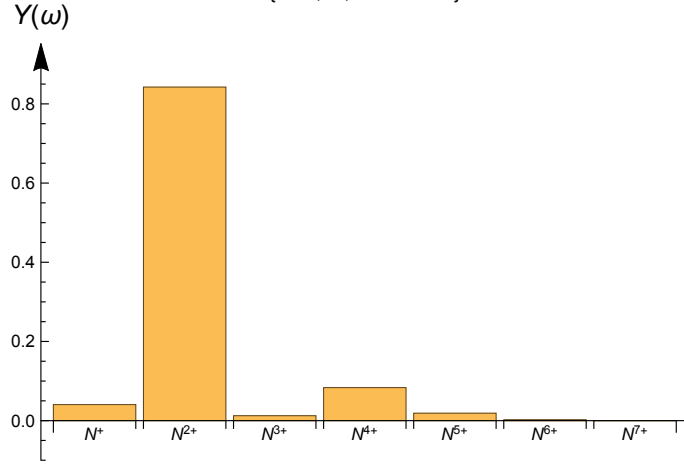

$\gamma_{\text{frag}} \rightarrow \infty$ ; with SCH, DCHTS, and DCHSS

```
optolegiy = dsionyieldcrateranalysisparam[
  optdamp280 * 0.26 * MilliJouleToHartree, photonenergy, 280 / t0ToFemtoSecond,
  nintdata, True, True, 1 / 1000, optfNppN, 1 - optfNppN, 100 * gammaFrag]
{0.96249, 0.0237827, 0.00619767, 0.00470221, 0.00136248, 0.00124916, 0.000199031,
  0.00001688, 0.958498, 0.000638571, 2.00361 × 10-131, -2.30467 × 10-131}
```

```
optolegiy = dsionyieldcrateranalysisparam[
  optdamp280 * 0.26 * MilliJouleToHartree, photonenergy, 280 / t0ToFemtoSecond,
  nintdata, True, True, 1 / 1000, optfNppN, 1 - optfNppN, 1000 * gammaFrag]
{0.962523, 0.0239687, 0.00577161, 0.00493769, 0.00127068, 0.00129888, 0.000210763,
  0.0000183697, 0.958498, 0.00063857, -4.77056 × 10-117, 6.32004 × 10-137}
```

```
optolegiy = dsionyieldcrateranalysisparam[
  optdamp280 * 0.26 * MilliJouleToHartree, photonenergy, 280 / t0ToFemtoSecond,
  nintdata, True, True, 1 / 2000, optfNppN, 1 - optfNppN, 10 000 * gammaFrag]
{0.962527, 0.0239875, 0.00572843, 0.00496172, 0.00126101, 0.00130404,
  0.000212006, 0.00001853, 0.958498, 0.00063857, 0., 2.53955 × 10-263}
```

```
optolegiy = dsionyieldcrateranalysisparam[
  optdamp280 * 0.26 * MilliJouleToHartree, photonenergy, 280 / t0ToFemtoSecond,
  nintdata, True, True, 1 / 3000, optfNppN, 1 - optfNppN, 100 000 * gammaFrag]
{0.962527, 0.0239894, 0.0057241, 0.00496413, 0.00126004, 0.00130455,
  0.000212131, 0.0000185462, 0.958498, 0.00063857, 0., 3.46797 × 10-263}
```

```
optolegiy = dsionyeldcrateranalysisparam[
  optdamp280 * 0.26 * MilliJouleToHartree, photonenergy, 280 / t0ToFemtoSecond,
  nintdata, True, True, 1 / 4000, optfNppN, 1 - optfNppN, 1 000 000 * gammaFrag]
{0.962527, 0.0239896, 0.00572367, 0.00496437, 0.00125995, 0.0013046,
  0.000212144, 0.0000185478, 0.958498, 0.00063857, 0., 8.07068 × 10-263}
```

```
optolegiynorm := 1 / Total[optolegiy[[2 ;; 8]]] * optolegiy
charge280DCHSSinfinitygamma = optolegiynorm[[2 ;; 8]]
{0.640186, 0.152742, 0.132479, 0.0336228, 0.0348146, 0.00566126, 0.000494965}
```

```
BarChart[optolegiynorm[[2 ;; 8]], PlotRange → {-0.03, 0.7},
  ChartLabels → {"N+", "N2+", "N3+", "N4+", "N5+", "N6+", "N7+"},
  AxesLabel → {"", "Y( $\omega$ )"},
  AxesStyle → {{Arrowheads[Automatic], AbsoluteThickness[0.6]},
    {Arrowheads[Automatic], AbsoluteThickness[0.6]}},
  LabelStyle → {FontFamily → "Arial"},
  PlotLabel → {optdamp280, 1 000 000 000 * gammaFrag,
    chrgExpt280 - optolegiynorm[[2 ;; 8]].Table[i, {i, 1, 7}]}]
{0.38, 24 188.8, -0.0174828}
```

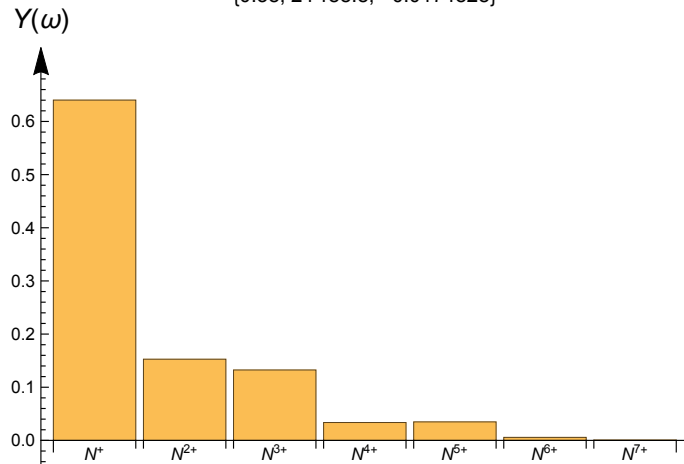

## Ion yields for 80 fs pulses

### Atomic ion yields

```
ionyi = ionyeldcrateranalysis[optdamp80 * 0.23 * MilliJouleToHartree,
  photonenergy, 80 / t0ToFemtoSecond, nintdata, True];
ionyinorm = 1 / Total[ionyi[[2 ;; 8]]] * ionyi
charge80atom := ionyinorm[[2 ;; 8]]
{50.7339, 0.0399273, 0.803402, 0.0116074,
  0.124334, 0.0190901, 0.00161725, 0.0000226506}
```

```
BarChart[ionyinorm[[2 ;;]], PlotRange → {-0.03, 0.9},
  ChartLabels → {"N+", "N2+", "N3+", "N4+", "N5+", "N6+", "N7+"},
  AxesLabel → {"", "Y( $\omega$ )"},
  AxesStyle → {{Arrowheads[Automatic], AbsoluteThickness[0.6]},
    {Arrowheads[Automatic], AbsoluteThickness[0.6]}},
  LabelStyle → {FontFamily → "Arial"},
  PlotLabel → {optdamp80, 0 * gammaFrag,
    chrgExpt80 - ionyinorm[[2 ;; 8]].Table[i, {i, 1, 7}]]]
{0.3, 0., -0.734127}
```

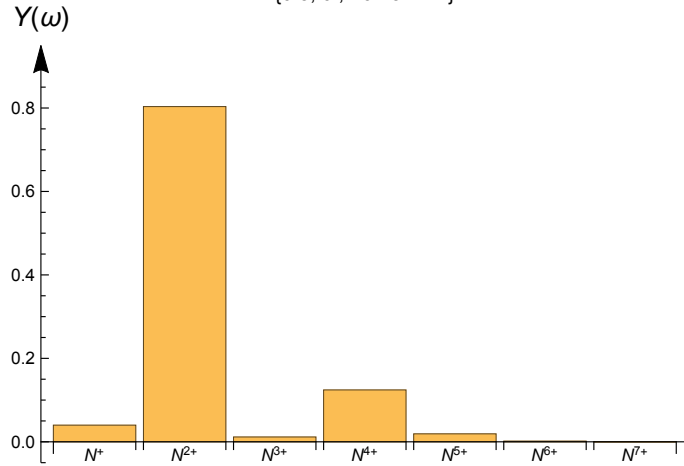

$\Upsilon_{\text{frag}} = 0$  meV; with SCH, DCHTS, and DCHSS

```
optolegiy = dsionyieldcrateranalysisparam[
  optdamp80 * 0.26 * MilliJouleToHartree, photonenergy, 80 / t0ToFemtoSecond,
  nintdata, True, True, 1 / 1000, optfNppN, 1 - optfNppN, 0 * gammaFrag];
optolegiynorm := 1 / Total[optolegiy[[2 ;; 8]]] * optolegiy
charge80DCHSSnogamma = optolegiynorm[[2 ;; 8]]
{0.0424182, 0.871567, 0.0185289, 0.0557419, 0.0107535, 0.00096335, 0.0000267844}
```

```
BarChart[optolegiynorm[[2 ;; 8]], PlotRange → {-0.08, 0.9},
  ChartLabels → {"N+", "N2+", "N3+", "N4+", "N5+", "N6+", "N7+"},
  AxesLabel → {"", "Y( $\omega$ )"},
  AxesStyle → {{Arrowheads[Automatic], AbsoluteThickness[0.6]},
    {Arrowheads[Automatic], AbsoluteThickness[0.6]}},
  LabelStyle → {FontFamily → "Arial"},
  PlotLabel → {optdamp80, 0 * gammaFrag,
    chrgExpt80 - optolegiynorm[[2 ;; 8]].Table[i, {i, 1, 7}]]
    {0.3, 0., -0.57377}
```

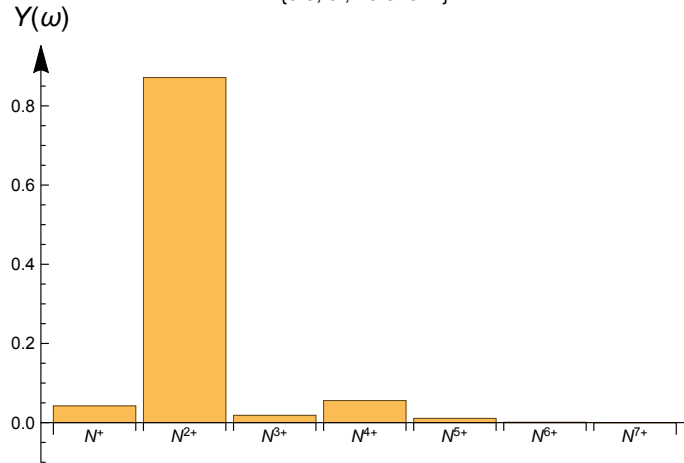

$\gamma_{\text{frag}} \rightarrow \infty$ ; with SCH, DCHTS, and DCHSS

```
optolegiy = dsionyieldcrateranalysisparam[
  optdamp80 * 0.26 * MilliJouleToHartree, photonenergy, 80 / t0ToFemtoSecond,
  nintdata, True, True, 1 / 1000, optfNppN, 1 - optfNppN, 100 * gammaFrag]
{0.968032, 0.0208679, 0.00653322, 0.00287612,
  0.00105077, 0.000577948, 0.0000591983, 2.8316 × 10-6,
  0.96453, 0.00059168, -1.09534 × 10-126, -2.92806 × 10-137}
```

```
optolegiy = dsionyieldcrateranalysisparam[
  optdamp80 * 0.26 * MilliJouleToHartree, photonenergy, 80 / t0ToFemtoSecond,
  nintdata, True, True, 1 / 1000, optfNppN, 1 - optfNppN, 1000 * gammaFrag]
{0.968112, 0.0213144, 0.00551314, 0.0033781,
  0.000938966, 0.000667703, 0.0000715104, 3.67738 × 10-6,
  0.96453, 0.000591678, 2.45229 × 10-114, -2.35067 × 10-135}
```

```
optolegiy = dsionyieldcrateranalysisparam[
  optdamp80 * 0.26 * MilliJouleToHartree, photonenergy, 80 / t0ToFemtoSecond,
  nintdata, True, True, 1 / 2000, optfNppN, 1 - optfNppN, 10 000 * gammaFrag]
{0.968121, 0.0213634, 0.00540196, 0.00343376,
  0.000924583, 0.000678375, 0.0000730722, 3.78989 × 10-6,
  0.96453, 0.000591682, -1.23712 × 10-304, 3.90606 × 10-267}
```

```
optolegiy = dsionyieldcrateranalysisparam[
  optdamp80 * 0.26 * MilliJouleToHartree, photonenergy, 80 / t0ToFemtoSecond,
  nintdata, True, True, 1 / 3000, optfNppN, 1 - optfNppN, 100 000 * gammaFrag]
{0.968122, 0.0213682, 0.00539077, 0.00343937, 0.000923112, 0.000679458,
  0.0000732319, 3.80147 × 10-6, 0.96453, 0.00059168, 0., 6.65665 × 10-268}
```

```

optolegiy = dsionyieldcrateranalysisparam[
  optdamp80 * 0.26 * MilliJouleToHartree, photonenergy, 80 / t0ToFemtoSecond,
  nintdata, True, True, 1 / 4000, optfNppN, 1 - optfNppN, 1 000 000 * gammaFrag]
{0.968122, 0.0213687, 0.00538965, 0.00343992, 0.000922963, 0.000679565,
  0.0000732477,  $3.8026 \times 10^{-6}$ , 0.96453, 0.000591679, 0.,  $1.74038 \times 10^{-267}$ }

optolegiynorm := 1 / Total[optolegiy[[2 ;; 8]]] * optolegiy
charge80DCHSSinfinitygamma = optolegiynorm[[2 ;; 8]]
{0.670331, 0.169072, 0.10791, 0.0289531, 0.0213178, 0.00229776, 0.000119287}

BarChart[optolegiynorm[[2 ;; 8]], PlotRange → {-0.03, 0.7},
  ChartLabels → {"N+", "N2+", "N3+", "N4+", "N5+", "N6+", "N7+"},
  AxesLabel → {"", "Y( $\omega$ )"},
  AxesStyle → {{Arrowheads[Automatic], AbsoluteThickness[0.6]},
    {Arrowheads[Automatic], AbsoluteThickness[0.6]}},
  LabelStyle → {FontFamily → "Arial"},
  PlotLabel → {optdamp80, 1 000 000 000 * gammaFrag,
    chrgExpt80 - optolegiynorm[[2 ;; 8]].Table[i, {i, 1, 7}]]]
{0.3, 24 188.8, -0.0191533}

```

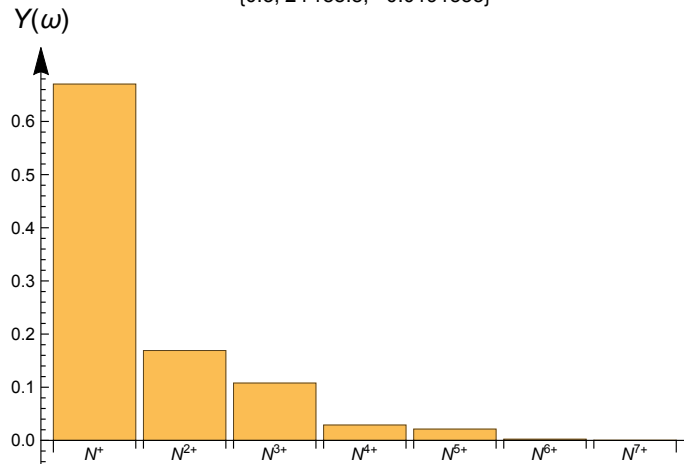

## Ion yields for 7 fs pulses

### Atomic ion yields

```

ionyi = ionyieldcrateranalysis[optdamp7 * 0.23 * MilliJouleToHartree,
  photonenergy, 7 / t0ToFemtoSecond, nintdata, True];
ionyinorm = 1 / Total[ionyi[[2 ;; 8]]] * ionyi
charge7atom := ionyinorm[[2 ;; 8]]
{88.4991, 0.043263, 0.882445, 0.00889122,
  0.061916, 0.0034086, 0.0000763158,  $2.7048 \times 10^{-7}$ }

```



```
BarChart[ionynorm[[2 ;;]], PlotRange → {-0.03, 0.9},
  ChartLabels → {"N+", "N2+", "N3+", "N4+", "N5+", "N6+", "N7+"},
  AxesLabel → {"", "Y( $\omega$ )"},
  AxesStyle → {{Arrowheads[Automatic], AbsoluteThickness[0.6]},
    {Arrowheads[Automatic], AbsoluteThickness[0.6]}},
  LabelStyle → {FontFamily → "Arial"},
  PlotLabel → {optdamp4, chrgExpt7 - ionynorm[[2 ;; 8]].Table[i, {i, 1, 7}]]}
{0.23, -0.764902}
```

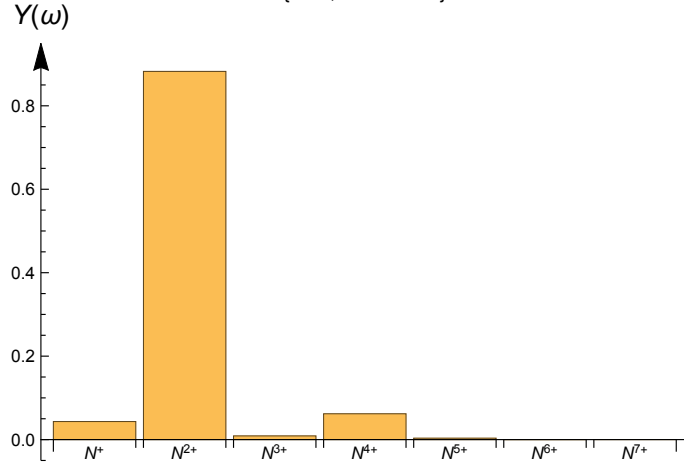

$\gamma_{\text{frag}} = 0$  meV; with SCH, DCHTS, and DCHSS

```
optolegiy = dsionyieldcrateranalysisparam[
  optdamp7 * 0.26 * MilliJouleToHartree, photonenergy, 7 / t0ToFemtoSecond,
  nintdata, True, True, 1 / 1000, optfNppN, 1 - optfNppN, 0 * gammaFrag];
optolegiynorm := 1 / Total[optolegiy[[2 ;; 8]]] * optolegiy
charge7DCHSSnogamma = optolegiynorm[[2 ;; 8]]
{0.0468123, 0.920655, 0.0217763,
  0.00932231, 0.00140511, 0.0000293046, 1.28864 × 10-7}
```

```
BarChart[optolegiynorm[[2 ;; 8]], PlotRange → {-0.08, 0.9},
  ChartLabels → {"N+", "N2+", "N3+", "N4+", "N5+", "N6+", "N7+"},
  AxesLabel → {"", "Y( $\omega$ )"},
  AxesStyle → {{Arrowheads[Automatic], AbsoluteThickness[0.6]},
    {Arrowheads[Automatic], AbsoluteThickness[0.6]}},
  LabelStyle → {FontFamily → "Arial"},
  PlotLabel → {optdamp7, 0 * gammaFrag,
    chrgExpt7 - optolegiynorm[[2 ;; 8]].Table[i, {i, 1, 7}]]
    {0.16, 0., -0.662851}
```

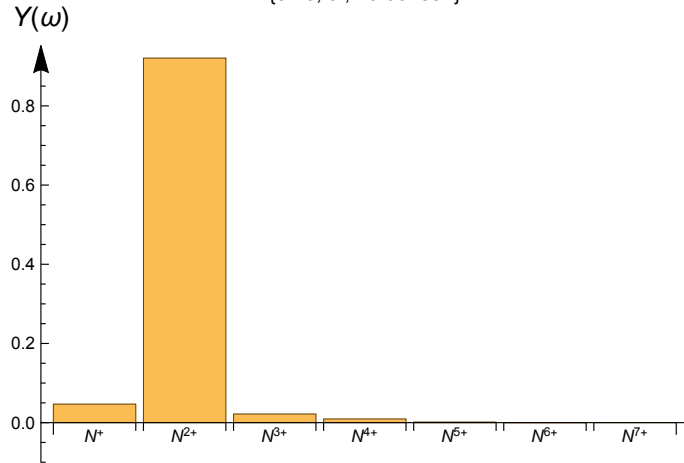

$\gamma_{\text{frag}} \rightarrow \infty$ ; with SCH, DCHTS, and DCHSS

```
optolegiy = dsionyieldcrateranalysisparam[
  optdamp7 * 0.26 * MilliJouleToHartree, photonenergy, 7 / t0ToFemtoSecond,
  nintdata, True, True, 1 / 1000, optfNppN, 1 - optfNppN, 100 * gammaFrag]
{0.980221, 0.013822, 0.00541136, 0.000385747,
  0.000136114, 0.000023545, 5.03508 × 10-7, 2.30921 × 10-9,
  0.9779, 0.000433713, -3.50456 × 10-181, 2.07607 × 10-218}
```

```
optolegiy = dsionyieldcrateranalysisparam[
  optdamp7 * 0.26 * MilliJouleToHartree, photonenergy, 7 / t0ToFemtoSecond,
  nintdata, True, True, 1 / 1000, optfNppN, 1 - optfNppN, 1000 * gammaFrag]
{0.980266, 0.0140744, 0.00483159, 0.000624175,
  0.000164367, 0.0000382921, 8.87089 × 10-7, 4.44928 × 10-9,
  0.9779, 0.000433713, -6.10601 × 10-142, 2.84598 × 10-222}
```

```
optolegiy = dsionyieldcrateranalysisparam[
  optdamp7 * 0.26 * MilliJouleToHartree, photonenergy, 7 / t0ToFemtoSecond,
  nintdata, True, True, 1 / 2000, optfNppN, 1 - optfNppN, 10 000 * gammaFrag]
{0.980284, 0.0141709, 0.00461144, 0.000713993, 0.000173214, 0.0000455194,
  1.10669 × 10-6, 5.80499 × 10-9, 0.9779, 0.000433712, 0., 2.76211 × 10-269}
```

```
optolegiy = dsionyieldcrateranalysisparam[
  optdamp7 * 0.26 * MilliJouleToHartree, photonenergy, 7 / t0ToFemtoSecond,
  nintdata, True, True, 1 / 3000, optfNppN, 1 - optfNppN, 100 000 * gammaFrag]
{0.980286, 0.0141826, 0.00458521, 0.000724676, 0.000174166, 0.0000464653,
  1.13746 × 10-6, 6.00449 × 10-9, 0.9779, 0.000433713, 0., 1.56731 × 10-268}
```

```

optolegiy = dsionyieldcrateranalysisparam[
  optdamp7 * 0.26 * MilliJouleToHartree, photonenergy, 7 / t0ToFemtoSecond,
  nintdata, True, True, 1 / 4000, optfNppN, 1 - optfNppN, 1 000 000 * gammaFrag]
{0.980286, 0.0141837, 0.00458255, 0.00072576, 0.000174262, 0.0000465623,
  1.14064 × 10-6, 6.02521 × 10-9, 0.9779, 0.000433713, 0., 1.12085 × 10-267}

optolegiy = dsionyieldcrateranalysisparam[
  optdamp7 * 0.26 * MilliJouleToHartree, photonenergy, 7 / t0ToFemtoSecond,
  nintdata, True, True, 1 / 4000, optfNppN, 1 - optfNppN, 10 000 000 * gammaFrag]
{0.980286, 0.0141839, 0.00458228, 0.000725869, 0.000174271, 0.0000465721,
  1.14096 × 10-6, 6.02727 × 10-9, 0.9779, 0.000433714, 0., 1.13529 × 10-267}

optolegiynorm := 1 / Total[optolegiy[[2 ;; 8]]] * optolegiy
charge7DCHSSinfinitygamma = optolegiynorm[[2 ;; 8]]
{0.719481, 0.232438, 0.03682, 0.00883997, 0.00236239, 0.0000578755, 3.05735 × 10-7}

BarChart[optolegiynorm[[2 ;; 8]], PlotRange → {-0.03, 0.7},
  ChartLabels → {"N+", "N2+", "N3+", "N4+", "N5+", "N6+", "N7+"},
  AxesLabel → {"", "Y(ω)"},
  AxesStyle → {{Arrowheads[Automatic], AbsoluteThickness[0.6]},
    {Arrowheads[Automatic], AbsoluteThickness[0.6]}},
  LabelStyle → {FontFamily → "Arial"},
  PlotLabel → {optdamp7, 1 000 000 000 * gammaFrag,
    chrgExpt7 - optolegiynorm[[2 ;; 8]].Table[i, {i, 1, 7}]]}
{0.16, 24 188.8, -0.00724767}

```

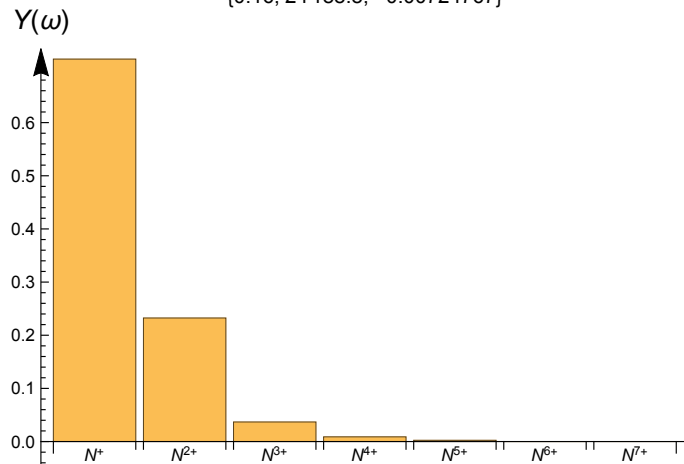

## Ion yields for 4 fs pulses

### Atomic ion yields

```

ionyi = ionyieldcrateranalysis[optdamp4 * 0.15 * MilliJouleToHartree,
  photonenergy, 4 / t0ToFemtoSecond, nintdata, True];
ionyinorm = 1 / Total[ionyi[[2 ;; ]]] * ionyi
charge4atom := ionyinorm[[2 ;; 8]]
{93.8979, 0.0435197, 0.889775, 0.00878724,
  0.0554718, 0.0024088, 0.0000375009, 9.13922 × 10-8}

```

```
BarChart[ionynorm[[2 ;;]], PlotRange → {-0.03, 0.9},
  ChartLabels → {"N+", "N2+", "N3+", "N4+", "N5+", "N6+", "N7+"},
  AxesLabel → {"", "Y( $\omega$ )"},
  AxesStyle → {{Arrowheads[Automatic], AbsoluteThickness[0.6]},
    {Arrowheads[Automatic], AbsoluteThickness[0.6]}},
  LabelStyle → {FontFamily → "Arial"},
  PlotLabel → {optdamp4, chrgExpt4 - ionynorm[[2 ;; 8]].Table[i, {i, 1, 7}]]}
{0.23, -0.784006}
```

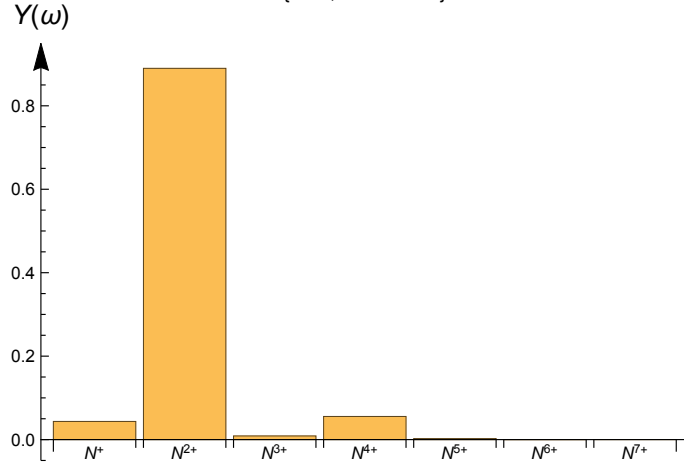

$\gamma_{\text{frag}} = 0$  meV; with SCH, DCHTS, and DCHSS

```
optolegiy = dsionyieldcrateranalysisparam[
  optdamp4 * 0.15 * MilliJouleToHartree, photonenergy, 4 / t0ToFemtoSecond,
  nintdata, True, True, 1 / 1000, optfNppN, 1 - optfNppN, 0 * gammaFrag];
optolegiynorm := 1 / Total[optolegiy[[2 ;; 8]]] * optolegiy
charge4DCHSSnogamma = optolegiynorm[[2 ;; 8]]
{0.047538, 0.929503, 0.0169888,
  0.00532554, 0.000637169, 7.332 × 10-6, 1.58046 × 10-8}
```

```
BarChart[optolegiynorm[[2 ;; 8]], PlotRange → {-0.08, 1},
  ChartLabels → {"N+", "N2+", "N3+", "N4+", "N5+", "N6+", "N7+"},
  AxesLabel → {"", "Y( $\omega$ )"},
  AxesStyle → {{Arrowheads[Automatic], AbsoluteThickness[0.6]},
    {Arrowheads[Automatic], AbsoluteThickness[0.6]}},
  LabelStyle → {FontFamily → "Arial"},
  PlotLabel → {optdamp4, 0 * gammaFrag,
    chrgExpt4 - optolegiynorm[[2 ;; 8]].Table[i, {i, 1, 7}]]]
{0.23, 0., -0.682461}
```

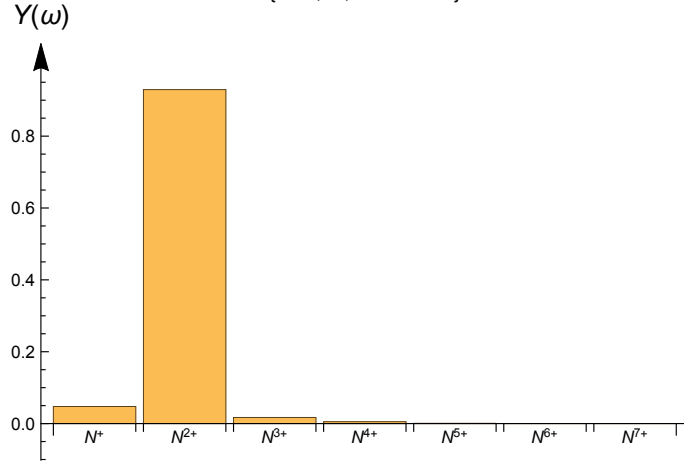

$\gamma_{\text{frag}} \rightarrow \infty$ ; with SCH, DCHTS, and DCHSS

```
optolegiy = dsionyieldcrateranalysisparam[
  optdamp4 * 0.15 * MilliJouleToHartree, photonenergy, 4 / t0ToFemtoSecond,
  nintdata, True, True, 1 / 1000, optfNppN, 1 - optfNppN, 100 * gammaFrag]
{0.983105, 0.012188, 0.00441825, 0.000217583,
  0.0000633525, 8.21971 × 10-6, 9.6861 × 10-8, 2.15279 × 10-10,
  0.981055, 0.000385001, -4.47619 × 10-200, -4.98264 × 10-237}
```

```
optolegiy = dsionyieldcrateranalysisparam[
  optdamp4 * 0.15 * MilliJouleToHartree, photonenergy, 4 / t0ToFemtoSecond,
  nintdata, True, True, 1 / 1000, optfNppN, 1 - optfNppN, 1000 * gammaFrag]
{0.983125, 0.0123014, 0.00415634, 0.000325182,
  0.0000787079, 0.0000131681, 1.69117 × 10-7, 4.10275 × 10-10,
  0.981055, 0.000385001, -5.10891 × 10-162, 7.91518 × 10-239}
```

```
optolegiy = dsionyieldcrateranalysisparam[
  optdamp4 * 0.15 * MilliJouleToHartree, photonenergy, 4 / t0ToFemtoSecond,
  nintdata, True, True, 1 / 2000, optfNppN, 1 - optfNppN, 10 000 * gammaFrag]
{0.983138, 0.012373, 0.00399208, 0.000392008, 0.0000875183, 0.0000171618,
  2.37148 × 10-7, 6.1259 × 10-10, 0.981055, 0.000384999, 0., 1.23827 × 10-270}
```

```
optolegiy = dsionyieldcrateranalysisparam[
  optdamp4 * 0.15 * MilliJouleToHartree, photonenergy, 4 / t0ToFemtoSecond,
  nintdata, True, True, 1 / 3000, optfNppN, 1 - optfNppN, 100 000 * gammaFrag]
{0.98314, 0.0123831, 0.00396924, 0.000401259, 0.0000886676, 0.0000177975,
  2.49067 × 10-7, 6.50415 × 10-10, 0.981055, 0.000385002, 0., 8.16181 × 10-269}
```

```

optolegiy = dsionyieldcrateranalysisparam[
  optdamp4 * 0.15 * MilliJouleToHartree, photonenergy, 4 / t0ToFemtoSecond,
  nintdata, True, True, 1 / 4000, optfNppN, 1 - optfNppN, 1 000 000 * gammaFrag]
{0.98314, 0.0123841, 0.00396688, 0.000402211, 0.0000887849, 0.0000178642,
   $2.5034 \times 10^{-7}$ ,  $6.54506 \times 10^{-10}$ , 0.981055, 0.000385001, 0.,  $7.05702 \times 10^{-268}$ }

optolegiy = dsionyieldcrateranalysisparam[
  optdamp4 * 0.15 * MilliJouleToHartree, photonenergy, 4 / t0ToFemtoSecond,
  nintdata, True, True, 1 / 4000, optfNppN, 1 - optfNppN, 10 000 000 * gammaFrag]
{0.98314, 0.0123842, 0.00396664, 0.000402307, 0.0000887966, 0.0000178709,
   $2.50466 \times 10^{-7}$ ,  $6.54905 \times 10^{-10}$ , 0.981055, 0.000385001, 0.,  $6.87919 \times 10^{-268}$ }

optolegiynorm := 1 / Total[optolegiy[[2 ;; 8]]] * optolegiy
charge4DCHSSinfinitygamma = optolegiynorm[[2 ;; 8]]
{0.734528, 0.235269, 0.0238615,
  0.00526669, 0.00105995, 0.0000148556,  $3.88436 \times 10^{-8}$ }

BarChart[optolegiynorm[[2 ;; 8]], PlotRange → {-0.03, 0.8},
  ChartLabels → {"N+", "N2+", "N3+", "N4+", "N5+", "N6+", "N7+"},
  AxesLabel → {"", "Y( $\omega$ )"},
  AxesStyle → {{Arrowheads[Automatic], AbsoluteThickness[0.6]},
    {Arrowheads[Automatic], AbsoluteThickness[0.6]}},
  LabelStyle → {FontFamily → "Arial"},
  PlotLabel → {optdamp4, 1 000 000 000 * gammaFrag,
    chrgExpt4 - optolegiynorm[[2 ;; 8]].Table[i, {i, 1, 7}]}]
{0.23, 24 188.8, -0.00352457}

```

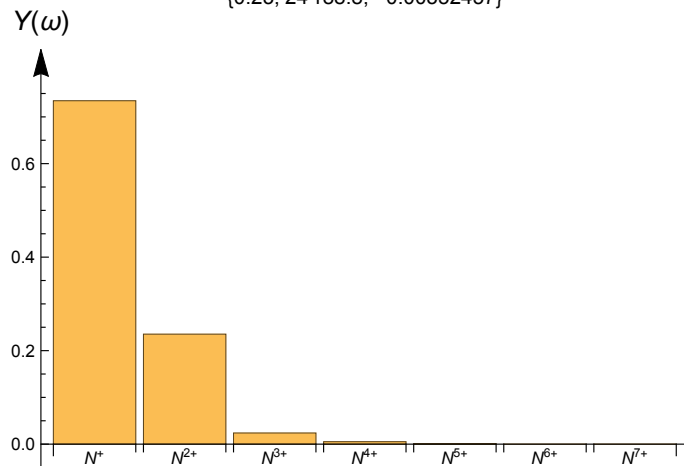

## Presentation of results

### 280 fs pulses

```
charge280 := {{normOleg280[[1]], charge280DCHSSinfinitygamma[[1]],
  charge280DCHSSnogamma[[1]], charge280atom[[1]]},
{normOleg280[[2]], charge280DCHSSinfinitygamma[[2]],
  charge280DCHSSnogamma[[2]], charge280atom[[2]]},
{normOleg280[[3]], charge280DCHSSinfinitygamma[[3]],
  charge280DCHSSnogamma[[3]], charge280atom[[3]]},
{normOleg280[[4]], charge280DCHSSinfinitygamma[[4]],
  charge280DCHSSnogamma[[4]], charge280atom[[4]]},
{normOleg280[[5]], charge280DCHSSinfinitygamma[[5]],
  charge280DCHSSnogamma[[5]], charge280atom[[5]]},
{normOleg280[[6]], charge280DCHSSinfinitygamma[[6]],
  charge280DCHSSnogamma[[6]], charge280atom[[6]]},
{normOleg280[[7]], charge280DCHSSinfinitygamma[[7]],
  charge280DCHSSnogamma[[7]], charge280atom[[7]]}}
```

```
BarChart[charge280, PlotRange → {-0.08, 1.0},
  ChartLabels → {Placed[{"N+", "N2+", "N3+", "N4+", "N5+", "N6+", "N7+"}, Below],
    Placed[{}, Above]},
  ChartLegends → Placed[{"Expt.", "γfrag→∞", "γfrag=0", "Atom"}, Top],
  ChartStyle → {Black, Red, Green, Blue}, AxesLabel → {"", "Ỹ"},
  AxesStyle → {{Arrowheads[Automatic], AbsoluteThickness[0.6]},
    {Arrowheads[Automatic], AbsoluteThickness[0.6]}},
  LabelStyle → {FontFamily → "Arial", FontSize → 18, FontSlant → Plain}]
```

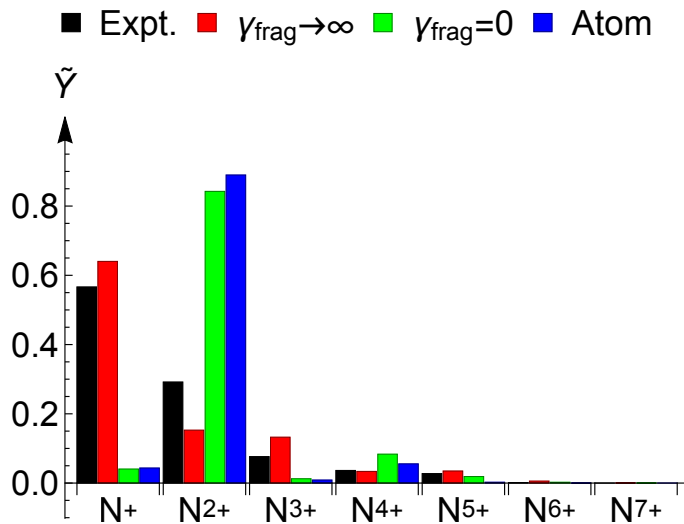

## 80 fs pulses

```
charge80 :=
  {{normOleg80[[1]], charge80DCHSSinfinitygamma[[1]], charge80DCHSSnogamma[[1]],
    charge80atom[[1]]}, {normOleg80[[2]], charge80DCHSSinfinitygamma[[2]],
    charge80DCHSSnogamma[[2]], charge80atom[[2]]},
  {normOleg80[[3]], charge80DCHSSinfinitygamma[[3]], charge80DCHSSnogamma[[3]],
    charge80atom[[3]]}, {normOleg80[[4]], charge80DCHSSinfinitygamma[[4]],
    charge80DCHSSnogamma[[4]], charge80atom[[4]]},
  {normOleg80[[5]], charge80DCHSSinfinitygamma[[5]], charge80DCHSSnogamma[[5]],
    charge80atom[[5]]}, {normOleg80[[6]], charge80DCHSSinfinitygamma[[6]],
    charge80DCHSSnogamma[[6]], charge80atom[[6]]},
  {normOleg80[[7]], charge80DCHSSinfinitygamma[[7]],
    charge80DCHSSnogamma[[7]], charge80atom[[7]]}}

BarChart[charge80, PlotRange → {-0.08, 1.0},
  ChartLabels → {Placed[{"N+", "N2+", "N3+", "N4+", "N5+", "N6+", "N7+"}, Below],
    Placed[{}, Above]},
  ChartLegends → Placed[{"Expt.", " $\gamma_{\text{frag}} \rightarrow \infty$ ", " $\gamma_{\text{frag}} = 0$ ", "Atom"}, Top],
  ChartStyle → {Black, Red, Green, Blue}, AxesLabel → {"", " $\tilde{Y}$ "},
  AxesStyle → {{Arrowheads[Automatic], AbsoluteThickness[0.6]},
    {Arrowheads[Automatic], AbsoluteThickness[0.6]}},
  LabelStyle → {FontFamily → "Arial", FontSize → 18, FontSlant → Plain}]
```

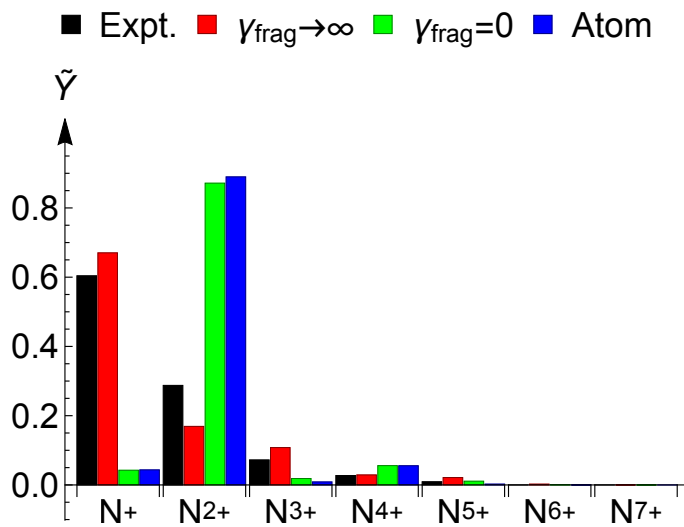

## 7 fs pulses

```
charge7 := {{normOleg7[[1]], charge7DCHSSinfinitygamma[[1]],
  charge7DCHSSnogamma[[1]], charge7atom[[1]]}, {normOleg7[[2]],
  charge7DCHSSinfinitygamma[[2]], charge7DCHSSnogamma[[2]], charge7atom[[2]]},
  {normOleg7[[3]], charge7DCHSSinfinitygamma[[3]], charge7DCHSSnogamma[[3]],
  charge7atom[[3]]}, {normOleg7[[4]], charge7DCHSSinfinitygamma[[4]],
  charge7DCHSSnogamma[[4]], charge7atom[[4]]}, {normOleg7[[5]],
  charge7DCHSSinfinitygamma[[5]], charge7DCHSSnogamma[[5]], charge7atom[[5]]},
  {normOleg7[[6]], charge7DCHSSinfinitygamma[[6]], charge7DCHSSnogamma[[6]],
  charge7atom[[6]]}, {normOleg7[[7]], charge7DCHSSinfinitygamma[[7]],
  charge7DCHSSnogamma[[7]], charge7atom[[7]]}}
```



```
BarChart[charge7, PlotRange → {-0.08, 1.0},
  ChartLabels → {Placed[{"N+", "N2+", "N3+", "N4+", "N5+", "N6+", "N7+"}, Below],
    Placed[{}, Above]},
  ChartLegends → Placed[{"Expt.", " $\gamma_{\text{frag}} \rightarrow \infty$ ", " $\gamma_{\text{frag}} = 0$ ", "Atom"}, Top],
  ChartStyle → {Black, Red, Green, Blue}, AxesLabel → {"", " $\tilde{Y}$ "},
  AxesStyle → {{Arrowheads[Automatic], AbsoluteThickness[0.6]},
    {Arrowheads[Automatic], AbsoluteThickness[0.6]}},
  LabelStyle → {FontFamily → "Arial", FontSize → 18, FontSlant → Plain}]
```

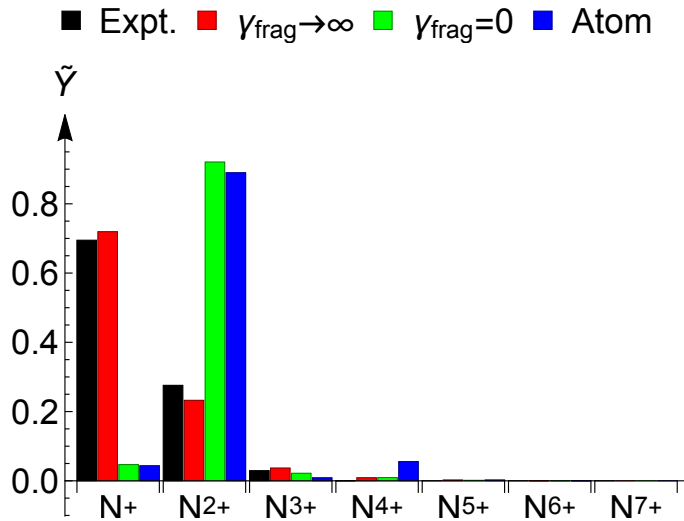

## 4 fs pulses

```
charge4 := {{normOleg4[[1]], charge4DCHSSinfinitygamma[[1]],
  charge4DCHSSnogamma[[1]], charge4atom[[1]]}, {normOleg4[[2]],
  charge4DCHSSinfinitygamma[[2]], charge4DCHSSnogamma[[2]], charge4atom[[2]]},
  {normOleg4[[3]], charge4DCHSSinfinitygamma[[3]], charge4DCHSSnogamma[[3]],
  charge4atom[[3]]}, {normOleg4[[4]], charge4DCHSSinfinitygamma[[4]],
  charge4DCHSSnogamma[[4]], charge4atom[[4]]}, {normOleg4[[5]],
  charge4DCHSSinfinitygamma[[5]], charge4DCHSSnogamma[[5]], charge4atom[[5]]},
  {normOleg4[[6]], charge4DCHSSinfinitygamma[[6]], charge4DCHSSnogamma[[6]],
  charge4atom[[6]]}, {normOleg4[[7]], charge4DCHSSinfinitygamma[[7]],
  charge4DCHSSnogamma[[7]], charge4atom[[7]]}}
```

```
BarChart[charge4, PlotRange → {-0.08, 1.0},
  ChartLabels → {Placed[{"N+", "N2+", "N3+", "N4+", "N5+", "N6+", "N7+"}, Below],
    Placed[{}, Above]},
  ChartLegends → Placed[{"Expt.", " $\gamma_{\text{frag}} \rightarrow \infty$ ", " $\gamma_{\text{frag}} = 0$ ", "Atom"}, Top],
  ChartStyle → {Black, Red, Green, Blue}, AxesLabel → {"", " $\tilde{Y}$ "},
  AxesStyle → {{Arrowheads[Automatic], AbsoluteThickness[0.6]},
    {Arrowheads[Automatic], AbsoluteThickness[0.6]}},
  LabelStyle → {FontFamily → "Arial", FontSize → 18, FontSlant → Plain}]
```

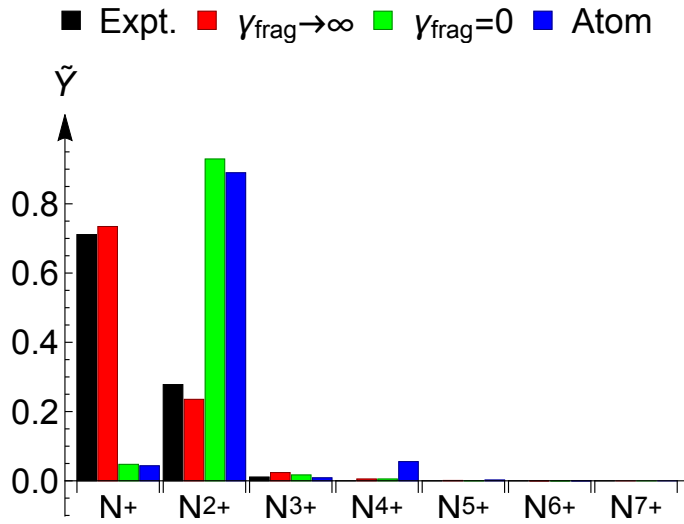

Supplement: Supplementary file 11 [file nitrogen_time.pdf]
